# Supplementary material for: Anisotropy factor spectra for weakly allowed electronic transitions in chiral ketones
Source: arXiv:2405.12893 ancillary file (2024-05-21)
Supplement: Supplementary file 1 [file suppmat.pdf]

# Supplementary Material:

## Anisotropy factor spectra for weakly allowed electronic transitions in chiral ketones

Leon A. Kerber and Daniel M. Reich  
*Dahlem Center for Complex Quantum Systems and Fachbereich Physik,  
Freie Universität Berlin, D-14195 Berlin, Germany*

Oliver Kreuz and Robert Berger  
*Fachbereich Chemie, Philipps-Universität Marburg, D-35032 Marburg, Germany*

Tom Ring and Hendrike Braun  
*Institut für Physik, Universität Kassel, D-34132 Kassel, Germany*

### GENERAL REMARKS

In this supplementary material we report the equilibrium structures,  $\mathbf{l}$ -matrix, which represents the mass weighted normal coordinates (See Ch. 2.4 of Ref [1]), harmonic vibrational wavenumbers of the electronic states, electric and magnetic transition dipole moments as well as first derivative of the electric transition dipole moments with respect to the ground state mass weighted normal coordinates. Equilibrium structures and mass weighted normal coordinates of various initial states are given in their Eckart frame. The equilibrium structures of the various final states are arranged such that they can be viewed as distorted structures of the initial state with the Eckart conditions fulfilled. For each normal mode and electronic state the corresponding column of the  $\mathbf{l}$  matrix is reported for this particular choice of orientation. Harmonic vibrational wavenumbers are reported together with the corresponding elements of the  $\mathbf{l}$ -matrix. The first derivatives of the transition electric dipole moment are reported together with the harmonic vibrational wavenumbers and  $\mathbf{l}$ -matrix elements of the initial states. Additionally, we report the parameters used for the rigorous prescreening conditions and its output, the maximum quantum number of the final state as well as the number of simultaneously excited modes.

## STRUCTURES

TABLE I. Energy-minimized  $S_0$  equilibrium structure of (1R,4S)-(-)-fenchone in units of Å in the Eckart frame.

|   |                    |                    |                    |
|---|--------------------|--------------------|--------------------|
| O | -0.102 968 259 729 | -2.012 812 629 8   | 0.741 982 280 754  |
| C | -0.026 273 593 808 | -0.915 601 137 144 | 0.248 790 236 397  |
| C | -1.217 103 339 822 | -0.000 925 488 347 | -0.104 606 734 699 |
| C | 1.250 293 152 954  | -0.168 069 117 905 | -0.126 218 624 375 |
| C | -0.464 816 685 914 | 1.258 285 487 023  | -0.621 023 128 576 |
| C | 0.747 944 870 123  | 0.637 803 065 749  | -1.343 492 911 312 |
| C | 1.356 043 148 258  | 0.964 822 361 646  | 0.943 760 257 535  |
| C | 0.246 872 540 693  | 1.975 518 551 674  | 0.541 645 343 866  |
| C | -2.117 001 691 614 | 0.207 912 527 831  | 1.115 197 805 79   |
| C | -2.049 851 440 568 | -0.654 452 719 15  | -1.219 054 131 154 |
| C | 2.476 013 009 843  | -1.038 464 370 311 | -0.269 960 541 53  |
| H | 0.493 370 898 448  | 0.008 975 729 063  | -2.196 272 352 553 |
| H | 1.235 216 922 329  | 0.575 614 802 616  | 1.955 618 761 997  |
| H | -1.097 213 208 938 | 1.910 364 637 069  | -1.223 408 088 548 |
| H | -1.567 196 522 887 | 0.565 287 278 657  | 1.985 065 525 328  |
| H | 1.473 702 157 401  | 1.385 386 962 32   | -1.668 804 084 893 |
| H | -0.418 315 408 285 | 2.229 375 485 839  | 1.364 213 305 716  |
| H | -1.480 848 280 342 | -0.802 166 703 761 | -2.136 579 406 892 |
| H | 2.350 188 316 319  | 1.411 099 718 129  | 0.885 164 147 345  |
| H | 0.684 840 473 678  | 2.908 836 735 588  | 0.185 037 965 544  |
| H | -2.585 237 199 397 | -0.737 280 199 977 | 1.390 892 571 237  |
| H | -2.413 964 549 918 | -1.628 127 068 686 | -0.889 703 516 236 |
| H | 2.338 320 264 333  | -1.783 799 029 884 | -1.055 387 849 62  |
| H | 2.677 037 711 105  | -1.575 652 799 477 | 0.658 277 984 072  |
| H | -2.905 562 425 5   | 0.929 564 281 177  | 0.888 599 875 885  |
| H | -2.911 014 055 118 | -0.024 533 005 829 | -1.453 325 296 141 |
| H | 3.352 581 526 311  | -0.435 727 152 358 | -0.517 233 957 174 |

TABLE II. Transition structure of  $S_1$  state of (1R,4S)-(-)-fenchone in units of Å in the Eckart frame.

|   |                    |                    |                    |
|---|--------------------|--------------------|--------------------|
| O | -0.105 441 149 653 | -2.084 139 162 617 | 0.742 924 046 603  |
| C | -0.027 238 944 678 | -0.887 399 431 054 | 0.294 726 909 581  |
| C | -1.240 262 703 499 | -0.012 004 905 303 | -0.103 746 317 59  |
| C | 1.271 266 947 167  | -0.145 336 340 646 | -0.110 759 537 929 |
| C | -0.461 490 116 814 | 1.242 022 910 932  | -0.597 953 014 029 |
| C | 0.741 110 840 83   | 0.633 194 085 729  | -1.331 565 559 554 |
| C | 1.430 883 980 876  | 1.008 859 310 238  | 0.919 644 108 958  |
| C | 0.253 754 542 844  | 1.962 257 632 125  | 0.567 825 014 092  |
| C | -2.179 839 914 705 | 0.238 864 137 902  | 1.081 699 288 689  |
| C | -2.056 416 667 35  | -0.662 522 525 373 | -1.237 672 224 405 |
| C | 2.480 118 806 469  | -1.034 010 282 075 | -0.294 233 223 959 |
| H | 0.489 399 676 873  | -0.010 442 969 786 | -2.171 659 630 372 |
| H | 1.395 559 151 466  | 0.635 585 004 365  | 1.941 735 726 509  |
| H | -1.104 521 259 758 | 1.897 452 071 839  | -1.187 259 348 611 |
| H | -1.643 743 563 399 | 0.572 985 503 561  | 1.967 583 743 485  |
| H | 1.455 548 702 929  | 1.391 344 866 21   | -1.666 578 007 04  |
| H | -0.401 387 819 228 | 2.159 386 026 129  | 1.413 089 156 25   |
| H | -1.459 833 277 719 | -0.826 158 130 428 | -2.133 224 932 521 |
| H | 2.399 209 734 196  | 1.500 643 030 273  | 0.776 241 267 536  |
| H | 0.627 452 348 234  | 2.927 679 196 353  | 0.223 234 246 574  |
| H | -2.709 584 909 651 | -0.678 233 010 316 | 1.341 213 969 991  |
| H | -2.450 133 698 382 | -1.626 085 117 409 | -0.914 286 431 263 |
| H | 2.291 226 192 828  | -1.808 022 396 31  | -1.039 146 462 618 |
| H | 2.753 163 849 048  | -1.525 515 900 45  | 0.640 757 102 766  |
| H | -2.924 600 285 86  | 0.996 324 961 879  | 0.818 874 031 763  |
| H | -2.901 925 184 16  | -0.020 018 149 332 | -1.501 597 509 883 |
| H | 3.332 945 939 665  | -0.436 229 777 94  | -0.624 982 490 344 |

TABLE III. Energy-minimized  $S_0$  equilibrium structure of (1S,4S)-(-)-camphor in units of Å in the Eckart frame.

|   |                    |                    |                    |
|---|--------------------|--------------------|--------------------|
| O | -2.540 824 725 417 | -0.229 302 461 518 | 0.246 557 271 693  |
| C | -0.244 484 830 089 | -0.500 089 680 937 | -0.562 671 039 566 |
| C | 0.946 934 903 978  | -0.307 725 111 378 | 0.433 092 876 692  |
| C | -1.386 715 328 19  | 0.114 815 457 04   | 0.246 568 889 912  |
| C | 0.694 006 623 547  | 1.220 282 688 305  | 0.607 484 564 847  |
| C | 0.052 892 438 737  | 0.590 323 657 999  | -1.636 797 414 295 |
| C | -0.777 391 319 389 | 1.268 281 303 345  | 1.049 139 187 066  |
| C | 0.733 920 508 31   | 1.739 343 748 045  | -0.843 074 377 288 |
| C | 0.789 018 534 985  | -1.116 331 494 745 | 1.724 942 183 963  |
| C | -0.533 679 777 067 | -1.877 502 288 845 | -1.108 935 960 224 |
| C | 2.316 075 545 651  | -0.640 448 281 712 | -0.160 189 824 144 |
| H | -0.198 421 996 774 | -1.026 921 345 157 | 2.176 613 628 319  |
| H | -0.859 747 849 536 | 0.905 505 296 944  | -2.143 685 398 314 |
| H | -0.919 045 925 903 | 1.083 100 666 433  | 2.114 557 077 498  |
| H | 0.712 244 748 701  | 0.175 221 252 563  | -2.399 493 587 498 |
| H | 1.383 112 777 23   | 1.723 169 078 86   | 1.285 851 090 52   |
| H | -0.719 263 087 304 | -2.592 108 981 259 | -0.305 563 542 112 |
| H | 2.513 283 149 589  | -0.141 870 340 129 | -1.106 778 711 731 |
| H | -1.280 440 617 773 | 2.207 509 476 375  | 0.813 673 401 88   |
| H | 0.959 147 422 517  | -2.176 906 114 204 | 1.531 296 479 572  |
| H | 0.300 023 233 827  | -2.243 255 409 504 | -1.711 440 360 367 |
| H | 1.754 935 258 488  | 1.909 245 478 759  | -1.182 615 190 463 |
| H | 0.201 756 518 981  | 2.685 773 820 264  | -0.942 061 149 279 |
| H | -1.426 427 534 638 | -1.858 040 297 552 | -1.735 712 773 302 |
| H | 2.408 679 310 275  | -1.715 330 381 985 | -0.327 347 430 53  |
| H | 1.525 698 786 89   | -0.796 450 398 308 | 2.465 590 355 427  |
| H | 3.104 924 518 722  | -0.349 195 940 674 | 0.537 837 421 419  |

TABLE IV. Transition structure of  $S_1$  state of (1S,4S)-(-)-camphor in units of Å in the Eckart frame.

|   |                    |                    |                    |
|---|--------------------|--------------------|--------------------|
| O | -2.588 888 236 017 | -0.237 933 989 319 | 0.269 509 317 793  |
| C | -0.236 048 647 105 | -0.491 326 882 535 | -0.585 511 924 786 |
| C | 0.946 255 100 122  | -0.306 843 381 079 | 0.431 907 249 295  |
| C | -1.370 209 563 246 | 0.170 098 693 71   | 0.238 008 974 967  |
| C | 0.685 080 374 585  | 1.212 043 803 223  | 0.602 848 360 166  |
| C | 0.104 606 310 32   | 0.563 042 014 947  | -1.672 841 665 612 |
| C | -0.772 499 580 982 | 1.262 878 789 665  | 1.093 401 842 666  |
| C | 0.706 964 347 594  | 1.737 016 765 288  | -0.851 567 169 399 |
| C | 0.785 398 340 369  | -1.127 004 457 014 | 1.712 031 094 11   |
| C | -0.533 800 224 128 | -1.881 917 738 878 | -1.095 888 528 866 |
| C | 2.323 468 338 51   | -0.629 662 263 074 | -0.160 551 668 078 |
| H | -0.216 668 171 484 | -1.061 407 761 052 | 2.132 070 819 104  |
| H | -0.784 579 269 652 | 0.843 759 541 456  | -2.234 317 234 079 |
| H | -0.872 827 988 071 | 1.045 887 060 177  | 2.168 446 891 394  |
| H | 0.826 117 055 044  | 0.153 493 646 432  | -2.387 425 799 825 |
| H | 1.374 191 756 692  | 1.726 476 301 917  | 1.274 098 735 027  |
| H | -0.783 212 983 736 | -2.562 426 460 834 | -0.281 320 771 732 |
| H | 2.549 397 852 553  | -0.075 843 764 932 | -1.068 579 076 372 |
| H | -1.240 548 548 041 | 2.240 294 505 709  | 0.922 825 018 601  |
| H | 0.991 165 935 451  | -2.181 062 854 623 | 1.515 692 787 701  |
| H | 0.333 838 004 564  | -2.280 098 317 383 | -1.626 226 755 695 |
| H | 1.720 666 463 827  | 1.971 929 258 279  | -1.175 684 791 123 |
| H | 0.120 815 132 565  | 2.651 398 084 291  | -0.945 515 345 649 |
| H | -1.374 150 719 084 | -1.870 764 792 811 | -1.791 151 148 623 |
| H | 2.402 290 076 069  | -1.694 254 361 561 | -0.388 965 918 373 |
| H | 1.497 453 190 208  | -0.792 076 152 405 | 2.469 892 328 817  |
| H | 3.099 844 831 793  | -0.395 898 483 999 | 0.572 074 494 039  |

TABLE V. Energy-minimized  $S_0$  equilibrium structure of equatorial (R)-(+)-3-methylcyclopentanone in units of Å in the Eckart frame.

|   |                    |                    |                    |
|---|--------------------|--------------------|--------------------|
| O | -2.371 549 589 198 | -0.600 721 186 089 | 0.051 594 456 358  |
| C | 0.022 480 221 389  | -1.049 607 087 603 | 0.037 321 624 385  |
| C | 1.161 507 198 154  | -0.104 362 121 176 | -0.364 778 890 511 |
| C | 0.690 408 682 852  | 1.261 886 883 102  | 0.175 041 951 524  |
| C | -0.819 845 994 024 | 1.272 762 223 815  | -0.073 713 941 345 |
| C | -1.239 156 624 852 | -0.193 702 281 499 | 0.012 046 640 006  |
| C | 2.539 576 195 337  | -0.524 351 999 938 | 0.123 061 325 969  |
| H | 0.158 492 720 851  | -1.393 028 563 779 | 1.070 519 096 212  |
| H | -0.090 721 536 95  | -1.937 298 272 051 | -0.584 816 454 774 |
| H | 1.179 857 195 988  | -0.042 412 251 563 | -1.459 354 357 248 |
| H | 1.213 831 765 546  | 2.095 578 101 76   | -0.294 007 516 842 |
| H | 0.894 045 792 207  | 1.312 261 033 131  | 1.249 511 976 193  |
| H | -1.054 446 453 818 | 1.615 362 431 06   | -1.087 299 107 431 |
| H | -1.404 638 448 552 | 1.883 467 740 668  | 0.613 819 524 831  |
| H | 2.830 051 494 353  | -1.494 000 627 184 | -0.286 701 087 361 |
| H | 2.554 524 214 809  | -0.604 018 550 452 | 1.213 556 925 141  |
| H | 3.300 118 208 604  | 0.203 307 257 242  | -0.169 556 387 449 |

TABLE VI. Transition structure of  $S_1$  state of equatorial (R)-(+)-3-methylcyclopentanone in units of Å in the Eckart frame.

|   |                    |                    |                    |
|---|--------------------|--------------------|--------------------|
| O | -2.393 228 364 749 | -0.615 876 075 814 | 0.082 887 622 094  |
| C | 0.022 681 454 682  | -1.070 807 957 257 | 0.007 008 212 517  |
| C | 1.162 923 075 493  | -0.098 185 674 024 | -0.368 960 491 775 |
| C | 0.686 537 671 238  | 1.263 968 978 946  | 0.153 147 193 846  |
| C | -0.833 948 921 87  | 1.289 159 122 59   | -0.076 525 544 732 |
| C | -1.178 607 662 825 | -0.171 197 539 078 | -0.000 627 391 763 |
| C | 2.525 497 251 231  | -0.530 287 399 891 | 0.157 538 199 97   |
| H | 0.186 303 003 246  | -1.522 527 280 138 | 1.001 092 247 152  |
| H | -0.068 926 453 809 | -1.906 837 877 058 | -0.697 514 146 787 |
| H | 1.204 245 388 086  | -0.050 318 125 964 | -1.462 029 288 922 |
| H | 1.188 507 818 646  | 2.097 229 379 006  | -0.343 669 130 227 |
| H | 0.896 085 576 46   | 1.339 858 696 063  | 1.223 577 535 694  |
| H | -1.097 361 515 989 | 1.716 127 985 976  | -1.058 983 596 709 |
| H | -1.371 076 996 17  | 1.885 879 880 685  | 0.670 384 593 784  |
| H | 2.806 532 753 213  | -1.513 129 320 44  | -0.226 363 886 203 |
| H | 2.520 830 587 626  | -0.583 527 426 184 | 1.249 200 529 505  |
| H | 3.301 245 554 144  | 0.178 405 798 879  | -0.141 087 752 586 |

TABLE VII. Energy-minimized  $S_0$  equilibrium structure of axial (R)-(+)-3-methylcyclopentanone in units of Å in the Eckart frame.

|   |                    |                    |                    |
|---|--------------------|--------------------|--------------------|
| O | 2.250 479 193 373  | -0.462 494 262 494 | -0.278 121 494 81  |
| C | 0.079 016 314 292  | -0.946 764 122 858 | 0.712 453 521 442  |
| C | -1.254 007 941 007 | -0.225 309 997 557 | 0.464 998 752 878  |
| C | -0.833 832 061 435 | 1.262 718 440 949  | 0.378 710 572 517  |
| C | 0.521 070 735 337  | 1.250 668 767 457  | -0.338 094 174 024 |
| C | 1.130 475 205 41   | -0.110 747 803 161 | -0.010 226 606 217 |
| C | -1.928 622 221 854 | -0.707 087 168 116 | -0.819 696 818 078 |
| H | 0.111 219 181 264  | -1.985 416 305 264 | 0.383 230 376 841  |
| H | 0.341 121 098 245  | -0.934 052 310 136 | 1.776 257 703 477  |
| H | -1.942 660 810 361 | -0.376 570 007 069 | 1.298 235 877 574  |
| H | -0.715 686 521 915 | 1.667 613 643 517  | 1.386 810 797 353  |
| H | -1.582 429 070 024 | 1.871 083 993 278  | -0.129 775 158 031 |
| H | 1.201 158 768 971  | 2.051 370 411 063  | -0.047 559 614 988 |
| H | 0.412 536 366 32   | 1.307 523 166 502  | -1.424 927 631 279 |
| H | -2.187 491 250 283 | -1.765 631 093 883 | -0.751 676 824 668 |
| H | -1.274 631 947 709 | -0.585 650 806 969 | -1.687 348 762 018 |
| H | -2.845 560 282 216 | -0.147 007 179 432 | -1.013 861 919 148 |

TABLE VIII. Transition structure of  $S_1$  state of axial (R)-(+)-3-methylcyclopentanone in units of Å in the Eckart frame.

|   |                    |                    |                    |
|---|--------------------|--------------------|--------------------|
| O | 2.292 482 321 219  | -0.458 340 586 629 | -0.254 433 892 466 |
| C | 0.083 804 822 643  | -0.974 144 951 988 | 0.698 998 570 771  |
| C | -1.246 860 825 084 | -0.221 062 963 01  | 0.463 803 356 727  |
| C | -0.824 457 858 757 | 1.254 683 975 312  | 0.370 837 523 585  |
| C | 0.529 467 572 652  | 1.258 343 692 797  | -0.365 762 930 728 |
| C | 1.075 280 635 066  | -0.091 796 806 436 | -0.003 653 047 317 |
| C | -1.951 219 858 126 | -0.704 149 522 132 | -0.802 535 395 043 |
| H | 0.069 577 799 557  | -1.993 185 722 952 | 0.293 726 754 494  |
| H | 0.317 971 811 574  | -1.072 211 363 885 | 1.772 759 557 686  |
| H | -1.909 884 024 625 | -0.376 572 757 113 | 1.319 667 286 429  |
| H | -0.689 512 101 79  | 1.668 659 301 917  | 1.371 924 869 004  |
| H | -1.567 546 065 908 | 1.866 126 664 751  | -0.145 757 807 224 |
| H | 1.184 963 767 537  | 2.077 142 384 193  | -0.044 756 699 961 |
| H | 0.413 768 422 332  | 1.370 900 336 25   | -1.456 609 090 447 |
| H | -2.216 690 543 097 | -1.760 293 806 523 | -0.725 911 647 743 |
| H | -1.309 749 543 481 | -0.585 218 096 223 | -1.678 974 531 949 |
| H | -2.869 039 260 755 | -0.138 892 483 925 | -0.977 406 268 67  |

# VIBRATIONAL STRUCTURE PARAMETERS

TABLE IX. Franck–Condon Herzberg–Teller (FCHT) prescreening settings [2, 3], resulting maximum number of simultaneously excited modes  $M_{\max}$  in the final state and summed intensity of all FCHT overlaps calculated as a share of the total intensity for the absorption spectra.

| Molecule                                  | Mode excitation error | Mode coupling error | $M_{\max}$ | $I_{\text{sum}}/D_{fi}$ |
|-------------------------------------------|-----------------------|---------------------|------------|-------------------------|
| Axial (R)-(+)-3-methylcyclopentanone      | 0.001                 | 0.1                 | 5          | 0.9817                  |
| Equatorial (R)-(+)-3-methylcyclopentanone | 0.001                 | 0.1                 | 6          | 0.9841                  |
| Camphor                                   | 0.001                 | 0.1                 | 5          | 0.8861                  |
| Fenchone                                  | 0.001                 | 0.1                 | 5          | 0.8744                  |

TABLE X. Electric and magnetic transition dipole moments calculated at the  $S_0$  equilibrium structure in the Eckart frame.

|                 | $\mu_x/(e a_0)$ | $\mu_y/(e a_0)$ | $\mu_z/(e a_0)$ | $m_x/(\text{ie}\hbar/m_e)$ | $m_y/(\text{ie}\hbar/m_e)$ | $m_z/(\text{ie}\hbar/m_e)$  |
|-----------------|-----------------|-----------------|-----------------|----------------------------|----------------------------|-----------------------------|
| Fenchone        | 0.002 167       | 0.006 400       | −0.011 532      | −0.000 337                 | −0.003 668                 | 0.001 725                   |
| Camphor         | −0.022 675      | 0.016 408       | −0.037 435      | 0.003 989                  | 0.001 224                  | $9.587\,798 \times 10^{-6}$ |
| axial 3MCP      | 0.035 116       | −0.015 372      | −0.000 201      | −0.003 957                 | 0.001 371                  | 0.001 012                   |
| equatorial 3MCP | −0.041 965      | −0.008 611      | −0.004 113      | −0.004 005                 | −0.001 452                 | 0.000 131                   |

**(1R,4S)-(-)-fenchone**

*Initial state*

Wavenumber/cm<sup>-1</sup>: 86.7777

| $\frac{\partial \mu_{x,y,z}}{\partial Q_r} / (e u^{-0.5})$        | 0.005 148 902 836  | 0.005 311 074 902  | -0.001 282 357 114                    |
|-------------------------------------------------------------------|--------------------|--------------------|---------------------------------------|
| <i>l</i> -matrix coefficients/(u <sup>1/2</sup> Å <sup>-1</sup> ) |                    |                    |                                       |
| O                                                                 | 0.000 260 746 416  | -0.000 148 817 213 | 6.120 628 200 000 × 10 <sup>-5</sup>  |
| C                                                                 | 0.000 332 832 520  | -0.000 103 819 884 | -0.000 267 479 919                    |
| C                                                                 | -0.004 000 454 799 | -0.002 744 406 114 | -0.000 494 718 411                    |
| C                                                                 | 0.000 252 812 977  | 0.001 396 697 694  | -0.000 334 720 790                    |
| C                                                                 | 0.004 541 848 374  | -0.000 926 109 450 | 0.000 486 505 530                     |
| C                                                                 | 0.011 148 269 561  | 0.020 880 511 639  | 0.016 760 528 498                     |
| C                                                                 | 0.027 092 753 304  | 0.024 711 111 346  | -0.037 228 819 972                    |
| C                                                                 | 0.118 179 988 950  | 0.005 563 636 528  | -0.137 608 972 385                    |
| C                                                                 | -0.139 930 889 140 | -0.119 710 735 833 | -0.109 843 098 013                    |
| C                                                                 | -0.039 179 141 358 | -0.042 089 298 568 | 0.061 860 579 291                     |
| C                                                                 | -0.000 526 627 236 | -0.003 302 614 975 | -6.068 479 900 000 × 10 <sup>-5</sup> |
| H                                                                 | -0.021 459 470 252 | -0.049 744 825 770 | -0.065 848 101 886                    |
| H                                                                 | -0.013 997 322 923 | -0.047 644 457 523 | 0.123 688 772 216                     |
| H                                                                 | -0.006 591 508 559 | 0.005 266 027 197  | -0.005 471 728 511                    |
| H                                                                 | 0.297 347 303 069  | 0.190 433 330 711  | 0.456 772 600 909                     |
| H                                                                 | -0.021 546 216 000 | -0.021 322 516 711 | 0.011 591 019 645                     |
| H                                                                 | -0.345 560 608 084 | 0.122 010 352 435  | 0.425 924 919 880                     |
| H                                                                 | 0.102 272 907 575  | -0.026 703 369 669 | -0.158 494 240 457                    |
| H                                                                 | -0.082 682 564 389 | -0.036 656 068 871 | 0.003 752 063 915                     |
| H                                                                 | -0.067 632 988 146 | -0.153 340 069 628 | 0.053 099 626 912                     |
| H                                                                 | 0.140 034 719 767  | 0.300 027 617 614  | -0.090 595 839 104                    |
| H                                                                 | 0.059 336 373 800  | 0.165 408 917 663  | -0.053 364 252 572                    |
| H                                                                 | 0.001 255 509 275  | 0.006 497 563 481  | 0.007 426 582 695                     |
| H                                                                 | -0.000 730 913 578 | 0.003 716 756 032  | -0.006 719 285 933                    |
| H                                                                 | 0.053 726 051 409  | -0.066 325 037 961 | 0.012 597 053 605                     |
| H                                                                 | -0.020 592 420 841 | 0.010 705 078 046  | -0.000 670 519 458                    |
| H                                                                 | 0.002 031 781 216  | -0.000 184 523 987 | -0.000 301 292 549                    |

Wavenumber/cm<sup>-1</sup>: 182.8622

| $\frac{\partial \mu_{x,y,z}}{\partial Q_r} / (e u^{-0.5})$   |                                     |                    |                    |
|--------------------------------------------------------------|-------------------------------------|--------------------|--------------------|
|                                                              | -0.012 410 080 131                  | 0.000 481 193 573  | -0.002 994 441 457 |
| $l$ -matrix coefficients/(u <sup>1/2</sup> Å <sup>-1</sup> ) |                                     |                    |                    |
| O                                                            | -0.000 209 862 967                  | -0.000 731 807 119 | 0.000 445 625 900  |
| C                                                            | 0.000 262 348 501                   | 0.000 782 374 766  | -0.001 186 500 416 |
| C                                                            | 0.002 763 751 122                   | 0.001 567 206 704  | -0.002 918 564 118 |
| C                                                            | -0.000 327 956 627                  | -0.000 879 740 083 | -0.000 424 561 696 |
| C                                                            | -0.004 549 784 666                  | 0.002 473 733 526  | -0.004 498 079 197 |
| C                                                            | -0.041 646 898 959                  | -0.071 337 085 904 | -0.056 492 052 871 |
| C                                                            | 0.010 807 886 953                   | 0.008 344 368 371  | -0.010 575 822 754 |
| C                                                            | 0.036 448 654 465                   | 0.005 118 800 948  | -0.041 669 695 163 |
| C                                                            | -0.046 199 036 461                  | -0.018 591 398 706 | -0.043 882 018 912 |
| C                                                            | 0.164 754 543 118                   | 0.082 585 803 040  | -0.198 961 420 432 |
| C                                                            | -0.002 477 223 663                  | -0.003 470 089 024 | -0.002 601 533 397 |
| H                                                            | 0.075 163 440 065                   | 0.174 356 632 505  | 0.234 074 626 158  |
| H                                                            | -0.004 085 087 988                  | -0.014 176 869 658 | 0.037 410 168 560  |
| H                                                            | 0.012 731 608 508                   | -0.013 404 793 099 | 0.011 556 138 341  |
| H                                                            | 0.102 689 439 142                   | 0.066 629 958 770  | 0.157 450 108 537  |
| H                                                            | 0.075 999 930 545                   | 0.077 766 089 962  | -0.036 799 005 206 |
| H                                                            | -0.102 931 793 434                  | 0.036 831 574 874  | 0.127 124 164 945  |
| H                                                            | -0.369 979 170 290                  | 0.093 986 493 825  | 0.578 202 860 424  |
| H                                                            | -0.031 827 565 667                  | -0.014 177 247 825 | 0.001 859 308 300  |
| H                                                            | -0.025 274 042 345                  | -0.055 700 819 831 | 0.020 119 142 588  |
| H                                                            | 0.016 636 635 105                   | 0.040 396 842 224  | -0.013 069 113 408 |
| H                                                            | -0.153 963 937 475                  | -0.438 834 605 935 | 0.142 690 173 915  |
| H                                                            | 0.001 685 291 737                   | 0.009 953 718 375  | 0.009 387 155 461  |
| H                                                            | $-7.413 222 900 000 \times 10^{-5}$ | -0.000 999 504 430 | 0.001 999 477 005  |
| H                                                            | 0.039 791 776 814                   | -0.040 660 526 055 | 0.010 985 087 436  |
| H                                                            | -0.055 183 225 401                  | 0.054 144 930 288  | -0.029 047 444 101 |
| H                                                            | 0.005 784 278 133                   | 0.004 041 427 359  | -0.001 923 104 283 |



Wavenumber/cm<sup>-1</sup>: 191.2878

| $\frac{\partial \mu_{x,y,z}}{\partial Q_r} / (e u^{-0.5})$        | 0.003 952 392 986  | 0.005 849 729 772  | -0.001 491 809 466 |
|-------------------------------------------------------------------|--------------------|--------------------|--------------------|
| <i>l</i> -matrix coefficients/(u <sup>1/2</sup> Å <sup>-1</sup> ) |                    |                    |                    |
| O                                                                 | -0.000 879 249 338 | -0.000 691 854 309 | 0.000 608 650 461  |
| C                                                                 | 0.000 645 813 387  | 0.000 361 052 591  | -0.000 555 337 834 |
| C                                                                 | 0.002 089 712 626  | 0.002 990 549 155  | -0.000 845 205 681 |
| C                                                                 | -0.000 350 507 421 | 0.001 405 923 634  | 0.000 181 489 058  |
| C                                                                 | 0.007 177 231 563  | -0.005 017 044 877 | 0.005 184 613 526  |
| C                                                                 | 0.025 885 707 319  | 0.040 513 891 850  | 0.020 362 986 220  |
| C                                                                 | 0.037 375 974 192  | 0.032 873 242 997  | -0.047 225 846 816 |
| C                                                                 | 0.129 988 392 981  | 0.022 575 641 945  | -0.148 359 034 660 |
| C                                                                 | 0.106 991 814 566  | 0.175 398 837 243  | 0.048 769 076 931  |
| C                                                                 | -0.003 309 193 975 | 0.020 833 119 400  | -0.006 780 815 416 |
| C                                                                 | -0.012 267 185 469 | -0.018 248 693 136 | 0.019 637 006 663  |
| H                                                                 | -0.029 672 871 850 | -0.072 893 315 144 | -0.097 978 220 169 |
| H                                                                 | -0.018 129 076 766 | -0.060 390 024 112 | 0.155 724 370 713  |
| H                                                                 | -0.018 394 672 976 | 0.017 131 767 309  | -0.017 084 782 174 |
| H                                                                 | -0.203 850 281 850 | -0.123 756 826 972 | -0.316 355 492 329 |
| H                                                                 | -0.065 111 677 149 | -0.066 086 020 823 | 0.030 999 830 335  |
| H                                                                 | -0.354 244 422 391 | 0.126 425 515 576  | 0.435 878 042 891  |
| H                                                                 | 0.000 831 338 146  | 0.000 330 820 344  | -0.001 548 055 335 |
| H                                                                 | -0.115 036 180 484 | -0.051 368 790 882 | 0.004 908 112 363  |
| H                                                                 | -0.095 118 490 940 | -0.214 136 954 292 | 0.074 242 110 080  |
| H                                                                 | -0.219 320 768 463 | -0.451 914 244 774 | 0.134 422 468 706  |
| H                                                                 | -0.018 425 666 551 | -0.055 924 022 714 | 0.017 281 498 723  |
| H                                                                 | -0.001 215 096 467 | -0.005 118 037 445 | -0.002 605 199 625 |
| H                                                                 | -0.011 367 024 808 | 0.028 544 880 910  | -0.051 192 115 976 |
| H                                                                 | 0.052 765 148 505  | -0.031 885 638 925 | 0.017 084 625 147  |
| H                                                                 | 0.029 787 458 426  | -0.019 676 019 081 | 0.006 788 826 398  |
| H                                                                 | 0.054 336 425 711  | 0.038 712 436 556  | -0.014 546 484 916 |

Wavenumber/cm<sup>-1</sup>: 200.556

| $\frac{\partial \mu_{x,y,z}}{\partial Q_r} / (e u^{-0.5})$        | 0.019 708 547 885  | 0.000 399 540 046  | 0.000 467 668 892  |
|-------------------------------------------------------------------|--------------------|--------------------|--------------------|
| <i>l</i> -matrix coefficients/(u <sup>1/2</sup> Å <sup>-1</sup> ) |                    |                    |                    |
| O                                                                 | 0.000 249 509 951  | 0.002 279 875 988  | -0.000 700 385 516 |
| C                                                                 | -0.000 446 614 736 | -0.002 207 137 415 | -0.000 228 726 960 |
| C                                                                 | 0.001 577 106 305  | -0.003 293 804 658 | 0.000 551 888 293  |
| C                                                                 | -0.001 698 452 397 | -0.003 114 680 333 | -0.001 156 033 987 |
| C                                                                 | -0.011 532 442 834 | 0.009 753 275 967  | -0.010 546 525 458 |
| C                                                                 | -0.099 671 969 969 | -0.158 572 272 063 | -0.099 773 687 139 |
| C                                                                 | 0.011 856 219 034  | 0.010 393 429 350  | -0.013 715 628 601 |
| C                                                                 | 0.027 487 265 734  | 0.003 089 173 657  | -0.030 727 764 046 |
| C                                                                 | 0.056 225 524 003  | -0.025 071 462 560 | 0.064 258 635 371  |
| C                                                                 | 0.018 528 974 212  | -0.161 268 381 419 | 0.051 638 106 270  |
| C                                                                 | -0.043 897 889 465 | -0.056 101 422 333 | -0.052 825 091 430 |
| H                                                                 | 0.137 081 738 853  | 0.329 460 032 556  | 0.446 533 488 757  |
| H                                                                 | -0.005 265 456 450 | -0.018 653 048 063 | 0.050 616 592 800  |
| H                                                                 | 0.036 069 680 688  | -0.033 736 545 168 | 0.032 902 553 210  |
| H                                                                 | -0.114 642 460 229 | -0.076 973 467 982 | -0.176 124 865 036 |
| H                                                                 | 0.214 291 477 968  | 0.220 540 939 002  | -0.102 006 076 690 |
| H                                                                 | -0.078 264 147 710 | 0.028 415 232 385  | 0.096 145 652 669  |
| H                                                                 | -0.008 049 196 578 | -0.007 336 010 793 | 0.018 452 887 693  |
| H                                                                 | -0.033 185 431 603 | -0.013 590 139 270 | 0.002 737 329 447  |
| H                                                                 | -0.015 692 278 702 | -0.036 114 708 796 | 0.012 453 818 313  |
| H                                                                 | 0.034 868 468 794  | 0.059 331 798 205  | -0.013 399 641 633 |
| H                                                                 | 0.159 572 856 842  | 0.411 511 554 354  | -0.143 233 321 021 |
| H                                                                 | 0.026 646 163 408  | 0.153 623 577 690  | 0.163 509 594 427  |
| H                                                                 | 0.009 837 460 351  | -0.037 571 879 817 | 0.056 346 062 147  |
| H                                                                 | -0.116 213 647 630 | 0.108 770 469 728  | -0.032 197 073 086 |
| H                                                                 | -0.220 865 757 725 | 0.155 713 473 161  | -0.053 960 463 018 |
| H                                                                 | 0.116 323 214 735  | 0.081 348 074 990  | -0.036 592 129 703 |

Wavenumber/cm<sup>-1</sup>: 207.6627

| $\frac{\partial \mu_{x,y,z}}{\partial Q_r} / (e u^{-0.5})$        | 0.016 329 587 301                   | 0.003 551 374 438                  | 0.002 245 869 125  |
|-------------------------------------------------------------------|-------------------------------------|------------------------------------|--------------------|
| <i>l</i> -matrix coefficients/(u <sup>1/2</sup> Å <sup>-1</sup> ) |                                     |                                    |                    |
| O                                                                 | -0.000 539 837 554                  | 0.001 173 403 682                  | -0.000 744 920 782 |
| C                                                                 | 0.000 113 834 849                   | -0.001 259 850 372                 | 0.000 104 567 713  |
| C                                                                 | $-8.254 878 900 000 \times 10^{-5}$ | $4.206 679 400 000 \times 10^{-5}$ | 0.000 156 668 218  |
| C                                                                 | 0.000 339 279 569                   | -0.002 370 781 089                 | 0.004 958 109 184  |
| C                                                                 | 0.008 923 264 621                   | -0.010 532 602 949                 | 0.009 596 213 089  |
| C                                                                 | -0.026 495 536 728                  | -0.038 860 131 376                 | -0.024 683 286 592 |
| C                                                                 | -0.019 518 443 304                  | -0.019 107 656 440                 | 0.031 575 983 610  |
| C                                                                 | -0.003 808 149 780                  | -0.006 715 154 252                 | 0.003 888 711 603  |
| C                                                                 | -0.012 863 605 435                  | 0.010 926 899 611                  | -0.017 382 234 655 |
| C                                                                 | -0.006 066 812 233                  | -0.015 696 481 730                 | 0.012 948 975 096  |
| C                                                                 | -0.007 493 871 614                  | -0.074 442 599 053                 | 0.284 330 026 303  |
| H                                                                 | 0.032 372 130 443                   | 0.079 538 041 693                  | 0.106 379 962 758  |
| H                                                                 | 0.013 836 213 561                   | 0.039 610 976 955                  | -0.110 450 113 009 |
| H                                                                 | -0.033 323 206 345                  | 0.033 780 359 802                  | -0.034 158 660 918 |
| H                                                                 | 0.029 551 653 301                   | 0.018 093 050 624                  | 0.042 329 461 689  |
| H                                                                 | 0.057 378 886 293                   | 0.059 718 718 782                  | -0.027 833 122 215 |
| H                                                                 | 0.002 280 528 712                   | -0.001 463 227 485                 | -0.003 883 034 524 |
| H                                                                 | 0.015 865 062 589                   | -0.005 012 192 769                 | -0.024 461 468 228 |
| H                                                                 | 0.054 828 944 265                   | 0.024 171 929 779                  | -0.001 169 610 020 |
| H                                                                 | 0.011 871 895 798                   | 0.026 080 170 615                  | -0.009 626 110 700 |
| H                                                                 | -0.014 715 423 178                  | -0.027 325 449 891                 | 0.008 908 880 921  |
| H                                                                 | 0.019 476 058 214                   | 0.051 263 859 183                  | -0.017 522 844 702 |
| H                                                                 | -0.055 875 162 424                  | -0.280 535 402 658                 | -0.274 438 580 407 |
| H                                                                 | -0.144 518 632 868                  | 0.386 851 220 144                  | -0.665 722 764 928 |
| H                                                                 | 0.031 300 108 535                   | -0.028 914 894 965                 | 0.009 368 029 493  |
| H                                                                 | -0.014 020 750 688                  | 0.008 918 318 117                  | -0.002 342 001 414 |
| H                                                                 | 0.226 961 565 142                   | 0.156 018 941 573                  | -0.046 968 995 452 |

Wavenumber/cm<sup>-1</sup>: 230.2238

| $\frac{\partial \mu_{x,y,z}}{\partial Q_r} / (e u^{-0.5})$        | 0.002 168 555 656  | -0.001 044 295 725 | 0.000 783 679 593  |
|-------------------------------------------------------------------|--------------------|--------------------|--------------------|
| <i>l</i> -matrix coefficients/(u <sup>1/2</sup> Å <sup>-1</sup> ) |                    |                    |                    |
| O                                                                 | -0.000 114 342 354 | 0.000 633 114 918  | -0.000 804 832 931 |
| C                                                                 | -0.000 519 156 524 | -0.000 685 695 811 | 0.001 453 449 382  |
| C                                                                 | 0.002 056 186 737  | -0.002 604 762 359 | 0.001 554 399 404  |
| C                                                                 | -0.000 300 772 509 | 0.000 848 029 572  | 0.000 371 235 831  |
| C                                                                 | 0.014 980 833 825  | -0.012 814 585 371 | 0.012 156 717 532  |
| C                                                                 | 0.035 550 765 170  | 0.057 025 583 739  | 0.036 467 777 641  |
| C                                                                 | 0.014 669 796 201  | 0.013 808 062 092  | -0.021 913 257 903 |
| C                                                                 | 0.030 202 978 161  | 0.005 156 916 248  | -0.034 406 135 195 |
| C                                                                 | 0.098 286 100 416  | -0.202 690 550 370 | 0.156 187 747 839  |
| C                                                                 | 0.014 194 484 722  | 0.043 609 177 656  | -0.037 286 412 104 |
| C                                                                 | -0.016 114 426 444 | -0.030 895 368 744 | 0.035 658 561 985  |
| H                                                                 | -0.049 044 226 191 | -0.119 008 207 387 | -0.160 968 960 758 |
| H                                                                 | -0.007 013 233 247 | -0.027 605 288 648 | 0.071 963 485 179  |
| H                                                                 | -0.046 144 971 669 | 0.047 056 472 635  | -0.044 368 719 668 |
| H                                                                 | -0.194 646 094 168 | -0.143 215 773 202 | -0.295 753 272 376 |
| H                                                                 | -0.076 747 244 612 | -0.077 888 330 150 | 0.036 760 184 798  |
| H                                                                 | -0.079 312 293 820 | 0.029 689 186 787  | 0.099 012 960 994  |
| H                                                                 | -0.046 905 290 741 | 0.015 324 434 730  | 0.071 526 193 268  |
| H                                                                 | -0.044 766 515 206 | -0.019 620 955 242 | 0.001 712 626 358  |
| H                                                                 | -0.021 604 877 554 | -0.048 473 360 689 | 0.016 601 664 022  |
| H                                                                 | 0.249 768 136 757  | 0.480 687 029 422  | -0.127 680 319 504 |
| H                                                                 | -0.048 954 576 803 | -0.132 912 838 695 | 0.046 487 140 937  |
| H                                                                 | -0.001 382 484 557 | -0.005 751 533 280 | -0.001 212 954 636 |
| H                                                                 | -0.023 105 864 155 | 0.057 171 472 091  | -0.101 954 924 966 |
| H                                                                 | -0.400 995 154 093 | 0.363 805 001 576  | -0.114 844 092 323 |
| H                                                                 | 0.045 280 835 069  | -0.031 251 691 901 | 0.007 728 276 657  |
| H                                                                 | 0.079 773 486 574  | 0.055 617 147 349  | -0.020 442 607 946 |

Wavenumber/cm<sup>-1</sup>: 261.8736

| $\frac{\partial \mu_{x,y,z}}{\partial Q_r} / (e u^{-0.5})$   |                                      |                    |                                       |
|--------------------------------------------------------------|--------------------------------------|--------------------|---------------------------------------|
|                                                              | -0.006 821 212 060                   | -0.000 812 456 435 | 0.002 587 905 946                     |
| $l$ -matrix coefficients/(u <sup>1/2</sup> Å <sup>-1</sup> ) |                                      |                    |                                       |
| O                                                            | 4.142 832 000 000 × 10 <sup>-6</sup> | -0.000 525 002 634 | 0.000 272 731 495                     |
| C                                                            | 0.001 608 785 780                    | 0.000 864 076 673  | -7.338 789 400 000 × 10 <sup>-5</sup> |
| C                                                            | -0.002 331 650 255                   | 0.003 217 539 395  | -0.000 707 307 415                    |
| C                                                            | -0.001 995 062 478                   | -0.002 877 814 913 | -0.000 788 566 880                    |
| C                                                            | -0.005 067 094 496                   | 0.002 660 516 671  | -0.003 299 400 298                    |
| C                                                            | -0.061 033 324 979                   | -0.091 908 883 658 | -0.051 283 650 827                    |
| C                                                            | -0.013 556 774 405                   | -0.010 055 374 452 | 0.013 651 627 250                     |
| C                                                            | 0.010 472 932 307                    | -0.003 668 538 924 | -0.012 518 679 351                    |
| C                                                            | -0.005 331 453 377                   | -0.007 408 982 562 | 0.000 292 166 866                     |
| C                                                            | -0.143 817 429 834                   | 0.205 189 907 383  | 0.029 991 241 760                     |
| C                                                            | -0.063 714 585 471                   | -0.087 254 919 813 | -0.041 372 553 731                    |
| H                                                            | 0.074 191 339 870                    | 0.176 834 934 001  | 0.240 809 050 190                     |
| H                                                            | 0.005 440 412 411                    | 0.016 152 468 390  | -0.041 563 182 850                    |
| H                                                            | 0.013 428 157 510                    | -0.014 834 381 877 | 0.012 474 899 267                     |
| H                                                            | 0.002 849 123 299                    | 0.001 079 978 446  | 0.006 568 036 235                     |
| H                                                            | 0.136 227 214 304                    | 0.140 795 550 855  | -0.065 743 340 306                    |
| H                                                            | -0.037 216 351 291                   | 0.012 855 906 702  | 0.045 455 340 577                     |
| H                                                            | 0.214 894 439 084                    | -0.040 170 963 928 | -0.346 981 184 212                    |
| H                                                            | 0.044 608 530 726                    | 0.020 964 246 231  | -0.001 614 818 351                    |
| H                                                            | 0.001 542 170 586                    | 0.001 676 197 210  | -0.001 114 046 440                    |
| H                                                            | 0.013 344 839 878                    | 0.028 573 588 785  | -0.011 155 829 389                    |
| H                                                            | -0.143 499 668 635                   | -0.352 136 806 272 | 0.130 458 642 167                     |
| H                                                            | 0.033 177 054 680                    | 0.181 899 736 141  | 0.195 855 248 824                     |
| H                                                            | -0.003 488 542 549                   | -0.010 226 765 744 | 0.004 759 156 654                     |
| H                                                            | 0.005 380 412 836                    | -0.006 116 983 328 | -0.000 432 044 984                    |
| H                                                            | 0.431 266 602 458                    | -0.317 061 052 306 | 0.117 367 026 707                     |
| H                                                            | 0.190 843 613 580                    | 0.131 575 179 850  | -0.058 024 165 772                    |

Wavenumber/cm<sup>-1</sup>: 294.1185

| $\frac{\partial \mu_{x,y,z}}{\partial Q_r} / (e u^{-0.5})$        |                                       |                    |                                       |
|-------------------------------------------------------------------|---------------------------------------|--------------------|---------------------------------------|
|                                                                   | -0.007 807 318 730                    | -0.001 281 797 424 | -0.006 487 555 332                    |
| <i>l</i> -matrix coefficients/(u <sup>1/2</sup> Å <sup>-1</sup> ) |                                       |                    |                                       |
| O                                                                 | 9.321 714 100 000 × 10 <sup>-5</sup>  | -0.001 814 559 253 | 0.000 733 637 206                     |
| C                                                                 | -0.001 427 569 334                    | 0.002 391 017 136  | -0.001 043 200 344                    |
| C                                                                 | -4.788 542 200 000 × 10 <sup>-5</sup> | 0.000 238 902 540  | -5.472 611 500 000 × 10 <sup>-5</sup> |
| C                                                                 | 0.002 916 536 364                     | 0.002 596 020 693  | 0.000 609 852 943                     |
| C                                                                 | 0.000 397 951 526                     | -0.001 772 700 434 | 0.000 566 923 712                     |
| C                                                                 | -0.054 172 493 795                    | -0.083 389 633 963 | -0.047 868 632 282                    |
| C                                                                 | 0.031 224 918 770                     | 0.021 667 994 104  | -0.025 642 057 729                    |
| C                                                                 | 0.019 502 429 201                     | 0.013 901 033 006  | -0.019 611 787 995                    |
| C                                                                 | 0.027 550 766 268                     | -0.022 170 139 788 | 0.030 630 413 243                     |
| C                                                                 | -0.053 579 873 473                    | 0.046 004 107 855  | 0.022 364 036 510                     |
| C                                                                 | 0.143 076 175 122                     | 0.217 491 423 010  | 0.053 112 772 719                     |
| H                                                                 | 0.067 072 429 022                     | 0.164 161 522 699  | 0.220 925 328 309                     |
| H                                                                 | -0.009 702 841 607                    | -0.032 095 535 598 | 0.082 150 473 869                     |
| H                                                                 | -0.004 497 820 691                    | 0.004 882 241 629  | -0.005 324 553 603                    |
| H                                                                 | -0.050 708 276 843                    | -0.034 738 103 346 | -0.075 486 951 827                    |
| H                                                                 | 0.121 670 640 583                     | 0.122 887 137 378  | -0.056 080 502 085                    |
| H                                                                 | -0.036 164 419 963                    | 0.014 282 283 004  | 0.045 760 299 015                     |
| H                                                                 | 0.081 848 772 853                     | -0.017 005 575 010 | -0.131 949 529 074                    |
| H                                                                 | -0.098 788 848 032                    | -0.046 600 799 115 | 0.004 663 589 772                     |
| H                                                                 | -0.029 414 125 442                    | -0.062 545 330 932 | 0.023 853 963 984                     |
| H                                                                 | 0.024 391 785 966                     | 0.044 534 655 979  | -0.009 561 876 269                    |
| H                                                                 | -0.022 640 278 190                    | -0.048 063 641 358 | 0.019 808 954 546                     |
| H                                                                 | -0.071 918 904 074                    | -0.393 025 486 643 | -0.430 314 590 537                    |
| H                                                                 | 0.033 045 089 286                     | -0.045 433 405 793 | 0.110 606 679 631                     |
| H                                                                 | -0.069 922 564 850                    | 0.065 406 696 085  | -0.019 646 161 698                    |
| H                                                                 | 0.125 837 658 549                     | -0.093 912 892 511 | 0.035 787 263 771                     |
| H                                                                 | -0.458 979 752 732                    | -0.315 399 923 917 | 0.136 789 452 437                     |

Wavenumber/cm<sup>-1</sup>: 300.8309

| $\frac{\partial \mu_{x,y,z}}{\partial Q_r} / (e u^{-0.5})$        |                                      |                    |                    |
|-------------------------------------------------------------------|--------------------------------------|--------------------|--------------------|
|                                                                   | -0.011 176 317 443                   | 0.003 572 557 754  | -0.000 501 672 683 |
| <i>l</i> -matrix coefficients/(u <sup>1/2</sup> Å <sup>-1</sup> ) |                                      |                    |                    |
| O                                                                 | 2.356 101 400 000 × 10 <sup>-5</sup> | 0.001 098 123 739  | -0.000 118 667 362 |
| C                                                                 | 1.814 955 900 000 × 10 <sup>-5</sup> | -0.004 169 852 722 | 0.000 765 290 664  |
| C                                                                 | -0.003 318 593 871                   | -0.000 741 748 235 | 0.000 155 837 679  |
| C                                                                 | 0.003 162 674 221                    | -0.000 634 602 869 | 0.000 119 051 152  |
| C                                                                 | -0.109 660 684 106                   | 0.113 429 885 072  | -0.104 019 039 414 |
| C                                                                 | 0.024 966 281 507                    | 0.020 199 533 513  | -0.019 693 715 166 |
| C                                                                 | 0.120 115 562 488                    | 0.089 464 473 546  | -0.118 049 800 679 |
| C                                                                 | -0.024 347 833 228                   | 0.069 952 539 643  | 0.041 867 913 158  |
| C                                                                 | -0.015 383 807 974                   | -0.001 697 774 876 | -0.004 093 906 713 |
| C                                                                 | -0.012 054 599 245                   | 0.010 642 342 715  | 0.001 603 948 107  |
| C                                                                 | -0.006 809 327 479                   | -0.034 219 265 818 | 0.033 735 836 352  |
| H                                                                 | 0.006 186 894 315                    | 0.019 357 891 866  | 0.024 047 001 905  |
| H                                                                 | -0.047 154 966 066                   | -0.148 833 965 077 | 0.392 046 959 252  |
| H                                                                 | 0.370 032 152 073                    | -0.381 330 481 338 | 0.354 570 942 367  |
| H                                                                 | 0.007 581 920 253                    | 0.004 864 200 256  | 0.014 160 775 805  |
| H                                                                 | -0.089 199 153 347                   | -0.091 437 596 087 | 0.039 809 875 192  |
| H                                                                 | 0.170 421 291 324                    | -0.055 262 034 267 | -0.212 637 269 450 |
| H                                                                 | 0.011 715 672 773                    | -0.001 742 015 097 | -0.019 275 983 305 |
| H                                                                 | -0.362 761 360 446                   | -0.163 128 669 736 | 0.018 864 316 150  |
| H                                                                 | -0.088 295 314 616                   | -0.175 995 334 278 | 0.071 076 667 839  |
| H                                                                 | 0.013 788 868 137                    | 0.028 374 802 251  | -0.009 656 501 000 |
| H                                                                 | -0.002 860 747 891                   | -0.009 372 863 939 | 0.004 737 212 414  |
| H                                                                 | 0.001 764 187 195                    | 0.014 026 464 618  | 0.019 641 213 897  |
| H                                                                 | -0.027 031 416 222                   | 0.071 199 209 345  | -0.125 623 234 720 |
| H                                                                 | 0.032 224 007 935                    | -0.029 389 324 010 | 0.008 565 762 303  |
| H                                                                 | 0.036 549 617 644                    | -0.023 994 005 383 | 0.009 999 689 435  |
| H                                                                 | 0.047 417 691 621                    | 0.033 090 962 047  | -0.011 272 870 325 |

Wavenumber/cm<sup>-1</sup>: 328.1666

| $\frac{\partial \mu_{x,y,z}}{\partial Q_r} / (e u^{-0.5})$        |                                       |                    |                    |
|-------------------------------------------------------------------|---------------------------------------|--------------------|--------------------|
|                                                                   | -0.001 313 625 997                    | -0.000 698 820 022 | 0.004 308 129 703  |
| <i>l</i> -matrix coefficients/(u <sup>1/2</sup> Å <sup>-1</sup> ) |                                       |                    |                    |
| O                                                                 | -8.039 124 300 000 × 10 <sup>-5</sup> | -0.001 534 567 668 | 0.001 116 441 268  |
| C                                                                 | -0.000 460 929 205                    | 0.003 108 575 365  | -0.001 995 897 544 |
| C                                                                 | 0.001 875 245 709                     | 0.000 530 336 067  | -0.000 168 819 148 |
| C                                                                 | -0.000 770 300 037                    | 0.002 313 652 375  | -0.002 193 696 208 |
| C                                                                 | 0.108 820 366 829                     | -0.113 867 866 733 | 0.104 285 378 944  |
| C                                                                 | -0.023 767 112 327                    | -0.023 336 777 548 | 0.013 517 838 218  |
| C                                                                 | 0.113 573 016 543                     | 0.098 095 613 934  | -0.146 713 025 040 |
| C                                                                 | -0.050 127 103 306                    | -0.014 860 303 690 | 0.055 374 289 496  |
| C                                                                 | -0.013 980 490 287                    | 0.011 632 656 986  | -0.020 659 719 861 |
| C                                                                 | 0.002 035 244 164                     | 0.004 628 982 836  | 0.006 283 607 747  |
| C                                                                 | -0.013 507 861 648                    | -0.030 139 876 770 | 0.000 774 934 816  |
| H                                                                 | -0.001 000 529 484                    | -0.003 946 966 139 | -0.003 109 132 788 |
| H                                                                 | -0.059 775 792 421                    | -0.184 445 169 803 | 0.486 450 323 731  |
| H                                                                 | -0.369 671 162 762                    | 0.382 568 829 834  | -0.353 286 839 401 |
| H                                                                 | 0.033 756 251 078                     | 0.023 572 033 617  | 0.052 220 995 912  |
| H                                                                 | 0.082 262 299 721                     | 0.082 710 924 315  | -0.035 184 563 542 |
| H                                                                 | 0.129 361 264 819                     | -0.044 901 563 998 | -0.159 383 552 930 |
| H                                                                 | 0.016 533 898 775                     | -0.004 154 949 407 | -0.024 957 583 757 |
| H                                                                 | -0.336 422 578 532                    | -0.151 016 384 551 | 0.016 269 051 636  |
| H                                                                 | 0.045 097 744 334                     | 0.096 081 092 839  | -0.031 753 379 691 |
| H                                                                 | -0.019 514 246 835                    | -0.035 393 196 128 | 0.006 901 522 975  |
| H                                                                 | -0.010 883 772 781                    | -0.022 899 588 188 | 0.007 591 529 556  |
| H                                                                 | 0.009 157 724 152                     | 0.048 570 339 061  | 0.054 977 132 518  |
| H                                                                 | -0.009 502 841 742                    | 0.022 157 371 371  | -0.044 275 438 303 |
| H                                                                 | 0.032 917 732 178                     | -0.031 290 296 322 | 0.010 856 624 950  |
| H                                                                 | -0.015 678 163 798                    | 0.010 599 126 443  | -0.004 077 180 575 |
| H                                                                 | 0.046 706 570 882                     | 0.031 562 673 045  | -0.013 046 231 596 |



Wavenumber/cm<sup>-1</sup>: 371.6839

| $\frac{\partial \mu_{x,y,z}}{\partial Q_r} / (e u^{-0.5})$        |                    |                    |                    |
|-------------------------------------------------------------------|--------------------|--------------------|--------------------|
|                                                                   | -0.002 983 368 787 | -0.001 523 061 177 | 0.010 651 361 906  |
| <i>l</i> -matrix coefficients/(u <sup>1/2</sup> Å <sup>-1</sup> ) |                    |                    |                    |
| O                                                                 | 0.000 176 459 613  | 0.001 124 608 230  | -0.000 779 131 110 |
| C                                                                 | -0.001 570 557 985 | -0.001 488 795 926 | 0.000 834 601 996  |
| C                                                                 | -0.000 123 016 982 | -0.002 520 043 380 | 0.000 680 246 497  |
| C                                                                 | 0.001 658 892 906  | -0.000 962 482 586 | -0.000 411 291 339 |
| C                                                                 | 0.047 072 801 583  | -0.046 521 853 913 | 0.042 112 694 404  |
| C                                                                 | 0.026 931 536 659  | 0.015 401 646 630  | -0.044 858 631 348 |
| C                                                                 | 0.033 342 627 606  | -0.017 632 394 963 | 0.089 114 872 033  |
| C                                                                 | 0.044 077 477 604  | 0.203 245 551 261  | -0.019 352 140 142 |
| C                                                                 | -0.009 962 187 136 | -0.006 351 698 391 | -0.005 508 048 866 |
| C                                                                 | -0.004 567 232 682 | -0.004 265 440 264 | 0.004 473 833 366  |
| C                                                                 | -0.006 301 419 444 | -0.007 282 876 127 | -0.012 152 688 530 |
| H                                                                 | 0.034 088 382 714  | 0.076 417 819 109  | 0.099 454 588 763  |
| H                                                                 | 0.046 783 949 701  | 0.126 343 074 421  | -0.322 217 914 330 |
| H                                                                 | -0.157 519 582 818 | 0.165 111 026 148  | -0.148 953 644 477 |
| H                                                                 | 0.013 363 413 770  | 0.007 975 185 772  | 0.022 486 670 278  |
| H                                                                 | -0.125 734 013 460 | -0.130 814 255 841 | 0.051 983 179 971  |
| H                                                                 | 0.161 136 089 693  | -0.039 598 789 127 | -0.193 252 308 092 |
| H                                                                 | 0.006 819 207 155  | -0.002 189 779 753 | -0.011 071 983 855 |
| H                                                                 | -0.155 483 769 440 | -0.072 004 209 191 | 0.018 747 694 936  |
| H                                                                 | -0.318 953 264 215 | -0.647 992 795 435 | 0.260 601 220 805  |
| H                                                                 | 0.009 730 113 856  | 0.020 958 954 793  | -0.004 057 660 095 |
| H                                                                 | 0.004 537 719 984  | 0.020 028 527 728  | -0.006 464 794 272 |
| H                                                                 | 0.004 301 750 134  | 0.028 365 367 710  | 0.028 655 263 582  |
| H                                                                 | 0.003 710 673 340  | -0.010 283 172 073 | 0.018 851 419 272  |
| H                                                                 | 0.008 704 609 818  | -0.009 123 171 816 | 0.002 706 444 348  |
| H                                                                 | 0.000 709 101 846  | -0.002 459 767 663 | 0.000 495 927 863  |
| H                                                                 | 0.012 415 571 118  | 0.010 430 051 293  | -0.004 489 244 733 |

Wavenumber/cm<sup>-1</sup>: 424.595

| $\frac{\partial \mu_{x,y,z}}{\partial Q_r} / (e u^{-0.5})$        |                    |                    |                    |
|-------------------------------------------------------------------|--------------------|--------------------|--------------------|
|                                                                   | -0.000 770 124 063 | 0.009 982 903 381  | 0.003 466 532 016  |
| <i>l</i> -matrix coefficients/(u <sup>1/2</sup> Å <sup>-1</sup> ) |                    |                    |                    |
| O                                                                 | 0.000 214 640 425  | 0.001 119 202 639  | -0.000 653 209 640 |
| C                                                                 | -0.001 841 169 268 | -0.002 100 662 587 | 0.001 667 496 476  |
| C                                                                 | -0.001 124 188 207 | -0.001 054 528 641 | 0.000 595 097 282  |
| C                                                                 | 0.003 542 827 481  | 0.000 163 928 421  | 0.000 605 607 213  |
| C                                                                 | 0.016 520 120 751  | -0.015 826 456 797 | 0.017 844 704 852  |
| C                                                                 | 0.118 325 804 772  | 0.077 944 777 988  | -0.168 742 086 354 |
| C                                                                 | -0.005 247 124 722 | 0.004 150 774 570  | -0.014 493 144 032 |
| C                                                                 | -0.016 489 834 296 | -0.066 288 657 239 | 0.009 332 122 314  |
| C                                                                 | -0.002 480 937 886 | -0.000 757 113 217 | 0.001 121 614 852  |
| C                                                                 | -0.030 123 335 022 | -0.001 595 103 234 | -0.001 364 321 004 |
| C                                                                 | 0.007 884 740 208  | 0.001 806 837 491  | -0.001 661 890 644 |
| H                                                                 | 0.124 455 826 231  | 0.280 245 420 288  | 0.354 858 621 414  |
| H                                                                 | -0.008 784 531 924 | -0.022 230 792 753 | 0.054 664 200 130  |
| H                                                                 | -0.058 731 514 351 | 0.060 776 620 509  | -0.061 331 627 636 |
| H                                                                 | -0.001 524 442 088 | -0.001 062 864 959 | -0.002 804 328 031 |
| H                                                                 | -0.523 286 008 342 | -0.547 601 342 817 | 0.218 712 280 094  |
| H                                                                 | -0.046 958 748 046 | 0.009 584 483 475  | 0.055 732 018 748  |
| H                                                                 | -0.006 482 602 831 | 0.000 629 301 346  | 0.005 438 580 809  |
| H                                                                 | 0.023 419 324 767  | 0.009 767 530 688  | -0.004 708 134 130 |
| H                                                                 | 0.104 697 551 729  | 0.213 406 475 177  | -0.086 278 787 290 |
| H                                                                 | 0.004 911 419 922  | 0.010 332 504 848  | -0.001 350 563 189 |
| H                                                                 | 0.022 465 847 019  | 0.066 879 992 091  | -0.023 028 842 244 |
| H                                                                 | 0.001 397 378 755  | 0.006 952 028 420  | 0.006 919 691 286  |
| H                                                                 | -0.003 337 029 542 | 0.006 619 313 791  | -0.010 728 431 187 |
| H                                                                 | 0.005 604 385 322  | -0.005 450 917 210 | 0.001 459 322 099  |
| H                                                                 | 0.082 720 312 983  | -0.063 394 892 694 | 0.022 809 769 430  |
| H                                                                 | -0.028 534 443 282 | -0.017 635 904 259 | 0.007 623 086 261  |

Wavenumber/cm<sup>-1</sup>: 450.8581

| $\frac{\partial \mu_{x,y,z}}{\partial Q_r} / (e u^{-0.5})$        | 0.007 498 485 804  | 0.002 783 560 097  | -0.009 035 241 004 |
|-------------------------------------------------------------------|--------------------|--------------------|--------------------|
| <i>l</i> -matrix coefficients/(u <sup>1/2</sup> Å <sup>-1</sup> ) |                    |                    |                    |
| O                                                                 | -0.000 430 295 155 | -0.001 066 625 582 | 0.000 535 631 938  |
| C                                                                 | 0.002 774 558 676  | 0.001 758 377 570  | -0.000 816 421 746 |
| C                                                                 | -0.000 235 747 263 | -0.000 618 321 532 | 0.000 324 862 738  |
| C                                                                 | -0.003 603 535 099 | -0.001 404 389 449 | 0.000 253 952 833  |
| C                                                                 | 0.008 568 957 751  | -0.006 379 604 312 | 0.006 857 785 989  |
| C                                                                 | 0.003 588 586 544  | -0.000 565 221 754 | -0.008 113 736 527 |
| C                                                                 | -0.175 071 838 755 | -0.034 119 816 381 | -0.121 550 332 940 |
| C                                                                 | 0.019 209 421 117  | 0.086 727 389 267  | -0.004 145 530 186 |
| C                                                                 | -0.005 267 189 686 | 0.000 212 071 881  | -0.001 520 745 024 |
| C                                                                 | -0.004 293 424 613 | -0.002 138 138 038 | -0.001 994 598 433 |
| C                                                                 | 0.003 728 354 059  | 0.003 429 329 523  | 0.007 315 511 828  |
| H                                                                 | 0.008 170 269 849  | 0.019 203 681 907  | 0.024 181 600 049  |
| H                                                                 | -0.077 696 277 740 | -0.189 504 857 756 | 0.472 401 341 201  |
| H                                                                 | -0.023 695 070 559 | 0.024 552 157 769  | -0.021 805 884 960 |
| H                                                                 | 0.001 645 969 195  | 0.001 318 570 420  | 0.003 788 686 479  |
| H                                                                 | -0.018 698 120 607 | -0.017 328 904 036 | 0.006 235 740 396  |
| H                                                                 | 0.076 479 339 651  | -0.019 381 976 594 | -0.094 327 011 793 |
| H                                                                 | -0.005 913 157 796 | 0.001 225 985 049  | 0.008 892 232 187  |
| H                                                                 | 0.671 486 927 440  | 0.310 844 637 662  | -0.059 533 799 200 |
| H                                                                 | -0.137 307 435 063 | -0.277 770 327 163 | 0.111 601 346 025  |
| H                                                                 | 0.003 566 152 067  | 0.007 858 764 972  | -0.003 139 915 447 |
| H                                                                 | 0.005 982 575 465  | 0.017 331 318 968  | -0.006 021 850 531 |
| H                                                                 | -0.000 933 300 979 | -0.014 124 293 065 | -0.015 128 198 086 |
| H                                                                 | -0.002 253 580 170 | 0.007 800 167 008  | -0.013 813 738 576 |
| H                                                                 | 0.011 819 890 619  | -0.011 085 857 932 | 0.004 106 939 397  |
| H                                                                 | 0.014 096 272 207  | -0.011 314 795 932 | 0.004 637 703 839  |
| H                                                                 | -0.005 161 259 191 | -0.007 278 482 351 | 0.001 728 253 817  |

Wavenumber/cm<sup>-1</sup>: 511.0485

| $\frac{\partial \mu_{x,y,z}}{\partial Q_r} / (e u^{-0.5})$        |                                      |                    |                    |
|-------------------------------------------------------------------|--------------------------------------|--------------------|--------------------|
|                                                                   | -0.000 624 469 813                   | 0.004 813 870 984  | 0.003 832 660 087  |
| <i>l</i> -matrix coefficients/(u <sup>1/2</sup> Å <sup>-1</sup> ) |                                      |                    |                    |
| O                                                                 | 3.026 964 300 000 × 10 <sup>-5</sup> | 0.002 392 753 799  | -0.001 110 399 821 |
| C                                                                 | 0.003 636 922 201                    | -0.005 535 743 517 | 0.002 198 180 442  |
| C                                                                 | -0.003 802 703 016                   | 0.002 001 364 339  | -0.001 592 695 950 |
| C                                                                 | -0.000 436 895 768                   | 0.000 957 925 007  | -0.000 212 178 553 |
| C                                                                 | 0.008 794 730 496                    | -0.005 212 746 412 | 0.006 434 571 860  |
| C                                                                 | -0.007 787 169 800                   | -0.001 187 382 348 | 0.022 916 926 500  |
| C                                                                 | 0.006 091 034 771                    | 0.002 061 380 157  | 0.001 919 071 118  |
| C                                                                 | 0.004 835 429 905                    | -0.002 420 132 591 | -0.005 652 599 925 |
| C                                                                 | -0.109 731 344 058                   | 0.050 547 861 889  | 0.057 159 263 308  |
| C                                                                 | -0.085 979 560 486                   | -0.017 816 125 512 | -0.073 742 026 163 |
| C                                                                 | -0.002 090 691 438                   | 0.003 070 227 255  | 0.002 086 753 432  |
| H                                                                 | -0.018 957 302 706                   | -0.044 321 672 817 | -0.058 246 598 092 |
| H                                                                 | 0.000 356 883 524                    | 0.003 556 648 521  | -0.009 510 616 888 |
| H                                                                 | -0.025 455 422 512                   | 0.022 880 326 031  | -0.022 648 109 577 |
| H                                                                 | -0.163 309 153 006                   | -0.097 814 070 188 | -0.237 555 485 864 |
| H                                                                 | 0.044 817 342 941                    | 0.048 253 985 384  | -0.017 856 981 785 |
| H                                                                 | -0.015 559 488 843                   | 0.006 425 673 705  | 0.018 787 360 738  |
| H                                                                 | -0.176 212 063 278                   | 0.041 431 017 853  | 0.265 121 816 225  |
| H                                                                 | -0.022 333 471 979                   | -0.010 599 556 737 | 0.001 675 165 344  |
| H                                                                 | 0.000 331 615 364                    | 0.000 111 672 017  | -0.001 162 538 355 |
| H                                                                 | 0.137 108 198 762                    | 0.295 597 007 163  | -0.080 368 313 646 |
| H                                                                 | 0.105 403 564 026                    | 0.293 967 429 959  | -0.106 020 187 794 |
| H                                                                 | -0.002 829 144 629                   | -0.013 393 512 559 | -0.013 609 965 478 |
| H                                                                 | 0.002 454 039 571                    | -0.004 788 156 840 | 0.008 424 249 088  |
| H                                                                 | 0.403 217 638 915                    | -0.372 864 967 801 | 0.125 151 326 398  |
| H                                                                 | 0.367 025 338 023                    | -0.275 829 812 460 | 0.094 198 035 415  |
| H                                                                 | 0.007 512 720 954                    | 0.006 492 748 350  | -0.001 705 722 487 |

Wavenumber/cm<sup>-1</sup>: 524.7886

| $\frac{\partial \mu_{x,y,z}}{\partial Q_r} / (e u^{-0.5})$        |                    |                    |                    |
|-------------------------------------------------------------------|--------------------|--------------------|--------------------|
|                                                                   | -0.005 610 607 932 | -0.000 246 662 410 | 0.011 848 925 989  |
| <i>l</i> -matrix coefficients/(u <sup>1/2</sup> Å <sup>-1</sup> ) |                    |                    |                    |
| O                                                                 | 0.000 105 850 000  | -0.002 659 852 463 | 0.001 005 449 382  |
| C                                                                 | 0.001 650 857 401  | 0.004 263 590 771  | -0.002 052 105 863 |
| C                                                                 | -0.000 378 053 136 | -0.000 685 242 934 | -0.000 180 568 958 |
| C                                                                 | 0.000 366 890 783  | -0.002 334 762 586 | 0.000 451 271 862  |
| C                                                                 | -0.001 701 408 181 | 0.001 541 893 782  | -0.001 741 283 224 |
| C                                                                 | 0.008 140 383 404  | 0.004 107 220 990  | -0.012 323 683 874 |
| C                                                                 | 0.005 476 374 855  | 0.004 665 622 215  | -0.010 200 695 473 |
| C                                                                 | -0.002 506 141 094 | -0.001 077 194 626 | 0.003 635 977 564  |
| C                                                                 | -0.042 291 438 984 | 0.014 166 262 867  | 0.018 312 199 379  |
| C                                                                 | 0.044 709 321 568  | 0.005 211 358 312  | 0.032 278 760 586  |
| C                                                                 | -0.136 285 384 115 | 0.065 894 352 118  | 0.028 600 895 367  |
| H                                                                 | 0.009 408 609 898  | 0.022 999 703 218  | 0.028 294 120 485  |
| H                                                                 | -0.004 977 647 168 | -0.012 223 478 993 | 0.030 557 340 018  |
| H                                                                 | 0.005 079 806 624  | -0.004 742 438 830 | 0.005 620 715 983  |
| H                                                                 | -0.055 591 647 090 | -0.031 484 442 075 | -0.078 901 568 631 |
| H                                                                 | -0.037 757 755 438 | -0.037 785 963 285 | 0.014 589 208 721  |
| H                                                                 | 0.004 826 153 566  | -0.001 625 261 020 | -0.008 502 269 911 |
| H                                                                 | 0.077 600 458 733  | -0.017 928 370 090 | -0.113 681 483 568 |
| H                                                                 | -0.014 135 576 227 | -0.004 830 240 546 | 0.001 137 362 580  |
| H                                                                 | 0.003 281 222 694  | 0.007 431 180 663  | -0.002 893 405 033 |
| H                                                                 | 0.054 741 481 723  | 0.117 883 664 793  | -0.030 391 407 076 |
| H                                                                 | -0.047 571 800 005 | -0.135 850 887 509 | 0.049 449 677 387  |
| H                                                                 | -0.073 813 599 424 | -0.336 234 501 800 | -0.358 580 154 550 |
| H                                                                 | 0.075 102 645 583  | -0.220 427 856 894 | 0.392 844 420 951  |
| H                                                                 | 0.145 907 058 154  | -0.135 155 761 393 | 0.047 296 910 746  |
| H                                                                 | -0.181 883 669 936 | 0.137 989 711 616  | -0.045 582 683 600 |
| H                                                                 | 0.463 330 101 620  | 0.332 044 049 352  | -0.131 268 748 406 |

Wavenumber/cm<sup>-1</sup>: 599.6642

| $\frac{\partial \mu_{x,y,z}}{\partial Q_r} / (e u^{-0.5})$        |                                      |                                      |                    |
|-------------------------------------------------------------------|--------------------------------------|--------------------------------------|--------------------|
|                                                                   | -0.005 450 327 416                   | 0.001 779 512 892                    | 0.005 283 649 566  |
| <i>l</i> -matrix coefficients/(u <sup>1/2</sup> Å <sup>-1</sup> ) |                                      |                                      |                    |
| O                                                                 | 4.183 701 100 000 × 10 <sup>-5</sup> | 0.000 558 469 540                    | -0.000 648 949 785 |
| C                                                                 | -0.001 428 902 266                   | -0.001 474 151 197                   | 0.001 071 079 271  |
| C                                                                 | 0.000 676 115 083                    | 2.173 183 700 000 × 10 <sup>-5</sup> | -0.001 244 724 570 |
| C                                                                 | 0.000 289 714 599                    | 0.000 593 110 849                    | -0.000 277 300 856 |
| C                                                                 | 0.001 191 102 774                    | -0.001 359 099 731                   | 0.001 923 126 237  |
| C                                                                 | 0.001 638 653 248                    | -0.002 536 519 847                   | -0.014 606 714 359 |
| C                                                                 | -0.008 058 392 920                   | -0.004 516 686 953                   | 0.005 222 201 083  |
| C                                                                 | 0.007 041 885 102                    | -0.003 982 450 962                   | -0.009 165 966 708 |
| C                                                                 | -0.084 859 406 501                   | 0.039 110 697 712                    | 0.055 544 960 999  |
| C                                                                 | 0.091 033 222 939                    | 0.015 388 953 717                    | 0.066 534 980 928  |
| C                                                                 | 0.065 036 224 665                    | -0.026 124 545 353                   | -0.011 763 844 885 |
| H                                                                 | 0.013 370 652 188                    | 0.029 684 853 413                    | 0.040 242 594 126  |
| H                                                                 | 0.000 200 642 403                    | 0.005 461 283 383                    | -0.015 278 805 069 |
| H                                                                 | -0.004 226 363 767                   | 0.005 005 836 456                    | -0.004 339 434 409 |
| H                                                                 | -0.152 916 179 877                   | -0.092 178 968 868                   | -0.222 990 044 080 |
| H                                                                 | -0.020 608 047 350                   | -0.022 686 461 631                   | 0.008 598 864 621  |
| H                                                                 | -0.026 165 516 951                   | 0.009 094 121 147                    | 0.032 358 532 474  |
| H                                                                 | 0.164 213 735 292                    | -0.037 875 257 577                   | -0.242 159 818 517 |
| H                                                                 | 0.025 434 230 031                    | 0.010 839 643 838                    | -0.002 217 455 393 |
| H                                                                 | 0.003 948 853 708                    | 0.005 997 143 327                    | -0.003 044 233 053 |
| H                                                                 | 0.119 581 852 415                    | 0.256 674 790 349                    | -0.066 875 661 145 |
| H                                                                 | -0.102 579 409 748                   | -0.295 718 390 018                   | 0.107 537 768 433  |
| H                                                                 | 0.032 759 314 827                    | 0.146 453 620 405                    | 0.155 476 726 688  |
| H                                                                 | -0.034 663 739 771                   | 0.100 721 607 910                    | -0.178 807 803 308 |
| H                                                                 | 0.324 075 477 196                    | -0.300 513 771 261                   | 0.102 780 526 065  |
| H                                                                 | -0.371 702 859 902                   | 0.282 103 605 812                    | -0.093 554 501 330 |
| H                                                                 | -0.221 365 867 205                   | -0.157 486 198 478                   | 0.063 003 036 795  |

Wavenumber/cm<sup>-1</sup>: 664.6703

| $\frac{\partial \mu_{x,y,z}}{\partial Q_r} / (e u^{-0.5})$        | 0.009 856 945 555                   | 4.160 022 496 696 $\times 10^{-5}$ | -0.002 191 273 885                  |
|-------------------------------------------------------------------|-------------------------------------|------------------------------------|-------------------------------------|
| <i>l</i> -matrix coefficients/(u <sup>1/2</sup> Å <sup>-1</sup> ) |                                     |                                    |                                     |
| O                                                                 | 0.038 831 529 948                   | 0.542 336 489 301                  | -0.243 739 825 844                  |
| C                                                                 | -0.057 040 419 841                  | -0.723 179 421 414                 | 0.327 445 291 426                   |
| C                                                                 | 0.011 771 119 289                   | 0.039 716 346 912                  | -0.013 845 614 956                  |
| C                                                                 | 0.008 104 464 821                   | 0.031 493 080 423                  | -0.017 400 744 312                  |
| C                                                                 | -0.007 987 342 491                  | 0.023 076 723 604                  | -0.010 755 438 983                  |
| C                                                                 | 0.003 498 861 227                   | 0.018 616 674 178                  | -0.016 117 413 412                  |
| C                                                                 | 0.001 846 938 579                   | 0.017 268 798 976                  | 0.012 001 085 993                   |
| C                                                                 | -6.552 156 500 000 $\times 10^{-5}$ | -0.002 721 334 463                 | 0.000 411 822 291                   |
| C                                                                 | -0.008 092 140 411                  | -0.003 772 327 327                 | 0.010 596 736 008                   |
| C                                                                 | -0.008 218 336 447                  | -0.008 669 302 239                 | -0.008 913 665 918                  |
| C                                                                 | 0.002 678 179 681                   | -0.010 005 730 892                 | 0.005 378 203 460                   |
| H                                                                 | -0.002 831 597 626                  | -0.010 294 246 692                 | 0.006 755 662 636                   |
| H                                                                 | -0.008 791 173 366                  | -0.015 435 237 342                 | -0.002 602 585 486                  |
| H                                                                 | -0.002 497 254 075                  | 0.009 569 635 020                  | -0.008 001 904 280                  |
| H                                                                 | 0.009 789 215 416                   | -0.009 373 607 262                 | 0.002 839 914 811                   |
| H                                                                 | 0.008 128 003 953                   | 0.005 904 920 488                  | 0.002 018 075 424                   |
| H                                                                 | 0.000 155 695 762                   | -0.003 538 352 430                 | 0.001 501 285 807                   |
| H                                                                 | 0.008 769 288 880                   | -0.004 286 968 967                 | 0.001 962 930 400                   |
| H                                                                 | 0.006 326 893 429                   | -0.007 134 286 126                 | -0.020 112 541 828                  |
| H                                                                 | 0.001 046 707 569                   | -0.002 623 993 275                 | -0.005 896 304 610                  |
| H                                                                 | 0.011 214 590 702                   | -0.009 241 499 400                 | 0.010 905 258 622                   |
| H                                                                 | 0.013 599 315 319                   | -0.012 117 207 821                 | 0.002 795 364 809                   |
| H                                                                 | 0.000 393 719 420                   | -0.008 434 030 039                 | -1.702 425 900 000 $\times 10^{-5}$ |
| H                                                                 | -0.015 708 920 147                  | -0.017 555 177 471                 | 0.002 355 623 101                   |
| H                                                                 | 0.011 958 691 843                   | 0.007 583 334 221                  | -0.026 352 927 167                  |
| H                                                                 | 0.010 176 431 379                   | 0.022 924 073 329                  | 0.013 876 651 845                   |
| H                                                                 | -0.021 742 015 728                  | 0.027 274 685 714                  | -0.007 881 761 709                  |

Wavenumber/cm<sup>-1</sup>: 724.8753

| $\frac{\partial \mu_{x,y,z}}{\partial Q_r} / (e u^{-0.5})$        | 0.041 056 540 017  | -0.004 004 822 338 | 0.005 870 688 593                     |
|-------------------------------------------------------------------|--------------------|--------------------|---------------------------------------|
| <i>l</i> -matrix coefficients/(u <sup>1/2</sup> Å <sup>-1</sup> ) |                    |                    |                                       |
| O                                                                 | 0.004 697 122 394  | -0.002 157 025 032 | -1.117 231 000 000 × 10 <sup>-6</sup> |
| C                                                                 | -0.034 067 247 819 | 0.008 940 874 459  | 0.000 172 341 516                     |
| C                                                                 | 0.043 077 516 544  | -0.056 855 602 046 | 0.023 920 308 373                     |
| C                                                                 | 0.051 477 938 176  | -0.018 405 742 470 | -0.001 919 508 618                    |
| C                                                                 | -0.026 177 207 154 | 0.032 513 493 111  | -0.013 729 824 764                    |
| C                                                                 | 0.047 766 454 714  | 0.004 269 130 023  | -0.130 181 959 254                    |
| C                                                                 | 0.055 977 150 488  | 0.021 306 357 674  | 0.074 290 432 897                     |
| C                                                                 | -0.025 728 689 901 | 0.164 611 913 955  | 0.083 597 657 645                     |
| C                                                                 | 0.022 777 401 810  | -0.032 966 151 873 | 0.062 428 656 948                     |
| C                                                                 | 0.020 836 852 487  | -0.026 425 546 900 | -0.033 976 217 323                    |
| C                                                                 | -0.004 387 030 949 | 0.008 631 162 628  | -0.001 906 600 793                    |
| H                                                                 | -0.200 772 907 374 | -0.170 153 601 306 | 0.165 880 625 963                     |
| H                                                                 | -0.197 834 744 278 | -0.073 600 818 453 | -0.043 252 941 525                    |
| H                                                                 | 0.010 009 191 697  | 0.022 632 665 618  | -0.015 525 532 388                    |
| H                                                                 | 0.075 506 717 210  | 0.229 546 436 097  | -0.134 081 595 938                    |
| H                                                                 | 0.014 968 723 374  | 0.128 237 248 981  | 0.282 657 236 683                     |
| H                                                                 | -0.121 854 538 581 | -0.427 908 348 446 | 0.055 149 476 841                     |
| H                                                                 | 0.060 566 056 368  | 0.139 976 213 120  | 0.007 794 341 305                     |
| H                                                                 | -0.021 226 888 638 | 0.043 654 767 155  | -0.206 618 120 835                    |
| H                                                                 | 0.227 162 915 591  | -0.210 403 564 219 | -0.314 106 673 491                    |
| H                                                                 | -0.138 254 053 520 | -0.006 667 901 982 | -0.240 065 557 615                    |
| H                                                                 | -0.117 829 268 010 | 0.080 865 674 219  | 0.112 616 530 096                     |
| H                                                                 | -0.009 579 825 387 | -0.006 473 903 558 | 0.008 894 864 966                     |
| H                                                                 | -0.010 571 667 449 | -0.005 378 453 534 | -0.003 294 419 044                    |
| H                                                                 | -0.050 911 363 273 | -0.031 959 525 324 | 0.111 823 871 050                     |
| H                                                                 | -0.053 427 385 785 | -0.082 037 805 094 | -0.006 986 458 253                    |
| H                                                                 | -0.007 823 342 276 | 0.013 666 748 258  | 0.002 695 817 544                     |



Wavenumber/cm<sup>-1</sup>: 788.4826

| $\frac{\partial \mu_{x,y,z}}{\partial Q_r} / (e u^{-0.5})$        | 0.066 087 480 061  | -0.005 542 189 317 | -0.005 209 555 136 |
|-------------------------------------------------------------------|--------------------|--------------------|--------------------|
| <i>l</i> -matrix coefficients/(u <sup>1/2</sup> Å <sup>-1</sup> ) |                    |                    |                    |
| O                                                                 | 0.000 381 408 246  | -0.030 798 090 259 | 0.012 924 246 868  |
| C                                                                 | -0.005 924 431 554 | 0.023 633 041 631  | -0.009 497 426 115 |
| C                                                                 | -0.015 945 878 581 | 0.079 400 269 498  | -0.042 442 914 676 |
| C                                                                 | 0.046 944 024 314  | -0.008 640 226 115 | -0.003 480 195 683 |
| C                                                                 | -0.003 912 174 630 | -0.014 534 166 168 | -0.005 513 459 046 |
| C                                                                 | 0.053 247 192 003  | 0.021 656 558 102  | -0.160 799 682 653 |
| C                                                                 | 0.046 406 941 915  | 0.004 658 396 399  | 0.057 849 459 262  |
| C                                                                 | 0.012 133 822 112  | -0.030 199 510 083 | -0.008 619 652 478 |
| C                                                                 | -0.032 224 138 525 | 0.081 983 213 972  | -0.046 650 940 632 |
| C                                                                 | -0.007 993 302 160 | 0.047 648 483 580  | -0.047 500 584 242 |
| C                                                                 | 0.004 216 673 090  | 0.012 047 166 917  | -0.005 540 315 019 |
| H                                                                 | -0.252 902 695 211 | -0.221 416 594 877 | 0.218 261 322 763  |
| H                                                                 | -0.174 713 396 709 | -0.068 380 929 675 | -0.039 141 676 755 |
| H                                                                 | -0.012 441 057 810 | -0.006 788 732 619 | 0.003 451 482 404  |
| H                                                                 | 0.020 416 993 042  | -0.384 774 871 778 | 0.143 305 458 216  |
| H                                                                 | 0.034 673 713 884  | 0.150 045 267 282  | 0.364 003 860 651  |
| H                                                                 | 0.029 733 604 672  | 0.103 955 248 530  | -0.010 978 370 194 |
| H                                                                 | 0.153 851 563 225  | -0.202 301 734 748 | 0.122 773 132 641  |
| H                                                                 | -0.023 208 736 501 | 0.042 378 405 308  | -0.184 449 828 188 |
| H                                                                 | -0.048 605 601 809 | 0.049 900 461 463  | 0.069 804 324 431  |
| H                                                                 | 0.116 306 474 127  | 0.047 684 593 817  | 0.319 372 465 490  |
| H                                                                 | -0.026 519 932 511 | -0.029 822 211 388 | -0.147 907 737 109 |
| H                                                                 | -0.016 042 766 662 | -0.034 908 201 852 | 0.038 651 485 520  |
| H                                                                 | -0.019 546 624 515 | -0.040 247 659 178 | -0.019 810 247 341 |
| H                                                                 | -0.011 627 063 160 | -0.064 244 017 529 | -0.239 049 838 806 |
| H                                                                 | -0.081 770 325 317 | -0.011 026 832 407 | 0.243 398 624 795  |
| H                                                                 | -0.023 788 950 197 | 0.041 314 891 723  | 0.006 438 938 763  |

Wavenumber/cm<sup>-1</sup>: 831.5055

| $\frac{\partial \mu_{x,y,z}}{\partial Q_r} / (e u^{-0.5})$        | 0.004 523 571 435  | -0.012 942 398 356 | 0.000 477 285 380  |
|-------------------------------------------------------------------|--------------------|--------------------|--------------------|
| <i>l</i> -matrix coefficients/(u <sup>1/2</sup> Å <sup>-1</sup> ) |                    |                    |                    |
| O                                                                 | -0.003 119 432 779 | -0.016 472 613 099 | 0.008 011 802 337  |
| C                                                                 | 0.021 831 947 247  | 0.010 379 862 565  | -0.007 415 341 469 |
| C                                                                 | -0.068 295 531 735 | 0.053 329 895 575  | -0.001 801 808 538 |
| C                                                                 | -0.016 929 196 992 | 0.001 851 449 093  | 0.010 841 244 245  |
| C                                                                 | 0.010 301 293 187  | -0.004 015 007 615 | 0.005 798 457 843  |
| C                                                                 | -0.034 536 571 711 | -0.009 475 584 727 | 0.100 298 282 702  |
| C                                                                 | 0.062 087 261 113  | 0.007 650 294 910  | 0.060 060 134 935  |
| C                                                                 | -0.028 010 024 931 | 0.134 560 845 819  | 0.055 644 457 421  |
| C                                                                 | -0.004 727 016 120 | 0.025 149 351 164  | -0.003 664 109 263 |
| C                                                                 | -0.068 231 163 184 | 0.085 571 975 349  | 0.055 745 571 487  |
| C                                                                 | 0.001 533 444 119  | -0.004 129 244 345 | 0.005 707 254 655  |
| H                                                                 | 0.175 696 890 907  | 0.138 351 968 740  | -0.142 752 139 049 |
| H                                                                 | -0.185 804 873 773 | -0.067 857 299 826 | -0.041 541 365 786 |
| H                                                                 | -0.015 479 916 723 | -0.005 430 893 633 | 0.012 231 109 734  |
| H                                                                 | 0.029 577 636 205  | -0.121 713 303 696 | 0.035 502 631 011  |
| H                                                                 | -0.015 225 383 644 | -0.100 907 123 185 | -0.240 085 164 018 |
| H                                                                 | -0.084 974 273 004 | -0.337 000 468 433 | 0.049 481 479 966  |
| H                                                                 | -0.107 526 726 467 | -0.379 584 354 130 | 0.011 146 977 791  |
| H                                                                 | -0.028 428 504 203 | 0.060 006 965 156  | -0.182 291 262 552 |
| H                                                                 | 0.188 642 453 399  | -0.167 594 993 461 | -0.240 935 874 064 |
| H                                                                 | 0.039 665 876 503  | 0.013 114 080 474  | 0.088 661 607 755  |
| H                                                                 | 0.315 159 672 502  | -0.202 638 809 154 | -0.273 225 350 311 |
| H                                                                 | 0.009 027 037 963  | 0.017 320 431 191  | -0.017 149 513 188 |
| H                                                                 | -0.003 863 344 776 | 0.012 672 950 463  | 0.010 315 652 808  |
| H                                                                 | 0.004 355 517 573  | -0.024 592 734 362 | -0.112 418 548 354 |
| H                                                                 | 0.117 533 828 570  | 0.207 365 645 820  | 0.055 622 137 736  |
| H                                                                 | 0.005 485 528 505  | -0.014 494 854 057 | -0.015 228 135 907 |

Wavenumber/cm<sup>-1</sup>: 838.9377

| $\frac{\partial \mu_{x,y,z}}{\partial Q_r} / (e u^{-0.5})$        |                    |                    |                    |
|-------------------------------------------------------------------|--------------------|--------------------|--------------------|
|                                                                   | -0.005 550 592 041 | 0.009 695 496 318  | -0.013 815 201 335 |
| <i>l</i> -matrix coefficients/(u <sup>1/2</sup> Å <sup>-1</sup> ) |                    |                    |                    |
| O                                                                 | 0.001 151 254 436  | 0.008 394 568 582  | -0.004 038 173 170 |
| C                                                                 | 0.000 801 994 124  | -0.014 239 116 698 | 0.004 233 262 613  |
| C                                                                 | 0.104 662 723 286  | 0.078 535 418 290  | -0.025 578 140 503 |
| C                                                                 | -0.050 659 041 327 | 0.000 909 547 308  | -0.002 755 401 693 |
| C                                                                 | -0.012 285 088 048 | -0.029 102 400 295 | 0.015 002 347 744  |
| C                                                                 | -0.023 165 016 873 | -0.002 284 762 818 | 0.067 647 438 263  |
| C                                                                 | -0.033 654 253 407 | -0.000 955 227 937 | -0.041 747 267 262 |
| C                                                                 | -0.012 245 771 241 | 0.014 427 647 287  | -0.009 121 834 734 |
| C                                                                 | 0.044 065 829 941  | 0.053 135 770 998  | 0.100 386 040 116  |
| C                                                                 | 0.021 768 830 591  | 0.041 359 420 015  | -0.099 283 294 885 |
| C                                                                 | -0.005 485 961 081 | -0.033 679 591 211 | -0.000 138 451 592 |
| H                                                                 | 0.102 575 319 255  | 0.087 512 643 953  | -0.085 690 559 831 |
| H                                                                 | 0.134 688 636 492  | 0.047 472 603 923  | 0.029 887 928 603  |
| H                                                                 | 0.017 660 013 033  | 0.006 784 602 493  | 0.005 095 925 216  |
| H                                                                 | 0.285 439 061 885  | -0.076 539 745 083 | -0.127 292 032 218 |
| H                                                                 | -0.009 881 139 178 | -0.068 306 936 854 | -0.154 680 251 486 |
| H                                                                 | -0.003 419 325 415 | -0.045 067 769 394 | 0.010 740 797 014  |
| H                                                                 | 0.271 848 241 487  | -0.142 087 073 338 | 0.175 146 888 744  |
| H                                                                 | 0.016 697 866 504  | -0.029 356 986 512 | 0.142 636 944 223  |
| H                                                                 | 0.029 572 091 497  | -0.017 533 056 488 | -0.011 601 907 402 |
| H                                                                 | -0.320 206 793 646 | 0.134 749 065 932  | -0.108 554 890 556 |
| H                                                                 | -0.239 749 211 507 | 0.064 391 144 472  | -0.116 139 866 197 |
| H                                                                 | -0.016 543 792 345 | 0.073 792 821 824  | -0.074 337 653 604 |
| H                                                                 | 0.049 651 537 817  | 0.099 362 385 090  | 0.050 386 911 408  |
| H                                                                 | -0.256 747 819 732 | -0.319 603 987 394 | -0.114 830 302 562 |
| H                                                                 | -0.222 642 654 436 | -0.168 974 222 894 | 0.337 975 532 549  |
| H                                                                 | 0.039 779 638 142  | -0.053 222 495 519 | 0.027 503 600 822  |

Wavenumber/cm<sup>-1</sup>: 846.6699

| $\frac{\partial \mu_{x,y,z}}{\partial Q_r} / (e u^{-0.5})$        | 0.034 460 039 293  | -0.019 231 346 717 | 0.001 653 410 372                    |
|-------------------------------------------------------------------|--------------------|--------------------|--------------------------------------|
| <i>l</i> -matrix coefficients/(u <sup>1/2</sup> Å <sup>-1</sup> ) |                    |                    |                                      |
| O                                                                 | -0.000 828 806 862 | 0.013 759 726 695  | -0.004 354 983 048                   |
| C                                                                 | 0.029 550 584 432  | -0.012 000 108 513 | 9.096 040 200 000 × 10 <sup>-5</sup> |
| C                                                                 | -0.057 322 564 972 | -0.004 740 324 697 | -0.008 955 424 107                   |
| C                                                                 | -0.061 151 576 345 | -0.050 932 420 654 | -0.017 219 890 090                   |
| C                                                                 | 0.013 012 015 363  | 0.036 618 174 889  | 0.005 291 174 468                    |
| C                                                                 | 0.054 410 548 514  | 0.006 162 256 758  | -0.095 907 603 672                   |
| C                                                                 | -0.110 675 459 089 | 0.010 429 900 960  | -0.116 781 781 060                   |
| C                                                                 | -0.016 749 230 431 | 0.039 980 477 160  | 0.008 865 436 176                    |
| C                                                                 | -0.013 363 495 145 | -0.031 098 628 705 | -0.016 472 423 147                   |
| C                                                                 | -0.040 943 959 319 | 0.045 464 676 950  | 0.003 927 196 454                    |
| C                                                                 | -0.036 642 981 842 | -0.071 054 891 960 | -0.011 350 621 689                   |
| H                                                                 | -0.142 559 777 357 | -0.148 341 016 946 | 0.140 881 998 858                    |
| H                                                                 | 0.407 913 623 874  | 0.131 273 407 089  | 0.084 584 363 370                    |
| H                                                                 | -0.024 650 746 536 | -0.022 418 728 102 | -0.009 167 976 249                   |
| H                                                                 | -0.092 975 937 761 | 0.077 353 539 856  | 0.021 782 510 904                    |
| H                                                                 | -0.013 443 404 462 | 0.121 621 646 739  | 0.213 407 054 563                    |
| H                                                                 | -0.031 140 700 829 | -0.139 196 124 001 | 0.018 285 583 933                    |
| H                                                                 | 0.002 183 332 742  | -0.198 545 285 410 | 0.038 840 326 554                    |
| H                                                                 | 0.057 169 877 447  | -0.097 853 961 152 | 0.415 481 185 325                    |
| H                                                                 | 0.071 429 747 140  | -0.068 944 370 894 | -0.104 027 624 409                   |
| H                                                                 | 0.094 745 221 045  | -0.053 905 172 341 | -0.006 822 742 009                   |
| H                                                                 | 0.162 056 792 843  | -0.097 549 327 014 | -0.122 788 135 920                   |
| H                                                                 | -0.065 453 667 596 | 0.188 920 510 828  | -0.182 373 669 888                   |
| H                                                                 | 0.148 963 664 590  | 0.268 933 163 678  | 0.126 343 211 073                    |
| H                                                                 | 0.097 163 675 403  | 0.118 882 452 657  | 0.050 138 769 020                    |
| H                                                                 | 0.048 014 373 023  | 0.112 020 304 766  | 0.084 155 557 862                    |
| H                                                                 | 0.111 933 945 746  | -0.139 469 554 868 | 0.106 492 448 466                    |

Wavenumber/cm<sup>-1</sup>: 893.6094

| $\frac{\partial \mu_{x,y,z}}{\partial Q_r} / (e u^{-0.5})$   |                    |                    |                    |
|--------------------------------------------------------------|--------------------|--------------------|--------------------|
|                                                              | -0.005 322 076 162 | 0.010 775 045 189  | 0.001 323 953 619  |
| $l$ -matrix coefficients/(u <sup>1/2</sup> Å <sup>-1</sup> ) |                    |                    |                    |
| O                                                            | -0.005 572 360 085 | -0.015 611 427 406 | 0.010 830 725 484  |
| C                                                            | -0.003 253 778 584 | 0.003 164 168 213  | -0.007 359 252 328 |
| C                                                            | -0.010 564 732 288 | 0.006 918 418 791  | -0.000 174 945 652 |
| C                                                            | 0.041 395 527 595  | 0.072 277 489 718  | -0.062 459 567 594 |
| C                                                            | 0.003 903 707 134  | 0.010 255 727 068  | -0.000 424 653 688 |
| C                                                            | 0.002 367 611 104  | -0.013 574 823 852 | -0.008 460 467 412 |
| C                                                            | -0.059 147 503 809 | -0.010 272 684 953 | -0.049 490 103 862 |
| C                                                            | -0.008 359 044 035 | -0.004 967 644 072 | -0.003 363 899 079 |
| C                                                            | 0.025 145 865 764  | -0.033 116 277 185 | 0.026 050 057 693  |
| C                                                            | -0.033 683 498 804 | 0.048 822 792 671  | -0.004 849 581 417 |
| C                                                            | 0.059 486 576 656  | 0.107 046 178 796  | -0.075 292 960 572 |
| H                                                            | -0.038 364 494 245 | -0.024 027 582 952 | 0.027 650 662 966  |
| H                                                            | 0.177 768 827 816  | 0.096 080 986 479  | 0.053 195 429 970  |
| H                                                            | -0.010 657 173 658 | -0.006 801 303 746 | 0.002 498 688 342  |
| H                                                            | 0.008 183 093 588  | 0.145 569 875 651  | -0.059 963 631 196 |
| H                                                            | 0.012 295 565 915  | 0.012 462 140 638  | 0.068 153 122 582  |
| H                                                            | -0.003 464 300 143 | -0.007 474 858 555 | -0.001 157 385 363 |
| H                                                            | 0.026 398 878 356  | -0.199 631 603 062 | 0.052 202 767 789  |
| H                                                            | 0.035 201 496 434  | -0.072 284 645 590 | 0.170 568 441 678  |
| H                                                            | 0.006 941 642 883  | -0.008 127 344 804 | -0.001 871 595 106 |
| H                                                            | -0.080 700 298 137 | -0.001 455 953 066 | -0.129 391 774 917 |
| H                                                            | 0.109 649 222 493  | -0.079 853 738 760 | -0.131 265 281 993 |
| H                                                            | -0.161 513 547 726 | -0.394 688 215 970 | 0.406 224 508 963  |
| H                                                            | 0.006 564 264 984  | -0.401 962 316 934 | -0.254 679 401 019 |
| H                                                            | -0.016 692 942 256 | -0.004 438 547 732 | 0.080 792 729 327  |
| H                                                            | 0.010 370 263 478  | 0.070 053 215 255  | 0.108 095 716 542  |
| H                                                            | -0.119 467 058 776 | 0.294 798 323 459  | 0.207 262 326 194  |

Wavenumber/cm<sup>-1</sup>: 897.8865

| $\frac{\partial \mu_{x,y,z}}{\partial Q_r} / (e u^{-0.5})$        | 0.013 576 541 166  | -0.002 306 040 288 | 0.004 233 400 468  |
|-------------------------------------------------------------------|--------------------|--------------------|--------------------|
| <i>l</i> -matrix coefficients/(u <sup>1/2</sup> Å <sup>-1</sup> ) |                    |                    |                    |
| O                                                                 | -0.002 306 091 204 | -0.003 815 600 903 | -0.001 255 042 488 |
| C                                                                 | 0.011 860 203 272  | -0.000 297 786 169 | 0.005 675 085 035  |
| C                                                                 | 0.002 985 023 538  | 0.016 047 780 569  | -0.019 235 162 626 |
| C                                                                 | -0.034 193 715 203 | 0.021 421 772 543  | -0.041 534 117 854 |
| C                                                                 | 0.003 059 437 207  | -0.003 345 386 435 | -0.007 772 760 289 |
| C                                                                 | -0.012 801 745 858 | -0.013 726 037 755 | 0.065 435 569 903  |
| C                                                                 | -0.041 392 484 900 | 0.002 107 810 890  | -0.040 936 821 995 |
| C                                                                 | -0.034 021 726 203 | 0.111 277 350 900  | 0.038 020 159 248  |
| C                                                                 | -0.067 157 484 990 | 0.062 906 445 951  | -0.067 535 532 796 |
| C                                                                 | 0.068 211 061 856  | -0.069 524 583 035 | -0.022 402 130 608 |
| C                                                                 | 0.017 542 201 117  | 0.014 197 498 642  | -0.046 854 594 920 |
| H                                                                 | 0.070 516 955 195  | 0.077 964 821 769  | -0.069 201 824 057 |
| H                                                                 | 0.166 072 941 374  | 0.072 758 278 358  | 0.045 365 658 862  |
| H                                                                 | -0.007 150 907 561 | 0.003 970 811 865  | 0.011 641 037 452  |
| H                                                                 | -0.049 563 087 840 | -0.326 738 299 316 | 0.153 851 840 428  |
| H                                                                 | -0.012 478 753 033 | -0.048 323 495 542 | -0.118 901 573 680 |
| H                                                                 | -0.064 822 855 662 | -0.289 529 269 277 | 0.049 467 260 476  |
| H                                                                 | 0.034 580 278 285  | 0.280 781 849 950  | -0.036 191 482 842 |
| H                                                                 | 0.026 492 276 499  | -0.043 287 347 649 | 0.169 506 914 998  |
| H                                                                 | 0.171 812 670 596  | -0.148 126 810 303 | -0.207 602 813 412 |
| H                                                                 | 0.231 074 626 265  | -0.014 273 283 014 | 0.323 942 085 038  |
| H                                                                 | -0.240 931 679 703 | 0.146 392 490 303  | 0.186 102 155 255  |
| H                                                                 | -0.131 641 169 612 | -0.102 131 481 059 | 0.115 198 124 127  |
| H                                                                 | 0.095 893 263 469  | -0.062 564 313 720 | -0.064 863 578 583 |
| H                                                                 | 0.083 674 624 774  | 0.055 128 742 411  | -0.193 293 503 020 |
| H                                                                 | -0.073 177 219 656 | -0.150 774 442 386 | -0.065 676 272 580 |
| H                                                                 | 0.005 392 783 748  | 0.077 000 062 123  | 0.179 061 998 924  |

Wavenumber/cm<sup>-1</sup>: 937.745

| $\frac{\partial \mu_{x,y,z}}{\partial Q_r} / (e u^{-0.5})$        | 0.000 915 007 469  | 0.010 004 798 181  | 0.008 309 367 393  |
|-------------------------------------------------------------------|--------------------|--------------------|--------------------|
| <i>l</i> -matrix coefficients/(u <sup>1/2</sup> Å <sup>-1</sup> ) |                    |                    |                    |
| O                                                                 | 0.001 204 398 800  | 0.007 420 182 731  | -0.004 898 840 965 |
| C                                                                 | 0.000 230 297 195  | -0.007 429 217 724 | 0.013 179 863 194  |
| C                                                                 | 0.006 119 755 741  | -0.007 634 500 036 | 0.005 226 334 724  |
| C                                                                 | -0.032 457 457 870 | -0.019 351 572 734 | -0.074 795 019 148 |
| C                                                                 | 0.005 062 699 349  | -0.003 404 678 070 | -0.005 283 830 855 |
| C                                                                 | -0.006 023 114 507 | 0.003 711 669 632  | 0.020 406 714 771  |
| C                                                                 | 0.069 268 633 867  | 0.003 885 683 025  | 0.067 274 880 986  |
| C                                                                 | 0.003 798 246 034  | -0.040 924 280 162 | -0.017 146 989 481 |
| C                                                                 | 0.014 001 288 781  | 0.003 295 395 004  | 0.018 523 080 771  |
| C                                                                 | -0.012 145 396 858 | -0.011 500 409 787 | 0.018 971 065 394  |
| C                                                                 | -0.023 441 609 200 | -0.073 040 601 692 | -0.142 808 174 069 |
| H                                                                 | 0.022 733 610 416  | -0.005 347 581 198 | 0.001 456 080 724  |
| H                                                                 | -0.189 547 478 326 | -0.058 477 878 217 | -0.036 544 001 054 |
| H                                                                 | -0.000 820 052 603 | 0.003 207 983 657  | 0.005 193 476 316  |
| H                                                                 | 0.039 513 970 841  | 0.020 191 490 967  | -0.028 435 663 556 |
| H                                                                 | -0.005 465 405 532 | -0.006 086 339 931 | -0.016 883 611 217 |
| H                                                                 | 0.033 475 071 206  | 0.108 603 264 820  | -0.009 544 843 115 |
| H                                                                 | -0.049 796 005 220 | 0.036 976 949 543  | -0.032 755 420 991 |
| H                                                                 | -0.024 131 009 487 | 0.059 034 087 519  | -0.181 194 480 822 |
| H                                                                 | -0.054 555 410 456 | 0.053 230 128 968  | 0.082 790 367 496  |
| H                                                                 | -0.060 879 876 438 | 0.016 442 914 777  | -0.048 805 841 014 |
| H                                                                 | 0.048 009 033 680  | -0.014 071 002 324 | 0.027 388 470 631  |
| H                                                                 | -0.426 457 584 659 | 0.016 973 174 753  | 0.021 698 030 270  |
| H                                                                 | 0.429 596 971 281  | 0.251 075 477 783  | 0.032 985 303 838  |
| H                                                                 | -0.041 956 387 352 | -0.046 760 102 007 | 0.004 096 467 546  |
| H                                                                 | 0.044 294 518 875  | 0.033 694 397 579  | -0.073 610 128 457 |
| H                                                                 | 0.146 913 199 580  | 0.027 806 605 508  | 0.604 633 966 490  |

Wavenumber/cm<sup>-1</sup>: 953.4586

| $\frac{\partial \mu_{x,y,z}}{\partial Q_r} / (e u^{-0.5})$        |                    |                                    |                    |
|-------------------------------------------------------------------|--------------------|------------------------------------|--------------------|
|                                                                   | -0.013 867 906 732 | 0.002 614 500 837                  | -0.003 468 563 202 |
| <i>l</i> -matrix coefficients/(u <sup>1/2</sup> Å <sup>-1</sup> ) |                    |                                    |                    |
| O                                                                 | 0.000 585 067 303  | -0.002 985 366 399                 | 0.002 287 031 589  |
| C                                                                 | -0.005 631 768 689 | 0.002 956 841 055                  | -0.001 792 795 566 |
| C                                                                 | 0.011 535 703 621  | 0.006 619 728 233                  | 0.043 172 973 371  |
| C                                                                 | 0.008 690 677 226  | 0.002 263 176 200                  | 0.002 931 133 585  |
| C                                                                 | -0.004 017 094 013 | 0.008 901 851 576                  | -0.011 454 836 222 |
| C                                                                 | 0.023 784 659 077  | 0.002 997 423 649                  | -0.055 660 572 845 |
| C                                                                 | -0.042 284 262 268 | 0.001 349 215 650                  | -0.037 290 761 010 |
| C                                                                 | -0.001 961 020 312 | -0.003 740 291 691                 | 0.001 398 499 723  |
| C                                                                 | 0.056 330 407 424  | 0.110 296 017 274                  | 0.056 842 431 665  |
| C                                                                 | -0.056 796 756 705 | -0.062 556 030 909                 | 0.091 440 890 413  |
| C                                                                 | 0.003 151 559 234  | 0.008 673 959 458                  | 0.008 999 879 061  |
| H                                                                 | -0.086 525 548 503 | -0.070 568 692 381                 | 0.071 125 049 495  |
| H                                                                 | 0.129 044 517 442  | 0.043 331 062 041                  | 0.028 360 128 991  |
| H                                                                 | 0.000 527 788 497  | $2.174 987 400 000 \times 10^{-5}$ | -0.011 321 106 949 |
| H                                                                 | 0.275 648 644 391  | -0.260 636 573 592                 | -0.043 228 439 608 |
| H                                                                 | 0.006 927 498 976  | 0.056 395 020 400                  | 0.125 112 853 212  |
| H                                                                 | 0.004 610 721 930  | -0.012 620 468 085                 | 0.005 448 126 594  |
| H                                                                 | -0.248 936 242 136 | 0.170 877 651 074                  | -0.162 325 097 585 |
| H                                                                 | 0.020 245 433 158  | -0.040 048 564 035                 | 0.126 547 657 581  |
| H                                                                 | -0.002 407 272 547 | -0.006 498 093 631                 | -0.014 794 641 455 |
| H                                                                 | -0.247 772 556 350 | 0.152 068 186 573                  | 0.022 067 986 057  |
| H                                                                 | 0.237 706 390 946  | -0.069 528 301 477                 | 0.120 413 554 573  |
| H                                                                 | 0.031 727 386 384  | -0.012 414 403 250                 | 0.007 375 144 599  |
| H                                                                 | -0.037 649 524 255 | -0.030 870 342 566                 | -0.007 165 362 338 |
| H                                                                 | -0.267 462 359 958 | -0.356 913 173 211                 | -0.216 306 526 418 |
| H                                                                 | 0.223 571 058 851  | 0.174 244 046 187                  | -0.354 717 039 114 |
| H                                                                 | -0.016 739 888 105 | 0.006 622 206 993                  | -0.046 023 985 148 |



Wavenumber/cm<sup>-1</sup>: 964.0326

| $\frac{\partial \mu_{x,y,z}}{\partial Q_r} / (e u^{-0.5})$        | 0.013 918 472 828  | 0.002 092 110 358  | 0.001 345 188 256  |
|-------------------------------------------------------------------|--------------------|--------------------|--------------------|
| <i>l</i> -matrix coefficients/(u <sup>1/2</sup> Å <sup>-1</sup> ) |                    |                    |                    |
| O                                                                 | 0.012 925 479 826  | 0.022 109 448 935  | -0.009 514 124 980 |
| C                                                                 | -0.084 455 959 527 | -0.015 455 948 838 | 0.007 300 897 854  |
| C                                                                 | 0.087 892 693 117  | 0.007 684 947 748  | 0.014 532 540 772  |
| C                                                                 | 0.049 033 101 240  | -0.017 099 793 111 | -0.000 706 906 833 |
| C                                                                 | -0.066 740 317 201 | -0.060 888 833 372 | 0.014 426 456 677  |
| C                                                                 | -0.013 150 163 399 | 0.034 444 321 450  | -0.026 941 740 810 |
| C                                                                 | -0.012 039 211 201 | 0.021 127 722 275  | 0.001 188 551 815  |
| C                                                                 | -0.013 004 420 570 | 0.032 154 528 140  | -0.013 277 648 678 |
| C                                                                 | 0.187 910 889 378  | -0.043 496 748 504 | -0.229 986 752 344 |
| C                                                                 | 0.144 643 964 493  | 0.112 522 780 636  | 0.180 410 699 434  |
| C                                                                 | 0.040 050 528 409  | -0.027 934 231 568 | -0.006 954 597 955 |
| H                                                                 | -0.003 496 044 930 | -0.030 150 892 783 | 0.021 481 494 173  |
| H                                                                 | 0.024 917 318 657  | -0.011 490 871 828 | -0.000 841 295 570 |
| H                                                                 | 0.084 460 916 251  | 0.063 223 270 251  | -0.010 776 133 742 |
| H                                                                 | -0.288 248 051 353 | 0.004 383 558 675  | 0.155 201 080 041  |
| H                                                                 | 0.047 194 765 442  | -0.022 590 023 433 | 0.030 387 859 971  |
| H                                                                 | -0.003 700 601 491 | -0.035 794 114 400 | 0.008 711 993 932  |
| H                                                                 | -0.251 439 976 810 | -0.128 746 796 912 | -0.116 897 068 803 |
| H                                                                 | 0.013 635 476 594  | -0.026 020 824 534 | 0.009 178 489 589  |
| H                                                                 | 0.061 059 331 984  | -0.014 613 623 212 | 0.016 288 849 849  |
| H                                                                 | -0.229 082 509 336 | 0.212 358 579 068  | 0.258 493 901 503  |
| H                                                                 | -0.182 527 904 937 | -0.013 319 498 278 | -0.302 604 972 586 |
| H                                                                 | -0.071 126 285 326 | 0.027 914 557 904  | -0.016 712 516 243 |
| H                                                                 | -0.052 039 163 758 | 0.036 056 449 403  | 0.035 325 497 450  |
| H                                                                 | -0.160 311 198 034 | -0.099 631 303 918 | 0.353 229 810 804  |
| H                                                                 | -0.112 226 698 891 | -0.257 945 336 481 | -0.201 817 821 855 |
| H                                                                 | -0.033 686 772 774 | 0.059 643 056 491  | 0.006 404 113 637  |

Wavenumber/cm<sup>-1</sup>: 969.6762

| $\frac{\partial \mu_{x,y,z}}{\partial Q_r} / (e u^{-0.5})$        | 0.008 568 162 828  | -0.003 932 696 823 | -0.002 333 209 795 |
|-------------------------------------------------------------------|--------------------|--------------------|--------------------|
| <i>l</i> -matrix coefficients/(u <sup>1/2</sup> Å <sup>-1</sup> ) |                    |                    |                    |
| O                                                                 | 0.007 391 640 467  | 0.022 235 475 995  | -0.011 666 014 889 |
| C                                                                 | -0.019 845 994 998 | -0.012 898 421 374 | 0.014 742 885 535  |
| C                                                                 | 0.001 101 038 145  | -0.007 060 678 791 | -0.002 254 256 213 |
| C                                                                 | 0.095 686 461 275  | -0.063 725 347 592 | -0.014 819 935 745 |
| C                                                                 | -0.009 181 083 604 | 0.003 964 304 311  | -0.012 857 794 678 |
| C                                                                 | -0.006 327 225 622 | 0.005 100 338 239  | 0.002 370 501 733  |
| C                                                                 | -0.005 639 172 330 | -0.001 730 092 083 | -0.000 820 464 788 |
| C                                                                 | 0.005 437 337 460  | 0.008 300 836 246  | 0.010 986 767 280  |
| C                                                                 | 0.024 924 217 849  | -0.000 699 260 575 | -0.025 184 148 935 |
| C                                                                 | 0.023 252 633 544  | 0.020 203 955 917  | 0.025 595 950 038  |
| C                                                                 | -0.387 003 241 037 | 0.248 292 919 886  | 0.036 440 844 853  |
| H                                                                 | -0.006 317 676 260 | -0.001 633 389 843 | 0.007 202 875 237  |
| H                                                                 | -0.011 211 662 767 | 0.010 837 627 907  | 0.000 777 063 498  |
| H                                                                 | -0.007 669 774 106 | 0.006 762 803 297  | 0.008 595 921 315  |
| H                                                                 | -0.032 726 837 753 | -0.007 536 959 975 | 0.020 715 460 437  |
| H                                                                 | -0.000 758 474 241 | 0.002 001 294 167  | 0.007 847 152 457  |
| H                                                                 | -0.009 454 592 665 | 0.000 876 834 094  | -0.005 261 232 199 |
| H                                                                 | -0.033 437 658 797 | -0.022 630 071 492 | -0.014 456 597 061 |
| H                                                                 | -0.003 651 312 295 | -0.002 129 861 708 | -0.010 633 880 948 |
| H                                                                 | -0.003 384 426 117 | 0.002 045 278 560  | -0.004 358 208 276 |
| H                                                                 | -0.031 031 841 977 | 0.028 029 952 308  | 0.030 822 806 820  |
| H                                                                 | -0.028 284 934 802 | -0.000 328 472 109 | -0.044 346 973 818 |
| H                                                                 | 0.434 774 722 029  | -0.137 510 068 557 | 0.098 073 389 073  |
| H                                                                 | 0.440 796 142 308  | -0.162 420 895 673 | -0.230 972 893 156 |
| H                                                                 | -0.024 990 868 050 | -0.019 555 839 439 | 0.036 895 550 860  |
| H                                                                 | -0.020 339 575 588 | -0.040 276 407 039 | -0.023 719 641 712 |
| H                                                                 | 0.266 492 861 949  | -0.434 648 103 904 | 0.051 238 562 317  |

Wavenumber/cm<sup>-1</sup>: 1007.8916

| $\frac{\partial \mu_{x,y,z}}{\partial Q_r} / (e u^{-0.5})$        | -0.008 131 112 313 | -0.026 957 136 605 | 0.011 894 311 273  |
|-------------------------------------------------------------------|--------------------|--------------------|--------------------|
| <i>l</i> -matrix coefficients/(u <sup>1/2</sup> Å <sup>-1</sup> ) |                    |                    |                    |
| O                                                                 | 0.004 986 081 507  | 0.000 242 869 154  | -0.004 688 351 083 |
| C                                                                 | -0.028 243 562 562 | 0.006 142 374 487  | 0.009 205 706 165  |
| C                                                                 | 0.032 745 901 009  | -0.010 362 297 149 | -0.018 138 350 827 |
| C                                                                 | 0.037 688 581 465  | -0.020 968 967 000 | -0.004 166 939 886 |
| C                                                                 | -0.019 881 795 745 | 0.000 456 778 799  | 0.023 779 381 579  |
| C                                                                 | -0.011 982 143 734 | 0.015 145 916 551  | -0.025 068 589 909 |
| C                                                                 | -0.014 408 359 651 | 0.015 390 106 073  | -0.003 434 066 437 |
| C                                                                 | 0.005 493 475 226  | -0.012 457 258 123 | -0.010 201 267 437 |
| C                                                                 | -0.190 509 061 439 | 0.040 131 468 764  | 0.210 198 617 101  |
| C                                                                 | 0.176 446 350 938  | 0.125 463 178 106  | 0.211 352 548 608  |
| C                                                                 | -0.003 120 394 573 | 0.002 502 417 137  | -0.002 356 029 705 |
| H                                                                 | 0.006 498 946 340  | -0.038 587 885 784 | 0.023 430 492 020  |
| H                                                                 | 0.016 799 436 202  | -0.004 035 699 513 | -0.000 237 881 506 |
| H                                                                 | 0.024 320 811 905  | 0.005 678 907 141  | -0.016 046 877 859 |
| H                                                                 | 0.281 212 283 907  | -0.003 900 617 420 | -0.159 716 485 219 |
| H                                                                 | 0.015 954 573 841  | 0.005 804 058 631  | 0.042 192 393 208  |
| H                                                                 | -0.005 917 118 870 | 0.023 719 804 281  | -0.014 163 103 389 |
| H                                                                 | -0.293 370 605 701 | -0.142 507 881 346 | -0.140 110 581 370 |
| H                                                                 | 0.011 680 258 209  | -0.027 965 045 574 | 0.007 960 327 441  |
| H                                                                 | -0.010 443 518 526 | 0.015 853 253 050  | 0.033 371 980 463  |
| H                                                                 | 0.210 672 606 148  | -0.192 537 476 691 | -0.234 166 974 274 |
| H                                                                 | -0.211 678 346 137 | -0.013 335 190 027 | -0.338 073 379 366 |
| H                                                                 | -0.011 343 341 433 | -0.000 514 844 075 | 0.000 971 652 026  |
| H                                                                 | -0.008 782 932 439 | 0.003 988 901 069  | 0.003 382 379 064  |
| H                                                                 | 0.145 061 276 521  | 0.092 613 891 023  | -0.311 096 582 081 |
| H                                                                 | -0.128 763 858 667 | -0.294 356 265 483 | -0.233 354 379 292 |
| H                                                                 | -0.007 324 183 046 | 0.011 813 712 263  | 0.004 020 597 291  |

Wavenumber/cm<sup>-1</sup>: 1017.7558

| $\frac{\partial \mu_{x,y,z}}{\partial Q_r} / (e u^{-0.5})$        | $1.090\,013\,505\,311 \times 10^{-5}$ | $0.008\,023\,435\,324$ | $0.002\,843\,211\,586$ |
|-------------------------------------------------------------------|---------------------------------------|------------------------|------------------------|
| <i>l</i> -matrix coefficients/(u <sup>1/2</sup> Å <sup>-1</sup> ) |                                       |                        |                        |
| O                                                                 | 0.048 896 054 942                     | -0.021 245 194 720     | 0.005 454 450 525      |
| C                                                                 | -0.258 512 413 074                    | 0.041 849 935 265      | 0.008 311 176 451      |
| C                                                                 | 0.115 954 962 930                     | -0.020 541 362 658     | -0.021 427 810 580     |
| C                                                                 | 0.521 962 219 788                     | -0.172 038 138 761     | -0.001 551 240 169     |
| C                                                                 | -0.076 092 805 050                    | -0.018 629 516 470     | 0.101 928 088 405      |
| C                                                                 | -0.211 357 081 944                    | 0.142 579 137 022      | -0.062 984 670 907     |
| C                                                                 | -0.153 072 106 584                    | 0.231 366 747 237      | 0.062 249 825 935      |
| C                                                                 | -0.060 476 886 496                    | -0.025 302 702 919     | -0.076 172 923 709     |
| C                                                                 | -0.042 249 254 269                    | 0.006 936 290 293      | 0.015 137 641 883      |
| C                                                                 | -0.069 626 217 878                    | -0.022 160 201 842     | -0.037 732 005 975     |
| C                                                                 | -0.127 213 780 512                    | 0.028 303 332 226      | -0.004 434 470 252     |
| H                                                                 | 0.170 474 739 344                     | -0.081 918 429 604     | -0.003 070 503 852     |
| H                                                                 | 0.117 280 978 271                     | -0.174 926 582 846     | -0.051 918 457 711     |
| H                                                                 | 0.138 731 481 409                     | 0.020 654 842 330      | -0.108 660 035 899     |
| H                                                                 | 0.024 106 602 116                     | -0.014 528 527 440     | -0.010 694 258 816     |
| H                                                                 | 0.200 029 286 876                     | -0.184 524 011 066     | 0.028 218 435 696      |
| H                                                                 | 0.036 268 555 834                     | -0.024 519 924 069     | 0.025 193 026 657      |
| H                                                                 | 0.078 408 289 986                     | 0.025 390 969 128      | 0.048 051 628 525      |
| H                                                                 | 0.142 723 856 734                     | -0.351 158 799 248     | -0.097 448 410 536     |
| H                                                                 | 0.098 805 257 364                     | -0.025 899 267 201     | 0.081 946 841 183      |
| H                                                                 | 0.042 028 897 922                     | -0.022 335 273 717     | 0.007 215 268 651      |
| H                                                                 | 0.071 810 980 380                     | -0.011 859 738 467     | 0.061 881 099 883      |
| H                                                                 | -0.028 415 276 446                    | 0.033 982 853 599      | -0.021 581 763 609     |
| H                                                                 | -0.020 110 073 543                    | 0.071 700 542 177      | 0.032 858 873 899      |
| H                                                                 | 0.017 297 826 668                     | 0.024 257 446 444      | -0.013 148 496 819     |
| H                                                                 | 0.028 004 417 578                     | 0.064 560 771 175      | 0.027 923 590 137      |
| H                                                                 | -0.067 179 222 625                    | 0.071 730 323 171      | 0.029 068 785 985      |

Wavenumber/cm<sup>-1</sup>: 1033.1774

| $\frac{\partial \mu_{x,y,z}}{\partial Q_r} / (e u^{-0.5})$        | 0.002 785 568 798  | 0.007 772 881 762  | -0.006 385 100 002 |
|-------------------------------------------------------------------|--------------------|--------------------|--------------------|
| <i>l</i> -matrix coefficients/(u <sup>1/2</sup> Å <sup>-1</sup> ) |                    |                    |                    |
| O                                                                 | -0.012 799 451 899 | 0.010 360 725 147  | -0.006 860 090 236 |
| C                                                                 | 0.058 820 963 093  | 0.004 473 651 307  | 0.008 719 262 270  |
| C                                                                 | -0.248 561 795 755 | -0.065 282 347 257 | -0.020 802 063 770 |
| C                                                                 | 0.108 470 495 769  | -0.097 011 446 798 | 0.055 162 794 132  |
| C                                                                 | 0.211 073 858 623  | 0.377 784 276 855  | 0.050 848 787 813  |
| C                                                                 | -0.050 611 541 706 | -0.025 889 736 676 | -0.021 507 490 952 |
| C                                                                 | -0.097 015 157 892 | 0.095 381 907 515  | 0.023 366 111 234  |
| C                                                                 | 0.147 859 815 960  | -0.153 003 392 057 | 0.119 148 279 874  |
| C                                                                 | 0.093 765 009 323  | 0.023 057 809 962  | -0.017 339 434 903 |
| C                                                                 | 0.090 515 557 582  | 0.011 860 010 919  | 0.020 061 008 311  |
| C                                                                 | -0.025 718 004 979 | 0.010 122 844 602  | -0.028 285 067 185 |
| H                                                                 | 0.134 409 440 313  | -0.047 626 949 921 | -0.021 519 022 107 |
| H                                                                 | 0.058 168 710 585  | -0.155 291 495 220 | -0.053 456 311 728 |
| H                                                                 | -0.309 579 019 113 | -0.422 391 185 495 | -0.176 074 361 320 |
| H                                                                 | -0.058 562 619 341 | -0.014 753 432 439 | 0.056 939 969 841  |
| H                                                                 | -0.094 805 695 575 | 0.075 001 150 937  | -0.012 200 857 170 |
| H                                                                 | -0.066 710 250 257 | 0.013 906 365 309  | -0.075 537 424 712 |
| H                                                                 | -0.051 081 746 221 | -0.019 962 710 052 | -0.037 592 382 100 |
| H                                                                 | 0.019 117 876 849  | -0.090 409 578 472 | -0.053 766 327 389 |
| H                                                                 | -0.306 729 082 165 | -0.005 356 910 322 | -0.297 939 592 672 |
| H                                                                 | -0.045 997 833 870 | 0.032 494 207 963  | -0.022 574 309 296 |
| H                                                                 | -0.079 466 537 523 | 0.033 381 488 986  | -0.010 982 853 889 |
| H                                                                 | -0.015 036 486 506 | -0.011 858 492 409 | 0.010 882 097 495  |
| H                                                                 | -0.036 690 747 603 | 0.024 815 891 970  | 0.012 829 631 827  |
| H                                                                 | -0.042 788 144 898 | -0.063 598 109 367 | -0.005 383 655 655 |
| H                                                                 | -0.028 885 167 938 | -0.048 149 872 725 | 0.038 237 336 579  |
| H                                                                 | -0.020 607 831 036 | 0.032 009 152 126  | 0.021 759 875 777  |

Wavenumber/cm<sup>-1</sup>: 1041.229

| $\frac{\partial \mu_{x,y,z}}{\partial Q_r} / (e u^{-0.5})$        |                    |                         |                        |
|-------------------------------------------------------------------|--------------------|-------------------------|------------------------|
| $9.612\,752\,766\,425 \times 10^{-5}$                             |                    | $-0.004\,225\,446\,090$ | $0.001\,856\,995\,208$ |
| <i>l</i> -matrix coefficients/(u <sup>1/2</sup> Å <sup>-1</sup> ) |                    |                         |                        |
| O                                                                 | -0.020 622 415 998 | 0.000 878 832 889       | -0.004 283 210 572     |
| C                                                                 | 0.119 134 558 499  | -0.003 771 508 861      | 0.011 927 841 948      |
| C                                                                 | -0.242 742 785 269 | 0.061 530 487 258       | -0.052 539 366 368     |
| C                                                                 | -0.085 594 837 519 | -0.050 233 684 107      | -0.079 252 038 542     |
| C                                                                 | 0.332 466 579 099  | -0.005 416 204 230      | -0.049 456 952 758     |
| C                                                                 | -0.068 277 412 499 | 0.009 779 016 211       | 0.041 688 577 284      |
| C                                                                 | 0.024 182 821 657  | 0.119 869 505 816       | 0.108 908 723 930      |
| C                                                                 | -0.327 627 506 764 | 0.023 016 474 357       | -0.259 651 840 299     |
| C                                                                 | 0.067 466 987 694  | -0.033 311 936 813      | 0.025 761 962 632      |
| C                                                                 | 0.076 073 796 781  | -0.031 424 572 661      | 0.025 615 499 570      |
| C                                                                 | 0.017 788 386 090  | 0.013 552 227 860       | 0.041 939 375 225      |
| H                                                                 | 0.098 734 509 429  | -0.095 378 669 947      | 0.053 110 643 499      |
| H                                                                 | 0.046 584 994 797  | -0.139 702 245 837      | -0.030 184 404 762     |
| H                                                                 | -0.198 946 969 860 | -0.063 243 045 260      | 0.232 992 374 726      |
| H                                                                 | -0.036 951 304 759 | 0.043 162 477 982       | 0.017 665 403 053      |
| H                                                                 | -0.074 467 530 508 | 0.059 895 111 583       | 0.028 918 971 764      |
| H                                                                 | 0.399 682 863 581  | -0.036 658 634 248      | 0.336 330 579 660      |
| H                                                                 | -0.051 043 280 658 | 0.021 141 319 907       | -0.042 246 523 318     |
| H                                                                 | 0.047 150 643 352  | -0.063 212 676 290      | -0.023 108 867 347     |
| H                                                                 | 0.251 448 243 062  | -0.051 066 681 498      | 0.196 987 874 753      |
| H                                                                 | -0.058 349 183 396 | 0.015 648 958 258       | -0.036 096 031 982     |
| H                                                                 | -0.071 989 439 833 | 0.020 333 248 599       | -0.009 191 281 391     |
| H                                                                 | -0.009 757 550 695 | 0.013 331 074 173       | 0.000 619 754 993      |
| H                                                                 | 0.005 939 071 594  | -0.045 346 835 717      | -0.018 540 518 894     |
| H                                                                 | 0.013 639 778 804  | -0.026 775 468 283      | -0.045 799 500 704     |
| H                                                                 | 0.016 975 798 386  | 0.003 389 102 254       | 0.035 646 864 821      |
| H                                                                 | 0.004 279 852 433  | -0.016 608 492 808      | -0.041 223 094 867     |

Wavenumber/cm<sup>-1</sup>: 1091.6058

| $\frac{\partial \mu_{x,y,z}}{\partial Q_r} / (e u^{-0.5})$        | 0.001 992 522 775  | 0.003 168 863 991  | -0.007 957 227 088 |
|-------------------------------------------------------------------|--------------------|--------------------|--------------------|
| <i>l</i> -matrix coefficients/(u <sup>1/2</sup> Å <sup>-1</sup> ) |                    |                    |                    |
| O                                                                 | -0.002 797 634 850 | 0.031 404 114 961  | -0.013 162 679 243 |
| C                                                                 | 0.105 378 803 260  | 0.010 159 638 627  | -0.005 655 745 748 |
| C                                                                 | 0.113 008 260 703  | -0.031 061 594 875 | -0.083 010 941 001 |
| C                                                                 | -0.382 771 402 916 | -0.240 717 894 128 | 0.179 563 326 189  |
| C                                                                 | -0.121 631 668 174 | 0.036 097 178 881  | 0.298 822 552 119  |
| C                                                                 | 0.048 353 507 417  | 0.140 435 180 452  | -0.144 021 539 054 |
| C                                                                 | 0.042 990 124 129  | 0.152 022 417 778  | 0.009 632 628 716  |
| C                                                                 | 0.025 521 977 010  | -0.026 773 821 986 | -0.144 611 961 773 |
| C                                                                 | -0.041 122 456 647 | 0.024 414 340 441  | 0.009 702 323 311  |
| C                                                                 | -0.049 557 531 383 | -0.012 035 522 251 | 0.019 408 088 601  |
| C                                                                 | 0.106 828 065 180  | 0.096 851 963 435  | -0.070 385 163 381 |
| H                                                                 | 0.157 099 968 730  | -0.176 433 593 031 | 0.071 586 282 227  |
| H                                                                 | 0.084 745 073 366  | -0.353 099 809 067 | -0.139 648 476 162 |
| H                                                                 | 0.238 404 382 136  | -0.072 061 908 563 | -0.286 912 483 512 |
| H                                                                 | 0.006 378 254 037  | -0.007 527 782 719 | -0.000 998 998 278 |
| H                                                                 | -0.053 710 827 238 | 0.070 753 721 139  | -0.116 233 676 871 |
| H                                                                 | 0.010 438 614 633  | -0.074 369 184 201 | -0.020 544 095 506 |
| H                                                                 | 0.041 445 007 060  | 0.030 855 651 597  | 0.034 109 292 845  |
| H                                                                 | -0.046 199 996 531 | 0.172 914 104 617  | 0.097 390 947 469  |
| H                                                                 | 0.065 369 325 635  | 0.014 431 964 371  | 0.095 146 198 595  |
| H                                                                 | 0.018 263 748 015  | -0.004 528 250 940 | 0.011 032 634 317  |
| H                                                                 | 0.017 277 914 077  | -0.018 152 504 113 | -0.008 766 003 592 |
| H                                                                 | -0.032 882 862 505 | -0.085 134 320 730 | 0.093 451 714 484  |
| H                                                                 | -0.088 042 848 480 | -0.058 026 273 369 | -0.036 006 559 683 |
| H                                                                 | -0.014 619 452 300 | 0.011 541 365 691  | 0.032 870 814 365  |
| H                                                                 | 0.010 656 149 916  | 0.015 210 336 520  | -0.028 998 280 049 |
| H                                                                 | 0.124 684 772 913  | -0.107 188 088 572 | 0.015 243 925 898  |

Wavenumber/cm<sup>-1</sup>: 1126.6285

| $\frac{\partial \mu_{x,y,z}}{\partial Q_r} / (e u^{-0.5})$        |                    |                    |                    |
|-------------------------------------------------------------------|--------------------|--------------------|--------------------|
|                                                                   | -0.000 346 264 068 | -0.012 140 626 457 | 0.017 079 533 029  |
| <i>l</i> -matrix coefficients/(u <sup>1/2</sup> Å <sup>-1</sup> ) |                    |                    |                    |
| O                                                                 | 0.010 033 055 465  | 0.035 547 749 654  | -0.013 869 210 618 |
| C                                                                 | -0.046 209 915 516 | 0.010 175 895 021  | -0.021 577 821 105 |
| C                                                                 | 0.054 510 925 881  | -0.162 999 802 902 | 0.202 391 084 317  |
| C                                                                 | 0.073 380 849 868  | -0.168 576 078 341 | 0.172 856 182 905  |
| C                                                                 | -0.060 376 199 459 | -0.008 878 561 499 | -0.283 682 901 922 |
| C                                                                 | 0.186 972 111 067  | -0.112 144 941 602 | 0.089 180 869 477  |
| C                                                                 | -0.129 478 819 841 | 0.133 542 646 817  | 0.058 086 764 561  |
| C                                                                 | 0.061 442 573 563  | 0.053 648 706 760  | -0.020 705 382 660 |
| C                                                                 | -0.018 609 915 959 | 0.053 681 140 100  | -0.051 170 681 419 |
| C                                                                 | -0.014 197 428 117 | 0.082 377 714 464  | -0.063 319 799 110 |
| C                                                                 | -0.019 913 698 418 | 0.055 872 452 830  | -0.083 252 881 542 |
| H                                                                 | -0.219 236 399 762 | 0.175 711 398 730  | -0.047 194 303 353 |
| H                                                                 | 0.189 420 906 745  | -0.385 354 256 867 | -0.116 018 346 315 |
| H                                                                 | -0.002 837 077 358 | 0.307 809 267 834  | 0.233 126 170 989  |
| H                                                                 | 0.035 027 452 893  | -0.052 987 058 490 | -0.011 478 563 458 |
| H                                                                 | -0.223 349 760 346 | 0.177 364 938 373  | -0.110 657 914 018 |
| H                                                                 | 0.120 895 275 332  | -0.033 024 342 097 | 0.094 484 030 917  |
| H                                                                 | -0.002 449 600 862 | -0.080 704 354 933 | 0.000 464 225 268  |
| H                                                                 | -0.007 464 787 430 | -0.036 620 270 582 | -0.029 608 995 884 |
| H                                                                 | -0.183 995 873 986 | 0.074 663 835 228  | -0.110 807 808 663 |
| H                                                                 | 0.064 431 506 717  | -0.024 467 343 389 | -0.024 521 329 983 |
| H                                                                 | 0.063 319 142 202  | 0.016 646 999 937  | 0.049 060 262 326  |
| H                                                                 | -0.017 029 227 657 | -0.045 017 833 047 | 0.039 857 469 048  |
| H                                                                 | -0.088 580 570 264 | 0.044 447 512 285  | 0.013 880 923 086  |
| H                                                                 | -0.033 521 089 120 | -0.005 396 159 559 | 0.039 553 578 559  |
| H                                                                 | -0.059 300 412 197 | -0.055 586 249 986 | -0.011 638 072 512 |
| H                                                                 | 0.022 578 908 936  | -0.000 597 855 308 | 0.050 878 339 686  |



Wavenumber/cm<sup>-1</sup>: 1134.4037

| $\frac{\partial \mu_{x,y,z}}{\partial Q_r} / (e u^{-0.5})$        | 0.000 682 577 379  | 0.011 035 983 360  | -0.004 090 283 909                    |
|-------------------------------------------------------------------|--------------------|--------------------|---------------------------------------|
| <i>l</i> -matrix coefficients/(u <sup>1/2</sup> Å <sup>-1</sup> ) |                    |                    |                                       |
| O                                                                 | 0.010 391 469 687  | 0.028 703 317 324  | -0.012 733 840 372                    |
| C                                                                 | -0.016 833 026 109 | 0.007 540 077 382  | -1.223 193 700 000 × 10 <sup>-5</sup> |
| C                                                                 | -0.110 544 848 066 | -0.019 844 826 052 | 0.124 981 519 386                     |
| C                                                                 | 0.122 641 025 321  | -0.270 654 686 257 | -0.084 292 162 692                    |
| C                                                                 | 0.094 059 526 286  | -0.122 283 110 685 | -0.141 998 337 710                    |
| C                                                                 | -0.226 161 143 743 | 0.236 921 223 876  | -0.017 335 770 719                    |
| C                                                                 | 0.004 128 815 529  | -0.201 680 893 709 | -0.001 509 146 362                    |
| C                                                                 | 0.082 286 617 688  | 0.147 263 718 505  | 0.053 893 846 804                     |
| C                                                                 | 0.033 870 622 799  | -0.005 639 724 624 | -0.016 784 086 292                    |
| C                                                                 | 0.030 920 913 836  | 0.018 702 939 171  | -0.051 470 397 047                    |
| C                                                                 | -0.029 631 466 332 | 0.088 888 777 472  | 0.065 251 767 134                     |
| H                                                                 | 0.235 814 052 272  | -0.221 759 530 836 | 0.115 105 796 706                     |
| H                                                                 | 0.052 057 902 060  | 0.034 448 229 578  | 0.044 135 893 398                     |
| H                                                                 | 0.083 570 362 102  | 0.131 489 933 759  | 0.080 064 925 360                     |
| H                                                                 | 0.003 788 832 446  | -0.003 479 983 458 | -0.002 200 099 757                    |
| H                                                                 | 0.166 520 611 520  | -0.145 586 061 491 | 0.022 585 664 394                     |
| H                                                                 | 0.125 182 182 012  | -0.031 812 524 697 | 0.121 691 226 905                     |
| H                                                                 | -0.028 498 760 908 | -0.034 731 434 341 | -0.029 490 635 657                    |
| H                                                                 | -0.215 865 498 687 | 0.440 636 794 383  | 0.118 282 976 577                     |
| H                                                                 | -0.260 803 767 006 | 0.103 315 000 116  | -0.185 708 121 908                    |
| H                                                                 | 0.004 249 995 940  | -0.006 440 621 420 | -0.028 119 720 443                    |
| H                                                                 | 0.006 897 688 696  | 0.030 035 863 374  | 0.057 867 070 421                     |
| H                                                                 | -0.111 056 012 570 | 0.049 204 564 455  | 0.010 667 880 178                     |
| H                                                                 | -0.031 637 598 449 | -0.033 794 493 345 | -0.012 405 388 933                    |
| H                                                                 | 0.010 607 364 786  | -0.010 573 315 157 | -0.030 737 555 049                    |
| H                                                                 | -0.013 754 390 444 | -0.006 810 507 745 | 0.039 179 274 283                     |
| H                                                                 | -0.015 785 940 661 | 0.008 454 587 452  | -0.031 050 514 005                    |

Wavenumber/cm<sup>-1</sup>: 1178.344

| $\frac{\partial \mu_{x,y,z}}{\partial Q_r} / (e u^{-0.5})$        | -0.011 949 359 481 | 0.014 733 623 213  | -0.005 683 501 934 |
|-------------------------------------------------------------------|--------------------|--------------------|--------------------|
| <i>l</i> -matrix coefficients/(u <sup>1/2</sup> Å <sup>-1</sup> ) |                    |                    |                    |
| O                                                                 | -0.015 247 483 634 | 0.003 482 944 288  | 0.011 261 791 495  |
| C                                                                 | 0.161 932 216 499  | -0.040 384 146 519 | -0.041 647 514 291 |
| C                                                                 | -0.469 038 860 540 | 0.226 057 792 569  | 0.084 173 694 983  |
| C                                                                 | 0.054 754 082 761  | -0.139 510 137 329 | 0.194 663 151 200  |
| C                                                                 | -0.104 875 423 225 | -0.259 976 873 004 | -0.032 383 202 589 |
| C                                                                 | 0.078 955 591 538  | 0.149 759 489 424  | -0.034 782 980 932 |
| C                                                                 | -0.007 290 441 278 | 0.096 817 361 963  | -0.118 055 715 070 |
| C                                                                 | 0.098 706 716 373  | 0.048 388 812 894  | 0.081 069 298 651  |
| C                                                                 | 0.172 694 823 772  | -0.074 601 546 185 | 0.009 239 194 713  |
| C                                                                 | 0.174 262 344 381  | -0.072 510 972 816 | -0.047 200 896 851 |
| C                                                                 | -0.031 299 244 121 | 0.039 896 862 187  | -0.080 819 706 508 |
| H                                                                 | -0.150 777 241 861 | 0.059 896 056 890  | 0.028 927 961 298  |
| H                                                                 | -0.009 913 965 840 | -0.100 883 476 252 | -0.084 532 142 271 |
| H                                                                 | -0.000 736 566 577 | 0.035 503 271 286  | 0.074 301 966 302  |
| H                                                                 | -0.058 947 762 254 | 0.070 770 432 956  | 0.027 112 010 071  |
| H                                                                 | 0.135 120 047 859  | -0.094 253 879 033 | -0.072 056 156 890 |
| H                                                                 | -0.253 426 143 847 | 0.035 204 759 194  | -0.209 280 608 614 |
| H                                                                 | -0.129 389 644 621 | 0.000 174 392 079  | -0.123 101 371 311 |
| H                                                                 | 0.037 329 445 056  | -0.050 558 939 818 | 0.037 563 462 201  |
| H                                                                 | 0.152 785 090 397  | -0.000 469 103 044 | 0.144 409 842 520  |
| H                                                                 | -0.079 519 395 878 | 0.024 310 599 302  | -0.066 061 559 225 |
| H                                                                 | -0.104 937 876 630 | 0.058 757 467 557  | 0.049 198 938 852  |
| H                                                                 | 0.002 660 151 859  | -0.046 433 415 567 | 0.033 606 371 856  |
| H                                                                 | -0.077 688 639 834 | 0.056 381 662 616  | 0.021 064 440 326  |
| H                                                                 | 0.078 349 390 244  | -0.035 641 376 102 | -0.170 967 414 084 |
| H                                                                 | 0.056 722 788 616  | 0.064 153 999 739  | 0.158 923 530 895  |
| H                                                                 | 0.018 496 031 822  | -0.000 818 548 005 | 0.056 813 734 378  |

Wavenumber/cm<sup>-1</sup>: 1192.5266

| $\frac{\partial \mu_{x,y,z}}{\partial Q_r} / (e u^{-0.5})$        | -0.002 260 109 285 | 0.013 028 326 511  | 0.007 117 759 687  |
|-------------------------------------------------------------------|--------------------|--------------------|--------------------|
| <i>l</i> -matrix coefficients/(u <sup>1/2</sup> Å <sup>-1</sup> ) |                    |                    |                    |
| O                                                                 | -0.005 288 108 405 | 0.068 630 993 332  | -0.036 566 363 174 |
| C                                                                 | -0.010 210 917 445 | 0.026 025 322 763  | 0.021 029 835 179  |
| C                                                                 | -0.191 944 322 972 | -0.470 984 731 591 | 0.154 614 892 374  |
| C                                                                 | 0.060 913 454 141  | -0.196 762 692 425 | -0.041 616 492 691 |
| C                                                                 | -0.017 419 788 430 | 0.183 392 132 741  | 0.030 169 278 199  |
| C                                                                 | 0.033 032 496 952  | -0.026 147 507 953 | -0.027 263 524 631 |
| C                                                                 | 0.138 350 361 220  | -0.003 122 508 732 | -0.078 373 091 180 |
| C                                                                 | -0.145 966 682 181 | -0.040 561 291 231 | 0.031 511 189 515  |
| C                                                                 | 0.090 868 044 082  | 0.201 435 966 317  | -0.040 260 059 533 |
| C                                                                 | 0.078 937 222 281  | 0.158 005 782 534  | -0.086 056 664 409 |
| C                                                                 | -0.007 475 157 907 | 0.090 153 939 342  | 0.013 279 978 780  |
| H                                                                 | 0.092 532 764 322  | -0.049 620 932 727 | -0.006 020 688 818 |
| H                                                                 | -0.175 913 314 683 | 0.271 750 835 473  | 0.055 852 029 425  |
| H                                                                 | 0.120 603 000 466  | 0.103 854 949 055  | -0.070 698 267 814 |
| H                                                                 | -0.050 320 131 788 | -0.123 454 710 390 | 0.108 804 301 693  |
| H                                                                 | -0.120 288 923 126 | 0.099 262 410 318  | -0.056 738 662 908 |
| H                                                                 | -0.081 145 488 050 | 0.107 415 360 124  | -0.054 890 134 857 |
| H                                                                 | -0.037 229 384 069 | -0.141 146 851 527 | -0.027 387 845 488 |
| H                                                                 | 0.063 607 444 928  | -0.041 217 929 077 | 0.064 100 141 995  |
| H                                                                 | 0.228 808 290 467  | -0.087 034 088 644 | 0.141 839 370 481  |
| H                                                                 | 0.125 002 245 096  | -0.046 821 026 282 | -0.172 153 100 838 |
| H                                                                 | 0.092 631 680 619  | 0.075 566 350 015  | 0.163 364 349 110  |
| H                                                                 | -0.081 608 814 168 | 0.024 163 524 797  | 0.016 488 093 627  |
| H                                                                 | -0.067 164 144 560 | -0.000 773 725 577 | 0.001 567 183 530  |
| H                                                                 | -0.117 110 992 898 | -0.092 966 971 279 | 0.024 982 460 136  |
| H                                                                 | -0.089 059 839 201 | -0.081 801 341 614 | 0.056 724 152 088  |
| H                                                                 | 0.017 323 965 833  | -0.019 400 239 671 | -0.020 876 485 141 |

Wavenumber/cm<sup>-1</sup>: 1220.278

| $\frac{\partial \mu_{x,y,z}}{\partial Q_r} / (e u^{-0.5})$        | 0.007 383 841 633  | -0.005 608 027 780 | 0.002 222 519 109  |
|-------------------------------------------------------------------|--------------------|--------------------|--------------------|
| <i>l</i> -matrix coefficients/(u <sup>1/2</sup> Å <sup>-1</sup> ) |                    |                    |                    |
| O                                                                 | -0.036 388 868 321 | -0.005 517 638 567 | 0.024 074 011 677  |
| C                                                                 | 0.092 087 093 372  | -0.053 266 307 446 | -0.086 320 500 011 |
| C                                                                 | -0.174 535 638 198 | -0.101 741 540 344 | 0.330 438 560 871  |
| C                                                                 | -0.147 596 010 974 | 0.461 461 987 802  | 0.115 759 900 925  |
| C                                                                 | 0.000 430 736 798  | 0.006 408 660 643  | 0.077 387 894 873  |
| C                                                                 | -0.071 235 423 237 | -0.004 204 990 868 | -0.131 041 643 445 |
| C                                                                 | -0.075 796 212 712 | -0.055 866 720 504 | 0.073 980 319 331  |
| C                                                                 | -0.026 943 855 300 | -0.022 403 703 173 | -0.094 584 117 222 |
| C                                                                 | 0.082 533 029 114  | 0.058 368 393 646  | -0.086 400 054 833 |
| C                                                                 | 0.077 581 771 904  | 0.040 846 087 554  | -0.124 534 020 816 |
| C                                                                 | 0.039 952 487 251  | -0.179 077 393 716 | -0.057 022 529 324 |
| H                                                                 | 0.005 350 588 265  | 0.036 585 118 746  | -0.070 825 587 964 |
| H                                                                 | 0.084 916 819 393  | -0.082 390 326 613 | 0.008 196 038 111  |
| H                                                                 | 0.275 602 599 873  | 0.041 471 132 042  | -0.221 268 072 864 |
| H                                                                 | 0.002 713 337 251  | -0.044 812 360 525 | 0.012 535 645 874  |
| H                                                                 | 0.209 666 311 649  | -0.154 488 909 217 | 0.116 452 564 228  |
| H                                                                 | 0.185 837 189 060  | -0.069 590 752 274 | 0.147 476 457 712  |
| H                                                                 | -0.096 165 571 560 | -0.107 474 246 231 | -0.086 975 002 441 |
| H                                                                 | 0.004 769 945 528  | -0.089 565 914 324 | -0.093 587 667 784 |
| H                                                                 | -0.121 007 309 123 | 0.022 801 554 642  | -0.086 802 199 884 |
| H                                                                 | 0.066 559 357 713  | -0.024 497 263 481 | -0.085 239 785 568 |
| H                                                                 | 0.012 503 539 347  | 0.057 693 105 698  | 0.102 405 307 587  |
| H                                                                 | 0.180 865 397 921  | -0.068 332 914 108 | -0.026 976 821 798 |
| H                                                                 | 0.107 548 443 472  | 0.029 596 710 468  | 0.011 868 992 001  |
| H                                                                 | -0.016 287 936 179 | -0.027 310 016 787 | -0.014 080 036 025 |
| H                                                                 | -0.045 827 668 396 | -0.036 548 208 461 | 0.079 319 852 771  |
| H                                                                 | -0.009 514 576 229 | 0.019 238 266 554  | 0.050 612 377 715  |

Wavenumber/cm<sup>-1</sup>: 1238.826

| $\frac{\partial \mu_{x,y,z}}{\partial Q_r} / (e u^{-0.5})$        | 0.004 698 438 860  | 0.001 632 985 700  | 0.014 188 860 441  |
|-------------------------------------------------------------------|--------------------|--------------------|--------------------|
| <i>l</i> -matrix coefficients/(u <sup>1/2</sup> Å <sup>-1</sup> ) |                    |                    |                    |
| O                                                                 | 0.004 665 337 615  | -0.019 243 532 743 | -0.011 908 054 037 |
| C                                                                 | -0.049 524 129 858 | 0.030 822 027 194  | 0.104 895 829 159  |
| C                                                                 | -0.169 613 202 968 | -0.201 742 785 577 | -0.476 687 895 844 |
| C                                                                 | 0.175 094 177 331  | 0.058 557 953 894  | -0.055 745 125 666 |
| C                                                                 | -0.134 202 746 775 | 0.005 746 235 148  | 0.208 476 783 351  |
| C                                                                 | 0.088 471 812 070  | -0.118 875 502 349 | -0.015 520 140 778 |
| C                                                                 | -0.102 383 541 014 | -0.149 396 529 152 | 0.118 524 197 126  |
| C                                                                 | 0.125 089 789 581  | 0.139 593 933 993  | -0.207 028 061 354 |
| C                                                                 | 0.088 655 742 793  | 0.112 041 020 244  | 0.178 773 686 486  |
| C                                                                 | 0.115 598 227 044  | 0.038 388 620 215  | 0.131 966 706 787  |
| C                                                                 | -0.068 407 680 283 | -0.012 326 748 728 | 0.003 035 413 916  |
| H                                                                 | -0.163 965 680 107 | 0.172 129 901 473  | -0.100 357 284 588 |
| H                                                                 | 0.143 070 513 338  | -0.036 421 789 956 | 0.057 554 130 725  |
| H                                                                 | 0.052 609 190 704  | 0.006 335 886 211  | -0.033 409 808 040 |
| H                                                                 | -0.178 330 316 488 | -0.000 326 841 217 | 0.190 166 143 044  |
| H                                                                 | 0.008 715 200 466  | -0.008 078 608 713 | 0.014 353 737 652  |
| H                                                                 | 0.068 078 382 383  | -0.171 082 262 981 | 0.031 233 287 135  |
| H                                                                 | 0.020 943 509 462  | 0.042 497 843 229  | 0.026 942 825 787  |
| H                                                                 | -0.147 554 830 667 | 0.211 447 511 422  | -0.050 507 806 569 |
| H                                                                 | -0.031 369 532 962 | 0.132 690 307 990  | 0.101 812 013 469  |
| H                                                                 | -0.005 601 869 621 | -0.013 476 578 597 | -0.145 067 154 728 |
| H                                                                 | 0.000 948 573 206  | 0.014 923 611 103  | 0.011 247 493 597  |
| H                                                                 | 0.014 403 671 337  | 0.015 146 960 026  | -0.021 724 311 358 |
| H                                                                 | 0.012 064 404 000  | 0.032 553 419 357  | 0.013 060 838 313  |
| H                                                                 | -0.044 619 141 131 | -0.083 700 863 565 | -0.082 943 994 479 |
| H                                                                 | 0.049 596 135 616  | 0.042 427 947 746  | 0.056 322 666 240  |
| H                                                                 | -0.054 997 235 185 | 0.055 105 564 206  | 0.010 893 004 058  |

Wavenumber/cm<sup>-1</sup>: 1247.1759

| $\frac{\partial \mu_{x,y,z}}{\partial Q_r} / (e u^{-0.5})$        | 0.000 159 877 264  | -0.010 884 367 267 | -0.012 114 330 242 |
|-------------------------------------------------------------------|--------------------|--------------------|--------------------|
| <i>l</i> -matrix coefficients/(u <sup>1/2</sup> Å <sup>-1</sup> ) |                    |                    |                    |
| O                                                                 | -0.034 256 508 035 | -0.037 020 374 204 | -0.010 268 469 524 |
| C                                                                 | 0.098 651 395 803  | 0.033 532 422 406  | 0.097 090 762 134  |
| C                                                                 | -0.059 908 145 282 | -0.127 509 245 012 | -0.085 906 218 652 |
| C                                                                 | -0.238 708 519 052 | 0.097 928 262 540  | -0.447 956 788 315 |
| C                                                                 | -0.089 668 286 292 | -0.062 281 117 636 | -0.084 614 379 077 |
| C                                                                 | 0.012 616 061 067  | 0.073 029 985 785  | 0.215 135 367 577  |
| C                                                                 | -0.035 203 579 194 | 0.196 338 827 376  | 0.105 560 008 276  |
| C                                                                 | 0.141 382 230 996  | -0.039 561 023 432 | 0.024 897 065 745  |
| C                                                                 | 0.039 546 160 860  | 0.044 844 817 110  | 0.046 918 539 588  |
| C                                                                 | 0.037 207 040 814  | 0.069 681 935 455  | 0.001 587 998 650  |
| C                                                                 | 0.103 813 451 057  | -0.065 326 786 623 | 0.244 513 032 530  |
| H                                                                 | 0.063 128 210 565  | -0.143 273 611 470 | 0.165 010 797 609  |
| H                                                                 | 0.088 791 922 317  | -0.211 703 886 520 | -0.063 047 254 165 |
| H                                                                 | 0.029 195 725 353  | 0.146 393 964 405  | 0.096 503 329 567  |
| H                                                                 | -0.058 283 463 678 | -0.008 471 377 623 | 0.065 339 035 071  |
| H                                                                 | 0.070 950 203 591  | -0.080 808 722 683 | -0.012 658 281 056 |
| H                                                                 | -0.177 995 081 568 | -0.011 711 123 874 | -0.170 616 376 376 |
| H                                                                 | -0.006 064 211 556 | -0.030 896 627 978 | -0.001 254 593 755 |
| H                                                                 | 0.093 945 859 805  | -0.189 784 512 815 | -0.068 461 012 775 |
| H                                                                 | -0.078 562 016 578 | 0.025 513 717 246  | -0.044 152 597 520 |
| H                                                                 | 0.005 102 496 057  | -0.005 536 961 929 | -0.054 092 233 935 |
| H                                                                 | 0.042 576 399 911  | 0.027 619 893 644  | 0.061 492 289 521  |
| H                                                                 | -0.107 446 680 346 | 0.147 840 094 978  | -0.074 061 387 569 |
| H                                                                 | 0.210 622 386 729  | -0.207 197 463 435 | -0.086 675 233 055 |
| H                                                                 | -0.020 917 469 543 | -0.034 064 285 359 | -0.025 971 117 841 |
| H                                                                 | -0.019 754 702 279 | -0.020 352 260 406 | 0.005 681 809 242  |
| H                                                                 | -0.032 389 137 342 | -0.017 851 405 243 | -0.156 786 672 007 |

Wavenumber/cm<sup>-1</sup>: 1267.216

| $\frac{\partial \mu_{x,y,z}}{\partial Q_r} / (e u^{-0.5})$   |                    |                    |                    |
|--------------------------------------------------------------|--------------------|--------------------|--------------------|
|                                                              | -0.006 919 908 711 | -0.004 741 886 312 | 0.003 612 202 953  |
| $l$ -matrix coefficients/(u <sup>1/2</sup> Å <sup>-1</sup> ) |                    |                    |                    |
| O                                                            | 0.016 667 655 064  | -0.016 901 306 775 | 0.007 424 067 275  |
| C                                                            | -0.091 942 439 420 | -0.008 950 031 373 | -0.022 267 024 963 |
| C                                                            | -0.020 885 498 455 | 0.167 783 563 852  | 0.347 862 919 647  |
| C                                                            | 0.101 819 697 601  | -0.143 453 001 592 | -0.273 441 762 424 |
| C                                                            | -0.208 493 024 993 | 0.106 670 983 255  | 0.053 588 368 575  |
| C                                                            | 0.193 073 637 587  | -0.052 502 992 576 | 0.057 602 901 988  |
| C                                                            | 0.031 780 274 450  | 0.044 794 208 927  | 0.182 826 302 495  |
| C                                                            | 0.059 684 711 906  | -0.091 973 777 796 | -0.153 263 958 111 |
| C                                                            | 0.029 414 520 347  | -0.074 694 525 539 | -0.137 353 882 670 |
| C                                                            | -0.007 331 422 506 | -0.050 623 794 478 | -0.133 269 191 806 |
| C                                                            | -0.037 576 891 084 | 0.099 885 946 095  | 0.182 081 485 849  |
| H                                                            | -0.248 924 986 531 | 0.169 120 855 975  | -0.029 577 631 685 |
| H                                                            | 0.058 856 828 083  | 0.033 343 844 548  | 0.066 947 095 107  |
| H                                                            | -0.059 098 863 470 | -0.234 928 043 535 | -0.274 876 422 152 |
| H                                                            | 0.098 157 479 944  | 0.008 665 790 821  | -0.108 723 586 564 |
| H                                                            | 0.014 743 797 613  | -0.013 509 182 291 | -0.074 827 791 748 |
| H                                                            | 0.111 524 450 718  | -0.113 398 330 338 | 0.059 584 597 831  |
| H                                                            | -0.084 536 726 465 | -0.054 137 485 768 | -0.081 720 917 303 |
| H                                                            | -0.066 231 167 512 | 0.176 849 754 056  | 0.021 820 989 159  |
| H                                                            | 0.072 679 945 312  | 0.011 086 817 664  | 0.129 054 560 509  |
| H                                                            | 0.003 798 133 735  | 0.008 972 846 551  | 0.048 552 174 258  |
| H                                                            | -0.026 693 124 357 | 0.014 084 657 609  | 0.022 891 854 229  |
| H                                                            | -0.189 322 488 639 | 0.152 805 401 709  | -0.038 498 392 492 |
| H                                                            | 0.075 237 336 863  | -0.113 132 885 368 | -0.053 105 173 195 |
| H                                                            | 0.056 347 937 836  | 0.038 042 121 497  | -0.009 303 224 823 |
| H                                                            | -0.017 783 637 890 | -0.004 399 038 755 | 0.040 795 661 932  |
| H                                                            | -0.036 183 669 700 | -0.001 556 092 745 | -0.108 861 946 264 |

Wavenumber/cm<sup>-1</sup>: 1276.1476

| $\frac{\partial \mu_{x,y,z}}{\partial Q_r} / (e \text{ u}^{-0.5})$ | 0.006 479 199 972  | 0.005 740 153 738  | 0.001 675 903 701  |
|--------------------------------------------------------------------|--------------------|--------------------|--------------------|
| <i>l</i> -matrix coefficients/(u <sup>1/2</sup> Å <sup>-1</sup> )  |                    |                    |                    |
| O                                                                  | 0.009 483 788 911  | -0.052 968 094 328 | 0.007 123 383 596  |
| C                                                                  | 0.017 624 618 570  | 0.013 359 713 415  | 0.072 957 907 435  |
| C                                                                  | -0.079 574 569 741 | 0.207 185 812 032  | -0.064 014 580 617 |
| C                                                                  | -0.001 242 259 449 | -0.111 168 576 208 | -0.086 572 797 058 |
| C                                                                  | -0.071 936 992 605 | 0.026 714 796 799  | 0.082 661 036 555  |
| C                                                                  | 0.107 707 328 294  | -0.061 239 277 907 | -0.094 116 331 833 |
| C                                                                  | -0.007 209 448 805 | -0.043 438 408 910 | 0.094 826 042 562  |
| C                                                                  | -0.095 870 832 193 | -0.004 278 595 461 | 0.033 164 029 425  |
| C                                                                  | 0.089 401 740 291  | -0.123 492 580 746 | 0.071 252 512 267  |
| C                                                                  | 0.067 175 660 915  | -0.112 193 265 964 | 0.002 918 875 711  |
| C                                                                  | 0.004 142 799 422  | 0.081 027 494 027  | 0.023 061 536 068  |
| H                                                                  | 0.080 724 633 170  | -0.067 444 765 123 | -0.008 583 328 661 |
| H                                                                  | -0.064 340 371 981 | 0.225 643 016 158  | 0.111 445 897 466  |
| H                                                                  | 0.366 812 142 347  | 0.248 943 581 762  | -0.124 831 044 759 |
| H                                                                  | -0.070 876 363 496 | 0.090 210 486 865  | 0.028 119 430 572  |
| H                                                                  | -0.261 311 314 259 | 0.224 528 861 048  | -0.124 342 997 207 |
| H                                                                  | 0.119 170 929 501  | 0.023 093 626 586  | 0.123 475 650 911  |
| H                                                                  | -0.061 478 480 077 | 0.044 575 053 371  | -0.060 977 531 707 |
| H                                                                  | 0.108 233 088 242  | -0.276 256 720 156 | -0.112 740 572 564 |
| H                                                                  | -0.256 181 855 660 | 0.020 583 462 521  | -0.217 907 195 488 |
| H                                                                  | -0.116 520 082 082 | 0.044 456 550 679  | 0.040 958 547 616  |
| H                                                                  | -0.101 147 987 197 | -0.001 928 334 649 | -0.051 378 820 400 |
| H                                                                  | -0.081 075 751 429 | 0.030 669 436 686  | 0.011 069 759 308  |
| H                                                                  | -0.040 137 677 591 | -0.019 594 162 586 | -0.010 576 391 561 |
| H                                                                  | 0.117 634 343 365  | 0.010 159 415 975  | -0.172 838 705 697 |
| H                                                                  | 0.082 892 511 161  | 0.097 785 956 638  | 0.102 201 068 561  |
| H                                                                  | 0.035 505 923 666  | -0.044 189 656 863 | -0.031 420 584 513 |



Wavenumber/cm<sup>-1</sup>: 1293.3606

| $\frac{\partial \mu_{x,y,z}}{\partial Q_r} / (e u^{-0.5})$        | -0.012 603 523 175 | -0.012 926 707 311 | -0.004 348 478 870 |
|-------------------------------------------------------------------|--------------------|--------------------|--------------------|
| <i>l</i> -matrix coefficients/(u <sup>1/2</sup> Å <sup>-1</sup> ) |                    |                    |                    |
| O                                                                 | 0.012 469 925 592  | 0.048 189 593 928  | -0.041 461 227 049 |
| C                                                                 | 0.005 686 812 659  | 0.068 585 918 362  | 0.086 380 448 791  |
| C                                                                 | 0.006 136 678 967  | -0.100 378 861 876 | -0.147 144 407 172 |
| C                                                                 | -0.161 049 558 534 | -0.127 724 078 163 | 0.053 129 252 860  |
| C                                                                 | -0.020 308 511 029 | -0.143 932 312 121 | -0.142 529 154 946 |
| C                                                                 | 0.030 605 845 087  | 0.148 203 559 707  | -0.041 493 604 952 |
| C                                                                 | 0.018 344 692 415  | 0.024 732 086 039  | 0.060 827 199 330  |
| C                                                                 | -0.027 017 690 812 | -0.040 088 875 224 | 0.100 597 809 755  |
| C                                                                 | -0.008 388 008 455 | 0.008 801 600 364  | 0.087 242 588 956  |
| C                                                                 | -0.019 784 963 842 | 0.131 789 262 946  | 0.043 613 290 747  |
| C                                                                 | 0.171 198 476 957  | 0.173 200 681 030  | -0.053 590 262 465 |
| H                                                                 | -0.300 519 919 033 | 0.164 554 104 807  | -0.008 902 125 051 |
| H                                                                 | -0.075 613 468 020 | 0.146 750 359 712  | 0.061 667 664 360  |
| H                                                                 | -0.080 890 792 069 | -0.166 373 679 221 | -0.098 041 059 874 |
| H                                                                 | -0.057 743 088 332 | 0.010 997 715 958  | 0.054 839 509 053  |
| H                                                                 | 0.310 003 819 218  | -0.262 288 436 812 | -0.037 286 944 972 |
| H                                                                 | 0.193 006 969 488  | 0.021 460 136 493  | 0.181 265 174 803  |
| H                                                                 | 0.068 521 248 211  | -0.018 402 138 624 | 0.067 293 062 388  |
| H                                                                 | 0.099 858 480 941  | -0.213 017 945 681 | -0.041 592 030 404 |
| H                                                                 | -0.107 985 198 055 | -0.027 564 406 934 | -0.133 926 146 364 |
| H                                                                 | -0.018 085 791 956 | -0.003 475 815 611 | -0.019 790 021 008 |
| H                                                                 | 0.099 813 531 987  | 0.008 937 472 931  | 0.048 081 702 823  |
| H                                                                 | -0.166 080 717 131 | -0.008 574 625 462 | 0.073 623 559 935  |
| H                                                                 | -0.171 050 895 774 | -0.021 367 614 836 | -0.004 676 026 824 |
| H                                                                 | -0.004 922 028 109 | -0.016 434 905 148 | -0.025 590 063 161 |
| H                                                                 | -0.056 160 538 315 | -0.072 757 395 713 | -0.092 110 083 942 |
| H                                                                 | 0.233 964 257 133  | -0.228 719 771 445 | -0.022 028 941 888 |

Wavenumber/cm<sup>-1</sup>: 1321.3037

| $\frac{\partial \mu_{x,y,z}}{\partial Q_r} / (e u^{-0.5})$        | 0.000 570 980 134  | -0.002 990 632 646 | -0.005 261 972 163 |
|-------------------------------------------------------------------|--------------------|--------------------|--------------------|
| <i>l</i> -matrix coefficients/(u <sup>1/2</sup> Å <sup>-1</sup> ) |                    |                    |                    |
| O                                                                 | 0.067 897 699 169  | 0.030 189 331 746  | 0.012 936 774 486  |
| C                                                                 | -0.280 792 089 313 | -0.029 788 167 521 | -0.136 731 202 952 |
| C                                                                 | 0.048 515 779 751  | 0.032 431 206 880  | 0.040 108 099 285  |
| C                                                                 | -0.050 435 581 541 | 0.035 412 874 733  | 0.037 109 972 471  |
| C                                                                 | 0.073 763 504 789  | 0.138 838 299 156  | 0.089 994 791 227  |
| C                                                                 | -0.139 544 293 512 | -0.214 566 496 943 | -0.038 279 532 383 |
| C                                                                 | 0.150 731 247 442  | -0.043 012 455 758 | 0.030 693 244 979  |
| C                                                                 | -0.110 736 552 202 | 0.011 529 263 220  | -0.080 973 418 774 |
| C                                                                 | 0.007 866 783 212  | 0.104 186 913 225  | -0.010 684 206 219 |
| C                                                                 | 0.095 131 480 111  | -0.206 337 874 887 | 0.000 889 538 134  |
| C                                                                 | 0.186 485 848 437  | 0.161 612 308 653  | 0.048 236 649 721  |
| H                                                                 | 0.034 635 206 020  | 0.134 433 020 370  | -0.175 399 300 056 |
| H                                                                 | 0.041 533 759 475  | -0.126 274 259 437 | -0.034 781 214 458 |
| H                                                                 | -0.017 453 697 197 | 0.124 367 100 347  | 0.157 022 496 212  |
| H                                                                 | -0.014 736 901 611 | -0.051 250 551 474 | 0.040 281 055 983  |
| H                                                                 | 0.113 852 390 280  | -0.089 472 353 670 | 0.266 220 050 555  |
| H                                                                 | -0.138 887 033 466 | 0.038 920 516 491  | -0.118 731 436 892 |
| H                                                                 | -0.102 840 045 393 | 0.055 634 941 822  | -0.098 170 470 706 |
| H                                                                 | 0.040 789 557 786  | 0.002 174 699 263  | 0.060 166 675 744  |
| H                                                                 | -0.059 397 063 017 | 0.002 063 417 782  | -0.062 696 241 350 |
| H                                                                 | 0.087 018 117 583  | -0.040 312 967 354 | -0.096 914 199 589 |
| H                                                                 | -0.167 291 105 652 | -0.023 987 572 981 | -0.117 342 356 699 |
| H                                                                 | -0.237 845 561 001 | 0.067 633 560 891  | 0.039 786 925 555  |
| H                                                                 | -0.071 831 214 989 | -0.093 085 022 216 | -0.038 657 965 961 |
| H                                                                 | -0.067 105 276 259 | -0.026 012 079 874 | 0.067 964 032 916  |
| H                                                                 | 0.138 318 665 175  | 0.167 786 389 137  | 0.196 626 319 446  |
| H                                                                 | 0.216 365 882 557  | -0.229 431 593 081 | -0.069 132 178 040 |

Wavenumber/cm<sup>-1</sup>: 1345.494

| $\frac{\partial \mu_{x,y,z}}{\partial Q_r} / (e u^{-0.5})$        | 0.002 456 922 037  | -0.008 698 206 323 | 0.005 797 745 706  |
|-------------------------------------------------------------------|--------------------|--------------------|--------------------|
| <i>l</i> -matrix coefficients/(u <sup>1/2</sup> Å <sup>-1</sup> ) |                    |                    |                    |
| O                                                                 | -0.089 401 924 318 | 0.051 136 334 093  | -0.016 716 645 339 |
| C                                                                 | 0.419 773 188 275  | -0.022 096 646 834 | -0.022 408 019 735 |
| C                                                                 | -0.180 781 608 345 | -0.050 608 626 172 | 0.067 121 742 321  |
| C                                                                 | 0.052 029 042 258  | -0.107 441 743 909 | -0.017 145 664 265 |
| C                                                                 | 0.026 481 360 006  | -0.008 838 671 747 | 0.174 946 932 404  |
| C                                                                 | 0.062 501 536 787  | 0.063 591 728 881  | -0.061 015 026 476 |
| C                                                                 | -0.019 988 493 362 | -0.126 957 104 774 | 0.126 993 046 569  |
| C                                                                 | -0.009 855 418 151 | 0.104 546 794 390  | -0.177 949 365 362 |
| C                                                                 | -0.117 968 179 862 | 0.109 580 900 454  | -0.242 462 710 955 |
| C                                                                 | -0.076 636 825 130 | -0.071 727 812 512 | 0.159 161 833 033  |
| C                                                                 | -0.077 420 279 959 | 0.067 203 742 912  | 0.012 239 387 838  |
| H                                                                 | -0.045 979 127 348 | -0.010 024 980 993 | 0.022 822 547 118  |
| H                                                                 | 0.040 376 558 788  | 0.118 688 630 739  | 0.101 157 037 451  |
| H                                                                 | -0.014 074 042 116 | 0.051 768 343 267  | 0.131 028 403 116  |
| H                                                                 | 0.215 745 094 137  | -0.119 012 980 351 | -0.163 910 556 399 |
| H                                                                 | 0.073 379 967 042  | -0.058 310 149 649 | -0.070 254 403 461 |
| H                                                                 | -0.084 392 932 563 | -0.114 787 645 199 | -0.071 872 450 935 |
| H                                                                 | 0.128 167 759 994  | 0.144 507 099 549  | 0.111 326 896 860  |
| H                                                                 | 0.048 504 945 121  | -0.180 325 809 257 | -0.137 318 395 926 |
| H                                                                 | -0.130 118 989 888 | 0.113 870 590 548  | 0.011 514 241 974  |
| H                                                                 | 0.149 689 005 500  | -0.044 044 550 457 | -0.009 056 093 422 |
| H                                                                 | -0.091 693 221 408 | -0.073 908 954 719 | -0.191 358 698 134 |
| H                                                                 | -0.051 085 094 207 | 0.019 992 566 570  | 0.008 258 605 324  |
| H                                                                 | -0.046 925 285 445 | 0.015 790 329 041  | 0.006 886 073 129  |
| H                                                                 | -0.142 505 965 624 | 0.024 473 937 547  | 0.298 594 526 533  |
| H                                                                 | 0.053 795 319 754  | 0.049 760 516 207  | -0.048 157 776 723 |
| H                                                                 | -0.016 417 833 672 | 0.005 395 194 536  | -0.000 311 549 956 |

Wavenumber/cm<sup>-1</sup>: 1359.4338

| $\frac{\partial \mu_{x,y,z}}{\partial Q_r} / (e u^{-0.5})$        | 0.012 683 050 894  | 0.011 714 517 346  | 0.019 676 056 805  |
|-------------------------------------------------------------------|--------------------|--------------------|--------------------|
| <i>l</i> -matrix coefficients/(u <sup>1/2</sup> Å <sup>-1</sup> ) |                    |                    |                    |
| O                                                                 | 0.031 474 752 883  | 0.009 055 843 292  | -0.028 205 155 895 |
| C                                                                 | -0.154 496 511 144 | 0.068 110 163 878  | 0.107 725 183 953  |
| C                                                                 | 0.012 849 196 842  | 0.015 427 682 965  | 0.088 679 624 554  |
| C                                                                 | -0.037 633 435 937 | 0.071 067 282 717  | -0.012 105 384 209 |
| C                                                                 | 0.024 359 034 648  | 0.006 870 399 455  | 0.173 338 681 158  |
| C                                                                 | 0.036 183 951 190  | -0.037 157 609 447 | -0.039 868 789 532 |
| C                                                                 | -0.079 490 806 485 | -0.184 514 232 937 | 0.148 472 868 681  |
| C                                                                 | 0.071 698 958 434  | 0.099 551 062 394  | -0.246 871 871 324 |
| C                                                                 | 0.034 274 312 680  | -0.149 714 821 965 | -0.018 831 485 055 |
| C                                                                 | -0.029 517 182 174 | 0.138 334 202 911  | -0.148 685 712 331 |
| C                                                                 | 0.125 600 703 382  | 0.072 313 663 206  | -0.122 948 433 823 |
| H                                                                 | 0.178 624 183 943  | -0.127 029 058 921 | 0.024 151 807 642  |
| H                                                                 | 0.114 593 581 570  | 0.095 757 666 893  | 0.116 407 612 655  |
| H                                                                 | -0.173 758 238 962 | -0.022 312 441 531 | 0.214 842 832 633  |
| H                                                                 | 0.042 811 151 183  | 0.073 925 316 391  | -0.075 102 526 335 |
| H                                                                 | -0.025 658 883 038 | 0.035 508 086 405  | 0.012 739 128 406  |
| H                                                                 | -0.174 566 529 200 | -0.179 625 528 488 | -0.166 292 482 478 |
| H                                                                 | -0.058 700 240 825 | -0.153 289 690 441 | -0.041 277 168 939 |
| H                                                                 | -0.014 532 352 532 | -0.102 275 067 423 | -0.185 989 183 602 |
| H                                                                 | -0.049 287 148 032 | 0.142 380 024 115  | 0.142 967 141 049  |
| H                                                                 | -0.107 345 642 290 | 0.061 782 261 574  | 0.147 434 873 355  |
| H                                                                 | 0.147 943 414 060  | 0.068 811 490 564  | 0.224 144 382 585  |
| H                                                                 | -0.009 405 282 142 | -0.078 100 165 973 | 0.064 829 601 737  |
| H                                                                 | -0.168 067 457 062 | 0.060 414 527 817  | 0.035 983 491 952  |
| H                                                                 | 0.116 691 934 395  | 0.038 935 480 882  | -0.120 009 195 172 |
| H                                                                 | -0.131 478 279 302 | -0.141 041 825 036 | -0.065 391 074 903 |
| H                                                                 | 0.173 522 905 803  | -0.156 111 913 160 | 0.028 352 096 082  |

Wavenumber/cm<sup>-1</sup>: 1395.3147

| $\frac{\partial \mu_{x,y,z}}{\partial Q_r} / (e u^{-0.5})$        | 0.002 508 703 905  | -0.000 267 605 277 | 0.006 107 431 875  |
|-------------------------------------------------------------------|--------------------|--------------------|--------------------|
| <i>l</i> -matrix coefficients/(u <sup>1/2</sup> Å <sup>-1</sup> ) |                    |                    |                    |
| O                                                                 | -0.051 510 961 155 | 0.017 825 454 834  | -0.006 818 545 194 |
| C                                                                 | 0.252 374 378 450  | -0.000 495 502 602 | 0.031 592 614 877  |
| C                                                                 | -0.128 777 740 525 | -0.036 188 286 197 | -0.005 857 116 912 |
| C                                                                 | 0.079 850 552 156  | -0.056 009 500 965 | 0.026 717 526 473  |
| C                                                                 | 0.128 456 154 359  | 0.113 434 507 540  | 0.067 402 984 995  |
| C                                                                 | -0.128 844 541 228 | -0.158 349 780 184 | -0.117 689 002 454 |
| C                                                                 | 0.174 165 336 394  | -0.047 334 485 472 | -0.010 549 958 950 |
| C                                                                 | -0.200 144 559 979 | 0.035 926 868 034  | -0.034 612 412 367 |
| C                                                                 | 0.041 663 669 055  | -0.201 067 307 580 | -0.005 068 073 088 |
| C                                                                 | -0.125 829 857 638 | 0.165 531 779 054  | 0.056 180 116 444  |
| C                                                                 | -0.077 129 240 608 | 0.056 479 336 809  | 0.118 844 622 110  |
| H                                                                 | -0.053 439 203 731 | 0.219 007 260 293  | -0.222 409 470 153 |
| H                                                                 | 0.033 016 104 246  | -0.185 044 967 479 | -0.069 186 362 863 |
| H                                                                 | 0.160 819 984 085  | 0.109 099 611 014  | -0.030 229 230 042 |
| H                                                                 | 0.013 224 266 617  | 0.105 637 774 621  | -0.070 233 074 179 |
| H                                                                 | 0.058 274 879 748  | -0.030 181 160 575 | 0.207 685 196 796  |
| H                                                                 | -0.124 004 340 646 | 0.111 381 631 252  | -0.094 394 893 226 |
| H                                                                 | 0.160 754 660 376  | -0.002 238 485 480 | 0.145 809 124 854  |
| H                                                                 | 0.026 138 419 239  | 0.055 928 738 023  | 0.107 398 653 002  |
| H                                                                 | -0.009 983 041 133 | -0.032 773 009 833 | -0.069 691 961 149 |
| H                                                                 | -0.171 955 247 259 | 0.084 084 863 569  | 0.164 403 484 618  |
| H                                                                 | 0.136 787 396 971  | -0.010 072 530 170 | 0.046 155 827 877  |
| H                                                                 | -0.120 124 287 522 | 0.102 603 658 567  | -0.030 371 883 122 |
| H                                                                 | 0.070 213 625 765  | -0.069 224 353 257 | -0.037 447 447 818 |
| H                                                                 | 0.151 072 440 311  | 0.040 955 173 464  | -0.190 025 887 104 |
| H                                                                 | -0.122 117 890 606 | -0.161 534 683 103 | -0.223 405 674 997 |
| H                                                                 | -0.057 940 578 330 | 0.033 455 932 307  | -0.045 158 868 822 |

Wavenumber/cm<sup>-1</sup>: 1417.7991

| $\frac{\partial \mu_{x,y,z}}{\partial Q_r} / (e u^{-0.5})$   | 0.001 380 492 207  | 0.001 555 088 425  | 0.001 511 052 584  |
|--------------------------------------------------------------|--------------------|--------------------|--------------------|
| $l$ -matrix coefficients/(u <sup>1/2</sup> Å <sup>-1</sup> ) |                    |                    |                    |
| O                                                            | -0.029 444 657 499 | 0.039 412 883 436  | -0.025 023 091 680 |
| C                                                            | 0.147 021 534 872  | 0.015 223 565 254  | 0.014 867 547 738  |
| C                                                            | -0.075 437 252 833 | -0.081 024 499 369 | -0.149 082 679 884 |
| C                                                            | 0.007 020 384 277  | 0.003 716 688 152  | -0.016 894 719 685 |
| C                                                            | 0.108 313 242 996  | -0.165 097 665 196 | -0.139 231 840 899 |
| C                                                            | -0.240 145 732 245 | -0.125 510 134 502 | -0.013 826 609 483 |
| C                                                            | -0.277 340 679 137 | 0.136 757 735 850  | -0.008 808 331 766 |
| C                                                            | 0.270 785 911 798  | -0.015 731 086 635 | 0.186 996 326 788  |
| C                                                            | -0.205 152 958 745 | -0.051 006 132 074 | -0.023 150 834 385 |
| C                                                            | 0.168 101 093 586  | 0.070 253 595 683  | 0.051 522 993 319  |
| C                                                            | 0.061 673 919 918  | 0.059 643 737 123  | 0.018 253 601 914  |
| H                                                            | 0.079 937 743 624  | 0.115 748 343 273  | -0.159 225 209 293 |
| H                                                            | 0.034 033 033 985  | 0.079 260 390 034  | 0.024 178 882 814  |
| H                                                            | 0.152 131 519 027  | -0.027 559 825 621 | -0.142 308 613 734 |
| H                                                            | 0.203 212 673 435  | -0.002 202 249 011 | -0.176 715 225 310 |
| H                                                            | -0.142 070 340 034 | 0.132 097 928 944  | 0.217 599 286 084  |
| H                                                            | 0.048 143 349 692  | -0.026 113 993 810 | 0.033 075 424 217  |
| H                                                            | -0.108 655 128 590 | -0.050 388 051 965 | -0.070 774 731 999 |
| H                                                            | -0.085 209 856 629 | 0.031 584 486 488  | -0.122 138 986 060 |
| H                                                            | 0.145 165 890 949  | -0.002 003 670 674 | 0.145 272 738 039  |
| H                                                            | -0.035 921 339 764 | 0.036 563 721 653  | 0.209 157 738 127  |
| H                                                            | 0.013 662 979 497  | 0.068 237 833 904  | 0.121 410 749 091  |
| H                                                            | -0.119 469 384 824 | 0.034 285 018 049  | 0.012 420 895 179  |
| H                                                            | -0.037 455 301 010 | -0.044 950 535 152 | -0.017 568 499 484 |
| H                                                            | -0.032 494 447 856 | 0.072 916 335 513  | 0.181 478 988 055  |
| H                                                            | 0.037 209 919 844  | 0.055 430 175 537  | 0.152 258 601 366  |
| H                                                            | 0.086 462 085 414  | -0.102 556 249 035 | -0.034 497 592 828 |

Wavenumber/cm<sup>-1</sup>: 1422.1175

| $\frac{\partial \mu_{x,y,z}}{\partial Q_r} / (e u^{-0.5})$   |                    |                    |                    |
|--------------------------------------------------------------|--------------------|--------------------|--------------------|
|                                                              | -0.006 620 094 181 | -0.004 665 146 544 | -0.007 860 394 588 |
| $l$ -matrix coefficients/(u <sup>1/2</sup> Å <sup>-1</sup> ) |                    |                    |                    |
| O                                                            | -0.001 811 990 110 | -0.020 668 556 750 | 0.007 979 308 004  |
| C                                                            | 0.024 230 938 428  | -0.010 550 675 432 | -0.002 419 247 799 |
| C                                                            | 0.087 103 734 841  | -0.042 552 621 086 | -0.230 955 000 745 |
| C                                                            | 0.012 135 094 078  | -0.045 443 498 264 | 0.045 739 747 670  |
| C                                                            | -0.058 743 743 440 | 0.022 777 236 959  | 0.076 507 812 642  |
| C                                                            | 0.118 593 881 460  | 0.074 582 188 433  | -0.052 180 421 571 |
| C                                                            | 0.257 951 618 724  | -0.130 321 531 376 | -0.009 679 856 653 |
| C                                                            | -0.249 493 652 790 | 0.101 088 849 223  | -0.066 445 245 895 |
| C                                                            | -0.266 346 284 463 | -0.016 576 312 293 | 0.102 369 941 940  |
| C                                                            | 0.253 192 101 101  | 0.087 553 532 646  | -0.064 003 767 615 |
| C                                                            | -0.093 618 266 438 | -0.038 405 484 921 | 0.046 420 971 669  |
| H                                                            | -0.093 291 576 381 | -0.011 179 789 680 | 0.045 297 090 298  |
| H                                                            | -0.027 917 187 533 | -0.109 338 431 901 | -0.039 424 125 886 |
| H                                                            | -0.068 540 811 698 | -0.038 955 453 321 | 0.024 253 413 412  |
| H                                                            | 0.161 621 831 023  | 0.008 711 121 575  | -0.124 974 226 194 |
| H                                                            | 0.072 032 881 137  | -0.056 174 521 371 | -0.109 767 464 000 |
| H                                                            | -0.028 105 971 281 | 0.066 854 918 953  | 0.006 129 625 422  |
| H                                                            | -0.254 071 880 364 | -0.158 470 634 702 | -0.190 824 067 732 |
| H                                                            | 0.094 603 686 176  | -0.064 169 889 278 | 0.117 287 333 642  |
| H                                                            | -0.126 760 073 829 | 0.018 217 237 529  | -0.120 534 461 041 |
| H                                                            | -0.047 459 867 217 | 0.038 361 508 348  | 0.225 990 126 795  |
| H                                                            | 0.051 456 836 986  | 0.125 607 493 044  | 0.259 657 056 963  |
| H                                                            | 0.046 412 707 572  | 0.023 571 210 078  | -0.028 818 302 643 |
| H                                                            | 0.083 149 598 925  | -0.003 599 171 341 | -0.006 807 443 150 |
| H                                                            | -0.054 327 802 343 | 0.074 333 845 944  | 0.203 130 711 184  |
| H                                                            | 0.019 427 576 254  | 0.045 785 458 508  | 0.236 691 412 474  |
| H                                                            | -0.114 447 998 349 | 0.115 362 706 608  | 0.004 755 067 532  |

Wavenumber/cm<sup>-1</sup>: 1483.5381

| $\frac{\partial \mu_{x,y,z}}{\partial Q_r} / (e u^{-0.5})$        |                    |                    |                    |
|-------------------------------------------------------------------|--------------------|--------------------|--------------------|
|                                                                   | -0.001 663 620 993 | 0.007 463 097 908  | -0.001 797 213 231 |
| <i>l</i> -matrix coefficients/(u <sup>1/2</sup> Å <sup>-1</sup> ) |                    |                    |                    |
| O                                                                 | 0.032 655 856 231  | 0.024 357 856 848  | -0.010 050 896 729 |
| C                                                                 | -0.155 613 763 659 | 0.016 679 429 743  | -0.000 908 705 468 |
| C                                                                 | 0.028 796 102 340  | 0.060 005 648 691  | 0.055 700 988 081  |
| C                                                                 | 0.044 196 344 102  | 0.070 319 892 863  | 0.135 321 155 320  |
| C                                                                 | 0.256 492 669 639  | -0.365 110 771 163 | 0.023 423 835 313  |
| C                                                                 | -0.114 925 091 456 | 0.158 260 633 869  | -0.057 994 259 560 |
| C                                                                 | 0.031 384 282 896  | -0.270 480 654 398 | -0.084 318 161 690 |
| C                                                                 | -0.079 344 264 041 | 0.317 531 491 456  | 0.046 875 480 663  |
| C                                                                 | 0.044 577 962 621  | 0.085 876 270 955  | -0.017 386 181 176 |
| C                                                                 | -0.056 303 267 808 | 0.006 267 048 028  | -0.053 897 574 909 |
| C                                                                 | 0.050 756 533 558  | 0.004 576 782 873  | 0.154 277 203 170  |
| H                                                                 | -0.108 647 545 947 | 0.047 413 461 306  | 0.005 122 363 297  |
| H                                                                 | 0.085 424 193 907  | -0.116 635 395 255 | -0.028 950 264 631 |
| H                                                                 | 0.061 597 284 052  | -0.270 069 046 050 | -0.155 466 932 860 |
| H                                                                 | -0.048 514 938 921 | -0.048 291 802 724 | 0.063 618 068 058  |
| H                                                                 | -0.251 572 731 112 | 0.209 246 893 188  | -0.123 038 838 434 |
| H                                                                 | -0.099 093 019 990 | 0.036 781 273 549  | -0.031 495 580 534 |
| H                                                                 | 0.017 430 205 228  | -0.021 284 224 832 | 0.009 274 958 948  |
| H                                                                 | 0.037 741 737 683  | -0.148 278 420 392 | -0.088 918 715 134 |
| H                                                                 | -0.016 623 713 561 | 0.098 992 133 757  | 0.041 358 698 773  |
| H                                                                 | 0.091 898 105 374  | -0.052 734 322 603 | -0.132 449 066 525 |
| H                                                                 | 0.036 428 978 476  | -0.008 473 448 020 | 0.012 061 066 159  |
| H                                                                 | -0.155 045 827 820 | 0.123 166 483 754  | -0.043 727 699 610 |
| H                                                                 | 0.160 956 255 759  | -0.139 272 317 400 | -0.070 382 419 425 |
| H                                                                 | -0.056 870 067 392 | -0.042 097 279 339 | 0.034 497 332 197  |
| H                                                                 | -0.041 064 398 908 | -0.049 009 823 115 | -0.060 282 512 818 |
| H                                                                 | -0.016 807 584 744 | -0.006 208 052 074 | -0.085 348 940 751 |



Wavenumber/cm<sup>-1</sup>: 1489.0172

| $\frac{\partial \mu_{x,y,z}}{\partial Q_r} / (e u^{-0.5})$        | 0.013 035 319 946  | 0.003 885 384 950  | 0.003 260 093 398  |
|-------------------------------------------------------------------|--------------------|--------------------|--------------------|
| <i>l</i> -matrix coefficients/(u <sup>1/2</sup> Å <sup>-1</sup> ) |                    |                    |                    |
| O                                                                 | 0.062 442 647 022  | -0.008 954 051 445 | -0.021 472 181 471 |
| C                                                                 | -0.379 391 662 222 | 0.063 503 120 092  | 0.084 018 972 252  |
| C                                                                 | -0.210 474 064 285 | -0.213 209 126 648 | 0.004 853 001 229  |
| C                                                                 | 0.004 217 013 852  | 0.105 664 961 888  | -0.045 157 399 745 |
| C                                                                 | 0.337 008 199 406  | 0.092 250 354 308  | 0.030 938 716 568  |
| C                                                                 | 0.016 451 079 569  | 0.207 694 538 228  | 0.220 478 030 539  |
| C                                                                 | -0.039 739 847 657 | -0.006 916 920 826 | -0.122 601 578 748 |
| C                                                                 | -0.046 277 813 015 | -0.145 156 451 158 | -0.140 900 937 228 |
| C                                                                 | -0.001 085 922 761 | -0.144 556 917 515 | -0.138 972 468 282 |
| C                                                                 | 0.091 365 273 319  | 0.017 791 847 743  | 0.218 172 794 497  |
| C                                                                 | 0.094 938 997 612  | -0.043 802 357 614 | -0.048 078 810 866 |
| H                                                                 | -0.249 530 810 342 | 0.018 190 453 699  | 0.172 859 050 086  |
| H                                                                 | -0.036 901 150 327 | -0.015 060 632 068 | -0.043 652 521 428 |
| H                                                                 | 0.209 473 516 221  | 0.066 583 117 021  | -0.062 298 532 965 |
| H                                                                 | 0.162 831 376 854  | 0.023 620 161 928  | -0.172 244 015 758 |
| H                                                                 | -0.018 454 318 638 | -0.020 405 941 783 | -0.176 139 620 977 |
| H                                                                 | -0.056 244 944 536 | -0.019 577 217 334 | -0.084 402 594 570 |
| H                                                                 | 0.086 269 453 176  | 0.095 205 841 665  | 0.087 976 282 635  |
| H                                                                 | -0.043 273 370 800 | 0.077 132 459 944  | 0.027 794 993 731  |
| H                                                                 | -0.003 265 454 377 | -0.045 631 100 302 | -0.040 095 275 349 |
| H                                                                 | -0.060 402 139 661 | 0.045 508 624 184  | 0.153 472 902 710  |
| H                                                                 | -0.032 129 179 957 | -0.019 263 661 171 | -0.071 944 693 508 |
| H                                                                 | 0.059 863 105 680  | -0.044 366 032 203 | 0.012 156 654 386  |
| H                                                                 | -0.011 699 958 763 | 0.021 076 157 411  | 0.015 470 539 667  |
| H                                                                 | 0.075 992 950 074  | 0.046 532 249 620  | -0.023 617 225 014 |
| H                                                                 | 0.076 693 940 888  | 0.070 243 940 948  | 0.058 979 373 269  |
| H                                                                 | 0.051 075 212 431  | -0.033 740 025 533 | 0.014 618 610 028  |

Wavenumber/cm<sup>-1</sup>: 1490.0499

| $\frac{\partial \mu_{x,y,z}}{\partial Q_r} / (e u^{-0.5})$        | 0.004 395 486 945  | -0.000 573 556 740 | -0.002 477 629 255 |
|-------------------------------------------------------------------|--------------------|--------------------|--------------------|
| <i>l</i> -matrix coefficients/(u <sup>1/2</sup> Å <sup>-1</sup> ) |                    |                    |                    |
| O                                                                 | 0.040 556 219 775  | -0.036 975 586 000 | 0.031 836 982 659  |
| C                                                                 | -0.195 715 617 778 | -0.029 635 037 030 | -0.027 753 908 175 |
| C                                                                 | -0.195 664 148 945 | -0.078 069 058 061 | -0.025 426 451 887 |
| C                                                                 | 0.033 416 219 678  | 0.137 192 193 018  | 0.222 773 181 028  |
| C                                                                 | -0.312 058 934 562 | 0.111 008 239 973  | -0.022 064 864 459 |
| C                                                                 | 0.235 204 643 202  | -0.044 660 459 949 | -0.312 648 344 078 |
| C                                                                 | -0.078 881 861 865 | -0.078 110 093 778 | -0.190 681 931 486 |
| C                                                                 | 0.068 343 457 021  | 0.083 385 867 319  | 0.168 742 915 423  |
| C                                                                 | 0.036 345 662 654  | -0.079 886 583 153 | -0.144 952 071 161 |
| C                                                                 | 0.068 446 233 132  | 0.083 831 694 563  | 0.201 673 623 391  |
| C                                                                 | 0.126 348 214 669  | -0.036 288 244 140 | 0.131 523 114 326  |
| H                                                                 | 0.202 575 342 106  | -0.141 981 777 530 | -0.038 570 810 075 |
| H                                                                 | -0.037 465 752 072 | -0.039 670 155 974 | -0.061 695 168 390 |
| H                                                                 | -0.188 286 840 304 | 0.041 660 852 189  | 0.102 470 827 663  |
| H                                                                 | 0.110 353 831 122  | 0.007 883 125 137  | -0.119 607 057 695 |
| H                                                                 | 0.058 060 250 758  | -0.010 643 373 578 | -0.112 532 810 838 |
| H                                                                 | 0.143 105 473 537  | 0.031 464 262 764  | 0.148 701 349 228  |
| H                                                                 | 0.116 149 620 496  | 0.079 106 954 803  | 0.110 612 845 692  |
| H                                                                 | -0.010 340 587 538 | -0.041 640 710 310 | -0.005 764 903 507 |
| H                                                                 | 0.049 933 471 313  | 0.013 331 393 311  | 0.056 315 126 653  |
| H                                                                 | -0.018 744 106 558 | 0.021 002 134 805  | 0.056 581 385 084  |
| H                                                                 | 0.025 365 437 035  | -0.000 260 823 441 | -0.008 343 527 770 |
| H                                                                 | -0.154 710 455 920 | 0.117 110 203 223  | -0.051 613 997 541 |
| H                                                                 | 0.185 478 812 826  | -0.164 188 628 119 | -0.085 438 887 207 |
| H                                                                 | 0.048 016 899 835  | 0.024 998 135 708  | -0.020 027 709 768 |
| H                                                                 | 0.028 326 528 800  | 0.009 848 855 764  | -0.008 499 992 024 |
| H                                                                 | 0.020 073 035 315  | -0.038 094 430 278 | -0.093 519 259 750 |

Wavenumber/cm<sup>-1</sup>: 1495.1243

| $\frac{\partial \mu_{x,y,z}}{\partial Q_r} / (e u^{-0.5})$        | 0.011 131 874 072  | 0.001 283 466 326  | 0.003 261 115 695  |
|-------------------------------------------------------------------|--------------------|--------------------|--------------------|
| <i>l</i> -matrix coefficients/(u <sup>1/2</sup> Å <sup>-1</sup> ) |                    |                    |                    |
| O                                                                 | 0.000 160 378 464  | -0.034 211 513 869 | -0.006 258 466 562 |
| C                                                                 | -0.064 355 711 148 | 0.012 175 391 883  | 0.059 664 594 777  |
| C                                                                 | -0.113 933 922 400 | -0.072 889 458 763 | 0.014 967 523 441  |
| C                                                                 | -0.018 830 301 761 | 0.041 003 916 399  | -0.210 087 983 363 |
| C                                                                 | -0.210 368 833 990 | 0.012 166 673 353  | -0.329 852 965 772 |
| C                                                                 | -0.016 411 706 997 | -0.112 827 625 923 | 0.114 970 036 591  |
| C                                                                 | 0.278 631 639 039  | -0.143 907 190 372 | 0.261 325 824 339  |
| C                                                                 | -0.115 152 526 275 | 0.339 924 536 333  | 0.168 237 895 404  |
| C                                                                 | 0.032 904 666 696  | -0.048 454 909 037 | -0.098 316 643 667 |
| C                                                                 | 0.045 534 873 165  | 0.012 278 307 861  | 0.139 031 475 485  |
| C                                                                 | 0.011 880 535 755  | 0.004 041 793 718  | -0.138 868 917 565 |
| H                                                                 | 0.123 392 481 506  | -0.071 972 028 527 | 0.020 543 750 837  |
| H                                                                 | 0.195 467 597 503  | -0.155 622 534 917 | 0.047 240 662 033  |
| H                                                                 | -0.017 025 942 762 | -0.112 699 645 078 | -0.271 329 873 355 |
| H                                                                 | 0.064 052 884 699  | -0.003 496 225 898 | -0.068 594 593 731 |
| H                                                                 | -0.028 797 451 311 | 0.002 508 896 965  | 0.058 428 926 238  |
| H                                                                 | -0.055 639 879 043 | 0.165 136 352 884  | 0.012 941 057 216  |
| H                                                                 | 0.073 652 517 028  | 0.088 182 702 580  | 0.064 324 027 567  |
| H                                                                 | 0.071 725 094 111  | -0.025 929 932 313 | 0.001 690 097 909  |
| H                                                                 | 0.076 055 677 932  | 0.055 162 010 718  | 0.066 370 714 709  |
| H                                                                 | -0.004 082 744 553 | 0.006 052 324 887  | 0.017 984 618 441  |
| H                                                                 | -0.040 925 804 707 | -0.014 556 635 242 | -0.078 833 761 092 |
| H                                                                 | 0.147 141 019 704  | -0.121 390 544 115 | 0.053 300 335 299  |
| H                                                                 | -0.162 696 726 106 | 0.132 493 480 084  | 0.075 444 547 363  |
| H                                                                 | 0.027 335 238 182  | 0.009 102 144 996  | -0.013 648 925 895 |
| H                                                                 | 0.059 556 241 856  | 0.063 339 687 651  | 0.027 247 202 852  |
| H                                                                 | 0.057 337 378 312  | -0.030 209 329 703 | 0.077 168 560 915  |

Wavenumber/cm<sup>-1</sup>: 1501.1141

| $\frac{\partial \mu_{x,y,z}}{\partial Q_r} / (e u^{-0.5})$        | 0.013 772 538 713  | 0.001 276 454 097  | 0.000 914 771 265  |
|-------------------------------------------------------------------|--------------------|--------------------|--------------------|
| <i>l</i> -matrix coefficients/(u <sup>1/2</sup> Å <sup>-1</sup> ) |                    |                    |                    |
| O                                                                 | 0.043 597 356 971  | -0.064 725 561 975 | -0.058 565 748 872 |
| C                                                                 | -0.158 773 546 253 | 0.126 827 012 318  | 0.316 527 413 702  |
| C                                                                 | -0.077 848 879 446 | 0.135 070 528 825  | -0.016 396 397 721 |
| C                                                                 | -0.062 375 515 467 | -0.050 208 062 928 | -0.244 908 971 719 |
| C                                                                 | 0.132 684 718 998  | -0.238 092 200 036 | 0.275 293 359 650  |
| C                                                                 | 0.201 908 753 041  | -0.102 790 126 435 | -0.288 956 483 915 |
| C                                                                 | -0.104 038 054 299 | 0.168 404 647 713  | 0.112 873 965 276  |
| C                                                                 | -0.119 111 964 370 | -0.023 556 277 054 | 0.202 963 205 933  |
| C                                                                 | 0.048 838 217 357  | 0.032 757 514 437  | -0.148 891 353 095 |
| C                                                                 | -0.025 690 360 355 | 0.027 298 602 357  | -0.017 117 902 715 |
| C                                                                 | 0.002 870 960 156  | -0.036 873 559 680 | -0.066 773 862 095 |
| H                                                                 | 0.022 257 714 401  | 0.051 207 902 846  | -0.132 462 543 094 |
| H                                                                 | 0.113 625 689 189  | -0.031 788 864 748 | 0.017 852 011 668  |
| H                                                                 | 0.021 113 937 862  | -0.024 007 203 048 | 0.147 542 817 357  |
| H                                                                 | 0.084 649 390 728  | -0.075 170 066 697 | -0.051 796 986 055 |
| H                                                                 | 0.058 856 447 362  | -0.003 427 067 739 | -0.022 587 937 506 |
| H                                                                 | -0.014 358 948 040 | 0.290 103 254 944  | -0.014 525 886 753 |
| H                                                                 | -0.012 132 325 561 | -0.023 501 711 204 | -0.001 767 780 901 |
| H                                                                 | -0.083 335 691 043 | 0.157 278 775 011  | -0.038 944 568 003 |
| H                                                                 | 0.062 747 242 458  | -0.151 219 809 847 | -0.202 102 947 614 |
| H                                                                 | 0.113 436 822 296  | -0.055 616 572 077 | -0.094 789 659 185 |
| H                                                                 | 0.034 791 578 302  | 0.012 380 002 500  | 0.054 431 893 484  |
| H                                                                 | 0.109 108 095 503  | -0.050 792 771 564 | -0.001 039 401 506 |
| H                                                                 | -0.019 420 488 389 | 0.046 136 591 732  | 0.017 897 848 315  |
| H                                                                 | -0.052 938 189 139 | -0.016 585 167 679 | 0.117 799 926 712  |
| H                                                                 | -0.036 652 038 437 | -0.036 911 743 741 | -0.017 778 504 456 |
| H                                                                 | -0.017 826 404 861 | 0.035 717 922 958  | 0.025 440 632 629  |

Wavenumber/cm<sup>-1</sup>: 1501.6501

| $\frac{\partial \mu_{x,y,z}}{\partial Q_r} / (e u^{-0.5})$        | 0.002 785 605 128  | 0.000 339 277 072  | 0.012 026 569 331  |
|-------------------------------------------------------------------|--------------------|--------------------|--------------------|
| <i>l</i> -matrix coefficients/(u <sup>1/2</sup> Å <sup>-1</sup> ) |                    |                    |                    |
| O                                                                 | -0.089 523 475 058 | -0.114 473 466 966 | 0.037 753 074 797  |
| C                                                                 | 0.212 822 807 898  | -0.067 889 980 875 | 0.112 671 765 474  |
| C                                                                 | 0.011 868 256 519  | 0.122 236 487 280  | -0.034 479 046 193 |
| C                                                                 | 0.227 756 543 605  | 0.256 857 134 764  | -0.092 816 908 572 |
| C                                                                 | -0.049 287 804 184 | 0.084 701 068 791  | 0.100 660 599 617  |
| C                                                                 | 0.160 269 088 798  | -0.088 710 561 719 | 0.289 864 343 578  |
| C                                                                 | -0.170 972 673 726 | -0.244 082 971 985 | -0.349 347 796 615 |
| C                                                                 | -0.121 749 553 635 | -0.022 408 663 123 | 0.043 655 751 809  |
| C                                                                 | -0.039 703 031 036 | 0.034 777 863 600  | 0.027 130 591 740  |
| C                                                                 | -0.049 355 931 853 | -0.009 498 503 809 | -0.084 082 945 209 |
| C                                                                 | -0.055 489 656 258 | 0.202 103 924 676  | -0.019 568 047 728 |
| H                                                                 | 0.009 887 964 811  | -0.118 277 207 080 | 0.164 459 898 095  |
| H                                                                 | 0.068 623 574 707  | -0.168 720 727 204 | -0.126 179 171 647 |
| H                                                                 | 0.064 131 107 061  | 0.007 826 994 192  | -0.069 385 589 545 |
| H                                                                 | -0.002 892 912 938 | -0.022 275 783 572 | 0.016 731 933 524  |
| H                                                                 | 0.028 228 412 273  | -0.058 639 356 204 | -0.033 379 519 128 |
| H                                                                 | 0.067 047 694 425  | 0.166 891 920 089  | 0.041 779 978 980  |
| H                                                                 | -0.037 195 664 682 | -0.041 694 535 814 | -0.033 214 306 106 |
| H                                                                 | -0.097 659 629 911 | 0.036 065 701 140  | -0.115 303 813 532 |
| H                                                                 | 0.120 158 713 130  | -0.117 235 879 769 | -0.086 281 461 302 |
| H                                                                 | 0.020 068 068 324  | -0.015 654 867 197 | -0.024 771 700 645 |
| H                                                                 | 0.010 103 278 050  | 0.006 553 621 739  | 0.031 989 315 003  |
| H                                                                 | -0.191 876 674 983 | 0.027 250 567 337  | 0.054 478 645 571  |
| H                                                                 | -0.201 238 299 529 | 0.041 388 204 257  | 0.026 034 534 045  |
| H                                                                 | -0.037 646 937 980 | -0.000 123 109 932 | 0.065 346 593 203  |
| H                                                                 | -0.039 142 966 352 | -0.038 243 546 505 | -0.032 769 756 127 |
| H                                                                 | 0.140 577 681 646  | -0.174 467 834 028 | -0.008 159 002 727 |

Wavenumber/cm<sup>-1</sup>: 1508.3978

| $\frac{\partial \mu_{x,y,z}}{\partial Q_r} / (e u^{-0.5})$        | 0.006 765 021 698                    | 0.001 462 358 528  | 0.002 104 989 323  |
|-------------------------------------------------------------------|--------------------------------------|--------------------|--------------------|
| <i>l</i> -matrix coefficients/(u <sup>1/2</sup> Å <sup>-1</sup> ) |                                      |                    |                    |
| O                                                                 | -0.043 822 448 489                   | 0.039 458 467 755  | -0.048 142 336 814 |
| C                                                                 | 0.124 446 872 214                    | 0.100 615 617 285  | 0.111 600 735 809  |
| C                                                                 | 0.161 689 884 100                    | -0.201 172 934 999 | 0.075 469 862 934  |
| C                                                                 | -0.041 517 742 639                   | -0.049 027 525 365 | 0.138 204 019 927  |
| C                                                                 | 0.057 851 808 901                    | 0.235 146 968 250  | -0.172 935 009 121 |
| C                                                                 | 8.378 239 600 000 × 10 <sup>-5</sup> | 0.189 100 110 984  | -0.223 124 522 891 |
| C                                                                 | -0.144 152 015 473                   | -0.171 222 054 965 | 0.152 730 796 167  |
| C                                                                 | -0.064 974 759 604                   | -0.032 105 724 131 | 0.037 488 959 114  |
| C                                                                 | -0.067 539 311 095                   | -0.037 091 448 409 | 0.164 897 376 336  |
| C                                                                 | -0.045 142 798 177                   | -0.135 026 637 087 | -0.099 389 349 011 |
| C                                                                 | 0.042 330 280 647                    | -0.055 879 116 223 | 0.048 008 112 538  |
| H                                                                 | -0.088 272 778 219                   | 0.002 339 050 975  | 0.000 137 302 704  |
| H                                                                 | 0.322 242 287 382                    | 0.032 814 512 597  | 0.118 081 895 755  |
| H                                                                 | -0.035 748 398 778                   | 0.071 860 924 932  | 0.007 048 824 516  |
| H                                                                 | -0.069 219 346 628                   | 0.049 736 695 933  | 0.055 029 769 293  |
| H                                                                 | 0.068 473 852 229                    | -0.048 480 623 224 | -0.153 231 494 265 |
| H                                                                 | -0.071 898 709 047                   | 0.215 685 391 928  | -0.100 818 783 322 |
| H                                                                 | -0.071 995 116 626                   | 0.024 131 075 962  | -0.076 569 364 564 |
| H                                                                 | -0.115 364 250 973                   | 0.069 183 142 477  | -0.317 245 521 935 |
| H                                                                 | 0.236 996 263 915                    | -0.135 567 035 800 | -0.011 619 064 446 |
| H                                                                 | -0.098 682 187 001                   | 0.039 017 478 344  | 0.082 267 522 035  |
| H                                                                 | -0.125 502 223 671                   | -0.031 633 150 720 | -0.132 024 359 405 |
| H                                                                 | -0.024 885 386 319                   | 0.027 553 317 233  | -0.021 481 288 175 |
| H                                                                 | 0.096 365 598 794                    | -0.059 517 331 026 | -0.030 680 753 072 |
| H                                                                 | 0.038 218 395 900                    | 0.012 624 925 055  | -0.076 539 097 363 |
| H                                                                 | 0.056 974 453 478                    | 0.095 873 528 757  | 0.074 926 741 714  |
| H                                                                 | -0.022 768 251 522                   | 0.017 969 343 160  | -0.029 621 950 456 |

Wavenumber/cm<sup>-1</sup>: 1515.3603

| $\frac{\partial \mu_{x,y,z}}{\partial Q_r} / (e u^{-0.5})$   |                    |                    |                    |
|--------------------------------------------------------------|--------------------|--------------------|--------------------|
|                                                              | -0.000 528 121 740 | -0.001 566 150 130 | 0.003 279 874 547  |
| $l$ -matrix coefficients/(u <sup>1/2</sup> Å <sup>-1</sup> ) |                    |                    |                    |
| O                                                            | 0.030 657 290 907  | -0.065 444 927 536 | 0.175 815 798 483  |
| C                                                            | -0.068 159 943 171 | -0.325 805 980 286 | -0.516 775 061 315 |
| C                                                            | -0.090 278 994 246 | 0.183 418 342 976  | -0.097 712 755 999 |
| C                                                            | 0.046 593 693 931  | 0.070 206 286 757  | 0.046 438 574 333  |
| C                                                            | -0.011 527 549 555 | -0.046 203 471 624 | -0.022 183 053 121 |
| C                                                            | -0.030 554 878 596 | 0.063 767 131 460  | -0.013 325 740 246 |
| C                                                            | 0.056 550 985 577  | 0.072 957 933 107  | 0.270 009 638 384  |
| C                                                            | -0.053 607 768 207 | -0.184 926 988 611 | -0.045 050 317 729 |
| C                                                            | -0.069 929 572 836 | 0.044 177 187 195  | 0.037 080 453 242  |
| C                                                            | 0.123 022 990 167  | 0.156 355 005 193  | 0.161 850 394 641  |
| C                                                            | -0.007 207 815 433 | 0.032 266 020 784  | 0.006 959 038 751  |
| H                                                            | -0.025 402 110 248 | -0.067 929 496 530 | 0.063 747 558 879  |
| H                                                            | 0.226 373 062 942  | 0.091 316 724 073  | 0.128 078 491 197  |
| H                                                            | 0.028 975 943 628  | 0.041 140 993 365  | 0.015 724 413 995  |
| H                                                            | -0.028 702 731 167 | -0.016 296 155 441 | 0.027 798 873 507  |
| H                                                            | -0.079 775 663 177 | 0.034 310 644 360  | -0.119 814 845 752 |
| H                                                            | -0.039 417 407 966 | 0.141 011 908 593  | -0.093 336 457 359 |
| H                                                            | 0.097 429 107 683  | -0.014 687 751 551 | 0.094 951 093 125  |
| H                                                            | -0.040 436 597 387 | 0.121 160 845 659  | -0.153 237 872 202 |
| H                                                            | 0.077 954 359 493  | -0.144 360 285 084 | -0.137 663 709 744 |
| H                                                            | 0.016 784 550 591  | -0.021 927 783 847 | -0.045 062 339 540 |
| H                                                            | 0.149 626 579 162  | 0.031 838 943 636  | 0.136 757 566 469  |
| H                                                            | -0.057 896 114 340 | 0.004 857 579 924  | 0.013 505 699 085  |
| H                                                            | -0.029 593 439 312 | -0.002 805 490 916 | 0.001 329 932 455  |
| H                                                            | -0.055 559 021 776 | -0.013 248 845 493 | 0.049 551 455 783  |
| H                                                            | -0.035 857 985 959 | -0.096 891 697 650 | -0.071 406 512 065 |
| H                                                            | 0.036 155 691 037  | -0.055 313 085 638 | -0.015 199 817 905 |

Wavenumber/cm<sup>-1</sup>: 1531.7053

| $\frac{\partial \mu_{x,y,z}}{\partial Q_r} / (e u^{-0.5})$   |                    |                    |                    |
|--------------------------------------------------------------|--------------------|--------------------|--------------------|
|                                                              | -0.002 812 454 161 | 0.001 068 571 678  | -0.006 463 723 305 |
| $l$ -matrix coefficients/(u <sup>1/2</sup> Å <sup>-1</sup> ) |                    |                    |                    |
| O                                                            | 0.016 044 613 679  | -0.346 941 545 026 | 0.050 967 557 117  |
| C                                                            | 0.030 399 833 420  | -0.039 222 130 849 | 0.475 186 731 343  |
| C                                                            | -0.068 068 783 615 | 0.259 120 264 792  | -0.119 807 819 058 |
| C                                                            | 0.080 131 545 081  | 0.088 931 123 888  | 0.129 789 643 821  |
| C                                                            | -0.125 381 642 913 | 0.153 814 447 059  | -0.270 899 807 269 |
| C                                                            | -0.226 474 885 745 | 0.244 922 203 666  | -0.118 543 220 586 |
| C                                                            | 0.141 723 063 422  | -0.069 351 686 225 | 0.077 163 365 138  |
| C                                                            | 0.018 739 117 639  | -0.241 818 453 888 | -0.163 637 812 675 |
| C                                                            | 0.049 217 615 219  | 0.033 628 072 413  | -0.087 489 016 350 |
| C                                                            | -0.018 232 733 163 | 0.050 567 386 414  | -0.016 024 603 590 |
| C                                                            | 0.091 987 642 848  | -0.037 829 920 481 | 0.018 226 045 288  |
| H                                                            | -0.003 859 055 200 | 0.078 710 032 522  | -0.057 285 758 921 |
| H                                                            | -0.017 907 294 174 | -0.020 121 688 261 | 0.016 893 603 131  |
| H                                                            | -0.019 815 005 038 | 0.110 868 376 480  | -0.027 384 305 266 |
| H                                                            | 0.050 790 017 479  | -0.085 130 000 420 | -0.008 492 954 952 |
| H                                                            | -0.085 055 199 176 | 0.108 950 550 716  | 0.007 119 461 315  |
| H                                                            | -0.022 636 261 820 | -0.107 673 238 721 | -0.060 033 987 550 |
| H                                                            | -0.011 438 642 863 | -0.023 005 967 999 | -0.002 532 040 481 |
| H                                                            | 0.024 544 945 960  | 0.027 018 547 687  | 0.098 405 886 596  |
| H                                                            | 0.010 945 001 689  | -0.046 799 313 943 | 0.022 831 253 208  |
| H                                                            | 0.116 974 040 363  | -0.066 766 272 081 | -0.107 228 950 372 |
| H                                                            | 0.029 761 438 556  | 0.021 289 088 824  | 0.053 160 556 224  |
| H                                                            | -0.011 508 904 615 | -0.007 117 601 339 | 0.008 701 858 884  |
| H                                                            | 0.012 170 644 967  | -0.024 373 802 930 | 0.002 192 921 171  |
| H                                                            | -0.066 323 327 485 | -0.026 635 329 404 | 0.141 479 820 480  |
| H                                                            | -0.035 208 227 094 | -0.032 899 927 920 | -0.030 085 809 549 |
| H                                                            | 0.054 253 585 655  | -0.052 474 554 491 | 0.001 676 213 752  |



Wavenumber/cm<sup>-1</sup>: 1809.6997

| $\frac{\partial \mu_{x,y,z}}{\partial Q_r} / (e u^{-0.5})$        | -0.001 579 983 157 | -0.010 283 073 069 | 0.026 786 354 578  |
|-------------------------------------------------------------------|--------------------|--------------------|--------------------|
| <i>l</i> -matrix coefficients/(u <sup>1/2</sup> Å <sup>-1</sup> ) |                    |                    |                    |
| O                                                                 | -0.142 302 618 182 | -0.259 188 881 797 | 0.139 914 563 531  |
| C                                                                 | -0.027 513 780 061 | -0.230 748 627 241 | -0.000 178 867 530 |
| C                                                                 | -0.042 020 593 645 | -0.144 747 789 298 | 0.069 183 527 953  |
| C                                                                 | 0.110 632 733 738  | 0.258 658 562 148  | -0.178 175 614 842 |
| C                                                                 | 0.270 187 163 158  | 0.024 196 785 444  | -0.077 838 609 215 |
| C                                                                 | 0.163 447 011 670  | 0.052 303 040 805  | -0.346 605 612 539 |
| C                                                                 | 0.074 482 221 565  | 0.197 801 280 082  | 0.099 962 582 510  |
| C                                                                 | 0.103 622 968 852  | 0.123 129 253 671  | 0.123 528 314 259  |
| C                                                                 | -0.162 499 291 598 | 0.026 627 299 987  | 0.234 344 446 931  |
| C                                                                 | -0.090 683 299 373 | -0.100 682 626 572 | -0.124 078 438 807 |
| C                                                                 | -0.102 782 996 631 | 0.108 428 863 225  | -0.019 739 164 536 |
| H                                                                 | -0.011 536 722 085 | -0.042 160 435 756 | -0.041 992 487 881 |
| H                                                                 | -0.104 354 170 209 | -0.041 375 585 715 | -0.022 707 291 015 |
| H                                                                 | 0.049 951 778 476  | 0.009 952 380 502  | 0.010 313 592 016  |
| H                                                                 | -0.045 815 849 908 | 0.035 652 867 659  | 0.055 514 163 302  |
| H                                                                 | 0.029 040 606 558  | -0.006 475 898 151 | -0.197 240 644 930 |
| H                                                                 | -0.053 054 001 765 | -0.110 031 232 903 | 0.013 632 854 641  |
| H                                                                 | 0.007 103 308 839  | 0.010 826 129 377  | -0.022 603 515 871 |
| H                                                                 | 0.039 949 399 490  | 0.039 596 142 856  | 0.196 572 471 470  |
| H                                                                 | -0.046 839 793 531 | 0.117 366 655 570  | 0.152 775 805 758  |
| H                                                                 | -0.064 298 391 574 | 0.027 063 348 364  | 0.108 130 986 403  |
| H                                                                 | -0.038 177 200 372 | -0.046 426 962 146 | -0.097 149 284 635 |
| H                                                                 | -0.091 016 052 280 | 0.003 240 877 685  | 0.031 299 330 026  |
| H                                                                 | -0.129 844 797 859 | 0.042 891 191 704  | 0.023 846 647 065  |
| H                                                                 | -0.035 816 321 527 | 0.012 017 894 473  | 0.039 774 173 641  |
| H                                                                 | -0.015 529 068 138 | -0.019 980 258 435 | -0.048 299 505 240 |
| H                                                                 | 0.052 385 079 865  | -0.086 784 920 423 | -0.001 251 759 286 |

Wavenumber/cm<sup>-1</sup>: 3029.8643

| $\frac{\partial \mu_{x,y,z}}{\partial Q_r} / (e u^{-0.5})$        |                    |                    |                    |
|-------------------------------------------------------------------|--------------------|--------------------|--------------------|
|                                                                   | -0.054 054 043 648 | 0.025 618 125 535  | -0.009 878 753 870 |
| <i>l</i> -matrix coefficients/(u <sup>1/2</sup> Å <sup>-1</sup> ) |                    |                    |                    |
| O                                                                 | 0.128 192 046 920  | -0.093 779 624 023 | 0.069 863 416 572  |
| C                                                                 | -0.005 793 713 368 | -0.116 216 238 962 | -0.069 583 621 253 |
| C                                                                 | -0.180 948 706 813 | 0.173 678 145 741  | -0.083 309 522 360 |
| C                                                                 | 0.071 097 495 799  | -0.240 086 283 812 | -0.040 669 702 151 |
| C                                                                 | 0.015 766 425 450  | 0.308 701 196 969  | 0.064 231 903 041  |
| C                                                                 | -0.055 715 856 922 | -0.047 225 431 866 | 0.106 046 574 125  |
| C                                                                 | -0.151 754 902 145 | 0.098 613 485 831  | -0.056 943 957 541 |
| C                                                                 | -0.084 139 452 446 | 0.346 935 194 118  | 0.102 672 930 642  |
| C                                                                 | -0.085 871 237 512 | 0.044 412 530 551  | 0.105 838 405 316  |
| C                                                                 | -0.111 505 148 664 | -0.097 698 982 986 | -0.164 136 246 088 |
| C                                                                 | 0.393 084 468 389  | -0.309 353 971 921 | -0.054 998 467 194 |
| H                                                                 | -0.130 033 928 011 | 0.024 732 160 170  | 0.036 400 468 926  |
| H                                                                 | -0.037 245 342 559 | 0.065 506 897 138  | -0.002 265 757 015 |
| H                                                                 | 0.059 665 830 246  | 0.084 234 954 226  | -0.047 406 675 284 |
| H                                                                 | 0.034 536 672 250  | -0.019 352 085 213 | 0.007 194 564 120  |
| H                                                                 | 0.028 070 784 410  | -0.077 705 625 723 | -0.018 901 782 151 |
| H                                                                 | -0.024 700 508 084 | 0.059 845 294 463  | 0.043 893 180 956  |
| H                                                                 | 0.001 582 719 883  | -0.069 115 572 432 | -0.020 264 356 891 |
| H                                                                 | -0.039 307 132 413 | 0.014 637 444 779  | -0.034 215 252 752 |
| H                                                                 | -0.013 804 476 407 | 0.113 621 423 401  | 0.074 420 470 471  |
| H                                                                 | 0.009 198 922 099  | -0.003 982 038 639 | 0.033 374 651 459  |
| H                                                                 | 0.033 176 875 278  | -0.033 252 399 616 | 0.015 448 997 319  |
| H                                                                 | 0.140 530 032 748  | -0.090 420 347 686 | -0.020 829 842 335 |
| H                                                                 | 0.136 013 324 742  | -0.087 442 188 495 | -0.019 375 897 776 |
| H                                                                 | -0.052 194 422 300 | 0.014 137 103 886  | 0.126 040 474 365  |
| H                                                                 | -0.076 823 772 387 | -0.116 414 449 279 | -0.121 709 934 333 |
| H                                                                 | 0.096 438 214 031  | -0.063 796 390 442 | -0.016 526 323 149 |

Wavenumber/cm<sup>-1</sup>: 3031.7232

| $\frac{\partial \mu_{x,y,z}}{\partial Q_r} / (e u^{-0.5})$        |                    |                    |                    |
|-------------------------------------------------------------------|--------------------|--------------------|--------------------|
|                                                                   | -0.041 630 956 117 | 0.008 413 761 698  | -0.014 010 925 169 |
| <i>l</i> -matrix coefficients/(u <sup>1/2</sup> Å <sup>-1</sup> ) |                    |                    |                    |
| O                                                                 | 0.257 394 457 717  | -0.215 412 764 321 | 0.089 253 868 547  |
| C                                                                 | -0.104 927 879 205 | -0.148 137 507 462 | 0.033 044 900 401  |
| C                                                                 | 0.082 890 554 782  | 0.144 877 632 603  | -0.059 027 264 006 |
| C                                                                 | -0.375 590 038 246 | -0.144 455 407 064 | 0.037 155 022 028  |
| C                                                                 | 0.244 344 951 323  | 0.249 701 345 473  | -0.128 767 658 655 |
| C                                                                 | 0.092 194 468 808  | -0.078 991 833 906 | 0.003 317 646 183  |
| C                                                                 | -0.100 301 225 359 | -0.069 067 564 431 | -0.120 562 013 637 |
| C                                                                 | 0.060 534 211 703  | 0.129 029 690 678  | 0.082 606 257 815  |
| C                                                                 | 0.063 706 584 025  | -0.058 566 563 303 | -0.104 596 180 751 |
| C                                                                 | 0.041 247 195 312  | 0.008 366 406 369  | 0.114 755 761 091  |
| C                                                                 | -0.329 525 455 692 | 0.222 813 473 060  | 0.027 713 323 126  |
| H                                                                 | -0.010 180 733 710 | 0.008 544 832 488  | -0.011 438 699 845 |
| H                                                                 | 0.065 182 463 768  | 0.031 670 060 965  | -0.004 977 731 893 |
| H                                                                 | 0.086 213 074 428  | 0.065 682 698 122  | -0.060 026 985 037 |
| H                                                                 | -0.007 448 397 466 | -0.059 586 347 643 | 0.004 498 596 894  |
| H                                                                 | 0.150 936 108 559  | -0.124 221 308 189 | 0.045 078 517 642  |
| H                                                                 | -0.038 428 435 419 | -0.074 320 010 159 | 0.012 762 539 549  |
| H                                                                 | -0.021 548 388 202 | -0.052 358 838 360 | 0.021 202 418 061  |
| H                                                                 | -0.004 931 255 572 | -0.093 193 662 672 | -0.174 976 088 003 |
| H                                                                 | 0.022 120 160 378  | 0.085 440 646 568  | 0.156 546 208 603  |
| H                                                                 | 0.056 109 735 230  | -0.055 962 116 625 | -0.097 246 590 886 |
| H                                                                 | 0.048 291 197 464  | 0.015 843 405 191  | 0.113 348 634 338  |
| H                                                                 | -0.023 723 047 991 | 0.075 466 817 833  | -0.014 804 468 159 |
| H                                                                 | -0.033 358 483 352 | 0.065 154 208 036  | -0.006 253 775 704 |
| H                                                                 | -0.013 346 312 963 | -0.039 798 405 314 | 0.009 952 539 933  |
| H                                                                 | -0.016 292 247 412 | -0.037 668 482 566 | 0.028 586 114 038  |
| H                                                                 | -0.161 708 736 516 | 0.165 306 331 664  | 0.016 923 568 795  |

Wavenumber/cm<sup>-1</sup>: 3037.5697

| $\frac{\partial \mu_{x,y,z}}{\partial Q_r} / (e u^{-0.5})$        | -0.005 461 614 776 | 0.000 658 072 517  | 0.023 883 795 259  |
|-------------------------------------------------------------------|--------------------|--------------------|--------------------|
| <i>l</i> -matrix coefficients/(u <sup>1/2</sup> Å <sup>-1</sup> ) |                    |                    |                    |
| O                                                                 | -0.236 775 140 549 | -0.158 680 519 777 | 0.107 243 129 145  |
| C                                                                 | 0.154 252 558 676  | -0.181 560 290 004 | -0.011 829 847 212 |
| C                                                                 | 0.355 407 507 759  | -0.107 047 937 852 | -0.040 117 886 733 |
| C                                                                 | 0.051 275 752 457  | 0.016 051 587 440  | -0.069 876 978 147 |
| C                                                                 | -0.021 703 031 802 | 0.095 023 971 958  | 0.165 493 330 780  |
| C                                                                 | -0.259 574 664 673 | 0.063 310 747 199  | -0.065 199 114 333 |
| C                                                                 | -0.096 312 010 542 | 0.137 708 351 428  | 0.013 261 331 258  |
| C                                                                 | -0.061 524 180 828 | 0.203 194 670 111  | 0.103 545 569 638  |
| C                                                                 | 0.224 103 396 121  | -0.051 157 497 934 | -0.385 379 336 698 |
| C                                                                 | 0.050 317 971 575  | 0.070 780 786 627  | 0.173 462 665 581  |
| C                                                                 | 0.022 182 331 101  | -0.090 137 029 490 | 0.007 772 919 179  |
| H                                                                 | -0.203 693 372 963 | 0.001 816 512 016  | 0.032 738 385 847  |
| H                                                                 | -0.049 922 051 546 | 0.024 050 001 749  | -0.005 589 443 865 |
| H                                                                 | -0.083 517 787 002 | -0.014 173 430 365 | 0.082 720 082 179  |
| H                                                                 | -0.017 805 005 648 | 0.025 978 811 736  | -0.077 006 410 934 |
| H                                                                 | -0.075 602 139 785 | -0.029 788 102 523 | -0.125 747 050 227 |
| H                                                                 | -0.008 705 750 951 | 0.057 841 269 449  | 0.038 884 605 836  |
| H                                                                 | -0.110 133 891 205 | -0.031 782 474 785 | -0.017 546 574 226 |
| H                                                                 | -0.024 167 305 257 | 0.034 305 611 633  | 0.035 394 311 181  |
| H                                                                 | -0.025 065 165 031 | 0.057 668 432 767  | 0.016 865 802 793  |
| H                                                                 | 0.020 891 298 372  | 0.006 927 674 144  | -0.116 478 633 332 |
| H                                                                 | -0.022 519 847 081 | 0.054 918 206 876  | 0.109 953 288 060  |
| H                                                                 | -0.028 965 010 721 | -0.045 503 747 192 | 0.025 590 796 609  |
| H                                                                 | -0.052 487 713 614 | -0.017 876 807 415 | 0.020 504 508 720  |
| H                                                                 | 0.097 974 004 870  | -0.015 760 893 153 | -0.231 830 666 790 |
| H                                                                 | 0.029 287 776 361  | 0.080 452 200 800  | 0.156 296 540 396  |
| H                                                                 | 0.053 365 409 658  | -0.095 964 264 748 | 0.003 793 352 079  |

Wavenumber/cm<sup>-1</sup>: 3045.9823

| $\frac{\partial \mu_{x,y,z}}{\partial Q_r} / (e u^{-0.5})$        | 0.068 741 867 769  | 0.050 458 588 784  | 0.020 045 531 808  |
|-------------------------------------------------------------------|--------------------|--------------------|--------------------|
| <i>l</i> -matrix coefficients/(u <sup>1/2</sup> Å <sup>-1</sup> ) |                    |                    |                    |
| O                                                                 | -0.103 850 656 823 | -0.209 838 820 808 | 0.130 091 707 391  |
| C                                                                 | -0.037 939 415 886 | -0.214 908 862 435 | -0.012 853 618 621 |
| C                                                                 | 0.026 220 324 303  | -0.122 608 485 639 | 0.105 253 254 060  |
| C                                                                 | -0.035 936 713 256 | -0.116 646 821 848 | -0.100 138 453 699 |
| C                                                                 | -0.052 424 588 905 | -0.057 592 960 931 | 0.028 058 354 601  |
| C                                                                 | 0.267 628 330 029  | 0.417 435 634 254  | 0.111 402 672 356  |
| C                                                                 | -0.017 267 766 446 | 0.042 489 496 559  | -0.185 735 824 106 |
| C                                                                 | 0.013 354 304 737  | 0.138 261 934 953  | -0.195 453 910 689 |
| C                                                                 | -0.112 691 217 526 | -0.024 439 078 271 | 0.017 484 519 464  |
| C                                                                 | -0.050 426 593 675 | 0.027 750 831 991  | 0.099 114 552 572  |
| C                                                                 | 0.050 417 899 607  | -0.054 419 111 074 | 0.003 172 192 323  |
| H                                                                 | 0.244 345 621 650  | 0.307 839 609 648  | -0.155 952 204 476 |
| H                                                                 | 0.019 142 621 633  | 0.071 980 690 670  | -0.029 351 814 207 |
| H                                                                 | -0.050 097 023 782 | -0.060 854 494 293 | -0.003 304 612 000 |
| H                                                                 | -0.066 456 283 758 | 0.004 156 103 347  | 0.022 794 750 840  |
| H                                                                 | 0.086 573 333 449  | 0.241 286 710 922  | 0.323 809 830 518  |
| H                                                                 | 0.053 564 888 915  | 0.106 512 958 921  | -0.035 814 915 258 |
| H                                                                 | -0.021 215 317 177 | 0.039 964 031 880  | 0.016 910 181 114  |
| H                                                                 | 0.004 547 277 994  | -0.017 293 688 405 | -0.115 111 118 471 |
| H                                                                 | 0.015 316 726 650  | 0.002 458 033 050  | -0.141 741 868 507 |
| H                                                                 | -0.070 487 036 814 | 0.009 369 339 367  | -0.002 247 506 702 |
| H                                                                 | -0.029 301 726 012 | 0.002 725 897 243  | -0.004 696 141 808 |
| H                                                                 | 0.047 259 178 043  | -0.037 082 280 522 | 0.015 448 528 788  |
| H                                                                 | 0.004 409 467 037  | 0.009 219 891 081  | 0.017 949 399 348  |
| H                                                                 | -0.005 376 508 348 | 0.004 706 636 505  | -0.052 118 264 893 |
| H                                                                 | -0.004 342 319 530 | 0.034 951 202 068  | 0.064 328 107 228  |
| H                                                                 | 0.010 041 237 332  | -0.005 858 896 310 | 0.008 511 015 161  |

Wavenumber/cm<sup>-1</sup>: 3052.8313

| $\frac{\partial \mu_{x,y,z}}{\partial Q_r} / (e u^{-0.5})$        | 0.042 370 280 874  | 0.035 962 342 806  | -0.024 050 145 869 |
|-------------------------------------------------------------------|--------------------|--------------------|--------------------|
| <i>l</i> -matrix coefficients/(u <sup>1/2</sup> Å <sup>-1</sup> ) |                    |                    |                    |
| O                                                                 | -0.067 218 933 816 | 0.071 547 709 610  | -0.076 632 297 096 |
| C                                                                 | 0.092 347 474 571  | 0.088 923 475 166  | 0.030 673 721 050  |
| C                                                                 | 0.141 246 664 020  | 0.197 372 236 847  | 0.239 697 037 917  |
| C                                                                 | 0.101 403 083 449  | -0.075 830 548 463 | -0.134 516 798 351 |
| C                                                                 | 0.087 790 386 968  | 0.005 017 569 656  | -0.182 016 464 031 |
| C                                                                 | 0.137 400 679 095  | -0.104 002 223 596 | -0.146 031 177 031 |
| C                                                                 | -0.215 485 810 450 | -0.045 554 214 079 | -0.069 597 472 991 |
| C                                                                 | -0.290 795 003 310 | -0.081 936 688 862 | -0.045 701 778 437 |
| C                                                                 | -0.222 222 675 511 | -0.076 735 623 205 | 0.095 329 035 726  |
| C                                                                 | 0.218 993 292 589  | 0.230 874 170 971  | 0.308 436 341 775  |
| C                                                                 | 0.133 583 377 673  | -0.125 636 497 143 | -0.050 556 871 642 |
| H                                                                 | 0.046 656 420 008  | -0.027 013 846 765 | -0.046 466 280 647 |
| H                                                                 | -0.081 178 440 455 | -0.041 311 721 295 | -0.033 683 369 726 |
| H                                                                 | 0.021 619 942 376  | -0.037 729 170 582 | -0.090 836 059 656 |
| H                                                                 | -0.191 424 550 821 | -0.063 230 111 242 | 0.125 242 926 080  |
| H                                                                 | 0.042 732 974 034  | -0.029 631 744 103 | -0.035 425 206 728 |
| H                                                                 | -0.174 234 084 044 | -0.173 302 322 561 | -0.040 722 664 929 |
| H                                                                 | 0.063 655 057 083  | 0.082 608 584 098  | 0.088 039 337 451  |
| H                                                                 | -0.080 412 496 106 | 0.031 098 575 256  | 0.027 495 457 542  |
| H                                                                 | -0.117 216 655 358 | 0.047 863 448 703  | 0.137 154 700 947  |
| H                                                                 | -0.040 634 259 908 | -0.073 478 281 084 | -0.106 741 746 918 |
| H                                                                 | 0.057 092 310 286  | 0.064 192 576 336  | 0.070 488 419 480  |
| H                                                                 | 0.032 325 031 056  | -0.046 576 558 627 | -0.004 231 186 197 |
| H                                                                 | 0.025 785 453 718  | -0.026 197 178 660 | -0.006 398 165 372 |
| H                                                                 | -0.088 882 228 191 | -0.061 508 612 542 | -0.012 084 591 547 |
| H                                                                 | 0.068 590 290 912  | 0.077 657 498 026  | 0.095 762 554 751  |
| H                                                                 | 0.047 263 611 735  | -0.051 613 903 337 | -0.020 094 253 671 |

Wavenumber/cm<sup>-1</sup>: 3058.8245

| $\frac{\partial \mu_{x,y,z}}{\partial Q_r} / (e u^{-0.5})$        | -0.007 440 111 983 | -0.005 242 564 099 | -0.010 149 076 672 |
|-------------------------------------------------------------------|--------------------|--------------------|--------------------|
| <i>l</i> -matrix coefficients/(u <sup>1/2</sup> Å <sup>-1</sup> ) |                    |                    |                    |
| O                                                                 | -0.008 147 195 296 | 0.148 809 695 597  | -0.068 711 243 763 |
| C                                                                 | 0.019 437 693 973  | 0.127 554 089 782  | -0.028 628 830 071 |
| C                                                                 | -0.027 222 315 172 | 0.053 949 845 746  | -0.054 774 693 716 |
| C                                                                 | 0.093 704 415 095  | 0.085 644 139 539  | 0.069 304 060 438  |
| C                                                                 | 0.096 279 190 037  | 0.075 972 296 884  | -0.014 428 663 060 |
| C                                                                 | 0.086 733 026 815  | -0.009 380 663 442 | 0.018 783 583 842  |
| C                                                                 | 0.099 480 656 753  | 0.014 667 619 591  | 0.132 829 683 460  |
| C                                                                 | 0.280 904 848 798  | 0.123 508 125 966  | -0.095 346 101 168 |
| C                                                                 | -0.277 797 555 610 | -0.351 238 657 490 | -0.142 138 914 593 |
| C                                                                 | -0.287 494 051 286 | -0.125 649 721 546 | 0.209 575 230 755  |
| C                                                                 | 0.027 750 269 166  | -0.005 111 411 405 | -0.033 689 426 305 |
| H                                                                 | 0.007 994 142 904  | -0.039 157 205 625 | 0.035 851 281 103  |
| H                                                                 | -0.070 336 689 383 | -0.007 718 945 909 | 0.021 890 090 688  |
| H                                                                 | 0.056 794 435 004  | 0.042 761 542 550  | -0.011 399 388 738 |
| H                                                                 | -0.135 977 204 458 | -0.275 202 485 541 | 0.068 670 565 630  |
| H                                                                 | 0.019 855 047 576  | -0.015 656 057 546 | -0.034 143 315 225 |
| H                                                                 | 0.094 472 299 729  | 0.123 079 326 504  | -0.038 636 381 090 |
| H                                                                 | -0.155 174 231 385 | -0.171 033 831 575 | 0.036 303 811 573  |
| H                                                                 | 0.051 670 417 360  | -0.034 677 568 060 | 0.128 756 769 800  |
| H                                                                 | 0.135 475 034 330  | -0.014 947 243 264 | -0.094 720 606 811 |
| H                                                                 | -0.158 319 780 665 | -0.122 307 447 962 | -0.245 040 760 577 |
| H                                                                 | -0.113 272 224 001 | 0.021 910 046 829  | 0.197 861 893 352  |
| H                                                                 | -0.029 593 454 935 | 0.011 860 520 197  | -0.016 543 936 242 |
| H                                                                 | 0.022 951 502 440  | -0.017 094 043 315 | -0.022 338 835 761 |
| H                                                                 | -0.023 500 064 822 | -0.025 886 246 385 | 0.004 459 164 110  |
| H                                                                 | -0.070 333 367 843 | -0.017 456 760 265 | 0.058 237 513 643  |
| H                                                                 | 0.013 903 886 118  | -0.016 532 379 908 | -0.027 705 084 203 |

Wavenumber/cm<sup>-1</sup>: 3082.0013

| $\frac{\partial \mu_{x,y,z}}{\partial Q_r} / (e u^{-0.5})$        | -0.038 112 739 481 | -0.046 097 038 495 | 0.004 577 270 669  |
|-------------------------------------------------------------------|--------------------|--------------------|--------------------|
| <i>l</i> -matrix coefficients/(u <sup>1/2</sup> Å <sup>-1</sup> ) |                    |                    |                    |
| O                                                                 | -0.029 628 571 778 | 0.004 247 776 349  | 0.022 665 575 720  |
| C                                                                 | 0.027 224 520 188  | 0.004 801 196 573  | 0.038 820 879 983  |
| C                                                                 | 0.017 231 972 756  | -0.048 802 694 617 | -0.167 679 261 736 |
| C                                                                 | 0.110 326 522 837  | 0.052 886 547 425  | 0.254 858 204 353  |
| C                                                                 | 0.096 213 807 239  | -0.089 523 306 396 | -0.132 352 098 233 |
| C                                                                 | 0.282 495 149 323  | -0.032 485 378 453 | 0.183 364 173 248  |
| C                                                                 | 0.040 779 365 740  | 0.197 085 319 318  | 0.125 302 525 541  |
| C                                                                 | -0.265 986 754 971 | -0.072 737 355 295 | 0.089 092 831 438  |
| C                                                                 | 0.126 593 727 815  | 0.075 956 414 745  | -0.113 042 385 658 |
| C                                                                 | -0.298 137 813 495 | -0.017 912 445 488 | 0.046 565 449 432  |
| C                                                                 | -0.039 096 153 684 | -0.088 067 108 571 | -0.279 782 967 988 |
| H                                                                 | 0.141 864 942 428  | -0.032 018 078 342 | 0.048 833 791 435  |
| H                                                                 | 0.087 179 806 368  | 0.106 356 631 573  | 0.063 748 134 700  |
| H                                                                 | 0.065 155 575 786  | -0.032 982 917 866 | -0.084 119 731 682 |
| H                                                                 | 0.029 990 569 585  | 0.131 682 020 055  | -0.076 914 830 548 |
| H                                                                 | 0.092 932 747 052  | -0.004 716 619 207 | 0.085 694 699 408  |
| H                                                                 | -0.135 075 082 220 | -0.123 558 329 400 | 0.007 453 799 162  |
| H                                                                 | -0.153 681 079 633 | -0.046 083 825 205 | -0.024 391 127 882 |
| H                                                                 | -0.024 911 548 874 | 0.130 312 309 411  | -0.041 014 259 989 |
| H                                                                 | -0.148 053 675 413 | 0.040 879 835 147  | 0.101 820 866 152  |
| H                                                                 | 0.122 541 204 426  | 0.005 369 381 990  | 0.057 079 543 445  |
| H                                                                 | -0.111 418 101 258 | 0.018 963 690 144  | 0.058 690 054 292  |
| H                                                                 | -0.160 250 390 855 | 0.037 987 449 225  | -0.116 809 053 955 |
| H                                                                 | 0.097 152 546 765  | -0.101 238 071 068 | -0.149 890 414 307 |
| H                                                                 | -0.028 961 500 920 | -0.061 015 115 298 | -0.066 888 667 062 |
| H                                                                 | -0.074 162 224 987 | 0.029 674 819 728  | 0.064 699 025 777  |
| H                                                                 | -0.019 327 682 941 | -0.051 643 509 650 | -0.174 141 124 666 |



Wavenumber/cm<sup>-1</sup>: 3084.6769

| $\frac{\partial \mu_{x,y,z}}{\partial Q_r} / (e u^{-0.5})$        |                    |                    |                                       |
|-------------------------------------------------------------------|--------------------|--------------------|---------------------------------------|
|                                                                   | -0.034 589 553 037 | -0.020 169 151 404 | -0.014 976 178 531                    |
| <i>l</i> -matrix coefficients/(u <sup>1/2</sup> Å <sup>-1</sup> ) |                    |                    |                                       |
| O                                                                 | 0.154 347 648 963  | -0.186 022 123 681 | -0.008 630 532 729                    |
| C                                                                 | 0.029 592 006 767  | -0.063 775 897 725 | 0.178 822 026 118                     |
| C                                                                 | 0.029 119 384 401  | -0.055 696 104 705 | 0.134 393 661 953                     |
| C                                                                 | -0.036 699 501 407 | 0.031 002 181 857  | 0.210 966 258 717                     |
| C                                                                 | -0.027 777 453 186 | -0.061 353 350 625 | 0.029 578 651 282                     |
| C                                                                 | -0.059 519 653 897 | -0.156 691 711 554 | 0.126 336 212 699                     |
| C                                                                 | -0.107 341 097 810 | 0.180 194 418 064  | 0.120 572 728 516                     |
| C                                                                 | 0.035 390 012 575  | 0.234 639 161 612  | -0.239 623 297 200                    |
| C                                                                 | -0.056 180 514 640 | -0.086 950 821 232 | 0.069 500 754 728                     |
| C                                                                 | 0.232 620 679 938  | 0.216 941 171 117  | -0.167 207 620 795                    |
| C                                                                 | -0.181 458 819 170 | -0.078 145 065 768 | -0.259 873 780 190                    |
| H                                                                 | -0.003 766 996 669 | -0.092 302 257 842 | 0.069 132 160 108                     |
| H                                                                 | -0.116 188 429 859 | 0.099 938 472 320  | 0.042 748 384 300                     |
| H                                                                 | -0.028 197 612 817 | -0.065 911 453 891 | -0.022 899 088 882                    |
| H                                                                 | -0.002 203 605 093 | -0.125 524 290 893 | 0.055 428 888 426                     |
| H                                                                 | -0.015 522 622 898 | -0.063 531 029 761 | -5.900 558 900 000 × 10 <sup>-5</sup> |
| H                                                                 | 0.020 126 962 657  | 0.183 636 690 323  | -0.093 828 061 299                    |
| H                                                                 | 0.123 671 745 837  | 0.136 344 864 354  | -0.023 342 539 759                    |
| H                                                                 | -0.015 348 051 921 | 0.023 911 905 209  | 0.089 938 763 280                     |
| H                                                                 | 0.054 556 961 379  | 0.007 610 598 309  | -0.174 311 465 656                    |
| H                                                                 | -0.106 297 070 637 | -0.001 706 639 704 | -0.051 980 825 063                    |
| H                                                                 | 0.026 410 841 474  | 0.040 233 481 004  | -0.161 771 959 972                    |
| H                                                                 | -0.177 212 897 624 | 0.047 480 776 400  | -0.121 543 553 834                    |
| H                                                                 | 0.015 706 668 702  | -0.110 969 488 817 | -0.141 754 521 784                    |
| H                                                                 | 0.052 910 663 589  | 0.059 497 838 112  | 0.048 273 361 341                     |
| H                                                                 | 0.095 790 436 366  | 0.100 520 022 466  | -0.054 423 852 047                    |
| H                                                                 | -0.048 308 851 291 | -0.050 985 615 426 | -0.127 581 476 444                    |

Wavenumber/cm<sup>-1</sup>: 3091.6317

| $\frac{\partial \mu_{x,y,z}}{\partial Q_r} / (e u^{-0.5})$        | 0.018 292 571 615  | -0.030 882 491 641 | 0.006 160 234 707  |
|-------------------------------------------------------------------|--------------------|--------------------|--------------------|
| <i>l</i> -matrix coefficients/(u <sup>1/2</sup> Å <sup>-1</sup> ) |                    |                    |                    |
| O                                                                 | -0.688 232 972 076 | 0.051 322 492 091  | 0.002 998 529 447  |
| C                                                                 | -0.127 762 450 077 | 0.026 427 861 663  | 0.029 317 520 281  |
| C                                                                 | 0.039 803 520 142  | 0.063 653 512 072  | -0.028 124 894 995 |
| C                                                                 | -0.027 201 232 933 | -0.043 621 607 377 | 0.081 519 143 836  |
| C                                                                 | 0.037 751 179 694  | 0.049 893 953 126  | -0.035 603 115 380 |
| C                                                                 | 0.036 290 274 448  | -0.035 667 819 407 | 0.049 220 799 825  |
| C                                                                 | 0.059 769 668 313  | 0.087 657 851 325  | -0.053 450 579 467 |
| C                                                                 | 0.005 684 081 000  | 0.056 502 219 994  | -0.022 061 489 381 |
| C                                                                 | 0.218 316 454 594  | -0.204 339 096 490 | 0.149 009 903 566  |
| C                                                                 | 0.232 997 327 392  | -0.165 455 792 652 | -0.033 261 946 742 |
| C                                                                 | 0.089 403 336 216  | 0.157 943 581 025  | -0.119 145 341 585 |
| H                                                                 | 0.019 153 921 784  | -0.007 239 560 189 | 0.009 884 552 133  |
| H                                                                 | 0.068 689 236 930  | 0.069 841 227 103  | 0.007 460 273 544  |
| H                                                                 | 0.024 683 360 708  | 0.013 178 702 678  | -0.025 980 465 252 |
| H                                                                 | 0.131 525 432 536  | -0.184 653 998 485 | 0.053 342 590 423  |
| H                                                                 | 0.034 850 011 643  | -0.027 858 413 940 | 0.028 377 643 555  |
| H                                                                 | -0.005 806 906 202 | -0.010 486 076 926 | -0.003 922 997 649 |
| H                                                                 | 0.122 259 478 204  | -0.097 827 257 965 | 0.032 625 041 818  |
| H                                                                 | 0.013 136 279 440  | 0.025 718 251 802  | -0.085 932 925 260 |
| H                                                                 | -0.013 913 224 257 | 0.029 457 615 350  | 0.009 040 522 622  |
| H                                                                 | 0.050 580 037 197  | -0.075 107 009 344 | -0.036 529 468 228 |
| H                                                                 | 0.077 289 932 545  | -0.035 448 590 924 | 0.035 725 196 642  |
| H                                                                 | 0.046 023 767 000  | 0.076 775 318 450  | -0.067 589 494 142 |
| H                                                                 | 0.096 624 259 809  | 0.017 697 405 738  | -0.065 175 716 368 |
| H                                                                 | 0.078 307 422 631  | -0.002 157 502 768 | 0.175 856 566 110  |
| H                                                                 | 0.067 038 862 566  | -0.082 182 105 081 | -0.099 612 849 639 |
| H                                                                 | -0.019 016 432 756 | 0.110 001 377 382  | -0.039 648 373 444 |

Wavenumber/cm<sup>-1</sup>: 3094.3547

| $\frac{\partial \mu_{x,y,z}}{\partial Q_r} / (e u^{-0.5})$        | 0.038 235 725 292  | -0.019 811 949 978 | 0.039 931 716 789  |
|-------------------------------------------------------------------|--------------------|--------------------|--------------------|
| <i>l</i> -matrix coefficients/(u <sup>1/2</sup> Å <sup>-1</sup> ) |                    |                    |                    |
| O                                                                 | -0.133 428 067 164 | -0.186 045 783 898 | 0.022 513 317 319  |
| C                                                                 | -0.026 072 069 139 | -0.121 819 069 397 | 0.117 488 261 757  |
| C                                                                 | -0.045 206 666 342 | -0.023 960 631 680 | 0.072 385 268 508  |
| C                                                                 | 0.033 207 575 876  | -0.087 936 611 341 | 0.081 534 209 472  |
| C                                                                 | 0.028 242 739 618  | -0.087 913 476 529 | 0.070 706 698 866  |
| C                                                                 | -0.080 214 710 228 | -0.234 876 625 014 | 0.042 239 771 563  |
| C                                                                 | 0.189 210 997 501  | 0.032 239 075 469  | -0.097 312 812 866 |
| C                                                                 | 0.106 944 805 160  | -0.048 426 598 322 | -0.004 316 684 448 |
| C                                                                 | -0.281 369 861 249 | 0.069 287 382 062  | -0.114 301 496 551 |
| C                                                                 | -0.121 177 290 427 | 0.215 278 471 392  | -0.024 920 075 392 |
| C                                                                 | 0.324 352 200 591  | 0.332 423 138 516  | -0.057 711 368 025 |
| H                                                                 | -0.056 409 451 779 | -0.103 825 880 889 | 0.048 327 049 239  |
| H                                                                 | 0.128 520 732 425  | 0.053 782 232 656  | -0.001 991 641 132 |
| H                                                                 | 0.014 250 599 248  | -0.022 378 976 206 | 0.017 034 675 093  |
| H                                                                 | -0.158 925 090 502 | 0.126 497 117 331  | -0.027 079 503 168 |
| H                                                                 | -0.019 763 589 922 | -0.095 710 126 869 | -0.043 983 014 456 |
| H                                                                 | 0.046 928 114 498  | -0.025 064 268 278 | 0.015 345 762 261  |
| H                                                                 | -0.080 923 700 558 | 0.177 835 849 670  | -0.053 098 290 383 |
| H                                                                 | 0.048 094 938 018  | 0.013 111 678 247  | -0.117 481 717 562 |
| H                                                                 | 0.003 540 009 204  | -0.005 415 708 642 | -0.013 354 426 941 |
| H                                                                 | -0.040 125 793 396 | 0.010 795 216 793  | 0.008 222 804 995  |
| H                                                                 | 0.004 466 956 989  | 0.018 819 020 192  | -0.090 475 141 848 |
| H                                                                 | 0.214 578 134 007  | 0.158 139 115 313  | -0.096 638 310 463 |
| H                                                                 | 0.141 480 439 902  | 0.038 200 828 254  | -0.060 628 383 031 |
| H                                                                 | -0.115 261 053 333 | -0.050 606 390 627 | -0.139 712 023 192 |
| H                                                                 | -0.065 680 086 060 | 0.062 550 044 370  | 0.104 393 615 671  |
| H                                                                 | 0.025 247 287 594  | 0.231 585 803 574  | 0.065 272 053 766  |

Wavenumber/cm<sup>-1</sup>: 3098.1798

| $\frac{\partial \mu_{x,y,z}}{\partial Q_r} / (e u^{-0.5})$        | 0.035 047 587 668  | -0.027 531 148 391 | -0.007 298 570 414 |
|-------------------------------------------------------------------|--------------------|--------------------|--------------------|
| <i>l</i> -matrix coefficients/(u <sup>1/2</sup> Å <sup>-1</sup> ) |                    |                    |                    |
| O                                                                 | 0.106 807 273 806  | -0.064 500 520 915 | -0.025 920 692 585 |
| C                                                                 | 0.011 006 922 078  | -0.036 594 371 568 | 0.005 560 084 105  |
| C                                                                 | -0.020 694 374 817 | -0.069 408 409 834 | 0.005 679 274 643  |
| C                                                                 | 0.017 368 826 020  | 0.016 383 780 394  | 0.005 289 548 736  |
| C                                                                 | -0.036 809 942 749 | -0.064 827 060 087 | 0.026 464 016 859  |
| C                                                                 | -0.033 467 333 327 | -0.038 717 750 390 | -0.015 348 659 320 |
| C                                                                 | 0.147 549 190 855  | 0.145 947 592 987  | -0.168 111 938 873 |
| C                                                                 | -0.115 550 725 931 | -0.056 560 599 614 | 0.057 860 418 806  |
| C                                                                 | -0.001 543 202 822 | -0.028 254 127 083 | 0.033 477 951 455  |
| C                                                                 | -0.082 073 702 690 | 0.154 756 849 311  | -0.068 631 361 974 |
| C                                                                 | 0.017 887 721 835  | -0.012 320 926 556 | 0.145 006 377 703  |
| H                                                                 | -0.020 105 416 069 | -0.012 400 843 862 | 0.000 961 126 722  |
| H                                                                 | 0.167 823 281 884  | 0.077 521 024 881  | -0.020 657 788 083 |
| H                                                                 | -0.019 805 048 373 | -0.026 739 011 811 | 0.010 111 278 593  |
| H                                                                 | 0.045 561 722 899  | -0.209 675 299 585 | 0.062 748 418 810  |
| H                                                                 | -0.018 655 778 272 | -0.006 072 062 956 | -0.013 685 648 601 |
| H                                                                 | -0.039 237 082 597 | -0.107 277 497 657 | 0.041 334 824 275  |
| H                                                                 | 0.083 740 244 323  | -0.304 641 035 956 | 0.101 792 835 719  |
| H                                                                 | 0.017 609 399 252  | 0.084 560 008 410  | -0.173 274 199 008 |
| H                                                                 | -0.110 363 823 333 | 0.034 928 826 986  | 0.057 339 448 172  |
| H                                                                 | -0.173 493 780 256 | 0.043 522 005 839  | -0.108 598 704 201 |
| H                                                                 | -0.396 267 473 362 | 0.219 442 435 738  | 0.080 945 722 886  |
| H                                                                 | 0.058 369 844 970  | 0.036 469 813 493  | -0.005 140 838 836 |
| H                                                                 | -0.077 793 440 642 | -0.051 504 751 853 | 0.032 185 970 486  |
| H                                                                 | 0.132 592 312 801  | 0.158 179 209 714  | 0.078 869 209 855  |
| H                                                                 | 0.223 665 601 048  | 0.287 939 758 750  | -0.278 911 568 109 |
| H                                                                 | 0.033 348 458 154  | -0.003 195 140 765 | 0.143 198 321 614  |

Wavenumber/cm<sup>-1</sup>: 3100.1553

| $\frac{\partial \mu_{x,y,z}}{\partial Q_r} / (e u^{-0.5})$        | -0.004 320 683 364 | -0.009 610 535 976 | 0.011 122 572 740  |
|-------------------------------------------------------------------|--------------------|--------------------|--------------------|
| <i>l</i> -matrix coefficients/(u <sup>1/2</sup> Å <sup>-1</sup> ) |                    |                    |                    |
| O                                                                 | -0.001 467 550 323 | -0.000 763 136 896 | 0.211 690 466 750  |
| C                                                                 | 0.005 712 792 430  | -0.104 063 963 590 | -0.043 787 713 915 |
| C                                                                 | 0.020 338 293 106  | -0.027 477 524 560 | -0.027 913 695 016 |
| C                                                                 | -0.020 248 160 717 | -0.069 484 573 959 | -0.067 151 694 915 |
| C                                                                 | 0.020 377 270 415  | -0.037 957 585 924 | -0.046 969 671 317 |
| C                                                                 | 0.029 116 625 922  | 0.002 452 272 695  | -0.018 318 543 805 |
| C                                                                 | -0.294 602 185 867 | -0.270 774 920 270 | 0.211 920 915 775  |
| C                                                                 | 0.002 213 023 306  | -0.060 934 802 102 | -0.034 625 916 580 |
| C                                                                 | 0.090 083 345 550  | 0.177 344 130 715  | -0.007 793 773 266 |
| C                                                                 | -0.064 960 488 715 | 0.036 919 990 236  | 0.010 573 213 731  |
| C                                                                 | 0.194 135 750 544  | 0.258 488 113 609  | -0.202 713 283 885 |
| H                                                                 | 0.017 838 791 839  | 0.013 137 184 098  | -0.017 948 081 962 |
| H                                                                 | -0.234 486 201 609 | -0.146 110 986 547 | 0.018 347 729 178  |
| H                                                                 | 0.003 373 206 857  | -0.011 860 607 103 | -0.011 617 363 106 |
| H                                                                 | 0.056 430 636 986  | 0.022 155 418 587  | -0.010 385 091 704 |
| H                                                                 | 0.013 049 454 210  | 0.005 089 735 702  | 0.014 122 629 253  |
| H                                                                 | -0.011 866 222 040 | 0.063 618 256 075  | -0.044 756 879 418 |
| H                                                                 | 0.031 207 050 004  | -0.201 721 624 797 | 0.066 860 300 650  |
| H                                                                 | -0.059 594 960 954 | -0.114 136 051 524 | 0.229 789 175 861  |
| H                                                                 | 0.082 395 798 640  | -0.063 720 903 635 | -0.032 550 455 163 |
| H                                                                 | -0.038 166 575 975 | 0.087 405 141 596  | 0.010 620 126 800  |
| H                                                                 | -0.219 464 123 123 | 0.112 885 124 368  | 0.084 533 391 060  |
| H                                                                 | 0.047 486 670 715  | -0.013 912 078 184 | 0.027 603 874 944  |
| H                                                                 | 0.227 486 384 405  | 0.189 496 143 195  | -0.029 589 925 238 |
| H                                                                 | 0.074 906 407 010  | 0.105 515 502 484  | -0.003 966 618 889 |
| H                                                                 | 0.114 312 984 977  | 0.137 820 196 880  | -0.143 333 462 800 |
| H                                                                 | -0.037 500 739 585 | 0.147 005 760 940  | -0.218 280 106 977 |

Wavenumber/cm<sup>-1</sup>: 3101.9745

| $\frac{\partial \mu_{x,y,z}}{\partial Q_r} / (e u^{-0.5})$   |                    |                    |                    |
|--------------------------------------------------------------|--------------------|--------------------|--------------------|
|                                                              | -0.034 652 940 719 | -0.018 744 446 107 | -0.001 508 715 967 |
| $l$ -matrix coefficients/(u <sup>1/2</sup> Å <sup>-1</sup> ) |                    |                    |                    |
| O                                                            | -0.015 454 759 771 | 0.122 919 561 606  | 0.220 117 839 524  |
| C                                                            | -0.011 741 385 678 | -0.002 146 283 152 | -0.053 219 938 868 |
| C                                                            | -0.005 379 954 542 | -0.005 232 222 758 | -0.063 347 262 312 |
| C                                                            | -0.010 393 081 305 | -0.014 086 250 998 | -0.029 779 309 327 |
| C                                                            | 0.008 731 649 833  | 0.015 469 651 157  | -0.035 145 162 305 |
| C                                                            | 0.006 751 117 568  | -0.034 618 426 713 | -0.046 342 964 497 |
| C                                                            | -0.035 885 422 574 | 0.001 111 904 342  | -0.030 732 324 337 |
| C                                                            | 0.043 194 382 280  | 0.048 164 020 001  | -0.097 982 669 469 |
| C                                                            | 0.147 843 623 960  | -0.419 026 523 718 | 0.117 376 902 898  |
| C                                                            | -0.140 896 258 247 | 0.331 539 260 341  | -0.157 310 599 682 |
| C                                                            | 0.003 329 793 385  | -0.023 862 401 922 | 0.136 535 551 618  |
| H                                                            | -0.005 677 823 108 | -0.012 798 247 314 | -0.008 829 057 932 |
| H                                                            | -0.035 196 910 428 | 0.002 096 930 146  | -0.011 129 030 988 |
| H                                                            | 0.006 692 308 991  | 0.000 787 402 651  | -0.017 583 966 422 |
| H                                                            | 0.021 559 345 711  | 0.109 055 119 341  | -0.047 952 401 921 |
| H                                                            | 0.002 221 569 472  | -0.013 198 925 596 | -0.021 349 466 292 |
| H                                                            | 0.016 921 638 014  | 0.046 345 587 322  | -0.033 790 311 399 |
| H                                                            | -0.037 448 619 583 | 0.057 633 889 706  | -0.037 528 250 201 |
| H                                                            | -0.001 793 584 676 | -0.015 528 789 881 | 0.010 492 408 813  |
| H                                                            | 0.030 556 382 246  | -0.002 181 312 925 | -0.050 273 201 019 |
| H                                                            | 0.349 241 653 800  | -0.239 167 483 433 | 0.153 823 295 749  |
| H                                                            | -0.159 168 736 264 | 0.127 977 056 589  | -0.081 823 683 112 |
| H                                                            | 0.004 796 349 077  | -0.062 086 221 674 | 0.092 187 340 774  |
| H                                                            | 0.004 923 320 120  | 0.058 849 987 793  | 0.076 821 384 211  |
| H                                                            | -0.188 334 233 080 | -0.371 026 934 458 | 0.047 188 292 661  |
| H                                                            | 0.034 983 885 905  | 0.197 106 443 660  | -0.049 188 294 001 |
| H                                                            | -0.001 877 458 427 | -0.019 111 268 030 | -0.000 697 147 979 |

Wavenumber/cm<sup>-1</sup>: 3108.1296

| $\frac{\partial \mu_{x,y,z}}{\partial Q_r} / (e u^{-0.5})$        |                    |                    |                    |
|-------------------------------------------------------------------|--------------------|--------------------|--------------------|
|                                                                   | -0.007 275 440 439 | -0.001 821 341 506 | -0.006 861 513 800 |
| <i>l</i> -matrix coefficients/(u <sup>1/2</sup> Å <sup>-1</sup> ) |                    |                    |                    |
| O                                                                 | -0.006 488 449 240 | 0.009 562 857 691  | 0.004 123 482 382  |
| C                                                                 | 0.004 111 423 651  | 0.008 447 444 251  | -0.008 675 075 846 |
| C                                                                 | 0.014 981 570 323  | 0.021 174 053 797  | 0.028 102 492 384  |
| C                                                                 | -0.000 779 883 401 | 0.004 174 803 520  | -0.026 868 279 036 |
| C                                                                 | 0.002 848 850 040  | 0.018 965 420 569  | -0.023 308 475 921 |
| C                                                                 | 0.014 745 318 667  | 0.037 081 773 038  | -0.008 993 257 537 |
| C                                                                 | -0.108 519 323 846 | -0.070 631 227 820 | 0.083 370 641 062  |
| C                                                                 | 0.033 739 747 277  | 0.037 419 072 600  | -0.060 495 799 086 |
| C                                                                 | 0.016 339 900 903  | 0.060 618 432 727  | 0.020 580 923 827  |
| C                                                                 | 0.043 987 151 918  | -0.106 406 012 207 | 0.082 740 902 603  |
| C                                                                 | -0.013 882 208 515 | 0.001 837 453 450  | -0.092 723 506 454 |
| H                                                                 | 0.011 722 071 189  | 0.011 281 177 144  | -0.005 496 371 029 |
| H                                                                 | -0.101 240 180 684 | -0.035 908 493 982 | 0.010 228 591 070  |
| H                                                                 | -0.001 324 282 889 | 0.000 242 488 095  | -0.009 617 781 548 |
| H                                                                 | -0.025 902 088 382 | 0.188 792 432 676  | -0.045 936 641 342 |
| H                                                                 | 0.002 356 085 854  | 0.015 371 010 643  | 0.002 276 319 811  |
| H                                                                 | 0.013 420 252 857  | 0.069 192 583 798  | -0.032 776 581 959 |
| H                                                                 | 0.052 389 463 525  | -0.166 501 220 530 | 0.069 985 665 397  |
| H                                                                 | -0.019 300 119 583 | -0.039 380 587 239 | 0.095 322 330 414  |
| H                                                                 | 0.054 211 389 617  | -0.020 388 509 491 | -0.044 889 261 965 |
| H                                                                 | 0.140 861 458 125  | -0.018 180 785 439 | 0.116 917 704 287  |
| H                                                                 | -0.074 740 894 890 | 0.027 935 031 809  | 0.098 317 769 934  |
| H                                                                 | 0.164 450 095 058  | 0.324 109 919 050  | -0.364 450 913 221 |
| H                                                                 | -0.285 297 864 417 | -0.381 911 941 408 | -0.187 499 107 532 |
| H                                                                 | -0.100 098 469 690 | -0.115 737 098 786 | -0.054 961 558 627 |
| H                                                                 | 0.073 367 751 686  | 0.010 548 483 680  | -0.084 480 321 018 |
| H                                                                 | 0.094 835 538 975  | 0.048 661 001 250  | 0.442 273 845 671  |

Wavenumber/cm<sup>-1</sup>: 3115.514

| $\frac{\partial \mu_{x,y,z}}{\partial Q_r} / (e u^{-0.5})$        |                    |                    |                    |
|-------------------------------------------------------------------|--------------------|--------------------|--------------------|
|                                                                   | -0.029 015 746 432 | -0.009 576 141 458 | 0.001 011 771 334  |
| <i>l</i> -matrix coefficients/(u <sup>1/2</sup> Å <sup>-1</sup> ) |                    |                    |                    |
| O                                                                 | -0.047 732 842 683 | -0.155 466 527 591 | -0.365 564 705 374 |
| C                                                                 | -0.014 287 664 215 | 0.028 720 783 352  | 0.056 934 140 636  |
| C                                                                 | -0.011 426 999 986 | 0.055 615 962 526  | 0.118 356 101 343  |
| C                                                                 | -0.012 031 917 539 | 0.021 954 524 711  | 0.059 816 591 088  |
| C                                                                 | -0.011 826 983 844 | 0.043 392 614 801  | 0.081 511 151 103  |
| C                                                                 | -0.045 548 505 429 | 0.005 166 766 994  | 0.051 043 027 615  |
| C                                                                 | 0.096 389 428 305  | 0.067 169 132 469  | -0.013 566 300 822 |
| C                                                                 | 0.095 328 775 475  | 0.076 895 671 598  | 0.006 292 274 809  |
| C                                                                 | -0.181 345 144 123 | 0.088 636 182 846  | -0.022 151 201 348 |
| C                                                                 | 0.180 303 642 703  | -0.165 681 272 296 | 0.097 860 097 667  |
| C                                                                 | -0.059 883 767 725 | -0.029 762 177 580 | -0.017 273 034 743 |
| H                                                                 | -0.021 502 870 445 | 0.003 318 955 266  | 0.017 379 683 943  |
| H                                                                 | 0.042 627 263 888  | 0.037 794 208 205  | 0.005 463 717 665  |
| H                                                                 | -0.004 280 617 592 | 0.014 353 107 328  | 0.026 726 063 656  |
| H                                                                 | -0.143 926 635 229 | 0.315 567 685 083  | -0.069 379 907 293 |
| H                                                                 | -0.009 353 760 972 | -0.003 749 698 954 | 0.009 681 873 423  |
| H                                                                 | 0.051 547 425 106  | 0.047 586 998 366  | 0.013 320 963 355  |
| H                                                                 | 0.154 527 477 166  | -0.285 340 179 606 | 0.130 132 707 669  |
| H                                                                 | 0.030 937 110 124  | 0.010 620 250 926  | -0.028 240 305 491 |
| H                                                                 | 0.028 110 309 399  | 0.011 575 382 615  | -0.027 312 119 717 |
| H                                                                 | 0.166 205 607 103  | -0.035 630 867 722 | 0.158 377 974 176  |
| H                                                                 | -0.113 234 967 884 | 0.052 542 320 827  | 0.142 902 104 826  |
| H                                                                 | -0.117 421 103 039 | -0.130 367 273 185 | 0.128 528 142 954  |
| H                                                                 | 0.110 702 298 803  | 0.134 337 857 394  | 0.049 422 895 945  |
| H                                                                 | -0.221 712 848 829 | -0.201 374 739 322 | -0.140 677 569 847 |
| H                                                                 | 0.167 323 040 938  | 0.025 431 028 191  | -0.194 025 785 738 |
| H                                                                 | -0.053 511 437 614 | -0.040 427 925 581 | -0.211 630 255 750 |



Wavenumber/cm<sup>-1</sup>: 3116.619

| $\frac{\partial \mu_{x,y,z}}{\partial Q_r} / (e u^{-0.5})$        | -0.020 082 314 065 | -0.002 560 444 925 | 0.002 218 614 882  |
|-------------------------------------------------------------------|--------------------|--------------------|--------------------|
| <i>l</i> -matrix coefficients/(u <sup>1/2</sup> Å <sup>-1</sup> ) |                    |                    |                    |
| O                                                                 | 0.038 133 359 654  | 0.260 855 095 916  | 0.534 140 897 916  |
| C                                                                 | -0.003 700 154 322 | 0.070 280 713 699  | 0.109 591 806 594  |
| C                                                                 | -0.015 736 957 141 | -0.004 249 916 369 | -0.018 648 085 239 |
| C                                                                 | -0.010 284 694 940 | -0.017 912 279 223 | -0.114 782 151 487 |
| C                                                                 | -0.016 799 168 883 | 0.044 788 169 484  | 0.114 526 661 125  |
| C                                                                 | -0.056 001 035 803 | 0.112 814 736 549  | -0.000 269 051 335 |
| C                                                                 | 0.158 311 524 346  | -0.086 183 929 148 | -0.064 901 000 080 |
| C                                                                 | 0.035 729 403 244  | -0.109 474 480 925 | 0.191 921 784 981  |
| C                                                                 | -0.253 738 234 959 | -0.082 627 755 919 | -0.189 613 131 557 |
| C                                                                 | 0.215 417 043 687  | -0.060 727 168 280 | -0.171 113 028 413 |
| C                                                                 | -0.086 696 029 152 | -0.094 087 326 651 | -0.313 697 404 327 |
| H                                                                 | -0.024 332 256 614 | 0.065 855 255 685  | -0.020 686 641 918 |
| H                                                                 | 0.107 937 489 135  | -0.042 727 833 437 | -0.018 745 769 789 |
| H                                                                 | -0.007 577 271 567 | 0.038 652 880 415  | 0.063 622 155 456  |
| H                                                                 | -0.131 116 470 472 | 0.005 840 772 522  | -0.030 952 323 109 |
| H                                                                 | -0.016 734 134 951 | 0.041 901 826 561  | 0.020 209 220 943  |
| H                                                                 | 0.023 818 117 101  | -0.091 729 139 504 | 0.084 921 202 686  |
| H                                                                 | 0.117 865 054 205  | -0.051 777 032 751 | -0.008 676 241 641 |
| H                                                                 | 0.037 034 201 335  | -0.011 348 006 666 | -0.071 236 019 739 |
| H                                                                 | -0.021 337 960 031 | -0.002 002 109 761 | 0.095 510 997 032  |
| H                                                                 | -0.051 118 618 150 | -0.038 730 134 462 | -0.068 520 406 874 |
| H                                                                 | 0.024 506 739 420  | -0.003 015 613 478 | -0.048 546 308 459 |
| H                                                                 | -0.070 377 451 561 | -0.014 021 618 481 | -0.096 325 691 220 |
| H                                                                 | 0.001 252 212 771  | -0.042 752 326 418 | -0.106 425 206 074 |
| H                                                                 | -0.089 272 441 106 | -0.056 794 091 913 | -0.103 184 569 128 |
| H                                                                 | 0.086 607 799 827  | -0.010 534 504 879 | -0.122 361 422 365 |
| H                                                                 | -0.023 445 828 856 | -0.041 176 903 114 | -0.119 163 967 078 |

*Final state*

Wavenumber/cm<sup>-1</sup>: 99.5158 , Max excitation: 3

| $l'$ -matrix coefficients/(u <sup>1/2</sup> Å <sup>-1</sup> ) |                    |                    |                                      |
|---------------------------------------------------------------|--------------------|--------------------|--------------------------------------|
| O                                                             | 0.000 433 519 480  | 0.000 674 963 111  | 4.091 718 000 000 × 10 <sup>-5</sup> |
| C                                                             | -0.000 542 904 778 | -0.001 181 671 354 | -0.000 727 257 223                   |
| C                                                             | -0.004 134 272 135 | -0.000 962 673 322 | 0.002 346 393 805                    |
| C                                                             | 0.000 561 822 825  | 0.001 777 962 833  | 0.000 322 471 929                    |
| C                                                             | 0.004 960 936 978  | -0.001 993 214 434 | 0.003 309 785 279                    |
| C                                                             | 0.039 481 407 360  | 0.080 931 687 753  | 0.078 812 937 908                    |
| C                                                             | 0.001 742 621 149  | 0.004 419 667 125  | -0.009 890 574 912                   |
| C                                                             | 0.019 601 537 744  | -0.000 992 840 000 | -0.025 032 360 284                   |
| C                                                             | -0.027 382 099 818 | -0.024 444 640 600 | -0.023 342 448 225                   |
| C                                                             | -0.168 983 185 637 | -0.068 994 094 368 | 0.198 322 093 422                    |
| C                                                             | 0.002 466 313 864  | 0.002 549 475 227  | 0.003 522 773 693                    |
| H                                                             | -0.096 344 804 391 | -0.233 506 128 168 | -0.298 567 363 871                   |
| H                                                             | -0.001 139 449 952 | -0.011 339 214 443 | 0.030 319 657 250                    |
| H                                                             | -0.010 925 022 194 | 0.010 805 495 110  | -0.009 007 573 487                   |
| H                                                             | 0.058 385 759 328  | 0.036 219 466 602  | 0.093 772 770 520                    |
| H                                                             | -0.049 974 983 052 | -0.051 261 785 510 | 0.028 052 033 993                    |
| H                                                             | -0.062 245 974 756 | 0.016 405 405 675  | 0.079 873 020 516                    |
| H                                                             | 0.405 152 373 165  | -0.107 942 524 120 | -0.586 771 895 477                   |
| H                                                             | -0.008 280 363 358 | -0.004 111 651 819 | 0.000 736 046 619                    |
| H                                                             | -0.005 531 997 143 | -0.017 381 428 025 | 0.004 932 953 340                    |
| H                                                             | 0.033 876 541 869  | 0.061 170 428 804  | -0.018 350 923 550                   |
| H                                                             | 0.150 385 223 562  | 0.395 344 235 305  | -0.127 111 295 125                   |
| H                                                             | -0.002 082 111 667 | -0.009 873 954 750 | -0.008 245 620 154                   |
| H                                                             | -0.000 916 753 007 | 0.002 933 818 571  | -0.006 200 775 608                   |
| H                                                             | 0.007 594 352 707  | -0.011 203 366 091 | 0.001 782 852 971                    |
| H                                                             | 0.041 106 171 260  | -0.044 261 011 991 | 0.026 744 697 892                    |
| H                                                             | -0.004 338 107 585 | -0.003 997 596 701 | 0.002 056 098 685                    |

Wavenumber/cm<sup>-1</sup>: 197.9356 , Max excitation: 2

| $l'$ -matrix coefficients/(u <sup>1/2</sup> Å <sup>-1</sup> ) |                                        |                    |
|---------------------------------------------------------------|----------------------------------------|--------------------|
| O -0.000 308 490 970                                          | $-3.660\,262\,200\,000 \times 10^{-5}$ | 0.000 516 393 286  |
| C 0.000 203 286 533                                           | $6.295\,873\,700\,000 \times 10^{-5}$  | -0.001 753 032 416 |
| C 0.003 092 439 993                                           | 0.001 335 922 277                      | 0.002 974 689 632  |
| C -0.000 495 628 422                                          | -0.000 899 573 922                     | 0.000 485 094 045  |
| C -0.000 365 553 572                                          | -0.000 940 249 271                     | 0.002 185 905 884  |
| C 0.007 505 404 781                                           | 0.013 790 445 527                      | 0.013 548 362 306  |
| C -0.009 029 582 653                                          | -0.015 276 038 031                     | 0.030 446 577 401  |
| C -0.087 549 084 251                                          | -0.005 209 442 582                     | 0.109 173 856 323  |
| C 0.165 141 836 592                                           | 0.111 325 082 941                      | 0.157 156 136 703  |
| C -0.037 035 675 330                                          | -0.005 844 856 543                     | 0.034 854 161 260  |
| C -0.002 488 608 709                                          | -0.000 743 652 164                     | 0.002 176 863 373  |
| H -0.017 057 919 351                                          | -0.041 841 911 061                     | -0.053 825 844 443 |
| H 0.003 942 216 331                                           | 0.037 669 410 584                      | -0.101 854 492 434 |
| H -0.003 083 157 048                                          | 0.004 261 486 687                      | -0.002 696 032 912 |
| H -0.374 003 843 365                                          | -0.230 677 645 104                     | -0.598 538 760 304 |
| H -0.009 349 686 948                                          | -0.009 570 013 540                     | 0.004 401 985 800  |
| H 0.271 827 005 085                                           | -0.073 110 281 982                     | -0.350 100 513 955 |
| H 0.077 710 886 245                                           | -0.020 290 675 425                     | -0.112 984 284 384 |
| H 0.029 736 244 076                                           | 0.014 408 623 168                      | -0.002 905 897 935 |
| H 0.036 164 000 804                                           | 0.101 753 479 506                      | -0.032 425 956 906 |
| H -0.135 120 525 976                                          | -0.253 412 780 669                     | 0.077 064 479 796  |
| H 0.023 204 820 517                                           | 0.060 949 581 028                      | -0.020 662 548 631 |
| H -0.001 473 651 153                                          | -0.004 976 497 597                     | -0.004 197 067 529 |
| H -0.000 388 039 550                                          | -0.000 390 875 888                     | 0.000 283 476 412  |
| H -0.071 620 502 733                                          | 0.091 254 402 845                      | -0.022 201 756 052 |
| H 0.025 865 670 702                                           | -0.021 800 624 399                     | 0.009 951 349 980  |
| H 0.010 321 307 797                                           | 0.009 004 669 267                      | -0.003 869 298 624 |

Wavenumber/cm<sup>-1</sup>: 209.2078 , Max excitation: 1

| $l'$ -matrix coefficients/(u <sup>1/2</sup> Å <sup>-1</sup> ) |                    |                                      |                                      |
|---------------------------------------------------------------|--------------------|--------------------------------------|--------------------------------------|
| O                                                             | 0.000 283 661 610  | -0.000 471 242 880                   | 5.951 595 900 000 × 10 <sup>-5</sup> |
| C                                                             | 0.000 359 530 188  | 0.000 878 772 963                    | -0.000 341 332 880                   |
| C                                                             | -0.002 734 233 640 | -0.001 981 386 217                   | 0.000 450 310 178                    |
| C                                                             | -0.000 594 165 891 | -0.003 688 396 859                   | 0.001 071 265 028                    |
| C                                                             | -0.010 734 231 576 | 0.007 190 086 025                    | -0.006 725 474 516                   |
| C                                                             | -0.042 497 354 889 | -0.082 509 142 896                   | -0.072 085 849 507                   |
| C                                                             | -0.022 784 278 820 | -0.042 336 660 786                   | 0.087 930 768 513                    |
| C                                                             | -0.129 156 545 262 | -0.021 754 589 043                   | 0.158 510 583 012                    |
| C                                                             | -0.090 605 675 920 | -0.080 194 585 204                   | -0.068 706 388 571                   |
| C                                                             | -0.035 450 879 355 | -0.030 829 488 230                   | 0.045 594 173 651                    |
| C                                                             | 0.007 843 383 279  | 0.007 070 557 332                    | 0.006 330 274 232                    |
| H                                                             | 0.086 472 956 140  | 0.215 530 499 404                    | 0.276 991 424 763                    |
| H                                                             | 0.011 994 293 010  | 0.108 070 978 533                    | -0.292 318 533 201                   |
| H                                                             | 0.026 563 654 760  | -0.024 505 396 400                   | 0.023 200 702 566                    |
| H                                                             | 0.177 828 180 796  | 0.107 376 893 118                    | 0.288 027 326 987                    |
| H                                                             | 0.068 571 969 861  | 0.070 858 220 156                    | -0.037 618 174 672                   |
| H                                                             | 0.376 891 691 187  | -0.103 332 419 857                   | -0.484 298 839 923                   |
| H                                                             | 0.079 633 842 360  | -0.022 519 467 650                   | -0.116 264 678 191                   |
| H                                                             | 0.075 254 222 706  | 0.037 176 973 880                    | -0.006 918 802 774                   |
| H                                                             | 0.068 192 478 953  | 0.191 439 595 319                    | -0.060 203 328 782                   |
| H                                                             | 0.112 775 327 067  | 0.204 054 372 461                    | -0.061 889 848 256                   |
| H                                                             | 0.049 294 825 230  | 0.131 631 306 862                    | -0.041 894 547 564                   |
| H                                                             | -0.004 990 530 845 | -0.016 640 451 072                   | -0.016 641 982 314                   |
| H                                                             | -0.004 067 152 919 | 0.008 334 558 059                    | -0.013 103 259 987                   |
| H                                                             | 0.025 488 690 079  | -0.036 022 905 534                   | 0.007 885 035 746                    |
| H                                                             | -0.006 274 800 329 | 7.903 379 800 000 × 10 <sup>-5</sup> | 0.002 217 676 033                    |
| H                                                             | -0.018 190 163 873 | -0.013 028 365 264                   | 0.007 793 694 272                    |

Wavenumber/cm<sup>-1</sup>: 223.8886 , Max excitation: 3

| $l'$ -matrix coefficients/(u <sup>1/2</sup> Å <sup>-1</sup> ) |                    |                                       |
|---------------------------------------------------------------|--------------------|---------------------------------------|
| O -0.000 217 541 663                                          | -0.000 110 403 761 | -2.198 260 000 000 × 10 <sup>-5</sup> |
| C 0.000 575 430 008                                           | 0.001 010 225 867  | 0.000 558 915 754                     |
| C 0.000 213 237 026                                           | -0.001 513 293 239 | 0.000 265 680 239                     |
| C -0.001 827 495 663                                          | -0.003 826 917 644 | -0.000 826 521 478                    |
| C -0.010 044 384 972                                          | 0.008 105 492 888  | -0.007 873 167 025                    |
| C -0.080 692 554 209                                          | -0.157 601 227 125 | -0.145 394 509 527                    |
| C 0.008 803 745 721                                           | 0.016 920 024 783  | -0.033 846 146 154                    |
| C 0.066 049 933 758                                           | 0.012 056 561 307  | -0.079 651 948 671                    |
| C 0.045 854 509 557                                           | 0.025 400 936 104  | 0.043 690 918 036                     |
| C -0.061 311 434 473                                          | -0.068 421 234 405 | 0.076 965 312 815                     |
| C -0.032 285 925 646                                          | -0.041 665 971 118 | -0.034 298 716 489                    |
| H 0.174 961 827 629                                           | 0.432 700 999 745  | 0.557 648 740 243                     |
| H -0.004 651 295 899                                          | -0.043 568 452 745 | 0.118 189 571 236                     |
| H 0.029 693 217 148                                           | -0.028 077 530 419 | 0.024 998 119 550                     |
| H -0.098 988 896 832                                          | -0.060 619 067 832 | -0.159 388 377 876                    |
| H 0.112 195 582 302                                           | 0.116 885 364 789  | -0.061 365 243 529                    |
| H -0.193 522 771 306                                          | 0.052 952 176 008  | 0.248 026 288 231                     |
| H 0.121 284 401 452                                           | -0.035 922 404 163 | -0.176 358 898 272                    |
| H -0.024 956 678 339                                          | -0.011 508 078 301 | 0.002 609 684 592                     |
| H -0.034 354 872 687                                          | -0.096 150 560 324 | 0.030 479 922 362                     |
| H -0.029 408 119 491                                          | -0.056 724 228 664 | 0.018 145 635 430                     |
| H 0.107 097 405 068                                           | 0.264 984 047 960  | -0.088 613 493 995                    |
| H 0.027 044 217 960                                           | 0.115 735 722 312  | 0.111 947 674 084                     |
| H 0.009 244 536 347                                           | -0.023 033 037 981 | 0.038 290 699 004                     |
| H -0.029 227 200 991                                          | 0.033 685 803 503  | -0.010 052 369 363                    |
| H -0.018 630 584 354                                          | 0.007 666 683 609  | 0.000 435 767 344                     |
| H 0.076 308 124 843                                           | 0.054 744 807 384  | -0.032 133 479 567                    |

Wavenumber/cm<sup>-1</sup>: 237.359 , Max excitation: 1

| $l'$ -matrix coefficients/(u <sup>1/2</sup> Å <sup>-1</sup> ) |                    |                                       |                    |
|---------------------------------------------------------------|--------------------|---------------------------------------|--------------------|
| O                                                             | 0.000 394 741 561  | 0.000 324 736 251                     | 0.000 174 845 656  |
| C                                                             | 0.000 368 939 967  | -0.000 330 407 782                    | 0.000 277 405 853  |
| C                                                             | -0.000 139 132 506 | -0.000 208 336 260                    | 0.000 237 435 958  |
| C                                                             | -0.001 536 534 836 | $4.726\,999\,300\,000 \times 10^{-5}$ | -0.005 283 759 028 |
| C                                                             | -0.001 915 956 835 | 0.002 412 419 523                     | -0.002 144 981 468 |
| C                                                             | 0.012 634 103 620  | 0.023 102 791 026                     | 0.024 332 903 600  |
| C                                                             | 0.009 087 894 491  | 0.022 605 693 838                     | -0.051 852 824 496 |
| C                                                             | -0.030 760 772 427 | -0.004 294 736 990                    | 0.037 516 617 853  |
| C                                                             | -0.012 429 870 579 | -0.035 867 893 701                    | 0.004 975 587 464  |
| C                                                             | 0.010 052 774 288  | -0.000 269 826 944                    | -0.008 818 020 301 |
| C                                                             | -0.074 997 920 651 | -0.052 967 298 748                    | -0.274 938 969 676 |
| H                                                             | -0.026 572 155 674 | -0.068 229 294 133                    | -0.086 024 852 270 |
| H                                                             | -0.008 385 027 146 | -0.063 467 086 591                    | 0.181 365 527 215  |
| H                                                             | 0.008 990 521 788  | -0.007 911 125 671                    | 0.009 984 631 779  |
| H                                                             | 0.010 154 825 163  | 0.005 729 479 910                     | 0.019 846 302 001  |
| H                                                             | -0.015 494 782 801 | -0.016 423 733 227                    | 0.008 927 101 498  |
| H                                                             | 0.090 989 912 241  | -0.024 371 105 274                    | -0.116 746 204 876 |
| H                                                             | -0.020 170 993 364 | 0.005 471 858 481                     | 0.029 928 827 218  |
| H                                                             | -0.023 725 339 474 | -0.010 155 715 984                    | 0.001 200 933 863  |
| H                                                             | 0.015 086 321 343  | 0.040 662 250 741                     | -0.012 607 126 100 |
| H                                                             | 0.055 429 082 361  | 0.096 957 179 119                     | -0.029 682 968 377 |
| H                                                             | -0.005 487 202 239 | -0.012 589 545 116                    | 0.004 253 984 509  |
| H                                                             | 0.118 522 699 777  | 0.472 438 774 131                     | 0.443 387 353 791  |
| H                                                             | 0.148 687 413 852  | -0.286 337 860 348                    | 0.525 894 663 237  |
| H                                                             | -0.024 537 310 124 | 0.021 528 292 930                     | -0.009 199 281 775 |
| H                                                             | -0.009 633 416 869 | 0.007 932 676 478                     | -0.003 623 977 948 |
| H                                                             | -0.006 003 752 563 | -0.004 530 490 044                    | -0.015 894 960 157 |

Wavenumber/cm<sup>-1</sup>: 238.7606 , Max excitation: 3

| $l'$ -matrix coefficients/(u <sup>1/2</sup> Å <sup>-1</sup> ) |                    |                    |                    |
|---------------------------------------------------------------|--------------------|--------------------|--------------------|
| O                                                             | 0.000 148 682 428  | 0.000 172 731 305  | -0.000 238 972 739 |
| C                                                             | -0.001 117 702 118 | -0.000 206 704 884 | 0.001 671 828 889  |
| C                                                             | 0.001 107 485 951  | -0.002 573 960 913 | 0.000 723 442 126  |
| C                                                             | 0.003 174 618 142  | 0.003 496 199 815  | -0.001 469 155 073 |
| C                                                             | 0.002 129 947 293  | -0.001 696 961 687 | 0.001 944 227 284  |
| C                                                             | -0.002 613 132 522 | -0.008 917 117 153 | -0.008 249 977 274 |
| C                                                             | 0.043 656 677 705  | 0.088 095 733 616  | -0.195 406 393 269 |
| C                                                             | -0.041 376 485 889 | 0.006 049 857 405  | 0.055 063 693 901  |
| C                                                             | 0.000 451 291 916  | -0.097 561 680 854 | 0.047 091 565 639  |
| C                                                             | 0.020 226 751 941  | -0.062 104 799 800 | -0.000 645 630 331 |
| C                                                             | 0.073 171 255 384  | 0.103 437 713 112  | 0.038 423 378 569  |
| H                                                             | 0.009 361 769 969  | 0.026 195 827 421  | 0.032 335 724 941  |
| H                                                             | -0.030 815 449 324 | -0.242 587 701 444 | 0.658 495 466 457  |
| H                                                             | -0.007 181 538 978 | 0.008 760 330 287  | -0.006 952 613 183 |
| H                                                             | -0.037 376 321 755 | -0.029 757 194 978 | -0.055 569 313 578 |
| H                                                             | 0.003 457 064 955  | 0.001 970 624 261  | -0.000 502 271 077 |
| H                                                             | 0.142 682 698 401  | -0.036 711 610 383 | -0.185 067 542 630 |
| H                                                             | -0.051 613 860 022 | 0.009 994 011 718  | 0.076 327 914 519  |
| H                                                             | -0.129 162 498 386 | -0.064 099 197 291 | 0.009 903 148 360  |
| H                                                             | 0.005 025 418 152  | 0.018 008 695 274  | -0.002 931 785 824 |
| H                                                             | 0.147 062 701 354  | 0.251 516 703 803  | -0.066 819 374 702 |
| H                                                             | 0.059 877 715 710  | 0.144 825 229 309  | -0.050 881 943 321 |
| H                                                             | -0.054 195 064 791 | -0.222 320 992 207 | -0.218 768 190 775 |
| H                                                             | 0.005 529 105 369  | 0.007 169 523 202  | 0.000 739 350 607  |
| H                                                             | -0.116 307 019 867 | 0.114 029 658 251  | -0.039 764 719 511 |
| H                                                             | -0.081 347 128 431 | 0.061 220 198 817  | -0.024 569 627 488 |
| H                                                             | -0.206 682 715 915 | -0.145 620 868 195 | 0.085 041 377 102  |

Wavenumber/cm<sup>-1</sup>: 259.9371 , Max excitation: 2

| $l'$ -matrix coefficients/(u <sup>1/2</sup> Å <sup>-1</sup> ) |                    |                    |
|---------------------------------------------------------------|--------------------|--------------------|
| O 6.787 234 000 000 × 10 <sup>-6</sup>                        | -0.000 438 517 292 | -0.000 160 860 224 |
| C -0.000 339 848 537                                          | 0.002 881 481 739  | -0.001 319 154 466 |
| C 0.004 219 057 493                                           | -0.005 873 134 747 | 0.002 099 076 230  |
| C -0.003 109 853 585                                          | -0.002 424 694 244 | 0.001 666 401 565  |
| C 0.009 820 617 271                                           | -0.008 239 474 489 | 0.007 501 950 401  |
| C 0.015 032 794 644                                           | 0.030 987 114 548  | 0.031 153 371 847  |
| C -0.015 899 473 733                                          | -0.025 606 970 044 | 0.053 302 227 119  |
| C 0.012 140 512 693                                           | -0.010 645 554 648 | -0.017 092 370 169 |
| C 0.013 988 645 716                                           | -0.149 667 584 081 | 0.090 195 834 196  |
| C 0.067 018 406 534                                           | -0.146 445 345 645 | -0.020 418 217 270 |
| C -0.062 398 785 585                                          | -0.121 347 338 593 | 0.053 985 674 699  |
| H -0.036 202 581 428                                          | -0.090 017 166 613 | -0.115 620 345 875 |
| H 0.009 310 085 276                                           | 0.065 553 140 918  | -0.178 279 644 679 |
| H -0.030 743 501 927                                          | 0.032 265 870 316  | -0.028 939 192 686 |
| H -0.087 683 494 810                                          | -0.065 893 949 605 | -0.138 780 585 033 |
| H -0.016 476 923 518                                          | -0.014 943 042 527 | 0.008 816 545 303  |
| H -0.050 741 622 916                                          | 0.013 586 771 018  | 0.066 337 117 816  |
| H -0.165 372 836 613                                          | 0.034 165 936 334  | 0.245 425 522 087  |
| H 0.047 977 808 623                                           | 0.024 792 926 957  | -0.004 227 476 997 |
| H 0.009 853 038 088                                           | 0.023 127 412 054  | -0.009 711 968 409 |
| H 0.230 992 209 324                                           | 0.393 683 359 853  | -0.102 345 337 412 |
| H 0.136 594 197 790                                           | 0.317 813 546 398  | -0.114 235 551 957 |
| H 0.030 949 795 913                                           | 0.129 930 693 209  | 0.137 913 339 440  |
| H -0.069 385 416 922                                          | 0.111 453 259 661  | -0.226 816 330 922 |
| H -0.198 058 782 919                                          | 0.194 758 302 713  | -0.068 531 177 912 |
| H -0.209 718 982 357                                          | 0.156 800 483 305  | -0.065 764 643 647 |
| H 0.258 971 110 094                                           | 0.181 050 522 396  | -0.098 705 910 627 |



Wavenumber/cm<sup>-1</sup>: 280.8876 , Max excitation: 2

| $l'$ -matrix coefficients/(u <sup>1/2</sup> Å <sup>-1</sup> ) |                                      |                    |                    |
|---------------------------------------------------------------|--------------------------------------|--------------------|--------------------|
| O                                                             | -0.000 179 995 908                   | 0.000 190 102 285  | 0.000 116 404 548  |
| C                                                             | 0.001 932 358 339                    | 0.000 203 764 459  | -0.000 161 084 257 |
| C                                                             | -0.002 029 200 199                   | 0.001 436 604 755  | -0.000 253 803 600 |
| C                                                             | -0.002 844 324 552                   | -0.002 485 611 311 | 0.000 706 559 323  |
| C                                                             | 3.811 320 800 000 × 10 <sup>-5</sup> | -0.000 832 304 812 | 0.001 050 724 846  |
| C                                                             | -0.005 999 283 384                   | -0.010 029 858 157 | -0.008 276 486 054 |
| C                                                             | 0.014 376 742 773                    | 0.034 725 572 475  | -0.080 470 654 841 |
| C                                                             | -0.021 942 771 707                   | -0.001 431 742 744 | 0.028 325 432 664  |
| C                                                             | -0.009 568 757 128                   | -0.063 989 791 749 | 0.023 202 998 164  |
| C                                                             | -0.061 031 138 585                   | 0.178 000 870 863  | 0.003 945 447 602  |
| C                                                             | -0.074 518 682 788                   | -0.157 175 463 104 | 0.083 812 534 093  |
| H                                                             | 0.010 204 698 149                    | 0.024 317 056 075  | 0.032 272 016 660  |
| H                                                             | -0.012 258 507 309                   | -0.101 075 563 256 | 0.273 880 168 747  |
| H                                                             | -0.001 013 847 265                   | -0.000 224 243 056 | -0.001 251 500 527 |
| H                                                             | -0.009 449 492 879                   | -0.011 439 355 174 | -0.012 511 319 834 |
| H                                                             | 0.008 947 608 817                    | 0.010 929 630 477  | -0.005 621 136 321 |
| H                                                             | 0.068 596 876 800                    | -0.018 044 118 753 | -0.089 790 175 360 |
| H                                                             | 0.154 152 293 467                    | -0.027 759 229 565 | -0.228 920 482 369 |
| H                                                             | -0.038 230 819 178                   | -0.017 916 635 811 | 0.002 301 119 017  |
| H                                                             | 0.009 581 094 668                    | 0.026 632 465 857  | -0.007 772 155 761 |
| H                                                             | 0.100 441 050 878                    | 0.174 614 199 116  | -0.049 150 914 061 |
| H                                                             | -0.172 475 091 859                   | -0.408 601 521 716 | 0.147 680 431 434  |
| H                                                             | 0.037 565 341 206                    | 0.153 018 909 312  | 0.163 623 273 983  |
| H                                                             | -0.101 189 278 153                   | 0.164 535 994 591  | -0.332 465 794 861 |
| H                                                             | -0.058 683 405 414                   | 0.055 273 371 712  | -0.020 979 952 207 |
| H                                                             | 0.237 419 873 023                    | -0.176 836 678 369 | 0.072 451 718 869  |
| H                                                             | 0.324 903 906 310                    | 0.226 305 057 834  | -0.123 303 633 767 |

Wavenumber/cm<sup>-1</sup>: -286.6136, replaced by 286.6136 , Max excitation: 5

| $l'$ -matrix coefficients/(u <sup>1/2</sup> Å <sup>-1</sup> ) |                                       |                    |
|---------------------------------------------------------------|---------------------------------------|--------------------|
| O -0.000 125 345 413                                          | 0.000 408 515 376                     | -0.000 672 535 997 |
| C 0.001 179 837 755                                           | -2.249 694 900 000 × 10 <sup>-5</sup> | 0.001 485 869 634  |
| C -0.000 639 164 522                                          | 0.000 954 858 059                     | -0.000 376 213 036 |
| C -0.001 601 165 362                                          | -0.000 996 752 350                    | 0.000 193 737 148  |
| C -0.005 551 522 275                                          | 0.005 271 442 553                     | -0.004 058 160 373 |
| C 0.010 518 947 223                                           | 0.016 510 013 304                     | 0.011 315 067 315  |
| C 0.015 640 959 180                                           | 0.036 983 232 237                     | -0.085 375 826 298 |
| C -0.040 109 534 444                                          | -0.003 144 482 691                    | 0.050 458 991 972  |
| C -0.023 670 569 572                                          | 0.157 663 784 873                     | -0.105 507 927 152 |
| C 0.042 789 889 908                                           | -0.117 845 350 609                    | -0.000 803 810 997 |
| C -0.053 279 921 636                                          | -0.119 107 937 831                    | 0.054 007 926 294  |
| H -0.015 289 219 918                                          | -0.036 778 583 964                    | -0.047 579 548 703 |
| H -0.014 643 993 264                                          | -0.106 848 318 951                    | 0.290 002 130 017  |
| H 0.019 095 981 661                                           | -0.019 524 754 375                    | 0.018 129 873 976  |
| H 0.116 696 311 685                                           | 0.083 864 402 354                     | 0.179 300 765 176  |
| H -0.019 340 480 835                                          | -0.019 662 313 866                    | 0.009 482 961 216  |
| H 0.121 209 486 012                                           | -0.033 400 922 845                    | -0.158 685 341 726 |
| H -0.099 001 768 154                                          | 0.016 674 818 991                     | 0.147 988 133 329  |
| H -0.042 604 709 126                                          | -0.020 171 181 548                    | 0.002 504 249 197  |
| H 0.016 394 611 381                                           | 0.045 915 395 998                     | -0.013 877 965 755 |
| H -0.244 335 613 874                                          | -0.416 784 740 920                    | 0.107 383 671 293  |
| H 0.112 807 571 746                                           | 0.264 352 078 166                     | -0.096 722 233 740 |
| H 0.032 787 301 924                                           | 0.133 613 989 513                     | 0.141 610 114 116  |
| H -0.072 936 619 684                                          | 0.119 282 954 611                     | -0.242 541 802 998 |
| H 0.215 182 594 205                                           | -0.213 117 398 808                    | 0.075 125 030 492  |
| H -0.165 322 096 792                                          | 0.124 374 082 901                     | -0.050 403 876 152 |
| H 0.228 700 216 370                                           | 0.158 511 197 712                     | -0.087 502 644 800 |

Wavenumber/cm<sup>-1</sup>: 338.6642 , Max excitation: 2

| $l'$ -matrix coefficients/(u <sup>1/2</sup> Å <sup>-1</sup> ) |                    |                                      |                    |
|---------------------------------------------------------------|--------------------|--------------------------------------|--------------------|
| O                                                             | 0.000 256 133 702  | -0.001 491 202 289                   | 0.000 383 036 278  |
| C                                                             | -0.001 592 509 237 | 0.003 475 470 109                    | -0.000 739 873 752 |
| C                                                             | 0.004 359 874 917  | 2.239 916 200 000 × 10 <sup>-5</sup> | 0.000 717 941 033  |
| C                                                             | -0.002 123 205 192 | 0.002 144 920 292                    | -0.001 467 533 974 |
| C                                                             | 0.149 370 205 528  | -0.154 122 406 147                   | 0.137 076 384 744  |
| C                                                             | -0.026 506 185 700 | -0.029 094 813 540                   | 0.004 806 262 878  |
| C                                                             | -0.013 701 659 097 | -0.000 530 349 880                   | -0.010 693 254 023 |
| C                                                             | -0.020 647 948 324 | -0.097 793 855 727                   | 0.011 808 757 865  |
| C                                                             | 0.008 115 505 095  | 0.009 581 541 708                    | -0.011 267 448 587 |
| C                                                             | 0.004 431 058 526  | 0.001 957 521 723                    | 0.007 041 515 865  |
| C                                                             | -0.003 360 542 792 | 0.004 379 714 458                    | -0.006 170 348 615 |
| H                                                             | 0.011 009 882 242  | 0.021 847 798 115                    | 0.029 045 977 886  |
| H                                                             | -0.002 377 345 864 | -0.014 442 502 126                   | 0.039 301 813 431  |
| H                                                             | -0.508 414 870 923 | 0.522 412 452 247                    | -0.469 895 981 099 |
| H                                                             | 0.018 168 301 113  | 0.012 326 200 507                    | 0.026 407 434 422  |
| H                                                             | 0.078 934 666 007  | 0.080 655 141 514                    | -0.037 502 551 188 |
| H                                                             | -0.055 501 490 514 | 0.008 607 025 748                    | 0.072 733 557 189  |
| H                                                             | 0.016 229 810 262  | -0.004 528 658 733                   | -0.022 869 109 105 |
| H                                                             | 0.041 725 302 546  | 0.020 717 737 996                    | -0.007 304 951 484 |
| H                                                             | 0.129 994 360 876  | 0.320 061 125 352                    | -0.116 123 490 590 |
| H                                                             | -0.034 151 322 868 | -0.057 752 768 515                   | 0.015 029 042 139  |
| H                                                             | -0.010 875 544 957 | -0.019 979 605 805                   | 0.005 970 477 526  |
| H                                                             | -0.000 441 289 627 | -0.003 669 851 178                   | -0.003 530 080 752 |
| H                                                             | 0.007 723 592 614  | -0.015 237 771 084                   | 0.027 460 665 292  |
| H                                                             | -0.012 345 506 291 | 0.012 372 849 260                    | -0.003 404 287 168 |
| H                                                             | -0.024 425 641 002 | 0.017 108 499 726                    | -0.007 294 867 879 |
| H                                                             | 0.004 242 895 660  | 0.002 889 122 955                    | -0.002 147 320 745 |

Wavenumber/cm<sup>-1</sup>: 365.0201 , Max excitation: 3

| $l'$ -matrix coefficients/(u <sup>1/2</sup> Å <sup>-1</sup> ) |                    |                    |
|---------------------------------------------------------------|--------------------|--------------------|
| O                                                             | -0.000 242 099 339 | -0.000 204 069 343 |
| C                                                             | 0.001 426 520 923  | -0.000 575 031 602 |
| C                                                             | -0.001 026 771 843 | 0.002 646 119 524  |
| C                                                             | -0.000 405 599 006 | 0.000 551 512 019  |
| C                                                             | -0.066 996 223 379 | 0.066 749 915 001  |
| C                                                             | -0.003 905 222 150 | -0.001 569 701 692 |
| C                                                             | -0.023 765 705 226 | -0.002 997 223 466 |
| C                                                             | -0.035 912 253 634 | -0.222 515 981 993 |
| C                                                             | 0.004 360 874 401  | 0.006 202 951 843  |
| C                                                             | -0.003 520 836 014 | 0.004 651 369 470  |
| C                                                             | 0.004 446 101 756  | 0.010 132 249 687  |
| H                                                             | -0.006 923 999 602 | -0.015 118 475 420 |
| H                                                             | -0.005 254 453 575 | -0.027 095 366 828 |
| H                                                             | 0.224 734 965 688  | -0.233 306 747 557 |
| H                                                             | -0.017 143 829 815 | -0.010 064 743 731 |
| H                                                             | 0.021 232 389 097  | 0.022 493 196 045  |
| H                                                             | -0.168 131 517 284 | 0.026 547 876 850  |
| H                                                             | -0.006 901 336 171 | 0.002 208 799 219  |
| H                                                             | 0.084 232 904 462  | 0.042 905 472 969  |
| H                                                             | 0.296 573 077 803  | 0.728 681 821 464  |
| H                                                             | -0.001 379 330 450 | -0.002 766 135 480 |
| H                                                             | 0.001 087 810 663  | -0.004 263 970 521 |
| H                                                             | -0.005 684 238 512 | -0.024 429 318 281 |
| H                                                             | 0.001 601 121 198  | -0.003 576 118 241 |
| H                                                             | 0.006 477 685 575  | -0.005 851 733 153 |
| H                                                             | 0.020 973 438 396  | -0.014 986 720 611 |
| H                                                             | -0.011 999 887 875 | -0.008 596 671 381 |

Wavenumber/cm<sup>-1</sup>: 370.8415 , Max excitation: 3

| $l'$ -matrix coefficients/(u <sup>1/2</sup> Å <sup>-1</sup> ) |                    |                                       |                    |
|---------------------------------------------------------------|--------------------|---------------------------------------|--------------------|
| O                                                             | 0.000 225 033 640  | -0.001 435 943 184                    | 0.000 525 682 903  |
| C                                                             | 0.001 452 525 162  | 0.002 600 143 516                     | -0.001 079 133 968 |
| C                                                             | 0.000 137 724 699  | -3.385 335 400 000 × 10 <sup>-5</sup> | -0.000 190 619 623 |
| C                                                             | -0.001 328 338 409 | -0.002 802 010 873                    | 0.000 497 190 306  |
| C                                                             | -0.007 211 637 602 | 0.006 502 324 830                     | -0.007 506 723 832 |
| C                                                             | -0.044 489 718 473 | -0.039 893 194 243                    | 0.040 305 356 390  |
| C                                                             | -0.024 813 483 160 | -0.007 973 995 505                    | -0.013 480 578 805 |
| C                                                             | -0.000 641 445 973 | 0.013 807 075 222                     | 0.003 430 452 874  |
| C                                                             | -0.007 529 689 976 | 0.001 240 103 112                     | -0.005 202 023 541 |
| C                                                             | 0.012 191 077 578  | -0.003 629 299 656                    | 0.003 613 138 544  |
| C                                                             | -0.151 076 750 286 | 0.050 919 435 477                     | 0.031 064 911 172  |
| H                                                             | -0.022 333 838 229 | -0.048 092 965 846                    | -0.056 522 137 053 |
| H                                                             | -0.004 836 677 789 | -0.021 951 141 726                    | 0.056 845 038 665  |
| H                                                             | 0.025 154 638 102  | -0.025 414 309 750                    | 0.025 560 685 281  |
| H                                                             | 0.006 488 606 635  | 0.005 759 271 530                     | 0.011 909 374 159  |
| H                                                             | 0.174 504 515 478  | 0.188 673 558 583                     | -0.079 176 874 836 |
| H                                                             | 0.019 379 456 123  | -0.003 456 670 007                    | -0.026 598 541 138 |
| H                                                             | 0.005 742 159 919  | -0.001 264 602 160                    | -0.005 515 102 622 |
| H                                                             | 0.090 960 658 486  | 0.048 437 207 393                     | -0.015 381 871 538 |
| H                                                             | -0.017 796 907 492 | -0.041 966 217 953                    | 0.016 286 944 292  |
| H                                                             | 0.003 500 082 216  | 0.007 134 839 073                     | -0.002 424 313 011 |
| H                                                             | -0.005 730 446 824 | -0.016 646 645 829                    | 0.005 914 147 824  |
| H                                                             | -0.092 075 980 061 | -0.326 841 569 872                    | -0.316 662 993 935 |
| H                                                             | 0.107 438 796 246  | -0.210 108 421 262                    | 0.409 022 670 416  |
| H                                                             | 0.016 274 513 494  | -0.016 623 454 296                    | 0.006 984 005 295  |
| H                                                             | -0.040 364 816 685 | 0.031 592 194 286                     | -0.012 000 893 211 |
| H                                                             | 0.503 659 825 052  | 0.364 907 031 684                     | -0.197 945 761 502 |

Wavenumber/cm<sup>-1</sup>: 438.1744 , Max excitation: 2

| $l'$ -matrix coefficients/(u <sup>1/2</sup> Å <sup>-1</sup> ) |                    |                    |                                       |
|---------------------------------------------------------------|--------------------|--------------------|---------------------------------------|
| O                                                             | 0.000 763 322 869  | 0.001 737 189 542  | -0.000 821 668 039                    |
| C                                                             | -0.000 675 304 899 | -0.003 737 624 653 | 0.001 331 904 367                     |
| C                                                             | -0.002 994 689 659 | 0.001 325 700 286  | -0.000 396 879 677                    |
| C                                                             | 0.003 521 551 856  | 0.001 343 708 373  | -7.666 238 600 000 × 10 <sup>-5</sup> |
| C                                                             | 0.018 404 547 430  | -0.014 327 452 044 | 0.016 134 049 466                     |
| C                                                             | 0.080 145 941 953  | 0.073 063 493 908  | -0.063 085 055 364                    |
| C                                                             | 0.014 809 803 720  | 0.007 487 147 357  | -0.000 952 133 849                    |
| C                                                             | -0.001 530 275 011 | -0.011 703 495 305 | 0.001 258 865 363                     |
| C                                                             | -0.096 924 497 869 | 0.051 735 596 758  | 0.020 003 719 544                     |
| C                                                             | -0.101 735 613 441 | 0.016 345 490 882  | -0.059 566 829 697                    |
| C                                                             | -0.031 222 485 524 | 0.009 863 491 678  | 0.005 767 615 665                     |
| H                                                             | 0.032 500 233 405  | 0.070 771 405 945  | 0.078 390 296 341                     |
| H                                                             | -0.000 231 200 973 | 0.002 013 791 057  | -0.005 733 688 363                    |
| H                                                             | -0.060 182 055 833 | 0.060 298 448 952  | -0.057 236 277 680                    |
| H                                                             | -0.088 363 360 978 | -0.047 826 670 067 | -0.131 713 655 034                    |
| H                                                             | -0.308 447 763 945 | -0.328 687 069 120 | 0.137 848 858 200                     |
| H                                                             | -0.008 702 418 676 | 0.001 509 842 858  | 0.009 901 046 267                     |
| H                                                             | -0.121 293 666 387 | 0.031 103 983 534  | 0.163 603 367 110                     |
| H                                                             | -0.054 233 951 329 | -0.028 935 482 514 | 0.008 688 539 158                     |
| H                                                             | 0.014 532 845 607  | 0.036 195 712 758  | -0.014 503 971 095                    |
| H                                                             | 0.103 618 613 053  | 0.197 831 544 151  | -0.051 763 527 524                    |
| H                                                             | 0.079 507 691 442  | 0.215 417 385 795  | -0.077 336 862 870                    |
| H                                                             | -0.018 867 689 042 | -0.066 459 662 946 | -0.063 745 838 918                    |
| H                                                             | 0.021 573 495 933  | -0.043 148 792 114 | 0.084 028 263 708                     |
| H                                                             | 0.319 100 557 729  | -0.330 026 746 961 | 0.120 365 545 114                     |
| H                                                             | 0.392 527 638 964  | -0.306 875 754 920 | 0.117 578 035 360                     |
| H                                                             | 0.101 947 661 548  | 0.076 320 168 837  | -0.040 382 974 825                    |

Wavenumber/cm<sup>-1</sup>: 459.9383 , Max excitation: 2

| $l'$ -matrix coefficients/(u <sup>1/2</sup> Å <sup>-1</sup> ) |                    |                    |
|---------------------------------------------------------------|--------------------|--------------------|
| O -4.540 103 300 000 × 10 <sup>-5</sup>                       | -0.000 495 631 847 | 0.000 685 635 766  |
| C 0.001 652 141 456                                           | -0.000 761 494 668 | 0.000 119 803 940  |
| C -0.000 656 961 620                                          | 0.002 522 588 129  | -0.001 996 922 293 |
| C -0.004 056 738 158                                          | -0.000 119 280 806 | -0.000 408 550 992 |
| C -0.002 449 439 817                                          | 0.002 029 424 520  | -0.003 675 842 412 |
| C -0.123 203 736 732                                          | -0.109 229 827 670 | 0.107 129 516 142  |
| C -0.023 343 184 895                                          | -0.010 236 608 901 | -0.002 734 974 753 |
| C 0.008 307 206 627                                           | 0.017 985 302 100  | -0.008 414 276 357 |
| C -0.066 554 017 522                                          | 0.043 008 676 728  | 0.016 714 587 133  |
| C -0.055 495 869 869                                          | 0.010 368 318 859  | -0.039 792 107 718 |
| C 0.040 916 348 454                                           | -0.011 366 031 833 | -0.006 369 361 668 |
| H -0.057 792 402 965                                          | -0.129 233 043 838 | -0.148 195 530 374 |
| H -0.002 809 238 770                                          | -0.008 076 283 924 | 0.021 262 311 699  |
| H 0.010 897 825 101                                           | -0.012 782 646 582 | 0.013 309 498 711  |
| H -0.071 001 222 427                                          | -0.039 030 005 773 | -0.106 732 870 243 |
| H 0.480 918 092 668                                           | 0.513 931 285 492  | -0.214 487 685 980 |
| H -0.001 112 647 425                                          | 0.003 487 345 992  | 0.002 735 048 129  |
| H -0.080 517 941 433                                          | 0.021 485 762 743  | 0.111 740 215 235  |
| H 0.084 155 233 027                                           | 0.043 629 563 334  | -0.014 304 081 214 |
| H -0.026 261 779 306                                          | -0.064 993 603 635 | 0.024 603 423 482  |
| H 0.067 864 404 350                                           | 0.130 723 487 587  | -0.036 634 747 677 |
| H 0.045 975 232 634                                           | 0.119 747 968 068  | -0.043 466 728 476 |
| H 0.023 139 245 532                                           | 0.079 882 255 798  | 0.077 555 192 214  |
| H -0.026 746 996 211                                          | 0.055 433 040 359  | -0.108 684 178 971 |
| H 0.233 603 610 531                                           | -0.241 347 723 585 | 0.087 871 483 962  |
| H 0.229 759 469 807                                           | -0.179 362 159 137 | 0.068 283 723 957  |
| H -0.133 593 667 831                                          | -0.098 903 705 263 | 0.053 320 303 994  |

Wavenumber/cm<sup>-1</sup>: 486.9134 , Max excitation: 1

| $l'$ -matrix coefficients/(u <sup>1/2</sup> Å <sup>-1</sup> ) |                                       |                    |
|---------------------------------------------------------------|---------------------------------------|--------------------|
| O -0.000 100 391 100                                          | -7.427 531 200 000 × 10 <sup>-5</sup> | -0.000 782 015 391 |
| C -9.374 130 200 000 × 10 <sup>-5</sup>                       | -0.000 127 643 805                    | 0.001 373 825 243  |
| C 0.000 204 230 278                                           | -0.000 878 632 966                    | -0.002 504 298 353 |
| C 0.000 488 166 895                                           | 6.947 228 200 000 × 10 <sup>-5</sup>  | 0.000 227 584 955  |
| C 0.001 972 962 866                                           | -0.001 517 467 443                    | 0.001 918 624 911  |
| C 0.005 951 855 863                                           | 0.003 803 980 132                     | -0.010 932 948 147 |
| C 0.009 177 779 944                                           | 0.003 837 541 878                     | 0.000 918 979 811  |
| C 0.003 163 384 953                                           | -0.003 277 970 437                    | -0.004 541 166 264 |
| C -0.114 526 745 155                                          | 0.067 128 738 923                     | 0.032 588 777 464  |
| C 0.115 654 274 721                                           | -0.023 511 029 724                    | 0.066 208 922 837  |
| C 0.006 489 281 919                                           | 0.000 492 686 780                     | -0.000 430 829 292 |
| H 0.007 865 475 085                                           | 0.018 223 064 608                     | 0.023 115 391 366  |
| H -0.000 787 217 528                                          | 0.003 531 189 443                     | -0.009 525 007 432 |
| H -0.005 731 136 386                                          | 0.006 403 446 178                     | -0.004 782 256 464 |
| H -0.130 543 244 446                                          | -0.070 321 700 734                    | -0.195 236 760 657 |
| H -0.030 800 956 433                                          | -0.033 137 283 981                    | 0.013 685 746 587  |
| H -0.014 476 260 537                                          | 0.004 064 443 843                     | 0.017 711 671 340  |
| H 0.135 192 505 798                                           | -0.034 635 896 912                    | -0.178 581 302 705 |
| H -0.032 546 110 945                                          | -0.016 826 584 941                    | 0.005 446 512 183  |
| H 0.004 305 619 561                                           | 0.009 252 662 340                     | -0.003 567 351 747 |
| H 0.130 046 046 204                                           | 0.247 592 384 635                     | -0.062 285 136 269 |
| H -0.083 742 831 305                                          | -0.233 747 094 345                    | 0.084 948 896 489  |
| H 0.002 175 220 549                                           | 0.006 592 384 273                     | 0.005 962 569 373  |
| H -0.003 702 614 275                                          | 0.006 942 725 359                     | -0.012 993 922 546 |
| H 0.396 872 845 713                                           | -0.410 548 602 469                    | 0.150 834 146 524  |
| H -0.449 958 485 459                                          | 0.353 048 454 056                     | -0.133 358 429 654 |
| H -0.022 086 338 663                                          | -0.014 996 753 347                    | 0.008 917 955 469  |



Wavenumber/cm<sup>-1</sup>: 497.5894 , Max excitation: 1

| $l'$ -matrix coefficients/(u <sup>1/2</sup> Å <sup>-1</sup> ) |                    |                    |
|---------------------------------------------------------------|--------------------|--------------------|
| O                                                             | -0.000 375 401 654 | -0.002 122 411 884 |
| C                                                             | 0.000 744 390 088  | 0.001 273 228 110  |
| C                                                             | 0.000 286 505 971  | -0.000 969 468 897 |
| C                                                             | -0.003 636 679 103 | -0.000 935 421 980 |
| C                                                             | 0.002 896 868 221  | -0.000 414 626 571 |
| C                                                             | 0.026 438 293 991  | 0.023 331 684 951  |
| C                                                             | -0.227 829 385 523 | -0.096 193 858 383 |
| C                                                             | 0.012 224 266 936  | 0.026 586 977 936  |
| C                                                             | -0.003 639 811 247 | 0.002 140 065 452  |
| C                                                             | 0.002 048 078 577  | 0.000 534 073 510  |
| C                                                             | 0.016 057 984 028  | 0.002 127 431 454  |
| H                                                             | 0.011 642 376 809  | 0.024 928 094 521  |
| H                                                             | -0.026 919 865 451 | -0.075 990 125 852 |
| H                                                             | -0.005 159 210 857 | 0.004 777 577 196  |
| H                                                             | -0.003 542 801 555 | -0.001 926 118 070 |
| H                                                             | -0.101 300 430 457 | -0.106 813 565 924 |
| H                                                             | 0.004 184 342 922  | 0.000 690 587 554  |
| H                                                             | 0.005 678 633 745  | -0.001 520 789 524 |
| H                                                             | 0.810 771 543 087  | 0.419 952 346 190  |
| H                                                             | -0.039 960 995 182 | -0.095 413 583 872 |
| H                                                             | 0.003 670 255 951  | 0.007 108 508 070  |
| H                                                             | -0.002 592 090 380 | -0.008 069 144 883 |
| H                                                             | 0.007 227 637 295  | 0.017 026 467 022  |
| H                                                             | -0.007 605 643 270 | 0.014 998 923 845  |
| H                                                             | 0.011 555 922 095  | -0.012 068 316 917 |
| H                                                             | -0.011 730 944 456 | 0.007 648 077 918  |
| H                                                             | -0.052 364 728 803 | -0.040 095 109 699 |

Wavenumber/cm<sup>-1</sup>: 593.1099 , Max excitation: 1

| $l'$ -matrix coefficients/(u <sup>1/2</sup> Å <sup>-1</sup> ) |                    |                    |                    |
|---------------------------------------------------------------|--------------------|--------------------|--------------------|
| O                                                             | 0.000 266 960 740  | -0.008 770 767 426 | 0.003 327 237 673  |
| C                                                             | 0.006 260 782 017  | 0.010 750 447 644  | -0.004 418 225 315 |
| C                                                             | -0.022 698 383 862 | 0.053 793 529 153  | -0.025 754 970 558 |
| C                                                             | -0.018 114 867 490 | 0.013 850 579 532  | 0.001 001 237 023  |
| C                                                             | 0.023 591 391 853  | -0.036 760 657 469 | 0.005 787 019 032  |
| C                                                             | -0.041 969 486 595 | 0.003 476 958 639  | 0.095 670 708 233  |
| C                                                             | -0.048 570 414 023 | -0.020 783 008 133 | -0.052 795 741 260 |
| C                                                             | 0.038 283 995 066  | -0.173 503 481 194 | -0.093 789 876 123 |
| C                                                             | -0.021 498 581 168 | 0.051 577 721 634  | -0.077 254 144 801 |
| C                                                             | -0.019 075 372 878 | 0.031 511 316 050  | 0.025 434 135 222  |
| C                                                             | 0.002 090 348 924  | -0.002 854 523 311 | 0.002 272 869 688  |
| H                                                             | 0.143 744 713 468  | 0.116 796 396 685  | -0.116 580 662 097 |
| H                                                             | 0.141 084 246 284  | 0.056 329 861 513  | 0.018 444 227 469  |
| H                                                             | -0.009 083 578 013 | -0.017 821 315 023 | 0.017 626 861 087  |
| H                                                             | -0.097 424 410 256 | -0.291 572 694 125 | 0.159 907 646 908  |
| H                                                             | -0.003 574 269 450 | -0.098 198 044 387 | -0.196 679 508 569 |
| H                                                             | 0.111 951 622 485  | 0.476 640 698 505  | -0.046 143 959 752 |
| H                                                             | -0.040 288 532 505 | -0.143 941 791 928 | 0.005 817 721 629  |
| H                                                             | 0.029 628 373 482  | -0.032 512 444 266 | 0.145 553 105 070  |
| H                                                             | -0.252 677 686 877 | 0.209 285 724 635  | 0.356 871 059 495  |
| H                                                             | 0.140 857 575 064  | 0.011 145 609 341  | 0.297 775 240 880  |
| H                                                             | 0.096 220 990 254  | -0.074 596 557 047 | -0.113 154 264 274 |
| H                                                             | 0.011 121 485 088  | -0.003 950 956 854 | 0.001 791 756 627  |
| H                                                             | 0.001 364 817 553  | -0.008 939 400 711 | -0.003 475 973 410 |
| H                                                             | 0.046 522 672 639  | 0.014 786 693 190  | -0.134 126 983 979 |
| H                                                             | 0.032 677 774 628  | 0.060 718 810 011  | 0.027 453 241 645  |
| H                                                             | -0.002 120 811 632 | -0.001 243 671 036 | -0.006 817 943 245 |

Wavenumber/cm<sup>-1</sup>: 630.2699 , Max excitation: 3

| $l'$ -matrix coefficients/(u <sup>1/2</sup> Å <sup>-1</sup> ) |                    |                    |                    |
|---------------------------------------------------------------|--------------------|--------------------|--------------------|
| O                                                             | 0.001 313 304 594  | 0.006 231 925 889  | -0.001 857 159 548 |
| C                                                             | -0.004 224 365 405 | -0.015 380 494 338 | 0.005 423 186 881  |
| C                                                             | -0.012 080 441 492 | 0.063 304 779 596  | -0.032 234 330 860 |
| C                                                             | 0.038 557 929 088  | -0.007 509 899 647 | -0.003 873 821 842 |
| C                                                             | -0.012 649 912 885 | -0.000 730 403 703 | -0.008 716 510 995 |
| C                                                             | 0.059 127 306 135  | 0.011 377 279 824  | -0.162 029 885 960 |
| C                                                             | 0.065 471 623 767  | 0.013 715 194 920  | 0.071 935 562 155  |
| C                                                             | -0.001 063 067 762 | 0.032 850 478 076  | 0.021 269 636 905  |
| C                                                             | -0.026 029 511 223 | 0.085 585 251 664  | -0.057 752 995 222 |
| C                                                             | -0.005 553 392 003 | 0.047 242 226 728  | -0.039 611 566 079 |
| C                                                             | 0.011 962 543 206  | 0.024 104 754 100  | -0.008 499 845 239 |
| H                                                             | -0.251 410 044 582 | -0.210 677 699 324 | 0.213 820 596 908  |
| H                                                             | -0.210 640 835 006 | -0.087 662 118 826 | -0.028 083 059 903 |
| H                                                             | -0.011 897 360 432 | -0.000 807 035 328 | -0.001 594 286 559 |
| H                                                             | -0.020 581 465 899 | -0.387 136 852 646 | 0.155 829 624 123  |
| H                                                             | 0.030 341 053 911  | 0.154 989 579 496  | 0.358 994 447 655  |
| H                                                             | -0.009 535 501 732 | -0.065 229 053 718 | 0.012 207 902 795  |
| H                                                             | 0.117 508 689 666  | -0.192 901 136 775 | 0.109 601 808 529  |
| H                                                             | -0.048 690 657 165 | 0.049 024 838 527  | -0.223 347 225 167 |
| H                                                             | 0.043 158 697 011  | -0.030 723 442 679 | -0.056 571 889 764 |
| H                                                             | 0.121 727 864 432  | 0.037 411 568 893  | 0.332 652 000 968  |
| H                                                             | -0.007 147 091 991 | -0.034 510 474 406 | -0.140 172 158 526 |
| H                                                             | -0.009 109 924 871 | -0.060 179 591 987 | 0.069 871 270 080  |
| H                                                             | -0.039 802 551 596 | -0.078 185 572 990 | -0.031 788 071 525 |
| H                                                             | 0.005 133 939 850  | -0.051 871 370 641 | -0.229 919 017 445 |
| H                                                             | -0.072 819 419 286 | -0.001 643 458 832 | 0.206 186 406 947  |
| H                                                             | -0.033 332 223 892 | 0.056 539 728 560  | -0.001 252 533 815 |

Wavenumber/cm<sup>-1</sup>: 704.0003 , Max excitation: 2

| $l'$ -matrix coefficients/(u <sup>1/2</sup> Å <sup>-1</sup> ) |                    |                    |                                      |
|---------------------------------------------------------------|--------------------|--------------------|--------------------------------------|
| O                                                             | 0.002 798 027 111  | 0.005 251 827 942  | 3.323 041 500 000 × 10 <sup>-5</sup> |
| C                                                             | 0.004 516 113 498  | -0.006 894 086 299 | -0.003 344 279 735                   |
| C                                                             | -0.044 954 434 405 | 0.044 644 547 586  | 0.003 731 648 339                    |
| C                                                             | -0.033 639 418 038 | -0.021 808 752 284 | 0.002 991 582 731                    |
| C                                                             | 0.010 334 774 249  | 0.002 889 132 032  | 0.010 639 491 634                    |
| C                                                             | -0.034 525 168 614 | -0.003 636 129 485 | 0.103 740 541 452                    |
| C                                                             | 0.003 744 372 842  | 0.012 577 074 887  | 0.001 980 226 978                    |
| C                                                             | -0.038 807 755 747 | 0.123 085 910 602  | 0.049 522 089 361                    |
| C                                                             | -0.000 853 717 391 | 0.021 889 416 126  | -0.005 504 349 189                   |
| C                                                             | -0.069 496 614 245 | 0.100 367 093 601  | 0.046 850 726 693                    |
| C                                                             | -0.022 606 533 595 | -0.046 642 353 866 | 0.012 973 534 183                    |
| H                                                             | 0.182 774 904 022  | 0.128 051 906 112  | -0.138 780 730 157                   |
| H                                                             | 0.012 779 316 681  | -0.004 283 247 109 | -0.000 860 751 135                   |
| H                                                             | -0.012 409 429 814 | -0.007 889 503 365 | 0.006 800 732 711                    |
| H                                                             | 0.017 465 793 564  | -0.097 472 158 462 | 0.028 816 118 145                    |
| H                                                             | -0.020 274 873 683 | -0.098 995 793 395 | -0.241 681 311 616                   |
| H                                                             | -0.062 349 523 025 | -0.336 677 624 913 | 0.041 411 525 541                    |
| H                                                             | -0.099 616 814 141 | -0.410 412 210 210 | 0.025 020 717 253                    |
| H                                                             | 0.002 451 970 330  | 0.005 064 092 806  | 0.017 141 060 367                    |
| H                                                             | 0.189 615 871 903  | -0.148 816 007 565 | -0.243 160 569 537                   |
| H                                                             | 0.024 029 736 368  | 0.013 166 854 956  | 0.070 381 869 953                    |
| H                                                             | 0.310 172 659 609  | -0.211 823 718 319 | -0.283 105 555 292                   |
| H                                                             | -0.014 919 139 243 | 0.131 768 275 708  | -0.140 082 375 105                   |
| H                                                             | 0.075 717 497 535  | 0.170 601 824 122  | 0.073 973 628 497                    |
| H                                                             | 0.000 594 894 215  | -0.024 116 296 588 | -0.083 566 427 060                   |
| H                                                             | 0.097 790 142 109  | 0.188 794 083 780  | 0.078 868 542 969                    |
| H                                                             | 0.066 172 794 766  | -0.099 660 884 975 | 0.016 892 864 927                    |

Wavenumber/cm<sup>-1</sup>: 788.7609 , Max excitation: 2

| $l'$ -matrix coefficients/(u <sup>1/2</sup> Å <sup>-1</sup> ) |                    |                    |
|---------------------------------------------------------------|--------------------|--------------------|
| O                                                             | -0.003 898 679 334 | -0.011 681 352 276 |
| C                                                             | 0.003 512 279 744  | 0.010 397 000 863  |
| C                                                             | -0.026 796 897 143 | -0.004 983 757 156 |
| C                                                             | 0.042 288 681 660  | 0.064 389 481 277  |
| C                                                             | 0.008 017 887 230  | -0.003 344 840 410 |
| C                                                             | -0.034 858 865 397 | -0.011 913 583 953 |
| C                                                             | 0.023 909 807 721  | -0.007 363 407 179 |
| C                                                             | -0.008 295 697 118 | 0.031 087 839 383  |
| C                                                             | 0.003 815 675 278  | -0.013 206 891 116 |
| C                                                             | -0.024 366 775 252 | 0.017 778 111 180  |
| C                                                             | 0.070 975 554 972  | 0.143 520 030 304  |
| H                                                             | 0.105 407 635 856  | 0.104 187 509 468  |
| H                                                             | -0.089 850 513 509 | -0.010 333 559 601 |
| H                                                             | -0.006 326 732 471 | -0.001 997 612 195 |
| H                                                             | -0.016 471 013 152 | 0.043 381 638 746  |
| H                                                             | 0.006 125 413 446  | -0.082 659 294 044 |
| H                                                             | -0.021 514 145 972 | -0.078 200 319 479 |
| H                                                             | -0.093 064 729 681 | -0.076 694 143 261 |
| H                                                             | -0.016 421 364 466 | 0.008 955 056 742  |
| H                                                             | 0.046 121 551 292  | -0.038 732 907 124 |
| H                                                             | 0.010 633 371 552  | -0.012 619 979 032 |
| H                                                             | 0.130 438 578 936  | -0.070 529 882 475 |
| H                                                             | 0.025 803 673 764  | -0.393 477 744 688 |
| H                                                             | -0.186 179 274 144 | -0.515 266 907 272 |
| H                                                             | 0.018 884 514 845  | 0.025 838 981 636  |
| H                                                             | 0.076 575 922 537  | 0.082 015 605 648  |
| H                                                             | -0.175 541 278 637 | 0.281 282 465 484  |

Wavenumber/cm<sup>-1</sup>: 799.5457 , Max excitation: 1

| $l'$ -matrix coefficients/(u <sup>1/2</sup> Å <sup>-1</sup> ) |                    |                    |
|---------------------------------------------------------------|--------------------|--------------------|
| O                                                             | -0.002 273 172 610 | -0.006 086 634 495 |
| C                                                             | 0.003 271 426 763  | -0.002 711 907 174 |
| C                                                             | 0.091 581 787 176  | 0.082 489 749 192  |
| C                                                             | -0.023 096 073 609 | 0.023 148 607 891  |
| C                                                             | -0.012 864 931 074 | -0.033 293 951 606 |
| C                                                             | -0.020 000 245 369 | -0.002 789 984 070 |
| C                                                             | -0.027 726 576 162 | -0.009 080 531 271 |
| C                                                             | -0.005 805 157 097 | -0.010 060 096 151 |
| C                                                             | 0.065 499 156 454  | 0.032 700 733 026  |
| C                                                             | 0.034 713 208 296  | 0.051 784 377 865  |
| C                                                             | 0.012 623 919 351  | 0.010 740 846 049  |
| H                                                             | 0.074 126 422 287  | 0.070 636 491 841  |
| H                                                             | 0.092 666 184 114  | 0.046 958 233 771  |
| H                                                             | 0.016 989 373 117  | 0.008 192 324 848  |
| H                                                             | 0.258 082 781 636  | -0.041 712 791 233 |
| H                                                             | -0.001 943 148 844 | -0.060 590 518 998 |
| H                                                             | 0.008 987 402 299  | 0.024 510 771 592  |
| H                                                             | 0.266 608 200 462  | -0.182 300 806 895 |
| H                                                             | 0.022 745 710 991  | -0.023 769 543 187 |
| H                                                             | -0.007 388 237 227 | 0.014 726 531 115  |
| H                                                             | -0.339 594 340 583 | 0.161 557 021 871  |
| H                                                             | -0.241 020 771 285 | 0.061 274 189 604  |
| H                                                             | -0.035 142 991 008 | -0.062 498 658 172 |
| H                                                             | 0.016 372 364 314  | -0.059 202 999 758 |
| H                                                             | -0.272 809 384 001 | -0.306 384 574 061 |
| H                                                             | -0.248 297 094 936 | -0.169 167 773 791 |
| H                                                             | -0.009 338 182 682 | 0.048 637 430 498  |
|                                                               |                    | 0.001 993 179 131  |
|                                                               |                    | 0.001 112 093 855  |
|                                                               |                    | -0.022 941 513 766 |
|                                                               |                    | -0.016 390 619 137 |
|                                                               |                    | 0.011 600 991 615  |
|                                                               |                    | 0.058 037 308 407  |
|                                                               |                    | -0.029 097 907 799 |
|                                                               |                    | -0.016 980 140 001 |
|                                                               |                    | 0.094 346 703 728  |
|                                                               |                    | -0.098 362 424 494 |
|                                                               |                    | -0.017 406 225 138 |
|                                                               |                    | -0.066 446 384 077 |
|                                                               |                    | 0.016 591 237 352  |
|                                                               |                    | 0.008 158 238 223  |
|                                                               |                    | -0.117 123 881 991 |
|                                                               |                    | -0.119 449 108 451 |
|                                                               |                    | -0.001 324 333 552 |
|                                                               |                    | 0.192 262 025 172  |
|                                                               |                    | 0.099 492 080 450  |
|                                                               |                    | 0.038 882 899 434  |
|                                                               |                    | -0.143 314 987 893 |
|                                                               |                    | -0.156 720 572 520 |
|                                                               |                    | 0.071 054 401 249  |
|                                                               |                    | -0.038 778 830 944 |
|                                                               |                    | -0.082 368 498 344 |
|                                                               |                    | 0.362 778 820 719  |
|                                                               |                    | 0.052 919 393 351  |

Wavenumber/cm<sup>-1</sup>: 819.5477 , Max excitation: 1

| $l'$ -matrix coefficients/(u <sup>1/2</sup> Å <sup>-1</sup> ) |                    |                    |                    |
|---------------------------------------------------------------|--------------------|--------------------|--------------------|
| O                                                             | 0.000 208 305 339  | 0.008 757 657 438  | -0.002 533 836 666 |
| C                                                             | -0.000 686 153 044 | -0.010 461 128 157 | -0.005 305 972 700 |
| C                                                             | 0.026 020 972 523  | 0.013 396 911 637  | -0.001 434 457 628 |
| C                                                             | 0.015 251 001 621  | 0.004 791 490 485  | 0.094 927 567 040  |
| C                                                             | -0.005 893 691 098 | -0.023 478 445 471 | 0.002 410 790 818  |
| C                                                             | -0.039 163 307 098 | 0.001 888 521 869  | 0.065 782 616 932  |
| C                                                             | 0.061 981 317 991  | 0.001 466 956 932  | 0.043 908 235 848  |
| C                                                             | 0.004 433 890 294  | 0.029 359 989 018  | 0.014 849 259 541  |
| C                                                             | -0.001 468 605 102 | 0.038 234 783 313  | -0.009 294 247 204 |
| C                                                             | 0.039 267 575 936  | -0.037 118 231 141 | -0.008 659 222 600 |
| C                                                             | 0.026 232 602 729  | 0.011 537 161 480  | 0.135 048 378 240  |
| H                                                             | 0.120 749 038 067  | 0.122 742 181 106  | -0.123 009 703 800 |
| H                                                             | -0.200 565 427 256 | -0.099 545 635 906 | -0.038 036 976 706 |
| H                                                             | 0.016 842 292 380  | 0.009 794 175 020  | 0.001 357 478 132  |
| H                                                             | 0.035 937 597 458  | -0.144 997 651 211 | 0.033 402 582 163  |
| H                                                             | 0.003 397 970 855  | -0.094 060 798 601 | -0.190 012 576 851 |
| H                                                             | -0.011 622 753 267 | -0.048 330 646 129 | 0.005 663 731 890  |
| H                                                             | 0.020 912 631 493  | 0.151 079 649 453  | -0.020 531 634 562 |
| H                                                             | -0.059 009 133 907 | 0.066 214 359 913  | -0.197 722 421 286 |
| H                                                             | 0.023 972 750 276  | -0.017 447 126 781 | -0.036 756 337 510 |
| H                                                             | -0.008 453 380 081 | 0.037 983 785 634  | 0.095 862 857 039  |
| H                                                             | -0.154 036 720 054 | 0.089 465 858 702  | 0.084 651 112 588  |
| H                                                             | 0.353 701 954 416  | 0.129 961 064 659  | -0.196 223 821 419 |
| H                                                             | -0.355 267 312 965 | -0.050 071 119 537 | 0.100 820 031 833  |
| H                                                             | -0.044 592 930 270 | -0.066 398 715 961 | -0.086 782 965 577 |
| H                                                             | -0.054 628 462 180 | -0.099 852 393 839 | -0.035 960 145 738 |
| H                                                             | -0.123 033 509 707 | -0.123 669 024 043 | -0.533 488 279 391 |

Wavenumber/cm<sup>-1</sup>: 831.1254 , Max excitation: 2

| $l'$ -matrix coefficients/(u <sup>1/2</sup> Å <sup>-1</sup> ) |                    |                    |                    |
|---------------------------------------------------------------|--------------------|--------------------|--------------------|
| O                                                             | 0.000 636 795 486  | 0.011 489 517 725  | -0.004 060 706 416 |
| C                                                             | -0.003 419 969 963 | -0.012 807 520 434 | 0.004 238 170 782  |
| C                                                             | -0.024 028 202 115 | -0.013 478 306 357 | 0.011 687 202 141  |
| C                                                             | 0.039 424 056 182  | -0.008 252 272 212 | 0.049 004 163 734  |
| C                                                             | -0.004 193 346 458 | 0.016 430 551 277  | 0.008 473 548 564  |
| C                                                             | 0.031 761 735 789  | 0.009 290 481 564  | -0.110 858 159 665 |
| C                                                             | -0.001 105 034 347 | -0.002 189 102 488 | -0.002 468 641 557 |
| C                                                             | 0.034 093 765 585  | -0.083 181 810 321 | -0.028 629 724 436 |
| C                                                             | 0.037 232 687 876  | -0.071 291 939 423 | 0.055 744 600 806  |
| C                                                             | -0.069 727 789 507 | 0.088 018 652 342  | 0.013 696 175 954  |
| C                                                             | 0.010 582 647 018  | 0.013 610 852 102  | 0.069 911 846 419  |
| H                                                             | -0.136 873 049 485 | -0.126 894 655 751 | 0.121 254 473 500  |
| H                                                             | -0.026 975 841 355 | -0.024 022 632 996 | -0.012 561 559 891 |
| H                                                             | -0.001 492 508 361 | -0.011 244 493 677 | -0.017 491 734 993 |
| H                                                             | 0.023 377 615 722  | 0.310 538 229 201  | -0.124 397 560 400 |
| H                                                             | 0.017 627 900 811  | 0.092 716 549 472  | 0.214 569 833 529  |
| H                                                             | 0.029 589 293 167  | 0.215 978 303 624  | -0.037 954 888 555 |
| H                                                             | -0.026 127 546 077 | -0.339 574 198 091 | 0.056 861 054 519  |
| H                                                             | -0.009 242 830 208 | 0.003 207 618 450  | -0.031 909 244 109 |
| H                                                             | -0.135 788 410 126 | 0.098 527 547 483  | 0.153 615 104 825  |
| H                                                             | -0.128 480 785 597 | -0.013 386 558 732 | -0.280 093 160 358 |
| H                                                             | 0.262 996 583 689  | -0.168 678 756 211 | -0.212 567 459 979 |
| H                                                             | 0.197 473 809 572  | 0.055 096 552 778  | -0.092 840 372 176 |
| H                                                             | -0.207 977 661 194 | -0.042 526 161 928 | 0.048 986 734 285  |
| H                                                             | -0.023 287 079 099 | 0.018 495 352 983  | 0.174 704 036 379  |
| H                                                             | 0.066 953 323 562  | 0.160 165 959 020  | 0.105 992 858 452  |
| H                                                             | -0.079 051 074 564 | -0.053 763 348 591 | -0.294 387 423 356 |



Wavenumber/cm<sup>-1</sup>: 883.8432 , Max excitation: 1

| $l'$ -matrix coefficients/(u <sup>1/2</sup> Å <sup>-1</sup> ) |                    |                                       |                    |
|---------------------------------------------------------------|--------------------|---------------------------------------|--------------------|
| O                                                             | 0.001 243 137 689  | 0.003 246 013 810                     | 0.001 572 094 007  |
| C                                                             | -0.009 508 092 420 | -0.005 022 361 154                    | -0.005 261 937 705 |
| C                                                             | 0.014 817 033 270  | -0.000 495 519 368                    | 0.018 198 991 275  |
| C                                                             | 0.005 613 184 131  | -0.008 668 538 667                    | -0.013 846 551 907 |
| C                                                             | -0.000 579 168 334 | -0.023 411 489 357                    | -0.007 257 061 085 |
| C                                                             | -0.031 672 538 756 | 0.007 499 089 249                     | 0.055 295 561 444  |
| C                                                             | 0.169 728 054 437  | 0.005 839 553 243                     | 0.150 090 225 072  |
| C                                                             | 0.024 504 815 354  | -0.055 788 763 480                    | -0.019 522 998 553 |
| C                                                             | 0.034 460 830 010  | -0.003 907 148 235                    | 0.027 361 727 853  |
| C                                                             | -0.012 891 295 586 | -4.186 485 500 000 × 10 <sup>-5</sup> | 0.024 496 519 182  |
| C                                                             | -0.023 578 957 522 | -0.039 333 794 395                    | -0.053 474 021 733 |
| H                                                             | 0.093 217 789 022  | 0.063 947 662 705                     | -0.068 683 835 556 |
| H                                                             | -0.510 087 242 222 | -0.197 922 170 268                    | -0.067 887 381 973 |
| H                                                             | 0.012 654 427 575  | 0.013 571 361 030                     | 0.008 007 531 539  |
| H                                                             | 0.066 403 843 067  | 0.053 340 472 286                     | -0.053 072 534 339 |
| H                                                             | 0.002 762 432 109  | -0.063 879 452 687                    | -0.119 999 292 359 |
| H                                                             | 0.037 452 847 661  | 0.185 982 582 127                     | -0.018 499 474 642 |
| H                                                             | -0.058 705 279 643 | -0.002 693 411 551                    | -0.033 606 712 898 |
| H                                                             | -0.126 440 149 754 | 0.136 971 710 419                     | -0.513 409 717 628 |
| H                                                             | -0.100 691 988 761 | 0.085 584 700 346                     | 0.141 316 868 942  |
| H                                                             | -0.125 174 010 858 | 0.046 291 242 009                     | -0.097 402 360 433 |
| H                                                             | 0.054 412 016 540  | -0.026 853 464 233                    | -0.005 671 513 380 |
| H                                                             | -0.168 540 282 202 | 0.028 196 853 108                     | -0.003 596 930 754 |
| H                                                             | 0.189 532 652 774  | 0.136 034 761 906                     | 0.009 482 504 484  |
| H                                                             | -0.090 479 943 844 | -0.083 746 915 760                    | 0.030 288 341 766  |
| H                                                             | 0.043 203 238 330  | 0.032 497 523 216                     | -0.063 823 694 287 |
| H                                                             | 0.085 604 387 086  | 0.005 479 966 449                     | 0.242 468 338 616  |

Wavenumber/cm<sup>-1</sup>: 900.2208 , Max excitation: 1

| $l'$ -matrix coefficients/(u <sup>1/2</sup> Å <sup>-1</sup> ) |                    |                    |
|---------------------------------------------------------------|--------------------|--------------------|
| O                                                             | -0.000 161 099 353 | 0.009 441 100 590  |
| C                                                             | 0.002 711 836 560  | -0.015 064 713 734 |
| C                                                             | 0.010 237 284 852  | 0.011 706 930 081  |
| C                                                             | -0.002 205 566 341 | -0.001 163 283 922 |
| C                                                             | -0.005 054 817 846 | 0.007 273 340 939  |
| C                                                             | 0.026 052 301 581  | 0.004 906 523 273  |
| C                                                             | -0.034 955 896 463 | -0.000 815 281 482 |
| C                                                             | -0.000 441 412 811 | -0.009 652 833 523 |
| C                                                             | 0.084 619 299 050  | 0.102 599 724 578  |
| C                                                             | -0.065 144 469 272 | -0.065 778 322 307 |
| C                                                             | 0.004 481 508 336  | 0.002 980 040 362  |
| H                                                             | -0.080 645 195 596 | -0.068 580 403 602 |
| H                                                             | 0.101 944 924 916  | 0.037 045 787 511  |
| H                                                             | 0.002 656 128 397  | 0.001 072 546 950  |
| H                                                             | 0.250 378 448 137  | -0.256 227 847 175 |
| H                                                             | 0.004 015 199 666  | 0.057 594 495 050  |
| H                                                             | 0.009 890 720 515  | 0.004 094 138 743  |
| H                                                             | -0.221 440 288 764 | 0.169 560 019 367  |
| H                                                             | 0.025 208 411 619  | -0.026 332 254 108 |
| H                                                             | -0.012 988 300 576 | 0.001 533 678 879  |
| H                                                             | -0.291 676 154 323 | 0.193 993 874 622  |
| H                                                             | 0.234 829 856 426  | -0.072 287 333 175 |
| H                                                             | 0.012 062 971 044  | -0.004 603 043 656 |
| H                                                             | -0.020 417 237 521 | -0.012 300 455 376 |
| H                                                             | -0.310 643 737 207 | -0.370 497 653 999 |
| H                                                             | 0.236 654 352 366  | 0.177 767 072 461  |
| H                                                             | -0.009 263 729 603 | 0.002 857 139 777  |

Wavenumber/cm<sup>-1</sup>: 927.757 , Max excitation: 1

| $l'$ -matrix coefficients/(u <sup>1/2</sup> Å <sup>-1</sup> ) |                    |                    |
|---------------------------------------------------------------|--------------------|--------------------|
| O                                                             | -0.002 390 286 095 | -0.024 638 389 457 |
| C                                                             | -0.006 079 941 297 | 0.032 160 671 113  |
| C                                                             | 0.014 445 980 021  | 0.005 412 027 567  |
| C                                                             | -0.059 774 159 384 | 0.042 345 800 834  |
| C                                                             | -0.009 314 189 530 | -0.027 241 771 010 |
| C                                                             | -0.002 817 642 293 | 0.010 884 598 421  |
| C                                                             | -0.001 118 249 841 | 0.010 697 501 256  |
| C                                                             | -0.013 763 264 404 | 0.005 170 832 892  |
| C                                                             | 0.073 391 354 827  | -0.027 974 514 191 |
| C                                                             | 0.054 732 489 224  | 0.036 947 815 290  |
| C                                                             | 0.352 624 410 229  | -0.234 099 838 736 |
| H                                                             | 0.005 030 705 337  | -0.015 916 876 342 |
| H                                                             | 0.022 746 131 662  | -0.011 244 101 513 |
| H                                                             | 0.033 251 671 948  | 0.010 363 214 915  |
| H                                                             | -0.118 066 264 001 | 0.025 843 230 018  |
| H                                                             | 0.021 825 258 382  | -0.009 960 425 271 |
| H                                                             | 0.008 829 846 180  | -0.015 880 661 371 |
| H                                                             | -0.095 294 182 544 | -0.037 944 787 262 |
| H                                                             | 0.011 824 358 312  | -0.011 869 080 477 |
| H                                                             | 0.032 731 455 869  | -0.008 567 094 784 |
| H                                                             | -0.077 844 045 784 | 0.076 533 670 059  |
| H                                                             | -0.066 224 950 186 | -0.002 459 379 163 |
| H                                                             | -0.441 221 094 656 | 0.124 859 115 484  |
| H                                                             | -0.375 194 425 893 | 0.170 942 856 906  |
| H                                                             | -0.053 264 131 109 | -0.017 883 009 753 |
| H                                                             | -0.036 359 835 513 | -0.092 063 191 844 |
| H                                                             | -0.252 072 138 671 | 0.416 350 793 973  |
|                                                               |                    | -0.009 594 478 497 |

Wavenumber/cm<sup>-1</sup>: 941.2022 , Max excitation: 1

| $l'$ -matrix coefficients/(u <sup>1/2</sup> Å <sup>-1</sup> ) |                    |                    |
|---------------------------------------------------------------|--------------------|--------------------|
| O                                                             | -0.002 038 026 820 | -0.036 355 233 732 |
| C                                                             | 0.014 051 039 426  | 0.045 704 186 316  |
| C                                                             | -0.023 685 330 302 | -0.015 706 578 836 |
| C                                                             | -0.018 564 959 192 | 0.027 748 943 019  |
| C                                                             | 0.040 906 938 515  | 0.040 369 875 041  |
| C                                                             | -0.011 871 412 661 | -0.021 671 699 179 |
| C                                                             | -0.002 264 664 025 | -0.003 714 393 289 |
| C                                                             | 0.007 855 692 213  | -0.028 674 430 808 |
| C                                                             | -0.197 020 369 489 | 0.065 577 464 441  |
| C                                                             | -0.142 395 333 515 | -0.094 862 017 371 |
| C                                                             | 0.133 835 344 432  | -0.093 200 266 211 |
| H                                                             | 0.023 230 470 538  | 0.027 556 000 284  |
| H                                                             | -0.007 495 899 244 | -0.001 833 842 674 |
| H                                                             | -0.043 779 275 963 | -0.039 756 090 309 |
| H                                                             | 0.305 704 090 179  | -0.052 382 091 539 |
| H                                                             | -0.016 505 922 517 | -0.008 798 026 667 |
| H                                                             | 0.004 674 068 410  | 0.027 644 473 326  |
| H                                                             | 0.234 417 267 336  | 0.097 347 017 426  |
| H                                                             | 0.000 118 173 264  | -0.007 149 119 426 |
| H                                                             | -0.043 330 224 413 | 0.008 516 229 804  |
| H                                                             | 0.218 353 741 492  | -0.210 471 168 570 |
| H                                                             | 0.176 364 890 967  | 0.001 278 262 712  |
| H                                                             | -0.164 660 851 724 | 0.044 769 188 613  |
| H                                                             | -0.145 194 948 669 | 0.064 470 278 052  |
| H                                                             | 0.156 343 628 926  | 0.063 480 321 949  |
| H                                                             | 0.099 691 490 220  | 0.237 157 063 827  |
| H                                                             | -0.102 338 325 402 | 0.163 748 851 351  |

Wavenumber/cm<sup>-1</sup>: 954.2106 , Max excitation: 1

| $l'$ -matrix coefficients/(u <sup>1/2</sup> Å <sup>-1</sup> ) |                    |                    |
|---------------------------------------------------------------|--------------------|--------------------|
| O                                                             | -0.001 121 309 976 | -0.007 656 865 882 |
| C                                                             | -0.001 661 277 734 | 0.009 133 058 599  |
| C                                                             | 0.018 778 743 719  | -0.000 518 944 228 |
| C                                                             | 0.007 174 023 204  | -0.007 768 729 331 |
| C                                                             | -0.013 640 390 262 | -0.000 190 001 827 |
| C                                                             | -0.000 676 857 743 | 0.005 922 828 119  |
| C                                                             | -0.004 507 986 161 | 0.004 218 185 192  |
| C                                                             | 0.008 714 621 606  | -0.009 194 301 146 |
| C                                                             | -0.176 235 471 121 | 0.056 621 134 026  |
| C                                                             | 0.181 027 616 387  | 0.119 830 421 657  |
| C                                                             | -0.005 709 593 687 | 0.004 502 932 894  |
| H                                                             | -0.002 846 371 750 | -0.035 513 063 701 |
| H                                                             | 0.006 167 333 079  | -0.001 159 201 265 |
| H                                                             | 0.013 155 502 920  | 0.001 836 713 234  |
| H                                                             | 0.289 041 006 532  | -0.042 487 324 269 |
| H                                                             | 0.005 170 881 799  | 0.018 092 937 063  |
| H                                                             | -0.010 168 620 023 | 0.022 842 718 498  |
| H                                                             | -0.314 283 153 472 | -0.119 240 532 954 |
| H                                                             | 0.004 063 256 054  | -0.006 323 852 778 |
| H                                                             | -0.012 954 653 738 | 0.015 425 368 423  |
| H                                                             | 0.177 410 880 447  | -0.177 887 666 815 |
| H                                                             | -0.214 501 863 910 | -0.009 455 589 247 |
| H                                                             | 0.001 622 880 632  | -0.006 363 639 597 |
| H                                                             | 0.002 875 095 154  | -0.002 667 534 828 |
| H                                                             | 0.131 400 104 595  | 0.045 043 668 357  |
| H                                                             | -0.120 042 774 084 | -0.300 677 332 624 |
| H                                                             | 0.002 572 772 128  | -0.001 142 099 356 |
|                                                               |                    | 0.005 488 110 161  |

Wavenumber/cm<sup>-1</sup>: 970.7835 , Max excitation: 1

| $l'$ -matrix coefficients/(u <sup>1/2</sup> Å <sup>-1</sup> ) |                    |                    |                    |
|---------------------------------------------------------------|--------------------|--------------------|--------------------|
| O                                                             | 0.037 146 231 096  | 0.542 829 661 696  | -0.199 479 896 704 |
| C                                                             | -0.048 937 130 475 | -0.681 103 729 734 | 0.243 892 850 376  |
| C                                                             | 0.128 718 444 858  | -0.071 059 133 171 | 0.052 234 242 426  |
| C                                                             | -0.134 962 181 286 | -0.053 942 958 490 | 0.055 086 166 394  |
| C                                                             | -0.105 030 931 705 | 0.057 809 340 512  | -0.005 090 437 626 |
| C                                                             | 0.073 466 180 439  | 0.023 786 177 349  | -0.027 500 653 359 |
| C                                                             | 0.042 614 119 654  | 0.023 895 542 051  | -0.017 071 279 837 |
| C                                                             | 0.028 646 561 006  | -0.015 316 421 518 | 0.010 112 581 730  |
| C                                                             | -0.055 678 943 064 | 0.029 662 905 520  | -0.002 940 298 702 |
| C                                                             | -0.042 306 286 725 | 0.019 233 595 918  | -0.023 606 943 386 |
| C                                                             | 0.064 587 030 018  | 0.009 000 564 333  | -0.028 438 298 122 |
| H                                                             | -0.002 362 181 531 | 0.006 779 791 890  | -0.002 991 816 832 |
| H                                                             | 0.002 765 297 945  | -0.025 766 349 686 | -0.016 904 001 727 |
| H                                                             | 0.088 628 360 638  | 0.081 094 298 468  | -0.064 373 957 100 |
| H                                                             | 0.030 041 950 336  | -0.020 749 700 111 | -0.016 022 431 762 |
| H                                                             | -0.043 479 983 551 | 0.040 601 620 587  | -0.079 274 806 174 |
| H                                                             | -0.033 636 915 909 | 0.011 527 124 785  | -0.032 067 107 597 |
| H                                                             | 0.024 939 849 632  | -0.007 653 729 383 | 0.020 082 072 599  |
| H                                                             | -0.003 711 788 519 | 0.059 951 181 867  | 0.051 093 678 090  |
| H                                                             | -0.023 638 300 638 | 0.006 037 064 624  | -0.006 130 263 673 |
| H                                                             | 0.047 085 509 029  | -0.026 853 441 784 | 0.001 953 520 193  |
| H                                                             | 0.025 503 801 578  | -0.005 588 516 593 | 0.010 722 250 636  |
| H                                                             | -0.046 386 493 261 | -0.017 074 872 465 | 0.027 571 750 187  |
| H                                                             | -0.044 370 485 999 | -0.011 923 499 652 | 0.004 619 055 767  |
| H                                                             | -0.006 411 090 784 | 0.025 279 562 223  | 0.020 549 411 349  |
| H                                                             | -0.018 974 667 352 | -0.009 565 895 391 | -0.022 699 848 581 |
| H                                                             | 0.024 757 282 073  | 0.002 750 358 702  | 0.012 568 819 572  |

Wavenumber/cm<sup>-1</sup>: 1001.2088 , Max excitation: 1

| $l'$ -matrix coefficients/(u <sup>1/2</sup> Å <sup>-1</sup> ) |                    |                    |
|---------------------------------------------------------------|--------------------|--------------------|
| O                                                             | -0.006 581 050 291 | -0.052 850 360 079 |
| C                                                             | 0.027 088 756 388  | 0.047 940 658 988  |
| C                                                             | 0.109 731 349 834  | 0.047 037 311 572  |
| C                                                             | -0.275 572 525 760 | 0.237 082 807 517  |
| C                                                             | -0.108 144 112 280 | -0.290 598 366 137 |
| C                                                             | 0.153 208 259 798  | -0.096 198 388 113 |
| C                                                             | 0.164 221 040 966  | -0.269 065 385 766 |
| C                                                             | -0.072 719 292 836 | 0.140 687 628 961  |
| C                                                             | -0.043 852 486 427 | -0.018 118 058 551 |
| C                                                             | -0.034 553 068 252 | 0.005 837 429 729  |
| C                                                             | 0.081 911 579 173  | -0.048 181 287 465 |
| H                                                             | -0.243 609 961 694 | 0.135 404 978 700  |
| H                                                             | -0.135 210 190 118 | 0.316 508 076 021  |
| H                                                             | 0.133 204 357 853  | 0.317 721 906 021  |
| H                                                             | 0.031 413 297 578  | 0.012 719 281 198  |
| H                                                             | -0.026 545 817 723 | 0.023 437 207 919  |
| H                                                             | 0.003 103 730 627  | 0.007 803 491 778  |
| H                                                             | 0.006 696 602 206  | -0.001 220 348 550 |
| H                                                             | -0.105 582 683 050 | 0.260 001 376 077  |
| H                                                             | 0.169 193 309 007  | 0.027 171 762 848  |
| H                                                             | 0.015 275 736 326  | -0.015 256 248 397 |
| H                                                             | 0.040 230 451 660  | -0.020 518 780 900 |
| H                                                             | 0.022 798 468 172  | 0.012 828 307 905  |
| H                                                             | 0.049 128 371 208  | -0.038 389 823 004 |
| H                                                             | 0.026 939 350 569  | 0.031 411 712 330  |
| H                                                             | 0.014 461 673 444  | 0.016 334 881 850  |
| H                                                             | 0.020 167 842 433  | -0.034 579 023 825 |

Wavenumber/cm<sup>-1</sup>: 1012.7247 , Max excitation: 1

| $l'$ -matrix coefficients/(u <sup>1/2</sup> Å <sup>-1</sup> ) |                    |                    |                    |
|---------------------------------------------------------------|--------------------|--------------------|--------------------|
| O                                                             | 0.004 420 066 045  | 0.047 451 307 111  | -0.017 083 522 239 |
| C                                                             | -0.013 194 349 502 | -0.050 979 206 763 | 0.019 673 603 129  |
| C                                                             | 0.021 896 928 615  | 0.044 010 402 537  | -0.009 362 255 188 |
| C                                                             | 0.088 183 160 760  | -0.141 328 504 812 | -0.054 507 334 715 |
| C                                                             | 0.051 367 068 854  | -0.193 970 489 260 | 0.016 564 219 847  |
| C                                                             | -0.123 464 138 237 | 0.131 542 507 831  | -0.021 560 615 512 |
| C                                                             | -0.009 357 383 644 | 0.201 583 835 960  | 0.099 162 511 451  |
| C                                                             | -0.329 151 422 151 | 0.060 125 566 471  | -0.270 356 199 886 |
| C                                                             | -0.026 474 577 444 | -0.020 723 188 976 | 0.021 537 942 156  |
| C                                                             | -0.022 523 697 859 | -0.025 888 278 535 | -0.006 181 894 399 |
| C                                                             | -0.029 882 183 016 | 0.043 376 900 752  | 0.030 541 918 412  |
| H                                                             | 0.109 017 817 973  | -0.118 318 108 363 | 0.069 876 982 906  |
| H                                                             | 0.074 997 125 882  | -0.167 120 691 754 | -0.048 916 585 008 |
| H                                                             | 0.144 968 592 979  | 0.186 783 022 772  | 0.140 300 545 653  |
| H                                                             | 0.025 031 281 976  | 0.022 385 704 225  | -0.025 771 621 427 |
| H                                                             | 0.100 708 225 981  | -0.080 024 410 721 | 0.026 394 941 447  |
| H                                                             | 0.309 759 193 256  | -0.032 821 017 771 | 0.246 860 298 999  |
| H                                                             | 0.016 840 487 161  | 0.025 412 969 577  | 0.008 726 449 160  |
| H                                                             | 0.107 999 914 800  | -0.173 646 783 458 | -0.038 168 187 204 |
| H                                                             | 0.407 535 507 452  | -0.033 738 494 864 | 0.329 667 536 125  |
| H                                                             | 0.003 539 685 051  | -0.014 293 021 332 | -0.009 812 370 185 |
| H                                                             | 0.013 336 673 344  | -0.007 434 626 558 | 0.014 536 659 584  |
| H                                                             | -0.017 457 384 465 | 0.015 728 301 521  | 0.004 394 183 656  |
| H                                                             | -0.007 615 002 354 | -0.022 045 226 039 | -0.010 433 363 427 |
| H                                                             | 0.028 248 205 000  | 0.019 466 068 715  | -0.018 802 130 952 |
| H                                                             | 0.025 440 362 758  | 0.033 991 175 098  | 0.003 371 759 809  |
| H                                                             | -0.004 710 495 747 | -0.008 205 221 303 | -0.021 833 226 209 |



Wavenumber/cm<sup>-1</sup>: 1028.4096 , Max excitation: 1

| $l'$ -matrix coefficients/(u <sup>1/2</sup> Å <sup>-1</sup> ) |                    |                    |                    |
|---------------------------------------------------------------|--------------------|--------------------|--------------------|
| O                                                             | -0.008 160 722 421 | -0.075 263 985 954 | 0.026 120 545 389  |
| C                                                             | 0.006 529 298 643  | 0.090 994 861 414  | -0.030 954 248 577 |
| C                                                             | 0.123 630 134 075  | 0.044 609 047 289  | -0.030 145 426 311 |
| C                                                             | 0.115 696 289 634  | -0.075 360 200 020 | 0.103 843 709 714  |
| C                                                             | -0.386 020 602 807 | -0.204 996 747 278 | 0.228 692 727 278  |
| C                                                             | -0.027 277 326 492 | 0.162 472 593 160  | -0.124 438 486 816 |
| C                                                             | -0.020 757 402 359 | 0.061 629 700 804  | -0.092 431 468 780 |
| C                                                             | 0.170 275 182 302  | 0.023 901 804 690  | 0.070 429 825 052  |
| C                                                             | -0.035 507 312 036 | -0.002 368 694 444 | -0.005 452 619 282 |
| C                                                             | -0.051 026 391 229 | -0.015 865 960 067 | -0.002 014 383 566 |
| C                                                             | -0.047 943 684 485 | 0.023 885 719 456  | -0.046 057 033 515 |
| H                                                             | 0.013 801 644 013  | -0.031 094 497 691 | 0.011 710 806 564  |
| H                                                             | -0.023 485 451 952 | -0.020 129 003 616 | -0.041 009 992 562 |
| H                                                             | 0.386 689 367 278  | 0.143 732 207 124  | -0.249 236 674 410 |
| H                                                             | 0.024 798 819 896  | -0.004 377 418 622 | -0.019 577 081 849 |
| H                                                             | 0.242 514 180 269  | -0.183 832 463 649 | -0.021 722 611 593 |
| H                                                             | -0.363 157 867 140 | -0.009 246 788 124 | -0.294 708 919 492 |
| H                                                             | 0.041 509 232 969  | 0.027 364 610 179  | 0.031 819 781 603  |
| H                                                             | 0.048 484 938 926  | -0.074 684 590 540 | 0.018 310 034 097  |
| H                                                             | 0.088 946 507 073  | 0.019 086 567 277  | 0.110 546 626 075  |
| H                                                             | 0.016 740 466 062  | -0.003 858 212 460 | 0.033 740 229 675  |
| H                                                             | 0.037 617 238 886  | -0.020 011 386 194 | 0.008 964 158 614  |
| H                                                             | 0.009 872 397 862  | -0.026 250 610 978 | 0.018 879 712 135  |
| H                                                             | -0.025 397 478 178 | 0.039 679 442 864  | 0.010 652 734 640  |
| H                                                             | 0.020 888 031 011  | 0.026 915 201 268  | -0.001 777 662 598 |
| H                                                             | 0.026 814 402 688  | 0.039 348 725 129  | -0.011 538 773 861 |
| H                                                             | 0.011 964 825 391  | 0.001 287 806 412  | 0.044 159 196 961  |

Wavenumber/cm<sup>-1</sup>: 1073.9261 , Max excitation: 1

| $l'$ -matrix coefficients/(u <sup>1/2</sup> Å <sup>-1</sup> ) |                    |                    |                    |
|---------------------------------------------------------------|--------------------|--------------------|--------------------|
| O                                                             | 0.003 448 953 914  | 0.024 800 970 164  | -0.009 628 270 117 |
| C                                                             | -0.004 668 484 863 | -0.035 740 354 521 | 0.022 851 525 830  |
| C                                                             | 0.022 628 495 291  | 0.028 039 576 647  | -0.089 929 115 104 |
| C                                                             | -0.125 453 972 593 | 0.030 143 548 287  | -0.175 177 781 346 |
| C                                                             | 0.149 475 006 925  | 0.056 706 737 026  | 0.200 451 072 429  |
| C                                                             | -0.275 600 462 828 | 0.174 053 553 390  | -0.103 121 500 126 |
| C                                                             | 0.130 161 988 648  | -0.220 785 908 674 | -0.027 575 151 622 |
| C                                                             | -0.059 967 345 517 | 0.004 087 731 431  | -0.011 710 624 222 |
| C                                                             | -0.011 835 141 875 | -0.011 680 876 980 | 0.023 626 929 635  |
| C                                                             | -0.017 468 441 304 | -0.033 772 019 563 | 0.024 951 699 609  |
| C                                                             | 0.049 551 020 194  | -0.002 251 066 718 | 0.101 037 803 018  |
| H                                                             | 0.383 093 845 333  | -0.305 971 625 281 | 0.104 241 416 536  |
| H                                                             | -0.112 573 444 564 | 0.303 084 887 090  | 0.120 783 361 247  |
| H                                                             | 0.062 715 286 271  | -0.208 372 929 812 | -0.209 527 677 510 |
| H                                                             | -0.011 024 955 555 | 0.012 927 227 776  | 0.005 304 106 964  |
| H                                                             | 0.185 393 563 975  | -0.141 808 400 334 | 0.105 190 251 266  |
| H                                                             | 0.074 376 121 346  | -0.002 148 346 921 | 0.066 751 920 213  |
| H                                                             | 0.019 493 860 927  | 0.035 425 009 525  | 0.015 027 570 065  |
| H                                                             | -0.125 243 280 208 | 0.289 247 099 517  | 0.096 743 117 001  |
| H                                                             | -0.005 186 438 537 | -0.012 618 279 588 | -0.027 116 727 742 |
| H                                                             | -0.016 041 186 351 | 0.005 881 291 495  | 0.011 667 078 931  |
| H                                                             | -0.019 061 473 468 | -0.009 246 719 913 | -0.016 621 240 611 |
| H                                                             | -0.044 452 713 162 | 0.051 460 597 252  | -0.017 528 549 359 |
| H                                                             | 0.067 931 068 385  | -0.081 384 594 104 | -0.031 942 448 428 |
| H                                                             | 0.005 927 206 675  | 0.004 815 735 542  | -0.001 392 609 500 |
| H                                                             | 0.019 948 309 079  | 0.020 031 743 128  | -0.003 129 681 258 |
| H                                                             | -0.004 791 119 551 | -0.021 472 724 576 | -0.060 668 291 127 |

Wavenumber/cm<sup>-1</sup>: 1105.3988 , Max excitation: 1

| $l'$ -matrix coefficients/(u <sup>1/2</sup> Å <sup>-1</sup> ) |                    |                    |                    |
|---------------------------------------------------------------|--------------------|--------------------|--------------------|
| O                                                             | 0.000 746 878 621  | 0.006 832 953 233  | -0.005 011 363 580 |
| C                                                             | -0.011 532 641 461 | 0.019 899 323 253  | -0.008 772 233 919 |
| C                                                             | -0.088 987 126 742 | -0.039 576 333 653 | 0.228 810 295 385  |
| C                                                             | 0.233 650 806 317  | -0.270 666 187 164 | -0.000 888 115 922 |
| C                                                             | 0.001 451 929 920  | -0.171 502 587 599 | -0.289 170 002 552 |
| C                                                             | -0.134 008 206 332 | 0.182 603 613 806  | 0.026 780 798 341  |
| C                                                             | -0.086 097 920 061 | -0.114 501 290 015 | 0.010 467 871 790  |
| C                                                             | 0.125 161 876 968  | 0.161 224 282 372  | 0.080 558 068 007  |
| C                                                             | 0.024 049 203 800  | 0.003 059 961 814  | -0.045 355 395 869 |
| C                                                             | 0.040 297 633 607  | 0.043 690 455 218  | -0.081 500 322 141 |
| C                                                             | -0.068 093 891 691 | 0.084 957 616 137  | 0.018 194 563 749  |
| H                                                             | 0.063 802 568 913  | -0.089 657 627 999 | 0.083 290 646 158  |
| H                                                             | 0.127 851 500 220  | -0.100 868 192 101 | -0.012 892 813 952 |
| H                                                             | 0.123 788 374 029  | 0.312 589 865 024  | 0.184 274 546 705  |
| H                                                             | 0.025 699 760 270  | -0.019 879 143 605 | -0.017 750 299 610 |
| H                                                             | 0.119 213 587 535  | -0.104 174 612 141 | -0.006 075 104 941 |
| H                                                             | 0.108 251 755 218  | -0.033 118 435 943 | 0.099 783 370 040  |
| H                                                             | -0.044 030 873 240 | -0.068 981 535 727 | -0.043 559 461 872 |
| H                                                             | -0.160 836 633 263 | 0.253 333 830 432  | 0.055 591 608 063  |
| H                                                             | -0.345 651 059 607 | 0.111 190 187 397  | -0.222 188 423 104 |
| H                                                             | 0.028 664 465 901  | -0.016 218 420 607 | -0.026 791 734 569 |
| H                                                             | 0.020 498 902 986  | 0.038 851 059 445  | 0.073 484 182 872  |
| H                                                             | -0.087 186 474 519 | 0.030 135 650 160  | 0.017 544 388 727  |
| H                                                             | -0.053 912 605 311 | 0.014 797 422 020  | 0.008 758 124 423  |
| H                                                             | 0.004 273 434 086  | -0.005 092 865 458 | -0.010 447 321 099 |
| H                                                             | -0.035 660 659 908 | -0.026 600 588 862 | 0.038 051 642 540  |
| H                                                             | -0.021 639 037 979 | 0.024 468 612 451  | 0.009 029 893 574  |

Wavenumber/cm<sup>-1</sup>: 1135.4342 , Max excitation: 1

| $l'$ -matrix coefficients/(u <sup>1/2</sup> Å <sup>-1</sup> ) |                    |                    |                    |
|---------------------------------------------------------------|--------------------|--------------------|--------------------|
| O                                                             | 0.005 124 620 895  | 0.113 554 065 142  | -0.038 934 368 116 |
| C                                                             | -0.011 433 295 307 | -0.137 185 164 575 | 0.039 723 390 873  |
| C                                                             | -0.158 647 025 040 | 0.056 199 289 204  | 0.128 830 632 733  |
| C                                                             | 0.289 101 171 516  | -0.033 080 809 460 | -0.195 684 321 310 |
| C                                                             | 0.077 537 207 736  | -0.057 395 287 351 | -0.215 749 708 324 |
| C                                                             | -0.106 369 113 893 | 0.053 025 850 272  | 0.089 083 664 346  |
| C                                                             | 0.043 767 507 643  | 0.027 913 393 223  | -0.082 025 784 999 |
| C                                                             | -0.053 913 393 436 | -0.047 881 116 866 | 0.231 071 849 835  |
| C                                                             | 0.047 145 135 871  | -0.026 111 942 784 | -0.018 133 181 534 |
| C                                                             | 0.059 352 668 714  | -0.010 957 844 302 | -0.046 926 469 257 |
| C                                                             | -0.084 307 887 703 | -0.012 451 514 142 | 0.092 002 669 939  |
| H                                                             | -0.009 716 664 758 | 0.007 434 953 588  | 0.026 742 385 953  |
| H                                                             | -0.220 042 949 845 | 0.390 323 263 238  | 0.105 232 890 532  |
| H                                                             | -0.181 654 168 133 | 0.003 903 607 438  | 0.180 653 193 902  |
| H                                                             | 0.002 203 501 729  | 0.006 567 436 841  | -0.005 887 220 485 |
| H                                                             | 0.136 477 875 004  | -0.123 975 666 053 | 0.061 795 383 718  |
| H                                                             | -0.232 740 125 598 | 0.156 052 597 738  | -0.138 824 541 916 |
| H                                                             | -0.058 186 099 502 | -0.027 131 494 534 | -0.057 931 351 525 |
| H                                                             | 0.184 202 229 906  | -0.326 586 110 989 | -0.054 584 171 795 |
| H                                                             | 0.126 971 153 956  | -0.086 690 327 153 | 0.013 760 888 286  |
| H                                                             | -0.014 404 248 797 | 0.007 094 550 558  | -0.012 100 666 514 |
| H                                                             | -0.030 697 033 367 | 0.030 525 611 575  | 0.030 779 941 603  |
| H                                                             | -0.034 301 321 522 | 0.079 824 945 136  | -0.055 854 993 725 |
| H                                                             | 0.042 087 231 489  | 0.010 343 711 335  | 0.007 339 437 782  |
| H                                                             | 0.017 668 895 068  | -0.012 031 629 079 | -0.042 072 102 371 |
| H                                                             | -0.002 387 442 134 | 0.003 117 631 690  | 0.051 279 257 231  |
| H                                                             | -0.098 804 101 460 | 0.077 532 623 226  | -0.031 819 636 921 |

Wavenumber/cm<sup>-1</sup>: 1158.4551 , Max excitation: 1

| $l'$ -matrix coefficients/(u <sup>1/2</sup> Å <sup>-1</sup> ) |                                       |                    |
|---------------------------------------------------------------|---------------------------------------|--------------------|
| O                                                             | -0.008 263 976 119                    | -0.027 744 339 576 |
| C                                                             | 0.011 439 460 537                     | 0.078 083 063 624  |
| C                                                             | -0.313 685 344 820                    | -0.460 048 662 393 |
| C                                                             | -0.007 725 213 226                    | -0.052 444 370 741 |
| C                                                             | -0.031 315 802 403                    | 0.175 597 674 160  |
| C                                                             | 0.065 607 071 695                     | -0.051 521 372 883 |
| C                                                             | 0.080 125 999 420                     | -0.027 655 907 393 |
| C                                                             | -0.102 504 405 058                    | -0.020 363 972 282 |
| C                                                             | 0.158 385 502 471                     | 0.219 489 226 061  |
| C                                                             | 0.144 764 086 055                     | 0.158 259 752 724  |
| C                                                             | -4.297 937 000 000 × 10 <sup>-5</sup> | 0.043 270 783 846  |
| H                                                             | 0.063 090 767 273                     | -0.016 511 172 821 |
| H                                                             | -0.085 897 360 757                    | 0.123 139 448 805  |
| H                                                             | 0.201 121 026 269                     | 0.108 713 670 715  |
| H                                                             | -0.097 738 131 169                    | -0.116 834 726 821 |
| H                                                             | -0.107 816 038 459                    | 0.095 765 890 116  |
| H                                                             | -0.003 154 862 592                    | 0.044 560 062 281  |
| H                                                             | -0.084 515 718 314                    | -0.163 330 984 667 |
| H                                                             | 0.011 326 715 366                     | 0.029 508 220 776  |
| H                                                             | 0.154 221 455 645                     | -0.034 473 742 393 |
| H                                                             | 0.141 237 151 088                     | -0.063 521 072 955 |
| H                                                             | 0.075 617 261 965                     | 0.103 048 405 786  |
| H                                                             | -0.014 583 699 725                    | -0.012 326 914 258 |
| H                                                             | -0.043 783 298 293                    | 0.016 614 874 950  |
| H                                                             | -0.127 447 212 541                    | -0.108 673 181 311 |
| H                                                             | -0.095 264 284 630                    | -0.085 161 808 655 |
| H                                                             | 0.029 083 670 985                     | -0.026 303 932 637 |

Wavenumber/cm<sup>-1</sup>: 1164.8891 , Max excitation: 1

| $l'$ -matrix coefficients/(u <sup>1/2</sup> Å <sup>-1</sup> ) |                    |                    |
|---------------------------------------------------------------|--------------------|--------------------|
| O                                                             | -0.016 298 300 986 | 0.026 335 201 801  |
| C                                                             | 0.056 722 250 873  | -0.061 883 348 957 |
| C                                                             | -0.006 569 385 546 | -0.051 084 561 929 |
| C                                                             | -0.089 165 704 271 | 0.521 298 749 383  |
| C                                                             | 0.006 749 166 405  | -0.019 420 726 595 |
| C                                                             | -0.107 235 910 629 | -0.037 771 894 969 |
| C                                                             | -0.115 735 191 685 | -0.027 646 922 415 |
| C                                                             | -0.014 278 019 695 | -0.045 124 293 034 |
| C                                                             | 0.002 567 989 947  | 0.018 817 369 932  |
| C                                                             | 0.008 603 350 036  | 0.033 612 816 122  |
| C                                                             | 0.022 822 997 224  | -0.234 766 759 906 |
| H                                                             | -0.038 219 665 307 | 0.084 556 140 344  |
| H                                                             | 0.081 389 951 685  | -0.011 981 101 531 |
| H                                                             | 0.205 682 183 365  | 0.064 874 734 710  |
| H                                                             | 0.036 552 298 381  | -0.031 110 578 411 |
| H                                                             | 0.254 324 283 940  | -0.197 288 350 842 |
| H                                                             | 0.181 295 408 007  | -0.044 096 237 532 |
| H                                                             | -0.038 971 546 639 | -0.063 023 444 296 |
| H                                                             | 0.068 628 803 979  | -0.262 758 848 334 |
| H                                                             | -0.193 074 939 124 | 0.005 585 491 598  |
| H                                                             | 0.045 779 440 754  | -0.018 441 053 256 |
| H                                                             | 0.023 650 111 053  | 0.021 517 443 265  |
| H                                                             | 0.203 220 305 000  | -0.048 531 654 661 |
| H                                                             | 0.163 447 768 094  | 0.015 016 654 598  |
| H                                                             | -0.009 753 587 582 | 0.008 167 507 644  |
| H                                                             | -0.039 822 687 022 | -0.032 900 549 952 |
| H                                                             | -0.066 188 975 893 | 0.073 997 012 759  |

Wavenumber/cm<sup>-1</sup>: 1184.7655 , Max excitation: 1

| $l'$ -matrix coefficients/(u <sup>1/2</sup> Å <sup>-1</sup> ) |                    |                    |                    |
|---------------------------------------------------------------|--------------------|--------------------|--------------------|
| O                                                             | 0.016 762 802 895  | 0.094 216 980 550  | -0.038 602 228 096 |
| C                                                             | -0.020 074 134 843 | -0.114 607 280 363 | 0.024 922 869 624  |
| C                                                             | -0.317 678 746 526 | 0.144 156 096 333  | -0.063 563 963 081 |
| C                                                             | 0.116 339 036 906  | 0.088 271 482 328  | 0.380 889 702 716  |
| C                                                             | 0.089 340 285 966  | -0.125 560 231 171 | 0.052 878 617 358  |
| C                                                             | -0.041 249 471 533 | 0.055 234 342 414  | -0.143 207 751 642 |
| C                                                             | -0.014 367 604 306 | -0.127 429 908 961 | -0.112 748 564 978 |
| C                                                             | 0.007 786 659 213  | 0.086 077 867 173  | -0.048 288 627 475 |
| C                                                             | 0.131 187 331 930  | -0.051 903 065 042 | 0.073 236 883 376  |
| C                                                             | 0.133 099 839 985  | -0.081 899 677 902 | -0.014 257 043 421 |
| C                                                             | -0.052 851 748 431 | -0.040 693 054 830 | -0.199 364 884 655 |
| H                                                             | -0.147 928 733 187 | 0.146 008 731 027  | -0.097 364 853 002 |
| H                                                             | 0.008 417 630 744  | -0.021 856 257 151 | -0.026 056 840 383 |
| H                                                             | -0.150 379 184 179 | -0.197 927 241 603 | 0.021 885 428 350  |
| H                                                             | -0.097 489 512 631 | 0.066 434 456 476  | 0.067 041 266 284  |
| H                                                             | 0.201 148 016 436  | -0.140 172 290 304 | 0.055 912 782 455  |
| H                                                             | 0.034 189 979 308  | -0.041 272 562 945 | 0.025 411 716 520  |
| H                                                             | -0.096 241 394 138 | 0.012 661 818 835  | -0.096 630 969 210 |
| H                                                             | -0.113 855 969 361 | 0.212 640 613 746  | 0.072 045 044 881  |
| H                                                             | 0.131 432 214 472  | 0.023 130 853 789  | 0.126 809 000 134  |
| H                                                             | -0.058 335 618 444 | 0.016 963 652 210  | -0.067 885 535 841 |
| H                                                             | -0.086 061 698 106 | 0.034 226 034 131  | 0.010 519 810 770  |
| H                                                             | 0.143 853 050 820  | -0.137 047 500 383 | 0.041 519 950 424  |
| H                                                             | -0.109 087 256 896 | 0.163 469 678 221  | 0.068 334 514 655  |
| H                                                             | 0.068 353 330 927  | -0.037 203 973 619 | -0.153 118 283 776 |
| H                                                             | 0.062 355 615 190  | 0.075 858 966 946  | 0.136 846 662 835  |
| H                                                             | 0.033 999 197 574  | 0.029 870 006 941  | 0.139 407 299 897  |

Wavenumber/cm<sup>-1</sup>: 1204.2572 , Max excitation: 1

| $l'$ -matrix coefficients/(u <sup>1/2</sup> Å <sup>-1</sup> ) |                    |                    |                    |
|---------------------------------------------------------------|--------------------|--------------------|--------------------|
| O                                                             | 0.010 211 337 539  | -0.021 108 534 238 | 0.003 874 380 720  |
| C                                                             | 0.000 767 255 128  | 0.003 040 030 674  | -0.011 710 228 722 |
| C                                                             | -0.240 186 262 938 | 0.188 165 252 651  | 0.296 357 854 433  |
| C                                                             | -0.404 392 121 025 | 0.057 906 650 810  | -0.171 111 931 089 |
| C                                                             | -0.018 769 718 348 | -0.108 864 295 476 | -0.037 258 994 795 |
| C                                                             | 0.112 654 444 647  | 0.144 543 974 385  | 0.118 219 887 844  |
| C                                                             | 0.026 257 815 628  | 0.155 224 607 921  | 0.021 453 071 492  |
| C                                                             | 0.113 900 676 595  | -0.070 883 152 530 | -0.021 523 037 500 |
| C                                                             | 0.108 208 773 292  | -0.064 189 036 926 | -0.061 053 197 591 |
| C                                                             | 0.124 164 301 714  | -0.075 330 194 003 | -0.147 445 381 503 |
| C                                                             | 0.191 453 711 848  | -0.015 836 396 887 | 0.110 145 350 893  |
| H                                                             | -0.014 451 622 114 | -0.114 194 325 558 | 0.169 160 783 959  |
| H                                                             | 0.078 487 926 623  | -0.264 119 721 115 | -0.105 566 240 402 |
| H                                                             | -0.072 112 863 684 | -0.115 680 442 402 | -0.031 966 781 325 |
| H                                                             | 0.009 650 406 582  | 0.033 123 144 218  | -0.027 331 593 360 |
| H                                                             | 0.056 436 469 838  | -0.040 443 041 109 | -0.086 170 106 375 |
| H                                                             | -0.138 828 933 375 | -0.023 826 933 382 | -0.138 900 816 580 |
| H                                                             | -0.163 767 808 452 | -0.067 816 952 581 | -0.163 459 302 669 |
| H                                                             | 0.009 064 264 483  | 0.043 411 327 616  | 0.034 191 336 432  |
| H                                                             | 0.058 877 287 043  | -0.005 237 592 561 | 0.069 172 514 240  |
| H                                                             | -0.010 584 606 295 | 0.006 045 152 712  | -0.026 666 147 613 |
| H                                                             | -0.069 233 801 143 | 0.061 058 247 652  | 0.078 519 393 651  |
| H                                                             | -0.091 413 689 777 | 0.062 764 191 292  | -0.010 220 723 567 |
| H                                                             | 0.102 566 777 293  | -0.165 706 442 980 | -0.068 138 319 768 |
| H                                                             | 0.068 690 925 235  | -0.005 878 485 862 | -0.091 132 502 436 |
| H                                                             | 0.018 709 377 260  | 0.043 693 272 374  | 0.152 945 185 678  |
| H                                                             | 0.068 696 119 973  | -0.101 049 135 692 | -0.101 516 124 115 |



Wavenumber/cm<sup>-1</sup>: 1221.4601 , Max excitation: 1

| $l'$ -matrix coefficients/(u <sup>1/2</sup> Å <sup>-1</sup> ) |                    |                    |
|---------------------------------------------------------------|--------------------|--------------------|
| O -0.000 507 237 426                                          | 0.071 463 527 409  | -0.018 543 203 116 |
| C 0.002 354 541 307                                           | -0.079 266 027 548 | 0.049 590 503 378  |
| C -0.125 351 621 379                                          | -0.195 073 505 598 | -0.425 199 489 555 |
| C 0.090 520 396 190                                           | 0.054 545 296 895  | -0.305 234 919 616 |
| C -0.139 284 264 191                                          | -0.041 349 553 222 | 0.072 138 630 900  |
| C 0.028 875 005 222                                           | -0.027 921 846 852 | 0.136 348 632 445  |
| C -0.088 287 744 911                                          | -0.013 344 479 170 | 0.182 013 324 896  |
| C 0.179 681 258 153                                           | 0.097 891 493 437  | -0.148 454 158 264 |
| C 0.082 481 828 117                                           | 0.109 434 788 536  | 0.185 683 066 805  |
| C 0.071 604 063 276                                           | 0.058 361 652 287  | 0.120 794 018 442  |
| C -0.028 410 668 990                                          | -0.041 669 089 696 | 0.185 067 984 080  |
| H -0.133 208 469 156                                          | 0.085 114 189 436  | 0.010 455 008 701  |
| H 0.164 295 474 704                                           | -0.062 270 551 102 | 0.036 252 966 738  |
| H -0.079 446 773 713                                          | 0.005 808 779 737  | 0.080 983 229 065  |
| H -0.194 838 234 104                                          | 0.012 697 660 268  | 0.189 787 028 936  |
| H 0.133 842 043 202                                           | -0.129 521 847 284 | 0.034 002 039 372  |
| H -0.043 853 689 897                                          | -0.148 720 209 014 | -0.077 066 825 853 |
| H 0.039 142 058 507                                           | 0.036 676 202 692  | 0.044 096 053 353  |
| H -0.072 152 465 071                                          | 0.053 923 745 416  | -0.090 233 113 990 |
| H -0.045 452 021 222                                          | 0.109 117 597 074  | 0.079 571 041 346  |
| H -0.001 432 955 110                                          | -0.014 272 372 703 | -0.147 352 951 466 |
| H 0.028 329 985 704                                           | 0.008 640 500 104  | 0.015 156 489 933  |
| H -0.073 806 922 367                                          | 0.122 253 658 153  | -0.073 732 304 714 |
| H 0.159 012 032 455                                           | -0.105 885 303 629 | -0.052 605 920 936 |
| H -0.044 090 667 604                                          | -0.078 220 204 189 | -0.083 712 078 991 |
| H 0.026 648 332 422                                           | 0.015 985 538 075  | 0.010 666 188 293  |
| H -0.117 044 501 808                                          | 0.074 561 447 592  | -0.084 472 976 661 |

Wavenumber/cm<sup>-1</sup>: 1248.4278 , Max excitation: 1

| $l'$ -matrix coefficients/(u <sup>1/2</sup> Å <sup>-1</sup> ) |                    |                    |                    |
|---------------------------------------------------------------|--------------------|--------------------|--------------------|
| O                                                             | 0.003 021 696 566  | 0.002 720 207 969  | 0.000 251 393 792  |
| C                                                             | -0.017 883 955 098 | -0.017 190 258 126 | -0.004 563 080 708 |
| C                                                             | -0.039 597 598 420 | 0.214 735 129 039  | 0.235 549 230 582  |
| C                                                             | 0.228 174 629 439  | -0.196 223 911 370 | -0.185 968 176 943 |
| C                                                             | -0.229 840 494 952 | 0.084 666 356 274  | 0.132 905 490 597  |
| C                                                             | 0.195 830 646 502  | -0.085 820 026 428 | -0.064 515 751 707 |
| C                                                             | -0.014 168 649 775 | -0.065 304 650 034 | 0.216 366 045 325  |
| C                                                             | 0.005 063 310 397  | -0.030 488 463 188 | -0.138 285 749 205 |
| C                                                             | 0.012 125 970 526  | -0.074 569 602 923 | -0.095 760 372 806 |
| C                                                             | 0.019 295 560 481  | -0.110 892 500 224 | -0.076 211 940 420 |
| C                                                             | -0.097 942 254 031 | 0.132 668 730 075  | 0.090 002 267 421  |
| H                                                             | -0.229 728 948 389 | 0.196 235 519 247  | -0.104 878 949 263 |
| H                                                             | 0.027 312 065 446  | 0.245 951 508 102  | 0.161 705 721 677  |
| H                                                             | 0.070 564 102 095  | -0.150 048 898 612 | -0.307 978 191 021 |
| H                                                             | 0.081 669 403 514  | 0.016 413 167 917  | -0.089 682 438 910 |
| H                                                             | -0.021 106 207 744 | 0.024 124 096 870  | -0.083 287 943 712 |
| H                                                             | 0.214 238 341 705  | -0.102 999 668 604 | 0.148 683 266 489  |
| H                                                             | -0.079 995 243 406 | -0.000 444 942 067 | -0.084 340 149 671 |
| H                                                             | -0.053 383 704 919 | 0.047 113 253 179  | -0.067 467 868 570 |
| H                                                             | -0.032 002 614 151 | 0.033 437 626 889  | 0.047 367 871 815  |
| H                                                             | -0.010 628 381 245 | 0.011 870 893 420  | 0.049 571 229 905  |
| H                                                             | -0.081 183 508 480 | -0.002 960 779 667 | -0.040 847 855 473 |
| H                                                             | -0.143 887 238 238 | 0.098 998 103 405  | -0.008 906 214 660 |
| H                                                             | -0.023 610 693 188 | -0.021 239 414 548 | -0.010 284 552 932 |
| H                                                             | 0.061 131 852 148  | 0.038 537 678 804  | -0.013 791 127 564 |
| H                                                             | 0.037 066 872 365  | 0.055 085 481 544  | 0.075 429 706 882  |
| H                                                             | -0.039 262 998 258 | 0.011 429 208 413  | -0.050 348 085 472 |

Wavenumber/cm<sup>-1</sup>: 1259.6611 , Max excitation: 0

| $\ell'$ -matrix coefficients/(u <sup>1/2</sup> Å <sup>-1</sup> ) |                    |                    |                    |
|------------------------------------------------------------------|--------------------|--------------------|--------------------|
| O                                                                | 0.013 370 596 594  | 0.010 537 775 087  | 0.002 485 865 478  |
| C                                                                | -0.004 119 173 705 | -0.026 552 056 617 | 0.022 722 253 949  |
| C                                                                | -0.137 648 315 312 | 0.177 724 436 200  | -0.213 690 744 460 |
| C                                                                | -0.111 362 814 590 | -0.017 071 915 293 | 0.011 963 932 043  |
| C                                                                | 0.017 369 814 972  | -0.038 246 788 217 | 0.097 595 558 769  |
| C                                                                | 0.037 295 524 970  | -0.059 852 149 855 | -0.079 233 761 830 |
| C                                                                | 0.008 862 902 137  | -0.041 168 830 872 | 0.038 388 719 238  |
| C                                                                | -0.082 331 863 852 | 0.045 397 512 326  | 0.038 236 006 125  |
| C                                                                | 0.129 767 654 116  | -0.086 429 809 135 | 0.182 404 877 100  |
| C                                                                | 0.120 375 807 171  | -0.155 019 672 715 | 0.032 885 328 484  |
| C                                                                | 0.070 024 219 506  | 0.039 593 160 849  | -0.041 290 468 001 |
| H                                                                | 0.135 509 222 923  | -0.087 973 215 056 | -0.008 048 774 839 |
| H                                                                | -0.057 638 002 432 | 0.113 508 284 811  | 0.054 463 234 410  |
| H                                                                | 0.293 996 985 250  | 0.274 803 216 313  | 0.029 453 305 560  |
| H                                                                | -0.187 672 696 693 | 0.115 530 657 709  | 0.132 226 226 053  |
| H                                                                | -0.202 312 418 386 | 0.170 554 106 007  | -0.051 485 187 687 |
| H                                                                | 0.019 335 540 538  | 0.032 049 572 701  | 0.042 250 335 034  |
| H                                                                | -0.083 804 149 609 | 0.064 526 896 733  | -0.087 902 851 890 |
| H                                                                | 0.114 330 147 749  | -0.259 835 424 715 | -0.087 635 917 654 |
| H                                                                | -0.241 936 605 974 | 0.027 101 011 824  | -0.190 243 487 660 |
| H                                                                | -0.122 990 445 754 | 0.045 026 045 826  | -0.036 354 475 517 |
| H                                                                | -0.129 449 329 964 | 0.000 315 866 127  | -0.068 048 862 055 |
| H                                                                | -0.025 049 881 351 | -0.019 661 906 190 | 0.029 013 473 787  |
| H                                                                | -0.062 189 872 419 | -0.000 788 426 416 | 0.005 638 681 615  |
| H                                                                | 0.124 251 804 241  | -0.031 228 903 182 | -0.238 911 111 719 |
| H                                                                | 0.125 865 702 700  | 0.146 717 301 649  | 0.163 550 328 713  |
| H                                                                | 0.079 982 429 553  | -0.074 698 027 666 | -0.008 483 994 837 |

Wavenumber/cm<sup>-1</sup>: 1264.5459 , Max excitation: 1

| $l'$ -matrix coefficients/(u <sup>1/2</sup> Å <sup>-1</sup> ) |                    |                    |
|---------------------------------------------------------------|--------------------|--------------------|
| O                                                             | -0.002 657 857 253 | 0.009 884 519 222  |
| C                                                             | -0.004 518 020 389 | -0.066 038 763 639 |
| C                                                             | -0.017 837 751 957 | 0.100 025 621 757  |
| C                                                             | 0.204 137 260 949  | 0.123 314 687 869  |
| C                                                             | 0.021 991 643 190  | 0.120 927 818 562  |
| C                                                             | -0.017 688 008 638 | -0.140 158 091 655 |
| C                                                             | -0.051 559 629 496 | -0.066 865 423 217 |
| C                                                             | 0.029 775 835 688  | 0.068 861 683 116  |
| C                                                             | 0.005 940 924 509  | -0.028 896 297 899 |
| C                                                             | 0.014 722 530 018  | -0.130 597 081 921 |
| C                                                             | -0.192 117 024 448 | -0.205 694 439 723 |
| H                                                             | 0.269 235 673 544  | -0.127 802 288 273 |
| H                                                             | 0.099 487 079 468  | -0.091 003 784 750 |
| H                                                             | 0.047 708 796 013  | 0.144 355 536 939  |
| H                                                             | 0.070 508 108 550  | -0.006 765 710 859 |
| H                                                             | -0.269 700 712 165 | 0.232 421 556 400  |
| H                                                             | -0.181 976 631 798 | -0.058 836 842 728 |
| H                                                             | -0.072 850 239 916 | 0.011 314 985 575  |
| H                                                             | -0.108 178 933 776 | 0.168 392 578 598  |
| H                                                             | 0.081 410 575 009  | 0.054 826 671 453  |
| H                                                             | 0.007 115 934 091  | 0.009 450 413 619  |
| H                                                             | -0.095 136 654 522 | -0.005 068 144 342 |
| H                                                             | 0.215 393 294 320  | -0.016 690 158 173 |
| H                                                             | 0.176 519 774 618  | 0.048 603 250 761  |
| H                                                             | 0.017 358 244 436  | 0.022 964 969 745  |
| H                                                             | 0.050 498 666 445  | 0.073 100 103 079  |
| H                                                             | -0.272 114 454 526 | 0.278 467 271 438  |

Wavenumber/cm<sup>-1</sup>: 1295.6522 , Max excitation: 1

| $l'$ -matrix coefficients/(u <sup>1/2</sup> Å <sup>-1</sup> ) |                    |                    |
|---------------------------------------------------------------|--------------------|--------------------|
| O                                                             | -0.000 604 490 553 | -0.028 306 311 212 |
| C                                                             | -0.018 222 015 585 | -0.001 567 135 657 |
| C                                                             | 0.048 051 399 867  | 0.006 383 378 198  |
| C                                                             | 0.022 875 322 583  | -0.001 051 806 796 |
| C                                                             | -0.102 845 422 799 | -0.124 845 778 669 |
| C                                                             | 0.093 170 282 682  | 0.168 203 626 392  |
| C                                                             | -0.102 611 682 859 | 0.157 009 621 068  |
| C                                                             | 0.106 232 841 947  | -0.096 304 205 983 |
| C                                                             | 0.032 215 300 889  | -0.100 037 632 823 |
| C                                                             | 0.012 768 385 504  | 0.123 712 194 562  |
| C                                                             | -0.123 113 191 879 | -0.175 786 316 631 |
| H                                                             | -0.060 678 458 650 | -0.091 785 765 460 |
| H                                                             | -0.113 369 167 203 | 0.040 529 916 611  |
| H                                                             | 0.105 035 880 953  | -0.106 275 825 780 |
| H                                                             | -0.115 117 908 872 | 0.092 384 726 016  |
| H                                                             | -0.154 997 362 781 | 0.107 927 396 929  |
| H                                                             | 0.221 364 876 735  | 0.068 891 661 039  |
| H                                                             | 0.002 384 578 752  | -0.062 991 111 170 |
| H                                                             | -0.037 857 991 243 | 0.089 696 862 787  |
| H                                                             | 0.110 236 023 098  | -0.085 913 590 678 |
| H                                                             | -0.123 844 426 816 | 0.047 397 017 445  |
| H                                                             | 0.101 430 680 284  | 0.037 652 605 753  |
| H                                                             | 0.199 363 273 188  | -0.040 300 043 006 |
| H                                                             | 0.130 024 905 697  | 0.037 967 605 213  |
| H                                                             | 0.109 188 647 854  | -0.003 818 053 792 |
| H                                                             | -0.063 141 265 113 | -0.076 068 760 755 |
| H                                                             | -0.198 949 774 060 | 0.210 347 720 464  |
|                                                               |                    | 0.015 975 528 680  |
|                                                               |                    | 0.019 511 219 936  |
|                                                               |                    | -0.101 567 342 521 |
|                                                               |                    | -0.032 801 175 960 |
|                                                               |                    | -0.208 010 983 980 |
|                                                               |                    | 0.110 107 174 652  |
|                                                               |                    | -0.123 609 615 487 |
|                                                               |                    | 0.222 044 384 014  |
|                                                               |                    | 0.158 164 081 733  |
|                                                               |                    | -0.028 599 187 313 |
|                                                               |                    | 0.012 272 850 644  |
|                                                               |                    | 0.163 407 092 062  |
|                                                               |                    | -0.040 784 511 602 |
|                                                               |                    | -0.284 101 544 233 |
|                                                               |                    | 0.074 371 116 173  |
|                                                               |                    | -0.216 801 461 711 |
|                                                               |                    | 0.187 830 173 211  |
|                                                               |                    | 0.008 462 593 943  |
|                                                               |                    | 0.068 540 202 638  |
|                                                               |                    | -0.011 257 241 229 |
|                                                               |                    | 0.039 606 782 225  |
|                                                               |                    | 0.117 949 832 489  |
|                                                               |                    | -0.063 540 309 508 |
|                                                               |                    | 0.000 229 416 801  |
|                                                               |                    | -0.179 609 966 984 |
|                                                               |                    | -0.061 742 590 030 |
|                                                               |                    | 0.038 823 761 581  |

Wavenumber/cm<sup>-1</sup>: 1331.6331 , Max excitation: 1

| $l'$ -matrix coefficients/(u <sup>1/2</sup> Å <sup>-1</sup> ) |                    |                    |
|---------------------------------------------------------------|--------------------|--------------------|
| O                                                             | -0.000 514 616 686 | 0.015 325 062 262  |
| C                                                             | 0.045 236 114 320  | 0.008 337 311 669  |
| C                                                             | -0.048 314 124 610 | -0.012 756 649 176 |
| C                                                             | -0.084 330 143 177 | 0.005 515 175 598  |
| C                                                             | -0.049 665 983 683 | -0.149 075 577 759 |
| C                                                             | 0.187 643 266 471  | 0.212 220 487 981  |
| C                                                             | -0.186 635 421 970 | -0.069 813 005 879 |
| C                                                             | 0.173 342 423 900  | 0.070 067 883 010  |
| C                                                             | -0.025 840 668 196 | 0.105 339 259 624  |
| C                                                             | -0.014 354 504 886 | -0.010 110 054 418 |
| C                                                             | 0.005 745 995 504  | -0.044 309 366 661 |
| H                                                             | 0.064 919 155 339  | -0.260 581 860 448 |
| H                                                             | -0.006 296 681 608 | 0.265 123 289 518  |
| H                                                             | -0.155 243 449 754 | -0.092 422 513 856 |
| H                                                             | 0.057 981 889 469  | -0.076 692 494 840 |
| H                                                             | -0.048 577 610 620 | 0.021 620 030 663  |
| H                                                             | 0.038 955 252 562  | -0.195 298 933 539 |
| H                                                             | 0.028 145 982 627  | 0.025 942 758 383  |
| H                                                             | -0.008 728 964 293 | -0.175 778 535 520 |
| H                                                             | -0.076 711 410 375 | 0.114 846 801 544  |
| H                                                             | 0.114 079 287 431  | -0.052 799 323 909 |
| H                                                             | -0.013 579 599 653 | -0.010 247 625 649 |
| H                                                             | 0.196 125 418 159  | -0.163 365 999 444 |
| H                                                             | -0.167 559 953 623 | 0.159 886 597 239  |
| H                                                             | -0.103 065 189 289 | -0.008 025 810 656 |
| H                                                             | 0.010 016 857 809  | 0.008 341 176 295  |
| H                                                             | 0.061 830 697 323  | -0.020 015 905 397 |

Wavenumber/cm<sup>-1</sup>: 1334.8421 , Max excitation: 1

| $l'$ -matrix coefficients/(u <sup>1/2</sup> Å <sup>-1</sup> ) |                    |                    |                    |
|---------------------------------------------------------------|--------------------|--------------------|--------------------|
| O                                                             | 0.001 154 736 748  | -0.024 431 824 467 | 0.003 884 185 508  |
| C                                                             | -0.008 049 090 857 | -0.007 510 285 370 | -0.034 896 998 895 |
| C                                                             | -0.005 447 339 609 | 0.020 072 062 139  | 0.018 028 621 092  |
| C                                                             | 0.000 377 723 775  | -0.012 376 205 344 | 0.017 769 334 584  |
| C                                                             | 0.004 450 763 678  | -0.028 765 187 521 | -0.071 862 071 593 |
| C                                                             | 0.012 890 130 494  | 0.086 225 444 754  | 0.059 772 329 065  |
| C                                                             | 0.020 177 069 553  | 0.086 950 019 342  | -0.145 303 456 380 |
| C                                                             | -0.028 227 813 783 | -0.055 728 771 780 | 0.143 634 331 419  |
| C                                                             | 0.024 461 829 711  | 0.254 479 196 111  | -0.082 278 055 150 |
| C                                                             | -0.003 749 441 478 | -0.274 188 166 917 | 0.126 685 437 132  |
| C                                                             | -0.029 248 223 126 | -0.054 639 105 326 | 0.058 209 409 102  |
| H                                                             | -0.130 300 609 328 | 0.028 376 767 765  | 0.055 598 604 125  |
| H                                                             | -0.092 898 449 795 | -0.071 164 274 204 | -0.081 395 856 224 |
| H                                                             | 0.078 532 493 209  | 0.005 929 414 041  | -0.087 711 869 859 |
| H                                                             | -0.041 225 984 526 | -0.144 288 727 207 | 0.089 040 955 056  |
| H                                                             | 0.017 628 650 978  | -0.030 935 883 326 | -0.074 887 369 498 |
| H                                                             | 0.105 797 866 401  | 0.103 793 659 705  | 0.103 722 836 393  |
| H                                                             | 0.046 022 133 294  | 0.202 475 085 143  | 0.015 687 687 475  |
| H                                                             | 0.015 526 052 467  | 0.048 911 300 117  | 0.111 713 548 665  |
| H                                                             | 0.018 470 051 379  | -0.076 960 067 280 | -0.101 115 417 624 |
| H                                                             | 0.241 312 902 421  | -0.135 484 822 097 | -0.273 936 962 665 |
| H                                                             | -0.239 033 047 577 | -0.106 766 826 804 | -0.346 547 236 024 |
| H                                                             | 0.018 099 615 241  | 0.027 805 070 972  | -0.034 910 418 499 |
| H                                                             | 0.095 490 999 600  | -0.035 252 269 889 | -0.025 818 433 252 |
| H                                                             | -0.205 914 254 382 | -0.061 217 648 355 | 0.209 672 607 216  |
| H                                                             | 0.191 029 773 776  | 0.217 124 868 625  | 0.125 648 154 780  |
| H                                                             | -0.080 457 102 276 | 0.074 873 371 325  | -0.010 081 753 391 |

Wavenumber/cm<sup>-1</sup>: 1372.9393 , Max excitation: 4

| $l'$ -matrix coefficients/(u <sup>1/2</sup> Å <sup>-1</sup> ) |                    |                    |
|---------------------------------------------------------------|--------------------|--------------------|
| O                                                             | -0.004 663 307 701 | 0.016 002 687 423  |
| C                                                             | 0.001 539 656 263  | 0.000 118 939 644  |
| C                                                             | 0.141 931 459 991  | 0.023 760 066 819  |
| C                                                             | -0.028 343 841 093 | 0.034 180 550 335  |
| C                                                             | -0.079 657 333 970 | -0.060 883 234 840 |
| C                                                             | -0.217 716 474 233 | -0.213 863 023 522 |
| C                                                             | -0.343 719 460 089 | 0.215 532 171 520  |
| C                                                             | 0.371 472 368 229  | -0.113 259 995 115 |
| C                                                             | -0.051 879 409 862 | 0.068 901 839 054  |
| C                                                             | 0.070 000 545 260  | -0.067 322 830 686 |
| C                                                             | 0.101 823 891 983  | 0.050 760 200 524  |
| H                                                             | 0.209 019 320 820  | 0.043 575 221 289  |
| H                                                             | 0.025 479 703 456  | 0.139 373 425 151  |
| H                                                             | 0.011 419 689 445  | 0.027 125 723 773  |
| H                                                             | -0.025 380 798 819 | -0.021 135 852 245 |
| H                                                             | -0.076 212 594 538 | 0.077 107 675 316  |
| H                                                             | 0.099 297 047 268  | -0.041 205 410 892 |
| H                                                             | -0.114 765 500 696 | -0.033 962 129 556 |
| H                                                             | -0.134 213 258 704 | 0.094 183 919 273  |
| H                                                             | 0.203 942 284 879  | -0.037 971 161 757 |
| H                                                             | 0.034 288 872 865  | -0.022 349 277 086 |
| H                                                             | -0.053 607 057 851 | 0.023 446 259 802  |
| H                                                             | -0.056 344 327 140 | -0.030 411 032 681 |
| H                                                             | -0.121 215 427 186 | 0.011 272 553 119  |
| H                                                             | -0.056 398 789 850 | -0.004 957 828 914 |
| H                                                             | 0.045 020 477 865  | 0.073 551 863 320  |
| H                                                             | 0.147 510 477 322  | -0.147 117 074 601 |



Wavenumber/cm<sup>-1</sup>: 1388.8345 , Max excitation: 0

| $l'$ -matrix coefficients/(u <sup>1/2</sup> Å <sup>-1</sup> ) |                    |                    |                    |
|---------------------------------------------------------------|--------------------|--------------------|--------------------|
| O                                                             | 0.005 721 273 423  | 0.074 883 660 968  | -0.024 031 230 737 |
| C                                                             | 0.033 382 892 308  | -0.011 982 501 279 | 0.017 459 702 289  |
| C                                                             | -0.242 655 381 919 | -0.067 616 061 903 | 0.035 754 702 303  |
| C                                                             | 0.020 505 147 351  | 0.018 037 394 641  | 0.040 240 874 084  |
| C                                                             | 0.450 624 291 902  | -0.273 648 854 792 | -0.021 526 536 297 |
| C                                                             | -0.235 296 855 084 | 0.126 261 219 931  | 0.035 637 560 554  |
| C                                                             | -0.167 501 733 831 | -0.076 756 727 859 | -0.019 347 054 618 |
| C                                                             | 0.098 656 862 534  | 0.127 548 493 247  | 0.014 378 629 387  |
| C                                                             | 0.027 849 215 088  | -0.056 901 618 586 | -0.128 577 104 907 |
| C                                                             | -0.047 108 631 234 | 0.055 549 423 352  | 0.140 406 570 943  |
| C                                                             | 0.043 680 464 475  | 0.029 529 485 479  | 0.069 241 510 238  |
| H                                                             | -0.163 469 343 031 | 0.142 395 702 538  | -0.038 887 693 781 |
| H                                                             | 0.064 365 452 213  | 0.023 747 174 814  | 0.013 790 628 379  |
| H                                                             | 0.271 056 082 838  | -0.122 731 664 865 | -0.205 778 405 584 |
| H                                                             | 0.091 620 314 504  | -0.013 372 130 393 | -0.090 657 328 455 |
| H                                                             | -0.252 023 452 412 | 0.197 767 534 941  | -0.017 716 725 546 |
| H                                                             | -0.102 931 998 888 | -0.047 616 654 554 | -0.081 134 226 017 |
| H                                                             | 0.145 147 709 629  | 0.077 987 439 980  | 0.136 793 021 687  |
| H                                                             | -0.045 401 808 835 | -0.064 828 676 417 | -0.137 525 383 386 |
| H                                                             | 0.041 014 226 035  | 0.066 444 696 234  | 0.102 615 826 911  |
| H                                                             | 0.003 943 499 661  | 0.005 446 203 444  | 0.030 508 608 604  |
| H                                                             | 0.023 235 517 430  | -0.035 550 498 264 | -0.068 311 181 164 |
| H                                                             | -0.115 429 666 650 | 0.065 321 195 815  | -0.007 796 137 280 |
| H                                                             | 0.049 016 368 705  | -0.076 700 958 815 | -0.035 528 897 336 |
| H                                                             | 0.016 576 603 791  | 0.006 570 902 097  | 0.002 849 098 117  |
| H                                                             | -0.007 804 802 536 | -0.031 764 830 234 | -0.093 699 750 802 |
| H                                                             | 0.019 956 551 427  | -0.042 770 210 246 | -0.047 800 643 337 |

Wavenumber/cm<sup>-1</sup>: 1413.0925 , Max excitation: 1

| $l'$ -matrix coefficients/(u <sup>1/2</sup> Å <sup>-1</sup> ) |                    |                    |                    |
|---------------------------------------------------------------|--------------------|--------------------|--------------------|
| O                                                             | 0.000 458 872 176  | 0.012 826 796 764  | -0.002 854 354 362 |
| C                                                             | -0.013 242 389 351 | -0.005 420 253 805 | -0.018 113 440 880 |
| C                                                             | 0.183 418 008 791  | -0.011 047 081 999 | -0.239 782 601 767 |
| C                                                             | 0.025 081 731 976  | -0.012 531 047 302 | 0.066 450 224 198  |
| C                                                             | 0.017 046 889 937  | -0.235 701 891 826 | -0.002 871 915 413 |
| C                                                             | -0.049 961 569 241 | 0.055 382 122 365  | -0.046 699 462 913 |
| C                                                             | 0.124 001 292 044  | -0.152 147 474 108 | -0.016 140 536 443 |
| C                                                             | -0.107 671 840 042 | 0.244 563 294 116  | 0.067 395 308 270  |
| C                                                             | -0.274 319 368 269 | 0.114 514 153 681  | 0.110 412 102 222  |
| C                                                             | 0.240 641 740 784  | 0.023 832 747 460  | -0.097 185 466 905 |
| C                                                             | -0.027 155 510 886 | 0.000 735 724 463  | 0.064 516 742 313  |
| H                                                             | -0.044 090 537 731 | 0.021 023 299 433  | -0.009 626 077 626 |
| H                                                             | 0.022 320 552 915  | -0.083 714 562 006 | -0.017 870 197 266 |
| H                                                             | -0.031 549 846 307 | -0.187 641 533 072 | -0.094 788 007 273 |
| H                                                             | 0.117 648 768 523  | -0.052 637 901 858 | -0.053 105 283 357 |
| H                                                             | -0.102 731 944 574 | 0.088 117 029 035  | -0.035 992 916 275 |
| H                                                             | -0.021 519 350 421 | 0.030 179 012 728  | 0.036 441 128 521  |
| H                                                             | -0.273 439 505 821 | -0.153 102 829 453 | -0.228 729 467 296 |
| H                                                             | 0.080 665 542 041  | -0.128 863 000 926 | 0.001 068 458 265  |
| H                                                             | -0.073 650 702 360 | 0.080 202 466 628  | -0.001 373 404 323 |
| H                                                             | 0.043 844 542 082  | -0.017 521 291 503 | 0.110 256 802 969  |
| H                                                             | 0.012 555 890 635  | 0.114 218 577 349  | 0.222 740 057 357  |
| H                                                             | -0.039 039 572 729 | 0.046 714 401 666  | -0.020 121 936 151 |
| H                                                             | 0.069 448 681 774  | -0.042 535 768 308 | -0.026 173 278 328 |
| H                                                             | -0.151 205 519 860 | 0.043 553 279 398  | 0.279 748 605 389  |
| H                                                             | 0.031 827 374 327  | 0.075 333 744 873  | 0.256 183 685 496  |
| H                                                             | -0.049 690 585 152 | 0.039 006 125 221  | -0.020 598 486 182 |

Wavenumber/cm<sup>-1</sup>: 1415.0986 , Max excitation: 1

| $l'$ -matrix coefficients/(u <sup>1/2</sup> Å <sup>-1</sup> ) |                    |                    |
|---------------------------------------------------------------|--------------------|--------------------|
| O                                                             | -0.001 648 639 421 | -0.000 596 835 661 |
| C                                                             | 0.039 241 936 857  | -0.003 491 018 342 |
| C                                                             | 0.165 301 413 971  | 0.226 299 218 748  |
| C                                                             | 0.010 117 993 728  | 0.008 527 871 601  |
| C                                                             | -0.155 370 598 708 | -0.226 930 741 064 |
| C                                                             | -0.034 051 718 519 | -0.076 200 116 426 |
| C                                                             | 0.096 939 194 704  | -0.161 472 499 767 |
| C                                                             | -0.051 286 003 153 | 0.291 246 833 769  |
| C                                                             | 0.192 984 111 402  | 0.111 674 055 146  |
| C                                                             | -0.226 529 598 453 | -0.023 798 071 423 |
| C                                                             | -0.001 551 202 500 | 0.014 617 034 597  |
| H                                                             | 0.165 683 009 016  | -0.032 201 979 721 |
| H                                                             | 0.114 047 670 614  | -0.079 249 844 825 |
| H                                                             | -0.146 794 274 519 | -0.197 484 806 614 |
| H                                                             | -0.237 750 321 926 | -0.020 129 627 048 |
| H                                                             | -0.105 220 989 856 | 0.108 076 682 940  |
| H                                                             | -0.033 467 648 416 | 0.052 755 812 799  |
| H                                                             | 0.070 182 609 871  | -0.025 904 324 852 |
| H                                                             | 0.047 287 745 259  | -0.105 882 897 339 |
| H                                                             | 0.010 384 252 286  | 0.081 491 069 104  |
| H                                                             | 0.107 187 336 373  | -0.080 309 903 769 |
| H                                                             | 0.042 564 957 466  | -0.042 884 637 301 |
| H                                                             | -0.045 037 001 156 | 0.032 885 836 798  |
| H                                                             | 0.033 103 703 135  | -0.034 461 725 411 |
| H                                                             | -0.023 799 512 209 | -0.086 835 242 075 |
| H                                                             | -0.104 135 336 669 | -0.123 761 921 671 |
| H                                                             | -0.011 233 402 286 | 0.002 326 976 509  |

Wavenumber/cm<sup>-1</sup>: 1474.2549 , Max excitation: 1

| $l'$ -matrix coefficients/(u <sup>1/2</sup> Å <sup>-1</sup> ) |                    |                    |
|---------------------------------------------------------------|--------------------|--------------------|
| O                                                             | -0.006 912 474 907 | -0.009 994 441 396 |
| C                                                             | -0.107 083 292 152 | 0.008 119 655 004  |
| C                                                             | 0.266 121 859 761  | 0.021 876 051 209  |
| C                                                             | 0.017 359 566 400  | -0.024 253 438 363 |
| C                                                             | 0.237 410 992 575  | 0.021 439 453 185  |
| C                                                             | -0.192 810 730 206 | 0.063 735 595 415  |
| C                                                             | 0.167 748 144 907  | -0.000 480 080 780 |
| C                                                             | -0.145 763 180 964 | -0.087 155 812 971 |
| C                                                             | 0.007 031 804 766  | 0.056 926 240 672  |
| C                                                             | -0.049 700 601 085 | -0.084 212 811 502 |
| C                                                             | -0.073 850 466 553 | 0.036 614 033 117  |
| H                                                             | -0.201 020 297 688 | 0.082 575 693 147  |
| H                                                             | 0.118 822 748 722  | -0.014 124 249 891 |
| H                                                             | 0.154 588 801 376  | -0.035 811 465 736 |
| H                                                             | -0.147 917 826 545 | 0.010 800 298 618  |
| H                                                             | -0.031 623 174 783 | -0.025 496 603 651 |
| H                                                             | -0.159 379 707 511 | 0.022 525 891 993  |
| H                                                             | -0.080 357 043 473 | -0.057 884 569 248 |
| H                                                             | -0.004 087 619 456 | 0.089 301 148 434  |
| H                                                             | -0.005 045 765 441 | -0.044 260 573 023 |
| H                                                             | 0.005 968 930 203  | -0.018 845 043 029 |
| H                                                             | -0.022 691 506 962 | -0.010 782 358 181 |
| H                                                             | 0.153 468 105 450  | -0.129 080 546 278 |
| H                                                             | -0.210 254 337 019 | 0.178 490 371 767  |
| H                                                             | -0.015 373 458 296 | -0.032 079 747 691 |
| H                                                             | -0.013 132 059 254 | -0.002 877 993 557 |
| H                                                             | 0.049 022 305 859  | -0.016 157 241 072 |
|                                                               |                    | 0.091 396 567 151  |

Wavenumber/cm<sup>-1</sup>: 1481.9108 , Max excitation: 1

| $l'$ -matrix coefficients/(u <sup>1/2</sup> Å <sup>-1</sup> ) |                    |                    |                    |
|---------------------------------------------------------------|--------------------|--------------------|--------------------|
| O                                                             | 0.001 292 251 998  | 0.014 053 562 119  | -0.006 568 017 332 |
| C                                                             | -0.012 822 535 098 | 0.010 840 961 739  | 0.002 920 215 492  |
| C                                                             | 0.226 969 556 695  | 0.133 089 106 954  | 0.052 498 928 479  |
| C                                                             | 0.058 136 030 919  | -0.010 357 158 297 | 0.176 432 000 733  |
| C                                                             | 0.216 937 021 127  | -0.060 699 577 204 | 0.326 795 063 008  |
| C                                                             | -0.020 749 653 939 | 0.114 346 572 621  | -0.028 324 782 240 |
| C                                                             | -0.238 541 710 012 | 0.072 387 685 277  | -0.264 664 573 099 |
| C                                                             | 0.097 838 434 875  | -0.256 846 342 004 | -0.221 183 698 851 |
| C                                                             | 0.008 224 157 116  | 0.082 734 792 580  | 0.110 710 593 921  |
| C                                                             | -0.104 267 113 670 | -0.044 319 728 662 | -0.234 454 961 574 |
| C                                                             | -0.006 743 213 088 | 0.020 643 777 008  | 0.108 257 305 539  |
| H                                                             | -0.127 606 728 194 | 0.062 305 281 288  | 0.009 772 011 211  |
| H                                                             | -0.236 463 562 595 | 0.107 044 860 466  | -0.052 713 701 799 |
| H                                                             | 0.007 123 243 124  | 0.037 701 567 950  | 0.221 019 410 090  |
| H                                                             | -0.120 763 082 385 | -0.006 897 838 026 | 0.120 617 148 506  |
| H                                                             | -0.016 681 041 141 | 0.024 921 516 448  | -0.044 914 770 782 |
| H                                                             | 0.051 547 229 661  | -0.203 124 363 185 | -0.018 795 544 828 |
| H                                                             | -0.091 170 009 635 | -0.116 218 756 105 | -0.090 809 181 877 |
| H                                                             | -0.030 699 752 718 | -0.026 146 957 204 | 0.039 352 071 567  |
| H                                                             | -0.109 065 801 659 | -0.014 150 379 045 | -0.038 250 468 961 |
| H                                                             | 0.041 429 652 643  | -0.032 376 562 770 | -0.086 871 913 965 |
| H                                                             | 0.039 429 025 733  | 0.006 206 154 740  | 0.078 793 280 133  |
| H                                                             | -0.133 851 184 133 | 0.098 199 776 253  | -0.032 544 504 811 |
| H                                                             | 0.113 368 826 634  | -0.103 758 145 544 | -0.062 508 493 403 |
| H                                                             | -0.041 216 037 482 | -0.027 714 294 843 | 0.005 947 865 054  |
| H                                                             | -0.086 738 929 789 | -0.088 066 505 708 | -0.064 572 912 000 |
| H                                                             | -0.040 420 504 781 | 0.012 682 307 202  | -0.057 412 246 765 |

Wavenumber/cm<sup>-1</sup>: 1485.2699 , Max excitation: 0

| $l'$ -matrix coefficients/(u <sup>1/2</sup> Å <sup>-1</sup> ) |                    |                    |
|---------------------------------------------------------------|--------------------|--------------------|
| O                                                             | -0.026 636 172 867 | -0.011 690 641 858 |
| C                                                             | -0.138 690 907 794 | 0.001 593 740 360  |
| C                                                             | 0.117 988 079 845  | -0.167 558 330 595 |
| C                                                             | 0.201 093 016 301  | 0.237 555 917 468  |
| C                                                             | -0.172 780 083 247 | 0.276 923 982 213  |
| C                                                             | -0.072 139 154 704 | 0.062 755 664 184  |
| C                                                             | -0.016 752 066 935 | -0.326 616 441 477 |
| C                                                             | 0.046 392 843 678  | 0.096 347 724 526  |
| C                                                             | 0.026 205 711 513  | -0.048 596 511 485 |
| C                                                             | -0.002 747 469 404 | -0.074 178 557 273 |
| C                                                             | 0.084 037 012 409  | 0.063 103 763 350  |
| H                                                             | 0.017 346 868 103  | -0.101 425 980 568 |
| H                                                             | -0.067 566 912 331 | -0.072 308 871 427 |
| H                                                             | -0.040 249 626 640 | 0.003 587 411 082  |
| H                                                             | -0.037 165 247 554 | 0.041 940 490 678  |
| H                                                             | -0.035 970 492 054 | -0.009 788 873 832 |
| H                                                             | 0.052 893 826 081  | -0.182 163 687 789 |
| H                                                             | -0.008 623 353 919 | 0.031 170 774 640  |
| H                                                             | 0.043 443 845 098  | -0.170 448 591 764 |
| H                                                             | 0.015 880 204 394  | 0.106 783 810 485  |
| H                                                             | -0.067 138 954 163 | 0.040 087 101 226  |
| H                                                             | -0.071 898 618 907 | -0.023 087 414 345 |
| H                                                             | -0.158 986 010 336 | 0.061 714 022 873  |
| H                                                             | -0.006 464 317 206 | -0.058 958 627 388 |
| H                                                             | 0.071 140 360 393  | 0.009 142 369 424  |
| H                                                             | 0.051 288 961 029  | 0.067 264 237 681  |
| H                                                             | 0.097 552 134 014  | -0.115 763 949 682 |

Wavenumber/cm<sup>-1</sup>: 1488.1387 , Max excitation: 1

| $l'$ -matrix coefficients/(u <sup>1/2</sup> Å <sup>-1</sup> ) |                    |                    |                    |
|---------------------------------------------------------------|--------------------|--------------------|--------------------|
| O                                                             | 0.011 337 197 049  | 0.032 225 374 120  | -0.019 754 453 953 |
| C                                                             | 0.171 267 883 216  | -0.033 609 978 400 | 0.000 738 975 024  |
| C                                                             | -0.162 837 559 885 | 0.127 221 549 315  | -0.044 251 587 350 |
| C                                                             | -0.041 597 566 673 | -0.055 701 595 836 | -0.163 847 001 553 |
| C                                                             | -0.071 572 478 009 | -0.132 210 853 583 | 0.075 999 189 850  |
| C                                                             | -0.067 546 165 035 | -0.216 886 432 598 | 0.301 607 592 699  |
| C                                                             | 0.155 467 665 144  | 0.133 742 692 351  | -0.156 133 005 701 |
| C                                                             | 0.075 682 050 915  | 0.102 567 378 204  | -0.066 178 618 145 |
| C                                                             | 0.059 209 091 968  | 0.004 450 433 589  | -0.120 020 270 967 |
| C                                                             | 0.002 947 123 078  | 0.065 904 686 016  | 0.043 853 309 027  |
| C                                                             | -0.091 129 506 267 | 0.039 196 373 775  | -0.046 593 764 984 |
| H                                                             | 0.084 320 997 967  | 0.050 230 817 553  | -0.030 022 360 370 |
| H                                                             | -0.351 362 623 736 | -0.085 063 897 609 | -0.104 180 174 213 |
| H                                                             | 0.039 307 190 784  | -0.067 545 236 449 | -0.076 296 472 781 |
| H                                                             | 0.054 882 726 330  | -0.018 456 895 550 | -0.051 328 388 863 |
| H                                                             | -0.020 850 077 353 | 0.015 954 467 119  | 0.258 657 871 211  |
| H                                                             | 0.077 463 481 053  | -0.258 075 934 003 | 0.090 208 747 140  |
| H                                                             | 0.035 487 566 945  | -0.003 386 712 784 | 0.041 115 581 410  |
| H                                                             | 0.157 983 740 592  | -0.081 245 948 785 | 0.332 512 860 369  |
| H                                                             | -0.233 726 680 736 | 0.166 673 350 059  | 0.093 412 753 426  |
| H                                                             | 0.047 196 144 584  | -0.013 788 218 229 | -0.028 912 205 546 |
| H                                                             | 0.045 838 640 129  | 0.016 657 866 037  | 0.057 129 899 989  |
| H                                                             | 0.067 502 060 580  | -0.039 689 079 568 | 0.017 107 529 331  |
| H                                                             | -0.099 923 858 455 | 0.081 062 122 325  | 0.045 373 663 591  |
| H                                                             | -0.008 148 170 519 | 0.000 463 057 357  | 0.027 420 765 321  |
| H                                                             | -0.029 530 798 406 | -0.041 871 970 482 | -0.041 458 512 210 |
| H                                                             | -0.014 790 232 695 | 0.029 998 857 851  | 0.051 455 105 632  |

Wavenumber/cm<sup>-1</sup>: 1492.9931 , Max excitation: 1

| $l'$ -matrix coefficients/(u <sup>1/2</sup> Å <sup>-1</sup> ) |                    |                    |
|---------------------------------------------------------------|--------------------|--------------------|
| O                                                             | -0.017 798 718 916 | 0.038 392 704 867  |
| C                                                             | 0.301 634 661 513  | -0.065 999 834 469 |
| C                                                             | -0.104 778 681 562 | 0.155 776 753 054  |
| C                                                             | 0.122 670 912 143  | 0.154 374 650 176  |
| C                                                             | 0.023 993 198 308  | -0.045 035 200 083 |
| C                                                             | 0.232 416 650 896  | -0.180 611 946 843 |
| C                                                             | -0.244 672 349 059 | -0.207 090 274 836 |
| C                                                             | -0.149 412 886 385 | 0.014 757 262 364  |
| C                                                             | -0.047 299 446 654 | 0.022 447 812 613  |
| C                                                             | -0.034 413 567 217 | 0.026 885 293 325  |
| C                                                             | -0.106 110 541 319 | 0.150 128 468 977  |
| H                                                             | 0.029 143 180 308  | -0.090 730 629 905 |
| H                                                             | 0.116 051 125 515  | -0.132 738 727 397 |
| H                                                             | 0.086 657 650 050  | -0.015 831 894 101 |
| H                                                             | 0.019 764 527 764  | -0.014 019 811 357 |
| H                                                             | 0.058 107 826 242  | -0.072 486 458 358 |
| H                                                             | 0.037 671 259 247  | 0.264 566 081 329  |
| H                                                             | -0.012 121 117 810 | -0.034 280 387 867 |
| H                                                             | -0.130 554 875 765 | 0.034 169 287 488  |
| H                                                             | 0.126 586 673 991  | -0.129 055 288 321 |
| H                                                             | 0.013 695 771 330  | -0.011 605 561 939 |
| H                                                             | 0.036 334 053 325  | 0.013 615 457 102  |
| H                                                             | -0.117 583 227 837 | 0.025 245 821 946  |
| H                                                             | -0.145 395 355 972 | 0.048 264 657 119  |
| H                                                             | -0.035 629 374 163 | 0.006 701 588 218  |
| H                                                             | -0.046 894 461 747 | -0.053 554 094 964 |
| H                                                             | 0.055 693 270 043  | -0.079 704 238 798 |



Wavenumber/cm<sup>-1</sup>: 1497.2585 , Max excitation: 1

| $l'$ -matrix coefficients/(u <sup>1/2</sup> Å <sup>-1</sup> ) |                    |                    |
|---------------------------------------------------------------|--------------------|--------------------|
| O                                                             | -0.005 193 115 416 | -0.019 706 688 880 |
| C                                                             | 0.757 246 725 063  | -0.015 394 656 611 |
| C                                                             | -0.092 788 554 630 | 0.091 720 065 960  |
| C                                                             | -0.173 092 246 462 | -0.196 686 596 312 |
| C                                                             | -0.074 437 209 946 | 0.219 716 936 994  |
| C                                                             | -0.175 087 063 072 | 0.104 976 061 591  |
| C                                                             | 0.035 898 260 254  | -0.107 156 194 441 |
| C                                                             | 0.015 797 141 306  | -0.092 084 868 211 |
| C                                                             | -0.107 641 188 717 | 0.045 474 132 414  |
| C                                                             | -0.062 109 523 920 | -0.028 910 339 898 |
| C                                                             | -0.052 475 497 212 | -0.035 332 897 684 |
| H                                                             | -0.057 966 762 285 | 0.024 829 034 327  |
| H                                                             | 0.034 565 301 184  | 0.045 125 091 080  |
| H                                                             | -0.008 388 400 428 | 0.082 716 702 731  |
| H                                                             | -0.037 148 893 964 | 0.022 336 218 180  |
| H                                                             | -0.013 133 387 980 | -0.006 912 325 346 |
| H                                                             | -0.032 962 702 952 | -0.058 249 080 979 |
| H                                                             | -0.026 656 559 063 | 0.000 555 035 235  |
| H                                                             | 0.001 391 347 260  | -0.039 491 752 788 |
| H                                                             | 0.045 461 958 476  | -0.011 444 899 513 |
| H                                                             | -0.030 456 110 462 | 0.013 080 367 793  |
| H                                                             | -0.036 114 676 422 | -0.005 599 371 327 |
| H                                                             | 0.008 854 621 107  | 0.007 497 521 615  |
| H                                                             | 0.057 570 765 743  | -0.023 315 272 461 |
| H                                                             | -0.040 812 291 838 | 0.010 259 169 205  |
| H                                                             | -0.015 199 075 927 | -0.001 497 663 882 |
| H                                                             | -0.074 479 073 498 | 0.065 841 686 243  |
|                                                               |                    | 0.004 878 372 637  |

Wavenumber/cm<sup>-1</sup>: 1501.7157 , Max excitation: 1

| $l'$ -matrix coefficients/(u <sup>1/2</sup> Å <sup>-1</sup> ) |                    |                    |                    |
|---------------------------------------------------------------|--------------------|--------------------|--------------------|
| O                                                             | 0.024 181 822 994  | -0.122 614 312 415 | 0.042 591 295 354  |
| C                                                             | -0.120 222 983 561 | -0.132 443 565 972 | 0.012 453 385 073  |
| C                                                             | -0.105 951 062 546 | 0.362 285 011 874  | -0.162 230 222 481 |
| C                                                             | 0.163 569 762 319  | 0.159 595 293 579  | 0.165 552 732 062  |
| C                                                             | -0.255 802 701 710 | -0.075 224 021 904 | -0.088 569 367 499 |
| C                                                             | -0.193 044 335 891 | 0.120 181 995 652  | 0.104 097 461 792  |
| C                                                             | 0.155 317 789 487  | -0.070 021 934 426 | 0.080 248 908 295  |
| C                                                             | -0.036 066 527 756 | -0.356 580 157 534 | -0.196 408 835 152 |
| C                                                             | 0.090 882 503 896  | 0.012 945 267 647  | -0.173 687 289 937 |
| C                                                             | 0.129 985 096 832  | 0.168 440 878 003  | 0.180 558 324 611  |
| C                                                             | 0.066 512 901 899  | -0.002 032 642 205 | 0.028 452 785 962  |
| H                                                             | 0.042 059 999 296  | -0.011 283 285 642 | 0.037 593 928 895  |
| H                                                             | 0.092 318 309 113  | 0.029 326 236 137  | 0.043 244 830 587  |
| H                                                             | -0.024 470 222 007 | 0.050 530 807 752  | -0.002 696 955 631 |
| H                                                             | 0.046 916 639 897  | -0.081 416 530 688 | -0.031 671 853 227 |
| H                                                             | -0.153 219 419 132 | 0.122 978 089 677  | 0.023 709 508 329  |
| H                                                             | 0.021 258 723 133  | 0.010 757 271 371  | -0.060 754 553 409 |
| H                                                             | 0.043 814 560 804  | -0.020 885 015 233 | 0.070 992 687 690  |
| H                                                             | 0.003 808 106 339  | 0.049 469 223 519  | -0.024 978 247 348 |
| H                                                             | 0.022 592 209 292  | -0.150 197 960 485 | -0.149 518 632 313 |
| H                                                             | 0.119 448 041 819  | -0.075 240 486 684 | -0.141 700 160 047 |
| H                                                             | 0.115 957 101 334  | 0.058 396 364 731  | 0.171 701 396 108  |
| H                                                             | -0.055 656 142 629 | 0.017 564 112 551  | 0.008 887 900 316  |
| H                                                             | 0.009 066 250 949  | -0.029 844 368 238 | -0.004 240 747 746 |
| H                                                             | -0.050 791 013 966 | -0.025 050 036 943 | 0.083 298 847 647  |
| H                                                             | -0.018 317 259 072 | -0.047 311 228 736 | -0.011 085 516 486 |
| H                                                             | 0.050 706 997 506  | -0.055 312 978 183 | -0.011 485 593 908 |

Wavenumber/cm<sup>-1</sup>: 1507.2351 , Max excitation: 1

| $l'$ -matrix coefficients/(u <sup>1/2</sup> Å <sup>-1</sup> ) |                    |                    |                    |
|---------------------------------------------------------------|--------------------|--------------------|--------------------|
| O                                                             | 0.059 934 925 032  | 0.310 998 841 765  | -0.134 786 427 741 |
| C                                                             | -0.035 769 267 864 | 0.265 518 082 103  | -0.084 618 712 772 |
| C                                                             | 0.177 218 117 206  | -0.050 664 853 217 | 0.012 663 406 225  |
| C                                                             | -0.173 937 528 471 | -0.375 730 973 121 | 0.129 546 896 109  |
| C                                                             | -0.165 917 941 715 | -0.016 038 345 114 | 0.162 033 674 442  |
| C                                                             | -0.126 901 756 879 | -0.044 589 439 383 | 0.268 918 061 157  |
| C                                                             | -0.134 753 942 549 | -0.102 808 241 384 | -0.115 319 663 193 |
| C                                                             | -0.124 935 300 871 | 0.054 442 779 580  | -0.038 043 867 147 |
| C                                                             | 0.188 989 606 485  | -0.051 951 815 335 | -0.226 144 710 226 |
| C                                                             | 0.081 206 652 892  | 0.060 407 309 311  | 0.118 111 489 673  |
| C                                                             | 0.155 288 055 413  | -0.151 969 019 223 | -0.007 590 903 109 |
| H                                                             | -0.041 654 551 430 | 0.069 103 047 424  | 0.016 968 201 105  |
| H                                                             | 0.059 703 079 704  | 0.077 066 851 958  | 0.009 007 099 129  |
| H                                                             | -0.067 696 270 676 | -0.049 342 376 725 | 0.019 833 033 943  |
| H                                                             | 0.025 325 911 690  | 0.000 778 556 385  | -0.053 660 025 725 |
| H                                                             | 0.007 526 698 107  | -0.020 859 437 577 | 0.161 338 094 272  |
| H                                                             | 0.022 104 303 812  | 0.117 190 459 446  | 0.011 684 388 945  |
| H                                                             | -0.029 670 182 041 | -0.003 517 679 037 | 0.003 161 829 212  |
| H                                                             | -0.052 389 730 704 | -0.046 700 137 704 | -0.178 630 774 780 |
| H                                                             | 0.013 140 085 036  | -0.035 986 764 674 | -0.102 655 810 787 |
| H                                                             | 0.024 609 863 589  | 0.001 857 958 732  | -0.069 792 705 325 |
| H                                                             | 0.002 304 398 317  | 0.034 608 232 702  | 0.059 018 455 572  |
| H                                                             | 0.136 599 115 868  | -0.034 355 402 696 | -0.036 980 497 697 |
| H                                                             | 0.142 317 986 388  | -0.044 113 987 010 | -0.030 281 696 989 |
| H                                                             | 0.080 664 835 838  | -0.009 673 560 867 | -0.118 329 797 210 |
| H                                                             | 0.032 709 587 460  | 0.049 049 201 217  | 0.086 206 518 801  |
| H                                                             | -0.043 743 640 277 | 0.082 846 596 406  | 0.002 211 419 922  |

Wavenumber/cm<sup>-1</sup>: 1525.988 , Max excitation: 1

| $l'$ -matrix coefficients/(u <sup>1/2</sup> Å <sup>-1</sup> ) |                    |                    |
|---------------------------------------------------------------|--------------------|--------------------|
| O                                                             | -0.031 824 421 981 | 0.171 865 582 311  |
| C                                                             | 0.068 314 743 697  | 0.124 639 731 315  |
| C                                                             | 0.158 167 333 203  | -0.203 287 799 997 |
| C                                                             | -0.192 357 559 595 | 0.135 423 956 754  |
| C                                                             | 0.028 240 008 040  | -0.271 531 818 015 |
| C                                                             | 0.087 564 900 189  | -0.029 511 964 006 |
| C                                                             | 0.127 665 941 404  | -0.108 125 864 907 |
| C                                                             | 0.117 143 599 320  | -0.293 510 766 798 |
| C                                                             | 0.037 714 371 747  | -0.028 333 187 930 |
| C                                                             | 0.096 787 798 595  | 0.072 281 832 971  |
| C                                                             | -0.457 385 005 398 | 0.340 438 132 769  |
| H                                                             | 0.130 372 404 542  | -0.042 435 567 993 |
| H                                                             | 0.059 056 856 707  | -0.037 677 356 192 |
| H                                                             | -0.035 672 629 834 | -0.078 261 907 184 |
| H                                                             | -0.048 119 221 866 | 0.033 523 920 676  |
| H                                                             | 0.013 277 670 414  | 0.027 187 796 488  |
| H                                                             | 0.027 750 858 099  | -0.065 713 185 622 |
| H                                                             | 0.009 682 508 027  | 0.068 593 336 463  |
| H                                                             | 0.041 701 944 002  | -0.052 312 587 323 |
| H                                                             | 0.021 407 753 847  | -0.089 445 313 936 |
| H                                                             | -0.029 168 737 191 | 0.016 526 594 151  |
| H                                                             | -0.034 167 979 031 | 0.021 124 991 092  |
| H                                                             | -0.130 317 825 871 | 0.107 826 322 264  |
| H                                                             | -0.111 116 647 737 | 0.095 024 356 634  |
| H                                                             | 0.044 898 524 969  | -0.010 674 059 933 |
| H                                                             | 0.070 548 097 431  | 0.101 308 168 288  |
| H                                                             | -0.151 388 589 134 | 0.123 432 766 738  |

Wavenumber/cm<sup>-1</sup>: 3002.4521 , Max excitation: 2

| $l'$ -matrix coefficients/(u <sup>1/2</sup> Å <sup>-1</sup> ) |                    |                    |                    |
|---------------------------------------------------------------|--------------------|--------------------|--------------------|
| O                                                             | 0.016 530 271 683  | 0.221 387 388 811  | -0.108 463 922 165 |
| C                                                             | -0.085 348 113 048 | 0.183 357 322 904  | -0.063 965 029 320 |
| C                                                             | -0.296 790 842 817 | -0.089 859 321 369 | 0.107 568 234 310  |
| C                                                             | 0.129 281 293 830  | -0.037 501 320 437 | 0.030 638 675 171  |
| C                                                             | -0.139 582 210 885 | -0.235 648 784 401 | -0.013 363 270 648 |
| C                                                             | 0.186 511 232 711  | 0.097 985 656 045  | 0.121 067 604 615  |
| C                                                             | 0.105 212 258 696  | -0.039 003 513 528 | -0.019 304 239 680 |
| C                                                             | -0.007 155 039 186 | -0.155 435 478 803 | -0.167 872 357 696 |
| C                                                             | -0.208 643 173 865 | 0.099 058 278 521  | 0.361 498 224 236  |
| C                                                             | -0.019 938 033 152 | -0.056 818 739 346 | -0.193 355 393 408 |
| C                                                             | 0.179 880 151 847  | -0.087 647 676 710 | -0.026 391 709 068 |
| H                                                             | 0.213 236 738 658  | 0.095 624 283 770  | -0.064 858 340 837 |
| H                                                             | 0.023 915 856 189  | 0.015 662 268 340  | 0.004 525 272 238  |
| H                                                             | -0.011 550 736 139 | -0.057 273 958 543 | -0.023 330 608 935 |
| H                                                             | 0.020 683 275 610  | 0.036 954 886 475  | 0.052 758 822 832  |
| H                                                             | 0.005 414 258 316  | 0.145 410 771 835  | 0.190 922 333 474  |
| H                                                             | 0.036 204 048 324  | 0.033 543 964 066  | -0.037 999 148 515 |
| H                                                             | 0.123 508 816 336  | 0.066 623 933 621  | 0.014 204 399 422  |
| H                                                             | 0.018 747 146 400  | 0.012 674 895 417  | -0.005 694 466 816 |
| H                                                             | -0.001 247 122 804 | -0.076 669 401 176 | -0.137 438 459 930 |
| H                                                             | -0.069 678 727 027 | 0.052 447 812 271  | 0.171 948 057 778  |
| H                                                             | -0.009 802 742 573 | -0.054 651 463 527 | -0.173 293 833 525 |
| H                                                             | 0.054 463 164 529  | -0.019 962 613 264 | -0.013 338 522 115 |
| H                                                             | 0.071 266 863 017  | -0.029 800 308 573 | -0.015 254 663 818 |
| H                                                             | -0.053 636 539 103 | 0.048 514 337 162  | 0.143 676 442 268  |
| H                                                             | 0.010 502 875 866  | -0.027 489 279 359 | -0.134 085 442 435 |
| H                                                             | 0.042 600 231 010  | -0.013 776 181 969 | -0.011 880 002 564 |

Wavenumber/cm<sup>-1</sup>: 3016.5945 , Max excitation: 1

| $l'$ -matrix coefficients/(u <sup>1/2</sup> Å <sup>-1</sup> ) |                    |                    |
|---------------------------------------------------------------|--------------------|--------------------|
| O                                                             | -0.121 964 624 492 | 0.233 424 149 804  |
| C                                                             | 0.229 654 087 020  | 0.121 788 811 375  |
| C                                                             | 0.020 012 642 484  | -0.153 743 801 928 |
| C                                                             | 0.259 117 657 154  | 0.201 513 546 518  |
| C                                                             | -0.128 756 773 704 | -0.158 774 776 712 |
| C                                                             | -0.308 714 939 757 | -0.212 441 702 947 |
| C                                                             | 0.063 083 099 017  | 0.103 954 136 921  |
| C                                                             | -0.015 532 471 876 | -0.060 101 270 206 |
| C                                                             | 0.060 059 335 335  | 0.074 866 799 724  |
| C                                                             | 0.002 902 214 471  | 0.004 730 045 977  |
| C                                                             | 0.091 842 199 666  | -0.119 664 543 585 |
| H                                                             | -0.195 056 146 834 | -0.208 988 783 986 |
| H                                                             | -0.066 968 945 410 | -0.044 539 739 062 |
| H                                                             | -0.064 506 351 808 | -0.041 318 861 541 |
| H                                                             | 0.030 567 519 205  | 0.082 254 265 020  |
| H                                                             | -0.185 301 513 818 | -0.076 979 662 756 |
| H                                                             | 0.013 642 497 824  | 0.050 938 956 837  |
| H                                                             | -0.004 978 383 955 | 0.029 580 172 793  |
| H                                                             | 0.010 340 713 405  | 0.085 818 042 790  |
| H                                                             | -0.012 737 887 543 | -0.041 156 017 774 |
| H                                                             | -0.023 971 518 135 | 0.068 737 878 126  |
| H                                                             | -0.032 919 940 996 | -0.002 438 921 608 |
| H                                                             | -0.069 277 002 177 | -0.028 116 266 814 |
| H                                                             | -0.030 043 392 547 | -0.056 188 535 111 |
| H                                                             | 0.053 119 526 353  | 0.034 525 150 934  |
| H                                                             | 0.024 017 444 926  | 0.041 755 704 491  |
| H                                                             | 0.095 296 532 638  | -0.140 810 716 969 |

Wavenumber/cm<sup>-1</sup>: 3026.2253 , Max excitation: 1

| $l'$ -matrix coefficients/(u <sup>1/2</sup> Å <sup>-1</sup> ) |                    |                    |                    |
|---------------------------------------------------------------|--------------------|--------------------|--------------------|
| O                                                             | 0.150 098 457 911  | 0.145 133 149 774  | -0.157 889 203 573 |
| C                                                             | -0.187 080 265 271 | 0.072 362 770 391  | -0.288 015 504 231 |
| C                                                             | -0.099 492 782 906 | 0.268 298 492 043  | 0.048 046 933 613  |
| C                                                             | -0.085 036 068 364 | -0.066 930 562 358 | 0.182 715 522 202  |
| C                                                             | 0.127 930 381 535  | 0.103 063 752 800  | -0.107 301 283 907 |
| C                                                             | -0.018 345 303 317 | -0.417 691 617 103 | 0.026 063 313 379  |
| C                                                             | 0.007 009 515 126  | 0.022 197 051 119  | 0.032 576 152 567  |
| C                                                             | -0.030 024 967 362 | -0.033 581 706 059 | 0.081 882 328 546  |
| C                                                             | -0.113 601 295 810 | 0.002 977 341 818  | 0.190 265 554 381  |
| C                                                             | 0.211 731 336 464  | -0.025 939 927 193 | 0.028 017 842 001  |
| C                                                             | -0.045 274 619 822 | 0.074 189 857 659  | -0.037 919 906 277 |
| H                                                             | -0.078 190 298 658 | -0.230 042 803 366 | 0.114 607 476 505  |
| H                                                             | 0.065 077 738 436  | 0.050 982 590 594  | 0.029 080 517 755  |
| H                                                             | 0.103 638 457 440  | 0.049 956 310 911  | -0.080 841 548 511 |
| H                                                             | -0.032 445 579 724 | -0.051 416 187 833 | 0.075 648 879 199  |
| H                                                             | 0.036 843 916 106  | -0.223 275 937 389 | -0.135 685 555 522 |
| H                                                             | -0.067 526 320 607 | -0.130 848 543 777 | 0.005 585 371 390  |
| H                                                             | 0.142 821 686 520  | -0.029 878 644 650 | 0.069 248 596 661  |
| H                                                             | -0.008 550 354 672 | 0.004 617 453 230  | -0.065 711 674 018 |
| H                                                             | -0.039 079 012 463 | 0.045 474 033 094  | 0.147 353 040 553  |
| H                                                             | 0.020 900 516 636  | -0.048 123 616 408 | -0.006 239 020 005 |
| H                                                             | 0.123 380 099 814  | -0.021 258 697 050 | 0.043 204 966 547  |
| H                                                             | -0.015 150 858 237 | 0.058 321 544 147  | -0.049 293 332 918 |
| H                                                             | 0.068 858 523 842  | -0.017 402 495 271 | -0.056 245 929 425 |
| H                                                             | -0.079 795 588 833 | -0.017 742 287 650 | 0.135 845 120 334  |
| H                                                             | 0.026 764 482 164  | -0.098 816 981 353 | -0.108 428 528 496 |
| H                                                             | -0.064 056 491 046 | 0.084 872 467 380  | -0.028 736 765 413 |

Wavenumber/cm<sup>-1</sup>: 3027.8074 , Max excitation: 1

| $l'$ -matrix coefficients/(u <sup>1/2</sup> Å <sup>-1</sup> ) |                    |                    |
|---------------------------------------------------------------|--------------------|--------------------|
| O                                                             | -0.097 253 442 890 | 0.009 144 548 495  |
| C                                                             | 0.180 659 457 280  | -0.021 394 034 904 |
| C                                                             | 0.171 953 304 720  | 0.077 915 172 810  |
| C                                                             | 0.139 142 888 822  | -0.020 082 180 879 |
| C                                                             | 0.025 136 820 428  | -0.045 857 698 925 |
| C                                                             | 0.101 962 957 056  | 0.022 165 217 183  |
| C                                                             | -0.203 729 798 626 | -0.014 506 620 582 |
| C                                                             | -0.250 185 702 409 | -0.045 561 965 387 |
| C                                                             | -0.271 049 548 905 | -0.019 668 424 586 |
| C                                                             | 0.237 438 663 047  | 0.246 676 374 419  |
| C                                                             | 0.124 314 927 455  | -0.170 231 079 641 |
| H                                                             | 0.051 244 307 618  | 0.030 411 275 774  |
| H                                                             | -0.115 660 997 641 | -0.046 392 487 994 |
| H                                                             | -0.029 544 457 402 | -0.064 653 807 162 |
| H                                                             | -0.239 358 544 765 | 0.018 916 120 630  |
| H                                                             | 0.006 966 426 608  | 0.040 708 618 969  |
| H                                                             | -0.125 998 025 208 | -0.097 591 644 527 |
| H                                                             | 0.072 171 309 224  | 0.106 355 761 435  |
| H                                                             | -0.069 480 185 632 | 0.043 337 161 630  |
| H                                                             | -0.091 499 603 774 | 0.022 045 974 085  |
| H                                                             | -0.074 567 898 078 | -0.035 216 859 106 |
| H                                                             | 0.046 190 182 970  | 0.064 776 357 806  |
| H                                                             | 0.010 145 469 669  | -0.068 934 491 579 |
| H                                                             | -0.008 072 469 252 | -0.030 912 738 861 |
| H                                                             | -0.082 238 483 044 | -0.050 353 144 202 |
| H                                                             | 0.084 157 618 395  | 0.101 728 426 221  |
| H                                                             | 0.070 532 524 929  | -0.103 294 792 778 |



Wavenumber/cm<sup>-1</sup>: 3030.925 , Max excitation: 1

| $l'$ -matrix coefficients/(u <sup>1/2</sup> Å <sup>-1</sup> ) |                    |                    |
|---------------------------------------------------------------|--------------------|--------------------|
| O                                                             | -0.024 316 004 735 | -0.049 318 012 602 |
| C                                                             | 0.047 930 499 971  | -0.078 215 652 261 |
| C                                                             | -0.023 539 728 175 | -0.039 797 073 743 |
| C                                                             | 0.066 353 126 382  | 0.053 208 578 287  |
| C                                                             | 0.047 672 693 480  | 0.009 575 647 527  |
| C                                                             | 0.067 447 573 641  | -0.004 648 113 529 |
| C                                                             | 0.186 257 761 485  | 0.209 868 940 902  |
| C                                                             | 0.268 518 952 783  | 0.268 273 222 182  |
| C                                                             | -0.363 252 412 323 | -0.223 361 435 453 |
| C                                                             | -0.160 744 941 621 | -0.078 990 000 223 |
| C                                                             | -0.026 731 808 573 | -0.043 595 324 187 |
| H                                                             | 0.032 894 440 358  | -0.022 064 558 033 |
| H                                                             | 0.025 760 217 346  | 0.120 786 665 112  |
| H                                                             | 0.016 629 570 414  | -0.010 330 770 497 |
| H                                                             | -0.189 892 291 232 | -0.163 894 133 395 |
| H                                                             | 0.012 419 795 646  | 0.003 423 028 280  |
| H                                                             | 0.111 930 187 337  | 0.195 568 924 783  |
| H                                                             | -0.080 867 231 542 | -0.086 061 227 562 |
| H                                                             | 0.072 455 897 421  | 0.016 856 771 457  |
| H                                                             | 0.107 937 964 479  | 0.020 864 566 905  |
| H                                                             | -0.195 785 918 228 | -0.055 315 719 378 |
| H                                                             | -0.068 945 344 272 | 0.007 539 289 903  |
| H                                                             | -0.085 521 105 748 | 0.021 450 057 267  |
| H                                                             | 0.031 211 741 278  | -0.058 530 534 208 |
| H                                                             | -0.029 833 926 035 | -0.001 147 941 656 |
| H                                                             | -0.037 462 094 028 | -0.007 949 687 968 |
| H                                                             | -0.005 468 238 581 | -0.034 350 968 017 |

Wavenumber/cm<sup>-1</sup>: 3056.5151 , Max excitation: 1

| $l'$ -matrix coefficients/(u <sup>1/2</sup> Å <sup>-1</sup> ) |                    |                    |                    |
|---------------------------------------------------------------|--------------------|--------------------|--------------------|
| O                                                             | 0.022 762 843 289  | 0.355 067 965 934  | -0.004 450 886 392 |
| C                                                             | -0.024 993 165 167 | 0.354 098 764 723  | 0.209 274 119 248  |
| C                                                             | -0.037 635 069 831 | 0.099 799 109 811  | -0.129 934 466 548 |
| C                                                             | 0.083 623 455 343  | 0.024 833 325 225  | -0.131 315 626 030 |
| C                                                             | 0.078 191 334 062  | 0.069 722 548 194  | -0.143 714 957 784 |
| C                                                             | 0.072 084 010 508  | -0.014 382 493 801 | -0.143 815 843 556 |
| C                                                             | -0.061 975 028 173 | -0.259 734 066 327 | 0.135 200 326 368  |
| C                                                             | 0.100 082 881 132  | -0.125 559 461 523 | -0.001 788 063 305 |
| C                                                             | -0.041 131 558 281 | -0.278 563 204 048 | -0.018 890 550 474 |
| C                                                             | -0.258 017 991 200 | -0.081 995 605 561 | 0.104 672 748 654  |
| C                                                             | 0.114 692 096 012  | 0.021 607 250 588  | 0.030 155 925 019  |
| H                                                             | -0.001 962 477 372 | -0.020 905 971 351 | -0.024 170 989 395 |
| H                                                             | -0.140 940 953 500 | -0.174 125 471 191 | -0.001 846 899 877 |
| H                                                             | 0.059 689 804 863  | 0.059 794 023 004  | -0.036 687 865 617 |
| H                                                             | -0.004 239 584 104 | -0.226 771 938 669 | 0.045 888 887 428  |
| H                                                             | 0.019 771 753 450  | -0.015 262 713 303 | -0.070 874 028 436 |
| H                                                             | -0.002 449 481 804 | -0.024 691 871 272 | -0.025 818 751 628 |
| H                                                             | -0.136 727 606 127 | -0.115 417 833 013 | 0.003 586 845 093  |
| H                                                             | 0.008 455 162 311  | -0.077 971 692 491 | 0.194 976 312 041  |
| H                                                             | 0.086 466 115 684  | -0.047 010 895 433 | 0.032 104 365 367  |
| H                                                             | -0.017 932 716 344 | -0.116 817 116 768 | -0.144 452 990 337 |
| H                                                             | -0.091 331 272 601 | 0.017 194 399 508  | 0.131 326 672 829  |
| H                                                             | 0.077 420 337 239  | -0.015 410 300 462 | 0.020 865 267 491  |
| H                                                             | 0.009 602 648 268  | 0.036 804 743 088  | 0.031 885 441 328  |
| H                                                             | -0.007 418 755 577 | -0.036 789 093 404 | 0.109 541 462 147  |
| H                                                             | -0.070 226 412 878 | -0.015 343 680 279 | 0.035 834 728 846  |
| H                                                             | 0.035 107 736 430  | 0.014 582 849 803  | 0.026 792 438 144  |

Wavenumber/cm<sup>-1</sup>: 3073.7315 , Max excitation: 1

| $l'$ -matrix coefficients/(u <sup>1/2</sup> Å <sup>-1</sup> ) |                    |                    |
|---------------------------------------------------------------|--------------------|--------------------|
| O                                                             | -0.028 818 129 448 | 0.037 704 840 619  |
| C                                                             | 0.058 362 066 443  | 0.053 864 151 433  |
| C                                                             | 0.026 726 313 837  | -0.041 299 854 625 |
| C                                                             | 0.134 641 909 772  | 0.048 414 044 580  |
| C                                                             | 0.106 248 565 301  | -0.099 444 890 659 |
| C                                                             | 0.291 391 347 001  | -0.059 204 932 700 |
| C                                                             | 0.016 933 640 262  | 0.207 548 837 878  |
| C                                                             | -0.286 868 246 701 | -0.102 116 244 240 |
| C                                                             | 0.119 820 572 646  | 0.037 988 878 324  |
| C                                                             | -0.309 246 396 549 | 0.024 706 378 615  |
| C                                                             | -0.033 000 424 744 | -0.105 476 733 915 |
| H                                                             | 0.141 179 020 395  | -0.044 853 241 356 |
| H                                                             | 0.071 968 683 041  | 0.115 072 320 586  |
| H                                                             | 0.065 912 592 980  | -0.039 652 265 834 |
| H                                                             | 0.030 725 245 532  | 0.097 588 281 543  |
| H                                                             | 0.092 550 703 477  | -0.012 656 313 227 |
| H                                                             | -0.142 315 837 736 | -0.159 133 377 376 |
| H                                                             | -0.169 204 349 311 | -0.009 366 680 705 |
| H                                                             | -0.039 902 196 660 | 0.128 746 327 179  |
| H                                                             | -0.166 855 211 249 | 0.037 426 009 723  |
| H                                                             | 0.110 897 524 184  | -0.012 480 157 212 |
| H                                                             | -0.109 942 126 737 | 0.024 660 856 714  |
| H                                                             | -0.156 183 613 582 | 0.022 737 680 937  |
| H                                                             | 0.090 541 136 168  | -0.099 718 721 758 |
| H                                                             | -0.030 850 612 429 | -0.062 323 529 886 |
| H                                                             | -0.082 601 266 295 | 0.046 496 465 570  |
| H                                                             | -0.022 635 946 477 | -0.061 873 092 179 |

Wavenumber/cm<sup>-1</sup>: 3089.3435 , Max excitation: 1

| $l'$ -matrix coefficients/(u <sup>1/2</sup> Å <sup>-1</sup> ) |                    |                    |                    |
|---------------------------------------------------------------|--------------------|--------------------|--------------------|
| O                                                             | 0.014 678 740 546  | 0.210 198 009 392  | 0.547 970 991 526  |
| C                                                             | 0.009 334 422 431  | -0.233 766 164 583 | -0.685 394 704 864 |
| C                                                             | 0.007 550 275 066  | -0.026 997 321 218 | -0.062 870 498 603 |
| C                                                             | -0.009 739 720 940 | -0.024 086 937 199 | -0.021 465 655 588 |
| C                                                             | 0.008 791 331 165  | 0.000 448 173 312  | -0.008 294 677 655 |
| C                                                             | 0.053 720 920 512  | 0.077 373 305 247  | 0.000 298 938 394  |
| C                                                             | -0.089 372 176 808 | -0.084 332 152 612 | 0.088 573 029 639  |
| C                                                             | -0.022 124 557 045 | -0.027 462 654 035 | 0.025 430 377 643  |
| C                                                             | 0.112 413 858 634  | -0.069 773 401 332 | 0.039 013 239 031  |
| C                                                             | -0.133 162 663 565 | 0.089 926 376 202  | -0.037 796 242 585 |
| C                                                             | 0.045 334 133 842  | 0.035 678 123 544  | -0.012 452 693 627 |
| H                                                             | 0.033 201 491 855  | 0.037 250 011 184  | -0.015 937 226 293 |
| H                                                             | -0.059 107 182 072 | -0.045 046 930 863 | 0.018 542 758 991  |
| H                                                             | 0.003 806 733 689  | 0.003 521 211 706  | -0.000 644 659 169 |
| H                                                             | 0.049 831 638 754  | -0.051 067 381 046 | 0.013 446 054 101  |
| H                                                             | 0.017 804 397 963  | 0.035 953 222 769  | 0.036 448 082 058  |
| H                                                             | -0.015 763 335 771 | 0.006 040 406 947  | -0.002 784 649 484 |
| H                                                             | -0.053 372 677 694 | 0.043 570 831 562  | -0.023 785 737 468 |
| H                                                             | -0.017 463 637 130 | -0.028 312 859 391 | 0.075 709 096 393  |
| H                                                             | 0.011 442 942 398  | -0.014 321 934 054 | 0.008 729 770 635  |
| H                                                             | 0.014 257 071 701  | -0.013 640 365 797 | -0.004 021 153 819 |
| H                                                             | -0.030 349 932 914 | 0.020 307 785 567  | -0.017 792 394 928 |
| H                                                             | 0.026 475 452 742  | 0.015 623 472 462  | -0.012 583 566 103 |
| H                                                             | 0.008 695 367 564  | 0.004 160 460 344  | -0.005 642 979 667 |
| H                                                             | 0.046 584 363 837  | 0.003 371 587 572  | 0.042 836 972 395  |
| H                                                             | -0.046 225 034 458 | 0.031 089 190 175  | 0.021 716 436 143  |
| H                                                             | 0.011 262 166 905  | 0.021 901 455 906  | 0.012 548 725 915  |

Wavenumber/cm<sup>-1</sup>: 3091.3788 , Max excitation: 1

| $l'$ -matrix coefficients/(u <sup>1/2</sup> Å <sup>-1</sup> ) |                    |                    |                    |
|---------------------------------------------------------------|--------------------|--------------------|--------------------|
| O                                                             | 0.002 959 328 836  | 0.027 277 354 657  | -0.130 669 588 267 |
| C                                                             | -0.006 542 285 561 | -0.012 963 932 175 | -0.212 704 667 064 |
| C                                                             | -0.067 319 082 328 | 0.022 130 843 606  | -0.015 309 793 754 |
| C                                                             | 0.057 335 396 109  | -0.023 528 302 887 | -0.096 429 194 681 |
| C                                                             | 0.015 906 433 374  | 0.009 003 823 061  | 0.064 312 971 821  |
| C                                                             | -0.008 927 156 618 | 0.044 971 780 518  | -0.053 237 975 495 |
| C                                                             | 0.221 833 307 647  | -0.045 937 507 683 | -0.158 214 880 282 |
| C                                                             | 0.048 167 738 176  | -0.175 219 084 107 | 0.210 215 553 016  |
| C                                                             | -0.201 142 216 157 | 0.186 776 895 430  | -0.141 854 455 210 |
| C                                                             | -0.238 615 535 914 | -0.137 043 918 406 | 0.174 077 092 758  |
| C                                                             | 0.199 981 302 791  | 0.080 595 648 044  | 0.253 124 056 641  |
| H                                                             | -0.028 371 496 664 | 0.029 631 912 964  | -0.021 424 296 625 |
| H                                                             | 0.181 595 595 765  | -0.012 261 734 253 | -0.040 470 993 386 |
| H                                                             | 0.016 562 010 383  | 0.038 799 040 403  | 0.045 377 609 495  |
| H                                                             | -0.137 345 924 517 | 0.270 048 419 682  | -0.076 664 269 782 |
| H                                                             | -0.011 462 436 747 | 0.021 385 205 320  | -0.015 704 653 814 |
| H                                                             | 0.031 108 111 896  | -0.154 287 307 910 | 0.095 646 420 686  |
| H                                                             | -0.127 657 096 345 | -0.033 248 229 592 | 0.009 433 777 502  |
| H                                                             | 0.037 991 078 750  | 0.008 683 572 661  | -0.147 736 147 779 |
| H                                                             | -0.050 451 456 215 | 0.000 187 654 308  | 0.134 182 915 018  |
| H                                                             | 0.058 180 548 338  | 0.023 195 359 112  | 0.087 831 477 096  |
| H                                                             | 0.004 667 205 511  | -0.051 803 198 190 | 0.105 745 310 893  |
| H                                                             | 0.167 397 608 786  | -0.015 515 069 635 | 0.086 495 055 458  |
| H                                                             | -0.006 038 488 623 | 0.076 436 279 787  | 0.119 832 469 460  |
| H                                                             | -0.157 432 663 824 | -0.093 735 740 041 | -0.184 423 747 909 |
| H                                                             | -0.124 102 253 966 | -0.091 591 532 099 | 0.103 313 032 678  |
| H                                                             | 0.062 189 715 948  | 0.052 189 152 382  | 0.136 390 065 864  |

Wavenumber/cm<sup>-1</sup>: 3093.3404 , Max excitation: 1

| $l'$ -matrix coefficients/(u <sup>1/2</sup> Å <sup>-1</sup> ) |                    |                    |                    |
|---------------------------------------------------------------|--------------------|--------------------|--------------------|
| O                                                             | 0.020 454 518 533  | 0.124 356 275 130  | -0.189 070 090 303 |
| C                                                             | 0.043 685 843 966  | 0.078 366 421 200  | -0.228 518 902 520 |
| C                                                             | 0.036 775 608 358  | 0.029 222 185 596  | -0.040 977 517 610 |
| C                                                             | -0.027 072 098 678 | 0.092 353 482 351  | -0.050 306 969 598 |
| C                                                             | -0.026 026 777 340 | 0.103 831 455 570  | -0.008 812 113 122 |
| C                                                             | 0.061 122 791 371  | 0.255 241 543 973  | -0.021 935 026 413 |
| C                                                             | -0.008 718 870 699 | 0.062 604 005 661  | 0.001 290 841 648  |
| C                                                             | -0.076 317 169 673 | 0.034 389 952 636  | 0.091 773 909 480  |
| C                                                             | 0.159 741 955 433  | 0.014 093 221 560  | 0.056 497 269 613  |
| C                                                             | 0.123 696 821 925  | -0.342 897 231 229 | 0.120 272 621 839  |
| C                                                             | -0.294 795 230 159 | -0.318 655 899 944 | 0.148 036 961 697  |
| H                                                             | 0.038 914 099 464  | 0.112 964 553 623  | -0.042 597 348 630 |
| H                                                             | 0.011 884 315 771  | 0.002 641 368 181  | -0.004 745 066 395 |
| H                                                             | -0.014 844 224 296 | 0.036 339 108 741  | 0.012 261 356 158  |
| H                                                             | 0.083 171 281 451  | -0.053 201 291 940 | 0.014 383 979 006  |
| H                                                             | 0.014 520 081 880  | 0.100 041 185 604  | 0.047 386 994 839  |
| H                                                             | -0.025 211 093 057 | -0.029 235 205 728 | 0.032 369 477 405  |
| H                                                             | 0.080 065 310 386  | -0.241 294 433 931 | 0.089 680 773 011  |
| H                                                             | -0.010 087 802 265 | 0.032 111 847 469  | -0.002 762 506 474 |
| H                                                             | -0.040 949 489 990 | 0.028 252 023 487  | 0.058 777 160 549  |
| H                                                             | 0.013 630 616 301  | 0.018 160 385 789  | -0.002 251 244 634 |
| H                                                             | 0.008 801 133 267  | -0.048 258 031 432 | 0.154 136 725 361  |
| H                                                             | -0.208 568 878 308 | -0.188 140 548 510 | 0.174 308 113 042  |
| H                                                             | -0.101 558 599 167 | 0.017 408 059 999  | 0.105 700 698 039  |
| H                                                             | 0.072 743 983 933  | 0.048 070 489 890  | 0.067 102 468 904  |
| H                                                             | 0.058 197 636 539  | -0.123 429 226 592 | -0.096 347 525 811 |
| H                                                             | -0.034 905 556 099 | -0.237 387 093 232 | -0.086 524 821 490 |

Wavenumber/cm<sup>-1</sup>: 3094.9856 , Max excitation: 1

| $l'$ -matrix coefficients/(u <sup>1/2</sup> Å <sup>-1</sup> ) |                    |                    |                    |
|---------------------------------------------------------------|--------------------|--------------------|--------------------|
| O                                                             | 0.689 114 240 659  | -0.029 031 380 144 | -0.015 299 855 760 |
| C                                                             | -0.077 540 168 673 | 0.025 072 124 454  | 0.008 514 567 192  |
| C                                                             | -0.036 191 296 913 | 0.023 357 783 871  | 0.008 335 178 825  |
| C                                                             | -0.040 596 707 846 | 0.007 224 323 272  | 0.010 165 846 738  |
| C                                                             | -0.015 891 571 423 | 0.022 730 123 662  | -0.005 297 245 061 |
| C                                                             | -0.018 946 144 970 | 0.000 842 205 444  | 0.014 974 878 173  |
| C                                                             | -0.137 891 858 559 | -0.126 235 754 760 | 0.153 268 641 251  |
| C                                                             | 0.056 355 112 771  | 0.044 089 523 744  | -0.057 839 134 967 |
| C                                                             | -0.123 748 781 093 | 0.134 592 443 495  | -0.081 043 581 467 |
| C                                                             | -0.085 189 897 361 | 0.084 298 350 302  | -0.016 519 388 735 |
| C                                                             | -0.180 432 878 638 | -0.170 075 175 753 | -0.005 038 122 274 |
| H                                                             | -0.000 423 618 205 | -0.004 614 381 640 | 0.006 515 948 312  |
| H                                                             | -0.141 215 362 047 | -0.072 537 032 339 | 0.027 661 961 948  |
| H                                                             | 0.002 114 268 055  | 0.011 005 049 881  | -0.003 819 408 666 |
| H                                                             | -0.077 993 580 044 | 0.208 479 973 753  | -0.062 357 650 846 |
| H                                                             | -0.000 783 660 825 | -0.003 578 162 648 | 0.003 774 566 721  |
| H                                                             | 0.018 588 394 730  | 0.100 086 639 484  | -0.035 562 007 864 |
| H                                                             | -0.074 940 248 156 | 0.189 272 889 318  | -0.068 124 856 718 |
| H                                                             | -0.010 070 563 076 | -0.064 658 211 371 | 0.147 391 245 795  |
| H                                                             | 0.082 034 091 029  | -0.029 451 528 253 | -0.064 514 597 464 |
| H                                                             | 0.065 250 621 382  | 0.010 771 475 884  | 0.085 489 216 610  |
| H                                                             | 0.114 006 780 880  | -0.056 161 223 931 | -0.073 718 965 930 |
| H                                                             | -0.128 922 530 129 | -0.091 220 783 902 | 0.062 006 276 156  |
| H                                                             | -0.026 266 713 582 | -0.001 654 904 118 | 0.015 435 882 324  |
| H                                                             | -0.121 905 829 206 | -0.078 218 829 282 | -0.119 568 096 685 |
| H                                                             | -0.122 332 731 195 | -0.050 438 228 385 | 0.127 723 436 225  |
| H                                                             | -0.044 061 476 138 | -0.109 851 377 279 | -0.089 285 262 997 |

Wavenumber/cm<sup>-1</sup>: 3104.1416 , Max excitation: 1

| $l'$ -matrix coefficients/(u <sup>1/2</sup> Å <sup>-1</sup> ) |                    |                    |                                       |
|---------------------------------------------------------------|--------------------|--------------------|---------------------------------------|
| O                                                             | 0.412 513 963 056  | -0.009 311 326 652 | 0.021 403 023 815                     |
| C                                                             | 0.005 108 836 020  | 0.019 951 917 276  | 0.016 611 277 721                     |
| C                                                             | -0.025 889 083 002 | -0.045 723 197 342 | -0.002 480 344 139                    |
| C                                                             | 0.005 958 742 487  | 0.024 145 917 773  | -0.028 474 608 031                    |
| C                                                             | -0.036 046 230 123 | -0.039 895 664 281 | -0.003 817 845 076                    |
| C                                                             | -0.029 253 368 011 | -0.021 602 714 364 | -0.041 305 670 475                    |
| C                                                             | 0.062 232 478 222  | 0.092 080 196 896  | -0.132 297 488 790                    |
| C                                                             | -0.103 235 339 683 | -0.055 715 274 077 | 0.035 129 238 107                     |
| C                                                             | -0.037 763 717 110 | -0.002 687 523 219 | 0.002 959 614 990                     |
| C                                                             | -0.126 261 289 777 | 0.170 321 554 084  | -0.053 867 112 582                    |
| C                                                             | -0.086 339 978 171 | -0.146 048 309 130 | 0.168 684 956 418                     |
| H                                                             | -0.018 741 056 146 | -0.012 098 905 308 | -0.003 916 563 447                    |
| H                                                             | 0.099 135 355 777  | 0.052 417 234 040  | -0.026 364 573 659                    |
| H                                                             | -0.015 273 020 132 | -0.015 949 930 542 | 0.001 359 198 884                     |
| H                                                             | 0.011 626 382 410  | -0.170 348 330 990 | 0.051 005 694 735                     |
| H                                                             | -0.019 988 829 145 | -0.001 614 907 815 | -0.026 236 372 763                    |
| H                                                             | -0.033 556 554 098 | -0.089 993 718 321 | 0.025 304 628 549                     |
| H                                                             | -0.004 324 691 075 | -0.111 605 695 186 | 0.034 574 913 618                     |
| H                                                             | -0.006 063 092 025 | 0.052 169 732 390  | -0.116 998 449 790                    |
| H                                                             | -0.084 368 685 607 | 0.019 464 202 694  | 0.052 175 414 434                     |
| H                                                             | -0.152 227 139 397 | 0.049 107 033 208  | -0.109 553 849 866                    |
| H                                                             | -0.238 717 525 604 | 0.141 276 872 291  | 0.010 676 596 771                     |
| H                                                             | 0.073 305 460 180  | 0.138 579 066 227  | -0.164 700 813 791                    |
| H                                                             | -0.282 981 279 300 | -0.276 907 675 426 | -2.911 420 800 000 × 10 <sup>-5</sup> |
| H                                                             | 0.106 899 120 824  | 0.133 286 471 390  | 0.056 055 752 377                     |
| H                                                             | 0.100 987 113 238  | 0.191 561 136 595  | -0.111 735 913 394                    |
| H                                                             | 0.103 172 907 011  | -0.044 388 081 083 | 0.377 249 138 057                     |



Wavenumber/cm<sup>-1</sup>: 3111.8256 , Max excitation: 1

| $l'$ -matrix coefficients/(u <sup>1/2</sup> Å <sup>-1</sup> ) |                    |                    |                    |
|---------------------------------------------------------------|--------------------|--------------------|--------------------|
| O                                                             | 0.183 762 640 983  | -0.072 684 150 344 | 0.008 973 270 294  |
| C                                                             | -0.012 771 788 098 | -0.051 295 819 759 | 0.016 694 038 544  |
| C                                                             | -0.031 117 343 123 | -0.039 011 695 436 | -0.000 235 415 770 |
| C                                                             | 0.004 204 917 529  | -0.024 819 304 348 | -0.003 086 752 158 |
| C                                                             | -0.013 735 459 096 | -0.057 337 562 815 | 0.028 116 481 038  |
| C                                                             | -0.042 385 696 987 | -0.077 328 997 865 | -0.009 043 539 622 |
| C                                                             | 0.045 839 392 333  | 0.014 633 363 612  | -0.073 381 840 841 |
| C                                                             | -0.045 968 676 358 | -0.076 761 921 155 | 0.057 354 863 182  |
| C                                                             | -0.064 021 870 996 | 0.031 729 331 696  | -0.027 351 933 312 |
| C                                                             | -0.110 127 833 665 | 0.205 291 622 658  | -0.083 253 724 040 |
| C                                                             | 0.092 663 525 773  | 0.072 068 903 547  | 0.094 840 716 541  |
| H                                                             | -0.027 683 517 619 | -0.024 197 802 763 | 0.004 205 467 739  |
| H                                                             | 0.065 134 909 670  | 0.009 458 557 474  | -0.017 559 551 031 |
| H                                                             | -0.004 000 893 427 | -0.014 360 522 180 | 0.011 749 227 046  |
| H                                                             | -0.001 242 398 566 | -0.153 963 860 897 | 0.042 894 183 347  |
| H                                                             | -0.013 218 000 223 | -0.027 003 790 533 | -0.015 169 635 579 |
| H                                                             | -0.014 878 014 554 | -0.074 386 542 992 | 0.028 429 206 392  |
| H                                                             | -0.001 192 526 962 | -0.071 590 069 710 | 0.019 737 936 989  |
| H                                                             | 0.000 859 784 467  | 0.016 997 698 975  | -0.066 678 775 389 |
| H                                                             | -0.050 802 388 425 | 0.002 551 705 111  | 0.045 175 817 725  |
| H                                                             | -0.165 944 709 658 | 0.064 311 440 891  | -0.114 418 568 809 |
| H                                                             | -0.214 379 665 457 | 0.136 065 827 647  | -0.015 244 051 140 |
| H                                                             | -0.071 987 126 344 | -0.257 103 254 435 | 0.342 873 075 383  |
| H                                                             | 0.283 344 076 898  | 0.375 976 604 885  | 0.139 780 403 789  |
| H                                                             | 0.105 281 945 909  | 0.145 112 716 206  | 0.034 843 963 006  |
| H                                                             | 0.091 820 319 738  | 0.190 264 605 431  | -0.103 886 286 484 |
| H                                                             | -0.100 783 370 803 | -0.018 777 559 065 | -0.374 736 415 906 |

Wavenumber/cm<sup>-1</sup>: 3113.8672 , Max excitation: 1

| $l'$ -matrix coefficients/(u <sup>1/2</sup> Å <sup>-1</sup> ) |                                       |                    |                    |
|---------------------------------------------------------------|---------------------------------------|--------------------|--------------------|
| O                                                             | -0.081 266 532 150                    | 0.095 309 154 357  | 0.029 352 257 112  |
| C                                                             | 0.010 122 183 722                     | 0.076 031 992 264  | 0.027 031 243 505  |
| C                                                             | -0.004 920 706 954                    | 0.014 581 875 092  | -0.025 074 561 229 |
| C                                                             | 0.001 561 263 115                     | 0.020 013 952 812  | 0.000 787 243 693  |
| C                                                             | -0.006 441 910 438                    | 0.029 148 563 274  | -0.001 076 014 385 |
| C                                                             | -0.017 013 224 667                    | -0.032 403 845 258 | -0.037 012 277 084 |
| C                                                             | 0.156 332 255 462                     | 0.174 502 364 231  | -0.198 329 499 603 |
| C                                                             | 0.010 017 824 820                     | 0.050 302 679 175  | -0.032 301 323 904 |
| C                                                             | 0.057 143 998 227                     | -0.412 022 202 045 | 0.103 485 211 707  |
| C                                                             | -0.024 446 228 216                    | 0.228 124 335 412  | -0.143 372 671 324 |
| C                                                             | -0.095 612 925 547                    | -0.171 378 671 288 | 0.253 390 842 450  |
| H                                                             | -0.016 350 136 352                    | -0.019 018 260 085 | 0.000 760 012 012  |
| H                                                             | 0.134 683 744 415                     | 0.099 598 904 410  | -0.036 608 234 518 |
| H                                                             | -5.884 306 000 000 × 10 <sup>-5</sup> | 0.006 232 934 966  | -0.005 565 021 217 |
| H                                                             | 0.019 433 693 412                     | -0.101 024 911 136 | 0.022 269 175 974  |
| H                                                             | -0.009 090 885 835                    | -0.014 480 771 733 | -0.029 981 208 209 |
| H                                                             | 0.012 944 157 094                     | -0.040 541 213 062 | 0.011 663 727 259  |
| H                                                             | -0.075 807 884 077                    | 0.337 687 758 926  | -0.136 006 211 294 |
| H                                                             | 0.025 353 364 453                     | 0.058 130 579 346  | -0.162 837 598 020 |
| H                                                             | -0.048 901 159 698                    | 0.040 869 236 121  | 0.009 351 389 781  |
| H                                                             | 0.133 589 151 543                     | -0.191 864 724 526 | 0.013 651 747 300  |
| H                                                             | 0.179 764 750 092                     | -0.057 197 963 225 | -0.183 453 944 838 |
| H                                                             | -0.054 386 946 325                    | -0.115 079 177 890 | 0.148 715 321 053  |
| H                                                             | -0.058 968 646 960                    | 0.028 345 342 267  | 0.124 317 582 103  |
| H                                                             | -0.081 098 738 953                    | -0.193 582 411 693 | 0.095 073 513 712  |
| H                                                             | -0.137 946 712 949                    | -0.020 240 386 663 | 0.167 091 317 955  |
| H                                                             | 0.001 179 824 890                     | -0.117 817 050 982 | 0.025 748 409 673  |

Wavenumber/cm<sup>-1</sup>: 3124.7285 , Max excitation: 1

| $l'$ -matrix coefficients/(u <sup>1/2</sup> Å <sup>-1</sup> ) |                    |                    |                    |
|---------------------------------------------------------------|--------------------|--------------------|--------------------|
| O                                                             | 0.011 212 947 400  | 0.001 601 344 726  | 0.004 541 812 903  |
| C                                                             | 0.016 666 355 120  | 0.004 470 072 313  | 0.024 386 801 154  |
| C                                                             | 0.002 781 524 981  | -0.010 680 911 131 | -0.014 104 790 937 |
| C                                                             | 0.016 177 440 825  | -0.001 128 815 439 | -0.005 279 759 027 |
| C                                                             | 0.004 641 948 628  | -0.029 210 673 769 | -0.014 015 449 882 |
| C                                                             | 0.013 983 232 456  | 0.008 436 586 227  | 0.001 877 050 165  |
| C                                                             | 0.013 650 325 940  | -0.004 164 632 115 | -0.008 959 733 549 |
| C                                                             | -0.070 753 992 851 | -0.074 125 969 128 | 0.072 098 680 517  |
| C                                                             | -0.022 517 641 490 | 0.207 256 810 905  | -0.075 710 302 042 |
| C                                                             | 0.007 468 499 722  | -0.128 702 799 493 | 0.050 087 154 917  |
| C                                                             | 0.019 399 723 537  | 0.007 645 662 785  | -0.036 008 824 768 |
| H                                                             | 0.011 730 816 394  | 0.000 933 612 543  | -0.001 351 556 071 |
| H                                                             | 0.031 905 768 690  | -0.002 898 236 469 | -0.002 482 484 103 |
| H                                                             | -0.001 161 962 334 | -0.005 917 653 537 | -0.000 485 250 545 |
| H                                                             | 0.037 558 964 837  | -0.276 779 887 595 | 0.080 592 552 990  |
| H                                                             | 0.001 881 743 709  | 0.005 149 381 378  | 0.005 261 557 653  |
| H                                                             | -0.033 105 786 142 | -0.075 591 945 723 | 0.022 667 027 559  |
| H                                                             | -0.094 599 253 950 | 0.281 644 459 322  | -0.107 931 471 031 |
| H                                                             | -0.009 272 532 986 | 0.016 681 020 974  | -0.024 469 163 647 |
| H                                                             | -0.046 070 113 597 | 0.001 608 988 021  | 0.060 192 709 841  |
| H                                                             | -0.327 129 888 441 | 0.186 244 835 180  | -0.231 117 624 905 |
| H                                                             | 0.322 240 028 582  | -0.198 593 937 331 | -0.079 046 704 890 |
| H                                                             | 0.008 395 157 671  | 0.013 981 102 649  | -0.024 123 441 178 |
| H                                                             | 0.001 203 957 738  | -0.013 882 036 693 | -0.017 058 428 144 |
| H                                                             | 0.261 981 697 331  | 0.353 597 095 076  | 0.062 828 724 540  |
| H                                                             | -0.221 788 861 200 | -0.230 720 949 746 | 0.255 164 085 945  |
| H                                                             | 0.006 387 929 073  | 0.007 910 414 828  | 0.002 696 324 340  |

Wavenumber/cm<sup>-1</sup>: 3126.0951 , Max excitation: 1

| $l'$ -matrix coefficients/(u <sup>1/2</sup> Å <sup>-1</sup> ) |                    |                    |                    |
|---------------------------------------------------------------|--------------------|--------------------|--------------------|
| O                                                             | -0.034 361 584 288 | -0.217 601 183 621 | -0.433 044 459 315 |
| C                                                             | 0.004 504 091 430  | -0.112 022 466 540 | -0.176 020 125 410 |
| C                                                             | 0.020 640 998 920  | -0.001 719 925 237 | 0.017 620 464 427  |
| C                                                             | -0.002 021 306 432 | 0.000 153 208 468  | 0.078 996 587 844  |
| C                                                             | 0.017 926 827 581  | -0.048 171 734 346 | -0.130 630 974 424 |
| C                                                             | 0.073 032 781 851  | -0.089 721 684 543 | -0.019 788 424 496 |
| C                                                             | -0.201 931 242 119 | 0.041 148 806 233  | 0.086 660 856 930  |
| C                                                             | -0.047 216 442 369 | 0.111 518 495 595  | -0.211 128 749 465 |
| C                                                             | 0.277 116 099 219  | 0.071 081 773 024  | 0.213 498 124 741  |
| C                                                             | -0.231 909 136 278 | 0.086 273 095 509  | 0.160 560 267 112  |
| C                                                             | 0.113 003 247 594  | 0.108 525 253 733  | 0.314 370 872 535  |
| H                                                             | 0.035 911 750 259  | -0.050 965 937 229 | 0.007 830 123 678  |
| H                                                             | -0.137 680 089 334 | 0.017 658 196 989  | 0.024 978 709 786  |
| H                                                             | 0.005 034 503 349  | -0.042 276 751 582 | -0.068 869 515 668 |
| H                                                             | 0.145 043 852 904  | -0.015 811 074 872 | 0.036 439 836 924  |
| H                                                             | 0.019 824 396 908  | -0.027 278 032 270 | -0.014 039 330 639 |
| H                                                             | -0.032 675 860 487 | 0.109 051 882 881  | -0.093 600 563 325 |
| H                                                             | -0.120 043 991 478 | 0.047 831 484 278  | 0.005 829 674 221  |
| H                                                             | -0.038 989 374 682 | -0.007 898 331 906 | 0.094 309 543 397  |
| H                                                             | 0.031 129 794 366  | -0.002 666 464 084 | -0.111 093 908 094 |
| H                                                             | 0.059 369 758 751  | 0.036 798 857 823  | 0.077 266 390 688  |
| H                                                             | -0.048 219 103 050 | 0.017 490 952 211  | 0.047 143 429 116  |
| H                                                             | 0.095 183 427 679  | 0.021 287 957 993  | 0.086 510 743 250  |
| H                                                             | -0.005 319 668 165 | 0.045 567 099 217  | 0.110 406 017 568  |
| H                                                             | 0.094 682 819 284  | 0.055 132 872 874  | 0.117 971 492 890  |
| H                                                             | -0.081 147 677 535 | 0.033 258 623 277  | 0.114 866 847 465  |
| H                                                             | 0.034 895 468 684  | 0.053 054 459 345  | 0.135 892 869 374  |

(1S,4S)-(-)-camphor

*Initial state*

Wavenumber/cm<sup>-1</sup>: 111.1765

| $\frac{\partial \mu_{x,y,z}}{\partial Q_r} / (e u^{-0.5})$   |                    |                                        |                                        |
|--------------------------------------------------------------|--------------------|----------------------------------------|----------------------------------------|
|                                                              | -0.008 832 836 797 | 0.006 886 747 808                      | 0.008 022 239 747                      |
| $l$ -matrix coefficients/(u <sup>1/2</sup> Å <sup>-1</sup> ) |                    |                                        |                                        |
| O                                                            | -0.000 254 882 085 | $-7.808\,852\,800\,000 \times 10^{-5}$ | $-1.145\,480\,500\,000 \times 10^{-5}$ |
| C                                                            | 0.000 613 432 489  | -0.000 485 148 168                     | -0.000 563 324 899                     |
| C                                                            | -0.002 383 120 633 | 0.003 871 923 610                      | -0.003 112 165 056                     |
| C                                                            | 0.000 227 074 461  | $7.722\,215\,100\,000 \times 10^{-5}$  | $9.995\,739\,300\,000 \times 10^{-5}$  |
| C                                                            | 0.001 413 949 760  | $-4.352\,704\,900\,000 \times 10^{-5}$ | 0.000 217 027 595                      |
| C                                                            | 0.013 098 293 951  | -0.006 420 509 148                     | -0.007 363 265 627                     |
| C                                                            | -0.001 355 557 377 | 0.003 327 919 999                      | -0.003 901 106 909                     |
| C                                                            | 0.021 030 939 002  | -0.001 796 187 700                     | -0.005 914 017 447                     |
| C                                                            | 0.001 051 011 443  | 0.005 257 134 362                      | 0.003 968 819 135                      |
| C                                                            | -0.001 815 812 557 | 0.002 748 922 340                      | -0.007 550 406 894                     |
| C                                                            | 0.001 621 383 300  | 0.168 753 512 120                      | -0.241 144 756 525                     |
| H                                                            | 0.001 424 581 005  | 0.000 124 494 591                      | -0.000 974 592 955                     |
| H                                                            | -0.018 096 108 249 | 0.005 976 406 553                      | -0.009 422 328 767                     |
| H                                                            | -0.001 699 604 327 | -0.001 720 410 867                     | 0.011 556 141 331                      |
| H                                                            | -0.032 685 962 882 | 0.018 838 650 241                      | 0.035 168 822 088                      |
| H                                                            | -0.001 645 793 174 | -0.000 666 679 967                     | -0.001 692 215 475                     |
| H                                                            | -0.003 860 625 941 | -0.011 495 177 005                     | 0.012 952 232 783                      |
| H                                                            | -0.147 411 847 990 | -0.418 842 667 773                     | 0.779 396 476 546                      |
| H                                                            | 0.005 727 584 156  | -0.010 891 898 900                     | 0.002 774 259 606                      |
| H                                                            | 0.002 290 232 444  | -0.020 467 615 499                     | -0.002 715 769 350                     |
| H                                                            | -0.004 629 213 038 | 0.002 913 488 238                      | 0.004 600 477 359                      |
| H                                                            | -0.066 517 050 839 | -0.008 887 487 182                     | 0.022 781 394 356                      |
| H                                                            | -0.011 501 774 129 | 0.019 691 936 036                      | -0.001 557 878 858                     |
| H                                                            | 0.015 044 245 288  | -0.000 349 670 843                     | 0.010 134 670 234                      |
| H                                                            | 0.016 660 488 682  | -0.241 690 862 807                     | -0.053 628 739 900                     |
| H                                                            | -0.007 000 680 625 | -0.002 499 656 135                     | -0.005 193 724 854                     |
| H                                                            | 0.139 270 109 410  | 0.065 176 021 629                      | 0.111 550 275 755                      |

Wavenumber/cm<sup>-1</sup>: 164.8305

| $\frac{\partial \mu_{x,y,z}}{\partial Q_r} / (e u^{-0.5})$        |                    |                                       |                    |
|-------------------------------------------------------------------|--------------------|---------------------------------------|--------------------|
|                                                                   | -0.000 565 575 698 | 0.004 429 274 014                     | 0.002 310 522 212  |
| <i>l</i> -matrix coefficients/(u <sup>1/2</sup> Å <sup>-1</sup> ) |                    |                                       |                    |
| O                                                                 | -0.000 318 208 308 | $3.873\,350\,800\,000 \times 10^{-5}$ | -0.000 295 889 831 |
| C                                                                 | 0.000 658 434 312  | -0.000 323 590 031                    | 0.000 617 660 125  |
| C                                                                 | -0.004 796 860 170 | 0.002 585 613 843                     | -0.000 600 482 513 |
| C                                                                 | 0.000 858 602 319  | -0.000 733 233 302                    | 0.001 814 328 725  |
| C                                                                 | -0.003 464 676 252 | -0.003 226 407 712                    | -0.001 921 935 555 |
| C                                                                 | -0.009 627 434 736 | 0.004 588 151 937                     | 0.003 382 777 749  |
| C                                                                 | 0.009 146 919 123  | -0.052 122 984 486                    | 0.094 858 546 634  |
| C                                                                 | -0.044 870 796 409 | 0.007 140 513 363                     | 0.011 002 865 073  |
| C                                                                 | -0.261 142 948 346 | 0.064 270 590 886                     | 0.055 368 017 192  |
| C                                                                 | 0.008 591 652 315  | -0.003 872 333 833                    | 0.014 147 109 481  |
| C                                                                 | -0.002 584 081 687 | 0.002 716 811 737                     | -0.005 504 393 507 |
| H                                                                 | 0.722 168 312 075  | -0.076 816 460 337                    | -0.323 349 792 403 |
| H                                                                 | 0.015 309 944 748  | -0.004 985 874 783                    | 0.008 724 887 551  |
| H                                                                 | 0.036 765 427 638  | 0.054 371 814 781                     | -0.302 941 917 615 |
| H                                                                 | 0.018 227 445 654  | -0.010 586 572 921                    | -0.021 023 501 792 |
| H                                                                 | 0.010 154 870 535  | 0.008 728 217 332                     | 0.010 548 185 514  |
| H                                                                 | 0.004 341 988 464  | 0.016 214 231 014                     | -0.017 138 989 200 |
| H                                                                 | -0.001 752 170 252 | -0.004 853 119 740                    | 0.008 687 950 569  |
| H                                                                 | -0.071 073 419 885 | 0.136 989 211 516                     | -0.030 662 989 683 |
| H                                                                 | 0.022 766 901 093  | -0.243 837 131 025                    | -0.046 565 026 274 |
| H                                                                 | 0.006 195 958 115  | -0.002 707 256 252                    | -0.004 117 645 091 |
| H                                                                 | 0.133 030 871 381  | 0.020 660 394 305                     | -0.043 724 140 398 |
| H                                                                 | 0.024 895 463 949  | -0.045 267 007 388                    | 0.002 823 383 976  |
| H                                                                 | -0.040 122 114 453 | -0.000 422 976 791                    | -0.027 381 487 369 |
| H                                                                 | 0.001 543 206 215  | -0.011 483 184 469                    | -0.003 397 077 623 |
| H                                                                 | 0.164 275 602 458  | 0.085 482 686 062                     | 0.181 614 962 493  |
| H                                                                 | 0.015 095 941 507  | 0.005 787 241 748                     | 0.011 321 373 641  |

Wavenumber/cm<sup>-1</sup>: 184.7292

| $\frac{\partial \mu_{x,y,z}}{\partial Q_r} / (e u^{-0.5})$        | 0.005 496 006 274  | -0.004 209 466 821 | -0.006 899 518 470 |
|-------------------------------------------------------------------|--------------------|--------------------|--------------------|
| <i>l</i> -matrix coefficients/(u <sup>1/2</sup> Å <sup>-1</sup> ) |                    |                    |                    |
| O                                                                 | -0.000 746 062 052 | -0.000 742 780 621 | -0.000 258 419 145 |
| C                                                                 | 0.002 773 052 569  | -0.000 714 885 024 | 0.004 006 592 612  |
| C                                                                 | -0.001 415 020 764 | -0.002 156 032 529 | -0.001 680 953 991 |
| C                                                                 | 0.001 267 963 874  | 0.000 838 152 519  | -0.000 371 120 903 |
| C                                                                 | -0.014 656 826 650 | -0.009 021 929 920 | -0.013 681 237 844 |
| C                                                                 | -0.003 070 386 144 | 0.003 155 454 960  | 0.007 809 073 969  |
| C                                                                 | 0.001 110 451 270  | -0.001 834 669 152 | -0.000 326 251 752 |
| C                                                                 | -0.068 411 593 458 | 0.011 167 916 759  | 0.016 795 459 351  |
| C                                                                 | 0.009 341 565 481  | -0.063 858 323 463 | -0.037 777 607 821 |
| C                                                                 | 0.167 364 197 504  | -0.109 437 259 111 | 0.199 904 670 159  |
| C                                                                 | -0.009 165 148 948 | -0.008 033 707 973 | -0.023 891 423 026 |
| H                                                                 | -0.070 045 621 898 | 0.003 548 006 117  | 0.027 410 609 628  |
| H                                                                 | -0.011 084 084 231 | 0.007 804 992 268  | -0.005 696 750 826 |
| H                                                                 | 0.000 101 798 964  | -0.000 311 660 093 | 0.002 095 001 744  |
| H                                                                 | 0.021 573 988 785  | -0.012 655 896 488 | -0.023 291 602 642 |
| H                                                                 | 0.046 894 752 828  | 0.034 211 956 707  | 0.045 803 529 197  |
| H                                                                 | 0.098 058 371 670  | 0.329 871 918 863  | -0.374 691 525 105 |
| H                                                                 | -0.007 817 964 586 | -0.022 979 000 418 | 0.040 773 512 053  |
| H                                                                 | -0.002 060 818 946 | 0.003 787 099 934  | -0.001 266 875 964 |
| H                                                                 | -0.031 916 736 836 | 0.193 257 295 330  | 0.036 086 063 753  |
| H                                                                 | -0.094 453 535 341 | 0.037 531 413 122  | 0.087 701 550 482  |
| H                                                                 | 0.199 758 964 508  | 0.030 234 211 763  | -0.066 023 123 945 |
| H                                                                 | 0.036 776 694 278  | -0.070 854 852 998 | 0.008 378 767 609  |
| H                                                                 | -0.587 213 954 234 | 0.011 371 490 399  | -0.406 124 563 340 |
| H                                                                 | -0.003 965 394 955 | 0.036 913 544 345  | 0.004 231 862 064  |
| H                                                                 | 0.070 671 575 266  | 0.027 119 356 388  | 0.067 176 732 102  |
| H                                                                 | 0.043 798 633 294  | 0.015 104 657 267  | 0.037 951 709 309  |

Wavenumber/cm<sup>-1</sup>: 216.1537

| $\frac{\partial \mu_{x,y,z}}{\partial Q_r} / (e u^{-0.5})$        | -0.002 036 000 243                    | 0.002 842 333 651                    | 0.003 416 575 805  |
|-------------------------------------------------------------------|---------------------------------------|--------------------------------------|--------------------|
| <i>l</i> -matrix coefficients/(u <sup>1/2</sup> Å <sup>-1</sup> ) |                                       |                                      |                    |
| O                                                                 | -8.224 838 800 000 × 10 <sup>-5</sup> | 0.000 351 238 370                    | -0.000 330 679 907 |
| C                                                                 | 0.001 767 717 325                     | -0.000 996 709 946                   | 0.000 401 421 032  |
| C                                                                 | 0.000 770 750 408                     | 5.078 754 000 000 × 10 <sup>-6</sup> | 0.000 163 909 004  |
| C                                                                 | -0.000 512 702 073                    | -0.001 977 480 594                   | 0.001 956 283 831  |
| C                                                                 | 0.037 519 265 992                     | 0.022 684 751 810                    | 0.035 694 834 388  |
| C                                                                 | 0.125 979 995 998                     | -0.057 609 722 762                   | -0.016 584 225 442 |
| C                                                                 | 0.038 557 037 546                     | -0.129 587 730 706                   | 0.161 383 458 740  |
| C                                                                 | 0.131 307 220 500                     | -0.073 500 920 310                   | -0.020 118 093 273 |
| C                                                                 | 0.048 067 232 494                     | -0.021 309 621 842                   | -0.011 615 540 728 |
| C                                                                 | 0.031 081 696 878                     | -0.012 054 926 732                   | 0.013 081 010 907  |
| C                                                                 | 0.002 591 822 095                     | -0.018 001 522 156                   | 0.004 975 656 584  |
| H                                                                 | -0.126 948 753 790                    | 0.012 653 668 988                    | 0.056 450 624 616  |
| H                                                                 | -0.261 837 366 411                    | 0.091 229 454 415                    | -0.147 481 478 761 |
| H                                                                 | 0.061 405 589 033                     | 0.078 223 766 859                    | -0.473 834 221 729 |
| H                                                                 | -0.174 199 650 846                    | 0.109 250 922 256                    | 0.203 351 998 146  |
| H                                                                 | -0.122 040 057 914                    | -0.086 924 114 083                   | -0.119 420 539 264 |
| H                                                                 | 0.007 569 174 007                     | 0.021 265 317 610                    | -0.023 919 983 205 |
| H                                                                 | 0.002 842 750 904                     | 0.009 750 481 070                    | -0.019 070 412 522 |
| H                                                                 | -0.200 010 696 766                    | 0.378 258 681 640                    | -0.087 410 710 215 |
| H                                                                 | -0.008 938 763 468                    | 0.078 889 650 249                    | 0.014 423 906 945  |
| H                                                                 | -0.042 243 178 049                    | 0.019 223 268 814                    | 0.032 347 796 471  |
| H                                                                 | -0.284 586 641 753                    | -0.047 959 778 848                   | 0.097 189 196 300  |
| H                                                                 | -0.171 048 473 449                    | 0.305 150 026 898                    | -0.032 455 524 440 |
| H                                                                 | -0.074 713 747 984                    | 0.001 572 691 866                    | -0.053 339 182 586 |
| H                                                                 | -0.005 229 320 326                    | 0.058 604 231 175                    | 0.010 185 161 836  |
| H                                                                 | -0.029 937 177 939                    | -0.016 573 966 822                   | -0.032 893 938 805 |
| H                                                                 | -0.009 681 280 297                    | -0.004 830 923 642                   | -0.007 359 392 923 |



Wavenumber/cm<sup>-1</sup>: 224.5398

| $\frac{\partial \mu_{x,y,z}}{\partial Q_r} / (e u^{-0.5})$        | 0.001 507 721 683  | -0.003 087 657 018 | -0.005 708 279 851 |
|-------------------------------------------------------------------|--------------------|--------------------|--------------------|
| <i>l</i> -matrix coefficients/(u <sup>1/2</sup> Å <sup>-1</sup> ) |                    |                    |                    |
| O                                                                 | 0.001 164 180 959  | 0.000 854 711 483  | 0.000 106 162 082  |
| C                                                                 | -0.004 476 953 730 | -0.000 328 543 162 | 0.002 948 727 933  |
| C                                                                 | 0.000 697 172 503  | -0.000 466 397 613 | 0.000 441 080 801  |
| C                                                                 | -0.000 739 703 379 | -0.002 092 480 499 | -0.000 726 033 812 |
| C                                                                 | 0.007 296 978 475  | 0.004 978 231 643  | 0.007 688 943 818  |
| C                                                                 | -0.068 552 213 900 | 0.031 127 685 283  | 0.002 933 842 053  |
| C                                                                 | 0.014 414 336 781  | -0.046 657 112 914 | 0.056 484 541 086  |
| C                                                                 | -0.012 021 302 947 | 0.019 757 331 254  | -0.001 511 993 243 |
| C                                                                 | 0.022 118 235 214  | -0.039 473 773 298 | -0.021 753 025 873 |
| C                                                                 | -0.230 393 310 897 | -0.030 713 420 438 | 0.154 771 133 531  |
| C                                                                 | -0.005 306 839 248 | 0.011 544 736 770  | -0.006 692 816 203 |
| H                                                                 | -0.078 555 003 673 | 0.005 786 376 590  | 0.033 746 144 901  |
| H                                                                 | 0.153 282 672 748  | -0.055 342 420 459 | 0.085 577 472 830  |
| H                                                                 | 0.021 141 686 036  | 0.027 036 978 968  | -0.164 822 635 149 |
| H                                                                 | 0.085 707 896 031  | -0.051 153 235 776 | -0.100 873 368 633 |
| H                                                                 | -0.024 535 535 763 | -0.017 403 806 899 | -0.024 252 207 293 |
| H                                                                 | 0.071 415 112 939  | 0.333 587 293 023  | -0.375 947 823 245 |
| H                                                                 | -0.001 934 358 042 | -0.005 892 173 524 | 0.012 401 791 471  |
| H                                                                 | -0.071 380 521 887 | 0.136 462 812 854  | -0.031 704 250 387 |
| H                                                                 | -0.019 070 839 294 | 0.124 155 430 190  | 0.024 522 941 735  |
| H                                                                 | 0.495 190 755 032  | -0.217 629 288 017 | -0.351 830 330 276 |
| H                                                                 | 0.003 240 945 185  | 0.002 105 825 456  | -0.002 394 599 046 |
| H                                                                 | 0.039 189 245 071  | -0.068 361 029 044 | 0.006 336 795 960  |
| H                                                                 | 0.235 350 323 284  | -0.009 080 494 384 | 0.189 112 630 106  |
| H                                                                 | 0.002 470 542 951  | -0.041 283 520 586 | -0.006 465 459 017 |
| H                                                                 | 0.021 741 807 629  | 0.006 596 042 712  | 0.017 904 534 801  |
| H                                                                 | 0.018 180 380 592  | 0.007 630 576 297  | 0.016 563 603 419  |

Wavenumber/cm<sup>-1</sup>: 241.2607

| $\frac{\partial \mu_{x,y,z}}{\partial Q_r} / (e u^{-0.5})$   |                                      |                    |                    |
|--------------------------------------------------------------|--------------------------------------|--------------------|--------------------|
|                                                              | -0.005 832 893 554                   | 0.000 851 715 201  | 0.005 104 438 187  |
| $l$ -matrix coefficients/(u <sup>1/2</sup> Å <sup>-1</sup> ) |                                      |                    |                    |
| O                                                            | -0.000 145 811 101                   | -0.000 309 056 501 | 0.000 158 400 851  |
| C                                                            | 9.952 204 000 000 × 10 <sup>-6</sup> | 0.000 537 936 256  | -0.001 067 847 015 |
| C                                                            | 5.279 972 700 000 × 10 <sup>-5</sup> | -0.001 841 801 752 | 0.000 761 652 010  |
| C                                                            | 0.000 956 851 269                    | 0.000 476 269 443  | 0.000 742 417 501  |
| C                                                            | -0.013 827 293 643                   | -0.008 971 869 565 | -0.011 673 111 574 |
| C                                                            | -0.130 263 784 960                   | 0.058 420 005 035  | 0.014 700 689 474  |
| C                                                            | 0.032 110 802 040                    | -0.105 141 811 372 | 0.130 705 085 544  |
| C                                                            | -0.120 387 997 928                   | 0.056 506 331 245  | 0.019 506 571 206  |
| C                                                            | 0.067 536 119 840                    | -0.060 853 913 687 | -0.043 098 725 810 |
| C                                                            | 0.052 337 557 318                    | 0.037 939 411 329  | -0.107 880 527 192 |
| C                                                            | -0.012 219 905 254                   | -0.007 878 073 726 | -0.028 551 582 492 |
| H                                                            | -0.227 506 292 366                   | 0.021 769 849 333  | 0.099 850 212 857  |
| H                                                            | 0.274 351 812 017                    | -0.095 592 877 548 | 0.153 753 893 175  |
| H                                                            | 0.049 276 648 989                    | 0.062 641 452 757  | -0.385 104 666 942 |
| H                                                            | 0.174 470 821 073                    | -0.110 025 989 068 | -0.203 701 586 805 |
| H                                                            | 0.043 396 224 187                    | 0.032 147 248 005  | 0.042 981 869 486  |
| H                                                            | -0.050 718 330 307                   | -0.209 000 454 219 | 0.236 088 464 400  |
| H                                                            | -0.008 555 181 113                   | -0.027 658 831 244 | 0.047 449 338 047  |
| H                                                            | -0.158 859 480 809                   | 0.302 819 311 283  | -0.071 209 496 221 |
| H                                                            | -0.025 749 529 275                   | 0.187 883 671 261  | 0.034 804 109 510  |
| H                                                            | -0.173 233 927 167                   | 0.075 794 252 911  | 0.117 952 829 172  |
| H                                                            | 0.280 308 100 569                    | 0.047 848 344 374  | -0.094 312 333 112 |
| H                                                            | 0.135 348 316 077                    | -0.241 856 724 328 | 0.025 210 079 605  |
| H                                                            | 0.042 745 724 323                    | 0.002 147 012 779  | 0.019 330 236 394  |
| H                                                            | -0.003 288 379 326                   | 0.036 213 922 172  | 0.003 690 244 278  |
| H                                                            | 0.020 361 052 230                    | 0.001 761 676 822  | 0.013 769 835 999  |
| H                                                            | 0.055 225 880 277                    | 0.020 686 426 512  | 0.048 068 182 907  |

Wavenumber/cm<sup>-1</sup>: 261.3462

| $\frac{\partial \mu_{x,y,z}}{\partial Q_r} / (e u^{-0.5})$        |                    |                                       |                                       |
|-------------------------------------------------------------------|--------------------|---------------------------------------|---------------------------------------|
|                                                                   | -0.001 936 817 579 | -0.006 153 839 435                    | -0.002 375 504 871                    |
| <i>l</i> -matrix coefficients/(u <sup>1/2</sup> Å <sup>-1</sup> ) |                    |                                       |                                       |
| O                                                                 | -0.001 024 564 716 | -2.194 372 500 000 × 10 <sup>-5</sup> | 0.000 397 525 900                     |
| C                                                                 | 0.001 544 651 486  | 0.000 743 694 289                     | 5.888 214 400 000 × 10 <sup>-5</sup>  |
| C                                                                 | -0.003 217 206 970 | -0.003 025 587 544                    | -0.003 562 868 413                    |
| C                                                                 | 0.002 091 662 131  | -0.000 251 026 399                    | -6.107 358 000 000 × 10 <sup>-5</sup> |
| C                                                                 | -0.069 853 376 886 | -0.048 184 469 570                    | -0.067 728 285 499                    |
| C                                                                 | 0.114 281 910 382  | -0.051 387 096 690                    | -0.009 477 638 776                    |
| C                                                                 | 0.000 667 468 137  | 0.010 460 353 933                     | -0.024 497 268 436                    |
| C                                                                 | -0.045 634 527 026 | -0.023 076 889 466                    | 0.019 622 520 041                     |
| C                                                                 | -0.062 861 902 766 | -0.148 124 622 262                    | -0.090 802 100 336                    |
| C                                                                 | -0.061 550 947 576 | 0.026 944 166 500                     | -0.041 646 918 237                    |
| C                                                                 | -0.045 734 218 281 | -0.103 508 827 379                    | -0.069 949 380 942                    |
| H                                                                 | 0.028 856 073 016  | -0.012 975 093 045                    | -0.019 988 497 993                    |
| H                                                                 | -0.244 126 722 745 | 0.084 752 569 869                     | -0.136 727 330 465                    |
| H                                                                 | -0.012 721 633 920 | -0.012 232 544 149                    | 0.080 560 839 930                     |
| H                                                                 | -0.148 975 900 160 | 0.093 889 478 374                     | 0.172 845 948 581                     |
| H                                                                 | 0.233 642 062 621  | 0.170 992 147 359                     | 0.230 196 655 622                     |
| H                                                                 | -0.021 692 747 535 | -0.063 130 897 711                    | 0.073 034 889 570                     |
| H                                                                 | -0.008 418 034 285 | -0.021 233 394 986                    | 0.023 980 266 073                     |
| H                                                                 | 0.011 686 689 441  | -0.022 789 608 117                    | 0.004 666 594 475                     |
| H                                                                 | -0.074 415 457 056 | 0.417 317 495 413                     | 0.078 296 049 669                     |
| H                                                                 | 0.061 638 549 123  | -0.024 888 206 183                    | -0.049 862 364 043                    |
| H                                                                 | 0.188 540 549 110  | 0.026 485 949 763                     | -0.063 143 521 162                    |
| H                                                                 | -0.030 991 795 141 | 0.047 365 793 116                     | -0.003 029 077 360                    |
| H                                                                 | 0.172 496 519 315  | -0.003 329 289 810                    | 0.121 587 539 268                     |
| H                                                                 | -0.026 802 267 507 | 0.315 448 679 808                     | 0.043 530 638 006                     |
| H                                                                 | 0.265 336 841 088  | 0.108 511 185 525                     | 0.260 473 677 538                     |
| H                                                                 | 0.197 786 030 857  | 0.067 541 340 400                     | 0.176 317 006 739                     |

Wavenumber/cm<sup>-1</sup>: 289.7442

| $\frac{\partial \mu_{x,y,z}}{\partial Q_r} / (e u^{-0.5})$        | 0.005 981 806 743  | -0.010 098 018 779 | -0.013 961 995 355 |
|-------------------------------------------------------------------|--------------------|--------------------|--------------------|
| <i>l</i> -matrix coefficients/(u <sup>1/2</sup> Å <sup>-1</sup> ) |                    |                    |                    |
| O                                                                 | -0.001 965 019 328 | -0.000 560 519 841 | -0.000 119 440 574 |
| C                                                                 | 0.001 108 898 719  | 0.001 123 361 202  | 0.000 678 218 090  |
| C                                                                 | -0.000 176 532 830 | 0.004 790 229 896  | 0.000 674 443 744  |
| C                                                                 | 0.003 853 630 325  | 0.001 867 321 846  | 0.000 990 964 870  |
| C                                                                 | -0.102 613 716 915 | -0.074 080 861 582 | -0.099 071 674 195 |
| C                                                                 | 0.098 164 715 684  | -0.041 987 091 127 | -0.001 202 938 024 |
| C                                                                 | 0.029 726 865 657  | -0.055 221 287 306 | 0.019 281 354 930  |
| C                                                                 | -0.104 816 218 532 | -0.000 725 068 809 | 0.031 455 962 333  |
| C                                                                 | 0.079 985 174 541  | 0.130 430 915 279  | 0.068 545 591 979  |
| C                                                                 | -0.028 114 069 032 | -0.000 665 189 214 | 0.022 361 768 672  |
| C                                                                 | 0.014 303 102 539  | 0.053 419 505 328  | 0.030 922 693 242  |
| H                                                                 | -0.116 031 164 248 | 0.022 219 366 368  | 0.058 380 991 902  |
| H                                                                 | -0.223 797 301 412 | 0.078 448 970 044  | -0.123 859 222 414 |
| H                                                                 | 0.002 772 072 525  | -0.001 043 978 023 | -0.022 384 221 073 |
| H                                                                 | -0.112 783 406 322 | 0.069 048 962 570  | 0.130 916 063 119  |
| H                                                                 | 0.341 763 498 386  | 0.246 357 272 444  | 0.336 014 906 277  |
| H                                                                 | 0.006 416 602 061  | 0.034 405 537 699  | -0.039 174 120 460 |
| H                                                                 | 0.004 490 510 395  | 0.013 285 802 045  | -0.018 034 833 277 |
| H                                                                 | -0.098 873 784 312 | 0.186 786 321 545  | -0.047 637 909 964 |
| H                                                                 | 0.069 494 252 245  | -0.377 720 418 439 | -0.069 969 952 036 |
| H                                                                 | 0.073 679 746 439  | -0.031 703 296 826 | -0.052 968 185 660 |
| H                                                                 | 0.333 660 068 263  | 0.050 257 870 308  | -0.113 246 269 975 |
| H                                                                 | 0.026 341 340 411  | -0.055 175 573 172 | 0.006 441 626 885  |
| H                                                                 | 0.017 142 817 540  | -0.001 767 856 389 | 0.014 860 027 254  |
| H                                                                 | 0.016 114 452 067  | -0.174 194 428 949 | -0.025 282 585 689 |
| H                                                                 | -0.231 239 498 813 | -0.097 333 041 483 | -0.227 295 688 351 |
| H                                                                 | -0.071 709 794 340 | -0.025 059 744 367 | -0.063 928 207 493 |

Wavenumber/cm<sup>-1</sup>: 300.9781

| $\frac{\partial \mu_{x,y,z}}{\partial Q_r} / (e u^{-0.5})$        | 0.004 106 581 466  | -0.004 632 233 996                     | -0.011 876 185 083                     |
|-------------------------------------------------------------------|--------------------|----------------------------------------|----------------------------------------|
| <i>l</i> -matrix coefficients/(u <sup>1/2</sup> Å <sup>-1</sup> ) |                    |                                        |                                        |
| O                                                                 | 0.000 576 827 236  | $8.793\,385\,200\,000 \times 10^{-5}$  | $-4.155\,821\,300\,000 \times 10^{-5}$ |
| C                                                                 | 0.000 332 359 027  | 0.000 457 390 784                      | 0.000 635 614 025                      |
| C                                                                 | -0.001 645 327 699 | -0.001 337 353 140                     | -0.001 107 243 985                     |
| C                                                                 | -0.000 126 128 103 | $1.520\,857\,100\,000 \times 10^{-5}$  | -0.000 385 760 891                     |
| C                                                                 | -0.016 968 488 075 | -0.012 800 419 057                     | -0.016 792 538 919                     |
| C                                                                 | -0.064 853 249 732 | 0.028 415 355 555                      | 0.003 109 153 006                      |
| C                                                                 | 0.005 227 129 122  | -0.007 359 848 978                     | -0.003 506 157 230                     |
| C                                                                 | 0.052 222 253 178  | -0.026 042 011 844                     | -0.008 121 229 450                     |
| C                                                                 | 0.037 809 334 973  | 0.113 696 360 221                      | 0.068 749 104 475                      |
| C                                                                 | 0.006 613 823 316  | -0.015 014 385 916                     | 0.020 693 695 189                      |
| C                                                                 | -0.085 984 064 020 | -0.197 940 267 889                     | -0.128 977 886 481                     |
| H                                                                 | 0.000 297 197 323  | 0.009 559 498 483                      | 0.006 488 456 049                      |
| H                                                                 | 0.146 342 946 996  | -0.051 249 526 510                     | 0.081 275 703 172                      |
| H                                                                 | -0.001 741 079 149 | -0.004 965 153 456                     | 0.020 301 586 398                      |
| H                                                                 | 0.076 847 812 143  | -0.046 581 563 036                     | -0.090 726 541 276                     |
| H                                                                 | 0.058 714 734 478  | 0.043 368 246 415                      | 0.058 560 307 420                      |
| H                                                                 | 0.013 088 164 655  | 0.050 646 682 604                      | -0.057 899 829 392                     |
| H                                                                 | -0.013 990 969 196 | -0.038 655 538 429                     | 0.035 741 907 871                      |
| H                                                                 | -0.016 058 608 485 | 0.030 035 017 750                      | -0.008 327 046 349                     |
| H                                                                 | 0.057 345 132 958  | -0.322 858 728 865                     | -0.061 730 362 357                     |
| H                                                                 | -0.004 948 225 384 | 0.001 409 083 715                      | 0.006 736 043 963                      |
| H                                                                 | -0.119 952 452 333 | -0.018 404 259 221                     | 0.039 681 933 525                      |
| H                                                                 | -0.061 989 380 437 | 0.109 851 675 323                      | -0.012 384 505 409                     |
| H                                                                 | -0.030 985 906 745 | $-1.016\,399\,000\,000 \times 10^{-6}$ | -0.019 830 746 464                     |
| H                                                                 | -0.049 867 441 380 | 0.594 894 186 691                      | 0.081 750 785 120                      |
| H                                                                 | -0.188 525 423 692 | -0.077 477 628 434                     | -0.181 899 617 180                     |
| H                                                                 | 0.365 693 523 308  | 0.127 101 759 294                      | 0.329 233 917 531                      |

Wavenumber/cm<sup>-1</sup>: 385.032

| $\frac{\partial \mu_{x,y,z}}{\partial Q_r} / (e u^{-0.5})$        |                                       |                                      |                                      |
|-------------------------------------------------------------------|---------------------------------------|--------------------------------------|--------------------------------------|
|                                                                   | -0.001 143 088 568                    | 0.011 713 763 370                    | 0.010 533 099 713                    |
| <i>l</i> -matrix coefficients/(u <sup>1/2</sup> Å <sup>-1</sup> ) |                                       |                                      |                                      |
| O                                                                 | -5.165 465 200 000 × 10 <sup>-5</sup> | 6.532 782 000 000 × 10 <sup>-6</sup> | 6.913 395 200 000 × 10 <sup>-5</sup> |
| C                                                                 | -0.000 116 462 648                    | 0.001 603 078 724                    | 0.001 867 303 906                    |
| C                                                                 | -0.001 710 651 215                    | 0.003 195 800 038                    | -0.001 136 035 919                   |
| C                                                                 | 0.002 121 518 528                     | 0.000 421 935 442                    | -0.000 399 453 359                   |
| C                                                                 | -0.100 686 648 883                    | -0.075 999 216 422                   | -0.100 086 104 017                   |
| C                                                                 | -0.115 922 363 483                    | 0.057 536 621 305                    | 0.034 951 907 580                    |
| C                                                                 | 0.022 602 339 385                     | -0.029 872 543 561                   | -0.018 238 564 452                   |
| C                                                                 | 0.151 599 278 757                     | -0.109 787 305 384                   | -0.013 877 800 243                   |
| C                                                                 | -0.033 169 936 170                    | -0.036 317 722 305                   | -0.024 310 041 510                   |
| C                                                                 | 0.024 202 782 761                     | -0.002 310 647 453                   | 0.000 274 479 403                    |
| C                                                                 | 0.018 774 188 895                     | 0.056 109 602 894                    | 0.037 529 828 357                    |
| H                                                                 | 0.044 676 972 067                     | -0.007 973 731 797                   | -0.022 840 810 735                   |
| H                                                                 | 0.203 323 855 207                     | -0.071 610 091 827                   | 0.115 294 824 297                    |
| H                                                                 | -0.012 293 812 798                    | -0.016 850 238 712                   | 0.091 235 984 529                    |
| H                                                                 | 0.200 271 757 121                     | -0.123 961 977 470                   | -0.228 540 145 194                   |
| H                                                                 | 0.344 448 601 183                     | 0.250 433 867 708                    | 0.338 756 467 663                    |
| H                                                                 | 0.000 515 462 371                     | -0.008 485 258 054                   | 0.008 737 905 052                    |
| H                                                                 | 0.006 349 025 829                     | 0.019 986 028 543                    | -0.025 746 417 721                   |
| H                                                                 | -0.065 589 042 301                    | 0.120 253 309 067                    | -0.031 886 837 709                   |
| H                                                                 | -0.018 469 240 751                    | 0.093 868 788 731                    | 0.018 715 929 008                    |
| H                                                                 | -0.034 591 758 575                    | 0.013 780 566 722                    | 0.026 297 851 906                    |
| H                                                                 | -0.283 839 732 986                    | -0.048 123 250 836                   | 0.095 596 840 631                    |
| H                                                                 | -0.241 567 228 505                    | 0.423 671 680 925                    | -0.045 890 619 682                   |
| H                                                                 | -0.049 125 591 920                    | 0.001 165 903 043                    | -0.035 905 368 144                   |
| H                                                                 | 0.015 036 022 563                     | -0.185 111 686 970                   | -0.025 012 277 597                   |
| H                                                                 | 0.089 563 602 051                     | 0.037 151 979 765                    | 0.089 028 010 729                    |
| H                                                                 | -0.086 983 530 141                    | -0.030 753 176 757                   | -0.080 136 988 180                   |

Wavenumber/cm<sup>-1</sup>: 395.2943

| $\frac{\partial \mu_{x,y,z}}{\partial Q_r} / (e u^{-0.5})$        | 0.002 481 257 624  | -0.009 512 331 288                   | -0.000 418 736 724                    |
|-------------------------------------------------------------------|--------------------|--------------------------------------|---------------------------------------|
| <i>l</i> -matrix coefficients/(u <sup>1/2</sup> Å <sup>-1</sup> ) |                    |                                      |                                       |
| O                                                                 | 0.001 481 737 648  | 0.000 171 274 515                    | -0.000 203 371 342                    |
| C                                                                 | 0.001 737 094 706  | -0.002 024 133 823                   | -0.001 505 903 484                    |
| C                                                                 | 0.000 126 335 637  | -0.001 769 456 336                   | -3.663 610 300 000 × 10 <sup>-5</sup> |
| C                                                                 | -0.003 094 649 822 | 0.000 836 009 073                    | 0.001 833 785 439                     |
| C                                                                 | -0.063 103 555 179 | -0.045 778 696 603                   | -0.062 057 187 385                    |
| C                                                                 | -0.000 805 134 417 | -0.021 736 076 892                   | -0.123 052 658 107                    |
| C                                                                 | -0.057 214 232 676 | 0.064 551 649 703                    | 0.079 220 338 845                     |
| C                                                                 | 0.057 371 941 270  | 0.105 084 122 841                    | -0.043 358 487 102                    |
| C                                                                 | 0.009 360 163 466  | -0.008 289 077 140                   | 0.007 182 602 277                     |
| C                                                                 | 0.013 775 529 363  | -0.013 722 431 834                   | 0.006 121 889 640                     |
| C                                                                 | 0.019 363 662 875  | -0.005 750 722 412                   | 0.015 687 522 156                     |
| H                                                                 | 0.005 419 734 440  | -0.001 568 108 572                   | -0.002 033 102 481                    |
| H                                                                 | 0.262 430 304 522  | -0.092 902 988 756                   | 0.131 614 506 618                     |
| H                                                                 | 0.039 774 293 013  | 0.069 571 420 134                    | -0.351 314 736 441                    |
| H                                                                 | -0.265 477 149 754 | 0.162 245 662 408                    | 0.285 957 589 919                     |
| H                                                                 | 0.218 386 255 274  | 0.162 201 178 029                    | 0.214 681 913 375                     |
| H                                                                 | 0.009 679 464 956  | 0.032 858 406 725                    | -0.036 767 940 620                    |
| H                                                                 | 0.001 697 332 750  | 0.001 687 652 606                    | -0.002 987 801 748                    |
| H                                                                 | 0.151 095 725 257  | -0.289 818 908 137                   | 0.082 285 026 889                     |
| H                                                                 | -0.005 479 067 257 | 0.042 936 111 499                    | 0.008 474 187 867                     |
| H                                                                 | -0.039 595 201 687 | 0.017 725 983 407                    | 0.029 495 945 405                     |
| H                                                                 | -0.376 672 147 119 | -0.048 728 061 928                   | 0.122 880 424 692                     |
| H                                                                 | 0.185 125 440 541  | -0.303 816 024 283                   | 0.027 122 789 595                     |
| H                                                                 | -0.019 302 324 478 | 9.555 267 800 000 × 10 <sup>-5</sup> | -0.014 179 716 069                    |
| H                                                                 | -0.001 606 039 439 | 0.040 447 839 117                    | 0.008 068 696 614                     |
| H                                                                 | -0.030 309 252 681 | -0.014 507 000 683                   | -0.030 777 554 387                    |
| H                                                                 | -0.063 460 359 543 | -0.025 586 679 202                   | -0.057 593 908 720                    |

Wavenumber/cm<sup>-1</sup>: 416.2492

| $\frac{\partial \mu_{x,y,z}}{\partial Q_r} / (e u^{-0.5})$        | 0.005 182 822 774                      | -0.001 612 138 065                    | -0.006 089 206 438 |
|-------------------------------------------------------------------|----------------------------------------|---------------------------------------|--------------------|
| <i>l</i> -matrix coefficients/(u <sup>1/2</sup> Å <sup>-1</sup> ) |                                        |                                       |                    |
| O                                                                 | 0.000 883 888 640                      | $4.017\,866\,500\,000 \times 10^{-5}$ | -0.000 124 337 859 |
| C                                                                 | 0.000 429 118 412                      | -0.001 511 164 639                    | 0.000 112 307 825  |
| C                                                                 | -0.000 632 172 347                     | 0.000 407 469 860                     | 0.000 758 531 792  |
| C                                                                 | $-2.473\,858\,000\,000 \times 10^{-5}$ | 0.000 762 876 289                     | 0.001 137 782 281  |
| C                                                                 | 0.002 014 958 562                      | 0.003 102 911 064                     | 0.006 257 945 590  |
| C                                                                 | 0.001 152 590 870                      | -0.016 284 034 425                    | -0.086 102 127 514 |
| C                                                                 | 0.097 531 079 856                      | -0.126 659 936 252                    | -0.104 331 916 142 |
| C                                                                 | 0.016 257 706 839                      | 0.088 866 919 845                     | -0.026 017 817 125 |
| C                                                                 | -0.032 861 022 055                     | -0.008 213 738 145                    | -0.002 145 049 537 |
| C                                                                 | 0.012 651 286 691                      | -0.001 367 391 927                    | 0.002 702 071 263  |
| C                                                                 | 0.010 634 367 758                      | -0.010 214 233 566                    | 0.004 502 251 342  |
| H                                                                 | 0.079 141 399 317                      | -0.008 428 998 251                    | -0.036 636 256 981 |
| H                                                                 | 0.177 956 462 326                      | -0.062 832 717 713                    | 0.088 644 326 985  |
| H                                                                 | -0.054 730 526 503                     | -0.101 697 307 475                    | 0.500 959 854 875  |
| H                                                                 | -0.188 051 210 519                     | 0.114 728 039 217                     | 0.202 341 441 555  |
| H                                                                 | -0.012 363 350 264                     | -0.011 018 677 281                    | -0.016 987 275 866 |
| H                                                                 | 0.000 572 817 834                      | -0.000 897 267 428                    | 0.002 481 708 455  |
| H                                                                 | -0.000 226 742 647                     | -0.003 487 917 564                    | 0.005 471 947 603  |
| H                                                                 | -0.275 444 422 709                     | 0.529 436 556 363                     | -0.148 384 913 956 |
| H                                                                 | -0.006 957 490 314                     | 0.023 106 194 018                     | 0.004 597 167 528  |
| H                                                                 | -0.014 355 446 065                     | 0.006 929 641 741                     | 0.008 855 099 581  |
| H                                                                 | -0.215 522 369 427                     | -0.025 110 691 879                    | 0.068 705 030 998  |
| H                                                                 | 0.162 249 346 798                      | -0.269 708 015 353                    | 0.023 498 599 780  |
| H                                                                 | -0.030 788 454 501                     | 0.000 820 410 317                     | -0.022 570 178 341 |
| H                                                                 | -0.002 529 360 511                     | 0.048 800 160 976                     | 0.008 253 551 925  |
| H                                                                 | 0.039 158 960 363                      | 0.017 255 834 406                     | 0.040 664 095 661  |
| H                                                                 | -0.031 521 905 122                     | -0.012 583 785 084                    | -0.028 211 511 343 |



Wavenumber/cm<sup>-1</sup>: 475.833

| $\frac{\partial \mu_{x,y,z}}{\partial Q_r} / (e u^{-0.5})$   | 0.015 553 462 030  | -0.020 630 571 545                     | -0.008 686 391 856                     |
|--------------------------------------------------------------|--------------------|----------------------------------------|----------------------------------------|
| $l$ -matrix coefficients/(u <sup>1/2</sup> Å <sup>-1</sup> ) |                    |                                        |                                        |
| O                                                            | -0.001 052 503 476 | $-6.994\,295\,400\,000 \times 10^{-5}$ | $-5.077\,065\,500\,000 \times 10^{-5}$ |
| C                                                            | -0.000 271 721 798 | 0.000 312 441 893                      | 0.002 857 968 672                      |
| C                                                            | -0.002 150 935 265 | -0.001 118 875 690                     | -0.002 235 792 014                     |
| C                                                            | 0.002 108 247 721  | -0.000 945 897 379                     | -0.000 632 634 212                     |
| C                                                            | -0.024 572 598 717 | -0.017 609 344 824                     | -0.024 177 910 590                     |
| C                                                            | 0.045 903 656 531  | 0.006 296 010 284                      | 0.163 849 990 563                      |
| C                                                            | 0.003 673 521 894  | -0.011 662 968 133                     | 0.008 610 126 088                      |
| C                                                            | 0.047 565 209 208  | 0.131 966 885 618                      | -0.050 692 083 842                     |
| C                                                            | -0.006 013 513 307 | -0.002 184 667 129                     | -0.003 126 545 809                     |
| C                                                            | 0.005 616 422 081  | 0.007 529 047 463                      | 0.004 961 707 922                      |
| C                                                            | -0.017 336 500 900 | -0.006 602 552 351                     | -0.007 707 989 643                     |
| H                                                            | 0.007 938 619 383  | -0.001 035 040 080                     | -0.003 891 251 375                     |
| H                                                            | -0.455 883 621 966 | 0.163 690 469 075                      | -0.235 386 910 631                     |
| H                                                            | 0.003 458 757 534  | 0.002 808 194 280                      | -0.020 888 802 079                     |
| H                                                            | 0.302 341 919 024  | -0.183 308 928 365                     | -0.319 328 352 015                     |
| H                                                            | 0.082 938 677 282  | 0.062 443 324 991                      | 0.079 815 283 723                      |
| H                                                            | -0.004 289 862 214 | -0.019 148 308 438                     | 0.020 926 200 893                      |
| H                                                            | 0.002 989 857 781  | 0.011 651 469 866                      | -0.023 730 223 266                     |
| H                                                            | -0.017 717 679 860 | 0.035 670 501 824                      | -0.008 969 753 075                     |
| H                                                            | -0.000 723 953 121 | 0.002 737 974 847                      | 0.000 390 582 736                      |
| H                                                            | 0.020 770 141 942  | -0.009 877 242 798                     | -0.013 674 753 102                     |
| H                                                            | -0.402 845 462 737 | -0.049 494 857 400                     | 0.130 786 762 180                      |
| H                                                            | 0.240 918 863 577  | -0.397 029 476 719                     | 0.037 568 333 177                      |
| H                                                            | -0.036 194 824 601 | 0.000 772 597 308                      | -0.024 819 503 504                     |
| H                                                            | 0.000 241 892 564  | -0.012 798 825 780                     | -0.001 392 185 813                     |
| H                                                            | 0.014 826 963 735  | 0.006 021 773 949                      | 0.015 393 348 227                      |
| H                                                            | 0.057 214 753 967  | 0.021 333 729 694                      | 0.050 833 169 358                      |

Wavenumber/cm<sup>-1</sup>: 525.7475

| $\frac{\partial \mu_{x,y,z}}{\partial Q_r} / (e u^{-0.5})$        | 0.006 446 270 727  | -0.005 341 204 350                   | -0.001 520 163 395 |
|-------------------------------------------------------------------|--------------------|--------------------------------------|--------------------|
| <i>l</i> -matrix coefficients/(u <sup>1/2</sup> Å <sup>-1</sup> ) |                    |                                      |                    |
| O                                                                 | 0.002 010 216 020  | 0.000 736 384 544                    | -0.000 285 150 982 |
| C                                                                 | -0.000 938 685 553 | 8.119 457 100 000 × 10 <sup>-5</sup> | -0.002 184 033 153 |
| C                                                                 | 0.002 497 770 691  | -0.000 505 006 925                   | 0.001 645 689 213  |
| C                                                                 | -0.003 490 643 477 | 0.000 555 116 935                    | 0.001 115 430 170  |
| C                                                                 | -0.006 759 330 029 | -0.002 280 558 900                   | -0.006 118 883 587 |
| C                                                                 | 0.000 435 785 506  | 0.006 654 471 610                    | 0.032 934 696 175  |
| C                                                                 | 0.005 240 600 115  | -0.005 844 760 902                   | -0.006 477 559 966 |
| C                                                                 | -0.014 347 225 296 | -0.003 921 265 046                   | 0.004 731 777 050  |
| C                                                                 | 0.024 043 975 773  | -0.042 945 165 461                   | 0.084 894 151 631  |
| C                                                                 | -0.007 863 404 475 | -0.095 080 877 788                   | -0.045 712 745 293 |
| C                                                                 | 0.093 187 183 514  | -0.026 487 706 224                   | 0.014 872 567 807  |
| H                                                                 | 0.223 169 585 106  | -0.025 668 609 139                   | -0.094 146 731 486 |
| H                                                                 | -0.071 168 274 993 | 0.023 443 219 249                    | -0.034 325 274 055 |
| H                                                                 | -0.003 446 763 003 | -0.006 127 316 819                   | 0.028 185 677 547  |
| H                                                                 | 0.070 593 426 825  | -0.044 271 425 695                   | -0.076 182 712 788 |
| H                                                                 | 0.020 103 361 513  | 0.011 774 345 925                    | 0.019 828 263 097  |
| H                                                                 | 0.056 185 495 900  | 0.212 102 490 246                    | -0.251 772 805 707 |
| H                                                                 | -0.025 218 020 431 | -0.084 106 830 795                   | 0.155 949 037 382  |
| H                                                                 | -0.013 276 299 989 | 0.026 762 109 036                    | -0.008 503 272 018 |
| H                                                                 | -0.045 538 333 200 | 0.289 504 656 017                    | 0.061 427 690 718  |
| H                                                                 | -0.305 110 345 948 | 0.125 224 225 415                    | 0.215 644 811 879  |
| H                                                                 | 0.050 145 287 277  | 0.008 357 911 714                    | -0.016 473 566 484 |
| H                                                                 | -0.002 887 041 509 | 0.002 606 608 966                    | 0.000 149 095 800  |
| H                                                                 | 0.274 716 463 079  | -0.013 087 454 102                   | 0.191 459 523 180  |
| H                                                                 | -0.015 831 290 446 | 0.282 545 672 604                    | 0.044 918 902 037  |
| H                                                                 | -0.260 844 672 736 | -0.118 412 381 923                   | -0.256 295 218 493 |
| H                                                                 | -0.277 204 564 864 | -0.107 522 357 876                   | -0.253 854 065 274 |

Wavenumber/cm<sup>-1</sup>: 560.5317

| $\frac{\partial \mu_{x,y,z}}{\partial Q_r} / (e u^{-0.5})$        | 0.008 556 537 235                     | -0.006 310 816 219                   | 0.000 915 778 709  |
|-------------------------------------------------------------------|---------------------------------------|--------------------------------------|--------------------|
| <i>l</i> -matrix coefficients/(u <sup>1/2</sup> Å <sup>-1</sup> ) |                                       |                                      |                    |
| O                                                                 | 0.001 024 863 773                     | 0.000 508 830 222                    | 0.000 305 073 895  |
| C                                                                 | 0.002 478 267 347                     | 0.000 465 703 816                    | 0.000 173 617 810  |
| C                                                                 | -8.911 229 800 000 × 10 <sup>-5</sup> | -0.000 155 496 320                   | 0.001 012 395 384  |
| C                                                                 | -0.003 040 863 894                    | 5.873 886 000 000 × 10 <sup>-5</sup> | 0.000 858 437 490  |
| C                                                                 | 0.003 198 162 828                     | 0.000 623 220 284                    | 0.002 762 488 680  |
| C                                                                 | 0.005 318 423 905                     | -0.002 505 355 534                   | -0.005 981 692 870 |
| C                                                                 | 0.002 073 571 758                     | -0.003 348 983 816                   | 0.001 024 528 309  |
| C                                                                 | 0.004 431 010 879                     | 0.007 498 836 707                    | -0.002 815 749 777 |
| C                                                                 | -0.030 239 679 620                    | 0.042 040 701 392                    | -0.079 398 913 630 |
| C                                                                 | 0.001 537 833 883                     | -0.119 872 286 360                   | -0.053 436 663 772 |
| C                                                                 | -0.059 909 006 652                    | 0.024 586 380 882                    | -0.004 402 866 083 |
| H                                                                 | -0.191 786 843 540                    | 0.021 929 197 514                    | 0.081 316 456 638  |
| H                                                                 | -0.001 492 050 601                    | -0.000 649 293 716                   | -0.001 834 341 290 |
| H                                                                 | -0.000 576 032 562                    | -0.000 426 884 507                   | -0.000 973 856 734 |
| H                                                                 | -0.017 194 050 020                    | 0.009 416 210 506                    | 0.019 736 531 461  |
| H                                                                 | -0.010 068 358 552                    | -0.006 185 307 248                   | -0.010 029 586 967 |
| H                                                                 | 0.070 284 351 432                     | 0.265 593 127 728                    | -0.314 103 012 150 |
| H                                                                 | 0.018 575 435 726                     | 0.059 654 339 691                    | -0.109 466 171 953 |
| H                                                                 | -0.006 236 790 892                    | 0.010 194 567 376                    | -0.002 616 454 965 |
| H                                                                 | 0.043 653 641 966                     | -0.279 000 632 824                   | -0.060 253 620 120 |
| H                                                                 | -0.391 916 664 717                    | 0.161 746 913 483                    | 0.279 127 159 798  |
| H                                                                 | -0.027 099 093 953                    | -0.003 817 117 905                   | 0.009 447 660 355  |
| H                                                                 | 0.013 341 965 542                     | -0.021 979 827 176                   | 0.001 765 330 964  |
| H                                                                 | 0.314 339 445 201                     | -0.016 787 389 356                   | 0.217 232 170 917  |
| H                                                                 | 0.012 460 732 073                     | -0.212 732 926 551                   | -0.032 969 625 411 |
| H                                                                 | 0.253 338 561 927                     | 0.116 315 307 690                    | 0.248 348 439 802  |
| H                                                                 | 0.172 572 542 198                     | 0.069 402 252 222                    | 0.158 040 575 848  |

Wavenumber/cm<sup>-1</sup>: 575.1725

| $\frac{\partial \mu_{x,y,z}}{\partial Q_r} / (e u^{-0.5})$        | 0.006 754 188 680  | -0.027 633 141 550                    | -0.017 745 813 987                    |
|-------------------------------------------------------------------|--------------------|---------------------------------------|---------------------------------------|
| <i>l</i> -matrix coefficients/(u <sup>1/2</sup> Å <sup>-1</sup> ) |                    |                                       |                                       |
| O                                                                 | -0.000 439 654 528 | -2.563 373 600 000 × 10 <sup>-5</sup> | -4.720 740 200 000 × 10 <sup>-5</sup> |
| C                                                                 | 0.000 328 031 737  | -0.000 216 762 564                    | 0.000 314 756 330                     |
| C                                                                 | 0.001 468 721 311  | 0.000 853 227 096                     | -0.002 593 707 911                    |
| C                                                                 | -0.000 119 519 152 | 0.000 534 671 920                     | 9.734 424 000 000 × 10 <sup>-6</sup>  |
| C                                                                 | 0.001 164 742 001  | 0.000 793 660 700                     | 0.002 090 221 567                     |
| C                                                                 | 0.006 806 457 598  | -0.005 577 281 517                    | -0.016 302 994 066                    |
| C                                                                 | 0.001 494 836 888  | -0.000 554 279 770                    | -0.005 348 238 344                    |
| C                                                                 | 0.003 185 966 612  | -0.001 054 104 831                    | -0.000 262 935 894                    |
| C                                                                 | 0.033 597 100 153  | -0.054 119 428 669                    | 0.094 046 611 095                     |
| C                                                                 | 0.007 666 693 999  | -0.010 546 096 045                    | -0.014 801 021 215                    |
| C                                                                 | -0.129 452 306 436 | 0.048 159 271 328                     | -0.018 612 440 469                    |
| H                                                                 | 0.242 378 051 504  | -0.029 657 184 402                    | -0.099 714 513 250                    |
| H                                                                 | 0.020 128 094 223  | -0.007 706 564 208                    | 0.009 812 152 089                     |
| H                                                                 | -0.002 339 089 099 | -0.004 063 144 102                    | 0.020 757 572 631                     |
| H                                                                 | -0.042 066 866 303 | 0.024 244 554 900                     | 0.045 544 715 429                     |
| H                                                                 | -0.004 951 940 846 | -0.003 625 164 962                    | -0.005 023 345 295                    |
| H                                                                 | 0.002 787 418 110  | 0.012 371 598 341                     | -0.014 818 906 781                    |
| H                                                                 | 0.033 171 682 085  | 0.120 706 568 023                     | -0.219 556 758 315                    |
| H                                                                 | -0.004 131 222 970 | 0.007 759 443 232                     | -0.002 662 318 327                    |
| H                                                                 | -0.055 583 946 909 | 0.350 706 049 742                     | 0.075 526 342 468                     |
| H                                                                 | -0.062 056 009 798 | 0.026 412 514 077                     | 0.043 620 955 852                     |
| H                                                                 | -0.007 658 602 372 | -0.001 984 810 611                    | 0.002 410 809 756                     |
| H                                                                 | -0.001 348 437 940 | 0.003 434 197 311                     | -0.000 632 677 518                    |
| H                                                                 | 0.032 251 711 499  | -0.001 719 009 903                    | 0.021 184 079 807                     |
| H                                                                 | 0.024 157 904 761  | -0.435 044 364 900                    | -0.067 963 492 960                    |
| H                                                                 | -0.302 044 360 303 | -0.138 592 217 840                    | -0.295 084 747 864                    |
| H                                                                 | 0.384 018 104 137  | 0.151 861 292 180                     | 0.353 748 883 369                     |

Wavenumber/cm<sup>-1</sup>: 618.8105

| $\frac{\partial \mu_{x,y,z}}{\partial Q_r} / (e u^{-0.5})$        |                                     |                    |                                     |
|-------------------------------------------------------------------|-------------------------------------|--------------------|-------------------------------------|
|                                                                   | -9.248 310 736 543 $\times 10^{-5}$ | 0.039 362 534 903  | 0.026 867 440 236                   |
| <i>l</i> -matrix coefficients/(u <sup>1/2</sup> Å <sup>-1</sup> ) |                                     |                    |                                     |
| O                                                                 | -0.572 141 585 327                  | -0.169 230 134 095 | -0.000 446 252 031                  |
| C                                                                 | -0.032 037 676 515                  | -0.006 161 702 099 | 0.000 293 380 141                   |
| C                                                                 | -0.031 836 056 465                  | 0.001 195 945 348  | -0.003 199 588 891                  |
| C                                                                 | 0.764 113 492 574                   | 0.223 299 202 719  | 0.001 576 248 849                   |
| C                                                                 | -0.020 595 700 851                  | -0.011 114 289 020 | -0.006 273 827 279                  |
| C                                                                 | -0.006 798 143 490                  | -0.014 196 304 945 | 0.014 053 837 990                   |
| C                                                                 | -0.044 030 777 168                  | -0.011 638 885 953 | 0.002 383 104 012                   |
| C                                                                 | 0.003 942 276 806                   | 0.001 602 643 622  | -0.003 236 238 556                  |
| C                                                                 | 0.002 633 221 362                   | -0.000 906 362 082 | -0.002 679 420 844                  |
| C                                                                 | 0.012 860 680 443                   | 0.009 081 185 602  | 0.001 669 036 852                   |
| C                                                                 | 0.004 287 513 393                   | -0.002 396 875 364 | -3.198 950 600 000 $\times 10^{-5}$ |
| H                                                                 | 0.002 654 991 846                   | 0.008 855 561 321  | 0.001 391 745 060                   |
| H                                                                 | 0.012 734 979 969                   | 0.004 304 349 679  | -0.011 293 518 682                  |
| H                                                                 | 0.014 957 302 434                   | 0.019 768 484 935  | 0.007 170 850 665                   |
| H                                                                 | -0.008 359 621 827                  | 0.016 733 484 607  | -0.011 209 863 574                  |
| H                                                                 | -0.010 066 990 118                  | -0.003 809 758 647 | -0.003 856 591 061                  |
| H                                                                 | 0.003 700 553 387                   | -0.004 076 893 632 | -0.009 602 278 800                  |
| H                                                                 | 0.000 861 633 544                   | 0.002 519 215 902  | 0.001 537 568 176                   |
| H                                                                 | 0.023 765 966 399                   | 0.016 482 846 832  | 0.010 958 746 766                   |
| H                                                                 | 0.004 402 708 228                   | 0.001 137 366 962  | 0.000 656 298 783                   |
| H                                                                 | -0.021 412 666 621                  | -0.025 594 424 593 | -0.013 917 409 793                  |
| H                                                                 | -0.001 786 449 542                  | 0.001 292 752 502  | 0.000 385 439 172                   |
| H                                                                 | 0.001 868 167 683                   | 0.001 939 269 469  | 0.011 327 225 218                   |
| H                                                                 | 0.009 270 975 870                   | -0.017 169 326 274 | -0.002 330 872 467                  |
| H                                                                 | -0.001 067 357 355                  | 0.000 470 512 255  | 0.001 753 751 572                   |
| H                                                                 | -0.005 996 588 084                  | -0.004 264 485 969 | 0.007 345 852 734                   |
| H                                                                 | 0.001 378 074 290                   | 0.004 025 618 444  | -0.004 261 238 553                  |

Wavenumber/cm<sup>-1</sup>: 651.4632

| $\frac{\partial \mu_{x,y,z}}{\partial Q_r} / (e u^{-0.5})$        |                    |                    |                    |
|-------------------------------------------------------------------|--------------------|--------------------|--------------------|
|                                                                   | -0.007 376 576 816 | -0.003 946 673 888 | -0.010 112 646 306 |
| <i>l</i> -matrix coefficients/(u <sup>1/2</sup> Å <sup>-1</sup> ) |                    |                    |                    |
| O                                                                 | -0.001 859 451 190 | -0.002 846 587 906 | -0.000 549 555 756 |
| C                                                                 | 0.004 935 813 042  | -0.004 874 794 971 | -0.004 920 121 377 |
| C                                                                 | -0.041 242 316 445 | -0.025 569 956 876 | -0.045 576 440 799 |
| C                                                                 | -0.003 247 348 565 | 0.009 916 814 129  | 0.009 208 251 994  |
| C                                                                 | 0.013 049 591 075  | 0.024 724 655 624  | 0.020 560 878 393  |
| C                                                                 | -0.011 246 272 874 | -0.003 144 067 771 | -0.098 704 715 796 |
| C                                                                 | -0.036 275 400 581 | 0.011 780 207 539  | 0.023 838 576 574  |
| C                                                                 | 0.079 610 568 053  | 0.173 241 580 964  | -0.084 368 828 003 |
| C                                                                 | -0.047 655 684 189 | -0.034 580 168 525 | 0.011 306 228 450  |
| C                                                                 | 0.009 107 601 651  | 0.003 933 775 067  | -0.001 661 678 487 |
| C                                                                 | 0.015 640 129 919  | -0.019 884 826 756 | -0.085 274 624 545 |
| H                                                                 | 0.017 261 405 534  | 0.204 896 405 421  | 0.009 015 770 275  |
| H                                                                 | -0.091 967 908 441 | 0.073 464 527 207  | 0.196 403 249 909  |
| H                                                                 | 0.062 722 712 842  | -0.090 093 277 184 | -0.003 164 853 215 |
| H                                                                 | 0.161 943 232 354  | -0.039 751 007 712 | 0.147 504 016 917  |
| H                                                                 | 0.012 303 696 113  | 0.017 518 249 167  | -0.006 258 120 495 |
| H                                                                 | -0.026 208 799 204 | 0.000 245 169 879  | -0.006 590 377 360 |
| H                                                                 | -0.075 762 961 356 | 0.259 289 350 509  | 0.109 912 628 233  |
| H                                                                 | 0.041 003 270 886  | 0.001 870 836 040  | -0.101 399 652 759 |
| H                                                                 | 0.209 994 569 809  | 0.037 695 330 998  | -0.048 950 441 752 |
| H                                                                 | 0.004 543 227 654  | 0.011 128 509 277  | -0.002 699 730 653 |
| H                                                                 | 0.126 815 375 984  | -0.480 461 274 313 | 0.082 767 424 732  |
| H                                                                 | -0.416 542 736 078 | -0.194 897 423 408 | 0.190 040 648 506  |
| H                                                                 | -0.009 871 329 945 | -0.014 917 185 856 | 0.017 546 270 042  |
| H                                                                 | -0.005 213 297 791 | -0.053 117 749 911 | 0.302 855 821 044  |
| H                                                                 | -0.014 819 700 905 | -0.088 288 784 330 | 0.046 239 449 195  |
| H                                                                 | 0.071 007 225 634  | -0.101 133 359 460 | -0.048 732 072 097 |

Wavenumber/cm<sup>-1</sup>: 713.7381

| $\frac{\partial \mu_{x,y,z}}{\partial Q_r} / (e u^{-0.5})$        | 0.007 932 057 724  | -0.005 175 669 237 | -0.004 271 409 863 |
|-------------------------------------------------------------------|--------------------|--------------------|--------------------|
| <i>l</i> -matrix coefficients/(u <sup>1/2</sup> Å <sup>-1</sup> ) |                    |                    |                    |
| O                                                                 | -0.017 290 296 009 | -0.008 365 417 842 | -0.002 116 679 156 |
| C                                                                 | 0.003 575 860 973  | -0.045 787 127 707 | -0.048 115 941 735 |
| C                                                                 | 0.045 653 527 883  | 0.085 196 639 858  | 0.051 618 510 735  |
| C                                                                 | 0.012 561 365 478  | 0.025 484 535 036  | 0.012 934 325 781  |
| C                                                                 | -0.011 852 874 362 | -0.014 772 689 809 | 0.003 329 426 568  |
| C                                                                 | -0.027 075 683 194 | -0.009 698 482 475 | -0.155 527 454 578 |
| C                                                                 | 0.003 825 522 643  | -0.005 393 439 860 | -0.008 536 535 695 |
| C                                                                 | 0.014 004 238 748  | 0.038 180 340 241  | -0.025 134 792 565 |
| C                                                                 | 0.027 791 141 895  | 0.053 420 410 675  | 0.032 816 693 509  |
| C                                                                 | 0.022 236 873 477  | 0.000 246 950 314  | -0.004 042 038 444 |
| C                                                                 | 0.049 611 418 978  | 0.078 254 692 845  | 0.028 634 484 461  |
| H                                                                 | -0.092 493 194 131 | -0.260 314 780 770 | -0.146 901 201 468 |
| H                                                                 | -0.168 646 191 772 | 0.125 982 121 759  | 0.357 684 708 537  |
| H                                                                 | -0.009 744 978 622 | 0.025 651 032 827  | 0.001 177 433 887  |
| H                                                                 | 0.288 086 238 650  | -0.091 422 567 343 | 0.280 986 005 317  |
| H                                                                 | 0.014 184 884 782  | -0.012 487 879 176 | -0.008 609 738 318 |
| H                                                                 | -0.089 856 005 330 | 0.018 912 513 732  | -0.005 381 968 655 |
| H                                                                 | -0.218 471 710 394 | -0.295 536 774 665 | -0.205 416 845 651 |
| H                                                                 | -0.012 332 871 885 | -0.001 025 070 955 | 0.020 866 387 796  |
| H                                                                 | -0.199 833 320 109 | -0.047 873 467 846 | 0.131 834 169 695  |
| H                                                                 | 0.025 099 197 421  | 0.066 771 069 072  | -0.010 363 533 165 |
| H                                                                 | 0.019 820 507 814  | -0.075 392 742 386 | 0.008 537 226 113  |
| H                                                                 | -0.070 157 181 984 | -0.030 304 653 001 | 0.028 436 069 230  |
| H                                                                 | -0.032 533 956 450 | -0.039 973 235 853 | 0.050 527 963 980  |
| H                                                                 | 0.138 632 705 275  | 0.058 141 445 657  | -0.217 428 312 852 |
| H                                                                 | 0.150 475 517 122  | 0.031 314 875 284  | -0.149 149 361 338 |
| H                                                                 | -0.157 765 125 855 | -0.147 224 725 047 | 0.258 336 479 822  |

Wavenumber/cm<sup>-1</sup>: 756.1024

| $\frac{\partial \mu_{x,y,z}}{\partial Q_r} / (e u^{-0.5})$   |                    |                    |                                       |
|--------------------------------------------------------------|--------------------|--------------------|---------------------------------------|
| $l$ -matrix coefficients/(u <sup>1/2</sup> Å <sup>-1</sup> ) |                    |                    |                                       |
| O                                                            | -0.000 977 946 728 | -0.002 082 997 226 | 0.000 975 684 816                     |
| C                                                            | -0.045 031 400 062 | -0.002 631 762 165 | -0.002 834 123 123                    |
| C                                                            | 0.111 105 909 490  | -0.085 337 053 294 | 0.042 184 719 840                     |
| C                                                            | 0.001 663 435 579  | 0.006 619 416 700  | -0.009 974 707 276                    |
| C                                                            | -0.008 336 538 588 | 0.033 098 663 197  | -9.352 725 500 000 × 10 <sup>-5</sup> |
| C                                                            | 0.003 842 171 066  | 0.009 233 552 206  | -0.020 524 533 310                    |
| C                                                            | -0.008 993 318 845 | -0.005 364 980 889 | -0.002 177 274 212                    |
| C                                                            | 0.037 712 790 445  | 0.085 475 510 984  | -0.040 292 266 631                    |
| C                                                            | 0.123 946 756 874  | 0.008 229 184 911  | -0.055 570 484 053                    |
| C                                                            | -0.033 601 345 974 | -0.009 719 567 435 | 0.003 886 975 297                     |
| C                                                            | -0.034 739 463 089 | -0.045 476 903 579 | 0.052 609 654 913                     |
| H                                                            | 0.100 708 629 263  | -0.274 947 249 572 | 0.229 269 957 263                     |
| H                                                            | -0.019 000 426 311 | -0.000 561 732 309 | 0.028 331 390 649                     |
| H                                                            | 0.000 767 246 561  | 0.025 626 329 002  | 0.004 221 128 000                     |
| H                                                            | 0.017 006 512 541  | -0.006 470 545 457 | 0.014 744 044 710                     |
| H                                                            | 0.020 029 284 380  | -0.022 157 685 922 | 0.006 774 512 915                     |
| H                                                            | 0.149 181 597 486  | 0.001 820 825 271  | 0.039 991 062 215                     |
| H                                                            | 0.213 106 251 657  | -0.019 713 146 820 | 0.045 312 722 413                     |
| H                                                            | 0.000 348 578 536  | 0.006 052 314 053  | 0.010 934 090 883                     |
| H                                                            | -0.457 861 649 537 | -0.046 674 534 837 | -0.159 175 799 611                    |
| H                                                            | -0.018 683 948 747 | -0.068 067 488 847 | 0.020 522 069 040                     |
| H                                                            | 0.062 390 295 894  | -0.232 243 061 963 | 0.046 057 284 134                     |
| H                                                            | -0.208 294 950 463 | -0.097 802 981 437 | 0.095 554 283 676                     |
| H                                                            | 0.048 738 652 920  | 0.108 133 456 829  | -0.073 452 322 737                    |
| H                                                            | -0.181 280 696 203 | 0.006 703 931 113  | -0.159 392 756 461                    |
| H                                                            | -0.224 554 111 292 | 0.369 270 187 919  | 0.071 267 368 549                     |
| H                                                            | -0.008 110 534 134 | 0.279 606 941 990  | -0.111 671 066 835                    |



Wavenumber/cm<sup>-1</sup>: 835.7459

| $\frac{\partial \mu_{x,y,z}}{\partial Q_r} / (e u^{-0.5})$        | 0.021 051 867 327  | 0.000 222 295 994  | -0.004 402 970 741 |
|-------------------------------------------------------------------|--------------------|--------------------|--------------------|
| <i>l</i> -matrix coefficients/(u <sup>1/2</sup> Å <sup>-1</sup> ) |                    |                    |                    |
| O                                                                 | 0.011 294 538 735  | 0.004 990 472 092  | 0.000 508 489 025  |
| C                                                                 | -0.025 578 397 180 | 0.003 109 170 553  | 0.070 881 276 296  |
| C                                                                 | -0.010 849 103 771 | 0.075 876 472 528  | -0.017 872 467 299 |
| C                                                                 | 0.001 267 877 313  | -0.019 124 481 803 | -0.014 599 256 574 |
| C                                                                 | 0.010 454 863 488  | -0.013 282 345 221 | -0.017 249 397 400 |
| C                                                                 | 0.030 326 891 400  | 0.017 189 927 123  | 0.097 661 077 435  |
| C                                                                 | 0.017 284 533 966  | -0.012 659 763 602 | -0.014 301 502 806 |
| C                                                                 | 0.026 405 113 326  | 0.051 028 138 546  | 0.003 002 387 229  |
| C                                                                 | 0.042 173 323 967  | 0.067 856 019 696  | 0.062 151 464 426  |
| C                                                                 | -0.039 663 095 702 | -0.030 250 269 760 | 0.060 906 930 671  |
| C                                                                 | -0.005 952 474 616 | 0.027 091 540 204  | -0.071 196 284 033 |
| H                                                                 | -0.128 371 116 543 | -0.310 871 740 323 | -0.215 747 809 814 |
| H                                                                 | 0.113 993 739 625  | -0.101 072 175 638 | -0.250 260 337 437 |
| H                                                                 | -0.049 532 092 612 | 0.071 427 760 930  | 0.003 742 866 957  |
| H                                                                 | -0.198 643 604 275 | 0.066 884 866 106  | -0.202 562 869 948 |
| H                                                                 | -0.011 497 533 840 | -0.000 639 789 939 | 0.005 371 713 203  |
| H                                                                 | 0.140 884 939 472  | 0.100 404 065 230  | 0.136 404 033 139  |
| H                                                                 | -0.142 309 763 050 | 0.114 637 942 192  | 0.019 623 495 914  |
| H                                                                 | -0.022 583 713 035 | 0.004 838 625 771  | 0.076 817 207 499  |
| H                                                                 | -0.232 166 220 674 | -0.058 024 748 979 | 0.161 636 798 790  |
| H                                                                 | -0.163 149 174 509 | -0.035 161 735 610 | -0.187 944 164 355 |
| H                                                                 | 0.036 053 732 398  | -0.160 809 747 882 | 0.017 203 046 505  |
| H                                                                 | -0.137 055 833 118 | -0.070 263 094 076 | 0.042 860 028 419  |
| H                                                                 | 0.185 154 132 263  | 0.040 708 520 672  | -0.260 447 330 569 |
| H                                                                 | 0.162 308 353 523  | -0.019 776 739 211 | 0.236 928 453 990  |
| H                                                                 | 0.200 713 357 216  | 0.006 098 571 942  | -0.181 071 180 253 |
| H                                                                 | 0.042 861 663 454  | -0.244 172 355 000 | 0.045 228 739 569  |

Wavenumber/cm<sup>-1</sup>: 861.605

| $\frac{\partial \mu_{x,y,z}}{\partial Q_r} / (e u^{-0.5})$        | 0.000 818 029 200  | 0.005 735 208 623  | 0.013 160 673 864  |
|-------------------------------------------------------------------|--------------------|--------------------|--------------------|
| <i>l</i> -matrix coefficients/(u <sup>1/2</sup> Å <sup>-1</sup> ) |                    |                    |                    |
| O                                                                 | 0.005 925 644 014  | -0.001 393 787 296 | 0.000 970 766 514  |
| C                                                                 | -0.060 771 597 804 | 0.010 966 340 548  | 0.015 726 374 639  |
| C                                                                 | 0.011 523 112 102  | -0.006 808 459 438 | -0.051 354 276 081 |
| C                                                                 | 0.004 273 688 980  | -0.000 980 112 440 | -0.013 195 898 373 |
| C                                                                 | -0.011 383 602 151 | -0.011 244 105 111 | 0.007 823 652 567  |
| C                                                                 | -0.013 163 984 860 | -0.021 258 710 556 | -0.095 177 743 892 |
| C                                                                 | 0.011 566 870 089  | -0.002 977 949 128 | -0.006 405 731 930 |
| C                                                                 | -0.036 031 526 622 | -0.090 121 309 288 | 0.022 781 991 110  |
| C                                                                 | 0.031 918 938 262  | -0.059 823 376 052 | -0.018 818 481 501 |
| C                                                                 | -0.092 256 589 436 | 0.002 912 555 052  | 0.037 438 090 490  |
| C                                                                 | 0.000 566 944 272  | 0.041 367 036 597  | -0.075 659 350 429 |
| H                                                                 | 0.090 896 000 900  | 0.084 449 130 409  | 0.164 520 414 024  |
| H                                                                 | -0.114 448 667 031 | 0.068 228 907 046  | 0.238 397 487 565  |
| H                                                                 | -0.015 389 474 427 | 0.032 341 213 945  | 0.002 818 350 708  |
| H                                                                 | 0.193 695 042 466  | -0.028 728 548 204 | 0.172 843 308 998  |
| H                                                                 | -0.005 549 255 755 | 0.005 901 809 337  | -0.003 874 858 137 |
| H                                                                 | 0.375 815 922 746  | -0.017 936 740 734 | 0.077 938 877 880  |
| H                                                                 | -0.165 059 118 752 | 0.122 482 845 140  | 0.017 083 824 597  |
| H                                                                 | -0.016 530 258 864 | -0.001 698 489 367 | 0.034 882 840 334  |
| H                                                                 | -0.046 399 148 487 | 0.010 279 423 154  | -0.162 939 814 970 |
| H                                                                 | -0.109 713 123 482 | -0.209 992 884 657 | 0.001 987 462 445  |
| H                                                                 | -0.059 971 678 281 | 0.242 719 997 667  | -0.041 810 920 603 |
| H                                                                 | 0.215 901 283 008  | 0.102 152 267 319  | -0.086 759 771 109 |
| H                                                                 | 0.164 308 311 192  | 0.211 083 588 330  | -0.240 978 795 059 |
| H                                                                 | 0.133 545 775 300  | -0.025 382 715 143 | 0.268 409 256 976  |
| H                                                                 | -0.178 405 753 307 | 0.146 074 349 974  | 0.113 223 276 475  |
| H                                                                 | 0.044 464 841 717  | -0.260 157 864 905 | 0.050 844 643 595  |

Wavenumber/cm<sup>-1</sup>: 872.944

| $\frac{\partial \mu_{x,y,z}}{\partial Q_r} / (e u^{-0.5})$        |                    |                    |                    |
|-------------------------------------------------------------------|--------------------|--------------------|--------------------|
|                                                                   | -0.014 068 887 410 | -0.020 360 130 822 | -0.010 178 163 045 |
| <i>l</i> -matrix coefficients/(u <sup>1/2</sup> Å <sup>-1</sup> ) |                    |                    |                    |
| O                                                                 | 0.011 503 158 576  | -0.000 805 744 855 | -0.003 911 919 559 |
| C                                                                 | -0.080 003 204 958 | 0.008 410 660 868  | -0.034 927 649 607 |
| C                                                                 | 0.006 104 008 900  | 0.005 274 988 681  | 0.046 660 858 691  |
| C                                                                 | 0.001 104 824 589  | 0.003 269 635 923  | 0.014 859 503 738  |
| C                                                                 | -0.001 465 401 573 | 0.012 595 902 319  | -0.003 031 792 243 |
| C                                                                 | 0.011 721 818 562  | 0.006 850 073 543  | 0.017 424 015 748  |
| C                                                                 | -0.025 695 429 701 | 0.012 212 438 859  | 0.017 964 280 860  |
| C                                                                 | 0.020 002 600 852  | 0.035 310 418 890  | -0.019 009 454 195 |
| C                                                                 | -0.076 813 535 277 | 0.018 346 342 762  | 0.041 312 605 232  |
| C                                                                 | -0.120 648 298 620 | 0.052 382 811 353  | -0.023 862 984 591 |
| C                                                                 | 0.030 929 041 695  | -0.010 440 305 881 | 0.061 064 741 770  |
| H                                                                 | -0.087 876 618 638 | 0.085 572 995 501  | -0.179 142 963 249 |
| H                                                                 | 0.003 081 947 649  | -0.038 521 265 873 | -0.025 836 021 365 |
| H                                                                 | 0.043 361 211 198  | -0.074 499 928 994 | -0.004 365 314 412 |
| H                                                                 | -0.027 002 284 905 | 0.019 023 886 488  | -0.029 732 974 340 |
| H                                                                 | 0.013 321 221 078  | -0.014 547 164 686 | 0.000 716 120 640  |
| H                                                                 | 0.504 882 443 657  | -0.172 436 837 715 | -0.046 030 451 234 |
| H                                                                 | 0.048 868 385 026  | -0.157 979 345 180 | -0.064 865 754 115 |
| H                                                                 | 0.032 354 874 742  | 0.001 281 190 124  | -0.078 899 741 297 |
| H                                                                 | 0.210 591 908 751  | 0.021 729 721 630  | 0.101 181 484 967  |
| H                                                                 | 0.019 096 053 389  | -0.352 283 922 272 | 0.270 997 317 844  |
| H                                                                 | 0.028 035 508 170  | -0.093 320 001 652 | 0.022 171 510 172  |
| H                                                                 | -0.092 302 541 858 | -0.044 356 474 770 | 0.039 596 512 711  |
| H                                                                 | 0.047 077 513 846  | 0.326 450 337 964  | -0.090 242 998 238 |
| H                                                                 | -0.085 251 060 806 | 0.028 720 817 160  | -0.242 190 946 897 |
| H                                                                 | 0.182 933 869 734  | -0.187 389 209 133 | -0.105 019 561 907 |
| H                                                                 | -0.076 602 354 187 | 0.157 944 820 819  | 0.038 347 700 893  |

Wavenumber/cm<sup>-1</sup>: 925.5809

| $\frac{\partial \mu_{x,y,z}}{\partial Q_r} / (e u^{-0.5})$        |                    |                    |                    |
|-------------------------------------------------------------------|--------------------|--------------------|--------------------|
|                                                                   | -0.003 395 328 823 | 0.010 869 862 159  | -0.000 445 378 001 |
| <i>l</i> -matrix coefficients/(u <sup>1/2</sup> Å <sup>-1</sup> ) |                    |                    |                    |
| O                                                                 | -0.007 833 298 944 | -0.000 328 250 641 | 0.000 521 209 585  |
| C                                                                 | -0.006 111 748 392 | 0.007 424 578 038  | -0.071 335 768 948 |
| C                                                                 | -0.001 322 646 195 | 0.009 814 361 794  | -0.001 883 536 709 |
| C                                                                 | 0.009 026 038 072  | -0.000 502 442 516 | 0.000 941 279 964  |
| C                                                                 | 0.000 481 315 442  | -0.006 454 750 606 | -0.010 346 033 878 |
| C                                                                 | -0.003 523 685 777 | -0.001 559 382 605 | 0.002 693 060 087  |
| C                                                                 | 0.025 224 876 684  | -0.020 917 713 831 | -0.025 045 786 157 |
| C                                                                 | -0.013 735 599 200 | -0.029 534 100 598 | 0.007 588 022 609  |
| C                                                                 | 0.047 043 101 169  | 0.060 446 735 863  | 0.026 635 343 606  |
| C                                                                 | 0.004 717 167 313  | 0.082 337 340 990  | -0.104 215 058 097 |
| C                                                                 | -0.017 566 321 379 | -0.044 370 469 722 | -0.082 426 921 269 |
| H                                                                 | -0.070 078 317 156 | -0.258 459 652 742 | -0.108 664 081 904 |
| H                                                                 | -0.021 243 745 897 | 0.004 294 030 729  | 0.044 558 362 149  |
| H                                                                 | -0.061 800 594 745 | 0.094 877 040 034  | 0.004 895 900 815  |
| H                                                                 | 0.028 835 703 594  | -0.009 532 347 834 | 0.037 374 806 740  |
| H                                                                 | -0.004 274 443 795 | -0.001 924 169 950 | -0.000 316 796 420 |
| H                                                                 | 0.012 628 901 630  | -0.237 118 805 041 | -0.235 786 563 081 |
| H                                                                 | 0.018 139 339 875  | 0.282 137 063 338  | 0.143 451 239 394  |
| H                                                                 | -0.030 175 881 983 | 0.006 695 040 856  | 0.103 734 203 072  |
| H                                                                 | -0.214 482 835 221 | -0.046 060 443 520 | 0.106 047 860 284  |
| H                                                                 | 0.235 972 633 542  | -0.129 830 560 503 | 0.399 798 726 334  |
| H                                                                 | -0.016 295 925 312 | 0.077 956 000 125  | -0.005 617 538 192 |
| H                                                                 | 0.072 170 697 857  | 0.032 611 041 843  | -0.032 321 661 404 |
| H                                                                 | -0.252 495 244 706 | 0.055 173 282 434  | 0.342 464 220 534  |
| H                                                                 | -0.023 136 421 911 | -0.057 404 753 398 | 0.303 648 727 221  |
| H                                                                 | 0.107 218 921 404  | 0.033 409 059 313  | -0.104 832 868 858 |
| H                                                                 | 0.097 535 926 761  | -0.041 186 724 180 | -0.111 986 855 997 |

Wavenumber/cm<sup>-1</sup>: 944.1664

| $\frac{\partial \mu_{x,y,z}}{\partial Q_r} / (e u^{-0.5})$        | 0.009 321 920 553  | -0.036 518 501 719 | -0.029 204 266 409 |
|-------------------------------------------------------------------|--------------------|--------------------|--------------------|
| <i>l</i> -matrix coefficients/(u <sup>1/2</sup> Å <sup>-1</sup> ) |                    |                    |                    |
| O                                                                 | -0.001 024 922 812 | -0.001 281 368 436 | 0.000 778 062 878  |
| C                                                                 | 0.000 533 911 364  | -0.007 990 325 037 | 0.026 926 226 840  |
| C                                                                 | -0.032 230 705 187 | -0.020 467 400 989 | 0.018 005 549 179  |
| C                                                                 | 0.003 380 873 350  | 0.000 645 541 891  | -0.003 924 895 302 |
| C                                                                 | 0.004 765 253 829  | -0.008 522 709 306 | -0.005 203 987 233 |
| C                                                                 | -0.022 926 095 887 | -0.020 336 458 685 | -0.114 592 043 868 |
| C                                                                 | 0.015 217 776 830  | -0.015 884 161 668 | -0.014 326 458 801 |
| C                                                                 | -0.021 880 225 347 | -0.038 731 721 986 | 0.015 238 795 955  |
| C                                                                 | -0.032 391 634 997 | 0.064 473 944 845  | 0.043 918 089 905  |
| C                                                                 | -0.003 261 236 629 | -0.045 733 691 138 | 0.057 364 507 568  |
| C                                                                 | -0.026 352 019 647 | -0.118 988 239 716 | 0.013 548 002 638  |
| H                                                                 | -0.115 984 404 985 | -0.097 549 576 429 | -0.210 801 291 206 |
| H                                                                 | -0.113 802 710 966 | 0.093 857 723 318  | 0.242 283 626 773  |
| H                                                                 | -0.035 233 167 425 | 0.051 805 864 585  | 0.002 653 062 904  |
| H                                                                 | 0.196 091 693 995  | -0.040 480 748 124 | 0.177 043 611 860  |
| H                                                                 | -0.001 387 496 376 | 0.010 252 624 504  | -0.008 257 259 915 |
| H                                                                 | -0.003 159 069 846 | 0.132 576 593 778  | 0.133 203 887 485  |
| H                                                                 | 0.284 282 535 994  | 0.209 402 147 361  | 0.181 964 648 257  |
| H                                                                 | -0.016 166 824 465 | 0.001 100 519 819  | 0.057 730 193 027  |
| H                                                                 | 0.041 938 938 024  | -0.009 413 783 383 | 0.154 351 076 850  |
| H                                                                 | -0.126 106 275 745 | 0.072 763 940 133  | -0.216 133 398 528 |
| H                                                                 | -0.031 630 102 616 | 0.130 213 997 798  | -0.019 081 209 072 |
| H                                                                 | 0.116 187 034 542  | 0.057 162 249 223  | -0.058 841 300 456 |
| H                                                                 | 0.139 802 287 155  | -0.022 127 459 215 | -0.189 000 037 791 |
| H                                                                 | -0.245 143 759 126 | -0.042 829 950 739 | 0.026 207 564 626  |
| H                                                                 | 0.213 612 176 292  | -0.151 123 590 138 | -0.142 848 628 278 |
| H                                                                 | 0.098 257 860 785  | 0.339 710 248 698  | -0.261 138 209 468 |

Wavenumber/cm<sup>-1</sup>: 946.9164

| $\frac{\partial \mu_{x,y,z}}{\partial Q_r} / (e u^{-0.5})$        | 0.016 261 607 747  | -0.011 916 485 178                 | -0.005 352 663 679 |
|-------------------------------------------------------------------|--------------------|------------------------------------|--------------------|
| <i>l</i> -matrix coefficients/(u <sup>1/2</sup> Å <sup>-1</sup> ) |                    |                                    |                    |
| O                                                                 | -0.011 564 668 397 | -0.005 999 793 586                 | -0.002 877 124 791 |
| C                                                                 | 0.003 877 759 971  | -0.016 895 999 497                 | -0.021 194 313 934 |
| C                                                                 | 0.011 348 087 587  | -0.007 277 357 236                 | 0.011 308 668 583  |
| C                                                                 | -0.006 292 473 301 | 0.025 593 893 518                  | 0.026 036 543 224  |
| C                                                                 | 0.019 323 783 214  | 0.037 287 432 836                  | 0.012 936 015 929  |
| C                                                                 | 0.004 201 821 215  | 0.004 649 294 876                  | 0.010 288 932 244  |
| C                                                                 | -0.151 770 696 473 | 0.125 645 739 821                  | 0.158 891 079 238  |
| C                                                                 | -0.030 894 835 963 | -0.049 394 271 025                 | -0.007 990 627 307 |
| C                                                                 | 0.033 267 700 324  | -0.004 139 344 035                 | 0.061 693 801 385  |
| C                                                                 | 0.004 273 994 700  | -0.010 612 671 655                 | 0.002 963 233 401  |
| C                                                                 | 0.003 887 810 675  | -0.003 954 349 897                 | -0.027 772 169 796 |
| H                                                                 | -0.054 147 986 199 | -0.095 900 337 150                 | -0.098 934 885 842 |
| H                                                                 | 0.003 622 902 257  | -0.005 564 840 794                 | -0.007 483 223 485 |
| H                                                                 | 0.332 934 182 370  | -0.534 095 075 106                 | -0.024 934 053 246 |
| H                                                                 | -0.013 208 984 062 | -0.007 033 359 969                 | -0.005 752 929 383 |
| H                                                                 | 0.011 541 593 694  | -0.015 598 173 578                 | 0.022 874 726 957  |
| H                                                                 | -0.025 828 827 109 | 0.018 217 440 360                  | 0.013 045 885 312  |
| H                                                                 | -0.008 491 131 299 | 0.061 669 919 222                  | 0.025 662 717 033  |
| H                                                                 | 0.185 888 688 327  | -0.027 424 062 799                 | -0.609 276 653 869 |
| H                                                                 | -0.154 312 885 043 | -0.016 072 279 134                 | -0.045 445 953 954 |
| H                                                                 | 0.009 889 762 992  | 0.036 344 307 192                  | -0.010 743 447 308 |
| H                                                                 | -0.022 699 001 570 | 0.114 137 249 006                  | 0.005 565 301 405  |
| H                                                                 | 0.103 580 232 269  | 0.055 475 601 245                  | -0.019 444 896 287 |
| H                                                                 | -0.003 362 802 352 | $7.036 617 000 000 \times 10^{-5}$ | 0.007 070 224 987  |
| H                                                                 | -0.014 279 120 377 | -0.014 822 082 145                 | 0.077 245 182 691  |
| H                                                                 | 0.061 568 892 727  | 0.121 322 494 603                  | -0.095 094 239 845 |
| H                                                                 | 0.008 875 432 462  | -0.015 136 642 506                 | -0.007 047 250 767 |

Wavenumber/cm<sup>-1</sup>: 959.5562

| $\frac{\partial \mu_{x,y,z}}{\partial Q_r} / (e u^{-0.5})$        |                    |                    |                    |
|-------------------------------------------------------------------|--------------------|--------------------|--------------------|
|                                                                   | -0.006 208 946 791 | -0.002 376 312 374 | -0.005 413 196 329 |
| <i>l</i> -matrix coefficients/(u <sup>1/2</sup> Å <sup>-1</sup> ) |                    |                    |                    |
| O                                                                 | 0.004 378 794 690  | 0.002 022 630 676  | 0.003 808 376 157  |
| C                                                                 | 0.015 058 397 436  | -0.003 049 831 772 | 0.019 057 609 189  |
| C                                                                 | -0.009 229 904 559 | -0.000 441 776 286 | -0.009 058 461 900 |
| C                                                                 | -0.009 008 889 300 | -0.006 338 102 287 | -0.018 966 351 485 |
| C                                                                 | 0.023 071 627 844  | -0.038 647 416 127 | 0.010 094 722 662  |
| C                                                                 | -0.017 269 696 371 | -0.018 052 685 247 | -0.020 422 287 256 |
| C                                                                 | -0.024 121 280 304 | 0.038 368 610 742  | 0.035 837 162 189  |
| C                                                                 | 0.003 924 052 233  | 0.025 308 290 309  | -0.005 462 216 470 |
| C                                                                 | 0.002 935 859 592  | 0.166 322 249 396  | -0.247 185 477 408 |
| C                                                                 | 0.007 488 918 617  | 0.120 285 140 445  | 0.046 229 235 623  |
| C                                                                 | -0.235 021 492 957 | 0.067 496 465 598  | 0.081 801 475 509  |
| H                                                                 | 0.108 712 878 328  | -0.209 560 616 049 | 0.242 840 568 763  |
| H                                                                 | -0.007 996 352 256 | 0.041 845 016 506  | 0.032 795 746 080  |
| H                                                                 | 0.059 786 994 130  | -0.083 078 845 355 | -0.000 711 141 479 |
| H                                                                 | 0.035 813 310 994  | 0.006 115 505 122  | 0.027 445 108 805  |
| H                                                                 | -0.021 830 853 529 | 0.040 489 841 105  | -0.009 375 709 589 |
| H                                                                 | 0.015 339 605 644  | -0.107 621 190 002 | -0.105 878 352 765 |
| H                                                                 | 0.259 707 762 655  | -0.121 198 560 109 | 0.006 140 160 492  |
| H                                                                 | 0.009 673 020 336  | -0.013 285 328 418 | -0.104 753 656 534 |
| H                                                                 | 0.003 435 062 086  | -0.047 762 912 236 | 0.387 775 326 709  |
| H                                                                 | -0.092 635 389 200 | -0.145 400 540 936 | -0.018 008 232 400 |
| H                                                                 | 0.008 207 996 089  | -0.017 396 727 755 | 0.011 550 815 544  |
| H                                                                 | -0.023 211 783 485 | -0.007 694 756 605 | -0.014 170 811 162 |
| H                                                                 | 0.037 007 305 544  | -0.141 793 438 892 | -0.045 913 887 485 |
| H                                                                 | 0.316 045 999 656  | 0.054 468 916 683  | -0.050 865 770 153 |
| H                                                                 | -0.100 991 857 641 | -0.309 300 336 137 | 0.201 730 411 256  |
| H                                                                 | 0.211 465 566 547  | -0.159 396 203 238 | -0.202 701 940 187 |

Wavenumber/cm<sup>-1</sup>: 965.7962

| $\frac{\partial \mu_{x,y,z}}{\partial Q_r} / (e u^{-0.5})$        | 0.010 263 002 656                     | -0.015 348 525 242 | -0.012 755 236 848 |
|-------------------------------------------------------------------|---------------------------------------|--------------------|--------------------|
| <i>l</i> -matrix coefficients/(u <sup>1/2</sup> Å <sup>-1</sup> ) |                                       |                    |                    |
| O                                                                 | -0.028 772 820 012                    | -0.003 277 377 875 | 0.003 484 280 198  |
| C                                                                 | 0.016 846 955 822                     | 0.114 063 374 019  | 0.043 998 069 900  |
| C                                                                 | 0.002 608 081 163                     | -0.026 335 850 383 | 0.003 728 163 786  |
| C                                                                 | 0.028 191 029 245                     | -0.008 181 737 952 | -0.006 380 164 839 |
| C                                                                 | -0.008 901 982 448                    | -0.008 916 349 091 | -0.011 743 017 354 |
| C                                                                 | -0.003 578 909 210                    | -0.008 669 452 019 | -0.008 821 801 088 |
| C                                                                 | 0.004 255 303 078                     | 0.008 345 034 085  | 0.001 977 841 471  |
| C                                                                 | 0.001 521 678 969                     | -0.000 963 901 972 | 0.013 167 826 485  |
| C                                                                 | -0.006 147 710 393                    | 0.069 855 435 389  | -0.096 278 373 061 |
| C                                                                 | -0.079 265 944 669                    | -0.397 745 325 065 | -0.179 365 941 032 |
| C                                                                 | -0.053 560 982 046                    | 0.026 072 498 508  | 0.009 655 131 143  |
| H                                                                 | 0.039 581 227 171                     | -0.070 625 472 462 | 0.087 654 797 978  |
| H                                                                 | -0.003 098 193 311                    | -0.004 354 128 196 | -0.000 716 423 352 |
| H                                                                 | -5.078 307 300 000 × 10 <sup>-5</sup> | -0.021 962 479 706 | -0.004 217 127 210 |
| H                                                                 | 0.002 972 123 070                     | 0.007 999 577 139  | -0.006 474 554 323 |
| H                                                                 | -0.003 023 007 439                    | -0.005 618 563 440 | -0.001 764 703 417 |
| H                                                                 | 0.073 363 547 435                     | 0.298 607 931 298  | 0.322 531 709 496  |
| H                                                                 | 0.043 536 986 002                     | -0.020 075 662 856 | -0.000 806 020 194 |
| H                                                                 | 0.002 103 553 338                     | -0.002 688 399 841 | -0.018 435 979 456 |
| H                                                                 | 0.022 291 169 818                     | -0.014 424 512 800 | 0.147 655 333 316  |
| H                                                                 | 0.289 382 638 295                     | 0.364 546 566 470  | 0.116 517 498 591  |
| H                                                                 | -0.002 857 874 272                    | -0.004 152 444 053 | -0.006 919 274 215 |
| H                                                                 | -0.005 029 483 658                    | -0.005 547 090 590 | -0.013 228 410 177 |
| H                                                                 | -0.103 261 740 759                    | 0.486 356 235 164  | 0.102 840 238 817  |
| H                                                                 | 0.078 543 608 480                     | 0.010 127 728 219  | 0.016 625 336 329  |
| H                                                                 | -0.030 782 732 853                    | -0.136 716 933 911 | 0.076 074 176 982  |
| H                                                                 | 0.049 368 511 432                     | -0.065 911 156 175 | -0.037 047 509 362 |



Wavenumber/cm<sup>-1</sup>: 1001.6871

| $\frac{\partial \mu_{x,y,z}}{\partial Q_r} / (e u^{-0.5})$        | 0.011 268 785 024  | -0.001 540 419 978 | -0.003 669 460 915 |
|-------------------------------------------------------------------|--------------------|--------------------|--------------------|
| <i>l</i> -matrix coefficients/(u <sup>1/2</sup> Å <sup>-1</sup> ) |                    |                    |                    |
| O                                                                 | -0.005 946 907 884 | -0.001 313 477 412 | 0.000 267 556 843  |
| C                                                                 | -0.016 392 951 605 | 0.016 073 466 532  | 0.016 554 002 963  |
| C                                                                 | 0.053 976 991 518  | 0.011 206 537 862  | -0.063 329 321 797 |
| C                                                                 | 0.007 001 347 294  | -0.001 880 670 314 | -0.002 647 397 471 |
| C                                                                 | -0.022 064 898 206 | -0.010 934 542 322 | 0.022 785 352 470  |
| C                                                                 | 0.003 319 034 761  | -0.010 325 746 352 | -0.012 219 423 338 |
| C                                                                 | 0.012 323 899 368  | -0.004 187 910 254 | -0.017 346 171 340 |
| C                                                                 | 0.013 305 201 310  | 0.011 327 399 029  | -0.007 358 378 442 |
| C                                                                 | -0.019 221 113 202 | -0.138 822 748 313 | 0.233 648 046 184  |
| C                                                                 | 0.003 486 411 689  | -0.027 314 147 804 | -0.025 724 496 540 |
| C                                                                 | -0.307 942 784 300 | 0.073 861 486 535  | 0.122 146 433 012  |
| H                                                                 | -0.105 012 494 086 | 0.173 042 101 173  | -0.220 347 443 554 |
| H                                                                 | -0.016 153 652 516 | 0.007 302 597 855  | 0.034 809 394 438  |
| H                                                                 | -0.013 564 027 299 | 0.032 898 317 173  | 0.000 512 514 231  |
| H                                                                 | 0.020 785 772 091  | 0.007 606 645 036  | 0.010 638 053 159  |
| H                                                                 | 0.009 797 940 222  | 0.005 203 231 537  | -0.016 875 329 997 |
| H                                                                 | -0.009 263 299 607 | 0.014 012 766 969  | 0.010 626 056 916  |
| H                                                                 | 0.333 083 731 654  | -0.159 758 670 389 | 0.010 254 939 571  |
| H                                                                 | -0.022 009 091 392 | -0.000 260 959 653 | 0.046 360 870 981  |
| H                                                                 | 0.014 640 054 281  | 0.047 564 622 238  | -0.326 919 291 205 |
| H                                                                 | 0.034 101 277 341  | 0.019 830 247 836  | 0.025 346 849 455  |
| H                                                                 | 0.004 364 518 014  | -0.021 586 822 981 | -0.005 696 191 550 |
| H                                                                 | -0.028 944 413 985 | -0.013 289 261 204 | 0.017 989 636 487  |
| H                                                                 | -0.029 738 463 818 | 0.032 990 862 564  | 0.040 274 420 189  |
| H                                                                 | 0.391 721 583 924  | 0.067 891 643 512  | -0.092 972 854 632 |
| H                                                                 | 0.111 512 989 944  | 0.247 030 422 183  | -0.191 075 885 864 |
| H                                                                 | 0.268 030 555 647  | -0.175 645 008 450 | -0.263 974 689 915 |

Wavenumber/cm<sup>-1</sup>: 1031.5815

| $\frac{\partial \mu_{x,y,z}}{\partial Q_r} / (e u^{-0.5})$        | 0.002 516 867 788  | 0.018 268 323 074  | 0.012 464 435 863  |
|-------------------------------------------------------------------|--------------------|--------------------|--------------------|
| <i>l</i> -matrix coefficients/(u <sup>1/2</sup> Å <sup>-1</sup> ) |                    |                    |                    |
| O                                                                 | 0.003 780 894 649  | -0.037 212 023 911 | -0.029 953 448 692 |
| C                                                                 | -0.040 099 197 662 | -0.440 165 510 847 | -0.344 521 317 755 |
| C                                                                 | 0.096 915 605 833  | 0.072 753 413 425  | 0.172 563 753 415  |
| C                                                                 | -0.040 098 119 864 | 0.192 633 227 484  | 0.156 319 637 082  |
| C                                                                 | -0.004 312 176 572 | 0.132 824 602 855  | -0.059 332 807 962 |
| C                                                                 | 0.127 569 402 217  | 0.325 596 274 496  | -0.001 030 342 284 |
| C                                                                 | -0.017 768 838 618 | -0.071 553 021 694 | -0.023 871 511 672 |
| C                                                                 | -0.028 383 390 002 | -0.052 033 236 329 | 0.077 472 288 550  |
| C                                                                 | -0.039 686 911 483 | -0.021 717 436 496 | -0.062 617 156 755 |
| C                                                                 | 0.012 365 361 215  | 0.085 799 065 283  | 0.103 529 186 270  |
| C                                                                 | -0.068 488 746 830 | -0.020 305 132 472 | -0.057 460 881 960 |
| H                                                                 | 0.022 892 293 711  | 0.031 501 243 008  | 0.047 538 959 061  |
| H                                                                 | -0.112 386 633 382 | -0.277 461 112 494 | 0.031 029 196 833  |
| H                                                                 | -0.034 021 701 980 | 0.020 689 936 293  | -0.003 770 764 757 |
| H                                                                 | -0.188 996 568 870 | -0.406 645 558 794 | 0.070 058 125 219  |
| H                                                                 | 0.055 135 706 761  | -0.144 799 629 983 | 0.062 131 307 615  |
| H                                                                 | 0.008 045 117 064  | 0.026 309 791 456  | 0.026 838 354 610  |
| H                                                                 | 0.078 296 059 365  | 0.030 169 579 399  | 0.022 007 424 074  |
| H                                                                 | 0.034 223 476 737  | 0.006 061 844 924  | 0.010 697 358 985  |
| H                                                                 | 0.048 482 476 451  | -0.008 809 168 672 | 0.051 705 370 481  |
| H                                                                 | 0.018 685 747 585  | 0.115 885 636 303  | -0.009 443 591 200 |
| H                                                                 | -0.033 402 105 802 | -0.023 305 855 202 | -0.051 575 973 605 |
| H                                                                 | 0.002 406 495 189  | -0.012 047 976 696 | -0.006 140 820 253 |
| H                                                                 | 0.035 384 675 202  | 0.094 681 996 915  | -0.018 875 487 870 |
| H                                                                 | 0.082 342 620 207  | -0.005 958 534 735 | 0.047 329 837 994  |
| H                                                                 | -0.005 009 126 513 | 0.009 985 984 402  | -0.022 923 091 773 |
| H                                                                 | -0.020 282 789 909 | -0.011 627 691 751 | -0.002 817 505 155 |

Wavenumber/cm<sup>-1</sup>: 1039.0758

| $\frac{\partial \mu_{x,y,z}}{\partial Q_r} / (e u^{-0.5})$        |                                        |                    |                    |
|-------------------------------------------------------------------|----------------------------------------|--------------------|--------------------|
|                                                                   | $-3.276\,177\,660\,410 \times 10^{-5}$ | 0.023 465 655 869  | -0.003 808 457 703 |
| <i>l</i> -matrix coefficients/(u <sup>1/2</sup> Å <sup>-1</sup> ) |                                        |                    |                    |
| O                                                                 | -0.010 690 648 326                     | -0.019 595 043 491 | -0.007 277 702 894 |
| C                                                                 | 0.056 119 718 287                      | -0.078 064 048 429 | 0.051 713 905 245  |
| C                                                                 | -0.052 816 191 339                     | 0.147 200 657 828  | -0.062 705 245 908 |
| C                                                                 | -0.019 285 760 640                     | 0.065 727 966 743  | 0.031 444 002 560  |
| C                                                                 | -0.180 093 834 368                     | -0.252 102 838 120 | 0.147 794 425 292  |
| C                                                                 | 0.008 665 403 946                      | 0.025 403 789 480  | -0.075 720 677 596 |
| C                                                                 | 0.077 385 668 921                      | 0.025 766 076 274  | -0.033 083 035 761 |
| C                                                                 | 0.159 135 861 885                      | 0.165 208 638 293  | 0.329 339 164 121  |
| C                                                                 | 0.021 471 638 205                      | -0.033 653 443 695 | 0.012 374 985 062  |
| C                                                                 | -0.023 685 720 399                     | 0.027 459 574 383  | -0.033 627 861 596 |
| C                                                                 | 0.024 304 687 978                      | -0.063 038 176 876 | 0.008 672 773 050  |
| H                                                                 | 0.003 822 754 335                      | 0.018 415 783 990  | -0.001 765 022 043 |
| H                                                                 | -0.003 655 903 373                     | -0.000 972 992 506 | -0.019 597 206 575 |
| H                                                                 | 0.044 766 817 261                      | -0.058 331 330 310 | -0.020 926 779 703 |
| H                                                                 | -0.022 156 935 669                     | -0.053 174 573 688 | -0.013 261 385 591 |
| H                                                                 | 0.127 580 883 978                      | 0.235 748 418 154  | -0.374 219 519 382 |
| H                                                                 | 0.033 482 983 671                      | 0.022 582 115 728  | 0.014 774 536 184  |
| H                                                                 | -0.032 430 726 085                     | 0.036 089 532 596  | 0.022 829 558 507  |
| H                                                                 | -0.096 913 640 737                     | -0.073 056 133 029 | -0.056 985 212 656 |
| H                                                                 | -0.029 184 158 491                     | -0.013 667 891 941 | 0.010 995 672 203  |
| H                                                                 | 0.018 281 965 870                      | -0.008 348 408 867 | 0.035 634 106 833  |
| H                                                                 | -0.118 588 464 677                     | -0.100 152 565 415 | -0.472 883 902 637 |
| H                                                                 | -0.095 600 914 260                     | -0.078 628 673 772 | -0.366 593 328 417 |
| H                                                                 | -0.011 927 598 302                     | -0.024 400 971 483 | -0.000 163 205 565 |
| H                                                                 | 0.012 606 496 746                      | -0.008 191 916 301 | -0.032 683 649 055 |
| H                                                                 | -0.023 737 955 367                     | 0.028 989 822 836  | 0.015 378 652 265  |
| H                                                                 | -0.009 539 391 423                     | 0.051 925 457 270  | -0.010 182 305 473 |

Wavenumber/cm<sup>-1</sup>: 1056.6828

| $\frac{\partial \mu_{x,y,z}}{\partial Q_r} / (e u^{-0.5})$        | 0.004 327 998 126  | 0.008 318 192 543  | 0.015 651 514 340                     |
|-------------------------------------------------------------------|--------------------|--------------------|---------------------------------------|
| <i>l</i> -matrix coefficients/(u <sup>1/2</sup> Å <sup>-1</sup> ) |                    |                    |                                       |
| O                                                                 | 0.035 561 693 208  | 0.001 220 338 965  | -0.009 245 194 849                    |
| C                                                                 | -0.115 503 886 499 | 0.038 879 473 312  | -0.002 346 749 983                    |
| C                                                                 | 0.263 198 031 067  | -0.142 901 513 787 | -0.018 159 650 234                    |
| C                                                                 | -0.017 086 443 159 | 0.050 712 633 113  | 0.041 726 234 383                     |
| C                                                                 | -0.312 321 485 499 | 0.199 769 796 890  | 0.276 991 934 355                     |
| C                                                                 | 0.016 570 014 060  | -0.080 433 437 753 | 0.029 192 955 831                     |
| C                                                                 | -0.124 095 153 273 | -0.185 870 018 370 | -0.161 492 024 729                    |
| C                                                                 | 0.054 741 963 481  | -0.010 771 457 367 | -0.112 646 026 317                    |
| C                                                                 | -0.079 180 297 745 | 0.068 980 414 748  | -0.005 419 086 262                    |
| C                                                                 | 0.056 795 525 521  | -0.009 046 593 373 | 0.007 822 908 633                     |
| C                                                                 | -0.059 185 995 139 | 0.024 323 464 537  | -0.017 256 534 699                    |
| H                                                                 | 0.000 544 342 148  | -0.072 942 429 553 | 0.063 451 707 143                     |
| H                                                                 | 0.029 325 312 440  | 0.039 054 276 046  | -6.183 545 000 000 × 10 <sup>-6</sup> |
| H                                                                 | 0.220 604 037 976  | 0.117 013 913 291  | 0.013 621 132 768                     |
| H                                                                 | 0.019 201 217 526  | 0.103 221 835 941  | -0.048 915 190 995                    |
| H                                                                 | 0.457 161 534 299  | -0.174 843 817 316 | -0.300 783 028 537                    |
| H                                                                 | -0.046 939 344 559 | 0.005 494 628 578  | -0.004 943 243 880                    |
| H                                                                 | 0.002 407 859 397  | 0.005 736 818 235  | 0.002 375 508 071                     |
| H                                                                 | 0.190 526 923 081  | 0.088 187 729 940  | 0.044 651 735 230                     |
| H                                                                 | 0.059 275 729 351  | 0.028 648 704 653  | -0.005 887 782 832                    |
| H                                                                 | -0.028 206 499 284 | -0.027 927 368 687 | -0.041 321 000 181                    |
| H                                                                 | -0.018 890 929 702 | 0.053 893 264 584  | -0.109 502 294 554                    |
| H                                                                 | 0.061 479 183 597  | 0.054 614 867 323  | 0.218 176 274 662                     |
| H                                                                 | 0.000 527 924 137  | 0.020 764 168 206  | 0.021 714 142 213                     |
| H                                                                 | -0.009 650 282 836 | -0.002 928 394 386 | 0.051 948 777 736                     |
| H                                                                 | 0.047 650 420 414  | -0.057 283 638 963 | -0.033 282 792 685                    |
| H                                                                 | -0.035 638 028 172 | -0.025 542 145 776 | 0.032 931 542 250                     |

Wavenumber/cm<sup>-1</sup>: 1101.1646

| $\frac{\partial \mu_{x,y,z}}{\partial Q_r} / (e u^{-0.5})$        | 0.017 003 496 958  | -0.011 814 456 751 | -0.001 573 362 656                   |
|-------------------------------------------------------------------|--------------------|--------------------|--------------------------------------|
| <i>l</i> -matrix coefficients/(u <sup>1/2</sup> Å <sup>-1</sup> ) |                    |                    |                                      |
| O                                                                 | 0.026 214 581 013  | -0.010 975 598 853 | 9.169 584 200 000 × 10 <sup>-5</sup> |
| C                                                                 | 0.193 234 808 044  | -0.310 114 181 415 | -0.132 493 624 907                   |
| C                                                                 | -0.307 945 670 623 | 0.194 325 336 363  | -0.086 085 378 199                   |
| C                                                                 | -0.047 206 332 688 | 0.131 997 475 899  | 0.048 859 606 410                    |
| C                                                                 | 0.161 091 142 989  | -0.143 971 406 448 | 0.262 704 171 259                    |
| C                                                                 | -0.090 924 043 246 | -0.054 963 152 729 | 0.093 114 653 108                    |
| C                                                                 | -0.151 976 302 205 | -0.096 881 358 962 | -0.104 516 164 420                   |
| C                                                                 | -0.066 830 351 313 | 0.053 311 134 745  | -0.231 950 755 726                   |
| C                                                                 | 0.106 248 667 035  | -0.034 308 932 333 | 0.024 661 044 812                    |
| C                                                                 | -0.075 645 565 981 | 0.071 007 271 736  | 0.018 302 400 172                    |
| C                                                                 | 0.064 198 190 428  | -0.066 300 445 569 | 0.031 233 073 031                    |
| H                                                                 | -0.005 056 309 669 | 0.044 096 738 440  | -0.071 384 633 352                   |
| H                                                                 | 0.109 644 645 782  | 0.200 256 257 820  | -0.082 268 681 121                   |
| H                                                                 | 0.256 041 869 500  | 0.137 789 432 128  | 0.039 518 881 719                    |
| H                                                                 | -0.012 488 919 474 | -0.038 936 502 123 | 0.046 887 720 030                    |
| H                                                                 | 0.070 297 983 345  | 0.238 030 873 849  | -0.152 458 527 576                   |
| H                                                                 | 0.086 944 231 406  | 0.041 621 354 612  | 0.045 228 938 119                    |
| H                                                                 | -0.035 091 232 492 | 0.015 916 389 969  | 0.011 117 256 955                    |
| H                                                                 | -0.001 082 233 504 | 0.014 282 847 933  | 0.047 767 815 051                    |
| H                                                                 | -0.079 145 955 442 | -0.027 234 032 932 | 0.018 388 618 311                    |
| H                                                                 | 0.059 991 003 037  | 0.102 861 610 439  | 0.063 922 395 595                    |
| H                                                                 | 0.091 479 087 850  | 0.068 342 348 925  | 0.276 734 990 125                    |
| H                                                                 | 0.046 669 651 373  | 0.070 802 338 933  | 0.095 019 219 700                    |
| H                                                                 | 0.017 389 656 767  | 0.024 493 856 246  | -0.038 487 240 819                   |
| H                                                                 | 0.044 200 084 725  | -0.003 050 829 621 | -0.070 369 893 892                   |
| H                                                                 | -0.056 398 499 298 | 0.005 828 482 548  | 0.080 931 187 144                    |
| H                                                                 | 0.046 947 853 287  | 0.031 982 617 256  | -0.047 972 555 198                   |

Wavenumber/cm<sup>-1</sup>: 1120.796

| $\frac{\partial \mu_{x,y,z}}{\partial Q_r} / (e u^{-0.5})$        | 0.005 250 340 740  | 0.006 155 756 113  | 0.007 394 299 672  |
|-------------------------------------------------------------------|--------------------|--------------------|--------------------|
| <i>l</i> -matrix coefficients/(u <sup>1/2</sup> Å <sup>-1</sup> ) |                    |                    |                    |
| O                                                                 | -0.035 891 525 268 | -0.014 826 023 509 | -0.014 612 312 050 |
| C                                                                 | 0.321 275 167 596  | 0.058 486 824 559  | -0.068 644 189 768 |
| C                                                                 | -0.172 476 687 047 | -0.105 919 012 525 | 0.223 591 187 928  |
| C                                                                 | -0.032 312 389 920 | 0.036 681 243 911  | 0.103 509 231 222  |
| C                                                                 | -0.110 631 007 708 | 0.151 322 853 124  | -0.125 435 247 975 |
| C                                                                 | -0.019 951 365 412 | -0.167 671 551 474 | -0.006 691 193 695 |
| C                                                                 | 0.113 648 715 402  | -0.042 851 659 530 | 0.002 608 299 606  |
| C                                                                 | -0.091 144 272 275 | 0.064 012 785 687  | 0.063 392 335 587  |
| C                                                                 | 0.056 372 715 153  | 0.026 601 170 053  | -0.045 021 393 097 |
| C                                                                 | -0.103 584 090 440 | -0.010 675 773 619 | 0.016 067 787 766  |
| C                                                                 | 0.021 701 836 297  | 0.016 188 617 164  | -0.075 766 831 692 |
| H                                                                 | -0.006 266 640 125 | 0.033 993 267 606  | -0.069 734 691 509 |
| H                                                                 | 0.219 234 244 976  | 0.502 210 054 681  | -0.058 261 313 378 |
| H                                                                 | -0.192 443 470 977 | -0.083 431 449 728 | -0.041 285 572 942 |
| H                                                                 | -0.093 999 279 027 | -0.218 159 037 032 | 0.010 442 725 425  |
| H                                                                 | 0.020 513 078 641  | -0.137 111 932 310 | 0.040 955 145 911  |
| H                                                                 | 0.076 379 193 160  | -0.053 856 649 117 | -0.017 947 284 703 |
| H                                                                 | 0.085 088 796 359  | -0.029 150 769 079 | -0.022 817 524 408 |
| H                                                                 | 0.067 200 093 108  | 0.001 533 462 947  | -0.018 291 028 746 |
| H                                                                 | -0.032 836 380 433 | 0.003 309 063 657  | -0.024 613 154 520 |
| H                                                                 | 0.026 875 817 914  | 0.050 177 397 498  | 0.040 102 935 036  |
| H                                                                 | -0.102 140 718 253 | -0.139 102 932 080 | -0.277 197 442 564 |
| H                                                                 | 0.097 117 481 174  | 0.111 554 951 987  | 0.213 751 244 973  |
| H                                                                 | 0.030 889 585 590  | -0.049 034 783 768 | -0.074 819 132 639 |
| H                                                                 | 0.027 391 661 578  | -0.004 033 531 433 | 0.031 940 313 128  |
| H                                                                 | -0.013 016 828 235 | 0.014 269 345 280  | 0.010 271 618 452  |
| H                                                                 | -0.007 958 283 153 | -0.034 455 735 484 | 0.013 291 708 810  |

Wavenumber/cm<sup>-1</sup>: 1149.6317

| $\frac{\partial \mu_{x,y,z}}{\partial Q_r} / (e u^{-0.5})$        | 0.017 589 571 066  | -0.012 253 642 361 | -0.010 651 637 285 |
|-------------------------------------------------------------------|--------------------|--------------------|--------------------|
| <i>l</i> -matrix coefficients/(u <sup>1/2</sup> Å <sup>-1</sup> ) |                    |                    |                    |
| O                                                                 | -0.059 076 054 046 | -0.050 995 039 955 | -0.020 591 638 215 |
| C                                                                 | -0.058 779 295 080 | -0.167 482 752 893 | -0.060 209 100 280 |
| C                                                                 | 0.270 979 934 002  | 0.177 331 131 233  | -0.161 275 668 253 |
| C                                                                 | -0.039 988 579 356 | 0.089 360 684 991  | 0.035 275 731 528  |
| C                                                                 | -0.224 306 480 069 | -0.118 345 902 671 | 0.127 586 154 238  |
| C                                                                 | 0.022 470 343 952  | -0.067 359 099 597 | 0.090 788 182 633  |
| C                                                                 | 0.369 252 757 318  | 0.208 797 517 257  | 0.048 375 605 055  |
| C                                                                 | 0.005 869 487 564  | -0.009 270 550 281 | -0.228 330 054 463 |
| C                                                                 | -0.080 047 790 008 | -0.031 408 642 423 | 0.039 355 332 269  |
| C                                                                 | 0.008 180 910 256  | 0.048 098 960 717  | 0.019 542 860 650  |
| C                                                                 | -0.074 470 513 696 | -0.086 486 121 423 | 0.023 469 391 316  |
| H                                                                 | 0.013 615 272 866  | -0.035 935 403 453 | 0.093 556 907 143  |
| H                                                                 | 0.052 736 609 811  | 0.076 862 404 617  | 0.003 664 988 207  |
| H                                                                 | -0.218 992 974 878 | -0.182 640 192 156 | -0.070 718 302 074 |
| H                                                                 | 0.014 760 134 402  | 0.075 577 861 853  | -0.019 832 579 113 |
| H                                                                 | -0.044 566 700 143 | 0.008 632 739 413  | -0.017 801 840 184 |
| H                                                                 | 0.006 104 678 266  | 0.030 549 009 893  | 0.019 795 753 688  |
| H                                                                 | -0.060 984 828 286 | 0.074 320 367 930  | 0.051 544 296 337  |
| H                                                                 | -0.382 584 085 741 | -0.226 084 538 093 | -0.093 618 750 283 |
| H                                                                 | 0.046 186 820 437  | -0.002 821 857 453 | 0.034 183 279 459  |
| H                                                                 | 0.010 513 998 877  | 0.032 826 562 842  | 0.005 440 370 077  |
| H                                                                 | 0.025 618 744 189  | 0.039 710 631 427  | 0.030 249 555 604  |
| H                                                                 | 0.073 682 236 623  | 0.075 722 958 311  | 0.311 580 630 113  |
| H                                                                 | 0.004 253 427 496  | 0.029 527 851 687  | 0.002 668 002 895  |
| H                                                                 | 0.044 475 217 168  | -0.010 244 553 960 | -0.022 520 957 211 |
| H                                                                 | 0.021 205 852 698  | -0.004 917 977 787 | -0.028 865 884 282 |
| H                                                                 | -0.058 160 043 274 | 0.072 835 243 410  | 0.008 547 312 620  |

Wavenumber/cm<sup>-1</sup>: 1172.9845

| $\frac{\partial \mu_{x,y,z}}{\partial Q_r} / (e u^{-0.5})$        |                    |                    |                    |
|-------------------------------------------------------------------|--------------------|--------------------|--------------------|
|                                                                   | -0.036 531 400 608 | -0.019 527 420 494 | 0.001 876 336 812  |
| <i>l</i> -matrix coefficients/(u <sup>1/2</sup> Å <sup>-1</sup> ) |                    |                    |                    |
| O                                                                 | 0.000 265 853 781  | 0.018 206 587 049  | 0.017 503 283 742  |
| C                                                                 | -0.000 859 865 629 | 0.160 270 291 815  | 0.142 997 825 320  |
| C                                                                 | -0.161 171 166 110 | 0.111 906 068 906  | -0.449 131 138 504 |
| C                                                                 | 0.022 923 544 052  | -0.089 053 174 102 | -0.072 906 982 491 |
| C                                                                 | -0.038 783 806 265 | 0.090 423 204 846  | 0.062 064 182 275  |
| C                                                                 | 0.242 322 537 594  | 0.125 136 978 236  | -0.038 861 961 928 |
| C                                                                 | -0.014 346 040 339 | -0.021 263 764 290 | 0.012 331 161 901  |
| C                                                                 | -0.087 318 972 437 | -0.098 220 660 741 | -0.002 521 759 606 |
| C                                                                 | 0.092 693 679 292  | -0.025 845 930 364 | 0.119 516 880 428  |
| C                                                                 | -0.010 029 821 659 | -0.062 320 488 037 | -0.034 021 665 572 |
| C                                                                 | 0.065 175 785 882  | -0.051 175 558 308 | 0.182 419 603 403  |
| H                                                                 | -0.016 873 905 009 | -0.029 028 930 810 | -0.046 434 044 804 |
| H                                                                 | -0.082 872 754 012 | -0.162 846 066 706 | 0.146 310 913 758  |
| H                                                                 | 0.017 162 481 602  | 0.019 517 908 850  | 0.009 591 239 440  |
| H                                                                 | -0.161 600 634 910 | -0.311 771 736 279 | -0.020 266 744 518 |
| H                                                                 | -0.046 538 939 259 | 0.045 558 764 505  | 0.035 756 542 467  |
| H                                                                 | -0.000 824 261 454 | -0.026 397 988 775 | -0.016 162 465 587 |
| H                                                                 | -0.185 385 562 330 | 0.013 435 776 041  | 0.019 616 709 820  |
| H                                                                 | 0.097 908 099 978  | 0.048 857 497 122  | 0.003 970 103 803  |
| H                                                                 | -0.076 559 483 717 | -0.024 512 626 329 | 0.022 296 382 003  |
| H                                                                 | -0.007 536 151 239 | -0.046 038 855 904 | 0.002 247 574 575  |
| H                                                                 | -0.083 173 502 987 | -0.102 880 888 140 | -0.205 231 153 395 |
| H                                                                 | 0.111 989 438 550  | 0.085 105 517 454  | 0.351 981 553 260  |
| H                                                                 | -0.014 209 538 426 | -0.029 072 374 936 | 0.005 880 550 998  |
| H                                                                 | -0.025 096 700 861 | 0.012 702 281 234  | -0.135 892 277 706 |
| H                                                                 | -0.039 596 640 634 | -0.082 061 251 752 | 0.130 058 938 362  |
| H                                                                 | 0.130 339 411 244  | 0.034 112 773 821  | -0.103 810 702 520 |



Wavenumber/cm<sup>-1</sup>: 1190.994

| $\frac{\partial \mu_{x,y,z}}{\partial Q_r} / (e u^{-0.5})$        | 0.003 902 326 140  | 0.003 261 937 730  | 0.003 555 946 718  |
|-------------------------------------------------------------------|--------------------|--------------------|--------------------|
| <i>l</i> -matrix coefficients/(u <sup>1/2</sup> Å <sup>-1</sup> ) |                    |                    |                    |
| O                                                                 | 0.036 158 760 484  | 0.004 431 330 571  | -0.020 202 894 796 |
| C                                                                 | -0.045 355 231 246 | -0.073 650 822 447 | 0.091 185 895 869  |
| C                                                                 | -0.188 345 094 931 | 0.453 664 916 382  | 0.069 744 475 383  |
| C                                                                 | -0.002 175 302 132 | 0.005 408 286 348  | 0.094 617 515 876  |
| C                                                                 | -0.122 064 025 032 | 0.138 768 074 577  | -0.157 167 789 528 |
| C                                                                 | -0.045 080 132 614 | -0.055 005 513 529 | -0.016 996 812 088 |
| C                                                                 | 0.015 974 992 953  | -0.100 925 248 969 | -0.005 206 373 248 |
| C                                                                 | 0.108 182 433 557  | -0.091 742 752 203 | 0.020 565 430 210  |
| C                                                                 | 0.103 677 569 139  | -0.195 346 281 727 | -0.066 985 070 689 |
| C                                                                 | 0.001 737 449 776  | 0.033 406 582 702  | -0.067 152 301 604 |
| C                                                                 | 0.055 005 259 850  | -0.195 286 232 354 | 0.021 930 117 626  |
| H                                                                 | 0.026 899 016 997  | 0.161 073 442 627  | -0.056 758 142 370 |
| H                                                                 | -0.029 414 931 974 | -0.063 706 602 783 | -0.005 084 237 713 |
| H                                                                 | -0.142 869 820 439 | -0.060 436 110 616 | -0.028 122 947 085 |
| H                                                                 | 0.155 700 046 615  | 0.320 507 709 114  | -0.038 534 029 059 |
| H                                                                 | 0.117 954 421 950  | -0.311 638 363 526 | 0.054 253 963 377  |
| H                                                                 | 0.011 478 699 183  | 0.068 588 543 563  | 0.038 129 727 115  |
| H                                                                 | -0.056 270 008 421 | 0.094 219 115 078  | 0.065 113 024 757  |
| H                                                                 | 0.202 020 961 615  | 0.070 658 275 663  | -0.011 644 383 023 |
| H                                                                 | -0.072 041 050 913 | -0.107 804 183 478 | 0.207 356 963 720  |
| H                                                                 | 0.008 015 579 980  | -0.033 817 726 621 | 0.022 751 598 169  |
| H                                                                 | 0.002 308 202 191  | 0.053 687 928 411  | -0.033 934 603 929 |
| H                                                                 | -0.049 283 497 752 | -0.069 612 641 960 | 0.035 883 813 963  |
| H                                                                 | -0.027 744 772 667 | -0.036 553 074 726 | 0.019 814 268 987  |
| H                                                                 | 0.190 303 666 328  | -0.018 063 236 281 | -0.116 732 506 604 |
| H                                                                 | -0.095 693 718 273 | 0.097 953 786 373  | 0.042 356 501 766  |
| H                                                                 | 0.023 437 714 884  | 0.095 894 329 325  | -0.060 974 469 214 |

Wavenumber/cm<sup>-1</sup>: 1217.6651

| $\frac{\partial \mu_{x,y,z}}{\partial Q_r} / (e u^{-0.5})$   |                    |                    |                    |
|--------------------------------------------------------------|--------------------|--------------------|--------------------|
|                                                              | -0.007 309 665 903 | 0.007 120 811 795  | 0.001 140 995 624  |
| $l$ -matrix coefficients/(u <sup>1/2</sup> Å <sup>-1</sup> ) |                    |                    |                    |
| O                                                            | 0.062 216 729 112  | 0.018 105 913 536  | 0.023 207 399 904  |
| C                                                            | -0.208 039 063 140 | -0.347 836 511 373 | 0.167 728 121 525  |
| C                                                            | 0.260 424 481 215  | 0.120 904 407 246  | -0.109 515 414 955 |
| C                                                            | 0.016 695 348 223  | 0.018 960 329 052  | -0.119 993 124 663 |
| C                                                            | 0.165 577 111 931  | -0.016 252 379 685 | -0.102 234 846 856 |
| C                                                            | 0.103 503 917 096  | -0.124 541 064 246 | -0.094 186 038 005 |
| C                                                            | -0.207 742 055 082 | -0.014 823 338 866 | 0.084 461 256 020  |
| C                                                            | -0.141 698 110 855 | 0.071 235 199 594  | 0.103 140 479 547  |
| C                                                            | -0.122 262 679 656 | -0.063 565 177 432 | 0.011 495 653 457  |
| C                                                            | 0.079 586 593 747  | 0.142 093 305 100  | -0.097 085 360 614 |
| C                                                            | -0.073 723 946 743 | -0.007 645 251 111 | 0.027 941 442 250  |
| H                                                            | 0.018 405 498 049  | -0.026 531 736 700 | 0.118 440 111 659  |
| H                                                            | 0.132 014 003 389  | 0.334 426 636 211  | 0.019 528 178 314  |
| H                                                            | 0.171 417 472 462  | 0.153 296 851 326  | 0.081 370 688 086  |
| H                                                            | -0.019 708 681 471 | 0.048 902 712 525  | -0.116 452 174 132 |
| H                                                            | -0.170 139 419 356 | -0.019 628 639 945 | 0.207 165 202 912  |
| H                                                            | 0.008 480 509 073  | 0.183 522 154 994  | 0.099 974 683 633  |
| H                                                            | -0.036 880 945 786 | 0.034 268 822 866  | 0.025 689 511 672  |
| H                                                            | 0.064 048 434 290  | 0.063 407 551 854  | 0.023 189 988 257  |
| H                                                            | 0.075 038 545 840  | -0.008 676 760 488 | 0.046 218 348 271  |
| H                                                            | 0.010 829 578 161  | -0.077 203 816 047 | 0.038 066 188 782  |
| H                                                            | -0.084 331 280 634 | -0.162 106 064 361 | -0.193 631 517 116 |
| H                                                            | 0.084 996 113 546  | 0.087 701 558 038  | -0.014 563 817 572 |
| H                                                            | -0.052 193 605 244 | 0.009 637 220 435  | 0.082 250 457 833  |
| H                                                            | -0.007 244 542 070 | 0.001 596 551 581  | 0.005 883 420 903  |
| H                                                            | 0.037 372 731 282  | 0.036 223 885 637  | -0.086 525 435 972 |
| H                                                            | -0.039 237 315 483 | 0.033 539 727 934  | 0.013 645 205 479  |

Wavenumber/cm<sup>-1</sup>: 1226.8727

| $\frac{\partial \mu_{x,y,z}}{\partial Q_r} / (e u^{-0.5})$        | 0.015 116 964 667  | -0.007 026 216 698 | -0.005 875 423 869 |
|-------------------------------------------------------------------|--------------------|--------------------|--------------------|
| <i>l</i> -matrix coefficients/(u <sup>1/2</sup> Å <sup>-1</sup> ) |                    |                    |                    |
| O                                                                 | 0.051 603 089 197  | 0.009 588 178 099  | -0.035 068 146 358 |
| C                                                                 | -0.269 142 066 113 | -0.299 658 067 793 | -0.165 090 197 767 |
| C                                                                 | -0.219 299 887 698 | -0.228 621 934 240 | -0.010 792 342 468 |
| C                                                                 | 0.015 250 575 522  | -0.021 629 916 093 | 0.142 912 052 642  |
| C                                                                 | 0.003 054 592 240  | 0.079 303 053 544  | -0.007 347 371 012 |
| C                                                                 | 0.028 592 499 122  | -0.075 457 956 242 | 0.020 656 889 260  |
| C                                                                 | 0.030 773 268 973  | -0.010 118 887 511 | 0.059 485 448 821  |
| C                                                                 | 0.129 315 536 655  | 0.027 075 850 730  | -0.031 006 137 299 |
| C                                                                 | 0.074 268 819 478  | 0.106 142 323 604  | 0.012 056 244 906  |
| C                                                                 | 0.137 545 315 305  | 0.126 951 617 213  | 0.069 242 487 167  |
| C                                                                 | 0.090 435 236 931  | 0.120 704 251 310  | 0.020 858 173 477  |
| H                                                                 | -0.022 322 593 659 | -0.035 108 569 002 | -0.074 927 681 087 |
| H                                                                 | -0.015 696 414 277 | -0.059 646 981 785 | 0.022 358 572 363  |
| H                                                                 | -0.280 159 158 984 | -0.113 086 687 709 | -0.036 369 235 651 |
| H                                                                 | 0.107 647 834 056  | 0.278 716 508 295  | -0.071 491 233 180 |
| H                                                                 | -0.148 342 135 533 | 0.317 258 908 606  | -0.067 788 760 687 |
| H                                                                 | -0.056 777 801 062 | 0.076 620 012 909  | 0.031 351 728 355  |
| H                                                                 | 0.030 384 956 629  | -0.092 405 361 599 | -0.060 939 904 976 |
| H                                                                 | 0.206 632 745 663  | 0.104 358 382 931  | 0.025 174 334 525  |
| H                                                                 | -0.048 434 333 967 | 0.033 224 915 850  | -0.092 321 359 263 |
| H                                                                 | -0.019 741 937 278 | 0.006 437 488 451  | -0.034 507 563 334 |
| H                                                                 | -0.029 352 693 728 | 0.028 992 211 353  | -0.201 203 940 934 |
| H                                                                 | 0.027 556 043 340  | 0.024 940 112 457  | 0.172 359 182 507  |
| H                                                                 | 0.000 759 228 067  | 0.155 302 463 239  | 0.074 864 260 421  |
| H                                                                 | -0.117 374 531 705 | 0.013 480 018 214  | 0.022 351 795 785  |
| H                                                                 | -0.017 265 658 207 | -0.078 731 205 740 | 0.082 487 462 344  |
| H                                                                 | 0.105 115 487 251  | -0.093 386 517 272 | -0.034 767 889 222 |

Wavenumber/cm<sup>-1</sup>: 1247.3909

| $\frac{\partial \mu_{x,y,z}}{\partial Q_r} / (e u^{-0.5})$        |                    |                    |                    |
|-------------------------------------------------------------------|--------------------|--------------------|--------------------|
|                                                                   | -0.013 895 420 593 | 0.001 030 443 302  | -0.011 167 772 190 |
| <i>l</i> -matrix coefficients/(u <sup>1/2</sup> Å <sup>-1</sup> ) |                    |                    |                    |
| O                                                                 | 0.048 032 051 763  | 0.044 993 694 717  | -0.010 550 803 024 |
| C                                                                 | -0.289 985 253 949 | 0.240 365 993 208  | -0.175 532 694 521 |
| C                                                                 | -0.069 422 126 278 | 0.163 640 390 663  | 0.348 184 098 729  |
| C                                                                 | 0.070 245 534 979  | -0.173 850 025 801 | -0.004 821 966 899 |
| C                                                                 | 0.046 580 085 824  | -0.261 106 272 268 | 0.028 434 936 984  |
| C                                                                 | 0.201 248 635 515  | -0.119 172 822 986 | 0.070 602 186 156  |
| C                                                                 | -0.063 444 482 486 | 0.100 027 812 089  | -0.034 837 719 760 |
| C                                                                 | -0.148 069 141 008 | 0.159 314 538 186  | -0.075 939 099 619 |
| C                                                                 | 0.038 132 968 095  | -0.079 553 178 411 | -0.137 516 983 218 |
| C                                                                 | 0.129 699 089 385  | -0.117 086 670 209 | 0.085 453 970 249  |
| C                                                                 | 0.037 402 090 701  | -0.078 343 469 987 | -0.109 540 585 644 |
| H                                                                 | 0.022 566 673 535  | 0.132 184 626 658  | -0.045 506 010 414 |
| H                                                                 | -0.023 792 038 329 | -0.020 434 282 165 | 0.174 331 408 300  |
| H                                                                 | 0.102 348 144 503  | -0.007 002 449 325 | 0.000 491 067 554  |
| H                                                                 | -0.097 085 646 041 | -0.046 796 852 670 | -0.105 794 243 340 |
| H                                                                 | -0.008 420 271 269 | 0.106 296 112 374  | -0.101 397 406 500 |
| H                                                                 | -0.129 333 985 134 | -0.096 074 821 636 | -0.073 727 963 583 |
| H                                                                 | 0.096 968 052 620  | 0.034 199 161 198  | 0.016 208 456 673  |
| H                                                                 | -0.042 568 275 754 | 0.031 028 165 060  | 0.059 838 198 100  |
| H                                                                 | -0.013 066 566 380 | -0.051 296 185 943 | 0.123 897 905 752  |
| H                                                                 | -0.081 905 258 005 | -0.050 025 658 927 | -0.123 969 038 056 |
| H                                                                 | -0.018 792 440 900 | -0.127 019 953 373 | -0.035 190 703 343 |
| H                                                                 | 0.136 917 057 659  | 0.160 717 697 610  | 0.119 533 556 604  |
| H                                                                 | 0.014 024 498 381  | 0.181 489 537 996  | 0.051 767 560 501  |
| H                                                                 | 0.121 315 246 784  | -0.017 330 750 830 | 0.012 001 622 180  |
| H                                                                 | -0.039 125 123 244 | 0.122 093 032 212  | -0.048 577 498 168 |
| H                                                                 | -0.067 055 778 793 | 0.040 927 432 455  | 0.037 162 066 175  |

Wavenumber/cm<sup>-1</sup>: 1267.9828

| $\frac{\partial \mu_{x,y,z}}{\partial Q_r} / (e u^{-0.5})$        | -0.000 446 321 527 | -0.004 959 042 463 | 0.005 182 898 536  |
|-------------------------------------------------------------------|--------------------|--------------------|--------------------|
| <i>l</i> -matrix coefficients/(u <sup>1/2</sup> Å <sup>-1</sup> ) |                    |                    |                    |
| O                                                                 | -0.021 018 141 571 | 0.045 388 859 532  | -0.006 538 835 686 |
| C                                                                 | 0.107 766 670 442  | 0.107 548 541 818  | -0.350 278 239 996 |
| C                                                                 | 0.274 398 049 631  | 0.149 012 483 776  | -0.255 649 238 720 |
| C                                                                 | 0.041 783 475 507  | -0.173 555 378 563 | 0.090 851 565 006  |
| C                                                                 | 0.002 609 664 954  | -0.068 385 148 076 | -0.078 745 925 152 |
| C                                                                 | -0.085 413 988 911 | -0.095 045 507 164 | 0.167 287 691 798  |
| C                                                                 | -0.151 286 701 440 | 0.047 808 252 992  | 0.015 604 962 711  |
| C                                                                 | 0.068 884 754 344  | 0.023 070 704 683  | 0.037 183 170 457  |
| C                                                                 | -0.075 263 504 165 | -0.053 648 268 501 | 0.122 031 739 362  |
| C                                                                 | -0.085 122 468 947 | -0.065 402 855 887 | 0.220 947 560 985  |
| C                                                                 | -0.131 059 012 490 | -0.073 102 375 184 | 0.080 437 406 406  |
| H                                                                 | 0.010 167 721 028  | -0.071 678 485 357 | 0.117 168 228 698  |
| H                                                                 | 0.066 368 266 970  | 0.100 884 480 694  | -0.033 180 655 807 |
| H                                                                 | -0.121 914 128 984 | -0.066 374 714 411 | -0.016 813 984 448 |
| H                                                                 | 0.031 603 606 606  | 0.020 914 989 518  | 0.068 254 452 392  |
| H                                                                 | -0.105 339 474 268 | 0.083 137 392 256  | 0.008 931 150 509  |
| H                                                                 | -0.013 881 117 856 | -0.228 670 601 511 | -0.130 426 592 548 |
| H                                                                 | -0.120 692 547 306 | 0.080 935 988 259  | 0.059 526 862 604  |
| H                                                                 | 0.312 229 364 795  | 0.226 313 944 564  | 0.104 807 675 788  |
| H                                                                 | 0.041 773 495 468  | -0.001 326 994 511 | 0.008 426 255 608  |
| H                                                                 | 0.020 750 339 461  | 0.227 386 221 264  | -0.031 674 242 744 |
| H                                                                 | 0.004 501 399 061  | 0.018 352 474 537  | -0.031 094 491 666 |
| H                                                                 | -0.045 445 781 062 | -0.043 585 843 567 | -0.112 307 029 718 |
| H                                                                 | 0.085 883 541 284  | 0.109 162 387 755  | -0.093 140 013 150 |
| H                                                                 | 0.053 083 473 929  | 0.001 591 729 838  | -0.051 373 094 591 |
| H                                                                 | 0.027 307 388 831  | -0.020 985 085 171 | -0.007 595 754 410 |
| H                                                                 | -0.049 767 221 273 | 0.079 372 438 316  | -0.004 919 848 042 |

Wavenumber/cm<sup>-1</sup>: 1274.3858

| $\frac{\partial \mu_{x,y,z}}{\partial Q_r} / (e u^{-0.5})$        | 0.005 750 529 749  | 0.001 838 937 101  | -0.008 128 919 173 |
|-------------------------------------------------------------------|--------------------|--------------------|--------------------|
| <i>l</i> -matrix coefficients/(u <sup>1/2</sup> Å <sup>-1</sup> ) |                    |                    |                    |
| O                                                                 | 0.028 795 175 031  | -0.035 771 167 306 | -0.029 862 409 850 |
| C                                                                 | -0.203 721 733 114 | 0.039 032 744 128  | -0.183 197 259 646 |
| C                                                                 | -0.054 648 327 991 | -0.075 673 388 991 | -0.164 107 745 860 |
| C                                                                 | -0.040 128 826 507 | 0.173 633 426 279  | 0.091 134 592 125  |
| C                                                                 | 0.046 499 087 620  | 0.095 539 842 436  | -0.000 406 694 517 |
| C                                                                 | -0.007 485 484 373 | -0.076 752 060 679 | 0.054 305 968 396  |
| C                                                                 | 0.057 822 950 059  | -0.033 044 189 311 | -0.080 551 016 219 |
| C                                                                 | -0.104 519 931 866 | 0.028 112 943 265  | 0.082 871 513 108  |
| C                                                                 | 0.146 623 614 655  | 0.024 777 393 052  | 0.075 286 432 486  |
| C                                                                 | 0.206 277 768 654  | -0.055 972 634 843 | 0.132 725 233 683  |
| C                                                                 | 0.053 464 288 763  | 0.005 978 177 632  | 0.174 396 671 777  |
| H                                                                 | -0.028 528 889 028 | 0.022 005 833 242  | -0.129 637 185 024 |
| H                                                                 | 0.091 781 989 609  | 0.219 855 976 961  | -0.004 153 644 312 |
| H                                                                 | 0.068 185 241 298  | 0.002 284 590 498  | -0.016 705 523 871 |
| H                                                                 | -0.016 910 716 010 | 0.006 388 617 314  | -0.012 838 014 323 |
| H                                                                 | 0.123 652 422 746  | -0.297 947 945 954 | 0.126 792 222 269  |
| H                                                                 | -0.142 546 744 447 | -0.087 461 340 418 | -0.076 760 514 720 |
| H                                                                 | -0.183 566 067 743 | 0.006 893 571 148  | 0.009 843 848 433  |
| H                                                                 | -0.225 438 036 897 | -0.144 118 099 498 | -0.049 397 800 428 |
| H                                                                 | -0.080 501 362 608 | -0.006 738 049 253 | -0.022 391 576 268 |
| H                                                                 | -0.092 717 050 726 | -0.065 007 239 497 | -0.138 446 279 431 |
| H                                                                 | -0.010 236 185 878 | -0.070 582 523 563 | 0.049 491 674 465  |
| H                                                                 | -0.051 096 301 188 | -0.038 779 261 923 | -0.304 012 280 492 |
| H                                                                 | 0.029 004 680 379  | 0.291 187 714 293  | 0.082 803 244 969  |
| H                                                                 | -0.055 887 232 588 | 0.014 073 680 370  | -0.080 416 163 306 |
| H                                                                 | -0.051 627 060 952 | -0.112 558 039 681 | 0.164 910 597 580  |
| H                                                                 | 0.165 877 744 889  | -0.030 662 539 129 | -0.109 949 013 202 |

Wavenumber/cm<sup>-1</sup>: 1300.3418

| $\frac{\partial \mu_{x,y,z}}{\partial Q_r} / (e u^{-0.5})$        | -0.013 265 188 277 | -0.007 521 967 336 | 0.013 468 201 452  |
|-------------------------------------------------------------------|--------------------|--------------------|--------------------|
| <i>l</i> -matrix coefficients/(u <sup>1/2</sup> Å <sup>-1</sup> ) |                    |                    |                    |
| O                                                                 | -0.005 818 413 078 | 0.008 712 006 114  | 0.053 393 238 372  |
| C                                                                 | 0.087 433 406 071  | -0.030 725 068 662 | -0.159 397 679 302 |
| C                                                                 | -0.069 480 832 001 | -0.023 962 840 202 | 0.082 049 906 528  |
| C                                                                 | -0.011 268 790 295 | -0.004 365 572 212 | -0.276 939 312 297 |
| C                                                                 | -0.115 932 085 099 | 0.019 050 439 377  | 0.021 914 746 836  |
| C                                                                 | -0.058 755 555 492 | 0.022 304 727 232  | 0.090 193 565 720  |
| C                                                                 | -0.002 208 837 570 | 0.018 799 127 122  | 0.140 157 222 773  |
| C                                                                 | 0.139 017 668 372  | -0.097 803 276 243 | -0.040 879 548 790 |
| C                                                                 | 0.066 427 053 636  | 0.038 561 392 286  | -0.010 790 206 146 |
| C                                                                 | -0.084 833 433 232 | -0.000 529 337 376 | 0.165 930 474 638  |
| C                                                                 | 0.019 748 906 507  | -0.022 433 607 931 | -0.042 528 004 762 |
| H                                                                 | -0.011 595 637 248 | 0.027 460 437 473  | -0.074 955 600 248 |
| H                                                                 | -0.030 500 134 407 | -0.121 851 637 124 | -0.029 960 487 738 |
| H                                                                 | 0.380 021 272 060  | 0.275 902 114 067  | 0.133 252 030 231  |
| H                                                                 | 0.138 723 734 870  | 0.238 090 695 340  | 0.035 695 875 731  |
| H                                                                 | -0.177 792 023 848 | -0.087 534 846 199 | 0.221 556 814 580  |
| H                                                                 | 0.011 261 112 909  | -0.156 476 406 600 | -0.088 586 261 254 |
| H                                                                 | 0.041 015 724 740  | -0.002 530 441 946 | -0.002 893 844 498 |
| H                                                                 | -0.184 693 785 814 | -0.112 732 718 935 | -0.058 469 919 793 |
| H                                                                 | -0.023 828 471 775 | 0.008 461 398 350  | -0.027 692 268 109 |
| H                                                                 | 0.043 701 407 989  | 0.212 126 205 249  | 0.009 592 668 650  |
| H                                                                 | -0.087 577 178 370 | 0.000 174 094 031  | -0.375 849 392 721 |
| H                                                                 | -0.030 587 105 756 | -0.051 404 111 447 | 0.156 992 252 503  |
| H                                                                 | 0.058 369 840 532  | 0.055 334 228 258  | -0.068 372 669 273 |
| H                                                                 | 0.031 916 642 574  | -0.007 857 980 155 | 0.001 800 455 789  |
| H                                                                 | -0.017 811 620 563 | -0.034 459 592 069 | 0.051 740 831 940  |
| H                                                                 | -0.014 392 472 654 | 0.002 558 818 704  | 0.007 983 089 009  |

Wavenumber/cm<sup>-1</sup>: 1326.86

| $\frac{\partial \mu_{x,y,z}}{\partial Q_r} / (e u^{-0.5})$        | 0.006 061 821 679  | -0.001 239 024 396 | 0.009 993 485 254  |
|-------------------------------------------------------------------|--------------------|--------------------|--------------------|
| <i>l</i> -matrix coefficients/(u <sup>1/2</sup> Å <sup>-1</sup> ) |                    |                    |                    |
| O                                                                 | 0.013 984 782 457  | 0.050 742 726 738  | 0.076 136 008 639  |
| C                                                                 | -0.106 305 593 289 | -0.116 646 664 105 | 0.019 113 860 601  |
| C                                                                 | 0.010 797 807 099  | -0.019 538 191 230 | 0.058 387 710 871  |
| C                                                                 | 0.073 138 033 300  | -0.233 281 021 440 | -0.428 196 115 488 |
| C                                                                 | -0.214 712 343 716 | 0.018 088 496 058  | -0.176 424 540 327 |
| C                                                                 | -0.205 430 841 136 | 0.017 673 409 124  | 0.017 993 106 243  |
| C                                                                 | 0.042 483 781 560  | 0.114 658 898 831  | 0.296 488 514 457  |
| C                                                                 | 0.198 777 960 362  | 0.051 954 401 987  | 0.054 434 306 246  |
| C                                                                 | 0.052 153 644 683  | -0.039 939 481 109 | -0.048 201 371 495 |
| C                                                                 | 0.127 152 322 475  | 0.064 988 741 021  | 0.036 915 445 161  |
| C                                                                 | 0.034 470 326 015  | -0.015 470 005 500 | 0.065 667 992 089  |
| H                                                                 | -0.001 370 604 098 | 0.070 921 445 074  | -0.067 252 395 334 |
| H                                                                 | 0.069 909 316 902  | 0.143 149 150 749  | -0.139 150 948 240 |
| H                                                                 | -0.047 350 068 327 | 0.120 181 396 405  | 0.089 996 172 236  |
| H                                                                 | -0.087 651 236 876 | -0.311 607 339 900 | 0.153 615 752 463  |
| H                                                                 | 0.078 298 811 156  | 0.014 691 873 615  | -0.201 282 304 927 |
| H                                                                 | -0.062 305 481 725 | 0.053 965 812 011  | 0.018 310 622 333  |
| H                                                                 | -0.080 191 924 700 | 0.012 085 905 210  | 0.008 338 609 572  |
| H                                                                 | 0.069 159 016 048  | 0.028 348 841 943  | -0.061 346 885 882 |
| H                                                                 | -0.016 772 456 521 | -0.030 187 813 481 | 0.060 246 458 134  |
| H                                                                 | -0.050 752 848 456 | -0.076 005 590 596 | -0.046 838 966 005 |
| H                                                                 | 0.073 022 699 648  | 0.198 947 103 245  | 0.152 048 221 948  |
| H                                                                 | -0.074 030 267 207 | -0.050 536 328 111 | 0.081 189 914 835  |
| H                                                                 | -0.010 914 191 909 | 0.155 532 289 188  | 0.080 440 625 661  |
| H                                                                 | -0.011 176 171 504 | 0.000 975 830 234  | -0.027 634 132 968 |
| H                                                                 | -0.021 140 116 611 | 0.025 883 177 497  | 0.004 872 010 623  |
| H                                                                 | 0.074 312 625 213  | -0.014 782 297 217 | -0.050 496 185 398 |



Wavenumber/cm<sup>-1</sup>: 1334.3922

| $\frac{\partial \mu_{x,y,z}}{\partial Q_r} / (e u^{-0.5})$        | 0.009 665 822 941  | 0.003 193 112 490  | -0.001 499 543 114 |
|-------------------------------------------------------------------|--------------------|--------------------|--------------------|
| <i>l</i> -matrix coefficients/(u <sup>1/2</sup> Å <sup>-1</sup> ) |                    |                    |                    |
| O                                                                 | 0.077 623 736 420  | -0.061 024 892 603 | -0.030 056 112 480 |
| C                                                                 | 0.045 788 642 967  | 0.192 259 693 275  | 0.020 227 288 895  |
| C                                                                 | 0.034 546 549 517  | 0.039 140 707 583  | -0.016 802 573 797 |
| C                                                                 | -0.100 489 924 319 | 0.425 480 374 000  | 0.148 863 372 883  |
| C                                                                 | -0.027 254 044 316 | 0.008 197 529 265  | -0.084 473 894 003 |
| C                                                                 | -0.165 499 619 357 | -0.010 876 092 112 | 0.040 497 461 688  |
| C                                                                 | -0.004 844 523 869 | -0.286 389 842 080 | -0.009 337 324 672 |
| C                                                                 | 0.156 274 481 512  | -0.079 112 290 094 | 0.030 604 059 466  |
| C                                                                 | -0.041 751 964 345 | -0.027 446 222 730 | 0.012 005 745 556  |
| C                                                                 | 0.185 400 427 385  | -0.194 574 328 448 | -0.090 747 380 214 |
| C                                                                 | -0.061 610 305 812 | -0.078 639 035 899 | -0.059 760 390 620 |
| H                                                                 | 0.010 564 055 064  | -0.018 352 012 764 | 0.053 374 555 229  |
| H                                                                 | 0.024 015 294 519  | 0.021 240 643 763  | -0.102 819 800 857 |
| H                                                                 | 0.041 342 085 932  | 0.117 373 734 290  | 0.035 267 635 847  |
| H                                                                 | 0.002 804 453 267  | -0.105 291 449 152 | 0.111 129 804 205  |
| H                                                                 | -0.278 504 428 906 | 0.270 541 575 092  | 0.050 405 317 396  |
| H                                                                 | -0.120 551 335 683 | 0.001 915 184 892  | -0.013 521 642 567 |
| H                                                                 | 0.032 489 120 296  | 0.051 001 307 961  | 0.032 446 271 549  |
| H                                                                 | 0.074 225 832 414  | -0.067 440 567 248 | -0.114 299 777 777 |
| H                                                                 | 0.021 889 555 002  | -0.006 202 916 938 | 0.025 894 560 536  |
| H                                                                 | -0.124 460 326 215 | -0.281 629 377 246 | -0.132 866 784 710 |
| H                                                                 | 0.000 891 480 248  | 0.117 803 407 535  | -0.053 398 029 590 |
| H                                                                 | -0.054 465 080 439 | -0.061 696 287 382 | 0.157 259 871 243  |
| H                                                                 | -0.030 555 344 995 | 0.143 905 379 497  | 0.091 788 484 617  |
| H                                                                 | 0.123 571 536 861  | -0.009 690 062 514 | -0.008 461 683 464 |
| H                                                                 | 0.017 962 933 965  | 0.034 861 584 546  | -0.043 410 272 438 |
| H                                                                 | -0.121 450 779 393 | 0.076 071 907 534  | 0.061 761 670 475  |

Wavenumber/cm<sup>-1</sup>: 1348.6642

| $\frac{\partial \mu_{x,y,z}}{\partial Q_r} / (e u^{-0.5})$        |                    |                    |                    |
|-------------------------------------------------------------------|--------------------|--------------------|--------------------|
|                                                                   | -0.006 438 099 265 | 0.003 657 144 866  | -0.026 119 079 429 |
| <i>l</i> -matrix coefficients/(u <sup>1/2</sup> Å <sup>-1</sup> ) |                    |                    |                    |
| O                                                                 | -0.011 969 916 289 | -0.036 363 679 909 | 0.011 952 922 161  |
| C                                                                 | 0.040 423 022 098  | 0.032 835 266 727  | -0.011 597 120 436 |
| C                                                                 | 0.024 927 527 752  | 0.024 329 215 281  | -0.061 310 983 455 |
| C                                                                 | -0.063 786 412 538 | 0.194 416 861 696  | -0.032 291 834 781 |
| C                                                                 | 0.170 142 019 757  | 0.066 326 745 437  | -0.257 860 965 003 |
| C                                                                 | 0.020 727 420 468  | -0.113 050 634 399 | 0.044 011 598 351  |
| C                                                                 | -0.084 352 217 350 | -0.143 190 914 170 | 0.064 385 979 382  |
| C                                                                 | 0.017 016 600 854  | 0.029 841 711 941  | 0.157 911 895 375  |
| C                                                                 | -0.122 394 283 415 | -0.217 239 734 739 | -0.081 016 157 815 |
| C                                                                 | -0.078 030 305 239 | -0.050 811 871 597 | 0.087 459 392 879  |
| C                                                                 | 0.065 196 906 556  | 0.203 482 187 126  | 0.127 901 239 331  |
| H                                                                 | 0.048 260 009 164  | 0.071 500 914 515  | 0.128 807 805 173  |
| H                                                                 | -0.030 596 865 272 | -0.072 410 989 016 | 0.052 855 001 914  |
| H                                                                 | -0.058 967 146 522 | 0.059 286 780 100  | 0.029 369 590 452  |
| H                                                                 | 0.021 589 801 823  | 0.091 530 725 008  | -0.041 805 231 166 |
| H                                                                 | 0.133 614 507 132  | 0.085 355 523 178  | -0.210 594 055 091 |
| H                                                                 | 0.010 510 380 027  | -0.141 651 353 897 | -0.083 205 855 618 |
| H                                                                 | -0.057 180 329 165 | -0.105 498 207 054 | -0.066 228 838 094 |
| H                                                                 | -0.143 017 778 443 | -0.131 256 531 542 | -0.106 807 589 318 |
| H                                                                 | 0.048 067 311 511  | -0.099 984 102 474 | 0.267 080 448 526  |
| H                                                                 | 0.037 987 157 913  | 0.146 575 850 345  | 0.006 489 108 644  |
| H                                                                 | 0.007 760 031 294  | -0.024 532 028 089 | 0.036 432 905 974  |
| H                                                                 | 0.063 603 926 499  | 0.052 831 602 576  | 0.156 951 821 746  |
| H                                                                 | 0.042 298 694 015  | 0.005 587 038 544  | -0.066 355 459 954 |
| H                                                                 | -0.297 188 368 087 | 0.027 438 021 351  | 0.046 582 305 949  |
| H                                                                 | 0.039 295 919 153  | 0.221 333 940 933  | -0.215 190 460 498 |
| H                                                                 | 0.216 619 464 751  | -0.134 223 737 629 | -0.111 773 397 698 |

Wavenumber/cm<sup>-1</sup>: 1409.2449

| $\frac{\partial \mu_{x,y,z}}{\partial Q_r} / (e u^{-0.5})$        | 0.010 205 735 992  | -0.002 728 024 423 | -0.001 931 375 414 |
|-------------------------------------------------------------------|--------------------|--------------------|--------------------|
| <i>l</i> -matrix coefficients/(u <sup>1/2</sup> Å <sup>-1</sup> ) |                    |                    |                    |
| O                                                                 | -0.000 268 341 459 | -0.001 650 609 033 | -0.011 893 497 886 |
| C                                                                 | -0.017 321 298 401 | 0.002 131 282 420  | 0.068 986 220 401  |
| C                                                                 | -0.047 828 567 519 | 0.014 164 099 218  | 0.019 262 740 234  |
| C                                                                 | 0.015 400 179 265  | -0.055 142 371 227 | 0.027 512 404 732  |
| C                                                                 | -0.212 478 986 077 | -0.069 817 348 007 | 0.307 082 186 311  |
| C                                                                 | 0.034 670 909 701  | 0.234 304 946 191  | 0.092 127 419 812  |
| C                                                                 | 0.211 210 724 623  | -0.009 387 822 632 | -0.090 726 121 555 |
| C                                                                 | -0.043 905 127 413 | -0.082 304 024 112 | -0.321 517 041 376 |
| C                                                                 | -0.098 110 662 465 | -0.137 538 539 993 | -0.121 322 709 416 |
| C                                                                 | 0.024 486 108 904  | -0.048 473 987 478 | 0.005 395 901 057  |
| C                                                                 | 0.115 641 006 662  | 0.135 945 802 270  | 0.053 501 975 640  |
| H                                                                 | 0.040 679 227 300  | 0.077 175 993 725  | 0.092 229 067 693  |
| H                                                                 | 0.080 009 140 735  | 0.140 276 373 678  | -0.051 336 087 413 |
| H                                                                 | 0.055 849 441 883  | -0.018 283 044 839 | -0.028 456 187 273 |
| H                                                                 | 0.006 045 878 633  | -0.053 207 161 305 | 0.090 542 206 247  |
| H                                                                 | -0.178 008 980 608 | -0.014 297 624 115 | 0.201 708 384 075  |
| H                                                                 | -0.026 376 263 021 | -0.022 803 819 967 | -0.013 496 081 567 |
| H                                                                 | 0.000 632 291 169  | -0.099 445 677 108 | -0.064 985 362 887 |
| H                                                                 | 0.206 637 497 659  | 0.086 735 038 964  | 0.032 676 478 471  |
| H                                                                 | 0.036 385 126 724  | -0.074 397 822 626 | 0.228 048 475 434  |
| H                                                                 | -0.022 749 292 749 | -0.038 381 719 082 | -0.023 200 574 340 |
| H                                                                 | -0.027 734 377 704 | 0.015 105 014 149  | -0.113 526 715 817 |
| H                                                                 | -0.097 100 478 563 | -0.083 854 161 683 | -0.207 844 861 768 |
| H                                                                 | -0.001 257 199 943 | 0.040 312 939 579  | 0.014 575 360 626  |
| H                                                                 | -0.225 512 517 181 | 0.009 852 139 843  | 0.045 481 593 586  |
| H                                                                 | 0.032 988 912 910  | 0.214 508 136 140  | -0.201 540 700 295 |
| H                                                                 | 0.183 530 034 245  | -0.117 079 531 529 | -0.092 615 485 729 |

Wavenumber/cm<sup>-1</sup>: 1415.4804

| $\frac{\partial \mu_{x,y,z}}{\partial Q_r} / (e u^{-0.5})$        | 0.001 045 949 683  | -0.000 306 417 176 | 0.001 278 116 995  |
|-------------------------------------------------------------------|--------------------|--------------------|--------------------|
| <i>l</i> -matrix coefficients/(u <sup>1/2</sup> Å <sup>-1</sup> ) |                    |                    |                    |
| O                                                                 | -0.014 005 516 652 | -0.006 680 756 821 | -0.019 376 679 928 |
| C                                                                 | -0.000 538 076 246 | 0.029 360 502 679  | -0.063 452 045 194 |
| C                                                                 | 0.306 490 461 701  | -0.130 378 707 367 | -0.068 564 579 311 |
| C                                                                 | -0.008 962 158 428 | 0.004 888 325 846  | 0.104 881 495 106  |
| C                                                                 | -0.056 167 677 039 | 0.025 019 534 662  | 0.041 037 441 600  |
| C                                                                 | -0.072 004 777 426 | -0.111 457 200 742 | -0.067 610 817 992 |
| C                                                                 | 0.008 884 513 209  | 0.048 340 563 573  | -0.094 706 118 393 |
| C                                                                 | 0.067 474 759 826  | 0.091 372 506 240  | 0.046 889 322 987  |
| C                                                                 | 0.274 994 782 829  | -0.153 855 718 004 | -0.057 192 450 994 |
| C                                                                 | -0.042 087 396 759 | 0.042 416 358 419  | -0.065 639 775 800 |
| C                                                                 | -0.280 071 100 669 | 0.128 462 837 909  | 0.079 627 863 004  |
| H                                                                 | -0.045 702 753 709 | 0.324 101 579 139  | -0.365 210 055 642 |
| H                                                                 | -0.030 319 475 388 | -0.059 212 945 771 | -0.021 394 715 480 |
| H                                                                 | 0.103 899 773 158  | -0.035 578 851 259 | -0.021 444 196 446 |
| H                                                                 | -0.022 139 798 853 | -0.052 141 384 461 | -0.011 479 963 676 |
| H                                                                 | -0.120 590 195 586 | 0.072 077 577 399  | 0.072 082 139 609  |
| H                                                                 | 0.050 367 071 092  | 0.079 517 316 145  | 0.056 922 713 772  |
| H                                                                 | 0.026 866 343 976  | -0.042 693 885 131 | 0.005 280 875 976  |
| H                                                                 | -0.004 496 969 860 | 0.038 243 615 703  | 0.088 873 060 945  |
| H                                                                 | -0.182 108 346 956 | -0.143 319 579 228 | 0.302 653 284 939  |
| H                                                                 | 0.024 543 594 234  | -0.005 276 696 472 | 0.041 625 601 170  |
| H                                                                 | 0.015 938 901 562  | 0.045 122 557 058  | 0.010 833 900 119  |
| H                                                                 | 0.003 924 433 222  | 0.020 923 812 061  | 0.038 977 782 557  |
| H                                                                 | -0.012 343 745 580 | -0.119 718 561 256 | -0.019 442 225 034 |
| H                                                                 | -0.171 693 905 159 | 0.013 347 768 459  | 0.122 127 385 082  |
| H                                                                 | -0.151 448 347 885 | 0.003 811 835 075  | 0.192 230 075 784  |
| H                                                                 | -0.112 435 886 733 | -0.023 419 358 460 | 0.084 166 741 757  |

Wavenumber/cm<sup>-1</sup>: 1430.6761

| $\frac{\partial \mu_{x,y,z}}{\partial Q_r} / (e u^{-0.5})$        | -0.006 038 194 994 | -0.000 252 852 280 | -0.003 626 276 120 |
|-------------------------------------------------------------------|--------------------|--------------------|--------------------|
| <i>l</i> -matrix coefficients/(u <sup>1/2</sup> Å <sup>-1</sup> ) |                    |                    |                    |
| O                                                                 | -0.011 815 941 379 | -0.019 548 382 208 | -0.019 421 914 681 |
| C                                                                 | -0.021 391 705 991 | 0.022 761 191 371  | -0.054 720 464 007 |
| C                                                                 | 0.070 953 404 769  | -0.222 862 374 909 | 0.221 502 258 689  |
| C                                                                 | -0.024 197 621 957 | 0.043 247 945 201  | 0.067 404 260 871  |
| C                                                                 | -0.112 326 485 573 | 0.049 233 635 935  | 0.047 951 162 168  |
| C                                                                 | -0.059 825 605 925 | -0.184 112 745 361 | -0.101 080 267 343 |
| C                                                                 | 0.119 252 474 339  | -0.031 785 697 691 | -0.073 742 796 913 |
| C                                                                 | 0.035 901 342 029  | 0.207 434 796 743  | 0.069 427 984 662  |
| C                                                                 | -0.023 226 456 493 | 0.137 604 035 272  | -0.258 426 094 431 |
| C                                                                 | -0.070 047 805 583 | 0.048 657 209 741  | -0.032 889 818 822 |
| C                                                                 | 0.039 872 669 162  | -0.164 946 373 294 | 0.249 596 871 593  |
| H                                                                 | 0.027 505 490 364  | 0.005 211 000 489  | 0.003 584 782 816  |
| H                                                                 | -0.061 718 813 488 | -0.125 437 720 958 | 0.001 187 230 767  |
| H                                                                 | 0.111 741 807 876  | 0.033 423 581 523  | -0.003 625 928 511 |
| H                                                                 | -0.032 722 290 934 | -0.028 005 327 436 | -0.059 098 257 272 |
| H                                                                 | -0.163 002 713 022 | 0.082 275 949 953  | 0.098 573 122 484  |
| H                                                                 | 0.059 540 271 127  | 0.037 500 157 379  | 0.030 384 803 539  |
| H                                                                 | -0.440 414 246 324 | 0.160 458 490 464  | 0.090 090 206 287  |
| H                                                                 | 0.066 560 493 407  | 0.013 912 435 960  | 0.001 524 663 543  |
| H                                                                 | 0.062 500 780 174  | 0.049 177 672 654  | -0.063 380 058 879 |
| H                                                                 | 0.047 149 031 621  | 0.060 714 863 959  | 0.051 487 941 782  |
| H                                                                 | 0.038 966 080 878  | 0.000 133 997 758  | 0.073 305 611 147  |
| H                                                                 | 0.069 932 471 083  | 0.092 247 845 593  | -0.012 133 032 035 |
| H                                                                 | 0.000 606 613 717  | -0.124 136 091 821 | -0.041 683 029 457 |
| H                                                                 | 0.157 261 521 281  | 0.009 799 865 183  | -0.215 521 045 311 |
| H                                                                 | 0.052 224 440 424  | 0.091 097 016 432  | -0.154 609 289 517 |
| H                                                                 | 0.206 407 446 720  | 0.046 647 289 120  | -0.188 806 526 504 |

Wavenumber/cm<sup>-1</sup>: 1461.7038

| $\frac{\partial \mu_{x,y,z}}{\partial Q_r} / (e u^{-0.5})$        | 0.003 426 847 323  | -0.003 654 029 300 | -0.001 421 954 054 |
|-------------------------------------------------------------------|--------------------|--------------------|--------------------|
| <i>l</i> -matrix coefficients/(u <sup>1/2</sup> Å <sup>-1</sup> ) |                    |                    |                    |
| O                                                                 | -0.018 985 406 532 | 0.019 286 683 624  | 0.005 769 368 471  |
| C                                                                 | 0.015 193 854 766  | -0.005 839 897 230 | 0.083 237 110 623  |
| C                                                                 | 0.106 388 321 731  | -0.190 702 369 828 | 0.109 244 310 782  |
| C                                                                 | 0.027 049 384 755  | -0.072 068 603 156 | 0.024 062 392 534  |
| C                                                                 | 0.262 674 438 431  | 0.125 471 530 270  | 0.026 496 127 040  |
| C                                                                 | 0.031 785 897 804  | 0.354 759 371 217  | 0.017 624 435 499  |
| C                                                                 | -0.241 348 897 192 | 0.107 671 403 049  | 0.004 860 679 165  |
| C                                                                 | -0.079 483 680 681 | -0.357 427 719 409 | -0.089 794 827 607 |
| C                                                                 | 0.054 698 557 861  | 0.031 143 042 430  | -0.200 670 089 021 |
| C                                                                 | 0.013 862 234 075  | -0.054 280 506 512 | 0.010 205 857 347  |
| C                                                                 | -0.108 468 544 285 | -0.099 441 771 409 | 0.112 326 907 728  |
| H                                                                 | 0.006 641 596 584  | 0.110 639 830 140  | -0.103 956 754 314 |
| H                                                                 | 0.105 525 753 608  | 0.146 393 199 578  | -0.135 576 384 838 |
| H                                                                 | -0.101 233 017 131 | -0.122 399 762 216 | -0.026 679 114 635 |
| H                                                                 | 0.121 465 092 397  | 0.088 412 239 090  | 0.111 563 866 716  |
| H                                                                 | 0.120 547 043 992  | 0.178 031 619 290  | -0.140 148 321 032 |
| H                                                                 | -0.025 038 299 613 | -0.033 170 874 262 | -0.018 298 044 091 |
| H                                                                 | -0.204 142 961 242 | 0.112 434 637 812  | 0.073 440 442 886  |
| H                                                                 | -0.197 494 454 777 | -0.012 341 725 902 | 0.095 503 839 040  |
| H                                                                 | -0.011 740 790 232 | -0.018 827 952 838 | 0.073 546 197 002  |
| H                                                                 | -0.016 635 292 961 | -0.029 205 324 706 | -0.016 556 892 825 |
| H                                                                 | -0.078 223 629 604 | -0.045 442 934 928 | -0.164 550 775 404 |
| H                                                                 | -0.039 631 426 194 | -0.104 040 218 106 | 0.066 596 192 131  |
| H                                                                 | -0.000 482 215 717 | 0.032 514 122 683  | 0.010 477 567 793  |
| H                                                                 | 0.141 031 368 658  | 0.006 723 306 820  | -0.092 886 226 786 |
| H                                                                 | -0.012 633 857 494 | 0.088 271 294 639  | -0.063 870 455 629 |
| H                                                                 | -0.016 591 640 758 | 0.079 955 898 732  | -0.028 479 685 941 |

Wavenumber/cm<sup>-1</sup>: 1485.9241

| $\frac{\partial \mu_{x,y,z}}{\partial Q_r} / (e u^{-0.5})$        | 0.002 702 869 029  | -0.002 291 266 609 | -0.010 838 251 825 |
|-------------------------------------------------------------------|--------------------|--------------------|--------------------|
| <i>l</i> -matrix coefficients/(u <sup>1/2</sup> Å <sup>-1</sup> ) |                    |                    |                    |
| O                                                                 | 0.012 249 691 022  | 0.047 725 399 012  | -0.032 783 017 957 |
| C                                                                 | 0.078 981 833 013  | 0.040 072 197 820  | -0.149 933 940 793 |
| C                                                                 | -0.067 029 156 457 | 0.095 351 500 204  | 0.002 633 279 443  |
| C                                                                 | 0.048 157 933 044  | -0.143 349 464 983 | 0.226 937 246 653  |
| C                                                                 | 0.106 449 827 420  | -0.115 168 486 402 | 0.015 256 127 466  |
| C                                                                 | -0.242 763 251 989 | -0.131 801 451 816 | -0.062 802 629 768 |
| C                                                                 | -0.236 000 657 559 | 0.264 803 343 670  | -0.148 312 046 316 |
| C                                                                 | 0.206 322 621 554  | 0.014 282 610 716  | 0.094 478 515 959  |
| C                                                                 | -0.090 478 242 253 | -0.003 859 086 117 | 0.033 186 366 984  |
| C                                                                 | 0.084 299 855 185  | 0.035 824 033 279  | -0.097 880 356 260 |
| C                                                                 | 0.114 453 416 184  | 0.060 154 435 981  | 0.016 531 738 247  |
| H                                                                 | 0.022 208 253 643  | -0.072 503 854 766 | 0.129 393 606 749  |
| H                                                                 | -0.009 468 416 972 | -0.098 138 872 061 | -0.165 240 823 840 |
| H                                                                 | 0.153 927 170 222  | -0.166 348 002 064 | -0.051 744 965 803 |
| H                                                                 | 0.034 725 116 879  | -0.120 057 760 657 | 0.115 326 146 080  |
| H                                                                 | 0.033 462 630 552  | -0.191 549 723 452 | 0.120 216 929 930  |
| H                                                                 | -0.017 606 229 824 | 0.149 270 387 718  | 0.086 957 809 116  |
| H                                                                 | -0.010 003 351 716 | -0.051 055 895 234 | -0.040 926 942 247 |
| H                                                                 | -0.223 969 616 755 | 0.059 755 836 151  | 0.234 781 225 036  |
| H                                                                 | 0.044 198 660 645  | 0.015 098 465 441  | -0.015 946 286 101 |
| H                                                                 | -0.054 672 990 408 | -0.173 910 756 454 | -0.022 861 481 071 |
| H                                                                 | -0.021 071 315 586 | 0.115 355 333 394  | -0.161 998 994 500 |
| H                                                                 | -0.034 221 161 904 | -0.028 191 364 821 | 0.233 390 245 364  |
| H                                                                 | -0.036 704 138 532 | 0.005 877 295 361  | 0.055 957 834 601  |
| H                                                                 | -0.122 170 019 304 | 0.002 526 645 043  | 0.008 999 207 625  |
| H                                                                 | 0.044 942 396 406  | 0.030 936 265 710  | -0.072 705 488 878 |
| H                                                                 | 0.139 354 604 998  | -0.068 704 533 801 | -0.081 674 661 901 |

Wavenumber/cm<sup>-1</sup>: 1489.0039

| $\frac{\partial \mu_{x,y,z}}{\partial Q_r} / (e u^{-0.5})$        |                    |                    |                    |
|-------------------------------------------------------------------|--------------------|--------------------|--------------------|
|                                                                   | -0.002 802 575 548 | 0.000 361 597 689  | 0.003 090 487 920  |
| <i>l</i> -matrix coefficients/(u <sup>1/2</sup> Å <sup>-1</sup> ) |                    |                    |                    |
| O                                                                 | 0.068 346 241 024  | 0.007 325 539 579  | 0.015 922 772 394  |
| C                                                                 | 0.042 362 093 337  | 0.087 109 857 349  | -0.151 315 098 529 |
| C                                                                 | 0.112 277 388 444  | 0.020 935 925 253  | 0.107 625 355 546  |
| C                                                                 | -0.018 380 495 267 | 0.164 985 202 478  | -0.017 390 811 012 |
| C                                                                 | -0.057 144 337 337 | -0.340 246 965 104 | -0.216 998 864 844 |
| C                                                                 | 0.078 353 002 993  | 0.064 168 847 106  | 0.450 724 418 466  |
| C                                                                 | -0.178 056 352 844 | -0.062 942 270 920 | 0.167 017 670 371  |
| C                                                                 | -0.035 370 197 950 | 0.041 636 097 100  | -0.261 900 914 470 |
| C                                                                 | 0.068 902 578 121  | 0.086 903 330 439  | -0.010 020 812 832 |
| C                                                                 | -0.024 535 584 365 | -0.013 381 919 741 | -0.175 703 599 850 |
| C                                                                 | -0.029 742 113 630 | 0.061 066 152 220  | 0.110 717 619 517  |
| H                                                                 | -0.017 565 544 413 | -0.004 395 623 226 | -0.078 853 608 200 |
| H                                                                 | 0.021 903 191 246  | -0.058 321 979 142 | 0.086 000 404 121  |
| H                                                                 | -0.121 518 735 887 | 0.064 205 575 790  | 0.052 519 581 755  |
| H                                                                 | 0.035 131 599 219  | 0.026 874 624 555  | 0.138 177 972 112  |
| H                                                                 | 0.032 128 550 429  | -0.147 065 478 875 | -0.079 971 692 011 |
| H                                                                 | 0.059 388 036 907  | 0.188 947 795 427  | 0.139 271 243 238  |
| H                                                                 | -0.114 891 818 274 | -0.005 815 088 775 | -0.001 401 753 745 |
| H                                                                 | 0.043 910 633 013  | 0.007 737 569 327  | -0.053 983 124 740 |
| H                                                                 | -0.017 431 521 520 | 0.040 149 176 367  | -0.119 003 356 377 |
| H                                                                 | 0.000 868 095 300  | -0.142 932 926 950 | 0.043 814 899 679  |
| H                                                                 | -0.013 566 840 876 | -0.070 974 016 086 | -0.126 966 175 040 |
| H                                                                 | 0.035 012 807 415  | 0.035 298 571 807  | -0.073 088 676 374 |
| H                                                                 | -0.047 268 282 101 | -0.214 554 141 769 | 0.002 638 583 548  |
| H                                                                 | -0.118 970 004 644 | 0.014 211 750 923  | -0.010 146 751 610 |
| H                                                                 | -0.019 124 609 295 | -0.095 090 502 129 | 0.086 581 435 547  |
| H                                                                 | 0.112 381 832 864  | -0.047 987 484 090 | -0.078 536 659 956 |



Wavenumber/cm<sup>-1</sup>: 1492.8433

| $\frac{\partial \mu_{x,y,z}}{\partial Q_r} / (e u^{-0.5})$    |                    |                    |                    |
|---------------------------------------------------------------|--------------------|--------------------|--------------------|
| $-6.004\,759\,065\,680 \times 10^{-5} - 0.003\,588\,460\,658$ |                    |                    |                    |
| $-0.003\,417\,378\,998$                                       |                    |                    |                    |
| $l$ -matrix coefficients/(u <sup>1/2</sup> Å <sup>-1</sup> )  |                    |                    |                    |
| O                                                             | -0.030 605 323 663 | 0.008 721 709 111  | -0.036 467 705 833 |
| C                                                             | -0.067 057 973 712 | 0.089 958 336 292  | -0.271 057 396 175 |
| C                                                             | -0.056 495 051 187 | -0.010 488 041 303 | -0.022 605 500 585 |
| C                                                             | 0.010 814 091 702  | -0.125 550 584 891 | 0.068 934 299 049  |
| C                                                             | -0.136 168 553 942 | 0.226 263 175 328  | -0.176 741 917 787 |
| C                                                             | 0.166 456 470 217  | -0.060 454 764 060 | 0.300 345 349 409  |
| C                                                             | 0.167 279 116 769  | 0.094 162 894 305  | -0.116 560 428 114 |
| C                                                             | -0.076 032 700 886 | -0.342 234 816 976 | 0.227 192 700 140  |
| C                                                             | -0.035 343 553 767 | -0.035 575 240 818 | 0.033 683 933 900  |
| C                                                             | -0.018 604 372 247 | 0.105 342 144 197  | -0.090 249 405 838 |
| C                                                             | 0.065 570 225 751  | -0.020 179 576 943 | -0.037 788 609 430 |
| H                                                             | 0.011 776 340 882  | -0.026 583 865 767 | 0.062 998 515 761  |
| H                                                             | 0.032 750 898 144  | 0.163 050 522 231  | 0.226 805 831 754  |
| H                                                             | 0.268 668 065 098  | 0.045 166 598 761  | -0.002 863 396 712 |
| H                                                             | -0.083 741 227 905 | 0.041 279 357 722  | -0.057 021 668 844 |
| H                                                             | -0.071 237 654 091 | 0.187 510 872 875  | -0.111 893 283 048 |
| H                                                             | 0.064 342 676 965  | 0.190 524 914 933  | 0.133 710 961 639  |
| H                                                             | 0.030 605 854 754  | -0.006 679 754 705 | -0.010 198 783 519 |
| H                                                             | -0.060 327 818 623 | -0.013 337 441 935 | 0.032 489 856 053  |
| H                                                             | 0.017 825 659 935  | -0.009 757 422 510 | 0.028 596 990 265  |
| H                                                             | 0.015 818 331 736  | -0.056 181 999 810 | 0.056 328 653 188  |
| H                                                             | -0.032 215 822 696 | 0.063 005 548 184  | 0.121 392 871 823  |
| H                                                             | -0.173 575 732 479 | -0.192 236 562 783 | -0.004 954 164 148 |
| H                                                             | -0.029 392 500 574 | -0.157 470 353 288 | 0.005 368 565 207  |
| H                                                             | 0.029 930 946 657  | -0.006 049 795 061 | -0.009 336 093 578 |
| H                                                             | 0.019 220 669 102  | 0.018 131 994 510  | -0.030 402 562 779 |
| H                                                             | 0.011 003 845 985  | -0.003 254 685 141 | -0.002 841 826 005 |

Wavenumber/cm<sup>-1</sup>: 1497.9724

| $\frac{\partial \mu_{x,y,z}}{\partial Q_r} / (e u^{-0.5})$        | 0.004 836 324 931  | -0.004 613 106 037 | -0.011 939 798 593 |
|-------------------------------------------------------------------|--------------------|--------------------|--------------------|
| <i>l</i> -matrix coefficients/(u <sup>1/2</sup> Å <sup>-1</sup> ) |                    |                    |                    |
| O                                                                 | -0.119 469 829 441 | -0.004 301 532 590 | 0.040 995 598 989  |
| C                                                                 | 0.098 130 636 049  | 0.081 392 220 764  | -0.240 814 035 472 |
| C                                                                 | -0.085 056 141 929 | -0.097 290 891 158 | -0.113 103 401 514 |
| C                                                                 | -0.045 752 490 372 | -0.094 141 749 526 | -0.188 412 647 992 |
| C                                                                 | 0.270 985 205 295  | 0.350 680 257 086  | 0.329 573 669 824  |
| C                                                                 | -0.082 856 763 625 | -0.239 025 152 280 | 0.194 166 906 630  |
| C                                                                 | 0.004 406 486 298  | -0.035 700 971 994 | 0.169 748 612 998  |
| C                                                                 | 0.026 586 157 225  | 0.141 197 645 180  | -0.126 371 130 686 |
| C                                                                 | -0.043 260 092 776 | -0.106 807 011 295 | 0.019 445 306 224  |
| C                                                                 | 0.049 418 506 814  | 0.062 721 529 331  | -0.082 213 781 921 |
| C                                                                 | -0.024 176 706 039 | -0.049 614 984 924 | -0.050 262 929 402 |
| H                                                                 | 0.022 330 055 870  | 0.025 579 537 983  | 0.072 616 756 094  |
| H                                                                 | -0.050 273 108 968 | -0.146 274 649 601 | 0.052 425 245 893  |
| H                                                                 | -0.195 933 119 025 | 0.049 751 563 074  | 0.033 266 829 567  |
| H                                                                 | -0.021 666 971 132 | -0.049 383 452 974 | 0.046 129 652 527  |
| H                                                                 | 0.127 211 858 222  | 0.033 679 029 535  | 0.099 485 212 816  |
| H                                                                 | 0.008 248 489 074  | 0.169 463 188 636  | 0.109 697 463 362  |
| H                                                                 | 0.032 119 312 071  | 0.033 788 852 102  | 0.018 662 071 928  |
| H                                                                 | -0.037 501 352 958 | -0.062 838 955 846 | -0.095 412 764 306 |
| H                                                                 | 0.023 444 421 176  | -0.051 271 045 592 | 0.149 506 294 561  |
| H                                                                 | -0.041 767 399 786 | -0.140 162 093 692 | -0.001 852 336 721 |
| H                                                                 | -0.014 405 113 101 | -0.060 025 289 804 | -0.154 258 059 280 |
| H                                                                 | 0.030 480 839 317  | 0.040 083 850 634  | -0.182 766 912 718 |
| H                                                                 | -0.038 620 385 655 | -0.029 760 661 919 | 0.048 364 712 683  |
| H                                                                 | 0.118 358 520 576  | -0.003 196 338 105 | -0.018 646 219 795 |
| H                                                                 | 0.024 115 227 403  | 0.103 666 127 657  | -0.087 448 103 648 |
| H                                                                 | -0.091 563 247 774 | 0.057 743 835 925  | 0.051 515 128 286  |

Wavenumber/cm<sup>-1</sup>: 1503.8381

| $\frac{\partial \mu_{x,y,z}}{\partial Q_r} / (e u^{-0.5})$        | 0.001 440 410 551  | 0.000 435 960 769  | 0.008 486 902 557  |
|-------------------------------------------------------------------|--------------------|--------------------|--------------------|
| <i>l</i> -matrix coefficients/(u <sup>1/2</sup> Å <sup>-1</sup> ) |                    |                    |                    |
| O                                                                 | -0.138 153 144 231 | -0.028 521 501 889 | 0.013 895 670 901  |
| C                                                                 | 0.275 875 599 880  | -0.067 977 486 818 | -0.040 425 994 102 |
| C                                                                 | -0.016 969 243 542 | -0.039 370 417 233 | -0.046 662 653 936 |
| C                                                                 | -0.081 057 372 167 | -0.073 091 445 958 | -0.032 204 399 145 |
| C                                                                 | -0.116 047 968 370 | -0.002 357 547 461 | -0.139 136 143 176 |
| C                                                                 | -0.093 698 752 177 | 0.104 801 464 579  | 0.059 938 952 143  |
| C                                                                 | 0.227 816 673 781  | 0.114 277 330 354  | -0.061 450 721 278 |
| C                                                                 | -0.265 838 264 168 | -0.021 454 489 070 | 0.162 759 976 670  |
| C                                                                 | -0.011 762 646 092 | -0.040 620 209 148 | 0.032 669 545 306  |
| C                                                                 | 0.123 873 893 584  | 0.046 440 311 786  | 0.010 111 873 151  |
| C                                                                 | -0.066 756 665 582 | 0.027 176 286 969  | 0.002 774 338 551  |
| H                                                                 | 0.004 242 879 893  | -0.003 876 046 222 | 0.024 813 917 085  |
| H                                                                 | 0.019 371 981 842  | -0.199 442 735 666 | -0.204 357 989 389 |
| H                                                                 | 0.157 959 987 244  | 0.025 973 701 811  | -0.007 048 671 175 |
| H                                                                 | 0.245 235 746 464  | 0.143 631 806 388  | 0.190 391 028 616  |
| H                                                                 | 0.006 066 233 150  | 0.024 703 202 172  | -0.099 535 330 423 |
| H                                                                 | -0.066 072 612 462 | 0.074 564 806 515  | 0.034 358 769 097  |
| H                                                                 | -0.009 665 894 917 | 0.001 909 264 730  | 0.001 193 741 050  |
| H                                                                 | 0.120 891 245 992  | 0.075 780 249 177  | 0.040 927 992 516  |
| H                                                                 | 0.000 624 863 921  | -0.014 722 858 816 | 0.028 595 303 444  |
| H                                                                 | -0.086 986 303 802 | -0.161 166 340 099 | -0.057 692 316 369 |
| H                                                                 | 0.006 847 291 956  | -0.398 052 948 117 | 0.105 677 317 368  |
| H                                                                 | 0.288 254 621 897  | 0.192 442 149 731  | -0.002 389 742 334 |
| H                                                                 | -0.021 567 121 243 | 0.162 833 742 435  | 0.086 010 983 835  |
| H                                                                 | -0.018 251 189 137 | 0.008 877 273 935  | -0.007 532 404 752 |
| H                                                                 | 0.008 453 711 025  | 0.010 259 503 761  | -0.012 946 969 241 |
| H                                                                 | -0.020 195 218 823 | 0.004 830 293 750  | 0.002 382 244 648  |

Wavenumber/cm<sup>-1</sup>: 1513.8816

| $\frac{\partial \mu_{x,y,z}}{\partial Q_r} / (e u^{-0.5})$        | 0.002 531 326 781  | -0.000 908 923 773 | 0.000 702 006 349  |
|-------------------------------------------------------------------|--------------------|--------------------|--------------------|
| <i>l</i> -matrix coefficients/(u <sup>1/2</sup> Å <sup>-1</sup> ) |                    |                    |                    |
| O                                                                 | 0.179 242 903 733  | 0.036 402 336 716  | -0.042 770 858 571 |
| C                                                                 | -0.477 449 539 151 | 0.133 766 027 700  | -0.088 619 904 005 |
| C                                                                 | 0.081 567 281 327  | 0.161 127 217 933  | 0.096 154 006 860  |
| C                                                                 | 0.163 278 188 393  | -0.062 086 741 597 | -0.039 583 853 009 |
| C                                                                 | 0.076 628 730 144  | 0.120 842 637 449  | 0.089 428 564 847  |
| C                                                                 | -0.222 057 926 923 | 0.045 861 073 499  | 0.010 757 632 820  |
| C                                                                 | 0.090 801 219 063  | -0.183 904 297 063 | -0.112 849 318 720 |
| C                                                                 | -0.066 606 899 748 | -0.052 730 868 317 | 0.082 796 938 699  |
| C                                                                 | -0.003 906 200 439 | -0.041 091 956 017 | 0.141 917 802 356  |
| C                                                                 | -0.126 172 411 341 | -0.028 924 163 881 | -0.046 543 345 154 |
| C                                                                 | 0.115 710 715 243  | 0.011 205 249 682  | -0.043 308 307 468 |
| H                                                                 | -0.016 338 844 504 | -0.038 694 902 176 | 0.015 180 952 683  |
| H                                                                 | 0.101 430 743 090  | -0.009 659 994 335 | -0.306 578 767 509 |
| H                                                                 | -0.034 730 610 748 | -0.003 382 975 306 | -0.033 936 505 854 |
| H                                                                 | 0.156 277 421 810  | -0.113 968 696 676 | 0.263 620 616 229  |
| H                                                                 | -0.014 163 051 701 | 0.106 957 971 198  | 0.010 628 466 324  |
| H                                                                 | 0.081 424 575 342  | 0.000 456 537 742  | 0.021 571 194 231  |
| H                                                                 | 0.048 156 152 963  | -0.019 010 720 862 | -0.021 725 981 194 |
| H                                                                 | -0.020 954 954 909 | -0.098 191 051 772 | -0.113 919 594 134 |
| H                                                                 | -0.008 026 731 326 | -0.000 798 069 805 | -0.025 897 891 727 |
| H                                                                 | 0.090 773 928 229  | 0.126 885 810 978  | 0.079 447 475 978  |
| H                                                                 | -0.003 228 611 935 | -0.187 810 337 859 | -0.013 862 673 210 |
| H                                                                 | 0.134 267 564 449  | 0.069 059 648 623  | 0.010 974 346 056  |
| H                                                                 | 0.008 402 999 342  | -0.234 110 867 882 | -0.081 595 237 503 |
| H                                                                 | -0.007 990 009 083 | -0.001 718 030 690 | -0.001 322 617 848 |
| H                                                                 | -0.021 938 415 251 | -0.076 030 308 496 | 0.089 377 148 372  |
| H                                                                 | 0.063 563 092 290  | -0.024 241 481 456 | -0.032 755 316 226 |

Wavenumber/cm<sup>-1</sup>: 1518.8964

| $\frac{\partial \mu_{x,y,z}}{\partial Q_r} / (e u^{-0.5})$        | 0.002 970 910 708  | -0.004 216 914 370 | -0.013 442 627 651 |
|-------------------------------------------------------------------|--------------------|--------------------|--------------------|
| <i>l</i> -matrix coefficients/(u <sup>1/2</sup> Å <sup>-1</sup> ) |                    |                    |                    |
| O                                                                 | -0.279 162 843 456 | -0.080 892 469 801 | -0.007 656 796 733 |
| C                                                                 | 0.070 716 761 822  | 0.057 298 001 982  | -0.193 950 383 300 |
| C                                                                 | 0.173 617 050 786  | 0.348 497 081 019  | 0.241 492 731 904  |
| C                                                                 | -0.178 370 343 757 | -0.095 281 655 964 | -0.042 006 654 611 |
| C                                                                 | 0.254 429 906 177  | -0.065 052 179 467 | 0.205 244 810 708  |
| C                                                                 | -0.016 597 667 135 | -0.031 037 532 592 | -0.264 052 257 872 |
| C                                                                 | 0.198 937 755 606  | -0.019 907 828 285 | 0.088 917 798 151  |
| C                                                                 | -0.046 409 880 320 | -0.225 559 409 328 | 0.080 867 716 617  |
| C                                                                 | 0.054 903 465 111  | 0.094 797 208 815  | -0.041 993 825 129 |
| C                                                                 | -0.003 204 719 339 | -0.063 878 367 929 | -0.061 325 975 452 |
| C                                                                 | -0.100 418 437 012 | 0.087 528 726 553  | 0.103 964 557 176  |
| H                                                                 | -0.009 482 630 362 | -0.036 495 390 891 | -0.054 993 317 712 |
| H                                                                 | -0.023 434 348 932 | 0.045 941 527 883  | -0.012 118 252 701 |
| H                                                                 | -0.053 295 843 691 | 0.162 848 797 300  | 0.039 375 659 172  |
| H                                                                 | -0.036 882 167 750 | 0.048 786 390 587  | -0.137 429 448 648 |
| H                                                                 | 0.085 832 578 919  | 0.048 500 446 149  | 0.000 495 900 022  |
| H                                                                 | -0.035 872 953 073 | 0.025 996 643 386  | 0.014 005 159 676  |
| H                                                                 | -0.084 871 070 228 | -0.042 016 622 824 | -0.016 547 985 252 |
| H                                                                 | 0.165 422 247 778  | 0.011 256 719 501  | -0.143 534 440 988 |
| H                                                                 | 0.017 379 284 128  | 0.055 610 174 281  | -0.162 112 472 521 |
| H                                                                 | -0.052 717 418 805 | -0.104 786 235 656 | -0.037 005 543 205 |
| H                                                                 | -0.044 084 968 265 | 0.030 359 121 422  | -0.017 706 001 225 |
| H                                                                 | -0.073 404 464 607 | -0.093 213 970 486 | 0.093 178 969 694  |
| H                                                                 | -0.025 682 109 467 | 0.014 932 642 251  | 0.015 289 012 656  |
| H                                                                 | -0.202 012 333 571 | 0.008 302 584 496  | 0.047 079 478 943  |
| H                                                                 | -0.017 909 923 620 | -0.088 807 249 688 | 0.071 371 667 427  |
| H                                                                 | 0.096 182 009 096  | -0.066 650 679 006 | -0.073 272 162 644 |

Wavenumber/cm<sup>-1</sup>: 1527.0376

| $\frac{\partial \mu_{x,y,z}}{\partial Q_r} / (e u^{-0.5})$        | 0.002 421 361 132  | 0.001 198 026 077  | 0.010 569 693 054  |
|-------------------------------------------------------------------|--------------------|--------------------|--------------------|
| <i>l</i> -matrix coefficients/(u <sup>1/2</sup> Å <sup>-1</sup> ) |                    |                    |                    |
| O                                                                 | 0.065 278 814 784  | 0.102 748 214 018  | 0.105 301 325 837  |
| C                                                                 | 0.049 102 461 663  | 0.062 946 531 953  | 0.125 121 775 597  |
| C                                                                 | -0.067 649 515 393 | 0.093 866 953 973  | -0.041 175 486 304 |
| C                                                                 | 0.103 926 445 100  | -0.077 576 798 688 | -0.201 035 245 725 |
| C                                                                 | 0.092 442 056 609  | -0.165 172 051 099 | 0.012 714 015 274  |
| C                                                                 | -0.061 000 762 332 | -0.146 410 556 113 | 0.191 938 722 553  |
| C                                                                 | 0.064 046 027 649  | -0.346 059 584 755 | -0.327 961 900 020 |
| C                                                                 | -0.028 826 030 593 | -0.137 176 946 177 | 0.079 897 312 445  |
| C                                                                 | 0.013 391 659 717  | 0.161 009 272 839  | -0.238 875 955 829 |
| C                                                                 | 0.075 407 215 630  | 0.377 463 682 342  | 0.162 244 010 169  |
| C                                                                 | -0.229 751 471 771 | 0.059 427 758 540  | 0.097 847 847 242  |
| H                                                                 | 0.016 231 780 519  | 0.016 442 560 380  | -0.042 343 105 897 |
| H                                                                 | -0.021 637 206 355 | -0.064 321 291 485 | 0.050 421 775 088  |
| H                                                                 | -0.044 704 894 251 | -0.173 145 459 089 | -0.117 245 334 194 |
| H                                                                 | -0.023 915 942 675 | -0.076 170 812 628 | 0.070 165 347 559  |
| H                                                                 | -0.009 470 799 225 | -0.060 608 491 974 | 0.047 803 608 878  |
| H                                                                 | -0.005 109 992 789 | 0.092 989 732 746  | 0.024 876 796 939  |
| H                                                                 | -0.019 578 942 612 | -0.001 761 317 819 | 0.029 532 740 923  |
| H                                                                 | 0.014 530 424 830  | -0.094 257 136 414 | -0.052 868 328 048 |
| H                                                                 | 0.023 408 514 968  | 0.055 257 764 231  | -0.094 399 699 446 |
| H                                                                 | -0.000 200 715 665 | 0.105 111 919 221  | 0.021 227 329 101  |
| H                                                                 | -0.037 485 559 809 | 0.003 474 947 973  | -0.039 221 069 694 |
| H                                                                 | -0.056 331 887 468 | -0.063 914 134 423 | 0.066 929 714 623  |
| H                                                                 | 0.013 510 975 109  | 0.173 465 296 622  | 0.060 611 777 855  |
| H                                                                 | -0.070 950 566 225 | 0.012 795 620 723  | 0.062 184 156 341  |
| H                                                                 | 0.021 173 682 149  | 0.047 792 880 582  | -0.086 856 459 508 |
| H                                                                 | -0.097 820 759 165 | 0.023 726 032 130  | 0.060 460 798 481  |

Wavenumber/cm<sup>-1</sup>: 1815.4509

| $\frac{\partial \mu_{x,y,z}}{\partial Q_r} / (e u^{-0.5})$        | 0.008 031 038 831  | -0.003 016 826 617 | -0.006 027 018 372 |
|-------------------------------------------------------------------|--------------------|--------------------|--------------------|
| <i>l</i> -matrix coefficients/(u <sup>1/2</sup> Å <sup>-1</sup> ) |                    |                    |                    |
| O                                                                 | -0.041 409 175 017 | -0.190 760 275 520 | 0.068 054 333 992  |
| C                                                                 | -0.092 907 858 457 | -0.138 447 966 137 | 0.108 363 137 986  |
| C                                                                 | 0.069 683 408 224  | 0.117 253 866 386  | 0.029 851 616 668  |
| C                                                                 | -0.160 635 632 618 | 0.308 675 594 591  | -0.393 206 848 664 |
| C                                                                 | 0.118 161 321 021  | 0.128 355 177 092  | 0.061 443 479 036  |
| C                                                                 | -0.065 307 740 558 | -0.104 954 275 808 | 0.280 279 125 763  |
| C                                                                 | 0.088 590 924 516  | 0.169 766 864 766  | -0.093 930 270 311 |
| C                                                                 | 0.016 227 468 390  | 0.021 270 782 245  | 0.129 954 886 968  |
| C                                                                 | -0.004 495 273 768 | 0.100 131 437 035  | -0.113 551 435 270 |
| C                                                                 | -0.054 971 043 498 | -0.247 721 754 292 | -0.096 719 616 921 |
| C                                                                 | 0.102 861 467 382  | -0.022 795 466 515 | -0.026 832 836 272 |
| H                                                                 | -0.018 899 020 574 | 0.023 348 231 721  | -0.074 550 356 093 |
| H                                                                 | -0.016 233 510 747 | -0.018 312 628 927 | 0.082 664 675 398  |
| H                                                                 | 0.063 891 624 800  | -0.310 571 422 913 | -0.081 708 240 952 |
| H                                                                 | -0.026 449 447 189 | -0.016 139 460 695 | 0.068 349 435 664  |
| H                                                                 | 0.024 628 391 366  | 0.030 817 643 675  | 0.033 803 878 217  |
| H                                                                 | -0.016 751 530 203 | -0.127 986 052 989 | -0.078 810 505 158 |
| H                                                                 | 0.053 821 079 696  | -0.031 874 467 737 | -0.016 702 358 653 |
| H                                                                 | 0.096 022 922 446  | 0.171 290 468 703  | 0.327 977 321 456  |
| H                                                                 | -0.027 703 435 812 | 0.033 263 530 790  | -0.079 652 159 084 |
| H                                                                 | -0.000 914 652 862 | -0.015 928 816 094 | -0.042 117 100 455 |
| H                                                                 | -0.013 333 424 017 | 0.002 241 955 493  | -0.017 848 867 675 |
| H                                                                 | -0.013 865 918 733 | -0.005 496 229 983 | 0.023 122 164 899  |
| H                                                                 | -0.003 120 977 114 | -0.047 737 080 052 | -0.045 931 772 984 |
| H                                                                 | -0.010 084 756 359 | -0.013 779 678 779 | 0.016 337 244 102  |
| H                                                                 | -0.022 032 292 598 | -0.031 825 695 827 | 0.015 537 899 789  |
| H                                                                 | 0.036 604 021 413  | -0.025 756 323 194 | -0.006 875 328 857 |

Wavenumber/cm<sup>-1</sup>: 3031.0741

| $\frac{\partial \mu_{x,y,z}}{\partial Q_r} / (e u^{-0.5})$        |                    |                    |                    |
|-------------------------------------------------------------------|--------------------|--------------------|--------------------|
|                                                                   | -0.021 896 717 676 | 0.000 955 568 189  | 0.005 039 228 180  |
| <i>l</i> -matrix coefficients/(u <sup>1/2</sup> Å <sup>-1</sup> ) |                    |                    |                    |
| O                                                                 | -0.042 577 145 551 | 0.007 292 676 595  | 0.151 968 483 170  |
| C                                                                 | 0.106 654 889 511  | 0.177 097 812 823  | -0.084 984 945 882 |
| C                                                                 | 0.211 934 803 908  | -0.111 207 407 128 | 0.112 576 935 102  |
| C                                                                 | -0.095 127 022 905 | 0.231 461 009 691  | -0.234 375 417 556 |
| C                                                                 | -0.118 911 210 782 | -0.138 160 176 433 | 0.076 261 001 928  |
| C                                                                 | -0.078 773 427 624 | -0.043 534 030 520 | -0.203 432 459 974 |
| C                                                                 | -0.182 352 636 733 | -0.056 235 995 227 | -0.025 761 748 027 |
| C                                                                 | -0.121 893 760 708 | -0.224 079 552 663 | -0.027 962 178 929 |
| C                                                                 | -0.048 136 138 091 | -0.101 545 786 530 | 0.246 863 989 835  |
| C                                                                 | 0.079 644 083 863  | 0.312 403 862 958  | 0.100 225 343 737  |
| C                                                                 | 0.339 314 842 301  | -0.062 794 669 369 | -0.161 043 453 003 |
| H                                                                 | -0.033 605 432 357 | 0.054 856 652 896  | 0.010 901 613 983  |
| H                                                                 | -0.063 268 273 801 | -0.012 444 468 098 | 0.010 232 092 884  |
| H                                                                 | -0.114 583 150 685 | -0.143 617 488 901 | -0.036 406 060 629 |
| H                                                                 | -0.064 510 381 596 | 0.019 811 193 315  | -0.114 036 478 977 |
| H                                                                 | -0.068 998 153 073 | 0.044 104 011 015  | -0.005 320 209 814 |
| H                                                                 | 0.028 498 048 344  | 0.117 485 796 047  | 0.053 941 156 978  |
| H                                                                 | 0.019 317 417 369  | 0.015 781 511 259  | -0.046 339 826 944 |
| H                                                                 | 0.011 401 897 202  | 0.042 047 264 089  | 0.090 862 167 841  |
| H                                                                 | -0.071 971 229 015 | -0.050 551 074 060 | 0.135 422 818 182  |
| H                                                                 | 0.014 975 986 974  | 0.068 906 449 685  | 0.030 726 494 931  |
| H                                                                 | -0.022 791 103 866 | -0.079 348 524 580 | 0.025 827 931 842  |
| H                                                                 | -0.003 423 315 881 | -0.047 257 305 854 | -0.009 799 578 750 |
| H                                                                 | 0.015 608 140 232  | 0.074 320 256 275  | 0.038 160 986 906  |
| H                                                                 | 0.098 454 284 746  | -0.010 654 548 840 | -0.098 831 946 796 |
| H                                                                 | -0.043 091 073 725 | -0.033 519 642 006 | 0.103 717 293 469  |
| H                                                                 | 0.148 811 308 405  | -0.031 689 284 921 | -0.098 479 836 003 |



Wavenumber/cm<sup>-1</sup>: 3035.3466

| $\frac{\partial \mu_{x,y,z}}{\partial Q_r} / (e u^{-0.5})$        |                    |                    |                    |
|-------------------------------------------------------------------|--------------------|--------------------|--------------------|
|                                                                   | -0.005 988 320 665 | -0.005 317 229 106 | -0.006 832 957 323 |
| <i>l</i> -matrix coefficients/(u <sup>1/2</sup> Å <sup>-1</sup> ) |                    |                    |                    |
| O                                                                 | 0.373 646 161 182  | 0.094 754 008 350  | 0.010 248 976 451  |
| C                                                                 | 0.056 494 596 702  | -0.023 807 485 693 | -0.142 393 032 836 |
| C                                                                 | -0.089 705 936 768 | 0.055 053 085 712  | -0.134 160 206 602 |
| C                                                                 | 0.232 349 697 828  | 0.187 730 835 724  | -0.007 479 340 828 |
| C                                                                 | -0.235 863 634 473 | -0.030 995 690 571 | 0.255 645 917 881  |
| C                                                                 | -0.087 453 672 367 | -0.165 240 432 471 | -0.099 801 974 567 |
| C                                                                 | -0.163 233 456 991 | 0.192 038 978 575  | 0.225 424 331 913  |
| C                                                                 | -0.121 556 702 878 | -0.306 077 884 560 | 0.190 178 188 875  |
| C                                                                 | 0.060 657 611 053  | 0.158 383 359 654  | -0.239 755 068 194 |
| C                                                                 | 0.008 872 760 755  | -0.103 110 077 304 | -0.083 280 038 347 |
| C                                                                 | -0.060 698 798 670 | -0.023 004 868 529 | 0.037 382 840 653  |
| H                                                                 | 0.031 415 965 400  | 0.046 318 869 887  | -0.038 252 743 275 |
| H                                                                 | -0.041 965 943 292 | -0.032 901 600 273 | 0.008 382 228 395  |
| H                                                                 | -0.165 996 939 683 | 0.077 201 504 501  | 0.053 107 432 923  |
| H                                                                 | -0.025 868 281 024 | 0.011 796 319 697  | -0.063 527 375 438 |
| H                                                                 | -0.013 897 102 027 | -0.029 835 061 100 | 0.032 549 363 101  |
| H                                                                 | 0.002 843 477 485  | -0.030 845 447 852 | -0.025 663 868 669 |
| H                                                                 | 0.060 170 774 611  | -0.054 212 280 615 | 0.002 298 295 982  |
| H                                                                 | -0.013 916 768 139 | 0.050 759 913 768  | -0.028 535 591 374 |
| H                                                                 | 0.041 020 878 088  | 0.042 456 474 906  | -0.026 555 601 310 |
| H                                                                 | 0.010 666 015 534  | -0.022 322 505 777 | -0.018 728 776 516 |
| H                                                                 | 0.009 241 557 481  | -0.195 738 833 280 | 0.140 060 993 569  |
| H                                                                 | 0.067 361 225 410  | -0.041 422 505 453 | -0.034 661 139 671 |
| H                                                                 | 0.010 658 193 315  | -0.035 688 134 450 | -0.035 917 514 865 |
| H                                                                 | -0.076 243 656 735 | -0.018 426 210 083 | 0.051 765 422 055  |
| H                                                                 | 0.033 755 669 564  | 0.101 729 890 438  | -0.109 720 033 060 |
| H                                                                 | -0.036 613 770 392 | -0.042 606 836 393 | 0.046 485 093 556  |

Wavenumber/cm<sup>-1</sup>: 3037.1754

| $\frac{\partial \mu_{x,y,z}}{\partial Q_r} / (e u^{-0.5})$        | 0.009 268 105 813  | -0.001 785 888 356 | -0.015 632 479 610 |
|-------------------------------------------------------------------|--------------------|--------------------|--------------------|
| <i>l</i> -matrix coefficients/(u <sup>1/2</sup> Å <sup>-1</sup> ) |                    |                    |                    |
| O                                                                 | -0.106 509 251 129 | -0.324 670 644 423 | -0.238 723 784 179 |
| C                                                                 | -0.233 202 975 879 | 0.167 891 058 612  | 0.092 235 124 664  |
| C                                                                 | -0.069 104 689 493 | -0.154 342 244 374 | -0.189 474 923 468 |
| C                                                                 | -0.200 494 620 373 | 0.132 073 518 272  | 0.137 804 697 676  |
| C                                                                 | 0.171 475 011 894  | -0.258 557 733 220 | -0.002 676 885 427 |
| C                                                                 | -0.042 200 034 264 | -0.080 882 769 147 | 0.040 245 910 645  |
| C                                                                 | 0.121 319 317 849  | 0.240 536 803 251  | 0.128 740 558 533  |
| C                                                                 | -0.045 669 713 719 | -0.109 145 619 163 | 0.040 135 468 072  |
| C                                                                 | 0.023 292 801 953  | 0.084 601 932 945  | -0.107 308 473 466 |
| C                                                                 | 0.081 530 483 129  | 0.226 563 568 934  | 0.085 231 421 540  |
| C                                                                 | 0.107 049 693 254  | -0.005 329 447 078 | 0.000 536 665 723  |
| H                                                                 | 0.015 009 280 311  | 0.066 245 321 777  | -0.021 227 813 240 |
| H                                                                 | 0.045 307 030 263  | -0.026 781 737 422 | -0.092 837 082 739 |
| H                                                                 | 0.007 505 664 473  | 0.192 762 372 357  | 0.054 630 493 765  |
| H                                                                 | 0.047 555 234 873  | -0.099 731 306 207 | 0.105 042 182 505  |
| H                                                                 | 0.113 369 968 112  | -0.137 985 590 265 | -0.018 196 070 367 |
| H                                                                 | 0.080 334 169 899  | 0.035 606 219 913  | 0.010 670 765 021  |
| H                                                                 | 0.097 595 938 085  | 0.025 798 163 405  | 0.028 037 804 610  |
| H                                                                 | 0.166 790 933 836  | 0.117 813 566 481  | -0.056 264 418 823 |
| H                                                                 | 0.011 769 043 095  | 0.008 341 142 278  | 0.064 431 292 474  |
| H                                                                 | 0.097 721 622 371  | 0.171 138 267 567  | 0.062 003 416 725  |
| H                                                                 | -0.040 176 774 999 | 0.023 372 519 537  | -0.042 090 203 604 |
| H                                                                 | -0.054 857 175 926 | -0.049 031 817 088 | 0.077 133 002 314  |
| H                                                                 | 0.054 561 792 643  | -0.031 145 776 487 | -0.020 691 903 244 |
| H                                                                 | 0.124 953 172 551  | 0.005 346 312 074  | 0.010 848 975 752  |
| H                                                                 | 0.015 045 440 184  | 0.100 830 623 804  | -0.072 113 728 659 |
| H                                                                 | -0.061 257 223 848 | 0.050 691 856 706  | 0.083 401 105 765  |

Wavenumber/cm<sup>-1</sup>: 3053.7413

| $\frac{\partial \mu_{x,y,z}}{\partial Q_r} / (e u^{-0.5})$        |                    |                    |                    |
|-------------------------------------------------------------------|--------------------|--------------------|--------------------|
|                                                                   | -0.023 086 948 488 | 0.012 668 274 155  | 0.048 371 306 224  |
| <i>l</i> -matrix coefficients/(u <sup>1/2</sup> Å <sup>-1</sup> ) |                    |                    |                    |
| O                                                                 | -0.261 821 409 836 | 0.103 922 136 819  | 0.026 835 925 703  |
| C                                                                 | 0.048 880 550 839  | -0.046 957 401 493 | 0.140 857 381 625  |
| C                                                                 | 0.258 652 370 985  | 0.136 714 753 571  | -0.151 362 389 281 |
| C                                                                 | -0.118 371 476 313 | -0.192 276 815 555 | 0.227 054 258 878  |
| C                                                                 | -0.090 983 647 817 | 0.105 103 936 352  | 0.029 719 167 515  |
| C                                                                 | 0.090 149 116 629  | -0.083 767 633 181 | 0.149 577 908 708  |
| C                                                                 | -0.182 160 751 125 | -0.104 484 678 543 | 0.034 983 582 556  |
| C                                                                 | 0.071 137 635 360  | 0.008 227 784 332  | 0.056 120 015 532  |
| C                                                                 | -0.099 833 660 273 | 0.216 900 746 761  | -0.304 755 746 089 |
| C                                                                 | -0.034 242 596 752 | 0.025 419 599 430  | 0.007 673 220 110  |
| C                                                                 | 0.367 469 548 712  | -0.157 553 542 284 | -0.126 236 359 113 |
| H                                                                 | -0.075 079 397 232 | 0.112 717 991 692  | -0.200 389 029 625 |
| H                                                                 | 0.055 601 711 107  | -0.035 477 086 677 | -0.014 764 981 047 |
| H                                                                 | -0.053 981 987 724 | 0.086 786 449 975  | 0.029 380 759 984  |
| H                                                                 | 0.059 972 783 669  | -0.063 156 970 397 | 0.093 117 518 674  |
| H                                                                 | -0.074 752 173 666 | 0.059 539 124 066  | 0.036 031 874 532  |
| H                                                                 | -0.046 644 572 424 | -0.020 815 801 758 | -0.031 351 988 365 |
| H                                                                 | 0.168 348 311 929  | -0.112 320 021 667 | -0.060 690 002 485 |
| H                                                                 | -0.087 722 834 815 | -0.072 708 776 343 | -0.091 788 181 747 |
| H                                                                 | -0.082 914 181 680 | 0.052 077 553 355  | -0.076 412 877 243 |
| H                                                                 | -0.027 244 105 825 | -0.002 569 183 174 | -0.015 816 059 843 |
| H                                                                 | 0.047 654 689 994  | -0.059 974 236 488 | 0.062 498 690 761  |
| H                                                                 | 0.061 863 826 519  | 0.017 933 157 195  | -0.058 016 098 621 |
| H                                                                 | -0.008 183 074 082 | 0.075 122 046 645  | 0.001 566 263 583  |
| H                                                                 | 0.022 309 842 410  | -0.062 707 798 853 | 0.025 094 334 135  |
| H                                                                 | -0.101 634 666 672 | 0.010 305 082 235  | 0.005 403 539 298  |
| H                                                                 | 0.113 002 569 788  | -0.078 879 260 797 | -0.030 433 426 370 |

Wavenumber/cm<sup>-1</sup>: 3059.8415

| $\frac{\partial \mu_{x,y,z}}{\partial Q_r} / (e u^{-0.5})$        | -0.011 265 102 919 | -0.017 006 290 551 | 0.058 726 145 153  |
|-------------------------------------------------------------------|--------------------|--------------------|--------------------|
| <i>l</i> -matrix coefficients/(u <sup>1/2</sup> Å <sup>-1</sup> ) |                    |                    |                    |
| O                                                                 | 0.042 348 480 922  | 0.173 608 161 694  | 0.115 426 750 367  |
| C                                                                 | 0.052 426 697 808  | -0.146 761 137 542 | -0.064 867 865 394 |
| C                                                                 | 0.075 482 693 840  | -0.180 260 737 744 | -0.062 975 813 068 |
| C                                                                 | 0.078 480 408 420  | -0.016 842 866 567 | -0.090 977 772 668 |
| C                                                                 | 0.087 501 800 497  | -0.184 211 628 048 | 0.093 886 117 992  |
| C                                                                 | -0.041 513 274 608 | 0.110 260 347 439  | 0.103 184 689 283  |
| C                                                                 | 0.009 423 238 476  | 0.126 545 805 696  | -0.337 827 942 377 |
| C                                                                 | -0.259 755 584 048 | 0.180 914 256 785  | 0.265 549 460 199  |
| C                                                                 | -0.029 116 563 883 | 0.024 066 973 168  | 0.052 862 861 084  |
| C                                                                 | -0.051 098 832 171 | -0.198 551 373 071 | -0.016 353 527 136 |
| C                                                                 | 0.145 738 196 412  | -0.037 429 773 997 | -0.061 638 028 682 |
| H                                                                 | -0.023 189 476 936 | 0.063 377 283 556  | -0.026 982 725 915 |
| H                                                                 | -0.018 663 483 439 | 0.000 395 323 293  | 0.021 605 142 563  |
| H                                                                 | -0.180 427 860 716 | 0.210 435 824 075  | -0.093 405 025 846 |
| H                                                                 | 0.032 809 351 816  | 0.111 448 292 356  | 0.026 991 835 101  |
| H                                                                 | 0.021 053 527 758  | -0.088 893 718 158 | 0.057 513 711 904  |
| H                                                                 | -0.028 213 114 082 | -0.025 253 750 379 | 0.021 400 547 226  |
| H                                                                 | 0.012 376 070 744  | 0.011 841 698 523  | -0.013 956 551 113 |
| H                                                                 | 0.090 572 882 973  | 0.027 772 514 418  | -0.323 376 968 116 |
| H                                                                 | -0.016 534 946 772 | -0.010 588 474 086 | 0.102 776 850 931  |
| H                                                                 | -0.026 592 279 447 | -0.100 668 205 796 | 0.005 360 982 780  |
| H                                                                 | -0.128 348 497 697 | 0.210 467 084 458  | -0.004 617 427 667 |
| H                                                                 | -0.207 692 650 871 | -0.009 484 468 580 | 0.202 540 042 906  |
| H                                                                 | -0.019 435 006 221 | -0.058 353 966 004 | 0.000 935 264 411  |
| H                                                                 | 0.094 756 364 330  | -0.006 014 376 904 | -0.024 822 373 886 |
| H                                                                 | -0.034 124 397 432 | 0.057 663 091 457  | 0.018 524 182 882  |
| H                                                                 | 0.029 687 583 708  | 0.026 657 675 188  | -0.019 026 266 242 |

Wavenumber/cm<sup>-1</sup>: 3060.5191

| $\frac{\partial \mu_{x,y,z}}{\partial Q_r} / (e u^{-0.5})$        |                    |                    |                    |
|-------------------------------------------------------------------|--------------------|--------------------|--------------------|
|                                                                   | -0.025 400 090 472 | 0.006 276 986 242  | 0.011 562 157 500  |
| <i>l</i> -matrix coefficients/(u <sup>1/2</sup> Å <sup>-1</sup> ) |                    |                    |                    |
| O                                                                 | -0.124 076 971 503 | 0.014 409 756 379  | 0.093 625 492 736  |
| C                                                                 | -0.054 491 983 873 | 0.105 018 493 081  | -0.083 008 633 160 |
| C                                                                 | -0.001 960 589 042 | 0.035 095 150 727  | -0.045 905 433 519 |
| C                                                                 | -0.116 713 215 817 | 0.072 540 766 781  | -0.075 606 128 745 |
| C                                                                 | -0.086 074 397 468 | 0.076 077 162 652  | -0.054 656 690 381 |
| C                                                                 | -0.038 395 291 092 | 0.137 151 325 697  | -0.084 642 364 478 |
| C                                                                 | -0.122 751 003 526 | 0.047 820 584 544  | -0.103 667 588 555 |
| C                                                                 | -0.095 056 782 630 | 0.138 892 492 060  | -0.040 817 359 961 |
| C                                                                 | 0.390 972 540 168  | -0.191 459 954 515 | -0.127 430 562 977 |
| C                                                                 | 0.025 114 911 905  | 0.045 228 377 288  | 0.078 229 306 184  |
| C                                                                 | 0.102 433 806 160  | -0.354 137 445 800 | 0.339 427 918 398  |
| H                                                                 | 0.131 268 661 105  | -0.194 952 398 623 | 0.033 987 594 726  |
| H                                                                 | -0.004 609 901 233 | 0.031 600 746 304  | -0.042 020 419 502 |
| H                                                                 | -0.039 770 064 877 | -0.009 242 837 047 | -0.032 946 264 181 |
| H                                                                 | 0.011 785 484 215  | 0.047 830 375 713  | -0.009 361 450 373 |
| H                                                                 | -0.045 935 302 437 | 0.040 365 937 804  | -0.008 088 765 834 |
| H                                                                 | 0.023 607 980 589  | 0.051 513 851 098  | 0.061 055 412 431  |
| H                                                                 | 0.158 756 181 244  | -0.222 146 523 512 | 0.058 246 103 043  |
| H                                                                 | -0.032 324 421 185 | 0.019 752 076 405  | -0.015 169 051 961 |
| H                                                                 | 0.235 627 123 087  | -0.022 589 140 512 | -0.106 980 080 477 |
| H                                                                 | 0.017 834 369 363  | -0.000 625 139 161 | 0.045 263 003 542  |
| H                                                                 | -0.026 141 971 145 | 0.043 492 477 499  | -0.009 309 663 956 |
| H                                                                 | -0.034 165 610 189 | 0.038 370 722 166  | -0.000 440 750 594 |
| H                                                                 | 0.007 104 667 151  | -0.042 641 795 983 | 0.021 311 432 661  |
| H                                                                 | -0.027 786 376 979 | -0.129 154 810 308 | 0.238 756 375 120  |
| H                                                                 | 0.130 752 488 717  | -0.011 451 757 518 | -0.073 175 572 015 |
| H                                                                 | -0.022 295 914 942 | -0.084 936 798 674 | 0.149 620 694 173  |

Wavenumber/cm<sup>-1</sup>: 3080.2581

| $\frac{\partial \mu_{x,y,z}}{\partial Q_r} / (e u^{-0.5})$        |                    |                    |                    |
|-------------------------------------------------------------------|--------------------|--------------------|--------------------|
|                                                                   | -0.021 644 090 706 | 0.010 377 967 905  | 0.027 793 562 785  |
| <i>l</i> -matrix coefficients/(u <sup>1/2</sup> Å <sup>-1</sup> ) |                    |                    |                    |
| O                                                                 | 0.172 805 514 301  | -0.093 272 667 762 | -0.176 767 100 006 |
| C                                                                 | 0.119 177 325 699  | -0.009 734 531 321 | 0.286 132 047 366  |
| C                                                                 | 0.086 580 692 769  | 0.063 742 392 734  | 0.210 013 640 140  |
| C                                                                 | 0.109 479 129 257  | 0.036 374 668 399  | 0.097 114 966 847  |
| C                                                                 | -0.001 873 420 084 | 0.184 250 110 254  | 0.019 953 164 908  |
| C                                                                 | -0.048 933 807 192 | -0.201 418 146 022 | 0.161 134 052 416  |
| C                                                                 | -0.052 259 745 464 | 0.278 728 808 560  | -0.092 767 590 230 |
| C                                                                 | -0.182 865 275 901 | -0.007 873 621 329 | -0.094 747 623 107 |
| C                                                                 | 0.003 678 744 031  | -0.294 419 330 911 | 0.011 599 332 908  |
| C                                                                 | 0.008 080 016 926  | 0.201 700 851 481  | -0.096 724 594 789 |
| C                                                                 | -0.089 313 869 538 | -0.102 721 395 617 | -0.096 368 175 036 |
| H                                                                 | -0.050 103 370 479 | -0.203 950 896 335 | -0.078 425 626 811 |
| H                                                                 | -0.034 530 590 732 | -0.132 616 295 418 | 0.036 634 849 184  |
| H                                                                 | -0.053 111 759 699 | 0.173 850 912 334  | -0.014 474 148 513 |
| H                                                                 | -0.008 831 907 338 | -0.079 280 369 699 | 0.063 510 427 905  |
| H                                                                 | -0.011 110 004 680 | 0.111 955 252 986  | -0.027 636 377 342 |
| H                                                                 | -0.040 369 693 997 | -0.039 018 839 680 | -0.125 977 480 969 |
| H                                                                 | -0.109 419 098 682 | -0.087 363 962 241 | -0.075 485 683 713 |
| H                                                                 | -0.010 041 775 421 | 0.055 705 585 257  | -0.137 934 335 818 |
| H                                                                 | 0.088 973 927 844  | -0.052 520 795 881 | -0.101 072 862 795 |
| H                                                                 | -0.009 996 006 377 | 0.106 178 394 111  | -0.074 163 718 376 |
| H                                                                 | -0.073 777 343 735 | 0.041 992 481 573  | -0.068 804 630 678 |
| H                                                                 | -0.109 508 194 366 | -0.035 915 710 822 | -0.044 370 533 105 |
| H                                                                 | 0.010 165 950 869  | 0.183 001 543 224  | -0.036 619 107 317 |
| H                                                                 | -0.084 612 562 995 | -0.041 414 582 840 | 0.014 459 094 677  |
| H                                                                 | -0.086 619 848 243 | -0.118 509 952 510 | 0.103 841 849 999  |
| H                                                                 | 0.060 980 136 399  | -0.023 554 378 479 | -0.128 451 055 848 |

Wavenumber/cm<sup>-1</sup>: 3081.8711

| $\frac{\partial \mu_{x,y,z}}{\partial Q_r} / (e u^{-0.5})$        |                    |                    |                    |
|-------------------------------------------------------------------|--------------------|--------------------|--------------------|
|                                                                   | -0.009 666 882 712 | -0.003 516 244 078 | -0.015 352 724 855 |
| <i>l</i> -matrix coefficients/(u <sup>1/2</sup> Å <sup>-1</sup> ) |                    |                    |                    |
| O                                                                 | -0.244 575 330 463 | 0.238 904 237 107  | 0.350 189 697 579  |
| C                                                                 | -0.114 957 944 794 | -0.031 522 377 604 | 0.002 899 336 167  |
| C                                                                 | -0.114 655 056 568 | -0.033 700 383 643 | 0.035 926 037 282  |
| C                                                                 | -0.171 031 563 358 | 0.084 929 801 244  | -0.000 923 090 963 |
| C                                                                 | -0.090 673 923 044 | -0.041 517 208 404 | 0.051 651 548 843  |
| C                                                                 | 0.354 446 234 974  | -0.203 830 196 875 | -0.023 950 133 828 |
| C                                                                 | -0.095 248 039 863 | 0.066 368 765 304  | -0.062 604 257 622 |
| C                                                                 | 0.072 190 343 610  | -0.082 670 037 251 | 0.042 301 963 515  |
| C                                                                 | 0.162 734 772 026  | -0.082 798 897 964 | 0.028 722 899 252  |
| C                                                                 | 0.234 046 468 747  | -0.037 364 266 362 | -0.187 742 167 452 |
| C                                                                 | -0.156 976 677 496 | 0.129 131 224 678  | -0.168 042 927 716 |
| H                                                                 | 0.040 816 410 044  | -0.106 600 864 506 | 0.014 879 941 439  |
| H                                                                 | 0.181 635 434 932  | -0.076 052 084 623 | -0.158 039 826 249 |
| H                                                                 | -0.053 964 149 724 | 0.024 808 167 430  | -0.019 467 102 660 |
| H                                                                 | 0.202 239 997 286  | -0.119 731 913 225 | 0.113 143 506 214  |
| H                                                                 | -0.030 260 322 546 | -0.023 984 489 379 | 0.027 811 728 504  |
| H                                                                 | 0.129 777 659 094  | -0.074 297 465 928 | -0.096 615 438 888 |
| H                                                                 | -0.092 289 373 605 | 0.041 427 297 874  | -0.052 900 221 168 |
| H                                                                 | -0.005 620 387 167 | 0.027 378 154 893  | -0.033 333 836 797 |
| H                                                                 | 0.142 870 021 830  | -0.009 023 596 185 | 0.010 227 949 007  |
| H                                                                 | 0.110 946 124 963  | 0.100 785 738 989  | -0.063 710 762 400 |
| H                                                                 | 0.027 590 259 245  | 0.025 407 276 996  | 0.057 618 657 899  |
| H                                                                 | -0.021 434 639 894 | -0.051 632 705 117 | -0.020 860 904 754 |
| H                                                                 | 0.078 544 911 522  | -0.062 375 194 037 | -0.073 018 858 619 |
| H                                                                 | -0.008 014 303 589 | 0.041 256 587 638  | -0.048 747 203 016 |
| H                                                                 | 0.025 431 507 610  | 0.045 325 209 228  | -0.000 372 932 725 |
| H                                                                 | -0.029 587 191 110 | 0.069 716 836 679  | -0.079 165 332 329 |

Wavenumber/cm<sup>-1</sup>: 3086.1091

| $\frac{\partial \mu_{x,y,z}}{\partial Q_r} / (e u^{-0.5})$        |                    |                    |                    |
|-------------------------------------------------------------------|--------------------|--------------------|--------------------|
|                                                                   | -0.013 812 437 722 | -0.019 801 950 383 | 0.002 201 338 083  |
| <i>l</i> -matrix coefficients/(u <sup>1/2</sup> Å <sup>-1</sup> ) |                    |                    |                    |
| O                                                                 | -0.137 666 130 369 | 0.118 523 340 981  | 0.013 629 703 670  |
| C                                                                 | -0.047 609 009 955 | -0.111 250 437 636 | 0.097 247 509 452  |
| C                                                                 | 0.025 074 666 464  | -0.047 558 382 475 | 0.048 455 343 867  |
| C                                                                 | -0.067 554 589 875 | -0.054 123 648 109 | 0.049 013 136 104  |
| C                                                                 | -0.000 754 243 142 | -0.048 281 067 044 | -0.018 196 825 017 |
| C                                                                 | -0.294 566 106 375 | 0.012 688 797 897  | 0.119 945 891 514  |
| C                                                                 | -0.049 472 767 966 | 0.098 121 604 919  | -0.202 994 124 077 |
| C                                                                 | 0.231 441 162 085  | -0.197 941 583 569 | -0.050 604 714 009 |
| C                                                                 | 0.182 071 910 970  | -0.110 625 721 510 | 0.025 294 655 688  |
| C                                                                 | -0.040 033 810 025 | -0.008 776 983 714 | -0.179 854 108 586 |
| C                                                                 | 0.160 253 396 515  | 0.265 789 899 655  | 0.157 062 298 496  |
| H                                                                 | 0.049 933 750 138  | -0.073 050 890 140 | 0.014 529 465 249  |
| H                                                                 | -0.139 529 278 939 | 0.071 034 298 162  | 0.173 214 449 813  |
| H                                                                 | -0.048 674 779 805 | 0.117 257 112 016  | -0.047 183 184 929 |
| H                                                                 | -0.211 974 317 061 | -0.000 523 603 310 | -0.073 912 025 118 |
| H                                                                 | -0.015 667 120 937 | -0.011 152 702 084 | 0.008 361 972 333  |
| H                                                                 | -0.038 037 216 707 | -0.057 282 133 903 | -0.106 835 251 952 |
| H                                                                 | 0.132 659 698 103  | 0.260 616 349 553  | 0.161 474 560 809  |
| H                                                                 | 0.003 405 570 245  | 0.015 442 928 532  | -0.151 271 633 027 |
| H                                                                 | 0.094 399 315 425  | -0.023 411 333 439 | -0.008 001 917 669 |
| H                                                                 | -0.000 195 789 069 | 0.032 601 886 380  | -0.057 632 157 869 |
| H                                                                 | 0.087 871 077 787  | -0.205 596 880 805 | -0.021 095 195 568 |
| H                                                                 | 0.198 543 350 992  | 0.013 076 005 427  | -0.047 180 519 780 |
| H                                                                 | 0.006 171 578 886  | 0.050 387 184 308  | -0.076 224 324 891 |
| H                                                                 | 0.058 099 382 450  | 0.109 188 330 574  | -0.156 960 574 230 |
| H                                                                 | 0.046 415 330 953  | -0.010 523 381 405 | 0.003 591 040 364  |
| H                                                                 | -0.016 178 180 795 | -0.063 115 955 694 | 0.174 210 287 992  |



Wavenumber/cm<sup>-1</sup>: 3089.5537

| $\frac{\partial \mu_{x,y,z}}{\partial Q_r} / (e u^{-0.5})$        |                    |                    |                    |
|-------------------------------------------------------------------|--------------------|--------------------|--------------------|
|                                                                   | -0.039 171 031 085 | 0.001 944 262 750  | 0.023 308 514 528  |
| <i>l</i> -matrix coefficients/(u <sup>1/2</sup> Å <sup>-1</sup> ) |                    |                    |                    |
| O                                                                 | -0.015 091 378 748 | 0.206 183 807 428  | 0.073 035 249 617  |
| C                                                                 | 0.007 149 551 829  | -0.078 898 937 062 | -0.004 723 328 148 |
| C                                                                 | 0.036 562 162 437  | -0.028 333 550 421 | 0.022 442 821 806  |
| C                                                                 | 0.048 060 751 625  | -0.030 940 597 317 | 0.087 186 863 369  |
| C                                                                 | 0.036 130 864 817  | -0.007 573 438 960 | -0.108 850 599 474 |
| C                                                                 | -0.068 637 408 660 | -0.150 272 915 061 | -0.047 536 848 585 |
| C                                                                 | 0.136 444 692 870  | -0.105 526 292 580 | 0.151 279 596 543  |
| C                                                                 | -0.308 569 734 023 | -0.001 938 572 126 | -0.136 037 093 770 |
| C                                                                 | -0.020 563 561 754 | 0.154 844 062 525  | 0.144 949 218 567  |
| C                                                                 | 0.030 968 809 735  | 0.079 344 895 454  | -0.433 024 477 534 |
| C                                                                 | 0.119 268 214 003  | -0.079 415 047 638 | 0.274 268 229 327  |
| H                                                                 | 0.051 283 923 379  | 0.193 974 641 894  | 0.130 784 930 333  |
| H                                                                 | -0.020 593 075 693 | -0.109 543 045 496 | -0.054 385 584 608 |
| H                                                                 | 0.095 185 696 744  | -0.067 280 962 592 | 0.043 534 742 036  |
| H                                                                 | 0.023 942 880 391  | -0.045 591 974 730 | 0.024 409 970 904  |
| H                                                                 | 0.038 994 017 128  | 0.019 424 574 039  | -0.076 027 860 433 |
| H                                                                 | -0.013 436 156 260 | -0.074 600 854 955 | -0.218 275 537 892 |
| H                                                                 | 0.092 727 648 659  | -0.012 731 981 893 | 0.094 987 898 154  |
| H                                                                 | 0.011 368 960 676  | -0.032 201 063 204 | 0.100 847 940 566  |
| H                                                                 | -0.174 704 589 894 | 0.015 130 656 367  | 0.052 248 811 809  |
| H                                                                 | 0.023 596 685 967  | 0.097 178 327 660  | -0.150 770 937 908 |
| H                                                                 | -0.119 336 460 710 | 0.091 704 465 137  | -0.085 119 559 028 |
| H                                                                 | -0.176 061 376 811 | -0.045 139 832 782 | -0.006 230 914 735 |
| H                                                                 | 0.029 102 504 320  | 0.101 525 151 657  | -0.154 114 892 299 |
| H                                                                 | 0.040 856 871 163  | -0.023 247 852 166 | 0.081 651 887 373  |
| H                                                                 | 0.107 758 335 442  | -0.042 696 209 584 | -0.032 332 433 106 |
| H                                                                 | -0.008 603 409 924 | -0.028 813 071 975 | 0.130 569 825 321  |

Wavenumber/cm<sup>-1</sup>: 3093.6732

| $\frac{\partial \mu_{x,y,z}}{\partial Q_r} / (e u^{-0.5})$        | 0.039 256 923 118  | -0.057 084 746 376 | -0.072 233 341 426 |
|-------------------------------------------------------------------|--------------------|--------------------|--------------------|
| <i>l</i> -matrix coefficients/(u <sup>1/2</sup> Å <sup>-1</sup> ) |                    |                    |                    |
| O                                                                 | 0.039 785 497 263  | -0.221 681 790 056 | -0.113 217 571 420 |
| C                                                                 | -0.006 049 143 338 | -0.018 559 483 498 | -0.011 969 727 720 |
| C                                                                 | 0.026 604 522 061  | -0.026 992 251 900 | 0.033 988 805 997  |
| C                                                                 | -0.007 756 664 164 | -0.034 182 803 293 | -0.065 810 476 041 |
| C                                                                 | -0.050 168 749 873 | -0.031 063 468 030 | 0.045 416 412 458  |
| C                                                                 | 0.233 047 392 695  | -0.057 322 220 859 | 0.005 027 666 589  |
| C                                                                 | -0.086 602 849 758 | -0.053 204 025 588 | -0.023 727 244 957 |
| C                                                                 | 0.066 041 584 727  | -0.009 285 076 911 | 0.072 884 129 750  |
| C                                                                 | 0.315 760 171 101  | 0.193 895 255 381  | 0.203 796 644 118  |
| C                                                                 | -0.536 164 623 142 | 0.138 318 789 652  | -0.135 687 101 292 |
| C                                                                 | 0.028 405 888 301  | 0.047 833 883 737  | -0.026 874 474 065 |
| H                                                                 | 0.092 336 759 847  | 0.004 181 565 179  | 0.071 665 723 915  |
| H                                                                 | 0.100 467 537 720  | -0.025 469 956 799 | -0.062 809 977 546 |
| H                                                                 | -0.040 723 055 981 | -0.022 666 056 302 | -0.010 030 144 401 |
| H                                                                 | 0.114 191 630 018  | -0.033 890 244 076 | 0.051 407 396 063  |
| H                                                                 | -0.029 951 877 835 | -0.014 825 370 501 | 0.033 106 714 038  |
| H                                                                 | -0.227 115 697 315 | 0.037 230 435 931  | -0.057 919 460 655 |
| H                                                                 | -0.010 441 513 605 | 0.001 623 631 457  | -0.016 816 386 991 |
| H                                                                 | -0.020 984 608 653 | -0.013 301 682 826 | -0.008 221 022 106 |
| H                                                                 | 0.185 606 616 623  | 0.056 193 107 943  | 0.137 542 848 438  |
| H                                                                 | -0.225 292 947 731 | -0.046 319 434 345 | -0.083 320 824 601 |
| H                                                                 | 0.026 737 246 436  | 0.021 490 726 096  | 0.055 916 747 331  |
| H                                                                 | 0.000 146 903 019  | -0.014 695 434 151 | 0.003 969 229 796  |
| H                                                                 | -0.178 550 022 536 | 0.183 152 460 165  | -0.002 981 883 275 |
| H                                                                 | 0.024 232 814 119  | 0.012 436 280 052  | 0.008 027 395 951  |
| H                                                                 | 0.077 134 323 398  | 0.183 287 709 592  | 0.018 956 238 997  |
| H                                                                 | 0.011 975 273 839  | 0.038 910 920 781  | -0.022 421 047 968 |

Wavenumber/cm<sup>-1</sup>: 3095.7133

| $\frac{\partial \mu_{x,y,z}}{\partial Q_r} / (e u^{-0.5})$        | 0.015 885 781 026  | -0.010 510 177 828                    | -0.029 684 095 864 |
|-------------------------------------------------------------------|--------------------|---------------------------------------|--------------------|
| <i>l</i> -matrix coefficients/(u <sup>1/2</sup> Å <sup>-1</sup> ) |                    |                                       |                    |
| O                                                                 | 0.011 193 840 033  | -0.099 665 743 244                    | -0.049 134 597 864 |
| C                                                                 | 0.015 563 815 131  | 0.026 691 214 205                     | 0.039 879 464 936  |
| C                                                                 | 0.003 740 558 417  | 0.050 306 258 250                     | 0.042 019 626 340  |
| C                                                                 | -0.018 793 846 041 | 0.016 614 495 698                     | -0.036 389 463 814 |
| C                                                                 | -0.050 238 298 203 | 0.065 094 943 902                     | 0.046 696 023 236  |
| C                                                                 | 0.146 238 295 971  | -0.044 834 711 149                    | 0.007 209 799 874  |
| C                                                                 | -0.101 430 975 267 | 0.079 074 225 434                     | -0.074 649 685 306 |
| C                                                                 | -0.019 747 318 707 | 0.045 067 836 872                     | 0.032 229 527 073  |
| C                                                                 | 0.105 239 149 120  | -0.071 200 995 660                    | -0.048 019 307 381 |
| C                                                                 | -0.030 611 035 251 | -1.749 974 800 000 × 10 <sup>-5</sup> | 0.134 401 306 984  |
| C                                                                 | -0.058 114 656 919 | -0.025 958 642 440                    | -0.067 477 277 327 |
| H                                                                 | 0.168 316 470 320  | 0.275 405 005 709                     | 0.226 877 374 030  |
| H                                                                 | 0.067 573 354 378  | -0.032 363 441 638                    | -0.055 033 872 754 |
| H                                                                 | -0.065 336 979 589 | 0.057 801 678 533                     | -0.020 567 914 945 |
| H                                                                 | 0.087 389 402 294  | -0.028 452 367 430                    | 0.049 693 024 553  |
| H                                                                 | -0.033 671 911 958 | 0.034 809 177 034                     | 0.020 509 154 363  |
| H                                                                 | 0.072 868 192 814  | -0.000 703 851 865                    | 0.056 610 796 238  |
| H                                                                 | 0.090 635 211 623  | 0.203 758 494 029                     | 0.115 542 451 347  |
| H                                                                 | -0.020 374 251 003 | 0.017 205 957 197                     | -0.064 291 177 933 |
| H                                                                 | -0.364 419 611 073 | -0.063 140 880 232                    | -0.134 393 692 803 |
| H                                                                 | -0.057 626 745 185 | 0.011 277 718 268                     | -0.034 557 220 063 |
| H                                                                 | -0.008 614 899 350 | 0.052 566 338 680                     | 0.021 238 281 158  |
| H                                                                 | -0.039 553 632 804 | -0.007 606 801 533                    | -0.001 592 581 737 |
| H                                                                 | -0.066 308 389 678 | -0.016 177 429 108                    | 0.120 215 653 547  |
| H                                                                 | -0.155 066 079 395 | 0.020 824 217 917                     | -0.284 886 932 364 |
| H                                                                 | 0.313 899 942 814  | -0.321 929 705 428                    | -0.167 447 020 820 |
| H                                                                 | -0.006 158 692 432 | -0.292 365 008 512                    | 0.085 834 378 438  |

Wavenumber/cm<sup>-1</sup>: 3098.3913

| $\frac{\partial \mu_{x,y,z}}{\partial Q_r} / (e u^{-0.5})$        | 0.011 071 400 819  | -0.053 403 787 137 | -0.029 846 256 979 |
|-------------------------------------------------------------------|--------------------|--------------------|--------------------|
| <i>l</i> -matrix coefficients/(u <sup>1/2</sup> Å <sup>-1</sup> ) |                    |                    |                    |
| O                                                                 | 0.052 403 845 494  | 0.036 256 027 471  | 0.107 739 828 577  |
| C                                                                 | 0.008 621 782 739  | -0.007 724 197 707 | -0.052 788 244 982 |
| C                                                                 | 0.007 759 737 811  | -0.010 655 481 017 | -0.025 389 848 744 |
| C                                                                 | 0.029 718 091 220  | 0.061 890 704 735  | 0.003 061 177 996  |
| C                                                                 | -0.014 814 204 182 | -0.012 290 373 748 | -0.015 318 273 631 |
| C                                                                 | 0.111 290 376 820  | -0.118 762 540 735 | -0.088 618 468 628 |
| C                                                                 | 0.028 668 454 156  | 0.038 976 374 716  | 0.009 995 478 417  |
| C                                                                 | -0.030 831 280 185 | -0.049 654 731 238 | -0.055 227 637 629 |
| C                                                                 | -0.135 651 428 943 | -0.280 683 010 707 | -0.220 163 544 634 |
| C                                                                 | -0.244 354 226 443 | -0.018 044 268 951 | 0.095 835 061 063  |
| C                                                                 | 0.207 431 929 957  | 0.358 240 104 859  | 0.213 360 787 794  |
| H                                                                 | -0.031 281 638 073 | -0.049 541 583 656 | -0.051 256 347 709 |
| H                                                                 | 0.056 498 208 321  | -0.049 704 401 267 | -0.078 803 009 417 |
| H                                                                 | 0.009 448 893 408  | 0.003 312 300 866  | 0.002 095 889 370  |
| H                                                                 | 0.074 333 685 083  | -0.048 061 830 850 | 0.017 570 720 410  |
| H                                                                 | 0.009 424 203 377  | -0.002 648 723 614 | -0.019 140 649 609 |
| H                                                                 | 0.093 208 717 720  | -0.014 332 027 821 | 0.056 879 047 593  |
| H                                                                 | 0.007 351 698 053  | -0.004 231 981 960 | -0.005 522 506 021 |
| H                                                                 | 0.010 961 681 331  | 0.013 497 543 235  | 0.008 587 318 895  |
| H                                                                 | -0.119 783 919 625 | -0.077 260 750 471 | -0.158 951 366 646 |
| H                                                                 | -0.181 917 134 044 | 0.010 012 993 223  | -0.136 127 011 574 |
| H                                                                 | -0.012 752 466 978 | 0.019 929 095 616  | -0.008 646 810 478 |
| H                                                                 | -0.039 195 302 838 | -0.031 585 217 636 | -0.021 736 017 558 |
| H                                                                 | -0.196 884 474 785 | -0.010 962 711 415 | 0.205 772 134 753  |
| H                                                                 | 0.241 512 017 965  | 0.094 228 731 942  | 0.224 959 965 849  |
| H                                                                 | -0.010 972 393 555 | -0.203 985 097 064 | -0.039 500 295 896 |
| H                                                                 | -0.007 714 504 262 | 0.340 504 055 826  | 0.041 467 506 830  |

Wavenumber/cm<sup>-1</sup>: 3102.541

| $\frac{\partial \mu_{x,y,z}}{\partial Q_r} / (e u^{-0.5})$        | 0.010 911 532 611  | 0.002 481 771 240  | -0.003 328 486 426 |
|-------------------------------------------------------------------|--------------------|--------------------|--------------------|
| <i>l</i> -matrix coefficients/(u <sup>1/2</sup> Å <sup>-1</sup> ) |                    |                    |                    |
| O                                                                 | 0.056 164 079 244  | -0.039 926 278 787 | 0.165 506 681 973  |
| C                                                                 | -0.001 421 440 489 | 0.027 550 793 473  | -0.039 811 174 545 |
| C                                                                 | -0.001 925 408 476 | 0.017 114 921 424  | -0.031 112 356 464 |
| C                                                                 | 0.031 545 054 294  | 0.043 704 809 573  | 0.010 017 850 542  |
| C                                                                 | -0.001 918 686 031 | 0.023 543 791 852  | -0.030 864 778 242 |
| C                                                                 | 0.120 606 387 837  | -0.088 252 579 175 | -0.084 373 500 380 |
| C                                                                 | 0.037 388 384 906  | 0.012 009 040 109  | 0.038 182 895 355  |
| C                                                                 | -0.092 343 290 687 | 0.025 408 201 471  | -0.056 335 751 730 |
| C                                                                 | -0.086 946 296 600 | -0.128 756 968 343 | -0.130 454 335 554 |
| C                                                                 | -0.110 757 885 378 | 0.000 389 536 482  | 0.082 738 641 224  |
| C                                                                 | 0.063 572 913 238  | 0.130 448 107 958  | 0.062 111 598 504  |
| H                                                                 | -0.054 854 320 895 | -0.103 710 547 094 | -0.090 090 607 949 |
| H                                                                 | 0.058 505 636 145  | -0.055 928 459 793 | -0.085 541 630 008 |
| H                                                                 | 0.027 227 275 831  | -0.021 042 887 469 | 0.009 607 550 243  |
| H                                                                 | 0.087 721 717 245  | -0.038 015 401 533 | 0.028 127 599 371  |
| H                                                                 | 0.009 999 486 414  | 0.011 883 309 388  | -0.023 583 558 378 |
| H                                                                 | -0.481 637 901 906 | 0.124 586 691 568  | 0.030 463 930 275  |
| H                                                                 | 0.104 545 225 416  | 0.191 399 046 342  | 0.116 588 819 121  |
| H                                                                 | 0.004 678 046 313  | 0.007 568 064 921  | 0.038 655 631 745  |
| H                                                                 | 0.037 020 581 944  | -0.021 135 041 338 | -0.069 984 574 798 |
| H                                                                 | 0.139 453 926 258  | -0.213 921 497 334 | 0.391 575 495 163  |
| H                                                                 | -0.038 346 347 105 | 0.071 265 906 967  | -0.018 524 856 479 |
| H                                                                 | -0.082 904 873 238 | -0.024 285 250 930 | -0.011 135 331 019 |
| H                                                                 | 0.221 645 273 737  | 0.087 577 571 152  | -0.334 373 894 311 |
| H                                                                 | -0.009 926 382 301 | 0.062 407 513 118  | -0.154 804 795 153 |
| H                                                                 | -0.082 494 915 919 | -0.027 790 153 402 | 0.014 930 212 128  |
| H                                                                 | -0.018 720 056 705 | -0.109 815 354 121 | 0.119 712 821 031  |

Wavenumber/cm<sup>-1</sup>: 3112.165

| $\frac{\partial \mu_{x,y,z}}{\partial Q_r} / (e u^{-0.5})$        |                    |                    |                    |
|-------------------------------------------------------------------|--------------------|--------------------|--------------------|
|                                                                   | -0.008 129 617 749 | 0.026 290 929 701  | 0.040 632 294 912  |
| <i>l</i> -matrix coefficients/(u <sup>1/2</sup> Å <sup>-1</sup> ) |                    |                    |                    |
| O                                                                 | -0.076 573 236 899 | 0.061 410 761 116  | -0.128 543 387 727 |
| C                                                                 | -0.024 764 980 324 | -0.028 021 852 608 | 0.060 243 527 749  |
| C                                                                 | 0.003 322 825 594  | -0.014 883 090 372 | 0.028 865 573 963  |
| C                                                                 | -0.042 605 080 758 | -0.015 998 461 495 | -0.008 719 336 595 |
| C                                                                 | -0.022 710 261 641 | -0.024 096 091 223 | 0.050 586 686 124  |
| C                                                                 | -0.074 387 827 718 | 0.025 503 620 394  | 0.075 681 868 572  |
| C                                                                 | -0.051 808 089 907 | 0.007 015 967 025  | -0.031 372 681 951 |
| C                                                                 | 0.080 277 632 854  | -0.048 913 256 231 | 0.050 850 571 893  |
| C                                                                 | 0.157 066 225 122  | -0.030 631 067 759 | 0.028 583 789 466  |
| C                                                                 | 0.037 672 642 172  | -0.012 859 868 290 | -0.008 668 955 123 |
| C                                                                 | -0.019 013 749 858 | 0.059 761 766 254  | -0.081 937 424 718 |
| H                                                                 | 0.146 810 172 272  | 0.203 755 625 237  | 0.185 924 455 747  |
| H                                                                 | -0.037 950 209 072 | 0.029 342 751 926  | 0.065 229 579 591  |
| H                                                                 | -0.034 089 749 813 | 0.025 638 354 555  | -0.007 609 367 950 |
| H                                                                 | -0.062 177 561 917 | 0.010 246 115 244  | -0.013 791 988 556 |
| H                                                                 | -0.015 249 298 997 | -0.009 395 578 867 | 0.025 281 090 092  |
| H                                                                 | -0.256 292 449 666 | 0.041 990 214 558  | -0.023 782 413 158 |
| H                                                                 | -0.169 172 567 086 | -0.238 686 570 736 | -0.192 830 881 424 |
| H                                                                 | -0.006 164 922 700 | 0.000 899 428 564  | -0.033 698 494 242 |
| H                                                                 | -0.225 217 856 272 | -0.040 548 542 636 | -0.054 928 012 769 |
| H                                                                 | 0.135 235 082 387  | -0.094 241 779 477 | 0.223 255 740 516  |
| H                                                                 | 0.035 641 622 656  | -0.068 213 415 370 | 0.024 005 448 674  |
| H                                                                 | 0.067 525 888 593  | 0.009 379 884 454  | 0.001 829 499 593  |
| H                                                                 | 0.174 979 146 731  | 0.046 306 432 504  | -0.235 597 198 469 |
| H                                                                 | 0.133 404 943 013  | -0.017 867 395 580 | 0.283 463 224 169  |
| H                                                                 | 0.248 615 492 402  | -0.194 717 485 557 | -0.113 632 289 227 |
| H                                                                 | 0.020 570 644 262  | 0.338 383 360 887  | -0.187 508 479 342 |

Wavenumber/cm<sup>-1</sup>: 3124.3321

| $\frac{\partial \mu_{x,y,z}}{\partial Q_r} / (e u^{-0.5})$        |                    |                                       |                    |
|-------------------------------------------------------------------|--------------------|---------------------------------------|--------------------|
|                                                                   | -0.015 629 199 967 | 0.006 622 147 935                     | -0.002 987 107 895 |
| <i>l</i> -matrix coefficients/(u <sup>1/2</sup> Å <sup>-1</sup> ) |                    |                                       |                    |
| O                                                                 | -0.142 818 816 775 | 0.466 779 360 631                     | -0.528 605 293 607 |
| C                                                                 | 0.012 883 961 646  | -0.081 979 907 865                    | 0.100 936 955 523  |
| C                                                                 | 0.068 105 035 389  | -0.016 770 743 781                    | 0.005 471 579 903  |
| C                                                                 | -0.018 739 724 371 | 0.054 602 219 375                     | -0.030 187 048 248 |
| C                                                                 | -0.013 062 543 719 | -0.040 957 382 907                    | 0.048 337 163 258  |
| C                                                                 | -0.047 764 452 119 | -0.124 849 190 450                    | 0.042 504 476 140  |
| C                                                                 | 0.037 815 542 710  | -0.141 629 376 642                    | 0.197 516 509 800  |
| C                                                                 | -0.206 883 531 422 | -0.018 235 174 564                    | 0.038 632 675 243  |
| C                                                                 | 0.243 513 704 164  | -0.073 448 851 962                    | -0.010 039 811 506 |
| C                                                                 | -0.012 060 415 132 | -0.128 006 809 753                    | 0.226 355 522 890  |
| C                                                                 | 0.057 294 655 466  | 0.118 736 699 229                     | -0.106 250 539 364 |
| H                                                                 | 0.056 462 182 391  | -0.103 792 490 290                    | -0.017 009 056 975 |
| H                                                                 | -0.014 853 787 883 | -0.071 710 094 917                    | -0.007 294 043 719 |
| H                                                                 | 0.049 135 824 974  | -0.124 046 213 060                    | 0.048 537 929 224  |
| H                                                                 | 0.013 138 879 609  | -0.029 229 349 023                    | 0.032 225 203 599  |
| H                                                                 | 0.008 188 127 497  | $5.240\,916\,400\,000 \times 10^{-5}$ | -0.006 831 959 139 |
| H                                                                 | 0.016 947 415 508  | -0.017 632 016 947                    | 0.088 115 952 107  |
| H                                                                 | 0.014 560 484 017  | 0.102 046 051 288                     | 0.004 847 456 977  |
| H                                                                 | -0.001 790 664 423 | -0.026 241 749 747                    | 0.145 451 216 829  |
| H                                                                 | 0.159 907 888 957  | -0.006 477 162 378                    | -0.004 890 652 481 |
| H                                                                 | -0.014 193 360 990 | -0.050 501 151 837                    | 0.059 180 876 488  |
| H                                                                 | -0.075 901 495 053 | 0.053 824 304 383                     | -0.007 269 785 183 |
| H                                                                 | -0.113 701 050 503 | -0.034 120 385 772                    | 0.027 374 236 582  |
| H                                                                 | -0.016 214 721 545 | -0.055 373 641 198                    | 0.083 341 981 317  |
| H                                                                 | 0.014 420 351 080  | 0.046 163 094 144                     | -0.107 177 745 630 |
| H                                                                 | 0.034 765 200 449  | 0.035 534 386 453                     | 0.009 182 788 742  |
| H                                                                 | 0.020 087 612 327  | -0.016 027 568 000                    | -0.013 603 157 939 |

*Final state*

Wavenumber/cm<sup>-1</sup>: 144.6073 , Max excitation: 3

---

| $l'$ -matrix coefficients/(u <sup>1/2</sup> Å <sup>-1</sup> ) |                                       |                                        |
|---------------------------------------------------------------|---------------------------------------|----------------------------------------|
| O                                                             | $4.539\,860\,800\,000 \times 10^{-5}$ | $-6.941\,328\,000\,000 \times 10^{-6}$ |
| C                                                             | $-0.000\,809\,624\,105$               | $0.000\,333\,109\,412$                 |
| C                                                             | $0.002\,759\,746\,465$                | $-0.003\,971\,428\,140$                |
| C                                                             | $3.349\,813\,200\,000 \times 10^{-5}$ | $0.000\,150\,801\,106$                 |
| C                                                             | $-0.000\,564\,782\,840$               | $0.000\,406\,536\,407$                 |
| C                                                             | $-0.009\,190\,037\,227$               | $0.003\,675\,456\,003$                 |
| C                                                             | $0.000\,218\,544\,948$                | $-0.000\,605\,954\,453$                |
| C                                                             | $-0.012\,198\,639\,164$               | $0.000\,450\,839\,754$                 |
| C                                                             | $0.004\,212\,281\,118$                | $-0.005\,105\,117\,253$                |
| C                                                             | $0.000\,655\,608\,941$                | $-0.002\,097\,509\,063$                |
| C                                                             | $-0.011\,407\,010\,033$               | $-0.184\,763\,062\,682$                |
| H                                                             | $-0.015\,755\,426\,201$               | $0.001\,037\,097\,357$                 |
| H                                                             | $0.016\,987\,321\,118$                | $-0.005\,244\,263\,367$                |
| H                                                             | $0.000\,518\,660\,859$                | $0.000\,291\,617\,773$                 |
| H                                                             | $0.022\,124\,214\,999$                | $-0.010\,740\,616\,303$                |
| H                                                             | $-0.000\,504\,081\,908$               | $-0.000\,604\,189\,071$                |
| H                                                             | $0.003\,808\,527\,754$                | $0.008\,700\,127\,317$                 |
| H                                                             | $0.170\,545\,718\,882$                | $0.466\,413\,013\,455$                 |
| H                                                             | $-0.001\,324\,075\,190$               | $0.002\,876\,153\,193$                 |
| H                                                             | $-0.002\,699\,401\,625$               | $0.020\,725\,723\,185$                 |
| H                                                             | $0.002\,778\,074\,408$                | $-0.002\,145\,970\,865$                |
| H                                                             | $0.038\,576\,790\,123$                | $0.007\,256\,469\,145$                 |
| H                                                             | $0.008\,510\,350\,075$                | $-0.012\,286\,501\,006$                |
| H                                                             | $-0.009\,308\,088\,552$               | $0.000\,199\,616\,739$                 |
| H                                                             | $-0.013\,860\,245\,181$               | $0.237\,585\,588\,936$                 |
| H                                                             | $0.003\,347\,550\,780$                | $0.000\,894\,392\,120$                 |
| H                                                             | $-0.133\,172\,733\,294$               | $-0.053\,785\,210\,140$                |

---



Wavenumber/cm<sup>-1</sup>: 187.924 , Max excitation: 2

| $l'$ -matrix coefficients/(u <sup>1/2</sup> Å <sup>-1</sup> ) |                                       |                    |
|---------------------------------------------------------------|---------------------------------------|--------------------|
| O                                                             | -4.699 669 300 000 × 10 <sup>-5</sup> | -0.000 121 677 818 |
| C                                                             | -0.000 133 191 602                    | -0.000 145 949 884 |
| C                                                             | -0.004 836 978 255                    | 0.002 222 581 232  |
| C                                                             | 0.000 652 237 215                     | 0.000 710 861 861  |
| C                                                             | -0.004 531 063 823                    | -0.003 195 395 385 |
| C                                                             | -0.008 020 531 131                    | 0.003 199 409 961  |
| C                                                             | -0.001 559 112 514                    | 0.000 412 800 354  |
| C                                                             | -0.030 852 698 138                    | 0.005 801 156 178  |
| C                                                             | -0.286 310 592 518                    | 0.055 797 156 883  |
| C                                                             | 0.000 860 495 993                     | -0.001 206 402 379 |
| C                                                             | -0.001 879 412 246                    | -0.003 914 316 644 |
| H                                                             | 0.809 955 313 164                     | -0.063 876 450 261 |
| H                                                             | 0.018 766 599 204                     | -0.005 780 184 011 |
| H                                                             | 0.001 868 742 108                     | 0.007 107 053 509  |
| H                                                             | 0.009 294 581 521                     | -0.004 780 217 947 |
| H                                                             | 0.013 786 332 212                     | 0.010 898 700 923  |
| H                                                             | 0.002 919 635 755                     | 0.008 727 712 957  |
| H                                                             | 0.002 980 712 736                     | 0.008 832 171 647  |
| H                                                             | 0.001 791 643 468                     | -0.003 316 002 719 |
| H                                                             | 0.027 942 143 374                     | -0.231 057 205 323 |
| H                                                             | 0.008 201 921 838                     | -0.003 755 684 365 |
| H                                                             | 0.084 827 303 203                     | 0.018 607 673 353  |
| H                                                             | 0.024 679 507 515                     | -0.039 085 623 797 |
| H                                                             | -0.013 723 121 855                    | -0.001 010 836 904 |
| H                                                             | 0.000 642 057 046                     | 0.000 723 710 370  |
| H                                                             | 0.159 740 847 153                     | 0.089 795 966 556  |
| H                                                             | 0.008 487 523 753                     | 0.002 433 152 537  |

Wavenumber/cm<sup>-1</sup>: 215.6031 , Max excitation: 2

| $l'$ -matrix coefficients/(u <sup>1/2</sup> Å <sup>-1</sup> ) |                                      |                                      |                    |
|---------------------------------------------------------------|--------------------------------------|--------------------------------------|--------------------|
| O                                                             | 4.026 656 300 000 × 10 <sup>-5</sup> | -0.000 140 109 014                   | -0.000 198 978 009 |
| C                                                             | 0.000 888 775 484                    | -0.001 357 136 380                   | 0.004 798 795 403  |
| C                                                             | -0.001 050 653 299                   | -0.001 230 561 477                   | -0.000 954 279 848 |
| C                                                             | 4.320 564 200 000 × 10 <sup>-5</sup> | -0.000 124 816 466                   | -0.000 326 354 110 |
| C                                                             | -0.005 441 242 703                   | -0.003 204 478 575                   | -0.004 862 399 335 |
| C                                                             | 0.018 584 327 343                    | -0.005 182 523 527                   | 0.009 342 512 633  |
| C                                                             | 0.000 432 901 190                    | -0.001 140 513 095                   | 0.000 565 174 272  |
| C                                                             | -0.036 718 354 445                   | 9.014 130 100 000 × 10 <sup>-5</sup> | 0.009 432 466 479  |
| C                                                             | 0.001 288 447 394                    | -0.035 481 216 954                   | -0.020 523 860 310 |
| C                                                             | 0.054 317 476 036                    | -0.119 640 780 842                   | 0.267 678 733 640  |
| C                                                             | -0.005 396 099 174                   | -0.001 295 362 385                   | -0.012 580 054 515 |
| H                                                             | -0.023 783 235 913                   | -0.000 706 486 504                   | 0.007 284 202 848  |
| H                                                             | -0.061 989 857 575                   | 0.022 946 903 743                    | -0.038 495 900 902 |
| H                                                             | 0.000 813 607 176                    | 0.000 528 394 125                    | -0.002 746 940 299 |
| H                                                             | -0.001 136 900 926                   | 0.002 126 077 993                    | 0.002 888 181 591  |
| H                                                             | 0.016 453 575 287                    | 0.012 173 095 746                    | 0.015 715 330 549  |
| H                                                             | 0.173 126 777 135                    | 0.452 503 412 472                    | -0.546 274 488 839 |
| H                                                             | -0.004 326 648 619                   | -0.011 951 871 380                   | 0.018 753 153 236  |
| H                                                             | -0.001 118 489 527                   | 0.002 468 511 311                    | -0.000 326 632 197 |
| H                                                             | -0.022 025 049 399                   | 0.107 172 621 605                    | 0.020 598 760 997  |
| H                                                             | 0.084 626 930 677                    | -0.042 390 039 639                   | -0.031 089 813 187 |
| H                                                             | 0.113 840 664 072                    | 0.023 671 252 597                    | -0.036 047 030 818 |
| H                                                             | 0.013 980 425 291                    | -0.025 448 719 972                   | 0.003 160 838 240  |
| H                                                             | -0.446 563 411 380                   | 0.003 901 197 295                    | -0.351 758 979 356 |
| H                                                             | -0.001 483 639 726                   | 0.010 427 982 534                    | 0.001 589 130 640  |
| H                                                             | 0.042 359 750 661                    | 0.018 603 054 027                    | 0.042 905 038 466  |
| H                                                             | 0.024 038 368 615                    | 0.006 423 886 112                    | 0.022 768 325 771  |

Wavenumber/cm<sup>-1</sup>: 222.9143 , Max excitation: 3

| $l'$ -matrix coefficients/(u <sup>1/2</sup> Å <sup>-1</sup> ) |                                       |                                       |                    |
|---------------------------------------------------------------|---------------------------------------|---------------------------------------|--------------------|
| O                                                             | 0.000 822 113 467                     | $3.277\,612\,400\,000 \times 10^{-5}$ | 0.000 277 898 957  |
| C                                                             | 0.004 956 111 461                     | -0.000 805 742 691                    | -0.000 750 081 290 |
| C                                                             | -0.001 011 701 057                    | 0.000 939 738 468                     | -0.001 679 766 282 |
| C                                                             | -0.002 715 372 982                    | 0.000 593 441 368                     | -0.001 031 335 261 |
| C                                                             | $7.774\,169\,800\,000 \times 10^{-5}$ | -0.001 630 624 062                    | -0.001 725 468 702 |
| C                                                             | 0.230 296 775 595                     | -0.080 001 256 026                    | 0.094 038 068 150  |
| C                                                             | 0.000 712 600 908                     | -0.000 417 184 206                    | 0.002 006 334 467  |
| C                                                             | 0.076 312 716 650                     | -0.069 601 515 994                    | -0.002 992 381 410 |
| C                                                             | -0.014 139 674 087                    | 0.006 839 767 790                     | 0.004 143 635 912  |
| C                                                             | 0.072 477 710 859                     | 0.003 551 192 918                     | -0.026 919 592 012 |
| C                                                             | -0.000 301 288 652                    | -0.014 073 621 320                    | 0.004 136 132 253  |
| H                                                             | 0.040 595 278 017                     | -0.003 078 195 428                    | -0.016 352 099 251 |
| H                                                             | -0.692 935 105 147                    | 0.223 099 442 261                     | -0.427 182 456 423 |
| H                                                             | $4.528\,932\,500\,000 \times 10^{-5}$ | 0.001 269 764 124                     | -0.005 522 235 882 |
| H                                                             | -0.101 714 839 309                    | 0.058 680 112 249                     | 0.116 435 131 208  |
| H                                                             | 0.000 980 410 700                     | 0.000 974 723 357                     | 0.001 542 182 048  |
| H                                                             | -0.024 782 814 963                    | -0.078 771 448 842                    | 0.093 996 484 084  |
| H                                                             | 0.003 037 220 078                     | 0.013 200 916 313                     | -0.021 526 816 699 |
| H                                                             | -0.002 486 783 584                    | 0.002 329 548 066                     | 0.000 277 979 850  |
| H                                                             | 0.003 894 612 466                     | -0.023 924 787 959                    | -0.004 903 518 617 |
| H                                                             | -0.137 019 811 903                    | 0.064 036 838 061                     | 0.083 583 742 030  |
| H                                                             | -0.096 206 361 311                    | -0.027 215 077 879                    | 0.032 487 944 547  |
| H                                                             | -0.170 167 828 584                    | 0.261 882 621 041                     | -0.025 365 190 704 |
| H                                                             | -0.091 846 383 799                    | 0.001 477 172 015                     | -0.081 745 051 651 |
| H                                                             | -0.002 692 721 313                    | 0.038 587 284 451                     | 0.008 763 745 218  |
| H                                                             | 0.004 488 594 005                     | 0.002 977 056 232                     | 0.006 709 597 311  |
| H                                                             | -0.002 187 153 514                    | -0.001 960 136 443                    | -0.001 271 930 144 |

Wavenumber/cm<sup>-1</sup>: 231.8692 , Max excitation: 2

| $l'$ -matrix coefficients/(u <sup>1/2</sup> Å <sup>-1</sup> ) |                                      |                    |                    |
|---------------------------------------------------------------|--------------------------------------|--------------------|--------------------|
| O                                                             | 5.762 604 000 000 × 10 <sup>-5</sup> | -0.000 229 432 610 | -0.000 245 534 673 |
| C                                                             | 0.005 057 856 934                    | -0.001 464 179 590 | -0.002 562 112 674 |
| C                                                             | -0.001 064 254 142                   | -0.001 480 801 222 | -0.000 217 985 648 |
| C                                                             | -0.001 702 342 969                   | 0.000 811 048 256  | 0.001 824 757 709  |
| C                                                             | -0.013 758 209 548                   | -0.008 417 954 986 | -0.012 367 434 570 |
| C                                                             | -0.043 013 269 511                   | 0.014 110 291 703  | -0.017 548 698 369 |
| C                                                             | 0.000 232 639 714                    | 0.000 268 893 050  | 0.000 542 328 164  |
| C                                                             | -0.086 285 187 627                   | 0.030 173 442 243  | 0.014 252 465 654  |
| C                                                             | 0.003 075 695 565                    | -0.020 289 158 940 | -0.016 575 021 309 |
| C                                                             | 0.272 286 002 561                    | -0.002 040 845 340 | -0.068 487 419 488 |
| C                                                             | -0.004 474 316 286                   | -0.015 962 102 741 | -0.017 050 937 083 |
| H                                                             | -0.033 475 310 342                   | 0.001 819 382 835  | 0.012 367 761 488  |
| H                                                             | 0.129 761 074 624                    | -0.038 537 070 844 | 0.079 412 469 072  |
| H                                                             | 0.000 571 355 410                    | 0.000 280 225 998  | -0.003 421 827 582 |
| H                                                             | 0.015 758 336 139                    | -0.010 675 300 820 | -0.018 558 813 237 |
| H                                                             | 0.044 322 744 629                    | 0.032 877 040 402  | 0.042 658 064 322  |
| H                                                             | -0.065 488 016 223                   | -0.227 150 541 655 | 0.273 537 998 434  |
| H                                                             | -0.005 157 016 474                   | -0.016 626 920 443 | 0.023 389 070 143  |
| H                                                             | 0.001 597 674 079                    | -0.003 200 035 406 | -0.000 439 266 305 |
| H                                                             | -0.011 039 933 296                   | 0.055 436 632 973  | 0.009 253 401 594  |
| H                                                             | -0.498 276 085 688                   | 0.228 528 592 731  | 0.304 450 516 739  |
| H                                                             | 0.203 064 812 601                    | 0.046 841 532 572  | -0.064 547 127 592 |
| H                                                             | 0.095 794 306 782                    | -0.150 795 622 181 | 0.016 136 618 730  |
| H                                                             | -0.383 446 819 745                   | 0.009 554 685 827  | -0.337 123 654 991 |
| H                                                             | -0.004 318 210 391                   | 0.066 113 756 598  | 0.012 924 538 393  |
| H                                                             | 0.033 870 827 091                    | 0.014 441 325 178  | 0.034 992 624 304  |
| H                                                             | 0.026 248 922 009                    | 0.006 820 116 654  | 0.023 935 779 169  |

Wavenumber/cm<sup>-1</sup>: 244.4076 , Max excitation: 1

| $l'$ -matrix coefficients/(u <sup>1/2</sup> Å <sup>-1</sup> ) |                    |                    |
|---------------------------------------------------------------|--------------------|--------------------|
| O                                                             | -0.000 970 851 910 | -0.000 477 097 377 |
| C                                                             | 0.000 470 271 723  | 0.001 002 506 861  |
| C                                                             | -0.002 578 117 171 | -0.003 925 454 406 |
| C                                                             | 0.002 076 692 870  | 0.000 359 540 573  |
| C                                                             | -0.047 459 681 850 | -0.031 061 689 961 |
| C                                                             | 0.057 951 053 951  | -0.019 417 990 968 |
| C                                                             | 0.001 307 625 162  | -0.001 863 445 053 |
| C                                                             | -0.165 862 001 299 | 0.046 051 590 916  |
| C                                                             | -0.024 432 115 137 | -0.129 925 342 438 |
| C                                                             | -0.084 574 249 136 | 0.026 246 729 511  |
| C                                                             | -0.049 023 631 262 | -0.087 916 240 814 |
| H                                                             | -0.055 812 450 392 | -0.003 756 606 459 |
| H                                                             | -0.186 553 217 628 | 0.059 636 090 555  |
| H                                                             | -0.001 832 834 368 | 0.000 610 043 222  |
| H                                                             | -0.013 031 789 661 | 0.008 063 134 503  |
| H                                                             | 0.156 328 401 091  | 0.116 627 875 574  |
| H                                                             | -0.018 717 797 642 | -0.032 237 331 634 |
| H                                                             | -0.011 466 986 395 | -0.030 905 400 234 |
| H                                                             | -0.001 002 469 388 | 0.003 919 835 762  |
| H                                                             | -0.074 837 680 590 | 0.359 478 965 966  |
| H                                                             | 0.123 443 846 007  | -0.055 541 029 500 |
| H                                                             | 0.413 065 109 164  | 0.093 069 521 752  |
| H                                                             | 0.161 859 215 524  | -0.256 725 210 827 |
| H                                                             | 0.187 683 011 659  | -0.002 589 179 807 |
| H                                                             | -0.020 233 355 350 | 0.281 459 708 131  |
| H                                                             | 0.217 024 806 842  | 0.095 265 986 578  |
| H                                                             | 0.205 399 022 357  | 0.057 473 429 033  |

Wavenumber/cm<sup>-1</sup>: -249.735, replaced by 249.735 , Max excitation: 5

| $l'$ -matrix coefficients/(u <sup>1/2</sup> Å <sup>-1</sup> ) |                    |                    |
|---------------------------------------------------------------|--------------------|--------------------|
| O                                                             | -0.000 868 779 605 | -0.000 385 042 512 |
| C                                                             | -0.000 454 481 333 | 0.000 919 550 897  |
| C                                                             | 0.001 378 025 285  | 0.003 786 527 622  |
| C                                                             | 0.001 158 052 387  | 0.000 839 298 425  |
| C                                                             | -0.029 075 225 595 | -0.020 014 821 493 |
| C                                                             | 0.058 797 802 524  | -0.018 246 951 318 |
| C                                                             | 0.000 758 946 754  | 0.000 704 360 148  |
| C                                                             | -0.177 122 662 899 | 0.074 055 348 455  |
| C                                                             | 0.051 222 985 893  | 0.113 988 922 078  |
| C                                                             | -0.024 877 955 141 | 0.007 192 506 541  |
| C                                                             | 0.048 896 283 147  | 0.126 681 434 655  |
| H                                                             | -0.056 916 905 477 | 0.012 244 826 632  |
| H                                                             | -0.201 407 537 538 | 0.065 241 192 684  |
| H                                                             | -0.000 505 226 991 | -0.003 128 828 812 |
| H                                                             | -0.000 360 278 629 | -0.001 480 219 318 |
| H                                                             | 0.093 355 480 670  | 0.067 241 780 859  |
| H                                                             | -0.001 818 357 523 | 0.000 402 341 409  |
| H                                                             | 0.011 823 833 082  | 0.029 928 071 680  |
| H                                                             | 0.002 808 724 737  | -0.004 232 402 678 |
| H                                                             | 0.069 518 920 505  | -0.323 101 459 083 |
| H                                                             | 0.057 014 003 119  | -0.026 197 826 762 |
| H                                                             | 0.389 072 226 262  | 0.089 578 698 175  |
| H                                                             | 0.224 016 965 546  | -0.348 919 947 726 |
| H                                                             | 0.031 406 572 912  | -0.001 451 501 091 |
| H                                                             | 0.030 574 990 487  | -0.411 103 965 694 |
| H                                                             | -0.191 642 894 747 | -0.085 807 051 949 |
| H                                                             | -0.214 193 967 049 | -0.058 430 499 433 |

Wavenumber/cm<sup>-1</sup>: 255.6989 , Max excitation: 2

| $l'$ -matrix coefficients/(u <sup>1/2</sup> Å <sup>-1</sup> ) |                                      |                                       |
|---------------------------------------------------------------|--------------------------------------|---------------------------------------|
| O -0.000 455 823 252                                          | -0.000 183 722 317                   | -5.964 485 300 000 × 10 <sup>-5</sup> |
| C 0.000 564 608 959                                           | 0.000 452 421 684                    | 2.134 195 000 000 × 10 <sup>-5</sup>  |
| C -0.000 895 596 749                                          | 6.475 389 300 000 × 10 <sup>-5</sup> | -0.000 369 648 773                    |
| C 0.000 770 889 135                                           | 0.000 449 433 023                    | -0.000 188 543 459                    |
| C -0.015 447 140 746                                          | -0.011 170 687 245                   | -0.014 510 367 039                    |
| C 0.003 565 172 256                                           | -0.002 519 135 658                   | -0.004 223 106 497                    |
| C 0.000 813 558 514                                           | -0.001 021 415 918                   | -8.175 772 400 000 × 10 <sup>-5</sup> |
| C -0.021 318 463 681                                          | 0.006 749 084 151                    | 0.003 762 771 820                     |
| C 0.058 272 976 941                                           | 0.172 419 945 677                    | 0.108 430 174 387                     |
| C -0.004 829 809 200                                          | -0.009 663 983 444                   | 0.016 374 446 402                     |
| C -0.072 463 011 560                                          | -0.160 074 354 408                   | -0.121 305 020 626                    |
| H -0.014 556 648 713                                          | 0.014 798 896 078                    | 0.016 061 246 316                     |
| H 0.002 252 136 929                                           | -0.000 616 126 255                   | 0.001 182 042 741                     |
| H 0.000 484 217 991                                           | -0.002 341 483 180                   | 0.001 997 541 893                     |
| H -0.015 799 027 943                                          | 0.009 284 407 104                    | 0.013 952 121 360                     |
| H 0.051 684 463 876                                           | 0.038 152 705 137                    | 0.050 553 666 188                     |
| H 0.013 124 195 389                                           | 0.038 910 222 595                    | -0.047 346 032 984                    |
| H -0.013 703 903 617                                          | -0.036 417 168 706                   | 0.029 819 643 251                     |
| H -0.001 613 740 580                                          | 0.003 891 815 977                    | -0.001 315 855 604                    |
| H 0.102 427 876 233                                           | -0.480 233 595 592                   | -0.092 474 576 670                    |
| H 0.010 586 397 262                                           | -0.004 790 674 320                   | -0.004 940 536 594                    |
| H 0.050 189 183 054                                           | 0.012 101 430 498                    | -0.017 045 578 045                    |
| H 0.022 388 523 471                                           | -0.035 309 122 403                   | 0.003 425 617 177                     |
| H -0.007 321 640 397                                          | -0.000 925 066 368                   | -0.004 032 955 665                    |
| H -0.034 855 881 562                                          | 0.504 375 452 560                    | 0.098 736 172 981                     |
| H -0.290 334 920 433                                          | -0.129 445 085 147                   | -0.298 195 558 795                    |
| H 0.302 801 324 895                                           | 0.084 186 992 550                    | 0.291 594 129 172                     |

Wavenumber/cm<sup>-1</sup>: 270.2718 , Max excitation: 2

| $l'$ -matrix coefficients/(u <sup>1/2</sup> Å <sup>-1</sup> ) |                                      |                    |                    |
|---------------------------------------------------------------|--------------------------------------|--------------------|--------------------|
| O                                                             | 0.001 483 797 602                    | 0.000 978 703 414  | -0.000 124 176 048 |
| C                                                             | -0.001 622 222 466                   | -0.001 487 346 780 | -0.000 793 708 106 |
| C                                                             | 0.002 327 340 686                    | -0.003 871 145 302 | 0.001 505 695 694  |
| C                                                             | -0.003 122 671 511                   | -0.002 890 500 944 | -0.000 855 294 679 |
| C                                                             | 0.152 133 172 557                    | 0.114 774 627 865  | 0.147 721 213 572  |
| C                                                             | 0.040 765 985 709                    | -0.016 430 887 201 | 0.012 544 328 015  |
| C                                                             | -0.006 294 176 205                   | 0.008 480 434 154  | 0.007 007 698 036  |
| C                                                             | -0.051 991 468 541                   | 0.112 398 912 348  | -0.018 269 702 471 |
| C                                                             | -0.002 374 193 060                   | -0.012 343 174 505 | 0.001 686 525 534  |
| C                                                             | 0.000 860 975 765                    | -0.001 252 212 771 | -0.002 158 221 559 |
| C                                                             | -0.001 882 796 914                   | -0.029 350 425 507 | -0.019 005 705 340 |
| H                                                             | 0.022 010 803 114                    | -0.002 609 415 870 | -0.008 973 169 729 |
| H                                                             | -0.120 677 810 444                   | 0.039 464 607 855  | -0.074 151 960 329 |
| H                                                             | 0.004 522 025 721                    | 0.004 219 625 442  | -0.023 298 099 754 |
| H                                                             | -0.022 516 199 375                   | 0.013 386 254 843  | 0.025 056 791 295  |
| H                                                             | -0.521 263 577 368                   | -0.385 539 145 937 | -0.503 916 015 817 |
| H                                                             | 9.770 376 900 000 × 10 <sup>-5</sup> | 0.000 850 308 378  | -0.000 677 687 900 |
| H                                                             | -0.005 319 827 885                   | -0.016 750 505 044 | 0.022 204 697 088  |
| H                                                             | 0.017 378 861 643                    | -0.030 078 113 326 | 0.004 628 819 073  |
| H                                                             | -0.010 207 381 696                   | 0.049 595 228 369  | 0.008 546 959 795  |
| H                                                             | -0.007 732 352 902                   | 0.003 690 495 730  | 0.003 899 032 733  |
| H                                                             | -0.066 226 089 897                   | -0.007 581 093 664 | 0.020 781 202 854  |
| H                                                             | 0.247 655 417 108                    | -0.370 531 516 343 | 0.038 402 366 982  |
| H                                                             | 0.004 303 118 953                    | 0.000 375 866 609  | 0.003 480 944 674  |
| H                                                             | -0.008 130 094 141                   | 0.113 278 916 218  | 0.023 023 993 075  |
| H                                                             | -0.004 709 329 551                   | -0.001 579 556 936 | -0.005 778 479 780 |
| H                                                             | 0.020 288 100 523                    | 0.005 878 248 868  | 0.020 638 168 523  |



Wavenumber/cm<sup>-1</sup>: 339.0068 , Max excitation: 2

| $l'$ -matrix coefficients/(u <sup>1/2</sup> Å <sup>-1</sup> ) |                                       |                    |
|---------------------------------------------------------------|---------------------------------------|--------------------|
| O -0.000 624 401 034                                          | 4.164 247 600 000 × 10 <sup>-5</sup>  | 0.000 161 882 245  |
| C -0.001 277 985 581                                          | 0.001 882 615 167                     | -0.001 000 415 776 |
| C 0.001 910 129 721                                           | 0.001 233 821 629                     | 0.001 536 880 232  |
| C 0.000 133 742 094                                           | -0.001 200 693 241                    | -0.000 977 758 651 |
| C 0.071 174 991 830                                           | 0.052 294 055 771                     | 0.067 811 424 280  |
| C -0.029 467 014 967                                          | 0.012 563 552 137                     | -0.009 271 210 453 |
| C 0.003 159 311 557                                           | -0.004 389 483 013                    | 0.006 482 287 917  |
| C -0.090 497 912 791                                          | -0.174 326 486 766                    | 0.069 434 949 720  |
| C 0.009 383 363 204                                           | 0.013 801 936 439                     | -0.001 817 402 181 |
| C -0.013 808 080 181                                          | 0.007 183 040 672                     | -0.009 011 785 422 |
| C -0.006 906 933 782                                          | 0.011 561 897 099                     | -0.004 136 962 423 |
| H -0.042 438 969 149                                          | 0.004 410 948 844                     | 0.017 876 748 444  |
| H 0.083 151 666 553                                           | -0.028 299 216 989                    | 0.052 518 370 476  |
| H 0.002 008 007 850                                           | 0.003 838 287 081                     | -0.019 097 045 488 |
| H 0.020 210 632 700                                           | -0.011 902 908 880                    | -0.022 237 963 926 |
| H -0.244 093 920 263                                          | -0.183 505 899 685                    | -0.232 897 635 070 |
| H -0.007 299 135 989                                          | -0.015 772 943 716                    | 0.019 282 142 077  |
| H -0.000 843 309 777                                          | -0.002 112 347 340                    | 0.004 128 498 917  |
| H -0.008 914 327 197                                          | 0.016 284 666 442                     | -0.002 081 788 525 |
| H 0.010 853 491 928                                           | -0.052 220 688 514                    | -0.010 691 399 949 |
| H 0.022 616 755 042                                           | -0.010 109 682 322                    | -0.015 154 138 057 |
| H 0.630 415 018 231                                           | 0.122 855 634 038                     | -0.196 068 967 996 |
| H -0.322 215 158 625                                          | 0.463 358 418 485                     | -0.041 707 575 475 |
| H 0.033 880 726 230                                           | -1.546 938 800 000 × 10 <sup>-5</sup> | 0.027 916 128 465  |
| H 0.001 476 846 324                                           | -0.040 880 573 352                    | -0.010 526 309 068 |
| H -0.002 321 962 544                                          | 0.000 320 695 427                     | -0.002 945 149 522 |
| H 0.019 990 211 684                                           | 0.007 657 833 272                     | 0.020 082 679 540  |

Wavenumber/cm<sup>-1</sup>: 366.8648 , Max excitation: 2

| $l'$ -matrix coefficients/(u <sup>1/2</sup> Å <sup>-1</sup> ) |                                      |                    |                                      |
|---------------------------------------------------------------|--------------------------------------|--------------------|--------------------------------------|
| O                                                             | 0.000 602 918 007                    | 0.000 449 444 762  | 0.000 102 001 476                    |
| C                                                             | -0.000 906 178 035                   | 0.000 159 274 679  | -0.002 223 313 815                   |
| C                                                             | 0.003 133 028 382                    | -0.000 895 643 586 | 0.001 838 194 661                    |
| C                                                             | -0.001 149 626 492                   | 0.000 705 513 942  | 8.789 198 400 000 × 10 <sup>-5</sup> |
| C                                                             | -0.009 262 485 700                   | -0.004 389 013 711 | -0.008 614 308 509                   |
| C                                                             | 0.017 611 118 095                    | -0.010 228 684 782 | -0.025 413 182 162                   |
| C                                                             | -0.002 211 377 349                   | 0.003 777 099 306  | 0.001 505 252 758                    |
| C                                                             | -0.019 458 430 035                   | -0.010 874 222 122 | 0.008 083 006 873                    |
| C                                                             | 0.023 803 981 089                    | -0.040 596 413 111 | 0.063 737 747 146                    |
| C                                                             | -0.000 924 977 785                   | -0.101 400 172 826 | -0.054 630 579 163                   |
| C                                                             | 0.099 859 256 945                    | -0.031 091 338 416 | 0.021 853 289 576                    |
| H                                                             | 0.162 172 810 777                    | -0.014 842 611 151 | -0.062 664 654 609                   |
| H                                                             | 0.018 831 870 343                    | -0.008 504 681 807 | 0.010 042 424 925                    |
| H                                                             | 6.983 400 700 000 × 10 <sup>-5</sup> | 0.001 792 674 157  | -0.009 149 088 943                   |
| H                                                             | -0.082 353 456 496                   | 0.044 943 624 695  | 0.077 664 465 672                    |
| H                                                             | 0.030 099 646 103                    | 0.019 897 591 194  | 0.029 111 180 684                    |
| H                                                             | 0.076 594 116 584                    | 0.201 831 144 065  | -0.255 344 880 204                   |
| H                                                             | -0.029 336 825 097                   | -0.093 958 719 583 | 0.151 399 418 900                    |
| H                                                             | 0.007 257 191 522                    | -0.014 851 816 790 | 0.002 159 910 730                    |
| H                                                             | -0.047 396 100 553                   | 0.250 293 073 558  | 0.053 297 414 029                    |
| H                                                             | -0.359 159 192 857                   | 0.156 409 626 743  | 0.213 031 819 516                    |
| H                                                             | 0.080 050 917 571                    | 0.017 308 400 986  | -0.025 107 565 129                   |
| H                                                             | -0.014 112 451 804                   | 0.017 941 197 796  | -0.001 273 782 307                   |
| H                                                             | 0.281 939 952 187                    | -0.011 526 167 841 | 0.228 609 317 088                    |
| H                                                             | -0.012 502 122 206                   | 0.297 589 669 889  | 0.065 710 003 052                    |
| H                                                             | -0.197 536 109 641                   | -0.097 748 189 892 | -0.207 329 939 862                   |
| H                                                             | -0.298 446 493 462                   | -0.095 803 404 574 | -0.292 047 557 796                   |

Wavenumber/cm<sup>-1</sup>: 390.5976 , Max excitation: 1

| $l'$ -matrix coefficients/(u <sup>1/2</sup> Å <sup>-1</sup> ) |                                       |                                       |
|---------------------------------------------------------------|---------------------------------------|---------------------------------------|
| O                                                             | -1.370 002 300 000 × 10 <sup>-5</sup> | -0.000 421 305 166                    |
| C                                                             | -0.002 745 481 909                    | -0.000 580 951 264                    |
| C                                                             | 0.000 654 607 272                     | 4.087 451 400 000 × 10 <sup>-5</sup>  |
| C                                                             | 0.001 564 206 773                     | 0.000 187 929 599                     |
| C                                                             | -0.005 494 515 544                    | -0.002 027 491 813                    |
| C                                                             | -8.332 269 000 000 × 10 <sup>-6</sup> | -0.001 410 951 041                    |
| C                                                             | -0.000 146 933 255                    | 0.000 152 897 564                     |
| C                                                             | -0.006 948 555 154                    | -0.009 306 710 645                    |
| C                                                             | 0.034 170 292 309                     | -0.049 693 456 795                    |
| C                                                             | -0.011 088 476 132                    | 0.110 179 567 208                     |
| C                                                             | 0.070 296 933 195                     | -0.029 114 282 988                    |
| H                                                             | 0.189 524 212 829                     | -0.017 205 205 603                    |
| H                                                             | 0.012 468 630 742                     | -0.003 028 993 396                    |
| H                                                             | 0.000 811 622 412                     | -8.611 063 400 000 × 10 <sup>-5</sup> |
| H                                                             | -0.013 264 308 327                    | 0.007 802 084 843                     |
| H                                                             | 0.017 419 199 130                     | 0.011 576 289 481                     |
| H                                                             | -0.081 905 209 937                    | -0.215 048 416 291                    |
| H                                                             | -0.023 679 974 843                    | -0.073 195 283 487                    |
| H                                                             | 0.000 295 791 994                     | 0.000 763 394 150                     |
| H                                                             | -0.058 576 277 302                    | 0.309 340 531 328                     |
| H                                                             | 0.401 929 623 886                     | -0.175 459 737 722                    |
| H                                                             | 0.039 082 680 585                     | 0.008 128 290 405                     |
| H                                                             | -0.016 631 640 267                    | 0.023 658 338 647                     |
| H                                                             | -0.278 595 488 314                    | 0.013 507 479 118                     |
| H                                                             | -0.010 802 775 922                    | 0.240 369 530 566                     |
| H                                                             | -0.250 111 537 634                    | -0.125 058 906 560                    |
| H                                                             | -0.204 944 431 822                    | -0.067 995 904 056                    |

Wavenumber/cm<sup>-1</sup>: 417.8993 , Max excitation: 2

| $l'$ -matrix coefficients/(u <sup>1/2</sup> Å <sup>-1</sup> ) |                    |                                        |                                       |
|---------------------------------------------------------------|--------------------|----------------------------------------|---------------------------------------|
| O                                                             | 0.000 334 968 883  | $-7.152\,919\,800\,000 \times 10^{-5}$ | $4.870\,767\,100\,000 \times 10^{-5}$ |
| C                                                             | -0.000 188 351 261 | $-3.496\,293\,000\,000 \times 10^{-5}$ | -0.000 393 012 552                    |
| C                                                             | -0.001 363 184 420 | -0.000 735 916 785                     | 0.002 539 134 321                     |
| C                                                             | 0.000 328 263 772  | -0.000 345 459 062                     | -0.000 101 260 443                    |
| C                                                             | -0.000 935 735 686 | -0.000 728 551 911                     | -0.001 495 026 785                    |
| C                                                             | 0.004 784 962 712  | -0.004 351 072 712                     | -0.012 245 946 930                    |
| C                                                             | 0.001 237 053 762  | -0.001 620 923 344                     | -0.001 110 446 818                    |
| C                                                             | -0.001 841 735 243 | 0.001 644 373 604                      | 0.000 125 730 629                     |
| C                                                             | -0.043 670 864 226 | 0.065 616 600 713                      | -0.098 633 539 729                    |
| C                                                             | -0.009 373 090 318 | 0.017 928 698 978                      | 0.018 141 728 434                     |
| C                                                             | 0.117 921 179 250  | -0.046 686 297 667                     | 0.021 557 807 432                     |
| H                                                             | -0.243 668 113 661 | 0.023 558 300 000                      | 0.092 136 375 362                     |
| H                                                             | 0.015 574 205 926  | -0.004 565 073 116                     | 0.007 759 878 154                     |
| H                                                             | -0.000 472 761 143 | -0.000 943 487 048                     | 0.004 695 215 229                     |
| H                                                             | -0.035 589 108 745 | 0.021 158 010 474                      | 0.034 336 338 826                     |
| H                                                             | 0.004 196 262 985  | 0.003 355 341 020                      | 0.003 848 051 674                     |
| H                                                             | -0.009 214 296 102 | -0.023 936 162 131                     | 0.030 900 785 759                     |
| H                                                             | -0.034 247 096 156 | -0.117 764 150 883                     | 0.185 812 679 886                     |
| H                                                             | -0.001 893 746 896 | 0.004 091 338 123                      | -0.000 678 367 552                    |
| H                                                             | 0.077 123 669 641  | -0.403 577 270 399                     | -0.087 685 165 667                    |
| H                                                             | 0.090 724 442 396  | -0.039 996 961 494                     | -0.054 286 342 308                    |
| H                                                             | 0.002 650 097 891  | 0.001 098 596 218                      | -0.000 951 023 874                    |
| H                                                             | 0.002 388 288 476  | -0.004 067 056 359                     | 0.000 382 811 751                     |
| H                                                             | -0.048 739 328 992 | 0.002 087 493 185                      | -0.038 372 572 424                    |
| H                                                             | -0.016 103 594 121 | 0.390 488 106 650                      | 0.084 905 022 945                     |
| H                                                             | 0.316 463 247 473  | 0.158 293 290 565                      | 0.330 092 639 364                     |
| H                                                             | -0.351 459 107 731 | -0.114 924 536 617                     | -0.345 877 287 157                    |

Wavenumber/cm<sup>-1</sup>: 468.9831 , Max excitation: 2

| $l'$ -matrix coefficients/(u <sup>1/2</sup> Å <sup>-1</sup> ) |                    |                    |                                       |
|---------------------------------------------------------------|--------------------|--------------------|---------------------------------------|
| O                                                             | 0.003 158 373 377  | 0.001 057 880 362  | -0.000 407 331 346                    |
| C                                                             | 0.003 913 492 959  | -0.003 961 771 821 | -0.001 305 514 639                    |
| C                                                             | 0.000 511 031 124  | 0.000 336 330 893  | -5.985 700 900 000 × 10 <sup>-5</sup> |
| C                                                             | -0.003 268 893 048 | 0.000 644 650 636  | 0.000 237 046 552                     |
| C                                                             | -0.001 224 451 065 | -0.000 850 374 018 | 0.000 129 258 642                     |
| C                                                             | 0.129 954 772 933  | -0.086 115 913 269 | -0.196 546 399 447                    |
| C                                                             | -0.003 068 161 342 | 0.004 443 194 165  | 0.005 367 127 016                     |
| C                                                             | -0.009 215 111 868 | 0.004 138 011 169  | 0.003 645 855 956                     |
| C                                                             | -0.003 575 098 488 | 0.001 265 079 344  | -0.005 708 633 182                    |
| C                                                             | -0.003 286 960 289 | 0.009 402 002 118  | 0.007 316 644 588                     |
| C                                                             | -0.017 823 676 760 | 0.010 651 651 391  | 0.008 536 742 811                     |
| H                                                             | -0.008 458 340 098 | 0.000 178 090 235  | 0.003 936 774 793                     |
| H                                                             | 0.164 371 855 103  | -0.055 399 611 031 | 0.076 873 006 526                     |
| H                                                             | 0.001 432 609 784  | 0.004 780 055 587  | -0.023 743 424 883                    |
| H                                                             | -0.632 099 237 773 | 0.349 958 800 028  | 0.594 329 531 919                     |
| H                                                             | 0.004 576 939 823  | 0.003 665 914 866  | 0.004 132 496 596                     |
| H                                                             | -0.006 793 510 485 | -0.013 622 688 812 | 0.020 799 276 114                     |
| H                                                             | 0.010 783 671 204  | 0.035 419 175 614  | -0.055 373 340 236                    |
| H                                                             | 0.008 982 702 069  | -0.020 397 990 813 | 0.004 429 512 009                     |
| H                                                             | 0.002 293 062 704  | -0.012 897 156 250 | -0.002 965 121 092                    |
| H                                                             | 0.041 209 004 561  | -0.015 826 844 278 | -0.026 114 707 764                    |
| H                                                             | 0.026 128 721 975  | 0.003 501 060 354  | -0.009 428 281 935                    |
| H                                                             | 0.009 703 211 071  | -0.014 415 692 359 | 0.001 383 698 568                     |
| H                                                             | -0.024 842 094 035 | 0.001 190 633 358  | -0.020 746 324 131                    |
| H                                                             | 0.004 260 022 118  | -0.086 778 318 486 | -0.018 726 428 873                    |
| H                                                             | 0.017 780 060 356  | 0.008 808 336 919  | 0.018 791 118 725                     |
| H                                                             | 0.047 340 513 295  | 0.014 903 184 957  | 0.049 836 239 758                     |

Wavenumber/cm<sup>-1</sup>: 492.1727 , Max excitation: 1

| $l'$ -matrix coefficients/(u <sup>1/2</sup> Å <sup>-1</sup> ) |                    |                                      |
|---------------------------------------------------------------|--------------------|--------------------------------------|
| O                                                             | -0.001 729 078 268 | -0.000 504 879 011                   |
| C                                                             | -0.000 432 616 122 | -0.000 154 594 385                   |
| C                                                             | -0.000 602 990 121 | 0.001 432 032 142                    |
| C                                                             | -0.001 982 794 476 | -0.004 356 806 481                   |
| C                                                             | 0.003 230 922 294  | 0.000 365 544 347                    |
| C                                                             | 0.004 178 983 813  | -0.003 698 353 471                   |
| C                                                             | 0.120 825 594 179  | -0.235 795 026 295                   |
| C                                                             | -0.001 704 179 359 | 0.008 588 396 695                    |
| C                                                             | -0.001 020 353 446 | -0.000 418 593 774                   |
| C                                                             | 0.001 466 869 970  | -0.001 626 857 976                   |
| C                                                             | 0.001 311 451 739  | 0.001 322 978 512                    |
| H                                                             | 0.008 031 122 578  | 0.000 616 106 325                    |
| H                                                             | 0.000 609 445 409  | -0.000 308 859 940                   |
| H                                                             | 0.016 023 574 798  | -0.022 500 790 251                   |
| H                                                             | -0.015 743 717 952 | 0.010 185 651 038                    |
| H                                                             | -0.012 643 171 566 | -0.010 902 047 747                   |
| H                                                             | 0.000 703 644 667  | 0.002 168 686 425                    |
| H                                                             | -0.000 464 238 193 | -0.002 065 329 921                   |
| H                                                             | -0.411 354 223 172 | 0.852 403 159 087                    |
| H                                                             | -0.001 413 166 624 | 0.006 888 981 587                    |
| H                                                             | -0.009 027 444 882 | 0.003 526 922 608                    |
| H                                                             | -0.012 896 384 339 | -0.000 344 070 664                   |
| H                                                             | 0.017 686 216 006  | -0.023 419 840 377                   |
| H                                                             | 0.003 919 062 529  | -0.000 124 500 012                   |
| H                                                             | 0.000 426 889 358  | -0.000 211 248 114                   |
| H                                                             | -0.004 887 341 829 | -0.003 429 182 333                   |
| H                                                             | -0.004 514 302 597 | -0.001 530 333 180                   |
|                                                               |                    | 4.113 556 000 000 × 10 <sup>-5</sup> |

Wavenumber/cm<sup>-1</sup>: 540.0304 , Max excitation: 1

| $l'$ -matrix coefficients/(u <sup>1/2</sup> Å <sup>-1</sup> ) |                                       |                                       |                                      |
|---------------------------------------------------------------|---------------------------------------|---------------------------------------|--------------------------------------|
| O                                                             | 0.005 530 942 904                     | 0.001 347 456 100                     | -0.001 384 249 544                   |
| C                                                             | 0.001 260 962 215                     | -0.003 789 380 624                    | -0.000 291 885 369                   |
| C                                                             | -8.135 611 200 000 × 10 <sup>-5</sup> | 0.000 158 931 255                     | 0.001 154 087 095                    |
| C                                                             | -0.000 451 648 144                    | 0.010 185 039 096                     | 0.008 961 869 362                    |
| C                                                             | -0.003 227 524 690                    | -0.005 779 931 261                    | -0.004 279 479 330                   |
| C                                                             | -0.005 496 759 227                    | 0.003 730 227 618                     | 0.005 124 476 327                    |
| C                                                             | -0.031 778 316 207                    | -0.063 194 146 497                    | 0.254 770 821 451                    |
| C                                                             | 0.004 014 031 233                     | 0.001 472 624 179                     | -0.003 329 621 070                   |
| C                                                             | 0.006 490 477 719                     | -0.001 028 551 157                    | -0.002 522 991 960                   |
| C                                                             | -0.001 598 970 107                    | 0.001 107 550 471                     | 2.476 260 100 000 × 10 <sup>-5</sup> |
| C                                                             | 0.000 114 643 849                     | 0.001 226 124 514                     | -0.000 757 062 486                   |
| H                                                             | -0.021 486 202 553                    | 0.002 422 300 837                     | 0.010 765 112 662                    |
| H                                                             | -0.000 305 126 615                    | 0.000 695 569 786                     | -0.000 285 294 149                   |
| H                                                             | 0.083 596 233 001                     | 0.212 193 068 814                     | -0.934 820 913 693                   |
| H                                                             | 0.016 450 558 225                     | -0.010 813 887 313                    | -0.015 065 916 686                   |
| H                                                             | 0.015 473 402 524                     | 0.014 699 638 602                     | 0.018 938 043 259                    |
| H                                                             | -0.000 495 058 265                    | -0.001 686 932 165                    | 0.002 051 932 044                    |
| H                                                             | 0.000 157 107 873                     | -0.001 400 566 946                    | 0.001 954 722 175                    |
| H                                                             | -0.002 223 813 032                    | -0.018 192 607 961                    | 0.033 107 015 317                    |
| H                                                             | 0.002 394 326 489                     | -0.001 051 360 595                    | -0.001 869 668 109                   |
| H                                                             | 0.005 633 946 249                     | -0.002 406 927 727                    | -0.002 324 384 193                   |
| H                                                             | -0.012 679 976 274                    | -0.002 097 192 701                    | 0.004 116 615 498                    |
| H                                                             | 0.002 128 606 252                     | -0.001 235 898 510                    | -0.000 715 998 590                   |
| H                                                             | 0.000 574 137 498                     | -7.359 811 400 000 × 10 <sup>-5</sup> | 0.000 515 418 504                    |
| H                                                             | 0.000 178 110 819                     | -0.002 078 385 677                    | -0.000 485 759 447                   |
| H                                                             | -0.003 445 085 775                    | -0.001 132 901 463                    | -0.002 843 280 208                   |
| H                                                             | -0.001 823 052 057                    | -0.000 203 170 780                    | -0.001 085 340 920                   |

Wavenumber/cm<sup>-1</sup>: 589.8313 , Max excitation: 2

| $l'$ -matrix coefficients/(u <sup>1/2</sup> Å <sup>-1</sup> ) |                    |                    |                                       |
|---------------------------------------------------------------|--------------------|--------------------|---------------------------------------|
| O                                                             | -0.015 632 607 632 | -0.005 573 289 335 | -0.000 766 110 873                    |
| C                                                             | 0.006 146 867 639  | 0.003 490 601 253  | 0.005 025 855 741                     |
| C                                                             | -0.054 786 125 983 | -0.045 304 909 062 | -0.060 484 980 826                    |
| C                                                             | 0.021 781 849 500  | 0.016 514 517 808  | 0.015 790 418 626                     |
| C                                                             | 0.012 922 180 334  | 0.029 498 211 561  | 0.017 185 197 998                     |
| C                                                             | -0.000 308 605 790 | 0.000 683 219 789  | -0.033 721 948 946                    |
| C                                                             | -0.056 646 445 629 | 0.032 261 775 844  | 0.052 930 272 647                     |
| C                                                             | 0.053 919 798 415  | 0.134 053 978 328  | -0.062 290 217 833                    |
| C                                                             | -0.067 980 341 966 | -0.069 805 062 774 | -0.006 254 072 670                    |
| C                                                             | 0.009 517 581 662  | 0.007 280 876 587  | -0.001 881 932 997                    |
| C                                                             | 0.002 139 704 231  | -0.026 625 330 553 | -0.084 976 376 932                    |
| H                                                             | 0.049 285 787 890  | 0.361 206 307 620  | 0.078 371 593 854                     |
| H                                                             | -0.028 051 258 519 | 0.024 339 232 278  | 0.051 660 846 162                     |
| H                                                             | 0.101 900 178 715  | -0.189 479 216 573 | -0.026 081 502 665                    |
| H                                                             | 0.044 096 705 759  | -0.005 239 142 369 | 0.041 988 493 564                     |
| H                                                             | 0.004 789 753 819  | 0.017 290 568 303  | -2.603 915 800 000 × 10 <sup>-5</sup> |
| H                                                             | -0.022 116 544 739 | -0.008 643 927 742 | -0.015 723 144 623                    |
| H                                                             | -0.017 348 818 112 | 0.282 064 816 988  | 0.157 724 125 109                     |
| H                                                             | 0.061 282 204 997  | -0.001 462 672 020 | -0.203 540 340 478                    |
| H                                                             | 0.335 122 764 608  | 0.073 636 264 980  | -0.095 978 830 157                    |
| H                                                             | 0.003 941 605 182  | -0.000 297 428 125 | 0.003 764 881 355                     |
| H                                                             | 0.119 982 234 711  | -0.366 837 161 644 | 0.062 569 530 753                     |
| H                                                             | -0.312 270 289 029 | -0.169 251 233 342 | 0.150 217 390 153                     |
| H                                                             | -0.014 006 165 835 | -0.017 152 243 728 | 0.019 837 186 999                     |
| H                                                             | -0.034 787 015 268 | -0.078 217 548 012 | 0.314 890 657 072                     |
| H                                                             | -0.077 920 338 456 | -0.119 273 304 935 | 0.111 762 688 450                     |
| H                                                             | 0.101 388 707 667  | -0.063 706 662 261 | -0.100 632 469 461                    |



Wavenumber/cm<sup>-1</sup>: 634.12 , Max excitation: 2

| $l'$ -matrix coefficients/(u <sup>1/2</sup> Å <sup>-1</sup> ) |                    |                    |
|---------------------------------------------------------------|--------------------|--------------------|
| O                                                             | -0.008 221 359 036 | -0.003 632 110 032 |
| C                                                             | 0.014 673 926 330  | 0.027 226 394 121  |
| C                                                             | -0.045 384 580 197 | -0.059 946 499 490 |
| C                                                             | 0.010 336 001 700  | 0.002 413 669 769  |
| C                                                             | 0.000 580 236 390  | -0.003 899 030 528 |
| C                                                             | 0.008 224 079 310  | 0.004 476 929 652  |
| C                                                             | 0.008 914 603 018  | 0.004 256 700 616  |
| C                                                             | -0.054 039 109 278 | -0.145 508 716 926 |
| C                                                             | -0.039 237 883 662 | -0.057 548 373 208 |
| C                                                             | -0.006 305 146 821 | 0.008 404 623 586  |
| C                                                             | -0.045 078 615 037 | -0.062 210 993 415 |
| H                                                             | 0.070 784 153 388  | 0.293 836 294 332  |
| H                                                             | 0.153 967 150 209  | -0.097 185 156 330 |
| H                                                             | 0.000 693 131 183  | -0.020 276 499 987 |
| H                                                             | -0.222 165 751 616 | 0.054 050 301 256  |
| H                                                             | -0.017 835 100 477 | 0.011 045 757 347  |
| H                                                             | 0.027 831 542 672  | -0.037 506 571 462 |
| H                                                             | 0.215 725 921 694  | 0.137 916 697 395  |
| H                                                             | -0.000 132 281 522 | -0.005 073 946 136 |
| H                                                             | 0.247 568 535 659  | 0.059 279 628 384  |
| H                                                             | 0.010 651 157 205  | -0.034 091 746 809 |
| H                                                             | -0.118 549 574 991 | 0.368 323 485 278  |
| H                                                             | 0.318 997 710 284  | 0.173 693 576 387  |
| H                                                             | -0.016 408 270 657 | 0.009 772 448 694  |
| H                                                             | -0.120 312 653 261 | -0.030 745 010 411 |
| H                                                             | -0.124 456 923 105 | -0.072 047 116 803 |
| H                                                             | 0.114 929 635 172  | 0.178 094 766 583  |
|                                                               |                    | -0.001 116 411 271 |
|                                                               |                    | 0.014 903 853 210  |
|                                                               |                    | -0.034 577 666 448 |
|                                                               |                    | -0.004 704 571 268 |
|                                                               |                    | -0.002 305 298 545 |
|                                                               |                    | 0.138 701 310 407  |
|                                                               |                    | 0.004 105 282 217  |
|                                                               |                    | 0.061 103 985 248  |
|                                                               |                    | -0.032 259 521 329 |
|                                                               |                    | -0.007 025 351 783 |
|                                                               |                    | 0.005 316 465 318  |
|                                                               |                    | 0.125 173 662 188  |
|                                                               |                    | -0.271 320 312 441 |
|                                                               |                    | -0.002 613 796 708 |
|                                                               |                    | -0.236 438 239 258 |
|                                                               |                    | 0.004 454 613 562  |
|                                                               |                    | -0.025 382 035 601 |
|                                                               |                    | 0.145 600 880 756  |
|                                                               |                    | -0.009 417 674 268 |
|                                                               |                    | -0.099 971 028 802 |
|                                                               |                    | 0.044 298 692 925  |
|                                                               |                    | -0.055 927 447 119 |
|                                                               |                    | -0.136 817 113 994 |
|                                                               |                    | 0.016 323 830 128  |
|                                                               |                    | 0.057 428 904 784  |
|                                                               |                    | 0.134 030 014 963  |
|                                                               |                    | -0.188 396 506 841 |

Wavenumber/cm<sup>-1</sup>: 689.337 , Max excitation: 2

| $l'$ -matrix coefficients/(u <sup>1/2</sup> Å <sup>-1</sup> ) |                    |                    |
|---------------------------------------------------------------|--------------------|--------------------|
| O                                                             | -0.027 691 732 048 | -0.008 910 498 895 |
| C                                                             | 0.041 617 767 401  | -0.011 537 096 642 |
| C                                                             | -0.068 020 544 352 | 0.089 476 248 401  |
| C                                                             | 0.037 088 001 524  | 0.016 246 656 378  |
| C                                                             | -0.000 124 412 458 | -0.038 360 318 615 |
| C                                                             | -0.013 094 207 862 | -0.014 862 422 058 |
| C                                                             | 0.002 562 999 734  | 0.006 988 002 177  |
| C                                                             | -0.029 843 383 406 | -0.078 700 738 511 |
| C                                                             | -0.105 457 821 183 | -0.010 370 151 477 |
| C                                                             | 0.066 977 701 808  | 0.011 850 798 356  |
| C                                                             | 0.045 320 308 941  | 0.085 110 127 082  |
| H                                                             | -0.057 542 470 007 | 0.227 783 689 263  |
| H                                                             | -0.047 964 212 358 | 0.050 199 059 230  |
| H                                                             | 0.009 195 936 421  | -0.038 093 678 118 |
| H                                                             | 0.085 043 792 793  | -0.021 785 826 519 |
| H                                                             | -0.015 975 499 139 | 0.016 752 421 655  |
| H                                                             | -0.253 750 018 298 | 0.005 465 856 445  |
| H                                                             | -0.268 718 163 560 | -0.128 124 674 700 |
| H                                                             | -0.002 061 625 693 | -0.008 986 364 507 |
| H                                                             | 0.374 933 522 618  | 0.046 236 801 777  |
| H                                                             | 0.051 696 141 804  | 0.121 627 635 929  |
| H                                                             | -0.071 111 355 470 | 0.217 322 292 750  |
| H                                                             | 0.189 623 276 652  | 0.104 928 254 839  |
| H                                                             | -0.109 850 946 746 | -0.155 096 063 698 |
| H                                                             | 0.218 852 765 870  | 0.021 053 082 573  |
| H                                                             | 0.160 011 141 983  | -0.299 440 464 860 |
| H                                                             | -0.072 751 799 357 | -0.317 104 358 221 |
|                                                               |                    | 0.188 986 774 324  |

Wavenumber/cm<sup>-1</sup>: 723.5275 , Max excitation: 1

| $l'$ -matrix coefficients/(u <sup>1/2</sup> Å <sup>-1</sup> ) |                    |                    |
|---------------------------------------------------------------|--------------------|--------------------|
| O                                                             | -0.018 630 539 926 | -0.003 998 484 256 |
| C                                                             | 0.025 127 706 821  | -0.006 762 876 809 |
| C                                                             | 0.043 228 533 806  | -0.067 563 772 686 |
| C                                                             | 0.019 174 192 243  | 0.016 019 783 051  |
| C                                                             | -0.004 928 629 116 | 0.024 865 067 520  |
| C                                                             | -0.013 631 697 499 | -0.006 494 680 508 |
| C                                                             | -0.045 968 715 776 | 0.029 670 648 086  |
| C                                                             | 0.004 413 324 107  | 0.023 534 777 120  |
| C                                                             | -0.000 735 667 959 | -0.024 244 601 800 |
| C                                                             | 0.079 899 803 405  | 0.014 327 969 449  |
| C                                                             | 0.009 262 518 130  | -0.036 216 042 036 |
| H                                                             | 0.064 523 961 979  | 0.096 208 842 941  |
| H                                                             | -0.066 883 380 670 | 0.057 508 710 602  |
| H                                                             | 0.084 185 341 082  | -0.146 093 871 798 |
| H                                                             | 0.096 061 665 702  | -0.036 622 596 502 |
| H                                                             | 0.014 100 170 421  | -0.013 205 532 490 |
| H                                                             | -0.258 870 984 657 | -0.071 145 029 782 |
| H                                                             | 0.178 002 583 928  | -0.230 083 347 779 |
| H                                                             | 0.045 201 818 337  | -0.002 617 292 106 |
| H                                                             | 0.029 514 567 667  | 0.022 629 758 543  |
| H                                                             | 0.178 021 307 779  | 0.117 905 932 011  |
| H                                                             | 0.018 221 672 185  | -0.043 075 862 055 |
| H                                                             | -0.042 917 072 393 | -0.018 128 685 668 |
| H                                                             | -0.253 040 364 439 | -0.083 464 500 271 |
| H                                                             | -0.195 671 930 815 | 0.072 202 402 406  |
| H                                                             | -0.121 198 778 225 | 0.060 892 419 667  |
| H                                                             | -0.094 907 307 086 | 0.346 463 924 920  |

Wavenumber/cm<sup>-1</sup>: 810.2768 , Max excitation: 1

| $l'$ -matrix coefficients/(u <sup>1/2</sup> Å <sup>-1</sup> ) |                    |                    |                    |
|---------------------------------------------------------------|--------------------|--------------------|--------------------|
| O                                                             | -0.002 668 595 237 | 0.001 141 945 770  | 0.002 326 369 003  |
| C                                                             | 0.061 951 059 718  | -0.004 338 861 410 | 0.019 694 239 621  |
| C                                                             | -0.028 514 255 706 | 0.013 909 797 775  | -0.015 566 902 193 |
| C                                                             | -0.004 226 065 087 | -0.016 060 731 994 | -0.019 175 174 924 |
| C                                                             | 0.005 442 726 076  | -0.010 865 728 643 | -0.010 105 425 591 |
| C                                                             | 0.002 913 989 111  | 0.009 452 143 478  | 0.061 496 948 063  |
| C                                                             | 0.056 400 043 303  | -0.043 588 553 109 | -0.058 350 733 350 |
| C                                                             | 0.011 878 241 139  | 0.041 673 742 709  | 0.002 921 243 964  |
| C                                                             | 0.018 356 105 556  | 0.068 695 693 103  | 0.010 168 789 843  |
| C                                                             | 0.125 061 110 006  | -0.008 255 654 279 | -0.016 023 564 511 |
| C                                                             | -0.033 594 552 984 | -0.052 825 402 264 | -0.042 150 329 720 |
| H                                                             | -0.058 574 443 707 | -0.205 201 256 335 | -0.107 008 382 462 |
| H                                                             | 0.086 830 785 784  | -0.035 418 647 783 | -0.146 916 396 694 |
| H                                                             | -0.112 647 723 062 | 0.208 843 173 418  | 0.028 805 347 028  |
| H                                                             | -0.117 844 693 924 | 0.017 286 124 712  | -0.122 949 203 152 |
| H                                                             | -0.010 161 176 443 | 0.009 293 157 096  | -0.003 249 719 070 |
| H                                                             | -0.475 249 247 888 | 0.059 614 590 663  | -0.102 360 451 284 |
| H                                                             | 0.102 229 588 512  | 0.210 975 717 012  | 0.153 851 825 945  |
| H                                                             | -0.057 963 523 676 | 0.008 209 137 945  | 0.227 579 305 070  |
| H                                                             | -0.113 941 378 556 | -0.038 994 011 842 | 0.142 890 064 110  |
| H                                                             | 0.091 128 059 135  | 0.258 515 912 248  | -0.082 131 073 346 |
| H                                                             | 0.031 645 705 031  | -0.111 799 866 724 | 0.012 809 325 307  |
| H                                                             | -0.090 033 346 486 | -0.051 829 385 251 | 0.026 910 530 578  |
| H                                                             | -0.181 570 009 365 | -0.275 730 951 324 | 0.238 101 567 030  |
| H                                                             | -0.051 930 753 171 | -0.051 486 248 320 | 0.181 266 954 621  |
| H                                                             | 0.117 878 427 937  | -0.054 556 935 505 | -0.078 847 316 395 |
| H                                                             | 0.106 352 240 068  | 0.055 336 517 151  | -0.146 424 224 056 |

Wavenumber/cm<sup>-1</sup>: 853.5702 , Max excitation: 1

| $l'$ -matrix coefficients/(u <sup>1/2</sup> Å <sup>-1</sup> ) |                                       |                    |
|---------------------------------------------------------------|---------------------------------------|--------------------|
| O                                                             | -0.021 709 530 417                    | -0.008 884 749 001 |
| C                                                             | 0.019 386 656 674                     | -0.020 558 566 465 |
| C                                                             | -0.019 527 440 064                    | 0.023 552 095 183  |
| C                                                             | 0.031 183 864 494                     | 0.027 732 428 217  |
| C                                                             | 0.013 628 502 167                     | 0.006 355 900 828  |
| C                                                             | 0.014 453 757 142                     | 0.026 313 336 094  |
| C                                                             | -0.059 643 065 320                    | 0.043 917 524 408  |
| C                                                             | 0.015 918 600 784                     | 0.051 205 667 649  |
| C                                                             | -0.047 141 256 885                    | 0.033 419 108 292  |
| C                                                             | 0.006 375 497 359                     | -0.049 139 834 853 |
| C                                                             | 0.001 336 108 430                     | -0.001 542 339 519 |
| H                                                             | -0.068 175 227 166                    | -0.001 499 676 456 |
| H                                                             | 0.143 959 815 817                     | -0.085 862 385 038 |
| H                                                             | 0.115 058 517 352                     | -0.224 859 886 724 |
| H                                                             | -0.208 163 622 058                    | 0.030 091 805 006  |
| H                                                             | -7.213 284 900 000 × 10 <sup>-5</sup> | -0.000 726 045 018 |
| H                                                             | -0.093 297 184 182                    | 0.189 063 534 207  |
| H                                                             | 0.076 957 272 574                     | -0.205 373 648 616 |
| H                                                             | 0.061 523 679 552                     | -0.009 425 867 176 |
| H                                                             | 0.108 221 961 929                     | 0.004 380 406 516  |
| H                                                             | -0.151 316 755 707                    | 0.124 341 500 526  |
| H                                                             | 0.037 900 094 670                     | -0.137 442 926 418 |
| H                                                             | -0.119 630 764 752                    | -0.063 757 877 181 |
| H                                                             | 0.191 755 980 172                     | -0.116 452 141 598 |
| H                                                             | -0.020 066 585 814                    | 0.061 947 929 132  |
| H                                                             | 0.154 680 424 618                     | -0.150 008 270 844 |
| H                                                             | -0.059 896 075 583                    | 0.133 370 312 676  |

Wavenumber/cm<sup>-1</sup>: 860.4897 , Max excitation: 1

| $l'$ -matrix coefficients/(u <sup>1/2</sup> Å <sup>-1</sup> ) |                    |                    |                    |
|---------------------------------------------------------------|--------------------|--------------------|--------------------|
| O                                                             | 0.012 754 504 708  | 0.005 785 499 208  | -0.001 738 418 118 |
| C                                                             | 0.036 491 673 814  | -0.013 740 807 226 | 0.057 456 125 777  |
| C                                                             | 0.021 115 744 408  | -0.034 283 290 247 | -0.041 229 009 069 |
| C                                                             | -0.024 884 068 071 | -0.012 728 101 517 | -0.001 783 588 655 |
| C                                                             | -0.007 026 152 265 | -0.001 616 433 878 | 0.014 425 961 035  |
| C                                                             | -0.016 000 521 669 | -0.014 389 366 218 | -0.087 357 211 996 |
| C                                                             | 0.015 848 742 657  | -0.006 487 193 565 | -0.019 942 326 730 |
| C                                                             | -0.014 908 721 462 | -0.035 417 904 192 | 0.009 738 197 057  |
| C                                                             | 0.055 288 721 740  | -0.078 967 195 663 | -0.036 811 092 605 |
| C                                                             | 0.052 743 157 918  | -0.068 766 967 683 | 0.095 350 153 561  |
| C                                                             | -0.016 921 767 434 | 0.020 345 492 415  | -0.000 963 672 106 |
| H                                                             | 0.127 365 671 111  | 0.110 849 767 436  | 0.254 565 759 416  |
| H                                                             | -0.080 701 428 293 | 0.082 461 679 281  | 0.152 699 378 763  |
| H                                                             | -0.024 834 935 908 | 0.053 544 128 619  | 0.007 647 859 415  |
| H                                                             | 0.131 164 601 061  | -0.036 300 170 443 | 0.139 698 172 120  |
| H                                                             | -0.000 499 940 750 | 0.009 406 452 206  | -0.004 642 672 997 |
| H                                                             | -0.271 129 105 296 | 0.247 357 063 245  | 0.146 942 369 484  |
| H                                                             | -0.017 714 521 649 | -0.000 210 434 099 | -0.004 552 867 751 |
| H                                                             | -0.015 481 584 458 | 0.002 139 092 248  | 0.062 598 949 221  |
| H                                                             | -0.089 369 840 594 | 0.014 230 189 137  | -0.246 602 060 037 |
| H                                                             | -0.142 109 498 877 | 0.241 525 676 564  | -0.427 318 636 208 |
| H                                                             | -0.033 689 717 726 | 0.096 071 878 199  | -0.023 190 162 509 |
| H                                                             | 0.087 936 325 958  | 0.050 377 188 244  | -0.032 773 423 376 |
| H                                                             | 0.162 972 146 954  | -0.216 789 443 219 | -0.173 413 378 219 |
| H                                                             | 0.033 456 375 449  | -0.001 072 758 911 | 0.032 994 294 697  |
| H                                                             | -0.284 225 109 176 | 0.226 384 873 339  | 0.162 877 966 274  |
| H                                                             | 0.014 817 464 879  | -0.053 658 859 238 | -0.002 231 721 503 |

Wavenumber/cm<sup>-1</sup>: 895.7501 , Max excitation: 1

| $l'$ -matrix coefficients/(u <sup>1/2</sup> Å <sup>-1</sup> ) |                    |                    |                    |
|---------------------------------------------------------------|--------------------|--------------------|--------------------|
| O                                                             | -0.029 010 329 656 | -0.008 853 028 765 | 0.000 299 351 917  |
| C                                                             | 0.013 493 235 734  | -0.009 452 163 984 | -0.019 593 049 950 |
| C                                                             | 0.030 473 881 870  | 0.024 535 143 619  | -0.014 491 227 485 |
| C                                                             | 0.037 356 302 334  | 0.029 889 878 678  | 0.018 456 645 951  |
| C                                                             | 0.006 588 878 387  | 0.011 462 320 753  | -0.001 031 348 936 |
| C                                                             | 0.018 464 523 001  | 0.024 167 603 164  | 0.120 084 210 527  |
| C                                                             | -0.077 994 008 632 | 0.064 545 294 006  | 0.086 755 808 824  |
| C                                                             | -0.009 131 244 723 | -0.019 204 016 569 | 0.001 941 628 762  |
| C                                                             | 0.095 487 634 528  | -0.036 122 697 785 | 0.004 348 425 326  |
| C                                                             | 0.034 372 423 006  | 0.022 494 469 963  | -0.031 651 509 723 |
| C                                                             | 0.003 811 298 376  | 0.081 195 468 043  | -0.053 081 333 789 |
| H                                                             | 0.056 180 203 270  | -0.123 287 647 995 | 0.115 358 719 799  |
| H                                                             | 0.130 977 408 920  | -0.093 579 230 563 | -0.231 725 092 439 |
| H                                                             | 0.151 945 519 820  | -0.281 688 665 655 | -0.038 991 483 703 |
| H                                                             | -0.193 137 717 062 | 0.026 510 552 878  | -0.197 816 401 629 |
| H                                                             | -0.005 214 823 205 | -0.011 636 598 114 | 0.020 006 224 265  |
| H                                                             | -0.109 160 444 770 | -0.058 425 787 588 | -0.091 799 273 478 |
| H                                                             | -0.209 751 223 815 | -0.011 240 804 796 | -0.075 140 698 589 |
| H                                                             | 0.075 557 655 975  | -0.010 534 733 260 | -0.317 443 595 501 |
| H                                                             | -0.296 984 234 824 | -0.038 163 519 723 | -0.152 830 713 697 |
| H                                                             | 0.081 485 820 593  | 0.030 478 909 036  | 0.100 520 811 250  |
| H                                                             | -0.007 701 791 324 | 0.021 504 741 133  | 0.001 904 737 633  |
| H                                                             | 0.022 907 714 241  | 0.013 697 104 365  | 0.005 010 104 404  |
| H                                                             | -0.125 171 209 799 | -0.048 570 489 059 | 0.153 046 547 807  |
| H                                                             | 0.201 333 062 130  | -0.008 141 219 745 | 0.157 799 650 564  |
| H                                                             | -0.157 338 649 999 | 0.281 791 811 227  | 0.038 582 951 969  |
| H                                                             | -0.028 234 961 136 | -0.321 440 725 030 | 0.126 606 470 352  |

Wavenumber/cm<sup>-1</sup>: 926.6705 , Max excitation: 1

| $l'$ -matrix coefficients/(u <sup>1/2</sup> Å <sup>-1</sup> ) |                    |                    |                    |
|---------------------------------------------------------------|--------------------|--------------------|--------------------|
| O                                                             | 0.026 650 615 616  | 0.009 216 359 753  | 0.001 210 721 487  |
| C                                                             | -0.003 499 903 537 | 0.024 808 164 627  | 0.015 489 498 932  |
| C                                                             | 0.019 171 171 811  | -0.003 629 604 960 | -0.014 269 297 349 |
| C                                                             | -0.038 287 987 422 | -0.041 812 284 435 | -0.030 218 291 699 |
| C                                                             | -0.014 696 665 790 | -0.004 196 307 359 | -0.002 769 092 026 |
| C                                                             | 0.016 378 794 127  | 0.015 143 259 990  | 0.095 636 361 979  |
| C                                                             | 0.094 270 297 697  | -0.063 876 456 408 | -0.096 122 493 264 |
| C                                                             | 0.036 775 319 257  | 0.081 201 803 465  | -0.010 871 220 603 |
| C                                                             | -0.018 491 173 173 | -0.064 242 428 329 | -0.046 500 705 201 |
| C                                                             | -0.004 935 676 224 | 0.010 385 887 432  | -0.017 649 790 391 |
| C                                                             | 0.017 096 521 119  | 0.071 935 904 023  | 0.053 687 282 349  |
| H                                                             | 0.095 498 180 797  | 0.223 354 394 698  | 0.184 055 128 080  |
| H                                                             | 0.119 780 810 813  | -0.085 440 864 881 | -0.216 331 324 692 |
| H                                                             | -0.177 189 137 033 | 0.329 768 127 375  | 0.047 506 075 063  |
| H                                                             | -0.171 281 763 283 | 0.040 625 387 997  | -0.189 896 336 842 |
| H                                                             | -0.001 867 660 007 | -0.001 028 551 826 | -0.006 174 964 607 |
| H                                                             | 0.034 048 430 821  | -0.043 648 921 029 | -0.030 537 907 157 |
| H                                                             | -0.124 466 534 206 | -0.236 897 089 515 | -0.173 422 709 318 |
| H                                                             | -0.094 993 568 327 | 0.014 463 940 757  | 0.373 645 417 734  |
| H                                                             | 0.151 388 743 802  | 0.041 828 358 256  | -0.121 670 227 055 |
| H                                                             | 0.018 632 824 058  | -0.042 200 182 587 | 0.063 693 282 385  |
| H                                                             | 0.065 169 640 906  | -0.222 596 291 311 | 0.021 273 195 326  |
| H                                                             | -0.195 109 810 658 | -0.112 625 706 407 | 0.077 407 737 716  |
| H                                                             | -0.030 426 524 377 | 0.021 794 649 480  | 0.032 145 098 011  |
| H                                                             | 0.120 359 089 206  | 0.061 376 375 454  | -0.183 012 534 909 |
| H                                                             | -0.176 590 789 759 | 0.010 534 303 383  | 0.145 105 455 263  |
| H                                                             | -0.097 379 191 973 | -0.124 804 496 946 | 0.156 374 929 864  |



Wavenumber/cm<sup>-1</sup>: 946.8875 , Max excitation: 1

| $l'$ -matrix coefficients/(u <sup>1/2</sup> Å <sup>-1</sup> ) |                    |                    |                    |
|---------------------------------------------------------------|--------------------|--------------------|--------------------|
| O                                                             | 0.008 316 135 894  | 0.003 725 710 093  | -0.002 300 668 899 |
| C                                                             | 0.019 111 414 175  | -0.030 487 419 162 | -0.002 705 452 248 |
| C                                                             | -0.020 843 553 626 | 0.003 871 802 478  | -0.002 332 877 194 |
| C                                                             | -0.013 491 548 757 | -0.003 861 215 699 | 0.005 550 698 675  |
| C                                                             | 0.024 269 045 735  | -0.037 905 392 305 | 0.010 390 184 048  |
| C                                                             | -0.016 885 093 371 | -0.015 446 465 962 | -0.022 999 588 895 |
| C                                                             | -0.014 179 955 793 | 0.023 671 234 637  | 0.014 750 215 012  |
| C                                                             | 0.004 627 963 124  | 0.029 374 585 609  | -0.005 640 836 703 |
| C                                                             | 0.026 232 790 692  | 0.133 974 131 047  | -0.223 520 865 862 |
| C                                                             | 0.021 217 751 475  | 0.203 995 436 630  | 0.071 760 023 781  |
| C                                                             | -0.232 260 931 915 | 0.062 734 551 937  | 0.080 737 735 666  |
| H                                                             | 0.110 940 042 109  | -0.167 601 841 514 | 0.239 638 974 470  |
| H                                                             | -0.014 452 890 180 | 0.047 137 674 008  | 0.038 794 575 109  |
| H                                                             | 0.026 521 401 387  | -0.038 383 386 781 | -0.004 642 304 779 |
| H                                                             | 0.037 809 554 739  | -0.001 057 081 654 | 0.040 181 259 576  |
| H                                                             | -0.020 146 874 451 | 0.040 014 298 137  | -0.011 211 027 979 |
| H                                                             | 0.013 669 914 705  | -0.182 226 879 663 | -0.170 749 277 624 |
| H                                                             | 0.264 404 609 110  | -0.132 051 136 440 | 0.000 834 717 313  |
| H                                                             | -0.002 542 634 620 | -0.004 984 588 674 | -0.046 042 461 320 |
| H                                                             | -0.036 669 128 983 | -0.046 246 780 770 | 0.301 122 038 076  |
| H                                                             | -0.140 373 015 231 | -0.221 276 241 555 | -0.025 084 487 632 |
| H                                                             | 0.010 467 787 012  | -0.022 670 358 448 | 0.010 116 501 665  |
| H                                                             | -0.027 351 540 892 | -0.011 196 501 244 | -0.011 420 212 926 |
| H                                                             | 0.046 620 974 499  | -0.233 198 868 591 | -0.040 903 071 321 |
| H                                                             | 0.319 740 796 333  | 0.052 621 818 848  | -0.051 992 592 344 |
| H                                                             | -0.136 557 279 923 | -0.228 747 575 261 | 0.202 850 505 423  |
| H                                                             | 0.212 784 157 881  | -0.141 937 481 623 | -0.206 843 280 581 |

Wavenumber/cm<sup>-1</sup>: 955.2112 , Max excitation: 1

| $l'$ -matrix coefficients/(u <sup>1/2</sup> Å <sup>-1</sup> ) |                    |                    |                    |
|---------------------------------------------------------------|--------------------|--------------------|--------------------|
| O                                                             | 0.045 314 206 394  | 0.016 432 842 567  | -0.001 303 222 929 |
| C                                                             | 0.019 149 531 210  | 0.092 867 963 366  | 0.036 508 849 571  |
| C                                                             | 0.007 306 729 929  | -0.029 046 403 872 | 0.005 759 251 629  |
| C                                                             | -0.061 472 428 604 | -0.022 295 262 312 | 0.001 644 698 916  |
| C                                                             | 0.002 818 644 344  | -0.006 915 792 848 | -0.003 074 657 773 |
| C                                                             | -0.003 260 560 555 | -0.006 052 652 788 | -0.014 844 662 896 |
| C                                                             | -0.014 522 980 628 | 0.003 616 119 813  | 0.002 820 929 220  |
| C                                                             | -0.000 992 397 844 | 0.003 637 250 556  | 0.012 868 066 256  |
| C                                                             | 0.002 810 162 548  | 0.089 644 236 148  | -0.138 718 593 945 |
| C                                                             | -0.067 973 571 312 | -0.369 056 686 495 | -0.152 208 581 851 |
| C                                                             | -0.120 567 676 992 | 0.046 245 729 470  | 0.029 825 036 281  |
| H                                                             | 0.064 159 921 490  | -0.091 501 925 324 | 0.140 854 913 623  |
| H                                                             | -0.005 087 530 386 | 0.002 053 601 266  | 0.003 656 608 310  |
| H                                                             | 0.023 606 203 962  | -0.022 059 070 829 | -0.003 128 859 141 |
| H                                                             | 0.003 984 721 266  | -0.001 170 882 860 | -0.001 218 709 154 |
| H                                                             | 0.005 601 189 762  | -0.001 964 314 327 | -0.006 314 761 806 |
| H                                                             | 0.040 294 802 092  | 0.292 607 180 488  | 0.294 313 463 656  |
| H                                                             | 0.115 022 307 860  | -0.057 429 268 447 | -0.002 312 807 308 |
| H                                                             | 0.009 992 297 278  | 0.000 269 340 044  | -0.030 087 254 323 |
| H                                                             | 0.007 812 390 748  | -0.022 116 209 851 | 0.186 825 531 623  |
| H                                                             | 0.260 148 569 040  | 0.348 800 141 299  | 0.099 728 497 549  |
| H                                                             | -0.001 438 599 463 | -0.008 709 133 265 | -0.005 617 261 811 |
| H                                                             | -0.008 208 403 036 | -0.006 165 652 586 | -0.015 637 002 451 |
| H                                                             | -0.088 361 001 235 | 0.437 551 774 127  | 0.066 687 322 700  |
| H                                                             | 0.171 391 798 101  | 0.021 653 921 816  | 0.009 696 909 816  |
| H                                                             | -0.069 246 079 799 | -0.164 349 337 906 | 0.119 292 896 385  |
| H                                                             | 0.106 891 772 720  | -0.111 672 339 876 | -0.094 114 663 704 |

Wavenumber/cm<sup>-1</sup>: 960.4353 , Max excitation: 1

| $l'$ -matrix coefficients/(u <sup>1/2</sup> Å <sup>-1</sup> ) |                    |                    |
|---------------------------------------------------------------|--------------------|--------------------|
| O                                                             | -0.066 365 893 430 | -0.022 106 585 102 |
| C                                                             | 0.016 573 155 505  | -0.007 039 397 275 |
| C                                                             | -0.043 192 955 364 | -0.025 076 984 652 |
| C                                                             | 0.085 083 268 876  | 0.031 877 669 102  |
| C                                                             | 0.007 469 152 178  | 0.003 442 606 986  |
| C                                                             | -0.008 609 340 807 | 0.008 356 772 441  |
| C                                                             | 0.008 493 063 845  | 0.002 243 230 121  |
| C                                                             | -0.008 359 408 197 | -0.007 055 998 997 |
| C                                                             | 0.035 098 047 875  | 0.149 374 517 024  |
| C                                                             | -0.007 552 384 092 | 0.012 368 686 446  |
| C                                                             | 0.278 904 602 421  | -0.062 744 946 037 |
| H                                                             | 0.128 106 939 753  | -0.172 365 218 547 |
| H                                                             | 0.019 274 786 660  | -0.005 969 470 029 |
| H                                                             | -0.013 234 799 270 | -0.011 238 955 688 |
| H                                                             | -0.019 180 893 175 | -0.007 548 761 140 |
| H                                                             | -0.017 841 231 116 | -0.004 940 676 299 |
| H                                                             | 0.011 274 659 389  | -0.005 014 526 988 |
| H                                                             | -0.309 164 631 362 | 0.154 595 594 102  |
| H                                                             | -0.002 002 631 798 | -0.006 101 830 985 |
| H                                                             | -0.038 192 433 190 | -0.053 653 005 535 |
| H                                                             | -0.023 341 057 164 | -0.004 680 513 454 |
| H                                                             | -0.004 292 500 517 | 0.015 874 485 668  |
| H                                                             | 0.021 704 722 320  | 0.011 162 295 543  |
| H                                                             | 0.030 565 124 703  | -0.017 716 085 753 |
| H                                                             | -0.361 843 844 150 | -0.061 394 419 667 |
| H                                                             | -0.160 145 793 141 | -0.250 369 846 825 |
| H                                                             | -0.253 480 416 522 | 0.142 401 539 408  |

Wavenumber/cm<sup>-1</sup>: 963.7768 , Max excitation: 1

| $l'$ -matrix coefficients/(u <sup>1/2</sup> Å <sup>-1</sup> ) |                    |                    |                    |
|---------------------------------------------------------------|--------------------|--------------------|--------------------|
| O                                                             | 0.507 685 851 704  | 0.177 207 805 082  | -0.010 286 276 810 |
| C                                                             | -0.078 346 998 573 | 0.107 671 318 176  | 0.088 035 807 927  |
| C                                                             | 0.115 710 899 949  | -0.090 332 347 072 | -0.058 493 607 369 |
| C                                                             | -0.652 514 250 269 | -0.295 675 665 977 | -0.043 620 214 942 |
| C                                                             | 0.033 750 931 642  | 0.101 796 939 017  | 0.071 619 574 075  |
| C                                                             | 0.023 263 909 529  | -0.034 841 548 264 | -0.012 861 266 488 |
| C                                                             | -0.100 870 133 750 | -0.005 139 646 434 | -0.001 225 933 013 |
| C                                                             | -0.017 049 950 906 | -0.029 739 418 889 | -0.040 163 443 657 |
| C                                                             | -0.035 352 051 124 | 0.034 767 488 530  | -0.001 366 598 268 |
| C                                                             | 0.034 620 101 850  | 0.006 098 839 749  | -0.005 986 529 273 |
| C                                                             | 0.029 812 081 633  | 0.021 547 506 214  | 0.001 879 647 212  |
| H                                                             | -0.001 451 171 931 | -0.042 261 822 080 | 0.025 920 932 417  |
| H                                                             | 0.007 712 470 245  | -0.003 948 130 967 | -0.002 414 287 765 |
| H                                                             | 0.145 450 592 417  | 0.003 632 118 123  | 0.013 555 116 941  |
| H                                                             | 0.013 501 133 236  | 0.073 273 489 976  | -0.050 399 272 065 |
| H                                                             | 0.116 840 833 170  | -0.039 453 675 474 | -0.027 066 326 542 |
| H                                                             | -0.049 063 980 050 | -0.025 691 438 329 | -0.039 370 986 484 |
| H                                                             | -0.070 865 823 311 | 0.014 746 637 881  | -0.009 265 402 693 |
| H                                                             | 0.120 395 743 233  | 0.060 613 031 370  | -0.029 552 832 432 |
| H                                                             | 0.033 327 913 489  | 0.010 449 133 569  | 0.020 797 318 678  |
| H                                                             | -0.030 091 137 357 | -0.061 467 286 224 | -0.022 639 278 913 |
| H                                                             | 0.005 692 000 941  | 0.032 204 030 798  | 0.040 548 234 636  |
| H                                                             | 0.028 243 147 037  | 0.020 012 443 480  | 0.037 860 395 277  |
| H                                                             | -0.010 522 585 004 | -0.055 125 744 827 | 0.019 068 988 148  |
| H                                                             | -0.085 635 324 321 | -0.005 400 435 057 | 0.025 612 514 954  |
| H                                                             | 0.027 567 076 693  | -0.054 089 748 080 | -0.004 934 769 722 |
| H                                                             | -0.040 414 424 643 | 0.001 132 217 762  | 0.050 795 175 170  |

Wavenumber/cm<sup>-1</sup>: 1000.216 , Max excitation: 1

| $l'$ -matrix coefficients/(u <sup>1/2</sup> Å <sup>-1</sup> ) |                    |                    |                    |
|---------------------------------------------------------------|--------------------|--------------------|--------------------|
| O                                                             | 0.078 927 249 174  | 0.025 350 699 913  | -0.005 690 654 347 |
| C                                                             | 0.007 738 039 748  | -0.019 068 103 613 | 0.107 413 214 094  |
| C                                                             | -0.041 992 975 757 | 0.159 817 674 192  | -0.075 217 136 583 |
| C                                                             | -0.102 846 105 610 | -0.031 702 116 166 | 0.010 996 446 944  |
| C                                                             | -0.099 825 769 033 | -0.273 552 027 935 | 0.074 407 587 042  |
| C                                                             | 0.019 997 929 476  | 0.032 834 328 848  | -0.103 022 661 331 |
| C                                                             | 0.064 186 940 829  | 0.057 532 516 284  | -0.005 075 624 651 |
| C                                                             | 0.137 947 808 341  | 0.161 945 203 579  | 0.371 901 116 002  |
| C                                                             | 0.017 105 405 214  | -0.044 829 230 380 | 0.014 189 084 795  |
| C                                                             | -0.009 765 591 769 | 0.015 309 239 975  | -0.052 458 572 594 |
| C                                                             | 0.032 641 614 785  | -0.058 785 101 218 | 0.016 125 228 617  |
| H                                                             | 0.004 491 830 395  | 0.021 827 102 385  | 0.003 883 060 512  |
| H                                                             | -0.024 565 807 283 | -0.037 251 970 893 | -0.007 738 892 087 |
| H                                                             | -0.001 034 063 916 | -0.074 362 364 271 | -0.024 985 898 206 |
| H                                                             | -0.005 096 125 401 | -0.030 786 741 764 | -0.020 948 765 250 |
| H                                                             | 0.039 341 654 292  | 0.234 854 840 458  | -0.295 056 593 888 |
| H                                                             | 0.018 875 428 388  | 0.023 143 760 120  | 0.010 536 623 393  |
| H                                                             | -0.049 443 216 471 | 0.034 580 568 403  | 0.021 691 814 133  |
| H                                                             | -0.099 067 219 899 | -0.056 260 087 429 | -0.049 115 333 732 |
| H                                                             | -0.025 290 812 360 | -0.017 824 176 592 | 0.017 597 582 591  |
| H                                                             | 0.011 760 537 937  | -0.028 984 933 417 | 0.036 203 834 435  |
| H                                                             | -0.106 111 674 210 | -0.117 578 977 661 | -0.470 445 124 502 |
| H                                                             | -0.100 227 265 150 | -0.098 302 764 091 | -0.424 228 837 420 |
| H                                                             | -0.025 421 023 718 | -0.036 449 863 006 | 0.013 672 992 085  |
| H                                                             | -0.006 038 530 929 | -0.004 581 769 274 | -0.036 843 966 919 |
| H                                                             | -0.024 897 672 903 | 0.032 443 926 233  | 0.011 047 597 418  |
| H                                                             | -0.008 674 596 771 | 0.056 251 998 424  | -0.002 752 488 671 |

Wavenumber/cm<sup>-1</sup>: 1017.8055 , Max excitation: 1

| $l'$ -matrix coefficients/(u <sup>1/2</sup> Å <sup>-1</sup> ) |                    |                    |                    |
|---------------------------------------------------------------|--------------------|--------------------|--------------------|
| O                                                             | 0.089 416 363 782  | 0.029 631 525 011  | -0.006 304 857 834 |
| C                                                             | -0.126 152 749 462 | -0.254 520 448 327 | -0.161 410 907 664 |
| C                                                             | 0.097 467 067 963  | 0.039 991 185 829  | 0.107 453 176 791  |
| C                                                             | -0.116 627 186 851 | -0.031 114 732 949 | 0.015 913 763 124  |
| C                                                             | 0.112 929 566 490  | 0.105 596 623 340  | -0.206 599 816 817 |
| C                                                             | 0.167 553 555 134  | 0.389 350 982 751  | -0.064 152 923 503 |
| C                                                             | 0.031 848 393 325  | 0.046 527 208 323  | 0.074 758 617 496  |
| C                                                             | -0.051 226 739 200 | -0.088 279 731 762 | 0.147 372 079 660  |
| C                                                             | -0.041 023 570 417 | -0.033 025 679 839 | -0.044 310 800 843 |
| C                                                             | 0.032 782 037 335  | 0.057 851 111 371  | 0.071 632 785 553  |
| C                                                             | -0.039 143 395 478 | 0.002 012 423 954  | -0.026 233 653 226 |
| H                                                             | 0.014 553 671 925  | 0.028 448 570 222  | 0.040 382 977 182  |
| H                                                             | -0.179 153 383 891 | -0.403 735 030 654 | 0.082 219 097 103  |
| H                                                             | -0.134 074 796 226 | -0.038 117 703 901 | -0.001 914 466 248 |
| H                                                             | -0.163 328 747 098 | -0.400 484 204 763 | 0.059 050 877 418  |
| H                                                             | -0.136 628 417 386 | -0.126 075 505 715 | 0.237 340 546 335  |
| H                                                             | -0.027 077 635 689 | 0.003 380 097 462  | -0.003 506 003 695 |
| H                                                             | 0.040 927 009 318  | 0.013 139 120 610  | 0.012 548 144 509  |
| H                                                             | -0.029 776 106 539 | -0.008 012 439 854 | -0.005 625 676 201 |
| H                                                             | 0.044 469 622 777  | -0.008 209 195 227 | 0.041 789 145 929  |
| H                                                             | -0.001 950 156 745 | 0.043 827 081 429  | -0.020 465 932 261 |
| H                                                             | -0.033 370 394 219 | -0.054 637 346 210 | -0.030 217 547 809 |
| H                                                             | -0.018 645 732 500 | -0.045 665 286 589 | -0.098 255 342 769 |
| H                                                             | 0.012 609 624 766  | 0.056 209 245 374  | 0.010 695 856 643  |
| H                                                             | 0.028 841 268 809  | -0.002 735 992 858 | 0.027 747 096 848  |
| H                                                             | 0.004 116 161 791  | 0.018 315 368 616  | -0.033 403 699 277 |
| H                                                             | -0.013 893 574 283 | -0.002 807 497 157 | 0.002 146 572 300  |

Wavenumber/cm<sup>-1</sup>: 1034.5678 , Max excitation: 1

| $l'$ -matrix coefficients/(u <sup>1/2</sup> Å <sup>-1</sup> ) |                    |                    |
|---------------------------------------------------------------|--------------------|--------------------|
| O                                                             | -0.114 484 061 603 | -0.034 865 542 142 |
| C                                                             | -0.097 491 915 631 | -0.041 810 324 583 |
| C                                                             | 0.236 425 535 160  | -0.153 038 209 281 |
| C                                                             | 0.159 985 669 582  | 0.068 349 001 255  |
| C                                                             | -0.348 331 579 869 | 0.224 998 638 856  |
| C                                                             | 0.093 700 721 205  | 0.073 802 451 677  |
| C                                                             | -0.104 742 569 655 | -0.150 156 579 789 |
| C                                                             | 0.076 922 566 610  | -0.010 786 011 821 |
| C                                                             | -0.074 906 405 558 | 0.063 756 032 220  |
| C                                                             | 0.048 250 456 872  | 0.017 217 809 601  |
| C                                                             | -0.068 023 627 388 | 0.031 792 026 710  |
| H                                                             | 0.005 383 814 500  | -0.059 051 827 168 |
| H                                                             | -0.045 152 328 598 | -0.114 148 845 621 |
| H                                                             | 0.156 711 220 743  | 0.104 608 703 980  |
| H                                                             | -0.063 057 605 378 | -0.104 734 635 516 |
| H                                                             | 0.410 653 514 178  | -0.193 796 582 263 |
| H                                                             | -0.034 607 425 381 | -0.009 129 430 836 |
| H                                                             | 0.047 195 003 128  | -0.006 618 691 088 |
| H                                                             | 0.225 485 678 763  | 0.095 891 239 240  |
| H                                                             | 0.057 334 839 172  | 0.030 726 327 617  |
| H                                                             | -0.026 201 433 120 | -0.008 736 470 366 |
| H                                                             | -0.077 021 138 598 | -0.011 786 624 204 |
| H                                                             | 0.037 312 768 664  | 0.026 680 713 786  |
| H                                                             | 0.011 357 057 996  | 0.041 017 594 894  |
| H                                                             | 0.013 684 911 050  | -0.004 938 743 202 |
| H                                                             | 0.037 975 521 528  | -0.040 337 344 226 |
| H                                                             | -0.030 957 285 775 | -0.035 214 943 317 |

Wavenumber/cm<sup>-1</sup>: 1074.6724 , Max excitation: 1

| $l'$ -matrix coefficients/(u <sup>1/2</sup> Å <sup>-1</sup> ) |                    |                    |
|---------------------------------------------------------------|--------------------|--------------------|
| O                                                             | -0.000 250 125 163 | -0.005 417 973 034 |
| C                                                             | 0.092 160 185 207  | 0.319 185 076 281  |
| C                                                             | 0.101 813 160 307  | -0.304 859 671 113 |
| C                                                             | -0.042 036 604 384 | -0.002 262 162 583 |
| C                                                             | -0.128 097 872 677 | 0.172 872 999 276  |
| C                                                             | -0.032 013 807 382 | -0.135 460 326 279 |
| C                                                             | 0.202 237 378 728  | 0.031 087 837 547  |
| C                                                             | 0.011 244 712 203  | 0.002 379 739 246  |
| C                                                             | -0.045 902 831 013 | 0.069 794 484 230  |
| C                                                             | -0.009 650 491 525 | -0.081 807 368 364 |
| C                                                             | -0.033 163 763 131 | 0.098 473 103 737  |
| H                                                             | -0.006 462 313 096 | -0.022 052 541 667 |
| H                                                             | 0.070 039 047 625  | 0.202 444 424 285  |
| H                                                             | -0.331 264 765 433 | -0.151 054 003 134 |
| H                                                             | 0.029 045 391 465  | 0.054 563 474 739  |
| H                                                             | -0.086 895 770 948 | -0.223 018 444 683 |
| H                                                             | -0.015 442 715 943 | -0.060 252 920 548 |
| H                                                             | 0.110 961 069 918  | -0.049 722 480 646 |
| H                                                             | -0.065 800 923 098 | -0.067 751 392 952 |
| H                                                             | 0.038 515 166 799  | 0.037 997 726 169  |
| H                                                             | -0.025 749 916 412 | -0.057 979 506 541 |
| H                                                             | -0.083 897 731 354 | -0.094 320 087 845 |
| H                                                             | -0.002 291 904 367 | -0.008 678 533 301 |
| H                                                             | 0.002 523 873 520  | -0.059 639 306 078 |
| H                                                             | -0.036 350 925 830 | -0.003 301 448 985 |
| H                                                             | 0.048 672 660 663  | 0.007 721 231 791  |
| H                                                             | -0.047 070 507 064 | -0.068 149 076 435 |
|                                                               |                    | 0.050 279 762 967  |



Wavenumber/cm<sup>-1</sup>: 1105.0316 , Max excitation: 1

| $l'$ -matrix coefficients/(u <sup>1/2</sup> Å <sup>-1</sup> ) |                    |                    |                    |
|---------------------------------------------------------------|--------------------|--------------------|--------------------|
| O                                                             | 0.044 558 379 784  | 0.006 413 016 118  | -0.012 291 149 723 |
| C                                                             | -0.040 862 826 203 | -0.112 339 237 494 | 0.016 482 470 202  |
| C                                                             | 0.140 218 183 012  | 0.219 950 921 507  | -0.284 352 554 295 |
| C                                                             | -0.103 624 478 322 | 0.011 900 463 054  | 0.051 582 421 019  |
| C                                                             | -0.227 994 154 946 | -0.037 134 873 353 | 0.116 124 767 129  |
| C                                                             | 0.146 388 670 819  | -0.034 596 682 490 | 0.040 442 225 232  |
| C                                                             | 0.287 492 746 166  | 0.131 145 893 245  | 0.018 424 891 041  |
| C                                                             | -0.045 611 568 420 | -0.026 933 079 726 | -0.168 544 929 852 |
| C                                                             | -0.025 015 014 040 | -0.047 123 305 518 | 0.065 993 329 271  |
| C                                                             | 0.001 832 586 139  | 0.026 658 703 435  | -0.010 192 727 913 |
| C                                                             | -0.034 759 663 573 | -0.100 273 277 522 | 0.076 026 361 775  |
| H                                                             | 0.008 040 909 406  | -0.036 290 764 891 | 0.059 945 150 767  |
| H                                                             | 0.045 303 429 214  | 0.113 112 948 558  | 0.073 755 014 112  |
| H                                                             | -0.249 414 911 016 | -0.175 482 153 745 | -0.074 060 451 741 |
| H                                                             | -0.076 430 282 826 | -0.123 166 187 672 | -0.046 548 939 976 |
| H                                                             | -0.021 755 984 022 | 0.002 920 883 764  | -0.024 716 867 372 |
| H                                                             | 0.013 548 870 848  | 0.029 877 678 516  | 0.018 626 236 349  |
| H                                                             | -0.110 386 651 912 | 0.062 076 726 357  | 0.050 534 181 913  |
| H                                                             | -0.262 278 766 414 | -0.143 515 112 319 | -0.069 504 874 673 |
| H                                                             | 0.000 339 986 188  | -0.020 747 462 008 | 0.057 050 018 368  |
| H                                                             | 0.012 206 438 817  | 0.005 914 745 532  | 0.017 628 452 882  |
| H                                                             | -0.041 020 487 269 | -0.042 982 725 688 | -0.155 861 406 688 |
| H                                                             | 0.127 811 383 089  | 0.137 292 752 501  | 0.477 811 485 841  |
| H                                                             | -0.007 125 056 421 | 0.013 849 661 211  | 0.007 953 896 272  |
| H                                                             | 0.043 849 433 191  | -0.000 167 834 209 | -0.072 457 202 563 |
| H                                                             | -0.006 041 841 665 | -0.028 926 457 156 | 0.029 060 743 361  |
| H                                                             | 0.007 312 585 019  | 0.072 789 829 693  | -0.030 944 484 232 |

Wavenumber/cm<sup>-1</sup>: 1124.7939 , Max excitation: 1

| $l'$ -matrix coefficients/(u <sup>1/2</sup> Å <sup>-1</sup> ) |                    |                    |
|---------------------------------------------------------------|--------------------|--------------------|
| O                                                             | -0.025 554 134 806 | -0.019 731 980 636 |
| C                                                             | -0.218 984 733 566 | 0.007 913 099 080  |
| C                                                             | 0.328 167 858 838  | 0.018 692 290 669  |
| C                                                             | 0.008 467 782 203  | 0.068 751 827 743  |
| C                                                             | -0.124 963 362 945 | -0.063 765 502 533 |
| C                                                             | -0.119 511 406 933 | 0.002 823 172 432  |
| C                                                             | 0.153 130 060 461  | 0.079 473 358 197  |
| C                                                             | 0.193 314 501 738  | -0.054 056 141 037 |
| C                                                             | -0.114 485 912 655 | -0.001 590 340 902 |
| C                                                             | 0.089 045 444 428  | -0.003 938 440 530 |
| C                                                             | -0.090 179 536 885 | -0.005 985 057 165 |
| H                                                             | 0.016 173 959 746  | -0.050 777 768 473 |
| H                                                             | -0.119 543 285 277 | -0.339 058 246 830 |
| H                                                             | -0.132 983 311 037 | -0.108 304 246 734 |
| H                                                             | 0.195 081 627 369  | 0.441 694 643 845  |
| H                                                             | 0.064 808 873 405  | -0.067 809 813 752 |
| H                                                             | -0.069 894 721 780 | 0.024 731 241 839  |
| H                                                             | 0.017 218 574 761  | 0.027 335 370 108  |
| H                                                             | -0.215 928 637 083 | -0.114 004 705 185 |
| H                                                             | 0.071 180 734 617  | 0.015 824 621 042  |
| H                                                             | -0.036 570 347 104 | -0.040 047 477 246 |
| H                                                             | 0.088 890 445 031  | 0.187 770 126 005  |
| H                                                             | -0.121 478 864 559 | -0.148 246 172 709 |
| H                                                             | -0.007 751 279 110 | 0.057 585 301 584  |
| H                                                             | 0.021 110 332 994  | -0.006 088 467 827 |
| H                                                             | 0.039 413 566 920  | 0.011 314 994 802  |
| H                                                             | -0.066 926 453 718 | 0.019 900 615 270  |

Wavenumber/cm<sup>-1</sup>: 1153.5657 , Max excitation: 1

| $l'$ -matrix coefficients/(u <sup>1/2</sup> Å <sup>-1</sup> ) |                    |                    |
|---------------------------------------------------------------|--------------------|--------------------|
| O                                                             | -0.031 328 646 761 | -0.013 080 751 308 |
| C                                                             | 0.051 329 544 358  | 0.302 216 959 632  |
| C                                                             | -0.206 170 872 060 | 0.261 340 656 605  |
| C                                                             | 0.050 156 391 207  | -0.005 829 792 062 |
| C                                                             | -0.096 640 689 656 | 0.204 304 952 384  |
| C                                                             | 0.008 553 626 461  | 0.048 454 654 986  |
| C                                                             | -0.009 321 024 610 | -0.116 653 845 084 |
| C                                                             | 0.093 047 507 176  | -0.183 768 238 355 |
| C                                                             | 0.128 118 339 701  | -0.122 156 503 843 |
| C                                                             | -0.025 358 475 679 | -0.107 611 729 987 |
| C                                                             | 0.073 442 052 070  | -0.122 663 450 793 |
| H                                                             | -0.000 610 256 156 | 0.072 691 027 176  |
| H                                                             | -0.118 703 999 712 | -0.273 408 691 158 |
| H                                                             | -0.055 339 770 821 | 0.006 111 566 945  |
| H                                                             | 0.085 760 125 676  | 0.147 415 924 651  |
| H                                                             | 0.041 345 170 060  | -0.271 197 364 976 |
| H                                                             | -0.000 101 275 724 | -0.025 675 185 290 |
| H                                                             | -0.169 519 317 232 | 0.046 921 282 116  |
| H                                                             | 0.213 858 324 668  | 0.068 583 974 889  |
| H                                                             | -0.096 707 192 484 | -0.079 575 339 714 |
| H                                                             | -0.013 906 470 059 | -0.075 712 551 695 |
| H                                                             | -0.026 856 043 877 | 0.023 401 899 808  |
| H                                                             | -0.050 514 466 681 | -0.101 313 563 626 |
| H                                                             | -0.027 083 030 285 | -0.089 769 720 687 |
| H                                                             | 0.065 409 436 435  | 0.010 518 063 699  |
| H                                                             | -0.077 012 526 548 | -0.010 033 314 012 |
| H                                                             | 0.122 974 461 938  | 0.059 008 220 014  |

Wavenumber/cm<sup>-1</sup>: 1172.5141 , Max excitation: 1

| $l'$ -matrix coefficients/(u <sup>1/2</sup> Å <sup>-1</sup> ) |                    |                    |                    |
|---------------------------------------------------------------|--------------------|--------------------|--------------------|
| O                                                             | 0.055 951 097 464  | 0.021 710 305 582  | 0.000 702 136 479  |
| C                                                             | -0.026 039 445 302 | -0.311 507 950 561 | 0.009 430 324 508  |
| C                                                             | 0.069 171 906 993  | 0.401 002 993 907  | 0.325 696 076 848  |
| C                                                             | -0.049 270 912 327 | -0.022 488 159 746 | -0.004 023 979 955 |
| C                                                             | -0.034 179 024 323 | 0.028 545 864 391  | -0.136 792 730 529 |
| C                                                             | -0.060 389 275 885 | -0.115 588 730 489 | -0.017 099 312 051 |
| C                                                             | -0.054 904 233 386 | -0.032 366 419 208 | 0.010 364 052 685  |
| C                                                             | -0.021 935 959 524 | 0.047 715 741 183  | 0.020 826 499 434  |
| C                                                             | -0.029 255 000 217 | -0.187 515 652 004 | -0.142 205 174 528 |
| C                                                             | -0.010 521 138 009 | 0.125 428 912 770  | -0.044 200 905 110 |
| C                                                             | -0.032 057 941 370 | -0.158 473 642 921 | -0.106 144 862 942 |
| H                                                             | 0.041 012 896 734  | 0.153 761 506 541  | 0.044 186 723 185  |
| H                                                             | 0.121 599 249 671  | 0.283 489 498 845  | -0.068 042 949 748 |
| H                                                             | 0.010 144 369 227  | 0.023 196 836 666  | 0.013 937 601 091  |
| H                                                             | 0.055 759 714 733  | 0.134 960 009 075  | -0.030 004 636 447 |
| H                                                             | 0.135 075 440 093  | -0.303 232 017 456 | 0.050 693 704 997  |
| H                                                             | 0.039 714 462 055  | 0.113 216 810 364  | 0.066 101 001 568  |
| H                                                             | 0.050 346 915 545  | 0.096 437 449 093  | 0.070 326 866 379  |
| H                                                             | 0.090 123 586 022  | 0.044 326 536 084  | 0.018 934 496 903  |
| H                                                             | 0.025 035 998 941  | -0.085 060 339 339 | 0.200 850 374 587  |
| H                                                             | 0.026 776 357 549  | 0.021 399 331 595  | 0.049 195 343 436  |
| H                                                             | -0.001 273 307 032 | -0.020 680 371 894 | -0.003 334 036 971 |
| H                                                             | 0.005 029 450 017  | 0.015 109 317 861  | -0.051 029 268 110 |
| H                                                             | -0.018 819 277 652 | -0.021 668 452 053 | 0.010 656 473 947  |
| H                                                             | 0.196 466 755 344  | -0.028 849 954 112 | -0.013 125 829 664 |
| H                                                             | -0.034 314 020 028 | 0.169 486 900 137  | -0.107 135 127 465 |
| H                                                             | -0.104 733 493 254 | 0.095 160 027 911  | 0.035 476 199 603  |

Wavenumber/cm<sup>-1</sup>: 1188.9917 , Max excitation: 1

| $l'$ -matrix coefficients/(u <sup>1/2</sup> Å <sup>-1</sup> ) |                    |                    |
|---------------------------------------------------------------|--------------------|--------------------|
| O                                                             | -0.066 708 256 068 | -0.024 207 643 888 |
| C                                                             | -0.131 305 703 211 | -0.306 410 750 063 |
| C                                                             | 0.281 411 924 270  | -0.079 110 388 115 |
| C                                                             | 0.095 353 897 159  | 0.060 186 533 538  |
| C                                                             | 0.120 478 373 980  | 0.103 129 647 162  |
| C                                                             | 0.018 749 840 688  | -0.058 825 936 781 |
| C                                                             | -0.143 988 459 400 | -0.010 333 433 815 |
| C                                                             | -0.018 966 529 365 | -0.030 790 631 501 |
| C                                                             | -0.128 495 885 543 | 0.029 375 052 122  |
| C                                                             | 0.072 406 607 765  | 0.149 528 363 136  |
| C                                                             | -0.083 550 513 575 | 0.078 834 626 755  |
| H                                                             | -0.001 954 474 000 | -0.148 915 178 427 |
| H                                                             | 0.059 835 682 413  | 0.150 453 703 633  |
| H                                                             | 0.055 605 483 651  | 0.075 928 098 310  |
| H                                                             | 0.071 991 417 485  | 0.172 069 189 629  |
| H                                                             | -0.231 504 465 679 | 0.018 130 866 997  |
| H                                                             | 0.027 974 804 258  | 0.193 726 998 295  |
| H                                                             | -0.093 493 743 832 | -0.016 955 235 132 |
| H                                                             | 0.160 022 707 298  | 0.101 022 854 221  |
| H                                                             | 0.064 195 144 393  | 0.040 588 555 339  |
| H                                                             | 0.004 793 039 314  | -0.086 481 915 873 |
| H                                                             | -0.052 526 632 537 | -0.067 405 383 699 |
| H                                                             | 0.001 779 738 514  | -0.014 178 627 597 |
| H                                                             | -0.053 200 336 932 | -0.024 721 011 146 |
| H                                                             | -0.120 646 335 878 | 0.021 609 782 429  |
| H                                                             | 0.053 999 185 916  | -0.076 820 349 490 |
| H                                                             | 0.035 514 364 433  | -0.019 241 134 495 |

Wavenumber/cm<sup>-1</sup>: 1215.938 , Max excitation: 1

| $l'$ -matrix coefficients/(u <sup>1/2</sup> Å <sup>-1</sup> ) |                    |                    |
|---------------------------------------------------------------|--------------------|--------------------|
| O                                                             | -0.081 162 342 356 | -0.018 494 748 339 |
| C                                                             | 0.235 564 072 859  | 0.357 114 492 523  |
| C                                                             | 0.391 514 982 150  | 0.142 156 260 779  |
| C                                                             | 0.058 989 792 002  | 0.008 686 459 566  |
| C                                                             | 0.029 003 959 422  | -0.157 581 320 793 |
| C                                                             | 0.003 568 217 674  | 0.049 585 311 061  |
| C                                                             | -0.085 616 899 907 | 0.062 228 823 887  |
| C                                                             | -0.148 958 080 368 | -0.009 205 242 176 |
| C                                                             | -0.158 476 445 554 | -0.057 183 865 717 |
| C                                                             | -0.135 417 014 207 | -0.155 492 751 148 |
| C                                                             | -0.155 469 771 147 | -0.067 002 725 714 |
| H                                                             | 0.019 161 967 250  | -0.077 286 340 784 |
| H                                                             | 0.020 000 207 509  | 0.079 325 955 343  |
| H                                                             | 0.233 432 688 010  | 0.063 571 604 631  |
| H                                                             | -0.112 276 416 766 | -0.271 978 460 903 |
| H                                                             | 0.036 861 892 133  | -0.178 419 969 585 |
| H                                                             | 0.041 962 858 574  | -0.123 292 383 781 |
| H                                                             | -0.047 395 098 577 | 0.075 411 262 591  |
| H                                                             | -0.129 531 976 099 | -0.028 673 696 798 |
| H                                                             | 0.092 500 758 635  | 0.009 733 500 648  |
| H                                                             | 0.017 274 199 853  | 0.018 429 260 598  |
| H                                                             | 0.020 691 776 726  | -0.056 400 694 807 |
| H                                                             | -0.007 230 445 270 | -0.002 736 270 746 |
| H                                                             | 0.012 895 256 592  | -0.142 889 691 860 |
| H                                                             | 0.062 160 685 521  | -0.004 656 698 427 |
| H                                                             | 0.060 168 023 302  | 0.032 682 154 796  |
| H                                                             | -0.117 112 593 753 | 0.082 617 799 757  |

Wavenumber/cm<sup>-1</sup>: 1218.1807 , Max excitation: 1

| $l'$ -matrix coefficients/(u <sup>1/2</sup> Å <sup>-1</sup> ) |                    |                    |                    |
|---------------------------------------------------------------|--------------------|--------------------|--------------------|
| O                                                             | 0.008 496 645 058  | 0.009 413 365 641  | -0.001 978 198 507 |
| C                                                             | 0.285 295 472 279  | -0.263 065 019 475 | 0.236 860 501 035  |
| C                                                             | -0.066 495 597 973 | -0.118 327 550 672 | -0.069 284 692 273 |
| C                                                             | -0.059 080 992 498 | -0.004 250 050 547 | 0.028 808 399 063  |
| C                                                             | -0.108 849 232 851 | 0.171 956 484 283  | 0.089 396 019 297  |
| C                                                             | -0.202 416 779 573 | 0.198 332 376 151  | -0.123 794 273 881 |
| C                                                             | 0.122 989 852 438  | -0.007 238 946 146 | -0.044 740 241 760 |
| C                                                             | 0.107 195 534 941  | -0.088 359 672 530 | -0.017 057 963 878 |
| C                                                             | 0.008 492 462 498  | 0.069 137 416 970  | 0.030 167 288 878  |
| C                                                             | -0.159 323 790 057 | 0.134 168 710 037  | -0.142 198 266 229 |
| C                                                             | 0.013 275 460 510  | 0.044 802 988 218  | 0.008 504 713 742  |
| H                                                             | -0.016 486 914 843 | -0.043 316 069 391 | -0.026 885 532 267 |
| H                                                             | 0.046 921 741 042  | 0.056 063 112 647  | -0.201 693 365 506 |
| H                                                             | -0.186 475 538 515 | -0.112 366 994 904 | -0.056 625 085 635 |
| H                                                             | -0.006 568 734 085 | -0.187 561 423 017 | 0.150 861 921 401  |
| H                                                             | 0.199 629 910 739  | -0.085 351 839 741 | -0.111 951 114 970 |
| H                                                             | 0.153 831 546 100  | 0.131 438 633 092  | 0.103 223 987 193  |
| H                                                             | 0.000 405 989 422  | -0.033 930 381 799 | -0.027 160 304 018 |
| H                                                             | -0.009 191 248 040 | -0.024 106 663 478 | -0.018 119 414 934 |
| H                                                             | -0.008 991 495 847 | 0.033 367 759 249  | -0.085 957 791 369 |
| H                                                             | 0.095 701 080 549  | 0.058 487 097 982  | 0.166 758 368 316  |
| H                                                             | 0.060 493 385 185  | 0.165 271 401 481  | 0.222 106 263 670  |
| H                                                             | -0.102 111 056 793 | -0.118 274 181 877 | -0.088 992 365 139 |
| H                                                             | -0.030 599 419 048 | -0.254 085 806 969 | -0.050 617 024 047 |
| H                                                             | -0.058 691 662 525 | 0.004 351 220 974  | 0.015 391 131 446  |
| H                                                             | 0.007 306 556 676  | -0.059 739 508 988 | 0.034 530 967 771  |
| H                                                             | 0.024 357 062 729  | -0.041 212 508 294 | -0.005 464 844 549 |

Wavenumber/cm<sup>-1</sup>: 1245.7664 , Max excitation: 1

| $l'$ -matrix coefficients/(u <sup>1/2</sup> Å <sup>-1</sup> ) |                    |                    |
|---------------------------------------------------------------|--------------------|--------------------|
| O                                                             | -0.033 781 778 452 | -0.021 905 526 641 |
| C                                                             | -0.154 872 791 320 | 0.092 099 082 462  |
| C                                                             | -0.095 786 291 194 | -0.038 720 856 743 |
| C                                                             | 0.053 650 552 879  | 0.077 307 515 321  |
| C                                                             | 0.081 145 705 652  | -0.071 209 061 917 |
| C                                                             | 0.170 960 065 727  | 0.041 373 282 098  |
| C                                                             | 0.017 972 191 497  | -0.018 448 106 792 |
| C                                                             | -0.141 888 570 040 | 0.008 855 753 642  |
| C                                                             | -0.022 465 046 738 | -0.001 083 374 502 |
| C                                                             | 0.112 454 021 973  | -0.001 519 948 608 |
| C                                                             | 0.061 555 147 809  | 0.046 512 023 043  |
| H                                                             | 0.011 361 250 148  | 0.047 261 633 534  |
| H                                                             | -0.104 847 918 898 | -0.171 678 957 984 |
| H                                                             | 0.124 970 927 783  | 0.024 530 681 885  |
| H                                                             | -0.044 565 594 491 | -0.023 470 134 182 |
| H                                                             | 0.034 408 063 193  | 0.027 874 717 762  |
| H                                                             | 0.008 253 895 792  | 0.288 233 280 099  |
| H                                                             | 0.120 979 452 059  | -0.044 144 464 600 |
| H                                                             | -0.171 079 489 905 | -0.091 361 107 911 |
| H                                                             | 0.007 181 269 642  | -0.009 720 079 652 |
| H                                                             | -0.057 702 609 041 | -0.332 196 135 189 |
| H                                                             | 0.004 076 818 177  | -0.067 604 926 056 |
| H                                                             | 0.093 209 622 226  | 0.102 679 106 868  |
| H                                                             | -0.128 109 963 218 | -0.175 924 447 054 |
| H                                                             | -0.021 867 599 122 | -0.006 716 086 285 |
| H                                                             | -0.000 134 736 057 | 0.083 231 669 723  |
| H                                                             | -0.027 109 225 591 | -0.030 313 011 080 |



Wavenumber/cm<sup>-1</sup>: 1262.6303 , Max excitation: 2

| $l'$ -matrix coefficients/(u <sup>1/2</sup> Å <sup>-1</sup> ) |                    |                    |
|---------------------------------------------------------------|--------------------|--------------------|
| O                                                             | -0.001 186 451 241 | 0.007 467 823 808  |
| C                                                             | 0.210 273 357 901  | 0.014 755 267 143  |
| C                                                             | 0.049 972 000 920  | 0.063 544 241 239  |
| C                                                             | -0.005 942 780 510 | -0.096 711 297 329 |
| C                                                             | -0.062 538 132 795 | -0.088 704 078 340 |
| C                                                             | -0.053 856 742 467 | 0.041 958 003 822  |
| C                                                             | -0.034 780 888 577 | 0.026 610 236 567  |
| C                                                             | 0.187 016 210 254  | -0.071 834 950 749 |
| C                                                             | -0.114 101 841 485 | -0.009 177 989 296 |
| C                                                             | -0.220 498 369 873 | 0.009 810 565 134  |
| C                                                             | -0.056 989 108 924 | -0.015 215 593 058 |
| H                                                             | 0.019 960 712 203  | -0.032 109 835 524 |
| H                                                             | -0.083 873 659 719 | -0.262 692 797 454 |
| H                                                             | 0.059 132 992 753  | 0.081 748 007 323  |
| H                                                             | 0.094 185 588 727  | 0.135 418 104 274  |
| H                                                             | -0.285 913 531 911 | 0.303 794 048 794  |
| H                                                             | 0.117 987 910 662  | -0.024 760 061 561 |
| H                                                             | 0.153 330 453 296  | 0.002 343 821 305  |
| H                                                             | 0.175 376 511 234  | 0.094 770 365 561  |
| H                                                             | 0.064 283 784 649  | 0.013 458 158 730  |
| H                                                             | 0.095 243 420 071  | 0.163 650 416 614  |
| H                                                             | -0.028 148 576 674 | 0.079 857 554 022  |
| H                                                             | 0.013 695 564 933  | -0.008 540 623 794 |
| H                                                             | 0.011 143 777 355  | -0.243 989 096 118 |
| H                                                             | 0.066 557 393 755  | -0.019 294 045 548 |
| H                                                             | 0.042 871 326 483  | 0.079 236 128 485  |
| H                                                             | -0.160 915 989 493 | 0.038 736 401 708  |

Wavenumber/cm<sup>-1</sup>: 1276.3806 , Max excitation: 1

| $l'$ -matrix coefficients/(u <sup>1/2</sup> Å <sup>-1</sup> ) |                    |                    |                    |
|---------------------------------------------------------------|--------------------|--------------------|--------------------|
| O                                                             | 0.018 496 928 966  | 0.010 166 417 437  | -0.001 103 741 887 |
| C                                                             | 0.063 125 350 067  | -0.114 206 134 173 | -0.050 185 155 983 |
| C                                                             | -0.110 203 224 068 | -0.058 750 524 209 | 0.047 082 746 314  |
| C                                                             | -0.056 718 154 884 | 0.043 085 228 878  | -0.064 233 918 636 |
| C                                                             | -0.057 597 371 869 | 0.034 668 000 942  | 0.195 724 638 655  |
| C                                                             | 0.004 736 507 067  | 0.092 395 349 403  | -0.014 557 530 846 |
| C                                                             | 0.079 965 267 808  | 0.011 997 141 024  | -0.010 469 528 303 |
| C                                                             | -0.015 501 155 526 | -0.100 000 276 891 | -0.083 984 347 588 |
| C                                                             | 0.094 542 346 451  | 0.091 379 413 827  | 0.015 576 283 154  |
| C                                                             | -0.086 144 371 440 | 0.069 651 579 242  | 0.051 359 060 830  |
| C                                                             | 0.041 620 488 297  | -0.008 915 743 070 | -0.024 523 751 650 |
| H                                                             | -0.023 564 852 092 | 0.010 883 297 626  | -0.110 541 604 718 |
| H                                                             | 0.006 005 873 914  | -0.027 235 685 088 | -0.038 747 259 100 |
| H                                                             | 0.413 383 308 004  | 0.242 076 013 439  | 0.086 677 175 981  |
| H                                                             | 0.098 843 642 842  | 0.181 601 106 671  | 0.004 429 775 038  |
| H                                                             | -0.029 660 429 552 | -0.278 990 503 881 | 0.291 787 889 692  |
| H                                                             | 0.048 434 488 672  | -0.030 659 308 965 | -0.006 306 596 440 |
| H                                                             | 0.022 619 996 260  | -0.011 915 617 980 | -0.010 189 621 100 |
| H                                                             | -0.406 844 454 475 | -0.232 746 845 664 | -0.137 537 174 127 |
| H                                                             | -0.037 922 007 199 | 0.031 330 756 050  | -0.093 745 328 539 |
| H                                                             | 0.053 630 397 221  | 0.136 937 937 832  | 0.050 351 199 590  |
| H                                                             | -0.071 747 105 287 | -0.065 594 736 918 | -0.257 435 957 168 |
| H                                                             | -0.026 873 832 759 | -0.046 939 438 752 | -0.037 875 038 556 |
| H                                                             | 0.027 291 319 911  | -0.049 425 278 686 | -0.044 986 744 354 |
| H                                                             | 0.010 355 614 170  | -0.005 196 166 816 | -0.002 234 939 467 |
| H                                                             | -0.026 761 792 489 | -0.091 676 276 543 | 0.103 531 425 025  |
| H                                                             | 0.014 701 565 787  | -0.014 573 482 639 | -0.006 072 566 728 |

Wavenumber/cm<sup>-1</sup>: 1303.1075 , Max excitation: 1

| $l'$ -matrix coefficients/(u <sup>1/2</sup> Å <sup>-1</sup> ) |                    |                    |                    |
|---------------------------------------------------------------|--------------------|--------------------|--------------------|
| O                                                             | -0.023 994 675 683 | -0.011 319 082 144 | 0.000 814 401 039  |
| C                                                             | 0.073 072 794 968  | -0.061 679 355 675 | -0.055 893 921 091 |
| C                                                             | 0.002 553 594 529  | 0.009 923 555 910  | -0.059 787 491 474 |
| C                                                             | -0.040 060 389 160 | 0.094 779 807 197  | 0.141 160 928 102  |
| C                                                             | 0.242 444 481 923  | 0.048 944 361 931  | -0.078 708 742 823 |
| C                                                             | 0.195 722 305 550  | -0.104 708 426 839 | 0.011 884 659 458  |
| C                                                             | -0.120 587 865 011 | -0.075 680 806 036 | -0.098 588 550 553 |
| C                                                             | -0.156 294 786 993 | 0.051 771 106 109  | 0.079 470 129 396  |
| C                                                             | -0.071 034 145 844 | -0.103 609 626 288 | -0.027 682 773 546 |
| C                                                             | -0.232 451 275 093 | 0.057 301 682 408  | 0.058 093 393 748  |
| C                                                             | 0.043 541 410 229  | 0.173 493 627 935  | 0.083 488 926 914  |
| H                                                             | 0.020 514 859 423  | 0.019 449 571 520  | 0.079 899 525 456  |
| H                                                             | -0.075 088 088 820 | -0.137 275 088 196 | 0.158 399 164 419  |
| H                                                             | -0.116 194 455 423 | -0.092 464 709 016 | -0.046 091 315 815 |
| H                                                             | 0.043 660 980 281  | 0.233 104 342 613  | -0.160 204 871 405 |
| H                                                             | 0.224 998 117 659  | -0.058 057 970 936 | -0.129 132 865 015 |
| H                                                             | 0.116 044 648 939  | -0.109 727 321 683 | -0.034 677 863 616 |
| H                                                             | -0.002 667 471 534 | -0.094 118 574 875 | -0.068 263 171 423 |
| H                                                             | -0.123 485 030 015 | -0.051 840 405 124 | 0.018 603 959 928  |
| H                                                             | 0.021 588 755 125  | -0.044 539 288 456 | 0.120 353 540 912  |
| H                                                             | 0.128 629 434 792  | 0.299 953 651 687  | 0.112 365 068 742  |
| H                                                             | -0.006 202 501 503 | -0.157 453 743 076 | 0.016 859 062 928  |
| H                                                             | 0.106 244 974 649  | 0.107 699 294 206  | -0.004 464 578 685 |
| H                                                             | 0.055 731 737 927  | -0.190 311 946 904 | -0.130 390 444 039 |
| H                                                             | -0.247 716 611 334 | 0.022 733 604 859  | 0.050 333 654 954  |
| H                                                             | 0.019 341 010 272  | 0.097 922 930 795  | -0.099 275 396 889 |
| H                                                             | 0.147 995 251 068  | -0.112 506 586 490 | -0.072 020 133 206 |

Wavenumber/cm<sup>-1</sup>: 1323.5873 , Max excitation: 1

| $l'$ -matrix coefficients/(u <sup>1/2</sup> Å <sup>-1</sup> ) |                    |                    |                    |
|---------------------------------------------------------------|--------------------|--------------------|--------------------|
| O                                                             | 0.007 997 119 163  | 0.011 424 374 898  | -0.006 224 197 199 |
| C                                                             | -0.010 031 517 746 | 0.002 859 683 090  | 0.019 175 313 509  |
| C                                                             | 0.040 042 094 334  | -0.001 384 687 817 | -0.042 716 751 796 |
| C                                                             | -0.019 079 743 448 | 0.049 803 907 722  | -0.127 463 767 412 |
| C                                                             | -0.052 960 225 603 | 0.062 590 540 489  | -0.220 912 154 048 |
| C                                                             | -0.165 921 794 858 | -0.036 217 074 723 | -0.020 777 360 495 |
| C                                                             | 0.027 741 288 998  | -0.109 705 910 735 | 0.198 034 328 065  |
| C                                                             | 0.181 620 331 642  | -0.000 641 004 783 | 0.140 143 805 615  |
| C                                                             | -0.074 042 224 531 | -0.184 671 186 769 | -0.079 444 865 577 |
| C                                                             | 0.063 629 036 231  | -0.017 207 287 683 | 0.026 344 002 186  |
| C                                                             | 0.049 330 858 921  | 0.141 563 404 712  | 0.124 461 803 647  |
| H                                                             | 0.033 472 577 062  | 0.077 145 633 351  | 0.085 768 642 551  |
| H                                                             | 0.041 944 590 895  | 0.062 670 598 834  | -0.111 405 826 430 |
| H                                                             | 0.132 448 779 886  | 0.313 452 491 219  | 0.137 097 706 501  |
| H                                                             | -0.028 014 541 972 | -0.160 466 476 249 | 0.098 441 651 061  |
| H                                                             | -0.008 222 357 947 | 0.090 034 949 648  | -0.127 082 372 459 |
| H                                                             | -0.042 885 008 340 | -0.015 445 456 896 | -0.020 802 567 780 |
| H                                                             | -0.066 874 005 839 | -0.073 677 424 614 | -0.054 654 696 732 |
| H                                                             | -0.180 741 173 391 | -0.178 004 733 263 | -0.260 002 843 250 |
| H                                                             | 0.030 219 886 928  | -0.090 312 983 594 | 0.238 170 304 176  |
| H                                                             | -0.032 715 983 982 | -0.049 887 763 479 | -0.040 603 025 852 |
| H                                                             | 0.022 721 709 110  | 0.151 916 995 022  | 0.057 466 929 987  |
| H                                                             | -0.048 801 064 820 | -0.049 983 397 500 | 0.180 118 865 709  |
| H                                                             | 0.003 820 650 685  | 0.096 705 309 605  | 0.025 241 843 075  |
| H                                                             | -0.238 180 909 264 | 0.021 251 782 984  | 0.030 039 409 269  |
| H                                                             | 0.022 934 215 028  | 0.185 729 078 941  | -0.166 364 139 703 |
| H                                                             | 0.187 799 594 705  | -0.105 576 727 454 | -0.104 778 582 545 |

Wavenumber/cm<sup>-1</sup>: 1330.351 , Max excitation: 1

| $l'$ -matrix coefficients/(u <sup>1/2</sup> Å <sup>-1</sup> ) |                    |                    |                    |
|---------------------------------------------------------------|--------------------|--------------------|--------------------|
| O                                                             | -0.013 212 950 698 | -0.009 217 119 863 | -0.001 221 074 110 |
| C                                                             | -0.012 884 535 944 | 0.016 884 456 017  | 0.081 117 046 117  |
| C                                                             | -0.033 224 354 883 | -0.001 691 217 915 | 0.005 434 422 489  |
| C                                                             | 0.034 026 599 077  | -0.090 634 735 741 | -0.010 844 761 525 |
| C                                                             | -0.171 891 500 259 | -0.091 373 757 591 | 0.305 214 000 419  |
| C                                                             | 0.046 323 742 299  | 0.229 072 474 405  | 0.109 191 191 667  |
| C                                                             | 0.161 540 102 876  | 0.095 230 759 518  | -0.111 867 787 397 |
| C                                                             | -0.054 797 036 016 | -0.083 536 248 922 | -0.322 515 469 176 |
| C                                                             | -0.066 565 556 319 | -0.144 231 431 677 | -0.122 767 923 602 |
| C                                                             | 0.012 060 249 342  | -0.066 205 838 516 | 0.032 246 003 864  |
| C                                                             | 0.092 813 495 918  | 0.160 223 579 956  | 0.046 609 025 636  |
| H                                                             | 0.030 926 730 211  | 0.101 526 159 248  | 0.060 522 694 338  |
| H                                                             | 0.059 448 073 912  | 0.108 077 052 148  | -0.018 784 449 972 |
| H                                                             | 0.024 108 173 226  | -0.140 370 552 424 | -0.069 597 312 136 |
| H                                                             | 0.018 225 799 670  | 0.012 968 143 882  | 0.068 288 174 021  |
| H                                                             | -0.128 086 584 706 | -0.039 926 344 030 | 0.179 777 609 154  |
| H                                                             | -0.028 416 158 546 | -0.061 023 635 774 | -0.035 328 276 870 |
| H                                                             | 0.043 094 996 677  | -0.114 331 507 614 | -0.080 924 743 163 |
| H                                                             | 0.190 232 413 410  | 0.123 958 185 213  | 0.139 877 070 757  |
| H                                                             | 0.009 293 132 626  | -0.086 307 195 621 | 0.250 276 405 159  |
| H                                                             | -0.017 066 763 271 | -0.012 781 223 435 | -0.026 810 057 237 |
| H                                                             | -0.033 777 255 805 | -0.020 599 709 740 | -0.140 220 389 778 |
| H                                                             | -0.067 443 537 701 | -0.068 237 919 935 | -0.188 130 713 406 |
| H                                                             | 0.007 365 882 057  | 0.055 216 307 314  | 0.005 200 667 886  |
| H                                                             | -0.255 632 436 131 | 0.010 540 505 757  | 0.069 944 864 310  |
| H                                                             | 0.017 550 670 452  | 0.209 039 989 758  | -0.176 128 268 102 |
| H                                                             | 0.157 269 487 457  | -0.122 969 791 762 | -0.073 886 166 340 |

Wavenumber/cm<sup>-1</sup>: 1380.0168 , Max excitation: 4

| $l'$ -matrix coefficients/(u <sup>1/2</sup> Å <sup>-1</sup> ) |                    |                    |
|---------------------------------------------------------------|--------------------|--------------------|
| O                                                             | -0.041 833 844 318 | -0.015 081 486 702 |
| C                                                             | -0.019 201 818 853 | -0.014 773 488 156 |
| C                                                             | 0.178 731 105 989  | -0.104 692 265 690 |
| C                                                             | 0.075 499 685 132  | -0.203 507 956 695 |
| C                                                             | -0.084 834 427 723 | -0.137 686 614 122 |
| C                                                             | -0.138 327 501 211 | -0.200 165 387 169 |
| C                                                             | -0.069 545 529 680 | 0.403 236 373 936  |
| C                                                             | 0.118 178 781 242  | 0.204 092 925 560  |
| C                                                             | 0.183 108 103 941  | -0.029 296 165 679 |
| C                                                             | -0.014 669 661 989 | 0.087 517 851 900  |
| C                                                             | -0.106 739 556 133 | 0.084 510 696 922  |
| H                                                             | -0.029 857 624 787 | 0.182 374 853 513  |
| H                                                             | -0.058 320 964 559 | -0.150 940 890 901 |
| H                                                             | 0.188 836 532 901  | -0.178 972 457 946 |
| H                                                             | -0.014 447 061 739 | -0.073 641 470 148 |
| H                                                             | -0.001 655 195 834 | -0.164 177 560 269 |
| H                                                             | 0.033 875 720 906  | 0.071 422 706 158  |
| H                                                             | -0.064 223 808 113 | -0.027 984 065 686 |
| H                                                             | -0.088 775 615 162 | 0.126 742 872 290  |
| H                                                             | -0.113 084 983 390 | -0.063 363 897 057 |
| H                                                             | 0.018 478 587 139  | 0.023 290 125 286  |
| H                                                             | 0.026 034 564 538  | 0.068 132 055 395  |
| H                                                             | 0.036 403 541 905  | 0.071 099 977 412  |
| H                                                             | -0.006 392 287 254 | -0.059 008 892 695 |
| H                                                             | -0.152 889 400 370 | 0.012 596 128 919  |
| H                                                             | -0.076 655 317 548 | -0.032 310 988 874 |
| H                                                             | 0.047 513 348 992  | -0.053 213 590 047 |

Wavenumber/cm<sup>-1</sup>: 1402.2666 , Max excitation: 1

| $l'$ -matrix coefficients/(u <sup>1/2</sup> Å <sup>-1</sup> ) |                    |                    |
|---------------------------------------------------------------|--------------------|--------------------|
| O                                                             | -0.021 341 405 914 | -0.009 045 903 043 |
| C                                                             | -0.059 966 315 782 | -0.003 015 140 268 |
| C                                                             | -0.025 073 101 414 | -0.152 279 784 582 |
| C                                                             | 0.018 550 968 091  | -0.083 616 566 535 |
| C                                                             | -0.162 930 800 322 | -0.021 043 493 737 |
| C                                                             | 0.037 381 757 631  | -0.118 935 072 483 |
| C                                                             | 0.166 949 473 022  | 0.035 278 000 205  |
| C                                                             | -0.024 786 820 753 | 0.197 015 509 403  |
| C                                                             | -0.098 982 655 009 | 0.172 692 350 267  |
| C                                                             | -0.070 537 015 523 | 0.062 214 865 988  |
| C                                                             | 0.130 949 572 053  | -0.165 481 010 872 |
| H                                                             | 0.034 016 792 495  | -0.095 166 290 728 |
| H                                                             | -0.052 401 708 804 | -0.080 323 381 372 |
| H                                                             | 0.022 706 984 151  | 0.070 774 265 643  |
| H                                                             | -0.048 342 313 965 | -0.017 293 074 393 |
| H                                                             | -0.077 645 501 992 | -0.011 722 401 480 |
| H                                                             | 0.055 149 272 487  | 0.031 523 465 757  |
| H                                                             | -0.407 666 026 911 | 0.131 502 632 356  |
| H                                                             | 0.114 492 057 386  | 0.024 214 577 427  |
| H                                                             | 0.112 944 490 715  | 0.094 584 328 287  |
| H                                                             | 0.047 821 581 579  | 0.081 938 457 227  |
| H                                                             | 0.041 239 465 353  | -0.013 702 877 333 |
| H                                                             | 0.049 229 662 711  | 0.084 536 734 808  |
| H                                                             | 0.002 656 588 134  | -0.114 670 850 066 |
| H                                                             | 0.134 720 106 471  | 0.017 712 721 931  |
| H                                                             | 0.086 413 355 895  | 0.073 158 341 682  |
| H                                                             | 0.275 001 374 312  | 0.025 363 566 188  |

Wavenumber/cm<sup>-1</sup>: 1413.4354 , Max excitation: 1

| $l'$ -matrix coefficients/(u <sup>1/2</sup> Å <sup>-1</sup> ) |                    |                    |
|---------------------------------------------------------------|--------------------|--------------------|
| O                                                             | -0.003 530 287 907 | -0.004 580 747 978 |
| C                                                             | -0.082 633 282 615 | -0.000 933 077 197 |
| C                                                             | -0.056 799 776 407 | 0.157 180 567 811  |
| C                                                             | 0.019 014 063 222  | -0.105 664 434 702 |
| C                                                             | -0.255 860 497 612 | -0.104 069 048 574 |
| C                                                             | 0.111 393 394 435  | -0.188 871 348 148 |
| C                                                             | 0.269 333 250 993  | -0.044 145 711 592 |
| C                                                             | -0.024 594 518 424 | 0.232 148 234 220  |
| C                                                             | 0.017 174 073 250  | -0.048 787 934 202 |
| C                                                             | -0.048 396 883 288 | 0.077 879 477 198  |
| C                                                             | 0.038 100 458 327  | 0.122 219 898 626  |
| H                                                             | -0.023 071 306 191 | -0.044 862 272 894 |
| H                                                             | -0.077 959 968 017 | -0.033 584 887 161 |
| H                                                             | -0.037 070 746 040 | 0.195 602 268 047  |
| H                                                             | -0.122 043 177 053 | -0.055 601 040 946 |
| H                                                             | -0.026 525 715 659 | -0.146 824 693 827 |
| H                                                             | 0.050 498 913 278  | 0.068 720 696 381  |
| H                                                             | 0.258 030 240 342  | -0.117 246 660 552 |
| H                                                             | 0.218 831 351 878  | 0.005 156 382 138  |
| H                                                             | -0.032 513 093 670 | -0.004 269 259 928 |
| H                                                             | 0.034 595 534 564  | 0.051 517 579 980  |
| H                                                             | 0.060 043 435 272  | 0.017 818 316 710  |
| H                                                             | -0.000 860 642 818 | 0.053 366 717 416  |
| H                                                             | -0.007 078 256 333 | -0.104 151 095 628 |
| H                                                             | -0.140 736 843 644 | -0.011 042 952 816 |
| H                                                             | -0.029 094 278 380 | -0.117 942 248 589 |
| H                                                             | -0.065 173 673 384 | -0.073 099 277 633 |
|                                                               |                    | 0.078 906 836 033  |



Wavenumber/cm<sup>-1</sup>: 1423.9832 , Max excitation: 1

| $l'$ -matrix coefficients/(u <sup>1/2</sup> Å <sup>-1</sup> ) |                    |                    |                    |
|---------------------------------------------------------------|--------------------|--------------------|--------------------|
| O                                                             | 0.006 737 673 717  | 0.006 588 428 077  | 0.003 810 361 040  |
| C                                                             | 0.021 319 821 076  | -0.014 086 330 077 | 0.010 906 676 024  |
| C                                                             | -0.263 581 309 253 | 0.223 907 022 500  | 0.024 086 642 151  |
| C                                                             | 0.054 832 105 396  | -0.149 790 691 486 | -0.098 105 392 235 |
| C                                                             | 0.071 343 429 152  | -0.216 200 420 585 | -0.160 452 934 922 |
| C                                                             | -0.067 403 050 701 | 0.033 168 821 441  | 0.071 989 314 431  |
| C                                                             | -0.143 432 319 985 | 0.230 844 141 494  | 0.073 224 219 438  |
| C                                                             | 0.055 553 579 724  | -0.049 708 327 130 | 0.019 796 935 417  |
| C                                                             | -0.204 017 839 245 | 0.090 780 038 578  | 0.131 459 212 389  |
| C                                                             | 0.065 373 490 544  | -0.004 623 533 060 | 0.012 452 415 177  |
| C                                                             | 0.273 355 014 212  | 0.037 105 457 494  | -0.087 749 837 475 |
| H                                                             | 0.023 765 105 168  | -0.273 634 373 019 | 0.282 981 004 875  |
| H                                                             | 0.018 898 157 176  | -0.017 376 224 573 | -0.051 646 350 086 |
| H                                                             | 0.021 995 482 441  | -0.099 253 740 799 | -0.009 368 258 953 |
| H                                                             | 0.040 265 264 747  | -0.003 451 147 209 | 0.088 152 705 499  |
| H                                                             | 0.164 834 708 005  | -0.257 014 370 565 | -0.047 357 025 291 |
| H                                                             | -0.041 921 373 411 | 0.014 876 258 495  | -0.001 948 689 994 |
| H                                                             | 0.094 635 242 845  | -0.073 722 611 224 | -0.075 538 071 699 |
| H                                                             | -0.092 189 026 473 | 0.057 598 796 263  | 0.141 362 760 145  |
| H                                                             | 0.122 210 741 732  | 0.112 643 737 137  | -0.243 066 192 585 |
| H                                                             | -0.039 268 687 802 | -0.069 113 474 757 | -0.037 017 533 823 |
| H                                                             | -0.020 030 405 755 | 0.017 046 780 311  | -0.083 001 226 213 |
| H                                                             | -0.006 207 017 620 | -0.017 236 298 305 | 0.136 944 030 242  |
| H                                                             | -0.009 293 098 495 | 0.092 359 091 832  | 0.037 196 699 986  |
| H                                                             | -0.075 966 691 526 | -0.006 366 206 601 | -0.001 785 397 009 |
| H                                                             | 0.092 711 972 308  | -0.058 736 174 670 | -0.065 711 709 476 |
| H                                                             | 0.150 453 940 043  | -0.071 045 168 063 | -0.077 117 800 646 |

Wavenumber/cm<sup>-1</sup>: 1476.9449 , Max excitation: 1

| $l'$ -matrix coefficients/(u <sup>1/2</sup> Å <sup>-1</sup> ) |                    |                    |
|---------------------------------------------------------------|--------------------|--------------------|
| O                                                             | -0.028 442 913 772 | -0.003 046 655 182 |
| C                                                             | -0.051 272 098 568 | 0.034 640 817 035  |
| C                                                             | 0.138 650 816 775  | -0.088 705 612 821 |
| C                                                             | 0.059 573 515 975  | -0.123 526 048 117 |
| C                                                             | 0.033 811 851 188  | -0.119 011 285 107 |
| C                                                             | 0.171 278 822 813  | 0.285 771 691 288  |
| C                                                             | -0.125 247 654 917 | 0.129 420 455 515  |
| C                                                             | -0.112 311 217 491 | -0.247 822 181 033 |
| C                                                             | 0.109 973 975 023  | 0.048 684 932 017  |
| C                                                             | -0.030 439 241 762 | 0.007 306 558 637  |
| C                                                             | -0.110 339 013 949 | 0.013 647 219 319  |
| H                                                             | -0.019 259 759 727 | 0.077 733 455 849  |
| H                                                             | 0.067 522 238 504  | 0.133 073 172 173  |
| H                                                             | -0.113 159 512 574 | 0.091 448 075 741  |
| H                                                             | 0.035 543 050 161  | 0.110 648 474 314  |
| H                                                             | 0.131 448 547 415  | 0.031 370 356 977  |
| H                                                             | 0.040 890 576 819  | 0.109 175 360 459  |
| H                                                             | -0.109 528 246 905 | 0.030 137 297 461  |
| H                                                             | -0.041 333 791 450 | 0.007 822 522 602  |
| H                                                             | -0.045 672 015 720 | 0.000 392 029 847  |
| H                                                             | 0.011 913 451 933  | -0.045 812 013 108 |
| H                                                             | -0.036 532 312 329 | -0.078 704 151 812 |
| H                                                             | -0.023 738 937 666 | -0.070 018 601 830 |
| H                                                             | -0.029 075 225 142 | -0.146 205 351 617 |
| H                                                             | -0.024 701 657 762 | 0.014 043 882 101  |
| H                                                             | -0.038 929 996 128 | -0.052 477 974 510 |
| H                                                             | 0.019 071 444 915  | 0.005 227 096 779  |

Wavenumber/cm<sup>-1</sup>: 1482.6821 , Max excitation: 1

| $l'$ -matrix coefficients/(u <sup>1/2</sup> Å <sup>-1</sup> ) |                    |                    |                    |
|---------------------------------------------------------------|--------------------|--------------------|--------------------|
| O                                                             | 0.146 283 631 626  | 0.059 016 141 160  | 0.005 027 968 326  |
| C                                                             | 0.103 538 641 200  | 0.055 329 570 438  | -0.209 714 509 896 |
| C                                                             | 0.108 416 651 987  | 0.080 866 071 376  | 0.102 533 168 990  |
| C                                                             | -0.110 058 052 454 | 0.310 715 888 003  | 0.312 346 237 436  |
| C                                                             | -0.034 616 590 610 | -0.312 304 941 704 | -0.048 237 028 808 |
| C                                                             | -0.095 679 008 770 | -0.062 650 106 197 | 0.207 606 634 282  |
| C                                                             | -0.213 033 877 224 | -0.289 829 921 980 | -0.111 341 124 950 |
| C                                                             | 0.135 954 071 191  | 0.179 153 492 114  | -0.209 538 397 420 |
| C                                                             | 0.041 073 694 450  | 0.055 033 242 499  | 0.000 938 224 377  |
| C                                                             | 0.016 801 866 244  | -0.012 652 331 575 | -0.136 463 124 041 |
| C                                                             | -0.029 099 613 266 | 0.062 615 769 765  | 0.082 159 833 609  |
| H                                                             | -0.008 332 006 296 | 0.002 723 033 843  | -0.047 662 349 451 |
| H                                                             | 0.010 458 824 663  | -0.090 346 180 368 | -0.037 266 879 958 |
| H                                                             | -0.094 004 450 695 | 0.009 473 929 012  | -0.001 943 919 362 |
| H                                                             | -0.011 563 314 664 | -0.119 941 499 074 | 0.130 684 091 597  |
| H                                                             | -0.087 937 996 573 | -0.147 548 240 881 | 0.106 171 543 230  |
| H                                                             | 0.029 297 037 166  | 0.153 456 810 949  | 0.100 044 397 635  |
| H                                                             | -0.074 767 316 016 | -0.017 064 731 778 | -0.013 050 541 514 |
| H                                                             | 0.048 339 155 917  | -0.021 866 953 534 | -0.043 571 160 086 |
| H                                                             | -0.008 481 735 409 | 0.026 599 051 372  | -0.075 790 745 408 |
| H                                                             | -0.019 576 914 069 | -0.135 443 734 811 | 0.016 882 174 788  |
| H                                                             | 0.004 490 671 207  | 0.074 809 002 315  | -0.156 196 910 409 |
| H                                                             | -0.011 778 804 379 | 0.025 656 290 615  | 0.013 929 292 803  |
| H                                                             | -0.039 119 551 044 | -0.130 369 005 238 | 0.012 863 783 184  |
| H                                                             | -0.133 678 909 020 | 0.010 923 290 342  | 0.014 862 628 764  |
| H                                                             | -0.013 715 786 712 | -0.059 139 684 847 | 0.056 885 287 616  |
| H                                                             | 0.092 340 067 045  | -0.045 832 475 022 | -0.063 353 480 016 |

Wavenumber/cm<sup>-1</sup>: 1487.5594 , Max excitation: 1

| $l'$ -matrix coefficients/(u <sup>1/2</sup> Å <sup>-1</sup> ) |                    |                    |                    |
|---------------------------------------------------------------|--------------------|--------------------|--------------------|
| O                                                             | 0.006 493 571 097  | -0.002 035 619 658 | -0.007 604 006 304 |
| C                                                             | 0.015 348 330 172  | -0.124 176 852 984 | 0.373 958 694 550  |
| C                                                             | 0.097 390 204 189  | 0.035 425 993 031  | 0.051 895 159 454  |
| C                                                             | 0.000 158 605 085  | 0.048 446 420 227  | -0.027 208 752 764 |
| C                                                             | -0.050 766 881 251 | -0.321 615 099 452 | -0.082 986 499 877 |
| C                                                             | -0.025 529 157 145 | 0.229 462 849 919  | -0.311 335 984 642 |
| C                                                             | -0.007 201 374 268 | -0.082 291 071 676 | 0.115 446 550 923  |
| C                                                             | -0.088 186 217 971 | 0.179 690 978 778  | -0.115 604 594 603 |
| C                                                             | 0.058 422 000 409  | 0.065 362 909 024  | -0.031 268 825 870 |
| C                                                             | 0.003 256 283 866  | -0.090 637 401 334 | 0.132 933 798 771  |
| C                                                             | -0.081 007 435 504 | 0.042 894 583 584  | 0.052 406 155 559  |
| H                                                             | -0.021 386 658 046 | 0.020 815 665 613  | -0.101 818 324 246 |
| H                                                             | 0.027 921 044 827  | -0.092 635 810 450 | -0.224 519 932 160 |
| H                                                             | -0.128 880 799 308 | 0.101 024 426 821  | 0.044 915 843 642  |
| H                                                             | 0.148 418 568 554  | 0.094 896 626 319  | 0.050 658 117 210  |
| H                                                             | 0.021 787 451 855  | -0.110 651 631 384 | -0.047 270 534 603 |
| H                                                             | -0.065 368 734 875 | -0.230 458 155 777 | -0.152 708 963 928 |
| H                                                             | -0.029 285 924 344 | -0.004 947 848 680 | 0.005 025 181 681  |
| H                                                             | 0.136 676 275 653  | 0.016 336 497 073  | -0.119 209 414 260 |
| H                                                             | -0.029 808 745 369 | 0.024 255 381 560  | -0.086 316 597 211 |
| H                                                             | -0.004 712 185 412 | 0.085 591 571 236  | -0.055 101 967 951 |
| H                                                             | 0.048 039 275 877  | -0.152 135 628 370 | 0.043 909 942 384  |
| H                                                             | 0.198 333 872 605  | 0.203 601 091 737  | 0.046 324 192 602  |
| H                                                             | 0.042 510 584 640  | 0.184 636 859 281  | -0.010 513 146 652 |
| H                                                             | -0.067 253 021 262 | 0.009 035 034 758  | 0.018 940 190 558  |
| H                                                             | -0.033 593 449 605 | -0.069 799 977 814 | 0.074 367 933 227  |
| H                                                             | 0.000 385 310 482  | -0.011 262 891 604 | -0.002 614 306 366 |

Wavenumber/cm<sup>-1</sup>: 1490.9102 , Max excitation: 1

| $l'$ -matrix coefficients/(u <sup>1/2</sup> Å <sup>-1</sup> ) |                    |                    |
|---------------------------------------------------------------|--------------------|--------------------|
| O                                                             | -0.099 288 410 174 | -0.019 423 831 562 |
| C                                                             | 0.070 668 885 749  | 0.063 134 624 049  |
| C                                                             | -0.035 559 814 928 | -0.052 296 904 475 |
| C                                                             | 0.027 918 408 771  | -0.151 746 760 173 |
| C                                                             | 0.348 843 152 889  | 0.174 288 810 852  |
| C                                                             | -0.194 369 139 947 | -0.129 153 461 449 |
| C                                                             | -0.076 113 208 110 | 0.037 576 854 333  |
| C                                                             | 0.014 998 768 581  | 0.228 085 093 536  |
| C                                                             | -0.024 086 107 757 | -0.078 592 674 545 |
| C                                                             | 0.033 352 407 459  | -0.006 609 029 177 |
| C                                                             | -0.055 583 233 590 | -0.013 072 079 288 |
| H                                                             | 0.011 949 042 652  | 0.017 320 464 193  |
| H                                                             | -0.011 950 542 789 | -0.194 235 350 722 |
| H                                                             | -0.282 157 807 515 | 0.064 573 107 872  |
| H                                                             | 0.063 828 423 767  | -0.071 236 769 837 |
| H                                                             | 0.187 824 861 091  | -0.054 725 636 973 |
| H                                                             | -0.009 826 030 220 | 0.080 535 078 401  |
| H                                                             | -0.000 913 624 647 | 0.024 187 994 313  |
| H                                                             | -0.034 828 627 487 | -0.028 427 705 219 |
| H                                                             | 0.012 453 071 898  | -0.036 823 262 468 |
| H                                                             | -0.034 006 155 066 | -0.097 915 350 060 |
| H                                                             | 0.001 720 446 701  | -0.118 873 754 602 |
| H                                                             | 0.125 244 762 444  | 0.139 404 104 307  |
| H                                                             | -0.027 453 352 389 | -0.002 900 249 137 |
| H                                                             | 0.058 734 323 286  | 0.002 721 571 484  |
| H                                                             | 0.013 441 987 393  | 0.067 673 229 576  |
| H                                                             | -0.058 447 858 291 | 0.038 896 770 011  |

Wavenumber/cm<sup>-1</sup>: 1496.6361 , Max excitation: 1

| $l'$ -matrix coefficients/(u <sup>1/2</sup> Å <sup>-1</sup> ) |                    |                    |                    |
|---------------------------------------------------------------|--------------------|--------------------|--------------------|
| O                                                             | 0.000 542 399 357  | -0.007 554 916 041 | -0.004 169 181 643 |
| C                                                             | -0.149 696 538 713 | -0.013 328 073 240 | 0.216 944 441 051  |
| C                                                             | 0.010 530 375 185  | -0.007 598 658 010 | 0.014 029 322 071  |
| C                                                             | 0.052 714 624 246  | 0.015 724 721 889  | -0.025 469 328 954 |
| C                                                             | 0.162 617 572 120  | -0.059 979 048 703 | 0.114 956 277 421  |
| C                                                             | 0.136 637 145 800  | -0.034 945 085 159 | -0.195 063 666 248 |
| C                                                             | -0.270 217 943 812 | -0.005 135 444 438 | 0.168 727 073 303  |
| C                                                             | 0.273 482 710 983  | 0.094 857 518 704  | -0.211 578 475 833 |
| C                                                             | 0.018 620 713 343  | 0.052 856 395 155  | -0.078 045 563 370 |
| C                                                             | -0.057 197 719 444 | -0.073 267 510 604 | 0.039 509 075 495  |
| C                                                             | 0.026 144 916 206  | -0.027 601 455 779 | 0.014 235 189 527  |
| H                                                             | -0.003 678 813 835 | 0.023 852 488 454  | -0.045 891 596 306 |
| H                                                             | -0.076 111 090 492 | 0.166 129 864 467  | 0.211 778 385 437  |
| H                                                             | -0.167 979 315 254 | 0.001 135 599 227  | 0.041 848 092 623  |
| H                                                             | -0.218 389 955 872 | -0.076 263 914 647 | -0.274 719 068 445 |
| H                                                             | 0.046 870 955 331  | -0.086 154 868 489 | 0.087 258 761 898  |
| H                                                             | 0.002 588 249 276  | -0.144 010 152 725 | -0.084 935 135 388 |
| H                                                             | 0.003 856 661 624  | 0.007 016 780 974  | 0.011 054 859 643  |
| H                                                             | -0.084 900 699 133 | -0.009 910 620 839 | 0.011 087 578 828  |
| H                                                             | -0.006 121 426 314 | 0.013 077 261 532  | -0.022 292 142 036 |
| H                                                             | 0.037 638 388 298  | 0.113 015 436 333  | -0.001 041 112 050 |
| H                                                             | -0.021 945 709 954 | 0.397 022 505 331  | -0.111 863 844 583 |
| H                                                             | -0.248 217 863 898 | -0.173 224 796 642 | 0.013 111 817 645  |
| H                                                             | 0.027 832 917 281  | -0.002 871 360 929 | -0.042 760 274 275 |
| H                                                             | 0.023 846 284 900  | -0.006 839 969 366 | 0.007 229 821 795  |
| H                                                             | -0.010 631 244 489 | 0.005 958 453 588  | -0.002 817 090 835 |
| H                                                             | -0.009 765 559 858 | 0.003 819 859 558  | 0.018 502 884 420  |

Wavenumber/cm<sup>-1</sup>: 1503.3768 , Max excitation: 0

| $l'$ -matrix coefficients/(u <sup>1/2</sup> Å <sup>-1</sup> ) |                    |                    |                    |
|---------------------------------------------------------------|--------------------|--------------------|--------------------|
| O                                                             | 0.036 633 603 911  | 0.040 554 268 497  | 0.008 429 420 813  |
| C                                                             | 0.396 580 675 122  | -0.144 265 794 449 | 0.162 126 116 763  |
| C                                                             | -0.223 696 010 832 | -0.347 690 476 967 | -0.262 635 304 946 |
| C                                                             | -0.053 304 667 983 | 0.079 209 442 095  | 0.103 518 438 376  |
| C                                                             | -0.208 791 067 364 | -0.022 930 381 993 | -0.215 508 085 460 |
| C                                                             | 0.117 279 303 888  | 0.007 276 994 477  | 0.210 264 292 181  |
| C                                                             | -0.145 011 188 313 | 0.077 149 570 708  | 0.058 905 954 829  |
| C                                                             | 0.040 586 697 344  | 0.219 741 040 374  | -0.122 842 459 393 |
| C                                                             | -0.042 415 248 812 | -0.055 515 889 054 | -0.052 454 424 988 |
| C                                                             | 0.099 865 179 354  | 0.102 452 025 915  | 0.081 170 049 296  |
| C                                                             | -0.015 813 068 199 | -0.066 085 906 077 | -0.056 496 190 155 |
| H                                                             | 0.019 737 261 351  | 0.031 331 825 477  | 0.052 848 453 153  |
| H                                                             | -0.056 291 872 289 | -0.088 307 346 083 | 0.162 925 349 548  |
| H                                                             | 0.055 178 144 749  | 0.002 900 598 916  | 0.026 254 531 248  |
| H                                                             | -0.020 924 414 965 | 0.054 387 105 172  | -0.025 974 379 231 |
| H                                                             | -0.023 733 445 333 | -0.101 653 330 658 | -0.030 748 899 728 |
| H                                                             | -0.036 298 277 672 | 0.022 600 726 644  | -0.003 169 152 054 |
| H                                                             | 0.027 957 251 992  | 0.048 639 318 468  | 0.033 349 795 136  |
| H                                                             | -0.090 653 748 119 | 0.008 059 514 033  | 0.066 203 147 804  |
| H                                                             | 0.008 544 475 045  | -0.039 810 116 125 | 0.132 000 886 141  |
| H                                                             | -0.042 188 548 005 | -0.050 639 198 314 | -0.032 577 452 477 |
| H                                                             | 0.037 117 594 633  | 0.025 928 422 438  | 0.013 382 176 942  |
| H                                                             | 0.025 607 572 341  | 0.067 754 307 338  | -0.091 726 395 004 |
| H                                                             | 0.001 954 768 087  | 0.183 095 771 131  | 0.060 137 248 449  |
| H                                                             | 0.163 813 236 706  | -0.002 724 724 670 | -0.035 099 832 655 |
| H                                                             | 0.033 802 952 603  | 0.124 408 902 336  | -0.121 465 680 570 |
| H                                                             | -0.129 723 436 987 | 0.072 530 190 069  | 0.084 395 972 824  |

Wavenumber/cm<sup>-1</sup>: 1509.2129 , Max excitation: 1

| $l'$ -matrix coefficients/(u <sup>1/2</sup> Å <sup>-1</sup> ) |                    |                    |
|---------------------------------------------------------------|--------------------|--------------------|
| O                                                             | -0.253 355 938 152 | -0.058 125 593 436 |
| C                                                             | 0.498 600 831 294  | -0.043 701 742 689 |
| C                                                             | 0.010 449 335 593  | 0.146 231 609 589  |
| C                                                             | -0.219 741 261 290 | -0.028 714 891 819 |
| C                                                             | 0.083 963 444 614  | -0.121 556 370 736 |
| C                                                             | 0.072 848 769 426  | -0.065 266 915 599 |
| C                                                             | 0.127 020 319 982  | 0.101 066 769 330  |
| C                                                             | -0.052 869 851 158 | -0.216 136 363 264 |
| C                                                             | 0.037 272 697 547  | 0.103 453 604 951  |
| C                                                             | 0.084 760 381 504  | 0.052 242 671 474  |
| C                                                             | -0.206 502 304 806 | 0.066 427 810 126  |
| H                                                             | 0.012 257 625 058  | 0.002 975 876 187  |
| H                                                             | -0.088 210 349 714 | -0.011 418 943 507 |
| H                                                             | -0.029 602 769 099 | 0.101 011 144 229  |
| H                                                             | -0.069 960 653 635 | 0.100 224 136 874  |
| H                                                             | 0.068 724 668 500  | -0.035 734 841 816 |
| H                                                             | -0.065 306 128 118 | 0.088 446 044 335  |
| H                                                             | -0.076 049 366 262 | -0.019 071 016 677 |
| H                                                             | 0.124 138 912 500  | 0.053 937 337 794  |
| H                                                             | 0.028 347 855 962  | 0.042 179 490 207  |
| H                                                             | -0.099 338 343 041 | -0.168 103 323 829 |
| H                                                             | -0.035 460 412 241 | 0.031 326 739 575  |
| H                                                             | -0.079 852 874 091 | -0.102 309 054 697 |
| H                                                             | -0.033 916 018 726 | 0.171 214 297 785  |
| H                                                             | -0.155 436 044 013 | 0.009 668 387 983  |
| H                                                             | 0.015 836 853 843  | 0.015 156 121 905  |
| H                                                             | -0.011 164 450 055 | -0.027 372 911 674 |



Wavenumber/cm<sup>-1</sup>: 1514.2094 , Max excitation: 0

| $l'$ -matrix coefficients/(u <sup>1/2</sup> Å <sup>-1</sup> ) |                    |                    |                    |
|---------------------------------------------------------------|--------------------|--------------------|--------------------|
| O                                                             | 0.099 837 838 869  | 0.044 536 074 970  | 0.003 157 052 593  |
| C                                                             | -0.069 978 718 422 | 0.051 279 691 879  | 0.227 041 531 405  |
| C                                                             | -0.121 220 777 556 | 0.080 840 914 192  | -0.104 846 455 262 |
| C                                                             | 0.149 725 005 992  | -0.148 261 308 757 | -0.202 141 737 495 |
| C                                                             | 0.162 172 984 764  | -0.120 973 241 882 | -0.001 486 178 189 |
| C                                                             | -0.082 156 808 774 | -0.146 347 583 782 | 0.267 322 500 283  |
| C                                                             | 0.110 860 495 060  | -0.247 354 562 390 | -0.251 465 226 234 |
| C                                                             | -0.001 571 974 086 | -0.080 241 095 070 | 0.087 595 691 257  |
| C                                                             | 0.022 774 168 569  | 0.185 020 858 593  | -0.293 950 677 117 |
| C                                                             | 0.045 860 114 555  | 0.288 292 110 712  | 0.130 996 906 298  |
| C                                                             | -0.286 834 328 230 | 0.068 007 743 110  | 0.124 629 621 157  |
| H                                                             | 0.023 176 614 430  | 0.012 316 850 617  | -0.043 699 934 395 |
| H                                                             | -0.015 430 719 396 | -0.060 003 428 187 | 0.057 247 222 329  |
| H                                                             | -0.017 304 021 526 | -0.082 945 867 495 | -0.080 262 679 753 |
| H                                                             | -0.022 348 039 574 | -0.089 786 710 284 | 0.106 834 471 337  |
| H                                                             | 0.034 723 594 417  | -0.078 994 975 417 | 0.043 648 438 709  |
| H                                                             | 0.002 903 075 651  | 0.028 270 627 199  | -0.012 211 190 632 |
| H                                                             | -0.012 274 390 474 | 0.002 382 295 041  | 0.044 555 450 715  |
| H                                                             | 0.029 298 656 717  | -0.075 183 593 660 | -0.078 164 799 289 |
| H                                                             | 0.037 370 681 700  | 0.064 574 088 138  | -0.107 904 703 434 |
| H                                                             | 0.022 124 608 309  | 0.131 238 348 527  | 0.019 619 685 785  |
| H                                                             | -0.036 105 677 090 | 0.015 051 620 154  | -0.054 833 914 699 |
| H                                                             | -0.048 473 255 403 | -0.050 665 073 605 | 0.070 062 081 166  |
| H                                                             | 0.024 743 189 777  | 0.133 355 491 512  | 0.024 793 096 186  |
| H                                                             | -0.067 024 164 509 | 0.013 545 012 265  | 0.075 021 065 644  |
| H                                                             | 0.029 216 301 509  | 0.066 078 129 183  | -0.112 278 172 546 |
| H                                                             | -0.139 442 988 991 | 0.034 060 936 762  | 0.091 277 126 022  |

Wavenumber/cm<sup>-1</sup>: 1524.4891 , Max excitation: 1

| $l'$ -matrix coefficients/(u <sup>1/2</sup> Å <sup>-1</sup> ) |                    |                    |                    |
|---------------------------------------------------------------|--------------------|--------------------|--------------------|
| O                                                             | 0.104 263 021 221  | 0.036 138 369 353  | 0.030 049 408 776  |
| C                                                             | -0.012 367 637 728 | 0.285 745 789 698  | -0.082 730 429 509 |
| C                                                             | 0.046 753 478 739  | -0.159 284 527 308 | -0.012 808 646 789 |
| C                                                             | 0.084 154 365 670  | 0.000 480 791 314  | 0.007 034 109 281  |
| C                                                             | -0.133 320 897 236 | -0.257 014 724 943 | 0.071 817 629 329  |
| C                                                             | -0.057 371 395 437 | -0.050 406 190 124 | -0.289 792 709 403 |
| C                                                             | -0.194 574 716 363 | -0.047 653 234 528 | 0.056 273 479 647  |
| C                                                             | -0.120 965 524 708 | -0.294 898 492 635 | -0.053 713 603 385 |
| C                                                             | -0.016 468 512 422 | -0.063 982 777 928 | 0.140 135 960 526  |
| C                                                             | 0.106 655 632 114  | 0.501 422 901 920  | 0.167 600 659 281  |
| C                                                             | 0.169 972 462 335  | -0.035 464 988 354 | -0.075 788 084 103 |
| H                                                             | -0.001 190 967 998 | 0.045 889 992 799  | 0.039 669 468 403  |
| H                                                             | -0.021 200 429 245 | -0.013 669 775 098 | -0.078 499 975 288 |
| H                                                             | -0.152 216 390 427 | 0.031 146 209 327  | 0.015 782 288 231  |
| H                                                             | -0.023 507 097 007 | -0.042 659 149 148 | -0.073 893 450 131 |
| H                                                             | -0.035 282 407 404 | -0.033 315 288 029 | -0.014 692 134 697 |
| H                                                             | 0.062 197 357 058  | 0.176 749 838 622  | 0.083 935 572 356  |
| H                                                             | 0.023 915 044 524  | 0.022 034 540 569  | -0.009 189 007 338 |
| H                                                             | -0.001 709 463 607 | 0.002 945 543 107  | -0.059 218 683 017 |
| H                                                             | -0.021 673 767 712 | -0.040 177 526 743 | 0.140 755 953 238  |
| H                                                             | 0.054 844 959 687  | 0.160 772 094 958  | 0.076 671 709 815  |
| H                                                             | -0.019 983 152 328 | -0.088 431 785 330 | 0.031 802 309 390  |
| H                                                             | -0.006 576 161 794 | -0.066 860 011 245 | -0.003 920 451 041 |
| H                                                             | 0.036 385 237 261  | 0.072 443 683 813  | 0.040 750 805 893  |
| H                                                             | 0.089 439 326 119  | -0.001 014 444 363 | -0.051 226 766 943 |
| H                                                             | -0.003 586 357 199 | 0.045 090 666 944  | 0.012 174 073 832  |
| H                                                             | 0.044 992 767 241  | 0.002 958 472 210  | -0.022 176 188 114 |

Wavenumber/cm<sup>-1</sup>: 2917.8171 , Max excitation: 1

| $l'$ -matrix coefficients/(u <sup>1/2</sup> Å <sup>-1</sup> ) |                    |                    |
|---------------------------------------------------------------|--------------------|--------------------|
| O                                                             | 0.289 373 800 925  | 0.079 314 435 989  |
| C                                                             | -0.047 088 156 728 | -0.087 895 834 024 |
| C                                                             | -0.038 166 228 628 | 0.086 815 891 720  |
| C                                                             | 0.156 395 895 625  | 0.177 396 291 192  |
| C                                                             | -0.217 317 664 926 | 0.005 713 582 240  |
| C                                                             | -0.049 317 455 299 | -0.156 822 310 731 |
| C                                                             | -0.217 034 799 199 | 0.185 858 572 536  |
| C                                                             | -0.050 685 455 552 | -0.208 999 880 311 |
| C                                                             | 0.045 785 127 749  | 0.234 689 414 154  |
| C                                                             | -0.018 664 893 870 | -0.191 789 697 967 |
| C                                                             | 0.081 436 492 107  | -0.075 529 679 627 |
| H                                                             | 0.014 268 484 862  | 0.079 072 060 785  |
| H                                                             | 0.007 077 395 752  | -0.021 919 045 887 |
| H                                                             | -0.142 759 071 690 | 0.090 868 042 708  |
| H                                                             | 0.010 212 474 131  | -0.032 483 619 413 |
| H                                                             | -0.027 230 380 901 | -0.030 327 677 949 |
| H                                                             | -0.005 552 363 306 | -0.075 872 621 401 |
| H                                                             | 0.140 626 048 082  | -0.081 326 082 404 |
| H                                                             | -0.033 066 589 030 | 0.058 710 522 501  |
| H                                                             | 0.022 133 398 202  | 0.062 425 004 374  |
| H                                                             | 0.013 804 691 321  | -0.027 828 704 922 |
| H                                                             | 0.033 237 097 442  | -0.167 145 757 185 |
| H                                                             | 0.078 258 439 185  | -0.011 317 633 674 |
| H                                                             | 0.011 593 988 430  | -0.064 722 711 338 |
| H                                                             | -0.036 052 068 486 | -0.039 513 075 572 |
| H                                                             | 0.010 099 407 333  | 0.106 745 592 647  |
| H                                                             | -0.025 269 336 066 | -0.055 854 182 290 |

Wavenumber/cm<sup>-1</sup>: 2976.4281 , Max excitation: 1

| $l'$ -matrix coefficients/(u <sup>1/2</sup> Å <sup>-1</sup> ) |                    |                                       |                    |
|---------------------------------------------------------------|--------------------|---------------------------------------|--------------------|
| O                                                             | 0.393 297 028 664  | 0.139 096 127 476                     | 0.066 021 830 505  |
| C                                                             | 0.032 420 893 827  | -0.007 033 712 656                    | -0.185 382 676 452 |
| C                                                             | -0.264 076 631 703 | -7.110 094 200 000 × 10 <sup>-5</sup> | 0.112 367 160 051  |
| C                                                             | 0.338 899 825 290  | -0.061 762 199 204                    | -0.059 884 306 972 |
| C                                                             | -0.127 439 815 187 | 0.050 329 714 657                     | -0.015 199 873 194 |
| C                                                             | 0.004 273 645 614  | 0.110 050 132 926                     | -0.236 781 087 643 |
| C                                                             | -0.031 392 701 372 | -0.045 888 670 718                    | 0.032 932 486 965  |
| C                                                             | 0.011 608 579 166  | 0.012 973 019 598                     | -0.079 426 758 414 |
| C                                                             | 0.107 523 302 185  | -0.160 219 846 471                    | 0.168 853 606 317  |
| C                                                             | -0.029 770 253 891 | -0.104 709 535 017                    | -0.031 374 670 114 |
| C                                                             | -0.424 293 862 961 | 0.090 428 572 896                     | 0.165 224 723 206  |
| H                                                             | 0.073 820 110 465  | -0.139 218 196 295                    | 0.168 089 811 072  |
| H                                                             | -0.036 443 313 771 | 0.051 877 345 312                     | -0.000 153 504 849 |
| H                                                             | 0.010 188 724 371  | -0.065 046 285 796                    | 0.003 277 782 201  |
| H                                                             | -0.032 490 458 472 | 0.082 879 229 002                     | -0.132 371 351 278 |
| H                                                             | -0.018 852 734 078 | 0.004 617 999 758                     | -0.015 707 419 337 |
| H                                                             | -0.003 303 787 927 | 0.019 149 417 108                     | 0.034 508 876 359  |
| H                                                             | -0.142 198 722 973 | 0.037 912 129 460                     | 0.052 049 205 211  |
| H                                                             | -0.077 426 476 099 | -0.039 065 392 560                    | 0.046 219 947 759  |
| H                                                             | 0.109 428 815 793  | -0.022 056 290 688                    | 0.000 182 036 131  |
| H                                                             | -0.025 111 717 343 | -0.072 973 343 219                    | -0.002 612 761 610 |
| H                                                             | 0.021 296 461 908  | -0.019 033 015 597                    | 0.017 670 497 484  |
| H                                                             | 0.035 118 999 994  | 0.023 294 172 701                     | -0.033 343 952 155 |
| H                                                             | -0.023 307 852 586 | -0.059 607 898 737                    | 0.008 200 191 201  |
| H                                                             | -0.122 154 630 875 | 0.030 991 274 633                     | 0.026 352 610 693  |
| H                                                             | 0.093 608 879 383  | -0.006 613 605 494                    | -0.026 904 060 730 |
| H                                                             | -0.109 589 366 881 | 0.018 819 566 915                     | 0.035 677 153 408  |

Wavenumber/cm<sup>-1</sup>: 3008.1543 , Max excitation: 1

| $l'$ -matrix coefficients/(u <sup>1/2</sup> Å <sup>-1</sup> ) |                    |                    |                    |
|---------------------------------------------------------------|--------------------|--------------------|--------------------|
| O                                                             | 0.071 999 752 563  | 0.177 329 501 526  | 0.074 244 081 397  |
| C                                                             | 0.285 890 035 296  | -0.080 286 325 000 | 0.165 613 649 533  |
| C                                                             | 0.241 578 109 885  | 0.190 106 744 487  | 0.184 493 794 351  |
| C                                                             | 0.128 266 407 766  | -0.093 695 237 647 | -0.227 040 245 494 |
| C                                                             | -0.139 728 062 613 | 0.246 136 830 247  | 0.039 320 763 097  |
| C                                                             | -0.106 964 194 851 | -0.088 814 952 097 | 0.087 699 610 505  |
| C                                                             | -0.191 886 648 505 | -0.198 357 158 353 | -0.007 917 119 554 |
| C                                                             | 0.022 509 776 296  | -0.052 154 981 766 | -0.081 827 409 810 |
| C                                                             | -0.115 133 139 084 | -0.028 599 794 951 | 0.010 807 233 517  |
| C                                                             | -0.055 910 814 604 | 0.071 247 191 535  | -0.016 207 331 576 |
| C                                                             | 0.093 122 211 517  | -0.062 618 593 659 | -0.129 732 150 564 |
| H                                                             | -0.073 286 690 643 | -0.005 168 450 077 | -0.092 627 529 488 |
| H                                                             | -0.117 663 353 427 | -0.052 251 319 647 | 0.150 332 308 956  |
| H                                                             | -0.034 454 095 992 | -0.150 894 706 146 | -0.016 853 269 742 |
| H                                                             | -0.108 432 107 094 | 0.018 310 591 454  | -0.080 608 482 463 |
| H                                                             | -0.113 052 701 397 | 0.170 664 068 022  | 0.009 918 465 618  |
| H                                                             | -0.086 818 202 194 | -0.012 050 763 533 | -0.054 228 139 780 |
| H                                                             | -0.034 447 867 296 | -0.057 394 373 044 | -0.076 976 406 198 |
| H                                                             | -0.152 442 502 683 | -0.092 816 159 492 | 0.073 826 320 914  |
| H                                                             | -0.078 806 918 035 | -0.002 207 175 343 | -0.078 889 494 846 |
| H                                                             | -0.085 524 314 380 | -0.043 523 918 560 | -0.068 490 489 294 |
| H                                                             | 0.043 143 890 933  | -0.127 114 491 340 | 0.010 762 809 188  |
| H                                                             | 0.091 502 657 439  | 0.030 328 927 049  | -0.115 341 971 246 |
| H                                                             | -0.037 085 683 769 | 0.184 921 198 465  | 0.021 908 885 614  |
| H                                                             | -0.100 676 000 626 | -0.027 212 527 373 | -0.041 554 406 945 |
| H                                                             | -0.092 827 810 466 | -0.120 884 498 391 | 0.108 334 790 743  |
| H                                                             | 0.135 682 692 374  | -0.084 233 854 668 | -0.132 334 948 098 |

Wavenumber/cm<sup>-1</sup>: 3031.0453 , Max excitation: 1

| $l'$ -matrix coefficients/(u <sup>1/2</sup> Å <sup>-1</sup> ) |                    |                    |
|---------------------------------------------------------------|--------------------|--------------------|
| O                                                             | -0.200 620 118 105 | -0.114 813 421 681 |
| C                                                             | -0.111 732 786 536 | 0.162 426 051 086  |
| C                                                             | -0.075 444 498 965 | 0.183 051 559 374  |
| C                                                             | -0.147 790 307 260 | -0.081 295 591 974 |
| C                                                             | -0.100 033 242 145 | 0.174 737 059 589  |
| C                                                             | 0.166 288 376 734  | -0.070 607 058 569 |
| C                                                             | -0.005 360 629 942 | -0.179 697 657 371 |
| C                                                             | 0.250 420 167 491  | -0.062 284 527 365 |
| C                                                             | 0.081 681 676 319  | 0.036 364 860 378  |
| C                                                             | 0.050 431 190 846  | 0.156 642 605 139  |
| C                                                             | -0.076 080 587 533 | -0.056 583 625 746 |
| H                                                             | 0.041 245 123 953  | -0.051 652 985 303 |
| H                                                             | 0.101 318 262 685  | -0.001 764 486 462 |
| H                                                             | 0.174 663 780 817  | -0.165 230 794 958 |
| H                                                             | 0.064 292 874 959  | -0.120 103 699 866 |
| H                                                             | -0.028 481 359 691 | 0.067 719 484 907  |
| H                                                             | 0.039 208 298 887  | 0.038 301 433 375  |
| H                                                             | 0.063 467 521 356  | -0.074 418 692 818 |
| H                                                             | -0.095 273 224 798 | -0.070 262 261 513 |
| H                                                             | 0.046 674 110 375  | 0.028 871 323 882  |
| H                                                             | 0.033 807 122 827  | 0.079 531 601 940  |
| H                                                             | 0.127 527 368 342  | -0.136 298 785 720 |
| H                                                             | 0.168 369 582 147  | 0.032 157 828 786  |
| H                                                             | 0.019 217 230 791  | 0.008 047 008 733  |
| H                                                             | -0.073 128 345 270 | -0.031 465 769 157 |
| H                                                             | 0.051 871 186 480  | -0.018 491 592 652 |
| H                                                             | -0.047 265 900 536 | -0.034 534 653 439 |

Wavenumber/cm<sup>-1</sup>: 3035.8722 , Max excitation: 1

| $l'$ -matrix coefficients/(u <sup>1/2</sup> Å <sup>-1</sup> ) |                    |                    |                    |
|---------------------------------------------------------------|--------------------|--------------------|--------------------|
| O                                                             | 0.074 856 466 981  | -0.008 334 922 936 | -0.016 287 815 219 |
| C                                                             | -0.014 469 183 180 | -0.066 095 205 097 | -0.027 081 547 390 |
| C                                                             | -0.071 225 047 387 | -0.035 409 549 215 | -0.023 397 243 016 |
| C                                                             | 0.073 536 889 697  | -0.057 251 476 740 | 0.080 558 274 489  |
| C                                                             | 0.052 653 113 060  | -0.106 477 419 794 | 0.034 832 332 479  |
| C                                                             | 0.122 099 077 986  | -0.095 673 401 192 | -0.013 442 065 395 |
| C                                                             | 0.126 009 205 547  | -0.142 980 404 917 | 0.181 452 114 017  |
| C                                                             | 0.173 855 814 782  | -0.137 262 787 348 | 0.038 497 885 325  |
| C                                                             | -0.365 305 582 036 | 0.263 923 559 466  | 0.109 919 457 159  |
| C                                                             | -0.006 030 927 209 | -0.086 356 149 665 | -0.049 598 710 395 |
| C                                                             | -0.128 301 235 317 | 0.365 384 318 008  | -0.291 151 661 313 |
| H                                                             | -0.106 946 547 882 | 0.221 090 651 923  | 0.000 251 529 726  |
| H                                                             | 0.051 810 928 576  | 0.002 372 623 542  | -0.014 255 733 659 |
| H                                                             | 0.078 901 529 845  | -0.078 325 671 883 | 0.048 968 119 981  |
| H                                                             | 0.027 831 553 217  | -0.047 973 352 601 | 0.001 043 546 004  |
| H                                                             | 0.042 512 599 489  | -0.068 199 461 689 | 0.011 042 777 485  |
| H                                                             | 0.010 642 162 893  | -0.033 983 133 185 | -0.018 069 188 009 |
| H                                                             | -0.141 294 124 144 | 0.203 462 335 567  | -0.046 179 488 093 |
| H                                                             | 0.021 719 316 983  | -0.040 526 292 713 | 0.107 763 476 352  |
| H                                                             | -0.229 183 503 725 | 0.035 738 035 237  | 0.120 488 058 747  |
| H                                                             | -0.002 757 047 032 | -0.013 746 332 662 | -0.024 324 504 049 |
| H                                                             | 0.063 605 988 757  | -0.061 230 061 082 | 0.039 670 134 452  |
| H                                                             | 0.077 023 614 404  | -0.025 594 619 405 | -0.011 767 340 109 |
| H                                                             | -0.006 481 691 587 | -0.026 514 958 411 | -0.008 400 459 228 |
| H                                                             | 0.040 917 307 461  | 0.134 326 695 142  | -0.189 821 992 802 |
| H                                                             | -0.090 181 278 142 | 0.056 117 444 552  | 0.026 448 364 874  |
| H                                                             | -0.008 017 615 224 | 0.115 172 584 664  | -0.118 077 264 973 |

Wavenumber/cm<sup>-1</sup>: 3038.8493 , Max excitation: 1

| $l'$ -matrix coefficients/(u <sup>1/2</sup> Å <sup>-1</sup> ) |                    |                    |                    |
|---------------------------------------------------------------|--------------------|--------------------|--------------------|
| O                                                             | 0.119 785 149 745  | -0.114 930 719 744 | -0.129 831 964 556 |
| C                                                             | -0.020 163 334 364 | -0.003 921 772 382 | 0.230 323 663 076  |
| C                                                             | -0.061 134 215 455 | 0.022 218 805 840  | 0.188 546 072 051  |
| C                                                             | -0.004 207 344 108 | 0.207 283 682 285  | 0.153 416 549 934  |
| C                                                             | 0.003 343 261 450  | 0.099 805 108 630  | 0.033 414 209 535  |
| C                                                             | 0.094 429 756 953  | -0.301 556 682 760 | 0.109 502 952 766  |
| C                                                             | 0.019 615 090 933  | 0.304 883 670 090  | 0.038 923 774 029  |
| C                                                             | -0.091 011 769 691 | -0.121 185 070 484 | -0.097 841 138 896 |
| C                                                             | 0.021 447 687 475  | -0.258 850 733 901 | 0.041 533 834 757  |
| C                                                             | 0.117 891 745 150  | 0.143 755 603 052  | -0.187 336 820 406 |
| C                                                             | -0.219 619 208 989 | 0.075 177 082 005  | -0.162 291 440 163 |
| H                                                             | -0.021 437 364 741 | -0.177 797 102 299 | -0.031 537 106 289 |
| H                                                             | 0.055 851 300 215  | -0.143 435 648 828 | -0.041 641 312 522 |
| H                                                             | 0.001 545 150 790  | 0.134 428 641 245  | 0.021 718 720 546  |
| H                                                             | 0.060 575 497 870  | -0.148 763 268 052 | 0.102 035 635 692  |
| H                                                             | 0.024 433 899 936  | 0.052 670 938 604  | -0.033 416 083 717 |
| H                                                             | 0.039 935 137 348  | -0.082 887 328 587 | -0.157 686 316 713 |
| H                                                             | -0.159 545 893 574 | -0.001 863 879 237 | -0.081 741 257 275 |
| H                                                             | 0.034 210 001 201  | 0.094 767 327 488  | -0.034 135 714 378 |
| H                                                             | 0.091 865 337 198  | -0.044 463 240 546 | -0.063 659 933 462 |
| H                                                             | 0.060 851 304 835  | 0.150 960 199 863  | -0.093 132 587 107 |
| H                                                             | -0.044 722 580 907 | 0.017 278 550 829  | -0.047 845 525 194 |
| H                                                             | -0.084 202 612 092 | -0.075 806 095 175 | -0.059 503 862 205 |
| H                                                             | 0.055 560 417 828  | 0.108 084 569 596  | -0.080 188 258 430 |
| H                                                             | -0.062 359 438 654 | 0.017 249 150 005  | -0.023 860 968 767 |
| H                                                             | -0.052 295 634 052 | -0.083 124 496 148 | 0.070 018 196 087  |
| H                                                             | 0.003 736 877 843  | 0.062 009 256 707  | -0.130 113 946 820 |



Wavenumber/cm<sup>-1</sup>: 3054.2663 , Max excitation: 1

| $l'$ -matrix coefficients/(u <sup>1/2</sup> Å <sup>-1</sup> ) |                    |                    |
|---------------------------------------------------------------|--------------------|--------------------|
| O -0.038 614 245 118                                          | -0.019 768 655 537 | -0.163 276 382 392 |
| C -0.058 827 275 537                                          | -0.070 298 817 894 | 0.071 274 800 555  |
| C -0.015 358 731 228                                          | -0.053 232 152 326 | 0.057 813 478 856  |
| C -0.138 992 223 568                                          | 0.258 997 638 767  | -0.108 846 009 338 |
| C 0.060 741 780 637                                           | -0.064 133 298 270 | -0.035 803 405 238 |
| C -0.446 212 773 706                                          | -0.002 462 782 163 | 0.065 909 686 042  |
| C 0.108 488 136 362                                           | 0.017 962 457 166  | 0.049 530 493 773  |
| C 0.130 839 963 238                                           | -0.208 566 116 720 | -0.090 370 664 112 |
| C 0.131 996 818 034                                           | -0.023 561 426 867 | 0.110 117 189 395  |
| C 0.080 161 087 811                                           | -0.010 169 304 690 | -0.152 951 313 168 |
| C 0.094 328 286 835                                           | 0.167 538 087 706  | 0.184 914 898 299  |
| H 0.063 319 018 865                                           | 0.009 791 885 600  | 0.089 946 454 945  |
| H -0.213 349 645 486                                          | 0.053 800 912 294  | 0.180 632 085 938  |
| H 0.070 122 742 611                                           | -0.052 876 109 747 | 0.008 087 309 869  |
| H -0.255 262 229 158                                          | 0.004 964 637 037  | -0.117 070 935 571 |
| H 0.037 530 334 621                                           | -0.017 945 097 666 | -0.031 455 506 034 |
| H 0.021 067 415 794                                           | -0.066 020 836 737 | -0.097 807 724 219 |
| H 0.086 561 393 537                                           | 0.180 787 982 442  | 0.148 382 167 236  |
| H 0.056 481 782 873                                           | 0.028 877 288 214  | 0.090 384 004 271  |
| H 0.013 854 807 303                                           | -0.011 195 020 929 | 0.027 983 121 078  |
| H 0.058 541 217 224                                           | 0.063 923 204 029  | -0.037 658 000 075 |
| H 0.062 744 977 444                                           | -0.215 135 483 453 | -0.056 188 086 103 |
| H 0.171 994 845 381                                           | 0.024 284 628 199  | -0.038 410 334 025 |
| H 0.052 035 497 891                                           | 0.011 299 565 609  | -0.078 455 007 906 |
| H 0.053 382 298 783                                           | 0.082 242 599 934  | -0.094 161 078 300 |
| H 0.087 335 988 712                                           | -0.009 635 412 439 | -0.012 131 437 499 |
| H -0.030 132 988 217                                          | -0.050 085 048 800 | 0.145 146 129 611  |

Wavenumber/cm<sup>-1</sup>: 3074.1397 , Max excitation: 1

| $l'$ -matrix coefficients/(u <sup>1/2</sup> Å <sup>-1</sup> ) |                    |                    |                    |
|---------------------------------------------------------------|--------------------|--------------------|--------------------|
| O                                                             | 0.276 758 028 351  | -0.171 425 791 148 | -0.228 207 566 229 |
| C                                                             | 0.066 223 685 732  | 0.028 773 186 202  | -0.023 261 731 373 |
| C                                                             | 0.048 354 950 470  | 0.022 965 564 885  | -0.014 735 054 613 |
| C                                                             | 0.161 728 029 286  | 0.045 713 401 438  | 0.144 735 903 228  |
| C                                                             | 0.103 436 320 342  | 0.061 396 247 862  | -0.104 901 892 686 |
| C                                                             | -0.157 948 384 488 | -0.009 736 438 056 | -0.057 963 116 363 |
| C                                                             | 0.228 476 063 494  | -0.055 249 829 406 | 0.229 819 449 252  |
| C                                                             | -0.347 537 742 872 | 0.101 431 570 520  | -0.129 411 405 429 |
| C                                                             | -0.263 880 150 702 | 0.107 128 875 871  | 0.018 252 803 278  |
| C                                                             | -0.086 288 443 659 | 0.082 901 630 421  | -0.071 400 351 886 |
| C                                                             | 0.076 779 720 186  | -0.188 061 189 741 | 0.221 968 101 318  |
| H                                                             | -0.062 189 059 573 | 0.138 956 786 642  | 0.014 379 536 217  |
| H                                                             | -0.064 773 758 848 | -0.062 341 418 516 | -0.018 212 963 565 |
| H                                                             | 0.142 244 640 414  | -0.060 751 665 620 | 0.065 274 848 592  |
| H                                                             | -0.025 995 283 275 | 0.021 646 248 943  | -0.012 562 417 249 |
| H                                                             | 0.072 774 716 137  | 0.032 776 328 519  | -0.085 834 263 647 |
| H                                                             | -0.074 275 688 950 | 0.021 952 342 520  | -0.038 567 495 611 |
| H                                                             | 0.056 688 675 046  | -0.099 380 947 847 | 0.041 780 012 190  |
| H                                                             | 0.039 658 485 987  | -0.017 185 225 701 | 0.138 728 579 257  |
| H                                                             | -0.202 782 077 999 | 0.007 435 930 268  | -0.000 602 415 438 |
| H                                                             | -0.031 784 380 392 | -0.004 496 961 747 | -0.010 417 487 972 |
| H                                                             | -0.142 671 218 653 | 0.126 016 953 238  | -0.102 075 957 675 |
| H                                                             | -0.191 324 908 338 | -0.022 560 126 351 | 0.017 602 664 533  |
| H                                                             | -0.009 848 491 988 | 0.073 849 257 975  | -0.038 357 211 132 |
| H                                                             | 0.009 984 269 430  | -0.068 199 403 869 | 0.122 344 543 719  |
| H                                                             | -0.030 052 515 764 | -0.056 869 739 388 | 0.001 419 521 420  |
| H                                                             | 0.000 821 719 217  | -0.028 822 648 413 | 0.078 671 045 858  |

Wavenumber/cm<sup>-1</sup>: 3081.0242 , Max excitation: 1

| $l'$ -matrix coefficients/(u <sup>1/2</sup> Å <sup>-1</sup> ) |                    |                    |                    |
|---------------------------------------------------------------|--------------------|--------------------|--------------------|
| O                                                             | 0.187 878 103 407  | -0.336 722 299 581 | -0.186 310 743 823 |
| C                                                             | 0.009 312 676 919  | 0.092 834 855 420  | 0.013 073 774 076  |
| C                                                             | -0.003 973 351 870 | 0.047 971 500 894  | -0.029 259 201 443 |
| C                                                             | 0.067 041 624 757  | -0.002 700 784 990 | 0.138 734 662 476  |
| C                                                             | 0.049 224 736 617  | 0.055 691 034 465  | 0.013 954 925 885  |
| C                                                             | -0.131 916 409 568 | 0.131 667 595 588  | 0.010 116 761 532  |
| C                                                             | 0.008 598 747 930  | 0.160 973 206 668  | -0.078 835 674 168 |
| C                                                             | 0.202 481 986 624  | 0.004 760 523 338  | -0.006 130 921 947 |
| C                                                             | -0.223 447 305 522 | -0.235 088 724 448 | -0.242 508 247 026 |
| C                                                             | -0.119 717 095 729 | -0.013 571 122 329 | 0.390 165 360 847  |
| C                                                             | 0.018 942 558 158  | 0.129 470 306 433  | -0.019 512 007 577 |
| H                                                             | -0.115 610 656 803 | -0.150 832 641 074 | -0.174 663 469 065 |
| H                                                             | -0.069 033 259 234 | 0.087 920 617 547  | 0.076 786 724 692  |
| H                                                             | -0.009 078 678 752 | 0.110 960 559 044  | -0.009 273 693 027 |
| H                                                             | -0.102 949 561 102 | 0.038 936 086 582  | -0.063 913 960 135 |
| H                                                             | 0.014 350 511 039  | 0.006 815 845 002  | 0.010 283 888 498  |
| H                                                             | -0.001 995 987 867 | 0.076 392 289 941  | 0.189 894 927 577  |
| H                                                             | -0.004 090 273 984 | 0.043 182 546 626  | -0.004 466 569 793 |
| H                                                             | 0.014 133 385 995  | 0.044 259 854 718  | -0.082 818 745 054 |
| H                                                             | 0.011 708 633 664  | -0.042 434 453 419 | -0.126 086 470 134 |
| H                                                             | -0.068 168 990 828 | -0.067 119 059 216 | 0.105 996 457 480  |
| H                                                             | 0.080 410 661 141  | -0.091 679 763 128 | 0.000 744 056 950  |
| H                                                             | 0.141 647 242 796  | 0.052 994 961 633  | -0.015 243 412 616 |
| H                                                             | -0.075 215 830 592 | -0.057 246 957 206 | 0.163 166 751 210  |
| H                                                             | 0.026 549 438 453  | 0.040 346 259 081  | -0.010 080 831 913 |
| H                                                             | -0.163 465 732 861 | -0.086 370 103 411 | 0.029 278 155 743  |
| H                                                             | -0.001 558 814 736 | 0.051 236 339 652  | -0.002 511 090 896 |

Wavenumber/cm<sup>-1</sup>: 3085.8103 , Max excitation: 1

| $l'$ -matrix coefficients/(u <sup>1/2</sup> Å <sup>-1</sup> ) |                    |                                       |                    |
|---------------------------------------------------------------|--------------------|---------------------------------------|--------------------|
| O                                                             | 0.154 560 004 247  | -0.379 044 333 839                    | 0.461 318 097 542  |
| C                                                             | 0.022 127 107 171  | 0.034 458 841 207                     | -0.063 336 780 793 |
| C                                                             | -0.045 412 132 145 | -0.004 488 268 236                    | -0.008 490 259 437 |
| C                                                             | -0.170 458 161 957 | 0.465 672 850 056                     | -0.500 319 586 306 |
| C                                                             | 0.007 793 966 547  | -5.090 896 400 000 × 10 <sup>-5</sup> | -0.001 145 957 693 |
| C                                                             | 0.144 233 379 995  | -0.023 365 419 776                    | -0.053 212 606 079 |
| C                                                             | 0.025 020 939 532  | -0.009 668 249 726                    | 0.020 553 730 384  |
| C                                                             | 0.022 449 636 570  | 0.012 135 737 150                     | -0.004 601 860 915 |
| C                                                             | -0.124 918 987 716 | -0.015 030 455 517                    | -0.028 623 688 732 |
| C                                                             | -0.051 571 706 847 | 0.033 221 670 313                     | 0.005 577 117 124  |
| C                                                             | -0.006 368 618 945 | -0.016 871 187 464                    | 0.060 135 111 748  |
| H                                                             | -0.049 949 239 811 | -0.031 977 091 814                    | -0.035 634 956 356 |
| H                                                             | 0.064 793 875 543  | -0.012 950 762 819                    | -0.052 026 640 092 |
| H                                                             | 0.011 521 978 540  | -0.132 867 539 040                    | -0.020 032 178 417 |
| H                                                             | 0.075 429 573 406  | -0.017 141 180 636                    | 0.023 667 417 708  |
| H                                                             | 0.004 605 181 281  | -0.004 477 380 803                    | -0.000 204 872 957 |
| H                                                             | -0.019 276 292 962 | 0.020 516 416 298                     | 0.009 183 422 602  |
| H                                                             | 0.018 421 159 298  | 0.009 864 325 468                     | 0.031 737 343 857  |
| H                                                             | 0.031 185 327 490  | 0.023 956 525 715                     | 0.122 527 011 436  |
| H                                                             | -0.004 370 933 418 | 0.000 920 123 940                     | -0.001 005 455 818 |
| H                                                             | -0.021 511 137 794 | -0.006 164 828 257                    | 0.002 355 378 019  |
| H                                                             | 0.004 585 545 704  | 0.025 808 044 254                     | 0.009 105 440 167  |
| H                                                             | -0.014 645 711 837 | -0.011 113 918 648                    | -0.007 341 386 823 |
| H                                                             | -0.018 604 976 276 | 0.011 761 662 838                     | 0.006 262 275 242  |
| H                                                             | -0.002 579 726 041 | -0.001 379 102 964                    | 0.000 588 979 142  |
| H                                                             | -0.070 354 021 994 | 0.014 022 623 492                     | 0.016 547 270 880  |
| H                                                             | -0.013 668 243 124 | -0.021 828 733 860                    | 0.035 932 730 837  |

Wavenumber/cm<sup>-1</sup>: 3088.6278 , Max excitation: 1

| $l'$ -matrix coefficients/(u <sup>1/2</sup> Å <sup>-1</sup> ) |                    |                    |
|---------------------------------------------------------------|--------------------|--------------------|
| O -0.055 198 877 915                                          | 0.183 270 098 103  | 0.067 267 071 308  |
| C 0.011 723 589 094                                           | 0.036 282 426 278  | -0.005 858 224 031 |
| C -0.054 361 197 680                                          | 0.023 390 085 851  | -0.029 743 443 236 |
| C -0.041 570 633 083                                          | 0.110 208 851 152  | -0.053 848 860 130 |
| C 0.026 015 134 562                                           | 0.017 978 916 283  | 0.000 488 792 322  |
| C -0.147 336 210 725                                          | 0.089 780 098 309  | -0.006 182 028 291 |
| C 0.052 854 255 622                                           | -0.008 802 488 210 | 0.070 644 158 078  |
| C -0.069 824 949 383                                          | 0.055 583 827 532  | 0.006 829 735 122  |
| C -0.205 000 734 457                                          | -0.058 297 819 005 | -0.094 681 342 549 |
| C 0.598 206 740 984                                           | -0.143 578 188 613 | 0.172 104 422 643  |
| C -0.165 470 112 922                                          | -0.210 128 841 286 | -0.141 086 389 978 |
| H -0.061 843 313 149                                          | 0.009 692 893 050  | -0.038 779 134 697 |
| H -0.067 643 276 421                                          | 0.030 635 715 937  | 0.040 748 000 857  |
| H 0.031 800 215 684                                           | -0.042 485 136 108 | 0.014 164 861 921  |
| H -0.066 118 067 897                                          | 0.051 499 930 823  | -0.039 967 003 841 |
| H 0.016 937 812 336                                           | 0.002 660 196 718  | -0.007 632 589 665 |
| H 0.183 014 954 415                                           | -0.019 930 479 694 | 0.070 957 616 072  |
| H -0.059 905 895 708                                          | -0.089 741 753 921 | -0.062 620 669 491 |
| H 0.016 115 357 689                                           | 0.004 156 236 653  | 0.064 166 997 711  |
| H -0.099 271 024 468                                          | -0.018 595 204 630 | -0.053 181 774 450 |
| H 0.273 888 200 020                                           | 0.027 458 156 376  | 0.162 721 033 961  |
| H -0.024 115 807 646                                          | 0.008 578 849 540  | -0.017 443 098 542 |
| H -0.014 494 126 359                                          | 0.021 097 241 880  | 0.022 448 126 814  |
| H 0.242 709 284 182                                           | -0.194 272 769 435 | -0.035 033 904 758 |
| H -0.105 516 818 629                                          | -0.068 207 371 877 | -0.022 577 098 451 |
| H -0.055 796 663 412                                          | -0.066 942 835 379 | -0.008 621 706 633 |
| H -0.007 918 257 109                                          | -0.083 431 020 077 | -0.076 586 392 969 |

Wavenumber/cm<sup>-1</sup>: 3095.047 , Max excitation: 1

| $l'$ -matrix coefficients/(u <sup>1/2</sup> Å <sup>-1</sup> ) |                    |                    |                    |
|---------------------------------------------------------------|--------------------|--------------------|--------------------|
| O                                                             | -0.024 072 494 346 | 0.127 436 823 035  | 0.037 483 524 622  |
| C                                                             | 0.019 692 294 843  | -0.018 573 322 676 | -0.005 175 847 693 |
| C                                                             | -0.001 270 282 219 | 0.005 886 320 711  | 0.009 544 936 847  |
| C                                                             | -0.004 585 919 954 | 0.030 832 508 924  | -0.039 233 344 602 |
| C                                                             | -0.021 029 294 989 | 0.010 335 070 230  | 0.000 835 436 867  |
| C                                                             | 0.035 017 621 582  | -0.057 336 334 865 | -0.022 265 782 532 |
| C                                                             | -0.016 302 913 508 | 0.025 209 465 003  | -0.016 173 056 853 |
| C                                                             | -0.057 063 750 101 | -0.013 428 744 305 | -0.018 723 331 392 |
| C                                                             | -0.058 332 451 239 | -0.123 853 749 884 | -0.092 405 904 934 |
| C                                                             | 0.063 279 857 766  | -0.045 730 295 568 | 0.041 425 171 381  |
| C                                                             | 0.058 994 130 117  | 0.080 213 764 307  | 0.100 860 270 672  |
| H                                                             | 0.045 763 642 188  | 0.126 131 504 032  | 0.096 187 154 569  |
| H                                                             | 0.023 734 046 195  | -0.028 663 422 928 | -0.034 230 625 993 |
| H                                                             | -0.015 235 103 743 | 0.008 005 163 197  | -0.005 947 881 727 |
| H                                                             | 0.033 942 619 463  | -0.019 983 870 650 | 0.018 857 224 035  |
| H                                                             | -0.006 064 992 987 | 0.012 670 848 518  | -0.007 250 941 562 |
| H                                                             | 0.488 571 226 303  | -0.124 667 948 183 | 0.062 574 142 404  |
| H                                                             | 0.037 004 400 602  | 0.045 381 010 585  | 0.048 516 548 077  |
| H                                                             | -0.003 587 578 804 | 0.005 897 582 958  | -0.010 332 096 606 |
| H                                                             | -0.243 655 897 949 | -0.064 123 394 648 | -0.118 632 792 171 |
| H                                                             | -0.144 363 608 790 | 0.179 816 168 053  | -0.400 089 563 462 |
| H                                                             | -0.023 989 729 420 | 0.022 527 338 737  | -0.008 366 781 060 |
| H                                                             | -0.039 626 515 260 | -0.018 326 656 692 | -0.005 505 795 658 |
| H                                                             | -0.287 179 592 375 | -0.100 632 169 596 | 0.380 631 854 102  |
| H                                                             | 0.033 543 426 949  | 0.027 932 931 073  | 0.009 291 634 324  |
| H                                                             | 0.139 407 741 739  | -0.227 957 716 964 | -0.089 439 649 656 |
| H                                                             | -0.005 871 363 442 | 0.015 721 437 486  | 0.057 006 591 050  |

Wavenumber/cm<sup>-1</sup>: 3101.5455 , Max excitation: 1

| $l'$ -matrix coefficients/(u <sup>1/2</sup> Å <sup>-1</sup> ) |                    |                    |                    |
|---------------------------------------------------------------|--------------------|--------------------|--------------------|
| O                                                             | -0.056 684 383 278 | 0.219 968 553 941  | 0.445 247 235 170  |
| C                                                             | -0.005 709 635 837 | -0.032 570 970 712 | -0.053 531 274 301 |
| C                                                             | -0.000 465 256 983 | -0.002 542 621 689 | -0.028 231 508 896 |
| C                                                             | 0.082 291 827 394  | -0.183 584 405 747 | 0.167 574 586 108  |
| C                                                             | -0.005 671 183 338 | 0.010 645 111 927  | -0.093 797 173 403 |
| C                                                             | 0.018 686 608 472  | -0.090 557 292 796 | -0.080 646 375 554 |
| C                                                             | 0.027 666 118 504  | 0.065 146 926 838  | -0.091 957 643 044 |
| C                                                             | -0.042 491 420 585 | -0.040 143 490 744 | -0.133 274 393 656 |
| C                                                             | -0.240 450 503 068 | -0.202 365 426 253 | -0.183 736 295 069 |
| C                                                             | 0.067 669 111 964  | -0.015 039 985 362 | -0.162 781 967 992 |
| C                                                             | 0.167 703 606 332  | 0.230 441 638 381  | 0.255 151 378 337  |
| H                                                             | -0.097 850 637 218 | -0.082 493 274 978 | -0.116 200 618 906 |
| H                                                             | 0.016 269 671 247  | -0.041 968 169 178 | -0.049 620 372 425 |
| H                                                             | 0.006 975 506 950  | 0.079 966 565 538  | -0.015 397 453 658 |
| H                                                             | 0.022 894 043 736  | -0.041 812 566 779 | 0.003 133 676 108  |
| H                                                             | 0.003 839 675 445  | 0.013 011 470 312  | -0.039 910 592 854 |
| H                                                             | -0.121 140 749 925 | 0.001 071 961 991  | -0.086 362 834 964 |
| H                                                             | 0.127 019 360 404  | 0.176 477 713 007  | 0.159 426 833 948  |
| H                                                             | -0.010 151 717 761 | -0.000 119 724 980 | -0.089 612 512 487 |
| H                                                             | -0.061 089 326 864 | -0.046 981 987 545 | -0.108 757 556 005 |
| H                                                             | 0.083 461 403 554  | -0.031 211 168 102 | 0.077 330 395 467  |
| H                                                             | -0.021 528 203 084 | 0.011 996 156 323  | -0.048 557 251 646 |
| H                                                             | -0.033 017 414 621 | -0.024 998 946 978 | -0.038 813 611 076 |
| H                                                             | 0.122 732 225 077  | 0.026 576 290 682  | -0.172 665 912 662 |
| H                                                             | 0.092 889 693 313  | 0.094 010 486 725  | -0.037 576 822 212 |
| H                                                             | -0.116 845 386 164 | -0.110 680 791 980 | 0.013 064 995 413  |
| H                                                             | -0.027 601 216 282 | 0.000 268 349 281  | 0.175 467 927 915  |

Wavenumber/cm<sup>-1</sup>: 3107.6782 , Max excitation: 1

| $l'$ -matrix coefficients/(u <sup>1/2</sup> Å <sup>-1</sup> ) |                    |                    |
|---------------------------------------------------------------|--------------------|--------------------|
| O                                                             | -0.047 450 324 191 | 0.192 126 293 410  |
| C                                                             | -0.012 139 681 333 | -0.038 284 997 018 |
| C                                                             | 0.000 351 135 455  | -0.055 468 447 926 |
| C                                                             | -0.009 347 649 681 | 0.041 391 904 172  |
| C                                                             | 0.023 069 344 980  | -0.075 314 656 147 |
| C                                                             | -0.094 569 842 774 | 0.003 149 208 244  |
| C                                                             | 0.080 044 619 525  | -0.093 592 976 328 |
| C                                                             | -0.007 755 300 146 | -0.052 101 827 424 |
| C                                                             | -0.060 896 262 549 | -0.019 832 651 981 |
| C                                                             | 0.015 678 708 513  | -0.034 995 821 408 |
| C                                                             | 0.094 790 837 765  | 0.104 938 959 714  |
| H                                                             | -0.102 993 827 117 | -0.207 759 045 986 |
| H                                                             | -0.042 756 467 232 | 0.012 998 274 069  |
| H                                                             | 0.049 598 247 411  | -0.078 367 507 472 |
| H                                                             | -0.049 466 368 922 | 0.013 647 413 230  |
| H                                                             | 0.024 332 999 406  | -0.034 468 377 106 |
| H                                                             | 0.122 530 492 236  | -0.045 400 416 491 |
| H                                                             | -0.128 238 568 206 | -0.254 850 616 209 |
| H                                                             | 0.020 100 299 551  | -0.020 815 761 132 |
| H                                                             | 0.247 758 952 662  | 0.032 293 757 656  |
| H                                                             | -0.026 075 290 732 | 0.049 112 526 653  |
| H                                                             | 0.001 309 486 267  | -0.036 134 585 891 |
| H                                                             | 0.015 180 930 503  | -0.002 248 991 176 |
| H                                                             | -0.066 485 120 165 | -0.035 156 963 717 |
| H                                                             | 0.223 835 101 383  | -0.036 391 449 133 |
| H                                                             | -0.219 308 928 252 | 0.184 711 016 085  |
| H                                                             | 0.018 836 639 057  | 0.453 204 426 806  |



Wavenumber/cm<sup>-1</sup>: 3119.1431 , Max excitation: 1

| $l'$ -matrix coefficients/(u <sup>1/2</sup> Å <sup>-1</sup> ) |                    |                    |
|---------------------------------------------------------------|--------------------|--------------------|
| O                                                             | -0.039 329 865 243 | 0.132 018 336 758  |
| C                                                             | 0.001 589 658 515  | -0.025 349 268 589 |
| C                                                             | 0.011 089 496 212  | -0.003 693 686 388 |
| C                                                             | -0.048 411 138 205 | 0.149 550 835 486  |
| C                                                             | -0.036 724 287 950 | -0.021 331 604 831 |
| C                                                             | 0.055 652 815 654  | -0.091 707 731 949 |
| C                                                             | -0.015 915 529 156 | -0.036 654 649 176 |
| C                                                             | -0.064 274 990 958 | -0.036 623 501 137 |
| C                                                             | 0.126 294 395 039  | -0.196 649 890 469 |
| C                                                             | -0.086 735 540 932 | -0.065 213 321 678 |
| C                                                             | 0.069 539 516 756  | 0.226 437 719 377  |
| H                                                             | 0.132 161 041 925  | 0.145 319 694 120  |
| H                                                             | 0.026 546 302 710  | -0.039 961 700 432 |
| H                                                             | -0.004 786 132 894 | -0.062 535 572 960 |
| H                                                             | 0.036 269 615 071  | -0.027 379 191 001 |
| H                                                             | -0.007 306 195 647 | 0.000 386 688 584  |
| H                                                             | -0.246 601 031 274 | 0.067 301 483 947  |
| H                                                             | -0.086 717 043 191 | -0.070 646 548 632 |
| H                                                             | 0.003 031 166 893  | 0.000 561 405 764  |
| H                                                             | -0.253 374 355 712 | -0.089 092 366 819 |
| H                                                             | 0.042 934 961 258  | -0.139 589 662 988 |
| H                                                             | -0.022 770 504 199 | 0.017 245 320 246  |
| H                                                             | -0.045 351 132 546 | -0.028 554 798 465 |
| H                                                             | 0.110 133 681 162  | 0.004 453 008 903  |
| H                                                             | 0.154 139 112 046  | 0.035 432 985 596  |
| H                                                             | 0.259 270 640 037  | -0.294 086 866 471 |
| H                                                             | 0.017 329 051 228  | 0.304 636 228 476  |

Wavenumber/cm<sup>-1</sup>: 3130.1554 , Max excitation: 1

| $l'$ -matrix coefficients/(u <sup>1/2</sup> Å <sup>-1</sup> ) |                    |                    |                    |
|---------------------------------------------------------------|--------------------|--------------------|--------------------|
| O                                                             | 0.048 664 689 280  | -0.293 885 789 599 | 0.254 930 390 660  |
| C                                                             | -0.023 136 651 771 | 0.037 327 493 377  | -0.017 414 475 141 |
| C                                                             | -0.040 446 687 646 | 0.003 766 438 206  | 0.020 844 918 973  |
| C                                                             | 0.009 065 196 837  | -0.147 984 551 872 | 0.118 030 054 151  |
| C                                                             | 0.006 634 067 828  | 0.023 712 011 091  | -0.020 579 049 300 |
| C                                                             | -0.079 677 110 676 | 0.140 145 776 607  | 0.031 146 338 150  |
| C                                                             | -0.069 028 233 983 | 0.132 693 379 789  | -0.194 057 175 725 |
| C                                                             | 0.227 182 404 772  | -0.004 692 883 549 | -0.003 439 113 278 |
| C                                                             | -0.091 125 632 266 | 0.098 981 593 823  | 0.073 475 483 446  |
| C                                                             | 0.079 727 513 669  | 0.102 602 842 787  | -0.250 288 671 138 |
| C                                                             | -0.067 564 902 644 | -0.134 874 848 612 | 0.044 021 520 031  |
| H                                                             | 0.039 928 010 916  | 0.228 543 108 457  | 0.146 084 742 383  |
| H                                                             | -0.048 145 336 005 | 0.084 717 928 759  | 0.070 714 350 781  |
| H                                                             | -0.056 858 330 266 | 0.141 518 059 023  | -0.039 722 618 801 |
| H                                                             | -0.083 587 691 563 | 0.036 852 533 237  | -0.049 600 116 922 |
| H                                                             | -0.015 149 283 990 | -0.003 108 759 190 | 0.018 915 116 213  |
| H                                                             | 0.002 210 116 768  | -0.012 948 777 140 | -0.114 738 350 065 |
| H                                                             | -0.104 699 543 677 | -0.237 537 109 641 | -0.129 676 970 436 |
| H                                                             | -0.011 815 485 316 | 0.026 322 271 773  | -0.159 115 512 389 |
| H                                                             | -0.262 692 534 453 | -0.012 625 828 989 | -0.005 923 542 248 |
| H                                                             | 0.045 789 284 586  | 0.066 120 359 226  | -0.063 131 811 154 |
| H                                                             | 0.093 335 206 692  | -0.099 795 472 912 | 0.013 935 222 366  |
| H                                                             | 0.151 977 812 213  | 0.052 677 561 572  | -0.019 082 238 154 |
| H                                                             | 0.047 444 553 848  | 0.055 047 750 091  | -0.102 214 334 639 |
| H                                                             | 0.034 153 748 282  | -0.086 627 145 110 | 0.253 461 461 649  |
| H                                                             | 0.135 607 938 511  | -0.116 375 878 050 | -0.067 687 506 064 |
| H                                                             | 0.005 590 002 165  | 0.179 298 598 912  | -0.083 490 460 725 |

**Equatorial (R)-(+)-3-methylcyclopentanone***Initial state*

Wavenumber/cm<sup>-1</sup>: 83.8034

| $\frac{\partial \mu_{x,y,z}}{\partial Q_r} / (e u^{-0.5})$        | -0.002 656 203 038 | 0.000 764 327 637  | 0.001 698 384 566  |
|-------------------------------------------------------------------|--------------------|--------------------|--------------------|
| <i>l</i> -matrix coefficients/(u <sup>1/2</sup> Å <sup>-1</sup> ) |                    |                    |                    |
| O                                                                 | 0.001 393 234 829  | 0.000 612 125 174  | 0.000 232 190 402  |
| C                                                                 | -0.034 039 640 669 | -0.193 782 093 410 | -0.199 955 981 059 |
| C                                                                 | 0.004 315 488 294  | 0.003 359 001 804  | -0.020 284 715 480 |
| C                                                                 | 0.009 500 813 235  | 0.017 330 978 756  | -0.018 076 693 209 |
| C                                                                 | -0.000 601 415 038 | 0.002 022 245 445  | -0.015 581 348 297 |
| C                                                                 | -0.004 240 438 762 | -0.000 543 638 488 | -0.002 454 284 556 |
| C                                                                 | 0.002 759 918 902  | 0.062 280 885 979  | 0.030 636 124 444  |
| H                                                                 | 0.026 976 155 713  | -0.076 763 402 595 | 0.180 213 641 006  |
| H                                                                 | 0.089 865 501 323  | 0.731 657 051 790  | 0.520 449 512 517  |
| H                                                                 | -0.003 983 085 060 | -0.004 148 041 266 | 0.066 002 543 124  |
| H                                                                 | -0.036 403 464 130 | -0.058 776 884 186 | 0.033 604 696 010  |
| H                                                                 | 0.006 585 727 335  | 0.002 876 112 231  | 0.030 461 494 994  |
| H                                                                 | 0.009 559 248 183  | -0.014 290 424 292 | 0.042 114 798 601  |
| H                                                                 | -0.009 093 042 088 | 0.009 827 305 744  | 0.010 587 349 633  |
| H                                                                 | 0.049 461 797 209  | -0.169 377 586 077 | -0.072 379 622 782 |
| H                                                                 | 0.001 553 661 679  | 0.010 481 310 810  | -0.060 288 187 989 |
| H                                                                 | -0.063 075 860 010 | -0.056 509 988 238 | 0.027 479 324 785  |

Wavenumber/cm<sup>-1</sup>: 172.4595

| $\frac{\partial \mu_{x,y,z}}{\partial Q_r} / (e u^{-0.5})$        | 0.004 350 358 302                     | 0.001 073 932 966                     | 0.000 606 376 397  |
|-------------------------------------------------------------------|---------------------------------------|---------------------------------------|--------------------|
| <i>l</i> -matrix coefficients/(u <sup>1/2</sup> Å <sup>-1</sup> ) |                                       |                                       |                    |
| O                                                                 | 0.000 248 113 568                     | 0.000 459 023 016                     | 0.000 452 246 904  |
| C                                                                 | -3.198 499 000 000 × 10 <sup>-6</sup> | 0.009 238 141 936                     | 0.000 518 588 539  |
| C                                                                 | -0.000 645 456 639                    | 0.001 236 757 447                     | -0.017 986 341 977 |
| C                                                                 | 0.027 926 066 528                     | 0.062 850 881 186                     | -0.092 689 831 616 |
| C                                                                 | 0.111 081 595 689                     | -0.110 383 900 301                    | -0.216 382 214 613 |
| C                                                                 | 0.000 223 170 783                     | -3.759 628 600 000 × 10 <sup>-5</sup> | -0.002 228 256 801 |
| C                                                                 | 0.012 551 725 913                     | -0.035 265 266 074                    | -0.039 048 777 892 |
| H                                                                 | 0.000 737 488 136                     | -0.004 934 046 072                    | 0.015 334 178 754  |
| H                                                                 | -0.002 088 672 332                    | -0.026 321 788 339                    | -0.018 889 665 402 |
| H                                                                 | -0.001 985 373 247                    | -0.002 066 509 283                    | 0.056 015 238 768  |
| H                                                                 | -0.140 020 870 516                    | -0.226 465 646 685                    | 0.128 711 710 566  |
| H                                                                 | 0.039 818 370 692                     | 0.013 532 346 006                     | 0.193 426 960 247  |
| H                                                                 | 0.061 153 121 926                     | -0.092 800 727 888                    | 0.229 565 544 947  |
| H                                                                 | -0.438 371 126 788                    | 0.465 797 770 969                     | 0.525 872 010 682  |
| H                                                                 | -0.038 157 859 874                    | 0.136 297 214 550                     | 0.055 638 546 779  |
| H                                                                 | 0.000 918 111 002                     | -0.008 818 868 797                    | 0.083 004 846 022  |
| H                                                                 | -0.004 703 172 211                    | -0.006 259 738 652                    | -0.000 784 156 510 |

Wavenumber/cm<sup>-1</sup>: 239.6735

| $\frac{\partial \mu_{x,y,z}}{\partial Q_r} / (e u^{-0.5})$        |                                       |                    |                                       |
|-------------------------------------------------------------------|---------------------------------------|--------------------|---------------------------------------|
|                                                                   | -0.000 579 758 660                    | 0.000 531 645 031  | 0.000 587 242 966                     |
| <i>l</i> -matrix coefficients/(u <sup>1/2</sup> Å <sup>-1</sup> ) |                                       |                    |                                       |
| O                                                                 | 0.000 576 429 351                     | -0.000 308 442 071 | -1.501 918 000 000 × 10 <sup>-6</sup> |
| C                                                                 | 0.006 728 127 954                     | 0.042 851 825 625  | 0.047 994 567 286                     |
| C                                                                 | 0.002 556 823 544                     | 0.003 597 485 964  | -0.005 730 700 569                    |
| C                                                                 | 0.057 350 395 898                     | 0.096 364 871 687  | -0.088 900 886 865                    |
| C                                                                 | -0.013 317 245 597                    | 0.013 785 458 539  | 0.021 054 884 411                     |
| C                                                                 | -0.001 009 931 407                    | -0.000 189 265 838 | 0.000 462 503 810                     |
| C                                                                 | 0.064 467 684 593                     | 0.245 813 198 175  | 0.024 092 036 362                     |
| H                                                                 | -0.007 757 776 688                    | 0.018 422 658 768  | -0.044 135 722 431                    |
| H                                                                 | -0.022 828 602 680                    | -0.170 034 348 557 | -0.120 862 211 086                    |
| H                                                                 | -9.127 782 500 000 × 10 <sup>-5</sup> | -0.001 229 498 021 | 0.018 690 559 261                     |
| H                                                                 | -0.217 863 741 389                    | -0.347 276 330 049 | 0.199 643 891 191                     |
| H                                                                 | 0.024 191 043 344                     | 0.010 132 986 904  | 0.108 418 097 023                     |
| H                                                                 | -0.003 354 948 395                    | 0.005 774 149 526  | -0.016 796 186 579                    |
| H                                                                 | 0.047 312 181 337                     | -0.051 053 475 884 | -0.057 118 146 314                    |
| H                                                                 | 0.154 697 422 333                     | -0.506 089 969 600 | -0.222 810 368 026                    |
| H                                                                 | 0.004 325 716 651                     | 0.016 965 798 116  | -0.017 412 749 988                    |
| H                                                                 | -0.384 034 678 546                    | -0.362 851 554 140 | 0.155 936 061 856                     |

Wavenumber/cm<sup>-1</sup>: 281.9514

| $\frac{\partial \mu_{x,y,z}}{\partial Q_r} / (e u^{-0.5})$        |                    |                    |                                       |
|-------------------------------------------------------------------|--------------------|--------------------|---------------------------------------|
|                                                                   | -0.002 296 377 072 | 0.001 561 948 429  | 0.002 154 292 491                     |
| <i>l</i> -matrix coefficients/(u <sup>1/2</sup> Å <sup>-1</sup> ) |                    |                    |                                       |
| O                                                                 | 0.000 739 926 283  | 0.000 273 154 357  | -9.681 880 500 000 × 10 <sup>-5</sup> |
| C                                                                 | -0.003 160 573 095 | -0.014 327 963 225 | -0.013 162 895 493                    |
| C                                                                 | 0.003 037 670 385  | -0.000 287 276 847 | -0.037 471 906 873                    |
| C                                                                 | 0.079 803 296 327  | 0.138 547 940 385  | -0.130 540 950 028                    |
| C                                                                 | -0.063 651 706 596 | 0.065 922 030 033  | 0.067 443 067 812                     |
| C                                                                 | -0.002 297 773 081 | -0.001 136 162 137 | 0.000 349 551 510                     |
| C                                                                 | 0.016 220 444 339  | -0.132 136 507 301 | -0.110 205 366 638                    |
| H                                                                 | 0.001 246 446 728  | -0.007 212 834 764 | 0.014 723 465 787                     |
| H                                                                 | 0.008 858 276 437  | 0.050 006 055 032  | 0.034 869 535 435                     |
| H                                                                 | -0.003 762 471 610 | -0.005 345 699 436 | 0.117 137 972 364                     |
| H                                                                 | -0.302 713 030 348 | -0.485 909 035 735 | 0.279 494 642 210                     |
| H                                                                 | 0.036 716 987 504  | 0.016 929 199 432  | 0.176 650 252 652                     |
| H                                                                 | 0.001 699 087 967  | -0.000 325 745 138 | 0.020 238 563 800                     |
| H                                                                 | 0.209 820 983 625  | -0.222 630 300 154 | -0.255 487 329 584                    |
| H                                                                 | -0.126 678 682 748 | 0.425 926 671 321  | 0.180 543 768 149                     |
| H                                                                 | 0.002 160 234 920  | -0.026 855 052 363 | 0.238 928 714 439                     |
| H                                                                 | 0.066 312 699 637  | 0.059 008 230 899  | -0.034 890 428 989                    |

Wavenumber/cm<sup>-1</sup>: 413.0915

| $\frac{\partial \mu_{x,y,z}}{\partial Q_r} / (e u^{-0.5})$        | 0.002 588 075 833  | -0.013 976 047 141                    | -0.001 749 051 690 |
|-------------------------------------------------------------------|--------------------|---------------------------------------|--------------------|
| <i>l</i> -matrix coefficients/(u <sup>1/2</sup> Å <sup>-1</sup> ) |                    |                                       |                    |
| O                                                                 | 0.000 369 355 912  | $4.470\,163\,400\,000 \times 10^{-5}$ | 0.000 113 712 525  |
| C                                                                 | -0.002 836 237 614 | -0.012 281 946 026                    | -0.012 936 203 024 |
| C                                                                 | 0.001 184 794 374  | 0.002 794 870 912                     | -0.030 978 939 923 |
| C                                                                 | -0.039 991 259 518 | -0.067 983 863 654                    | 0.063 634 016 963  |
| C                                                                 | 0.006 089 878 150  | -0.007 093 525 479                    | 0.002 403 928 116  |
| C                                                                 | -0.000 177 929 484 | 0.000 904 846 539                     | 0.000 298 359 753  |
| C                                                                 | 0.122 593 794 356  | 0.061 013 549 125                     | -0.247 891 070 608 |
| H                                                                 | -0.000 198 180 889 | -0.007 207 999 349                    | 0.016 363 167 734  |
| H                                                                 | 0.007 185 830 778  | 0.046 778 086 643                     | 0.031 990 294 209  |
| H                                                                 | 0.000 279 757 124  | -0.006 822 342 185                    | 0.094 848 931 296  |
| H                                                                 | 0.153 118 929 434  | 0.240 958 411 994                     | -0.139 585 481 717 |
| H                                                                 | -0.019 038 241 319 | -0.005 515 744 471                    | -0.079 212 591 164 |
| H                                                                 | -0.005 115 825 197 | 0.008 267 965 265                     | -0.023 613 099 997 |
| H                                                                 | -0.013 908 833 617 | 0.013 702 683 589                     | 0.016 320 052 634  |
| H                                                                 | -0.050 103 000 831 | 0.207 557 685 468                     | 0.069 541 124 644  |
| H                                                                 | 0.009 661 053 781  | -0.042 000 042 300                    | 0.652 261 062 788  |
| H                                                                 | -0.383 202 663 221 | -0.377 722 983 887                    | 0.138 951 511 779  |

Wavenumber/cm<sup>-1</sup>: 461.4561

| $\frac{\partial \mu_{x,y,z}}{\partial Q_r} / (e u^{-0.5})$        | -0.028 446 051 972 | 0.058 724 540 599  | -0.004 626 781 448 |
|-------------------------------------------------------------------|--------------------|--------------------|--------------------|
| <i>l</i> -matrix coefficients/(u <sup>1/2</sup> Å <sup>-1</sup> ) |                    |                    |                    |
| O                                                                 | 0.000 361 445 572  | -0.000 275 878 086 | 0.000 149 654 713  |
| C                                                                 | 0.001 312 210 036  | 0.022 572 642 118  | -0.007 455 848 291 |
| C                                                                 | 0.000 381 174 941  | 0.002 359 916 463  | -0.041 718 038 722 |
| C                                                                 | -0.066 405 111 355 | -0.069 563 641 232 | -0.120 157 819 528 |
| C                                                                 | -0.074 217 172 893 | 0.096 938 380 746  | -0.126 190 386 355 |
| C                                                                 | -0.001 100 664 946 | 0.002 138 732 236  | -0.001 963 536 292 |
| C                                                                 | -0.023 059 026 279 | 0.022 079 395 668  | 0.003 579 587 031  |
| H                                                                 | 0.008 181 421 181  | -0.021 246 386 340 | 0.065 612 893 390  |
| H                                                                 | -0.007 757 269 102 | -0.055 182 255 331 | -0.040 773 215 307 |
| H                                                                 | -0.003 596 881 326 | -0.007 034 895 265 | 0.139 147 937 848  |
| H                                                                 | 0.130 746 960 585  | 0.214 334 852 632  | -0.134 245 488 027 |
| H                                                                 | 0.098 611 230 540  | 0.019 338 932 574  | 0.549 571 926 306  |
| H                                                                 | 0.132 632 625 336  | -0.206 362 177 316 | 0.611 635 753 537  |
| H                                                                 | 0.122 740 911 805  | -0.129 687 485 615 | -0.167 292 231 243 |
| H                                                                 | 0.033 514 546 509  | -0.119 506 827 650 | -0.050 514 731 066 |
| H                                                                 | 0.000 783 016 763  | -0.003 690 959 513 | 0.057 690 042 837  |
| H                                                                 | 0.045 682 249 059  | 0.045 971 947 563  | -0.016 870 828 380 |

Wavenumber/cm<sup>-1</sup>: 489.0843

| $\frac{\partial \mu_{x,y,z}}{\partial Q_r} / (e \text{ u}^{-0.5})$ | 0.001 576 886 768  | -0.009 045 448 710 | -0.002 407 396 018 |
|--------------------------------------------------------------------|--------------------|--------------------|--------------------|
| <i>l</i> -matrix coefficients/(u <sup>1/2</sup> Å <sup>-1</sup> )  |                    |                    |                    |
| O                                                                  | 0.001 164 571 625  | 0.000 787 315 109  | 0.000 126 497 543  |
| C                                                                  | 0.004 323 392 253  | -0.021 292 736 789 | 0.032 273 454 199  |
| C                                                                  | -0.001 799 414 895 | -0.004 116 489 114 | 0.061 213 986 139  |
| C                                                                  | 0.040 119 100 233  | 0.025 109 236 828  | 0.129 211 575 640  |
| C                                                                  | -0.051 406 338 733 | 0.068 340 319 682  | -0.136 782 842 107 |
| C                                                                  | -0.001 910 708 628 | -0.000 248 280 101 | -0.001 106 515 684 |
| C                                                                  | 0.076 322 619 269  | -0.012 721 459 033 | 0.034 239 597 515  |
| H                                                                  | -0.018 012 354 956 | 0.046 467 492 639  | -0.138 663 916 923 |
| H                                                                  | 0.004 248 893 928  | 0.027 186 118 739  | 0.021 467 633 248  |
| H                                                                  | 0.005 461 123 934  | 0.011 228 461 072  | -0.203 550 965 032 |
| H                                                                  | -0.043 599 952 198 | -0.064 746 786 454 | 0.049 888 284 107  |
| H                                                                  | -0.089 198 049 745 | -0.020 775 110 931 | -0.498 917 878 336 |
| H                                                                  | 0.119 236 713 232  | -0.189 601 457 829 | 0.554 400 960 465  |
| H                                                                  | 0.052 701 116 947  | -0.047 628 264 907 | -0.075 729 593 973 |
| H                                                                  | -0.061 378 105 598 | 0.224 161 191 336  | 0.096 989 738 961  |
| H                                                                  | 0.001 854 747 655  | 0.021 982 267 477  | -0.301 944 765 428 |
| H                                                                  | -0.202 571 820 199 | -0.201 513 314 674 | 0.084 600 667 540  |

Wavenumber/cm<sup>-1</sup>: 539.998

| $\frac{\partial \mu_{x,y,z}}{\partial Q_r} / (e \text{ u}^{-0.5})$ | 0.007 013 586 525  | -0.039 054 396 451 | 0.004 108 271 171  |
|--------------------------------------------------------------------|--------------------|--------------------|--------------------|
| <i>l</i> -matrix coefficients/(u <sup>1/2</sup> Å <sup>-1</sup> )  |                    |                    |                    |
| O                                                                  | -0.000 505 484 104 | -0.000 272 264 680 | -0.000 256 100 160 |
| C                                                                  | 0.009 434 670 606  | -0.038 744 667 069 | 0.063 758 684 334  |
| C                                                                  | 0.001 689 803 223  | -0.002 759 328 783 | 0.042 494 798 463  |
| C                                                                  | 0.036 704 814 778  | 0.033 848 935 108  | 0.072 298 844 569  |
| C                                                                  | -0.015 596 964 487 | 0.021 572 071 319  | -0.057 418 894 721 |
| C                                                                  | -0.000 601 102 281 | -0.001 181 746 162 | 0.000 556 338 429  |
| C                                                                  | -0.115 117 219 171 | 0.029 942 675 538  | -0.080 023 791 507 |
| H                                                                  | -0.038 893 269 140 | 0.086 843 913 129  | -0.265 993 629 127 |
| H                                                                  | 0.005 505 613 554  | 0.047 759 852 066  | 0.041 510 495 064  |
| H                                                                  | 0.000 915 068 560  | 0.008 477 973 760  | -0.145 390 482 032 |
| H                                                                  | -0.063 162 290 958 | -0.104 438 539 368 | 0.069 049 083 628  |
| H                                                                  | -0.057 275 556 767 | -0.010 533 348 572 | -0.320 171 458 675 |
| H                                                                  | 0.046 358 015 122  | -0.073 234 360 227 | 0.211 218 725 169  |
| H                                                                  | 0.004 331 859 445  | -0.000 453 497 921 | -0.008 662 848 785 |
| H                                                                  | 0.098 470 201 749  | -0.360 574 648 977 | -0.161 149 125 210 |
| H                                                                  | -0.005 077 589 771 | -0.037 840 653 220 | 0.562 486 503 285  |
| H                                                                  | 0.299 033 977 167  | 0.297 754 563 383  | -0.125 707 141 219 |

Wavenumber/cm<sup>-1</sup>: 585.879

| $\frac{\partial \mu_{x,y,z}}{\partial Q_r} / (e u^{-0.5})$        | 0.022 113 372 411  | -0.021 338 178 684                   | 0.000 996 922 408  |
|-------------------------------------------------------------------|--------------------|--------------------------------------|--------------------|
| <i>l</i> -matrix coefficients/(u <sup>1/2</sup> Å <sup>-1</sup> ) |                    |                                      |                    |
| O                                                                 | -0.001 044 632 685 | -0.000 579 163 831                   | -0.000 202 264 557 |
| C                                                                 | 0.023 362 542 394  | -0.120 979 354 083                   | 0.177 474 313 462  |
| C                                                                 | -0.000 509 999 613 | -0.003 107 200 127                   | 0.072 033 495 744  |
| C                                                                 | -0.028 854 625 901 | -0.019 372 716 934                   | -0.085 009 529 487 |
| C                                                                 | 0.010 029 531 629  | -0.012 393 281 236                   | 0.029 512 957 924  |
| C                                                                 | 0.000 976 032 380  | 1.012 035 300 000 × 10 <sup>-5</sup> | 0.003 156 902 884  |
| C                                                                 | 0.028 027 967 776  | -0.007 573 487 253                   | 0.003 185 679 275  |
| H                                                                 | -0.108 626 974 756 | 0.249 468 693 050                    | -0.766 002 678 936 |
| H                                                                 | 0.024 804 250 674  | 0.165 895 294 787                    | 0.140 335 802 651  |
| H                                                                 | 0.006 065 546 940  | 0.013 947 172 670                    | -0.246 052 685 091 |
| H                                                                 | 0.034 744 933 068  | 0.057 675 542 474                    | -0.042 451 654 910 |
| H                                                                 | 0.062 061 180 616  | 0.011 237 270 970                    | 0.338 684 730 274  |
| H                                                                 | -0.024 827 430 112 | 0.039 323 257 274                    | -0.112 971 895 765 |
| H                                                                 | -0.006 576 331 723 | 0.004 751 321 878                    | 0.010 380 281 110  |
| H                                                                 | -0.024 200 078 457 | 0.091 282 207 692                    | 0.040 657 851 398  |
| H                                                                 | -0.001 511 775 025 | 0.004 519 069 485                    | -0.080 855 006 440 |
| H                                                                 | -0.071 795 379 338 | -0.071 683 622 871                   | 0.027 463 362 679  |

Wavenumber/cm<sup>-1</sup>: 728.19

| $\frac{\partial \mu_{x,y,z}}{\partial Q_r} / (e u^{-0.5})$        | 0.002 710 479 053                    | -0.005 520 983 474 | 0.001 475 865 729                    |
|-------------------------------------------------------------------|--------------------------------------|--------------------|--------------------------------------|
| <i>l</i> -matrix coefficients/(u <sup>1/2</sup> Å <sup>-1</sup> ) |                                      |                    |                                      |
| O                                                                 | -0.000 476 805 568                   | 0.000 268 026 093  | 9.733 569 800 000 × 10 <sup>-5</sup> |
| C                                                                 | -0.012 201 950 911                   | 0.032 876 819 637  | -0.087 342 023 577                   |
| C                                                                 | -0.004 999 470 362                   | -0.014 353 920 045 | 0.245 487 089 527                    |
| C                                                                 | -0.006 864 576 817                   | 0.002 174 215 676  | -0.056 504 623 571                   |
| C                                                                 | -0.001 115 333 813                   | 0.001 389 892 500  | 0.007 600 425 841                    |
| C                                                                 | 8.817 876 400 000 × 10 <sup>-5</sup> | -0.000 790 789 853 | -0.000 942 331 053                   |
| C                                                                 | 0.007 404 372 629                    | 0.000 391 206 638  | -0.036 186 719 156                   |
| H                                                                 | 0.048 007 876 048                    | -0.107 282 011 927 | 0.324 366 684 148                    |
| H                                                                 | -0.006 041 573 913                   | -0.007 227 626 859 | -0.014 211 409 645                   |
| H                                                                 | 0.017 783 439 569                    | 0.047 929 133 561  | -0.864 599 717 638                   |
| H                                                                 | -0.012 391 104 778                   | -0.013 504 390 836 | 0.004 658 557 283                    |
| H                                                                 | 0.037 933 191 465                    | 0.007 970 649 208  | 0.196 976 562 807                    |
| H                                                                 | -0.005 300 965 384                   | 0.007 086 496 452  | -0.017 087 482 707                   |
| H                                                                 | 0.006 300 497 757                    | -0.009 154 207 986 | -0.011 069 941 064                   |
| H                                                                 | -0.004 754 570 125                   | 0.029 522 285 855  | 0.010 243 717 298                    |
| H                                                                 | 0.000 761 877 805                    | -0.007 504 027 568 | 0.114 875 232 886                    |
| H                                                                 | -0.019 337 689 293                   | -0.023 768 731 227 | 0.006 531 323 087                    |

Wavenumber/cm<sup>-1</sup>: 813.1063

| $\frac{\partial \mu_{x,y,z}}{\partial Q_r} / (e u^{-0.5})$        | -0.003 657 280 463 | -0.005 611 697 746 | 0.000 520 740 157  |
|-------------------------------------------------------------------|--------------------|--------------------|--------------------|
| <i>l</i> -matrix coefficients/(u <sup>1/2</sup> Å <sup>-1</sup> ) |                    |                    |                    |
| O                                                                 | -0.563 380 526 785 | -0.202 503 396 383 | 0.019 885 727 025  |
| C                                                                 | -0.041 479 141 175 | -0.014 826 129 334 | 0.001 855 642 350  |
| C                                                                 | -0.028 518 584 876 | -0.003 105 950 265 | -0.002 412 248 416 |
| C                                                                 | -0.018 901 495 337 | -0.010 623 766 537 | 0.003 864 757 346  |
| C                                                                 | -0.043 015 066 155 | -0.012 695 910 983 | -0.002 004 443 233 |
| C                                                                 | 0.747 907 761 879  | 0.267 388 532 724  | -0.025 936 755 020 |
| C                                                                 | 0.004 167 028 918  | -0.000 387 163 156 | 0.000 504 817 507  |
| H                                                                 | 0.006 314 001 597  | -0.002 706 662 203 | 0.000 437 025 323  |
| H                                                                 | 0.043 464 518 587  | -0.005 058 826 168 | -0.001 356 069 925 |
| H                                                                 | 0.010 561 839 219  | 0.004 046 974 104  | 0.000 361 115 060  |
| H                                                                 | -0.005 239 816 004 | -0.005 481 625 037 | 0.002 976 796 418  |
| H                                                                 | 0.008 560 466 519  | 0.002 730 398 308  | -0.002 335 106 163 |
| H                                                                 | 0.009 064 936 981  | 0.003 831 425 418  | -0.000 482 589 617 |
| H                                                                 | 0.032 251 889 645  | 0.031 271 082 656  | 0.003 269 928 242  |
| H                                                                 | -0.000 263 165 772 | -0.000 707 972 528 | -0.000 209 442 240 |
| H                                                                 | -0.000 591 245 939 | -0.000 529 447 949 | 0.000 339 514 647  |
| H                                                                 | -0.000 353 108 800 | 0.000 110 830 438  | 0.001 062 709 916  |

Wavenumber/cm<sup>-1</sup>: 844.0097

| $\frac{\partial \mu_{x,y,z}}{\partial Q_r} / (e u^{-0.5})$        | -0.014 860 908 986 | -0.010 563 839 045 | -6.653 828 243 620 × 10 <sup>-5</sup> |
|-------------------------------------------------------------------|--------------------|--------------------|---------------------------------------|
| <i>l</i> -matrix coefficients/(u <sup>1/2</sup> Å <sup>-1</sup> ) |                    |                    |                                       |
| O                                                                 | 0.006 615 222 396  | 0.000 315 434 124  | -0.000 859 105 303                    |
| C                                                                 | 0.018 421 603 471  | 0.040 157 739 853  | -0.003 427 088 479                    |
| C                                                                 | -0.031 055 215 235 | -0.017 421 047 790 | -0.043 012 264 635                    |
| C                                                                 | -0.156 151 751 226 | -0.167 146 605 212 | -0.102 055 570 884                    |
| C                                                                 | 0.026 674 728 190  | -0.039 334 278 740 | -0.002 615 690 550                    |
| C                                                                 | -0.009 902 539 555 | 0.009 753 965 501  | 0.003 387 468 374                     |
| C                                                                 | 0.020 674 069 725  | -0.021 002 998 422 | -0.071 683 772 862                    |
| H                                                                 | -0.029 400 420 744 | -0.084 295 759 522 | -0.028 207 069 270                    |
| H                                                                 | 0.015 342 472 367  | -0.042 970 054 018 | 0.070 262 211 773                     |
| H                                                                 | 0.005 716 224 717  | 0.019 688 593 874  | -0.013 311 838 711                    |
| H                                                                 | 0.204 666 546 960  | 0.139 772 240 139  | 0.537 516 728 782                     |
| H                                                                 | 0.338 816 440 663  | 0.492 090 613 212  | -0.110 463 853 916                    |
| H                                                                 | -0.038 782 425 716 | 0.043 057 641 515  | 0.023 994 305 575                     |
| H                                                                 | -0.017 648 098 944 | 0.023 336 482 664  | -0.052 405 315 692                    |
| H                                                                 | -0.178 575 468 563 | -0.111 465 535 949 | 0.113 258 024 577                     |
| H                                                                 | 0.190 701 852 277  | 0.027 945 371 980  | -0.013 441 804 683                    |
| H                                                                 | -0.063 812 504 565 | 0.164 696 746 407  | 0.233 610 037 971                     |



Wavenumber/cm<sup>-1</sup>: 892.5475

| $\frac{\partial \mu_{x,y,z}}{\partial Q_r} / (e u^{-0.5})$        | 0.002 531 640 009                    | -0.041 779 459 059 | 0.003 827 310 471                    |
|-------------------------------------------------------------------|--------------------------------------|--------------------|--------------------------------------|
| <i>l</i> -matrix coefficients/(u <sup>1/2</sup> Å <sup>-1</sup> ) |                                      |                    |                                      |
| O                                                                 | 0.000 956 896 181                    | 0.002 418 269 107  | 6.090 587 900 000 × 10 <sup>-5</sup> |
| C                                                                 | 0.015 370 654 619                    | 0.008 904 711 110  | -0.005 765 086 889                   |
| C                                                                 | -0.073 204 687 655                   | -0.037 076 836 899 | 0.061 947 907 979                    |
| C                                                                 | -0.051 313 445 118                   | -0.067 707 960 396 | -0.052 105 817 827                   |
| C                                                                 | 0.016 945 103 830                    | -0.013 843 583 480 | -0.004 522 270 043                   |
| C                                                                 | 7.569 714 000 000 × 10 <sup>-6</sup> | -0.008 633 950 769 | 0.001 168 407 718                    |
| C                                                                 | -0.062 421 984 678                   | -0.053 013 725 534 | 0.126 683 743 308                    |
| H                                                                 | 0.002 932 894 375                    | 0.016 527 510 014  | 0.002 565 827 294                    |
| H                                                                 | -0.011 707 278 392                   | 0.009 942 188 727  | -0.006 884 043 192                   |
| H                                                                 | 0.071 415 386 904                    | 0.011 331 990 145  | 0.024 536 852 853                    |
| H                                                                 | 0.053 285 232 516                    | 0.080 926 358 638  | 0.226 778 114 564                    |
| H                                                                 | 0.152 982 594 366                    | 0.179 162 991 831  | -0.046 957 139 884                   |
| H                                                                 | -0.032 864 283 325                   | 0.026 604 037 055  | 0.015 546 152 455                    |
| H                                                                 | -0.013 201 280 130                   | 0.016 222 422 098  | -0.036 751 089 862                   |
| H                                                                 | 0.317 834 098 718                    | 0.296 535 465 545  | -0.467 321 409 350                   |
| H                                                                 | -0.266 965 429 980                   | 0.318 763 212 070  | 0.046 240 963 478                    |
| H                                                                 | 0.256 210 050 235                    | -0.374 079 993 377 | -0.197 803 122 569                   |

Wavenumber/cm<sup>-1</sup>: 938.6095

| $\frac{\partial \mu_{x,y,z}}{\partial Q_r} / (e u^{-0.5})$        | -0.011 459 261 319 | 0.019 140 200 504  | -0.003 563 054 390 |
|-------------------------------------------------------------------|--------------------|--------------------|--------------------|
| <i>l</i> -matrix coefficients/(u <sup>1/2</sup> Å <sup>-1</sup> ) |                    |                    |                    |
| O                                                                 | -0.001 397 579 644 | 0.002 256 925 970  | -0.001 365 232 090 |
| C                                                                 | -0.008 617 025 870 | 0.002 167 824 342  | 0.010 919 599 219  |
| C                                                                 | 0.002 444 516 129  | -0.110 562 024 858 | -0.025 949 916 773 |
| C                                                                 | 0.039 957 430 705  | 0.071 555 242 576  | 0.033 421 791 886  |
| C                                                                 | -0.014 638 875 435 | 0.007 601 191 526  | -0.007 752 388 689 |
| C                                                                 | 0.002 692 790 131  | -0.010 348 407 164 | 0.005 233 341 346  |
| C                                                                 | -0.025 559 978 385 | -0.155 470 146 463 | -0.049 031 212 519 |
| H                                                                 | -0.000 688 501 669 | 0.038 143 573 117  | 0.012 053 349 132  |
| H                                                                 | 0.024 111 339 035  | 0.029 196 615 500  | -0.042 895 450 789 |
| H                                                                 | -0.015 621 808 707 | 0.062 315 804 877  | -0.003 203 869 128 |
| H                                                                 | -0.057 244 968 814 | -0.025 006 951 668 | -0.136 389 964 503 |
| H                                                                 | -0.076 376 288 399 | -0.134 572 225 786 | 0.031 207 809 860  |
| H                                                                 | 0.016 300 824 784  | -0.016 342 647 880 | -0.013 400 520 872 |
| H                                                                 | 0.023 731 634 892  | -0.006 789 014 421 | 0.029 036 845 210  |
| H                                                                 | -0.256 119 534 626 | 0.032 167 305 969  | -0.321 612 984 594 |
| H                                                                 | 0.271 080 440 290  | 0.590 924 711 608  | 0.034 076 604 417  |
| H                                                                 | 0.089 240 249 060  | 0.094 301 913 834  | 0.531 030 897 845  |

Wavenumber/cm<sup>-1</sup>: 953.6317

| $\frac{\partial \mu_{x,y,z}}{\partial Q_r} / (e u^{-0.5})$        | -0.035 349 307 904                    | 0.030 182 932 005  | -0.001 274 270 719                   |
|-------------------------------------------------------------------|---------------------------------------|--------------------|--------------------------------------|
| <i>l</i> -matrix coefficients/(u <sup>1/2</sup> Å <sup>-1</sup> ) |                                       |                    |                                      |
| O                                                                 | -0.000 321 511 115                    | -0.002 613 009 634 | 1.820 979 900 000 × 10 <sup>-5</sup> |
| C                                                                 | -0.028 360 103 465                    | -0.128 368 570 359 | 0.048 437 797 135                    |
| C                                                                 | 0.076 741 541 357                     | -0.047 470 326 816 | 0.000 456 958 565                    |
| C                                                                 | -0.049 520 492 856                    | 0.019 799 011 163  | -0.032 171 502 582                   |
| C                                                                 | -0.172 138 346 380                    | 0.138 943 963 831  | -0.062 732 065 589                   |
| C                                                                 | -0.017 891 705 988                    | 0.012 840 666 684  | -0.003 435 490 198                   |
| C                                                                 | -0.015 465 925 572                    | 0.015 956 088 698  | 0.018 598 588 210                    |
| H                                                                 | 0.048 808 582 172                     | 0.297 742 337 762  | 0.108 956 040 830                    |
| H                                                                 | -0.012 838 657 771                    | 0.179 073 672 467  | -0.277 575 855 492                   |
| H                                                                 | -0.073 809 541 728                    | 0.060 252 576 958  | 0.000 557 435 929                    |
| H                                                                 | 0.069 772 567 053                     | 0.026 193 420 678  | 0.105 615 594 774                    |
| H                                                                 | 0.103 745 187 423                     | 0.064 588 657 810  | -0.030 139 560 580                   |
| H                                                                 | 0.366 413 800 366                     | -0.364 091 100 368 | -0.234 747 474 893                   |
| H                                                                 | 0.232 578 052 130                     | -0.261 798 085 819 | 0.461 763 619 457                    |
| H                                                                 | -0.006 720 296 067                    | 0.004 295 046 199  | 0.004 491 298 515                    |
| H                                                                 | -5.107 195 900 000 × 10 <sup>-5</sup> | -0.032 725 340 201 | 0.001 913 865 675                    |
| H                                                                 | -0.013 317 331 387                    | -0.003 511 808 959 | -0.034 428 669 869                   |

Wavenumber/cm<sup>-1</sup>: 1000.5647

| $\frac{\partial \mu_{x,y,z}}{\partial Q_r} / (e u^{-0.5})$        | 0.003 063 340 418  | -0.004 229 427 724 | 0.002 393 730 412  |
|-------------------------------------------------------------------|--------------------|--------------------|--------------------|
| <i>l</i> -matrix coefficients/(u <sup>1/2</sup> Å <sup>-1</sup> ) |                    |                    |                    |
| O                                                                 | -0.004 514 804 695 | 0.000 549 002 303  | 0.000 913 454 246  |
| C                                                                 | -0.032 434 461 092 | -0.219 505 822 890 | 0.068 397 933 535  |
| C                                                                 | 0.061 381 450 845  | -0.015 721 925 330 | 0.001 265 568 439  |
| C                                                                 | -0.036 280 734 727 | -0.011 287 265 207 | -0.003 980 407 964 |
| C                                                                 | 0.099 927 950 568  | -0.089 624 595 509 | 0.024 426 589 513  |
| C                                                                 | 0.013 960 905 086  | -0.031 582 106 285 | 0.020 714 681 560  |
| C                                                                 | 0.024 979 707 346  | -0.001 753 211 029 | 0.005 829 544 403  |
| H                                                                 | 0.052 806 537 327  | 0.538 605 515 692  | 0.195 917 242 742  |
| H                                                                 | -0.034 668 402 765 | 0.313 315 449 204  | -0.483 618 522 294 |
| H                                                                 | -0.033 882 299 043 | 0.011 870 542 591  | 0.001 715 159 210  |
| H                                                                 | 0.020 266 190 947  | -0.004 908 567 176 | 0.028 264 507 636  |
| H                                                                 | 0.039 049 368 417  | 0.014 115 353 041  | -0.008 614 283 139 |
| H                                                                 | -0.215 391 939 613 | 0.235 273 637 487  | 0.142 028 477 145  |
| H                                                                 | -0.131 504 440 440 | 0.158 901 698 849  | -0.275 497 855 593 |
| H                                                                 | -0.056 124 380 341 | -0.023 577 814 302 | 0.011 895 760 664  |
| H                                                                 | -0.024 810 317 501 | -0.020 756 124 284 | 0.000 696 051 791  |
| H                                                                 | -0.051 808 766 557 | 0.050 393 745 459  | -0.019 112 980 507 |

Wavenumber/cm<sup>-1</sup>: 1007.187

| $\frac{\partial \mu_{x,y,z}}{\partial Q_r} / (e u^{-0.5})$        | 0.029 760 793 202  | 0.010 598 206 934  | -0.001 411 676 697 |
|-------------------------------------------------------------------|--------------------|--------------------|--------------------|
| <i>l</i> -matrix coefficients/(u <sup>1/2</sup> Å <sup>-1</sup> ) |                    |                    |                    |
| O                                                                 | -0.009 820 472 708 | 0.000 587 853 731  | -0.001 099 425 750 |
| C                                                                 | 0.000 323 173 038  | -0.007 706 702 791 | -0.005 561 285 529 |
| C                                                                 | 0.076 647 411 418  | -0.018 285 421 333 | 0.020 184 231 586  |
| C                                                                 | 0.012 862 593 626  | -0.016 031 678 323 | -0.012 358 462 691 |
| C                                                                 | 0.005 736 945 846  | 0.010 345 592 926  | 0.008 807 007 040  |
| C                                                                 | 0.008 625 141 635  | -0.016 430 840 787 | 0.006 168 546 709  |
| C                                                                 | -0.411 074 953 732 | 0.122 432 918 289  | -0.136 932 697 872 |
| H                                                                 | 0.005 958 403 820  | 0.049 207 747 825  | 0.011 049 358 558  |
| H                                                                 | -0.020 555 743 470 | 0.024 353 301 472  | -0.032 869 584 491 |
| H                                                                 | -0.057 110 917 051 | 0.004 191 144 321  | 0.006 833 649 059  |
| H                                                                 | -0.024 995 540 491 | 0.010 585 535 299  | -0.004 232 595 034 |
| H                                                                 | -0.025 424 277 186 | -0.001 525 063 759 | -0.000 183 311 519 |
| H                                                                 | -0.011 995 046 414 | 0.020 154 371 268  | 0.010 308 184 144  |
| H                                                                 | -0.026 037 407 273 | 0.008 017 498 757  | -0.023 292 757 434 |
| H                                                                 | 0.426 384 353 188  | 0.058 036 246 256  | 0.256 790 218 317  |
| H                                                                 | 0.500 231 933 637  | -0.130 615 338 307 | -0.044 614 663 584 |
| H                                                                 | 0.332 012 875 256  | -0.301 312 135 886 | 0.237 768 583 626  |

Wavenumber/cm<sup>-1</sup>: 1084.4813

| $\frac{\partial \mu_{x,y,z}}{\partial Q_r} / (e u^{-0.5})$        | 0.017 146 864 370  | 0.004 822 179 625  | 0.001 167 622 554  |
|-------------------------------------------------------------------|--------------------|--------------------|--------------------|
| <i>l</i> -matrix coefficients/(u <sup>1/2</sup> Å <sup>-1</sup> ) |                    |                    |                    |
| O                                                                 | 0.011 876 153 341  | -0.007 646 405 097 | 0.003 173 835 354  |
| C                                                                 | -0.184 385 889 280 | 0.036 787 758 766  | -0.047 707 670 976 |
| C                                                                 | 0.484 734 383 246  | -0.095 375 333 849 | 0.018 064 845 956  |
| C                                                                 | -0.207 686 715 572 | 0.124 419 391 170  | -0.019 301 672 554 |
| C                                                                 | 0.016 505 219 819  | -0.056 208 341 696 | -0.000 598 128 421 |
| C                                                                 | -0.003 106 074 445 | 0.029 755 467 533  | -0.013 246 491 790 |
| C                                                                 | -0.096 069 218 679 | 0.007 907 445 621  | 0.130 355 972 052  |
| H                                                                 | 0.177 512 331 847  | -0.075 706 554 255 | -0.071 240 389 809 |
| H                                                                 | 0.107 668 042 727  | -0.083 976 339 464 | 0.080 920 024 129  |
| H                                                                 | -0.628 182 010 995 | 0.131 425 863 004  | -0.002 239 549 246 |
| H                                                                 | 0.153 448 540 116  | -0.092 993 329 342 | -0.004 326 356 080 |
| H                                                                 | 0.207 265 362 707  | -0.155 319 056 694 | -0.046 563 352 582 |
| H                                                                 | -0.037 262 087 862 | 0.042 903 151 968  | 0.028 049 341 410  |
| H                                                                 | 0.024 360 973 426  | 0.057 056 312 658  | -0.047 188 620 702 |
| H                                                                 | -0.045 748 967 750 | 0.057 290 142 860  | -0.104 694 373 428 |
| H                                                                 | 0.038 369 400 332  | -0.008 383 238 388 | 0.030 596 808 106  |
| H                                                                 | -0.079 238 312 649 | -0.005 064 810 344 | -0.109 197 894 005 |

Wavenumber/cm<sup>-1</sup>: 1148.8459

| $\frac{\partial \mu_{x,y,z}}{\partial Q_r} / (e u^{-0.5})$        | -0.001 676 697 528 | 0.022 444 495 102  | -0.003 036 280 505 |
|-------------------------------------------------------------------|--------------------|--------------------|--------------------|
| <i>l</i> -matrix coefficients/(u <sup>1/2</sup> Å <sup>-1</sup> ) |                    |                    |                    |
| O                                                                 | -0.010 302 808 044 | -0.019 081 194 091 | 0.005 364 645 966  |
| C                                                                 | -0.020 081 111 442 | -0.091 134 884 554 | -0.093 520 088 942 |
| C                                                                 | 0.120 230 297 207  | 0.415 614 845 005  | -0.012 832 165 834 |
| C                                                                 | 0.037 863 783 356  | -0.146 108 335 660 | 0.092 845 425 519  |
| C                                                                 | 0.025 405 423 425  | 0.040 928 624 723  | 0.026 415 663 897  |
| C                                                                 | -0.010 179 328 562 | 0.056 444 102 765  | -0.023 388 223 751 |
| C                                                                 | -0.029 116 659 007 | -0.117 202 176 333 | 0.018 799 389 122  |
| H                                                                 | 0.134 430 150 386  | 0.064 266 016 509  | -0.017 385 559 885 |
| H                                                                 | -0.126 054 611 454 | -0.045 394 629 211 | 0.018 627 924 334  |
| H                                                                 | -0.228 843 394 235 | -0.701 489 951 842 | -0.055 371 612 409 |
| H                                                                 | 0.046 314 025 037  | -0.098 237 748 281 | -0.034 554 723 418 |
| H                                                                 | -0.192 675 189 189 | 0.241 007 776 192  | 0.051 043 965 804  |
| H                                                                 | -0.002 239 580 314 | -0.056 601 206 716 | -0.011 872 864 466 |
| H                                                                 | -0.051 744 746 600 | -0.062 852 324 083 | 0.022 504 220 668  |
| H                                                                 | 0.068 192 434 817  | 0.021 351 065 119  | -0.053 922 970 599 |
| H                                                                 | 0.039 067 694 113  | 0.118 792 019 438  | 0.013 621 458 079  |
| H                                                                 | -0.073 867 849 410 | 0.047 895 286 343  | 0.017 216 495 198  |

Wavenumber/cm<sup>-1</sup>: 1160.1581

| $\frac{\partial \mu_{x,y,z}}{\partial Q_r} / (e u^{-0.5})$        | -0.003 412 212 051 | -0.007 815 761 885 | -0.004 712 199 027 |
|-------------------------------------------------------------------|--------------------|--------------------|--------------------|
| <i>l</i> -matrix coefficients/(u <sup>1/2</sup> Å <sup>-1</sup> ) |                    |                    |                    |
| O                                                                 | 0.045 567 243 564  | -0.010 557 841 788 | 0.005 353 623 969  |
| C                                                                 | -0.035 166 298 414 | -0.052 770 409 377 | 0.028 757 603 934  |
| C                                                                 | -0.054 707 974 237 | 0.138 556 015 249  | 0.047 543 382 939  |
| C                                                                 | -0.302 515 274 383 | 0.240 476 187 464  | 0.160 429 678 675  |
| C                                                                 | -0.021 592 042 808 | -0.194 936 645 844 | -0.083 870 345 121 |
| C                                                                 | -0.052 103 570 067 | 0.120 778 245 326  | -0.038 084 177 177 |
| C                                                                 | -0.002 655 189 869 | -0.047 657 408 545 | -0.134 332 878 332 |
| H                                                                 | 0.048 677 091 305  | -0.016 233 300 171 | 0.001 160 647 290  |
| H                                                                 | 0.050 005 355 940  | -0.013 034 631 628 | -0.006 161 203 041 |
| H                                                                 | 0.351 110 723 173  | -0.238 532 537 721 | 0.005 554 466 124  |
| H                                                                 | 0.324 167 747 403  | -0.269 597 755 229 | -0.091 245 380 160 |
| H                                                                 | 0.405 030 465 795  | -0.252 039 476 172 | -0.031 088 492 791 |
| H                                                                 | -0.069 104 393 458 | -0.009 156 989 133 | 0.008 336 216 404  |
| H                                                                 | 0.245 664 097 435  | 0.108 186 135 426  | 0.037 511 146 986  |
| H                                                                 | 0.104 360 057 138  | -0.030 956 060 194 | 0.076 429 035 292  |
| H                                                                 | -0.051 383 691 170 | 0.051 506 733 772  | -0.029 121 362 875 |
| H                                                                 | 0.028 012 141 910  | 0.006 177 358 521  | 0.074 805 153 618  |

Wavenumber/cm<sup>-1</sup>: 1172.9654

| $\frac{\partial \mu_{x,y,z}}{\partial Q_r} / (e \text{ u}^{-0.5})$ | -0.015 326 391 165 | 0.028 482 356 485  | 0.003 114 178 291  |
|--------------------------------------------------------------------|--------------------|--------------------|--------------------|
| <i>l</i> -matrix coefficients/(u <sup>1/2</sup> Å <sup>-1</sup> )  |                    |                    |                    |
| O                                                                  | -0.070 993 241 832 | -0.025 393 128 080 | 0.020 026 335 583  |
| C                                                                  | 0.084 505 127 800  | 0.014 773 301 369  | -0.047 244 699 415 |
| C                                                                  | -0.028 892 860 145 | 0.045 196 669 387  | 0.184 995 087 518  |
| C                                                                  | -0.062 128 924 982 | -0.103 009 138 125 | 0.053 569 454 315  |
| C                                                                  | 0.280 014 424 673  | 0.305 034 338 954  | -0.087 750 027 723 |
| C                                                                  | 0.003 613 667 909  | -0.048 823 948 372 | -0.092 770 349 145 |
| C                                                                  | 0.017 416 238 674  | -0.025 803 813 571 | -0.055 845 624 556 |
| H                                                                  | 0.091 163 699 121  | 0.034 273 331 820  | -0.012 469 879 339 |
| H                                                                  | -0.211 896 349 698 | -0.001 304 614 869 | 0.037 196 446 619  |
| H                                                                  | -0.052 822 102 184 | -0.012 664 791 144 | 0.054 983 735 017  |
| H                                                                  | -0.307 650 242 260 | 0.137 707 645 229  | -0.004 644 196 973 |
| H                                                                  | 0.368 497 401 627  | -0.214 909 867 003 | -0.048 787 655 751 |
| H                                                                  | -0.443 728 987 697 | -0.343 851 028 284 | -0.056 384 074 961 |
| H                                                                  | -0.135 919 131 296 | -0.173 061 123 915 | 0.022 569 826 075  |
| H                                                                  | 0.011 939 680 274  | -0.027 367 747 921 | 0.047 006 767 883  |
| H                                                                  | -0.041 554 886 310 | 0.022 573 872 958  | -0.007 181 619 314 |
| H                                                                  | -0.011 890 488 026 | 0.032 983 695 343  | 0.043 422 647 869  |

Wavenumber/cm<sup>-1</sup>: 1223.508

| $\frac{\partial \mu_{x,y,z}}{\partial Q_r} / (e \text{ u}^{-0.5})$ | 0.015 663 693 522  | 0.007 197 586 228  | 0.001 015 851 381  |
|--------------------------------------------------------------------|--------------------|--------------------|--------------------|
| <i>l</i> -matrix coefficients/(u <sup>1/2</sup> Å <sup>-1</sup> )  |                    |                    |                    |
| O                                                                  | -0.083 790 634 390 | -0.027 191 814 508 | -0.015 239 500 616 |
| C                                                                  | 0.503 538 535 179  | -0.079 035 151 369 | -0.093 943 035 717 |
| C                                                                  | -0.056 077 418 180 | 0.140 062 050 554  | -0.001 331 223 128 |
| C                                                                  | -0.056 923 819 585 | 0.072 020 141 243  | -0.081 534 876 276 |
| C                                                                  | -0.006 594 207 241 | -0.112 840 565 665 | -0.014 152 923 636 |
| C                                                                  | -0.041 266 014 648 | 0.088 757 845 928  | 0.093 040 499 965  |
| C                                                                  | -0.011 235 906 735 | -0.099 670 697 849 | 0.088 158 952 181  |
| H                                                                  | -0.489 650 797 344 | 0.043 786 365 670  | 0.084 882 089 083  |
| H                                                                  | -0.473 888 731 946 | -0.013 701 169 801 | 0.070 551 573 400  |
| H                                                                  | -0.223 092 773 547 | 0.107 022 922 867  | -0.001 220 995 780 |
| H                                                                  | 0.123 263 417 103  | -0.055 449 807 219 | -0.000 634 865 468 |
| H                                                                  | 0.078 800 561 868  | -0.141 308 885 542 | -0.035 322 689 674 |
| H                                                                  | 0.121 831 531 933  | 0.104 261 766 951  | 0.015 181 617 202  |
| H                                                                  | -0.009 479 122 921 | -0.042 305 981 508 | -0.002 399 696 641 |
| H                                                                  | 0.061 088 237 668  | 0.014 577 521 854  | -0.021 450 954 912 |
| H                                                                  | 0.086 028 659 312  | 0.027 312 723 813  | 0.025 431 687 942  |
| H                                                                  | -0.085 201 264 381 | 0.032 057 489 360  | -0.040 602 036 375 |

Wavenumber/cm<sup>-1</sup>: 1255.2132

| $\frac{\partial \mu_{x,y,z}}{\partial Q_r} / (e u^{-0.5})$        | 0.006 456 132 976  | -0.014 351 271 452 | -0.000 615 935 125 |
|-------------------------------------------------------------------|--------------------|--------------------|--------------------|
| <i>l</i> -matrix coefficients/(u <sup>1/2</sup> Å <sup>-1</sup> ) |                    |                    |                    |
| O                                                                 | 0.020 333 499 045  | 0.076 592 272 236  | 0.013 069 593 686  |
| C                                                                 | 0.069 952 669 138  | 0.078 772 664 804  | -0.126 413 845 768 |
| C                                                                 | -0.134 408 826 263 | -0.102 190 597 417 | 0.217 494 636 079  |
| C                                                                 | 0.211 564 724 924  | 0.052 768 413 364  | 0.017 601 815 103  |
| C                                                                 | -0.324 122 469 038 | -0.132 882 443 911 | -0.051 016 320 547 |
| C                                                                 | 0.074 813 887 654  | -0.198 752 485 709 | -0.107 254 399 342 |
| C                                                                 | 0.054 552 481 856  | 0.073 302 886 172  | -0.038 412 645 728 |
| H                                                                 | 0.275 074 880 452  | 0.078 728 247 119  | -0.052 740 201 634 |
| H                                                                 | -0.316 803 900 879 | -0.003 734 943 592 | 0.061 523 418 251  |
| H                                                                 | -0.168 482 929 661 | -0.156 919 284 953 | 0.056 089 240 281  |
| H                                                                 | -0.179 021 569 617 | 0.212 688 312 514  | 0.085 672 741 589  |
| H                                                                 | 0.113 474 330 596  | -0.062 884 543 832 | 0.004 735 822 599  |
| H                                                                 | 0.056 528 035 445  | 0.126 006 146 345  | 0.004 096 104 081  |
| H                                                                 | 0.362 884 571 122  | 0.365 808 324 581  | 0.012 251 537 454  |
| H                                                                 | -0.074 029 678 392 | -0.024 048 234 435 | 0.034 050 451 880  |
| H                                                                 | -0.056 821 795 015 | -0.032 978 029 799 | -0.008 498 168 330 |
| H                                                                 | 0.070 666 180 469  | -0.017 375 552 577 | 0.054 525 766 633  |

Wavenumber/cm<sup>-1</sup>: 1268.5206

| $\frac{\partial \mu_{x,y,z}}{\partial Q_r} / (e u^{-0.5})$        | 0.004 449 016 479  | 0.007 572 672 901  | 0.013 033 092 059  |
|-------------------------------------------------------------------|--------------------|--------------------|--------------------|
| <i>l</i> -matrix coefficients/(u <sup>1/2</sup> Å <sup>-1</sup> ) |                    |                    |                    |
| O                                                                 | 0.015 513 026 169  | 0.036 128 859 104  | 0.006 566 611 811  |
| C                                                                 | 0.057 920 841 975  | 0.049 210 245 769  | 0.116 093 997 359  |
| C                                                                 | -0.032 410 060 439 | -0.061 142 482 875 | -0.413 174 039 087 |
| C                                                                 | 0.051 350 204 131  | -0.008 069 835 311 | 0.353 100 650 477  |
| C                                                                 | -0.060 412 908 965 | 0.029 344 267 330  | -0.138 693 915 349 |
| C                                                                 | 0.037 989 484 880  | -0.113 828 736 280 | -0.049 325 513 343 |
| C                                                                 | -0.011 174 514 657 | 0.048 414 213 350  | 0.222 286 259 016  |
| H                                                                 | -0.300 158 137 199 | -0.078 830 366 438 | 0.042 512 253 335  |
| H                                                                 | 0.084 982 346 786  | 0.077 688 502 395  | -0.070 389 161 764 |
| H                                                                 | -0.072 317 712 049 | -0.057 395 729 382 | -0.122 153 746 462 |
| H                                                                 | -0.098 211 773 761 | -0.041 807 824 847 | -0.098 563 317 194 |
| H                                                                 | 0.090 743 671 540  | 0.194 739 987 768  | 0.075 468 246 798  |
| H                                                                 | -0.340 643 031 186 | -0.149 672 636 684 | -0.022 077 223 041 |
| H                                                                 | 0.299 249 175 393  | 0.197 206 650 247  | 0.058 077 704 975  |
| H                                                                 | -0.076 294 942 730 | 0.065 060 208 638  | -0.122 327 954 355 |
| H                                                                 | 0.210 334 014 140  | -0.104 665 097 872 | 0.045 060 596 667  |
| H                                                                 | -0.008 831 996 251 | -0.052 703 303 506 | -0.123 439 898 110 |

Wavenumber/cm<sup>-1</sup>: 1304.9958

| $\frac{\partial \mu_{x,y,z}}{\partial Q_r} / (e u^{-0.5})$        | 0.013 318 709 816  | 0.018 184 667 756  | -0.012 794 115 913 |
|-------------------------------------------------------------------|--------------------|--------------------|--------------------|
| <i>l</i> -matrix coefficients/(u <sup>1/2</sup> Å <sup>-1</sup> ) |                    |                    |                    |
| O                                                                 | 0.088 342 173 075  | -0.010 614 024 040 | -0.062 286 276 390 |
| C                                                                 | -0.099 793 584 627 | -0.166 004 100 389 | -0.133 392 867 160 |
| C                                                                 | -0.028 556 378 874 | 0.158 135 196 660  | 0.048 076 729 671  |
| C                                                                 | 0.162 093 257 505  | -0.104 769 890 429 | 0.042 709 605 657  |
| C                                                                 | -0.156 592 115 714 | -0.059 698 396 171 | -0.252 125 294 340 |
| C                                                                 | -0.036 266 739 250 | 0.200 678 291 933  | 0.335 741 206 266  |
| C                                                                 | 0.001 466 678 768  | -0.064 705 455 587 | 0.005 049 190 601  |
| H                                                                 | -0.212 125 748 616 | 0.064 924 931 462  | 0.030 492 863 004  |
| H                                                                 | 0.417 355 041 985  | -0.128 893 823 016 | -0.000 332 788 733 |
| H                                                                 | -0.074 711 860 775 | -0.087 878 737 094 | 0.004 899 902 667  |
| H                                                                 | -0.348 366 982 546 | 0.220 462 277 141  | 0.015 857 918 501  |
| H                                                                 | 0.286 211 694 903  | -0.130 514 708 139 | -0.028 581 191 150 |
| H                                                                 | 0.071 780 179 582  | 0.254 232 921 780  | -0.001 924 639 166 |
| H                                                                 | 0.009 323 719 914  | -0.089 136 153 508 | 0.042 340 611 885  |
| H                                                                 | 0.075 728 999 262  | -0.003 845 113 735 | 0.020 776 480 282  |
| H                                                                 | 0.018 771 100 877  | 0.029 702 428 613  | 0.006 762 583 906  |
| H                                                                 | -0.051 727 359 446 | 0.038 762 183 467  | -0.001 131 582 169 |

Wavenumber/cm<sup>-1</sup>: 1321.4815

| $\frac{\partial \mu_{x,y,z}}{\partial Q_r} / (e u^{-0.5})$        | -0.001 070 139 921 | 0.005 520 746 757  | -0.000 184 354 713 |
|-------------------------------------------------------------------|--------------------|--------------------|--------------------|
| <i>l</i> -matrix coefficients/(u <sup>1/2</sup> Å <sup>-1</sup> ) |                    |                    |                    |
| O                                                                 | 0.063 464 572 615  | -0.094 130 426 633 | 0.036 506 863 068  |
| C                                                                 | 0.082 857 305 571  | -0.256 108 488 384 | 0.074 893 138 771  |
| C                                                                 | -0.266 643 495 002 | 0.080 682 964 449  | -0.055 992 213 080 |
| C                                                                 | 0.169 895 605 536  | 0.031 688 676 311  | -0.055 281 334 506 |
| C                                                                 | 0.000 104 424 847  | -0.259 427 675 916 | 0.070 075 997 357  |
| C                                                                 | -0.205 735 632 464 | 0.573 227 219 898  | -0.223 193 541 892 |
| C                                                                 | 0.071 252 247 408  | -0.061 223 446 421 | 0.139 502 776 342  |
| H                                                                 | 0.318 651 539 911  | -0.040 023 621 877 | -0.012 736 348 865 |
| H                                                                 | 0.030 380 842 758  | -0.057 736 681 806 | -0.003 910 534 395 |
| H                                                                 | -0.103 098 824 088 | 0.197 007 978 104  | -0.007 310 580 601 |
| H                                                                 | -0.002 622 926 899 | 0.079 108 583 479  | 0.052 442 775 989  |
| H                                                                 | -0.084 268 442 453 | -0.000 982 923 683 | 0.010 082 710 977  |
| H                                                                 | -0.163 299 492 858 | -0.183 774 892 652 | 0.014 107 752 436  |
| H                                                                 | 0.069 948 155 173  | 0.021 095 131 500  | -0.006 482 402 933 |
| H                                                                 | 0.051 718 294 453  | 0.015 149 196 969  | -0.019 499 872 684 |
| H                                                                 | 0.161 897 376 831  | -0.027 673 205 867 | 0.037 791 334 677  |
| H                                                                 | -0.020 330 692 489 | -0.002 857 524 192 | -0.037 348 656 718 |

Wavenumber/cm<sup>-1</sup>: 1349.0515

| $\frac{\partial \mu_{x,y,z}}{\partial Q_r} / (e u^{-0.5})$        | -0.020 090 167 426 | 0.002 079 883 163  | -0.005 096 096 048 |
|-------------------------------------------------------------------|--------------------|--------------------|--------------------|
| <i>l</i> -matrix coefficients/(u <sup>1/2</sup> Å <sup>-1</sup> ) |                    |                    |                    |
| O                                                                 | -0.053 794 892 914 | -0.056 054 800 524 | -0.028 595 315 725 |
| C                                                                 | 0.172 438 161 266  | 0.134 157 729 868  | -0.208 541 613 219 |
| C                                                                 | -0.206 607 846 271 | -0.410 978 636 247 | 0.001 662 772 573  |
| C                                                                 | -0.066 807 458 924 | 0.213 364 927 442  | 0.116 131 853 226  |
| C                                                                 | 0.189 383 189 895  | -0.100 638 590 178 | -0.083 402 122 573 |
| C                                                                 | -0.088 349 458 451 | 0.185 590 489 495  | 0.165 378 003 699  |
| C                                                                 | 0.110 721 834 825  | 0.251 006 506 580  | 0.023 601 733 579  |
| H                                                                 | 0.027 647 690 609  | 0.116 422 784 402  | -0.028 397 349 170 |
| H                                                                 | 0.085 667 512 183  | -0.006 377 939 266 | 0.003 080 855 837  |
| H                                                                 | -0.151 969 578 545 | -0.321 568 355 769 | -0.013 103 735 715 |
| H                                                                 | 0.068 532 667 520  | -0.009 168 698 335 | 0.012 019 010 597  |
| H                                                                 | -0.028 117 774 588 | 0.036 007 178 774  | 0.035 121 830 899  |
| H                                                                 | -0.006 147 990 283 | 0.039 381 482 964  | 0.016 468 101 448  |
| H                                                                 | -0.117 027 009 977 | -0.250 773 771 056 | 0.030 153 147 776  |
| H                                                                 | -0.262 469 378 801 | -0.004 374 028 886 | -0.038 080 631 350 |
| H                                                                 | -0.041 751 777 317 | -0.161 992 175 228 | -0.008 845 251 655 |
| H                                                                 | 0.257 553 700 286  | -0.154 903 077 785 | 0.054 314 990 500  |

Wavenumber/cm<sup>-1</sup>: 1385.9831

| $\frac{\partial \mu_{x,y,z}}{\partial Q_r} / (e u^{-0.5})$        | 0.001 805 849 584  | 0.002 211 753 401  | -0.006 902 630 267 |
|-------------------------------------------------------------------|--------------------|--------------------|--------------------|
| <i>l</i> -matrix coefficients/(u <sup>1/2</sup> Å <sup>-1</sup> ) |                    |                    |                    |
| O                                                                 | -0.020 974 105 432 | -0.057 641 641 829 | 0.002 878 673 538  |
| C                                                                 | 0.114 261 165 186  | -0.171 419 069 518 | 0.010 359 354 281  |
| C                                                                 | 0.533 517 440 291  | -0.204 857 568 604 | 0.107 667 337 965  |
| C                                                                 | 0.079 005 032 250  | 0.060 124 925 452  | 0.089 214 986 377  |
| C                                                                 | -0.056 495 525 071 | -0.101 833 277 310 | -0.008 492 215 238 |
| C                                                                 | -0.116 328 016 730 | 0.297 385 776 318  | -0.022 346 262 493 |
| C                                                                 | -0.294 685 811 079 | 0.127 029 486 629  | -0.242 901 189 798 |
| H                                                                 | -0.182 033 041 860 | -0.024 042 873 487 | 0.043 891 910 011  |
| H                                                                 | -0.107 834 190 839 | -0.067 687 531 911 | 0.050 018 686 506  |
| H                                                                 | 0.202 210 485 801  | -0.038 307 631 956 | 0.033 190 987 868  |
| H                                                                 | -0.122 931 231 949 | 0.121 206 739 242  | 0.043 688 636 983  |
| H                                                                 | -0.131 774 503 159 | 0.158 405 760 654  | 0.050 034 639 369  |
| H                                                                 | -0.153 518 376 065 | -0.088 617 260 373 | 0.006 223 741 219  |
| H                                                                 | 0.107 001 733 945  | 0.065 590 666 143  | 0.020 737 214 202  |
| H                                                                 | -0.112 381 011 757 | -0.003 793 687 558 | 0.013 133 301 158  |
| H                                                                 | -0.271 950 849 594 | 0.062 386 429 819  | -0.065 679 981 383 |
| H                                                                 | -0.038 236 603 352 | 0.022 311 113 899  | 0.022 841 843 226  |



Wavenumber/cm<sup>-1</sup>: 1416.4701

| $\frac{\partial \mu_{x,y,z}}{\partial Q_r} / (e u^{-0.5})$        | 0.011 568 437 328  | 0.000 945 782 370  | -0.001 885 122 555 |
|-------------------------------------------------------------------|--------------------|--------------------|--------------------|
| <i>l</i> -matrix coefficients/(u <sup>1/2</sup> Å <sup>-1</sup> ) |                    |                    |                    |
| O                                                                 | -0.025 411 853 983 | -0.012 882 665 436 | 0.003 344 951 279  |
| C                                                                 | -0.042 759 140 208 | -0.095 982 528 342 | 0.091 728 383 526  |
| C                                                                 | 0.148 692 444 608  | -0.003 690 856 177 | -0.151 168 826 067 |
| C                                                                 | 0.083 489 197 383  | 0.015 146 743 818  | 0.082 588 399 793  |
| C                                                                 | -0.095 890 562 639 | 0.015 701 527 693  | -0.068 370 618 302 |
| C                                                                 | -0.009 779 481 400 | 0.022 663 605 055  | -0.008 492 653 498 |
| C                                                                 | -0.171 484 126 524 | 0.114 655 213 660  | 0.186 746 002 664  |
| H                                                                 | 0.268 670 738 869  | -0.054 695 648 223 | -0.025 335 231 074 |
| H                                                                 | -0.313 857 872 748 | -0.014 351 262 693 | 0.057 132 865 853  |
| H                                                                 | 0.355 631 046 102  | -0.064 350 808 147 | -0.038 368 235 021 |
| H                                                                 | -0.082 208 053 200 | 0.041 236 558 231  | -0.031 702 249 084 |
| H                                                                 | 0.245 343 045 267  | -0.060 943 753 994 | -0.017 598 247 006 |
| H                                                                 | 0.191 396 679 533  | 0.203 822 699 059  | 0.001 633 022 754  |
| H                                                                 | -0.242 957 068 258 | -0.176 683 238 547 | -0.035 062 878 658 |
| H                                                                 | -0.243 588 039 082 | 0.090 746 914 409  | -0.226 584 402 154 |
| H                                                                 | 0.310 298 778 011  | -0.125 692 013 388 | 0.031 832 473 182  |
| H                                                                 | -0.084 638 276 296 | -0.024 202 900 316 | -0.188 493 180 812 |

Wavenumber/cm<sup>-1</sup>: 1449.2099

| $\frac{\partial \mu_{x,y,z}}{\partial Q_r} / (e u^{-0.5})$        | 0.001 674 627 870  | 0.005 118 986 933  | 0.000 436 201 794  |
|-------------------------------------------------------------------|--------------------|--------------------|--------------------|
| <i>l</i> -matrix coefficients/(u <sup>1/2</sup> Å <sup>-1</sup> ) |                    |                    |                    |
| O                                                                 | -0.032 739 647 805 | -0.043 830 252 242 | 0.010 433 571 227  |
| C                                                                 | 0.066 266 399 651  | 0.062 099 059 904  | 0.043 517 368 850  |
| C                                                                 | -0.009 329 223 352 | -0.100 682 898 919 | -0.067 195 228 246 |
| C                                                                 | -0.450 159 179 702 | 0.115 450 041 063  | -0.021 517 992 147 |
| C                                                                 | 0.460 641 394 103  | -0.065 238 473 890 | 0.037 395 510 812  |
| C                                                                 | -0.045 946 018 081 | 0.020 314 160 938  | -0.035 104 627 252 |
| C                                                                 | -0.051 520 707 590 | -0.141 511 133 538 | 0.040 547 769 464  |
| H                                                                 | 0.092 607 400 007  | -0.034 819 552 324 | -0.016 981 498 119 |
| H                                                                 | 0.004 185 929 773  | 0.048 166 169 320  | -0.028 342 414 278 |
| H                                                                 | 0.059 962 049 520  | -0.086 929 086 553 | -0.020 875 950 556 |
| H                                                                 | -0.406 691 646 124 | 0.216 331 018 573  | 0.015 610 938 236  |
| H                                                                 | -0.124 719 289 643 | 0.047 632 143 602  | -0.008 587 955 347 |
| H                                                                 | 0.247 688 744 463  | 0.151 513 609 884  | 0.044 771 692 589  |
| H                                                                 | 0.285 482 928 663  | 0.073 535 700 921  | 0.054 155 845 045  |
| H                                                                 | 0.143 004 576 109  | 0.012 629 969 009  | -0.002 740 017 868 |
| H                                                                 | 0.105 298 907 968  | 0.035 406 798 088  | 0.015 380 298 305  |
| H                                                                 | -0.172 659 374 154 | 0.089 387 491 716  | -0.085 822 113 645 |

Wavenumber/cm<sup>-1</sup>: 1453.0804

| $\frac{\partial \mu_{x,y,z}}{\partial Q_r} / (e u^{-0.5})$        | 0.009 640 170 691  | 0.002 596 375 458  | -0.002 701 490 783 |
|-------------------------------------------------------------------|--------------------|--------------------|--------------------|
| <i>l</i> -matrix coefficients/(u <sup>1/2</sup> Å <sup>-1</sup> ) |                    |                    |                    |
| O                                                                 | 0.020 809 150 018  | -0.017 987 111 075 | -0.039 564 282 146 |
| C                                                                 | -0.100 070 534 382 | -0.069 592 385 943 | -0.104 878 753 910 |
| C                                                                 | -0.004 114 486 365 | 0.125 544 496 573  | 0.006 297 953 292  |
| C                                                                 | -0.132 465 966 967 | -0.246 074 382 378 | 0.199 832 009 194  |
| C                                                                 | 0.117 294 162 818  | -0.033 945 314 752 | -0.263 752 992 977 |
| C                                                                 | -0.003 399 200 145 | 0.047 480 786 004  | 0.196 309 855 473  |
| C                                                                 | 0.102 687 888 368  | 0.047 821 778 459  | -0.042 175 872 012 |
| H                                                                 | 0.203 145 741 945  | 0.122 222 551 488  | -0.011 573 888 952 |
| H                                                                 | -0.249 446 502 543 | -0.106 060 068 863 | 0.131 991 349 359  |
| H                                                                 | -0.017 065 162 080 | 0.378 329 333 335  | 0.021 388 168 093  |
| H                                                                 | -0.054 411 574 691 | -0.249 052 630 859 | -0.274 111 790 908 |
| H                                                                 | -0.028 054 528 684 | 0.334 017 854 359  | 0.031 472 350 985  |
| H                                                                 | -0.048 349 787 665 | 0.215 449 150 531  | 0.027 992 594 016  |
| H                                                                 | 0.180 261 458 102  | -0.097 630 224 429 | 0.127 557 414 957  |
| H                                                                 | -0.027 818 234 404 | -0.030 813 831 864 | 0.055 619 643 605  |
| H                                                                 | -0.107 506 256 747 | 0.010 025 399 496  | -0.008 009 128 092 |
| H                                                                 | 0.135 614 371 145  | -0.060 330 937 406 | 0.084 186 046 346  |

Wavenumber/cm<sup>-1</sup>: 1495.4646

| $\frac{\partial \mu_{x,y,z}}{\partial Q_r} / (e u^{-0.5})$        | 0.007 619 144 543  | 0.001 596 721 972  | 0.000 575 478 811  |
|-------------------------------------------------------------------|--------------------|--------------------|--------------------|
| <i>l</i> -matrix coefficients/(u <sup>1/2</sup> Å <sup>-1</sup> ) |                    |                    |                    |
| O                                                                 | 0.071 649 104 223  | -0.021 625 761 988 | 0.028 171 975 934  |
| C                                                                 | -0.177 591 647 938 | -0.269 576 932 936 | 0.112 876 126 805  |
| C                                                                 | 0.034 161 824 054  | 0.279 984 277 401  | -0.016 866 713 314 |
| C                                                                 | -0.181 244 341 744 | -0.164 810 511 104 | -0.183 596 048 814 |
| C                                                                 | 0.148 927 246 042  | 0.043 455 278 555  | 0.178 660 215 540  |
| C                                                                 | 0.006 108 442 512  | 0.046 775 800 418  | -0.134 306 470 844 |
| C                                                                 | 0.144 479 421 497  | 0.252 156 080 606  | 0.021 966 319 346  |
| H                                                                 | -0.231 301 640 044 | -0.079 206 089 794 | 0.056 392 350 804  |
| H                                                                 | -0.034 701 864 849 | -0.059 679 252 461 | 0.003 488 081 996  |
| H                                                                 | -0.041 384 323 384 | -0.057 932 043 537 | -0.014 387 215 735 |
| H                                                                 | -0.131 695 356 643 | 0.035 424 937 217  | 0.006 909 344 088  |
| H                                                                 | 0.025 151 123 200  | -0.139 317 273 956 | -0.062 599 566 110 |
| H                                                                 | 0.164 008 357 223  | -0.051 691 734 221 | -0.002 264 530 131 |
| H                                                                 | 0.100 438 127 182  | 0.174 951 126 100  | -0.047 747 971 589 |
| H                                                                 | -0.358 254 254 489 | -0.010 594 696 038 | -0.084 794 417 073 |
| H                                                                 | -0.051 116 362 204 | -0.153 878 376 825 | -0.008 599 165 283 |
| H                                                                 | 0.360 249 035 398  | -0.220 835 146 270 | 0.114 775 500 707  |

Wavenumber/cm<sup>-1</sup>: 1499.0696

| $\frac{\partial \mu_{x,y,z}}{\partial Q_r} / (e u^{-0.5})$        | -0.000 474 377 182 | 0.002 644 426 754  | -0.001 679 053 234 |
|-------------------------------------------------------------------|--------------------|--------------------|--------------------|
| <i>l</i> -matrix coefficients/(u <sup>1/2</sup> Å <sup>-1</sup> ) |                    |                    |                    |
| O                                                                 | -0.021 308 776 808 | 0.001 346 395 808  | 0.044 935 650 688  |
| C                                                                 | 0.237 669 052 361  | 0.220 436 760 423  | 0.285 129 989 830  |
| C                                                                 | 0.028 014 921 927  | -0.061 947 972 270 | -0.080 834 459 962 |
| C                                                                 | -0.023 792 112 303 | -0.259 230 047 637 | 0.137 372 406 450  |
| C                                                                 | -0.157 912 921 851 | -0.066 528 830 124 | 0.047 381 667 898  |
| C                                                                 | -0.081 836 473 723 | 0.172 290 158 421  | -0.226 508 051 203 |
| C                                                                 | 0.033 452 794 925  | -0.006 765 294 441 | -0.101 984 800 703 |
| H                                                                 | 0.050 789 290 103  | -0.258 820 936 469 | -0.032 867 639 878 |
| H                                                                 | 0.036 770 273 659  | 0.265 228 093 292  | -0.203 195 513 404 |
| H                                                                 | -0.171 672 705 368 | -0.040 610 117 884 | -0.027 010 623 757 |
| H                                                                 | -0.185 912 199 435 | -0.108 142 633 965 | -0.218 318 604 317 |
| H                                                                 | 0.256 225 652 797  | 0.087 287 062 901  | -0.023 161 778 625 |
| H                                                                 | 0.238 084 891 541  | 0.100 344 846 221  | -0.011 797 004 196 |
| H                                                                 | -0.181 339 915 512 | -0.041 478 441 774 | -0.080 207 204 918 |
| H                                                                 | 0.064 519 613 431  | -0.042 913 118 336 | 0.109 709 592 233  |
| H                                                                 | -0.222 827 360 036 | 0.054 683 175 785  | -0.019 806 534 319 |
| H                                                                 | 0.077 384 136 428  | -0.014 917 591 278 | 0.118 587 281 941  |

Wavenumber/cm<sup>-1</sup>: 1504.3158

| $\frac{\partial \mu_{x,y,z}}{\partial Q_r} / (e u^{-0.5})$        | -0.001 202 310 260 | -0.003 301 759 499 | 0.003 745 749 755  |
|-------------------------------------------------------------------|--------------------|--------------------|--------------------|
| <i>l</i> -matrix coefficients/(u <sup>1/2</sup> Å <sup>-1</sup> ) |                    |                    |                    |
| O                                                                 | 0.035 453 331 611  | -0.021 042 293 660 | 0.015 832 551 978  |
| C                                                                 | -0.366 114 098 855 | -0.144 373 740 438 | 0.192 918 607 391  |
| C                                                                 | 0.031 979 666 842  | 0.013 792 793 588  | -0.285 098 958 665 |
| C                                                                 | 0.113 521 147 921  | 0.435 618 717 638  | 0.133 947 571 527  |
| C                                                                 | 0.044 480 438 670  | -0.120 898 333 756 | -0.093 047 020 839 |
| C                                                                 | 0.063 592 965 382  | -0.075 286 857 941 | -0.047 736 831 140 |
| C                                                                 | 0.224 738 294 673  | -0.076 587 825 930 | -0.051 662 358 737 |
| H                                                                 | -0.087 563 481 625 | -0.139 938 109 713 | 0.016 061 988 671  |
| H                                                                 | -0.292 854 906 856 | 0.020 131 589 928  | -0.005 140 138 952 |
| H                                                                 | -0.119 012 220 055 | -0.003 167 123 972 | -0.081 972 855 923 |
| H                                                                 | -0.030 288 028 311 | 0.222 347 029 479  | 0.135 491 203 681  |
| H                                                                 | 0.002 960 650 377  | 0.016 284 456 458  | 0.048 374 076 642  |
| H                                                                 | -0.012 698 321 812 | 0.079 751 867 288  | 0.021 952 747 637  |
| H                                                                 | -0.116 258 149 371 | -0.219 150 508 272 | 0.030 944 051 757  |
| H                                                                 | 0.186 048 964 300  | -0.057 209 323 847 | 0.156 090 345 629  |
| H                                                                 | -0.176 168 898 386 | 0.067 497 726 828  | -0.003 797 597 233 |
| H                                                                 | 0.117 278 603 485  | -0.014 090 763 272 | 0.139 059 151 673  |

Wavenumber/cm<sup>-1</sup>: 1814.5434

| $\frac{\partial \mu_{x,y,z}}{\partial Q_r} / (e u^{-0.5})$        | 0.003 998 703 923  | -0.003 000 243 313 | 0.003 310 522 607  |
|-------------------------------------------------------------------|--------------------|--------------------|--------------------|
| <i>l</i> -matrix coefficients/(u <sup>1/2</sup> Å <sup>-1</sup> ) |                    |                    |                    |
| O                                                                 | -0.094 729 313 123 | -0.029 062 459 732 | 0.011 637 119 732  |
| C                                                                 | 0.234 458 188 495  | -0.468 954 215 594 | -0.073 892 773 338 |
| C                                                                 | -0.042 319 616 122 | -0.166 064 906 509 | -0.138 533 660 469 |
| C                                                                 | -0.097 336 765 143 | 0.206 288 204 376  | 0.144 140 047 891  |
| C                                                                 | -0.121 576 081 019 | 0.517 727 730 574  | 0.099 083 112 216  |
| C                                                                 | -0.077 660 365 040 | -0.048 327 442 889 | -0.032 234 660 666 |
| C                                                                 | 0.097 891 053 788  | -0.067 010 503 712 | -0.006 749 028 842 |
| H                                                                 | 0.128 924 350 056  | 0.036 263 624 589  | 0.029 901 248 973  |
| H                                                                 | 0.119 529 647 524  | -0.232 286 576 587 | 0.105 224 181 712  |
| H                                                                 | -0.029 037 528 529 | 0.017 076 476 571  | -0.035 541 082 852 |
| H                                                                 | -0.000 957 610 698 | -0.023 157 742 401 | -0.080 449 759 375 |
| H                                                                 | 0.082 606 018 941  | 0.134 263 332 337  | 0.014 473 162 218  |
| H                                                                 | 0.150 089 082 610  | 0.047 732 241 283  | -0.051 435 674 446 |
| H                                                                 | -0.121 285 349 389 | 0.240 341 437 106  | -0.125 061 643 034 |
| H                                                                 | 0.096 390 608 264  | -0.032 855 419 605 | 0.075 715 139 100  |
| H                                                                 | -0.061 254 276 554 | 0.027 134 708 178  | 0.003 246 696 584  |
| H                                                                 | 0.034 992 550 990  | -0.007 795 805 160 | 0.045 825 763 376  |

Wavenumber/cm<sup>-1</sup>: 2994.9642

| $\frac{\partial \mu_{x,y,z}}{\partial Q_r} / (e u^{-0.5})$        | 0.022 140 121 428  | -0.015 445 820 871 | 0.013 577 609 994                    |
|-------------------------------------------------------------------|--------------------|--------------------|--------------------------------------|
| <i>l</i> -matrix coefficients/(u <sup>1/2</sup> Å <sup>-1</sup> ) |                    |                    |                                      |
| O                                                                 | -0.329 376 259 491 | -0.102 384 530 353 | 3.015 814 500 000 × 10 <sup>-5</sup> |
| C                                                                 | 0.233 287 287 814  | -0.124 110 747 481 | 0.230 638 136 130                    |
| C                                                                 | 0.028 910 773 070  | 0.172 882 158 192  | 0.026 920 093 616                    |
| C                                                                 | 0.177 370 401 765  | 0.012 187 409 697  | -0.100 583 786 458                   |
| C                                                                 | 0.147 888 365 312  | 0.195 032 956 350  | -0.259 022 680 487                   |
| C                                                                 | -0.200 742 385 977 | -0.161 013 475 614 | 0.055 857 969 623                    |
| C                                                                 | -0.083 080 863 866 | 0.057 448 320 534  | -0.024 194 219 257                   |
| H                                                                 | 0.162 805 892 778  | -0.286 430 855 990 | -0.036 191 552 151                   |
| H                                                                 | 0.130 457 111 302  | 0.107 778 612 479  | -0.157 066 733 021                   |
| H                                                                 | -0.047 882 952 738 | -0.004 201 738 503 | 0.003 336 969 780                    |
| H                                                                 | 0.184 798 682 260  | 0.028 939 285 456  | 0.163 447 920 267                    |
| H                                                                 | -0.115 247 842 021 | -0.140 722 322 280 | 0.012 551 780 726                    |
| H                                                                 | -0.135 819 831 983 | 0.304 843 821 248  | 0.058 911 543 524                    |
| H                                                                 | 0.208 833 959 658  | -0.069 300 997 864 | 0.184 473 555 329                    |
| H                                                                 | -0.094 139 647 142 | -0.000 297 914 281 | -0.016 867 556 694                   |
| H                                                                 | -0.073 449 957 683 | -0.021 029 593 960 | -0.009 255 954 783                   |
| H                                                                 | 0.043 768 363 856  | -0.037 844 059 346 | 0.039 505 839 190                    |

Wavenumber/cm<sup>-1</sup>: 3012.0352

| $\frac{\partial \mu_{x,y,z}}{\partial Q_r} / (e \text{ u}^{-0.5})$ | -0.040 466 911 989 | 0.049 280 816 946  | -0.041 270 587 535 |
|--------------------------------------------------------------------|--------------------|--------------------|--------------------|
| <i>l</i> -matrix coefficients/(u <sup>1/2</sup> Å <sup>-1</sup> )  |                    |                    |                    |
| O                                                                  | 0.302 051 296 320  | 0.172 438 210 439  | -0.093 525 287 696 |
| C                                                                  | 0.092 938 153 800  | -0.060 836 794 308 | 0.095 843 149 657  |
| C                                                                  | 0.057 262 527 656  | -0.156 855 515 756 | -0.063 254 279 596 |
| C                                                                  | -0.388 715 700 981 | -0.153 318 931 172 | -0.114 900 988 587 |
| C                                                                  | -0.344 677 434 216 | 0.182 870 258 169  | -0.099 095 653 354 |
| C                                                                  | 0.202 494 369 601  | 0.200 627 479 766  | 0.212 502 653 547  |
| C                                                                  | 0.159 845 247 171  | -0.096 658 472 975 | 0.026 388 660 857  |
| H                                                                  | 0.091 135 368 870  | -0.170 043 090 012 | -0.036 381 083 006 |
| H                                                                  | -0.137 516 133 799 | 0.080 275 860 281  | -0.083 778 236 316 |
| H                                                                  | 0.030 886 988 044  | -0.095 497 230 215 | -0.020 214 125 104 |
| H                                                                  | -0.026 367 462 219 | 0.009 992 675 988  | 0.163 831 081 288  |
| H                                                                  | -0.254 813 020 432 | -0.190 315 061 851 | 0.003 371 591 681  |
| H                                                                  | -0.251 312 669 628 | 0.094 026 918 988  | 0.023 781 971 752  |
| H                                                                  | -0.030 300 441 595 | -0.025 299 739 116 | 0.103 243 535 585  |
| H                                                                  | 0.042 316 249 356  | -0.026 156 634 420 | -0.000 462 355 258 |
| H                                                                  | 0.042 394 400 305  | -0.041 614 723 335 | 0.006 798 944 617  |
| H                                                                  | 0.052 560 172 294  | -0.031 816 466 331 | 0.013 988 758 017  |

Wavenumber/cm<sup>-1</sup>: 3018.8814

| $\frac{\partial \mu_{x,y,z}}{\partial Q_r} / (e \text{ u}^{-0.5})$ | -0.006 486 703 963 | 0.002 407 775 369  | -0.007 960 575 560 |
|--------------------------------------------------------------------|--------------------|--------------------|--------------------|
| <i>l</i> -matrix coefficients/(u <sup>1/2</sup> Å <sup>-1</sup> )  |                    |                    |                    |
| O                                                                  | 0.348 433 598 106  | 0.198 269 327 709  | 0.121 241 516 350  |
| C                                                                  | 0.043 236 950 427  | -0.276 892 880 661 | 0.060 917 931 919  |
| C                                                                  | -0.285 111 474 825 | -0.034 029 734 601 | 0.220 017 130 816  |
| C                                                                  | -0.047 931 224 232 | 0.099 080 622 879  | 0.047 875 741 534  |
| C                                                                  | 0.069 395 430 027  | -0.005 845 787 114 | -0.071 896 846 322 |
| C                                                                  | 0.329 929 104 229  | -0.086 219 535 094 | -0.337 025 309 308 |
| C                                                                  | -0.370 077 618 685 | 0.084 318 686 643  | -0.071 802 017 530 |
| H                                                                  | -0.082 877 233 998 | -0.100 892 107 801 | 0.022 189 613 165  |
| H                                                                  | 0.086 121 835 004  | -0.055 799 397 611 | -0.031 021 369 446 |
| H                                                                  | -0.143 140 120 938 | 0.000 892 877 824  | 0.061 019 028 259  |
| H                                                                  | 0.027 541 306 528  | -0.048 371 767 669 | -0.076 163 715 721 |
| H                                                                  | -0.005 372 604 888 | 0.118 872 326 565  | 0.006 703 522 939  |
| H                                                                  | -0.034 933 866 422 | 0.173 694 549 746  | 0.056 829 266 524  |
| H                                                                  | -0.032 749 999 844 | -0.203 806 383 785 | 0.115 227 996 593  |
| H                                                                  | -0.113 368 015 023 | 0.031 653 477 528  | -0.044 410 343 535 |
| H                                                                  | -0.057 424 934 250 | 0.012 177 226 700  | -0.022 107 466 349 |
| H                                                                  | -0.132 539 339 316 | 0.039 674 283 460  | -0.046 900 248 461 |

Wavenumber/cm<sup>-1</sup>: 3024.1151

| $\frac{\partial \mu_{x,y,z}}{\partial Q_r} / (e u^{-0.5})$        | 0.003 918 427 995  | -0.032 761 231 968 | 0.024 255 588 714  |
|-------------------------------------------------------------------|--------------------|--------------------|--------------------|
| <i>l</i> -matrix coefficients/(u <sup>1/2</sup> Å <sup>-1</sup> ) |                    |                    |                    |
| O                                                                 | 0.217 382 998 113  | -0.540 644 185 362 | 0.034 769 828 434  |
| C                                                                 | -0.303 562 261 524 | 0.103 196 192 413  | -0.019 521 456 193 |
| C                                                                 | -0.105 169 190 601 | -0.197 853 620 315 | 0.186 099 240 556  |
| C                                                                 | 0.132 681 213 520  | -0.045 392 935 928 | -0.007 252 629 043 |
| C                                                                 | 0.064 777 351 619  | 0.387 321 216 741  | -0.054 259 943 464 |
| C                                                                 | -0.073 117 539 123 | 0.233 988 255 459  | -0.066 024 077 768 |
| C                                                                 | 0.042 809 336 423  | 0.042 241 763 353  | -0.022 382 209 697 |
| H                                                                 | -0.189 902 555 550 | -0.089 115 053 127 | -0.032 859 031 159 |
| H                                                                 | -0.184 025 704 140 | 0.103 192 081 770  | -0.093 749 113 954 |
| H                                                                 | -0.033 697 748 961 | -0.069 456 549 496 | 0.051 816 692 206  |
| H                                                                 | 0.117 525 266 069  | -0.079 388 806 933 | -0.032 335 573 444 |
| H                                                                 | 0.028 942 443 620  | 0.021 381 643 111  | -0.001 611 390 782 |
| H                                                                 | 0.041 505 526 798  | 0.170 926 966 629  | 0.000 595 281 428  |
| H                                                                 | 0.084 453 084 060  | 0.137 812 375 956  | 0.018 696 961 607  |
| H                                                                 | 0.074 681 831 107  | 0.040 475 149 144  | -0.026 661 353 313 |
| H                                                                 | 0.107 826 349 416  | 0.028 208 924 945  | -0.007 143 169 824 |
| H                                                                 | -0.079 446 221 736 | 0.082 817 466 872  | -0.072 781 382 183 |

Wavenumber/cm<sup>-1</sup>: 3030.0237

| $\frac{\partial \mu_{x,y,z}}{\partial Q_r} / (e u^{-0.5})$        | 0.004 772 291 430  | -0.048 894 670 781 | 0.040 944 874 358  |
|-------------------------------------------------------------------|--------------------|--------------------|--------------------|
| <i>l</i> -matrix coefficients/(u <sup>1/2</sup> Å <sup>-1</sup> ) |                    |                    |                    |
| O                                                                 | 0.150 603 357 865  | -0.033 938 773 568 | -0.273 617 053 687 |
| C                                                                 | -0.004 428 559 086 | -0.106 330 957 613 | 0.033 335 165 969  |
| C                                                                 | -0.187 515 869 634 | 0.046 285 724 104  | -0.083 992 090 089 |
| C                                                                 | 0.080 563 160 912  | 0.060 321 214 710  | 0.006 875 693 808  |
| C                                                                 | 0.164 945 680 853  | -0.027 531 112 235 | 0.021 804 899 242  |
| C                                                                 | 0.131 548 680 728  | 0.003 371 097 051  | 0.530 665 279 175  |
| C                                                                 | -0.316 464 777 813 | 0.095 158 574 085  | -0.021 202 302 411 |
| H                                                                 | 0.140 956 035 777  | -0.254 459 591 449 | -0.088 382 902 317 |
| H                                                                 | -0.120 718 601 822 | 0.109 476 980 980  | -0.170 566 921 987 |
| H                                                                 | -0.085 890 391 026 | 0.022 367 649 380  | -0.023 415 945 204 |
| H                                                                 | 0.029 564 599 656  | -0.003 891 112 220 | -0.029 772 151 374 |
| H                                                                 | 0.059 237 797 810  | 0.020 924 829 414  | -0.005 037 100 530 |
| H                                                                 | 0.129 498 592 186  | -0.291 569 086 990 | -0.114 443 772 490 |
| H                                                                 | 0.000 125 240 601  | 0.189 108 732 434  | -0.213 031 524 259 |
| H                                                                 | -0.066 474 624 082 | 0.021 474 707 241  | 0.027 453 744 671  |
| H                                                                 | -0.151 552 755 664 | 0.045 473 503 435  | -0.004 006 782 293 |
| H                                                                 | -0.081 338 094 557 | 0.030 269 762 774  | 0.028 520 564 729  |

Wavenumber/cm<sup>-1</sup>: 3078.86

| $\frac{\partial \mu_{x,y,z}}{\partial Q_r} / (e \text{ u}^{-0.5})$ | -0.008 225 518 454 | -0.011 730 960 889 | -0.001 709 639 102 |
|--------------------------------------------------------------------|--------------------|--------------------|--------------------|
| <i>l</i> -matrix coefficients/(u <sup>1/2</sup> Å <sup>-1</sup> )  |                    |                    |                    |
| O                                                                  | -0.148 309 498 871 | 0.117 055 245 053  | -0.069 755 724 457 |
| C                                                                  | -0.035 399 503 868 | -0.137 929 677 331 | -0.049 139 913 907 |
| C                                                                  | 0.081 366 344 804  | 0.036 178 669 511  | 0.449 141 833 018  |
| C                                                                  | -0.049 785 303 749 | 0.267 213 061 318  | -0.076 239 956 488 |
| C                                                                  | -0.090 536 940 868 | -0.086 317 345 087 | -0.013 345 033 183 |
| C                                                                  | -0.057 066 876 662 | -0.058 479 903 762 | 0.093 075 901 705  |
| C                                                                  | 0.291 358 415 403  | -0.122 441 406 950 | -0.081 150 431 554 |
| H                                                                  | -0.080 356 975 282 | -0.307 471 256 118 | -0.097 142 294 347 |
| H                                                                  | 0.003 830 217 131  | 0.116 366 559 393  | -0.243 920 606 135 |
| H                                                                  | 0.024 343 116 723  | 0.009 837 555 470  | 0.128 161 363 100  |
| H                                                                  | -0.083 349 791 224 | 0.004 935 682 802  | -0.230 015 722 800 |
| H                                                                  | 0.030 868 827 781  | 0.325 007 146 212  | -0.043 368 149 834 |
| H                                                                  | -0.052 861 275 343 | -0.088 821 372 355 | -0.020 397 618 177 |
| H                                                                  | -0.053 295 059 771 | -0.010 361 635 989 | -0.040 124 368 166 |
| H                                                                  | -0.006 663 053 620 | -0.012 830 863 388 | -0.144 824 936 861 |
| H                                                                  | 0.270 829 216 926  | -0.113 464 366 658 | -0.032 368 787 925 |
| H                                                                  | 0.054 474 691 846  | -0.038 223 929 564 | -0.110 806 579 069 |

Wavenumber/cm<sup>-1</sup>: 3083.8235

| $\frac{\partial \mu_{x,y,z}}{\partial Q_r} / (e \text{ u}^{-0.5})$ | -0.011 643 297 830 | -0.037 608 360 582 | 0.002 297 088 264  |
|--------------------------------------------------------------------|--------------------|--------------------|--------------------|
| <i>l</i> -matrix coefficients/(u <sup>1/2</sup> Å <sup>-1</sup> )  |                    |                    |                    |
| O                                                                  | 0.194 378 819 475  | -0.316 167 099 926 | 0.016 442 284 069  |
| C                                                                  | 0.120 315 278 353  | 0.253 708 350 890  | 0.062 086 162 376  |
| C                                                                  | 0.024 310 425 688  | 0.257 323 560 428  | 0.002 780 755 686  |
| C                                                                  | -0.051 283 978 179 | 0.278 016 126 978  | -0.021 536 238 593 |
| C                                                                  | -0.107 634 097 175 | 0.088 531 860 430  | -0.049 367 359 464 |
| C                                                                  | 0.063 597 169 525  | 0.017 195 591 259  | 0.002 024 775 063  |
| C                                                                  | -0.197 750 453 974 | -0.476 196 207 346 | -0.016 313 563 107 |
| H                                                                  | 0.057 708 450 903  | 0.131 055 679 521  | 0.035 447 202 469  |
| H                                                                  | 0.071 062 032 493  | 0.036 178 817 207  | 0.066 411 539 137  |
| H                                                                  | 0.010 230 146 516  | 0.082 826 903 155  | 0.001 186 333 993  |
| H                                                                  | -0.050 235 337 104 | 0.091 728 625 578  | -0.025 697 816 179 |
| H                                                                  | -0.019 727 692 096 | 0.111 888 281 925  | -0.007 360 740 026 |
| H                                                                  | -0.033 687 254 182 | 0.005 414 712 902  | -0.020 777 477 740 |
| H                                                                  | -0.050 343 559 085 | 0.020 650 256 177  | -0.026 027 477 745 |
| H                                                                  | -0.201 026 321 226 | -0.122 477 590 660 | -0.144 815 639 505 |
| H                                                                  | -0.121 142 380 474 | -0.324 292 047 982 | -0.017 364 884 019 |
| H                                                                  | 0.075 172 852 830  | -0.218 266 682 524 | 0.143 654 730 243  |

Wavenumber/cm<sup>-1</sup>: 3087.2009

| $\frac{\partial \mu_{x,y,z}}{\partial Q_r} / (e \text{ u}^{-0.5})$ | 0.006 981 974 921  | 0.036 021 362 570  | -0.004 979 807 849 |
|--------------------------------------------------------------------|--------------------|--------------------|--------------------|
| <i>l</i> -matrix coefficients/(u <sup>1/2</sup> Å <sup>-1</sup> )  |                    |                    |                    |
| O                                                                  | -0.043 753 127 938 | 0.071 961 208 109  | -0.023 951 671 930 |
| C                                                                  | -0.030 769 777 526 | -0.046 745 812 085 | 0.094 925 368 103  |
| C                                                                  | -0.011 982 319 534 | -0.091 585 291 226 | -0.018 324 414 267 |
| C                                                                  | 0.036 691 174 659  | -0.038 564 164 599 | -0.126 491 591 392 |
| C                                                                  | 0.023 992 830 226  | -0.012 840 867 971 | 0.018 465 061 630  |
| C                                                                  | -0.015 110 146 176 | 0.002 807 602 148  | 0.031 917 833 943  |
| C                                                                  | 0.028 790 759 614  | 0.083 993 956 279  | 0.016 561 814 345  |
| H                                                                  | -0.005 400 744 862 | 0.028 379 576 064  | 0.041 450 964 774  |
| H                                                                  | -0.024 735 809 762 | -0.036 012 940 579 | 0.064 570 467 977  |
| H                                                                  | -0.004 287 500 071 | -0.048 021 672 559 | -0.006 700 674 188 |
| H                                                                  | 0.006 922 592 999  | -0.034 505 423 954 | -0.082 700 458 790 |
| H                                                                  | 0.044 203 120 306  | 0.027 057 051 137  | -0.044 811 927 428 |
| H                                                                  | -0.023 127 672 456 | 0.003 812 309 806  | 0.014 442 830 397  |
| H                                                                  | 0.030 817 633 020  | -0.005 817 217 444 | 0.025 735 829 221  |
| H                                                                  | 0.287 962 284 540  | 0.282 355 967 539  | -0.406 802 761 358 |
| H                                                                  | -0.137 583 717 624 | -0.481 486 657 488 | -0.030 358 846 167 |
| H                                                                  | -0.109 580 073 094 | 0.332 868 084 812  | 0.461 729 604 747  |

Wavenumber/cm<sup>-1</sup>: 3096.9779

| $\frac{\partial \mu_{x,y,z}}{\partial Q_r} / (e \text{ u}^{-0.5})$ | -0.037 805 300 770 | 0.063 689 540 730  | 0.001 368 096 862  |
|--------------------------------------------------------------------|--------------------|--------------------|--------------------|
| <i>l</i> -matrix coefficients/(u <sup>1/2</sup> Å <sup>-1</sup> )  |                    |                    |                    |
| O                                                                  | 0.020 198 747 827  | -0.046 128 777 029 | -0.050 686 908 686 |
| C                                                                  | -0.004 156 451 477 | -0.013 958 255 376 | -0.198 780 069 375 |
| C                                                                  | 0.037 858 914 886  | -0.051 788 230 786 | -0.156 445 125 793 |
| C                                                                  | 0.089 657 247 042  | 0.092 534 351 207  | -0.407 692 855 023 |
| C                                                                  | -0.047 434 336 699 | 0.023 591 973 448  | 0.386 642 354 264  |
| C                                                                  | 0.014 869 999 023  | -0.015 050 106 131 | 0.051 725 662 376  |
| C                                                                  | -0.102 280 569 907 | -0.003 667 550 768 | 0.312 964 758 920  |
| H                                                                  | 0.014 545 878 177  | -0.052 285 431 106 | -0.075 556 893 323 |
| H                                                                  | -0.024 052 723 339 | 0.021 691 707 187  | -0.091 091 201 236 |
| H                                                                  | 0.084 964 986 712  | -0.074 233 739 098 | -0.045 771 968 688 |
| H                                                                  | -0.053 835 546 293 | -0.011 296 622 661 | -0.274 512 627 451 |
| H                                                                  | 0.186 609 342 663  | 0.141 004 648 163  | -0.155 216 329 887 |
| H                                                                  | -0.210 673 663 684 | 0.130 245 977 531  | 0.201 243 960 308  |
| H                                                                  | 0.092 658 271 626  | -0.090 097 033 499 | 0.290 500 234 296  |
| H                                                                  | -0.014 235 541 182 | -0.043 003 162 586 | 0.200 298 061 244  |
| H                                                                  | -0.125 977 381 324 | 0.093 370 991 070  | 0.098 957 393 718  |
| H                                                                  | 0.009 169 641 414  | -0.040 913 872 649 | 0.093 082 224 299  |



Wavenumber/cm<sup>-1</sup>: 3100.0486

| $\frac{\partial \mu_{x,y,z}}{\partial Q_r} / (e u^{-0.5})$        | 0.037 892 077 005  | -0.067 273 218 247 | 0.000 167 128 163  |
|-------------------------------------------------------------------|--------------------|--------------------|--------------------|
| <i>l</i> -matrix coefficients/(u <sup>1/2</sup> Å <sup>-1</sup> ) |                    |                    |                    |
| O                                                                 | -0.021 152 384 603 | -0.026 030 217 988 | -0.554 601 294 238 |
| C                                                                 | 0.004 791 464 662  | 0.035 588 661 438  | 0.491 318 847 896  |
| C                                                                 | -0.078 530 758 153 | -0.060 776 547 687 | 0.054 051 628 947  |
| C                                                                 | 0.047 577 119 861  | 0.018 162 505 041  | -0.037 562 155 438 |
| C                                                                 | -0.007 889 476 543 | 0.014 422 702 871  | 0.249 796 465 606  |
| C                                                                 | -0.003 051 178 973 | -0.009 917 941 840 | 0.062 637 615 941  |
| C                                                                 | 0.053 529 085 171  | 0.005 272 306 003  | -0.272 596 528 604 |
| H                                                                 | 0.013 500 203 773  | 0.170 303 978 083  | 0.195 198 609 920  |
| H                                                                 | 0.017 944 528 775  | -0.080 823 302 905 | 0.270 192 038 695  |
| H                                                                 | -0.110 886 718 011 | -0.069 176 213 038 | 0.010 669 731 555  |
| H                                                                 | -0.010 432 649 059 | -0.015 361 493 382 | -0.074 535 788 918 |
| H                                                                 | 0.080 088 887 031  | 0.045 139 499 802  | -0.025 430 868 498 |
| H                                                                 | -0.075 173 955 453 | 0.065 269 346 157  | 0.111 728 036 237  |
| H                                                                 | 0.035 092 773 878  | -0.041 221 983 821 | 0.146 168 646 930  |
| H                                                                 | -0.026 823 031 015 | -0.022 973 954 177 | -0.050 505 611 655 |
| H                                                                 | 0.111 243 716 941  | 0.062 917 594 569  | -0.075 760 529 691 |
| H                                                                 | -0.006 984 101 637 | -0.019 865 771 001 | -0.188 611 936 701 |

Wavenumber/cm<sup>-1</sup>: 108.8152 , Max excitation: 3

| <i>l'</i> -matrix coefficients/(u <sup>1/2</sup> Å <sup>-1</sup> ) |                    |                    |                                       |
|--------------------------------------------------------------------|--------------------|--------------------|---------------------------------------|
| O                                                                  | 0.000 300 196 849  | -0.000 257 454 849 | -5.601 228 000 000 × 10 <sup>-6</sup> |
| C                                                                  | -0.001 647 792 466 | -0.006 156 537 585 | -0.004 636 066 118                    |
| C                                                                  | 0.001 128 303 587  | 0.003 429 752 769  | 0.017 333 170 945                     |
| C                                                                  | 0.006 143 858 950  | 0.005 195 347 942  | 0.003 087 759 763                     |
| C                                                                  | -0.000 802 029 790 | 0.001 701 761 967  | 0.005 915 745 146                     |
| C                                                                  | -0.000 124 491 257 | -0.000 219 476 738 | -0.000 194 599 231                    |
| C                                                                  | 0.033 476 844 527  | 0.280 370 731 191  | 0.112 147 021 235                     |
| H                                                                  | -0.000 171 591 526 | -0.000 277 469 233 | -0.000 256 476 432                    |
| H                                                                  | -0.000 687 112 862 | 0.019 649 330 925  | 0.017 148 243 363                     |
| H                                                                  | 0.002 020 412 649  | 0.001 469 522 661  | -0.053 428 026 010                    |
| H                                                                  | -0.016 506 569 511 | -0.023 711 279 405 | 0.015 013 282 179                     |
| H                                                                  | -0.003 844 314 558 | -0.002 632 875 360 | -0.027 091 757 365                    |
| H                                                                  | -0.003 857 206 579 | 0.004 437 824 549  | -0.013 549 305 552                    |
| H                                                                  | 0.006 933 533 729  | -0.007 713 603 887 | -0.008 521 929 087                    |
| H                                                                  | 0.203 829 003 912  | -0.712 014 393 187 | -0.283 118 596 983                    |
| H                                                                  | 0.006 645 032 836  | 0.030 628 149 046  | -0.246 910 501 394                    |
| H                                                                  | -0.327 335 542 107 | -0.290 282 391 536 | 0.139 369 555 492                     |

*Final state*

Wavenumber/cm<sup>-1</sup>: 170.3257 , Max excitation: 2

| $l'$ -matrix coefficients/(u <sup>1/2</sup> Å <sup>-1</sup> ) |                    |                    |                    |
|---------------------------------------------------------------|--------------------|--------------------|--------------------|
| O                                                             | -0.000 654 355 801 | -0.000 151 335 696 | -0.000 101 875 408 |
| C                                                             | 0.002 219 487 747  | 0.000 699 132 117  | 0.003 364 881 806  |
| C                                                             | -0.004 331 335 445 | -0.003 924 837 155 | 0.055 120 766 614  |
| C                                                             | -0.014 365 504 525 | -0.034 798 088 088 | 0.060 315 632 442  |
| C                                                             | -0.001 057 745 687 | 0.000 408 134 412  | 0.005 891 680 179  |
| C                                                             | 0.000 741 552 562  | 0.000 197 495 495  | -0.000 490 927 217 |
| C                                                             | -0.134 609 738 771 | -0.084 609 410 139 | 0.243 291 721 880  |
| H                                                             | 0.000 453 591 761  | 0.006 859 972 302  | -0.012 463 089 334 |
| H                                                             | -0.002 059 889 898 | -0.003 918 168 139 | -0.002 478 643 826 |
| H                                                             | 0.005 719 610 265  | 0.008 506 365 175  | -0.173 894 057 552 |
| H                                                             | 0.077 093 327 104  | 0.131 152 917 013  | -0.077 274 450 663 |
| H                                                             | -0.025 695 693 425 | -0.013 329 113 134 | -0.135 313 606 183 |
| H                                                             | -0.004 455 515 632 | 0.005 316 915 415  | -0.011 698 324 406 |
| H                                                             | 0.007 328 521 011  | -0.007 125 449 405 | -0.008 951 886 342 |
| H                                                             | 0.028 099 528 549  | -0.139 681 314 733 | -0.036 535 366 490 |
| H                                                             | 0.001 168 369 958  | 0.025 040 229 500  | -0.649 113 498 798 |
| H                                                             | 0.437 596 531 085  | 0.409 017 536 786  | -0.160 452 937 679 |

Wavenumber/cm<sup>-1</sup>: -233.1903, replaced by 233.1903 , Max excitation: 7

| $l'$ -matrix coefficients/(u <sup>1/2</sup> Å <sup>-1</sup> ) |                    |                    |                    |
|---------------------------------------------------------------|--------------------|--------------------|--------------------|
| O                                                             | -0.001 866 986 676 | -0.000 903 917 376 | -0.000 105 833 194 |
| C                                                             | 0.000 748 782 715  | 0.001 654 199 442  | 0.000 572 158 133  |
| C                                                             | -0.003 311 090 583 | -0.001 717 633 837 | 0.037 245 756 292  |
| C                                                             | -0.068 459 977 962 | -0.150 543 730 578 | 0.244 326 646 330  |
| C                                                             | -0.002 220 999 811 | -0.000 867 711 461 | 0.019 356 052 351  |
| C                                                             | 0.002 291 437 554  | 0.002 002 289 902  | -0.000 907 992 809 |
| C                                                             | 0.029 250 945 867  | 0.024 198 525 609  | -0.069 998 141 900 |
| H                                                             | 0.000 434 759 753  | 0.000 523 943 427  | 0.000 746 403 630  |
| H                                                             | -0.000 536 893 730 | -0.000 964 329 953 | -0.001 390 383 358 |
| H                                                             | 0.007 111 381 239  | 0.003 126 009 108  | -0.121 835 255 438 |
| H                                                             | 0.340 799 071 540  | 0.563 999 090 206  | -0.335 809 071 789 |
| H                                                             | -0.104 110 668 792 | -0.043 510 201 284 | -0.515 113 459 450 |
| H                                                             | -0.012 830 408 311 | 0.016 690 344 890  | -0.036 231 532 665 |
| H                                                             | 0.020 661 059 281  | -0.020 348 349 459 | -0.025 995 057 303 |
| H                                                             | -0.000 700 802 725 | 0.016 161 933 715  | -0.000 139 094 785 |
| H                                                             | -0.002 035 032 319 | -0.006 191 893 798 | 0.204 309 685 465  |
| H                                                             | -0.097 403 487 973 | -0.093 441 494 640 | 0.035 871 480 568  |

Wavenumber/cm<sup>-1</sup>: 235.3464 , Max excitation: 1

| $l'$ -matrix coefficients/(u <sup>1/2</sup> Å <sup>-1</sup> ) |                    |                    |                    |
|---------------------------------------------------------------|--------------------|--------------------|--------------------|
| O                                                             | 0.001 300 423 587  | 0.000 696 944 995  | 0.000 279 177 651  |
| C                                                             | 0.000 460 846 403  | 0.003 596 812 931  | 0.013 224 922 672  |
| C                                                             | -0.000 809 351 493 | -0.003 581 519 062 | 0.059 436 052 472  |
| C                                                             | 0.108 018 044 931  | 0.129 930 072 773  | 0.124 246 751 621  |
| C                                                             | -0.011 926 989 086 | 0.010 869 879 016  | 0.018 831 229 707  |
| C                                                             | -0.001 774 417 160 | -0.001 443 573 251 | -0.001 244 246 116 |
| C                                                             | 0.052 528 531 477  | -0.023 056 671 995 | 0.008 604 761 431  |
| H                                                             | -0.001 561 684 617 | 0.011 782 436 789  | -0.021 585 848 495 |
| H                                                             | -0.003 187 082 875 | -0.026 132 910 534 | -0.023 151 378 424 |
| H                                                             | 0.008 059 258 619  | 0.008 088 319 518  | -0.200 159 175 761 |
| H                                                             | -0.244 560 580 988 | -0.406 192 086 721 | 0.263 486 002 845  |
| H                                                             | -0.124 007 083 224 | -0.037 906 880 954 | -0.690 251 041 230 |
| H                                                             | -0.005 439 962 871 | 0.006 244 309 959  | -0.011 597 692 783 |
| H                                                             | 0.041 441 028 970  | -0.041 336 356 777 | -0.055 798 586 184 |
| H                                                             | -0.053 318 096 755 | 0.199 371 306 537  | 0.078 765 557 199  |
| H                                                             | 0.003 978 848 332  | 0.007 446 234 300  | -0.164 371 847 433 |
| H                                                             | -0.132 289 451 636 | -0.125 658 316 358 | 0.053 416 437 249  |

Wavenumber/cm<sup>-1</sup>: 262.1587 , Max excitation: 2

| $l'$ -matrix coefficients/(u <sup>1/2</sup> Å <sup>-1</sup> ) |                                      |                    |
|---------------------------------------------------------------|--------------------------------------|--------------------|
| O -0.000 798 484 581                                          | 2.589 392 800 000 × 10 <sup>-5</sup> | 0.000 113 608 507  |
| C 0.000 856 529 793                                           | 0.010 923 739 690                    | 0.009 881 529 726  |
| C -0.003 009 258 686                                          | -0.000 400 285 301                   | 0.013 849 823 694  |
| C -0.043 462 109 060                                          | -0.053 071 685 660                   | -0.039 057 184 745 |
| C 0.009 476 876 235                                           | -0.009 049 504 777                   | -0.016 362 384 943 |
| C 0.001 447 568 932                                           | 0.001 210 215 171                    | 0.000 209 311 534  |
| C 0.134 466 080 123                                           | -0.031 085 035 234                   | 0.074 721 465 428  |
| H 0.001 097 373 461                                           | 0.002 077 817 861                    | -0.001 126 039 507 |
| H -0.003 077 603 894                                          | -0.040 109 062 289                   | -0.035 089 352 035 |
| H 0.004 288 194 657                                           | 0.001 866 053 694                    | -0.046 173 439 480 |
| H 0.100 101 624 644                                           | 0.172 115 740 831                    | -0.111 472 075 090 |
| H 0.044 848 469 560                                           | 0.011 151 386 293                    | 0.245 550 307 757  |
| H 0.004 080 647 417                                           | -0.005 558 419 453                   | 0.011 664 738 754  |
| H -0.033 172 733 571                                          | 0.034 830 996 704                    | 0.045 007 734 638  |
| H -0.110 177 173 913                                          | 0.426 947 444 862                    | 0.174 569 253 467  |
| H 0.015 438 504 876                                           | 0.025 421 642 449                    | -0.584 465 775 770 |
| H -0.364 669 929 455                                          | -0.347 604 986 918                   | 0.151 809 491 184  |

Wavenumber/cm<sup>-1</sup>: 367.1634 , Max excitation: 2

| $l'$ -matrix coefficients/(u <sup>1/2</sup> Å <sup>-1</sup> ) |                                      |                    |
|---------------------------------------------------------------|--------------------------------------|--------------------|
| O 0.000 177 886 090                                           | 0.000 216 609 273                    | -0.000 124 579 679 |
| C -0.007 073 184 527                                          | -0.028 096 603 075                   | -0.043 756 988 977 |
| C 0.010 063 092 829                                           | 0.010 758 472 616                    | -0.255 979 611 238 |
| C 0.009 215 273 581                                           | -0.000 507 216 735                   | 0.067 970 082 836  |
| C -0.005 662 099 242                                          | 0.004 825 097 121                    | 0.010 839 563 104  |
| C 0.000 644 328 383                                           | 4.697 865 000 000 × 10 <sup>-6</sup> | 0.001 182 104 705  |
| C 0.000 343 232 087                                           | -0.005 275 581 319                   | 0.048 919 099 096  |
| H 0.005 683 405 765                                           | -0.024 897 142 573                   | 0.045 201 922 676  |
| H 0.016 789 008 713                                           | 0.123 257 903 176                    | 0.104 634 341 287  |
| H -0.034 659 241 849                                          | -0.037 400 702 574                   | 0.893 955 591 911  |
| H 0.013 457 377 203                                           | 0.016 420 493 340                    | -0.006 065 593 783 |
| H -0.046 031 954 664                                          | -0.014 393 373 576                   | -0.233 753 074 827 |
| H -0.001 843 373 807                                          | 0.004 468 719 440                    | -0.009 983 794 784 |
| H 0.022 304 826 397                                           | -0.024 698 961 032                   | -0.029 976 163 025 |
| H -0.005 913 137 984                                          | 0.007 833 240 987                    | 0.005 977 449 834  |
| H 0.004 170 084 930                                           | 0.008 420 420 618                    | -0.183 036 755 200 |
| H -0.000 661 349 758                                          | 0.003 267 072 810                    | 0.003 229 785 831  |

Wavenumber/cm<sup>-1</sup>: 433.1698 , Max excitation: 2

| $l'$ -matrix coefficients/(u <sup>1/2</sup> Å <sup>-1</sup> ) |                                       |                    |                                       |
|---------------------------------------------------------------|---------------------------------------|--------------------|---------------------------------------|
| O                                                             | 0.003 346 033 979                     | 0.001 059 774 557  | -0.000 446 265 040                    |
| C                                                             | -0.016 636 361 183                    | -0.128 886 207 087 | -0.100 044 170 294                    |
| C                                                             | 0.001 269 464 475                     | -0.001 162 325 635 | 0.033 155 452 179                     |
| C                                                             | -0.005 451 149 526                    | -0.005 842 007 385 | -0.025 640 589 094                    |
| C                                                             | -0.107 027 070 146                    | 0.112 441 816 535  | 0.127 493 196 983                     |
| C                                                             | 0.001 402 715 552                     | 0.002 862 221 586  | -4.054 874 600 000 × 10 <sup>-5</sup> |
| C                                                             | 0.008 333 524 265                     | -0.009 094 648 581 | -0.004 033 426 901                    |
| H                                                             | -0.007 229 545 801                    | -0.002 997 618 351 | -0.036 263 907 080                    |
| H                                                             | 0.050 545 149 518                     | 0.447 747 135 795  | 0.389 543 582 850                     |
| H                                                             | 0.004 072 258 510                     | 0.004 165 013 315  | -0.118 677 093 563                    |
| H                                                             | 0.006 562 052 580                     | 0.014 548 721 213  | -0.010 581 156 410                    |
| H                                                             | 0.018 429 793 551                     | 0.006 686 233 310  | 0.101 095 430 218                     |
| H                                                             | -7.302 095 400 000 × 10 <sup>-5</sup> | -0.009 342 555 252 | 0.065 674 669 240                     |
| H                                                             | 0.353 678 748 746                     | -0.394 199 531 142 | -0.510 692 352 558                    |
| H                                                             | -0.014 390 018 872                    | 0.047 893 473 750  | 0.020 419 403 751                     |
| H                                                             | 0.001 577 731 384                     | 0.001 346 097 675  | -0.012 793 581 229                    |
| H                                                             | -0.018 794 328 139                    | -0.017 610 406 547 | 0.007 421 540 291                     |

Wavenumber/cm<sup>-1</sup>: 513.1785 , Max excitation: 1

| $l'$ -matrix coefficients/(u <sup>1/2</sup> Å <sup>-1</sup> ) |                    |                    |                    |
|---------------------------------------------------------------|--------------------|--------------------|--------------------|
| O                                                             | -0.000 454 446 457 | -0.001 142 340 429 | 0.000 152 406 047  |
| C                                                             | 0.024 000 322 497  | 0.153 463 697 228  | 0.135 573 763 092  |
| C                                                             | 0.000 109 876 100  | 0.000 350 070 289  | -0.032 168 403 932 |
| C                                                             | -0.004 669 629 618 | -0.007 630 053 393 | -0.011 150 267 734 |
| C                                                             | -0.084 956 399 640 | 0.086 272 767 776  | 0.121 708 533 280  |
| C                                                             | -0.003 076 168 845 | 0.010 912 969 148  | -0.004 408 631 585 |
| C                                                             | -0.002 873 840 206 | 0.005 742 189 071  | 0.004 161 757 903  |
| H                                                             | 0.005 032 299 200  | 0.015 810 555 709  | 0.016 784 258 722  |
| H                                                             | -0.065 922 843 340 | -0.551 470 019 007 | -0.480 343 207 712 |
| H                                                             | -0.003 695 680 047 | -0.004 400 396 129 | 0.114 733 935 473  |
| H                                                             | 0.010 818 641 323  | 0.017 947 536 543  | -0.010 860 566 176 |
| H                                                             | 0.008 338 041 042  | 0.002 765 425 839  | 0.048 757 648 873  |
| H                                                             | -0.011 444 812 422 | 0.009 168 694 892  | 0.008 989 203 303  |
| H                                                             | 0.294 694 768 746  | -0.324 055 055 040 | -0.421 620 317 746 |
| H                                                             | 0.006 133 795 273  | -0.023 138 933 430 | -0.007 234 772 794 |
| H                                                             | 0.000 641 521 174  | -0.001 747 472 816 | -0.005 859 951 320 |
| H                                                             | 0.003 913 595 108  | 0.003 742 001 520  | -0.001 699 754 514 |

Wavenumber/cm<sup>-1</sup>: 572.2854 , Max excitation: 2

| $l'$ -matrix coefficients/(u <sup>1/2</sup> Å <sup>-1</sup> ) |                    |                    |                    |
|---------------------------------------------------------------|--------------------|--------------------|--------------------|
| O                                                             | -0.004 397 349 905 | -0.001 071 160 619 | 0.000 996 554 375  |
| C                                                             | -0.018 534 115 117 | 0.048 260 233 497  | -0.137 042 903 456 |
| C                                                             | -0.000 478 399 748 | -0.001 670 844 417 | 0.009 424 031 545  |
| C                                                             | -0.000 156 978 798 | 0.006 383 824 997  | -0.013 089 146 805 |
| C                                                             | 0.049 764 322 495  | -0.066 412 184 431 | 0.205 633 591 722  |
| C                                                             | -0.002 056 226 934 | -0.006 865 412 297 | -0.002 779 405 828 |
| C                                                             | 0.001 032 207 033  | -0.005 024 045 250 | -0.000 700 271 401 |
| H                                                             | 0.079 797 923 168  | -0.211 132 331 573 | 0.482 341 616 753  |
| H                                                             | 0.002 750 022 643  | 0.031 995 885 388  | 0.003 685 938 275  |
| H                                                             | 0.000 528 526 904  | 0.000 117 237 696  | -0.040 288 245 438 |
| H                                                             | -0.009 823 124 182 | -0.020 839 260 333 | 0.011 371 462 060  |
| H                                                             | 0.005 211 910 094  | 0.002 866 835 186  | 0.038 497 704 372  |
| H                                                             | -0.185 875 826 547 | 0.299 643 891 954  | -0.717 128 461 557 |
| H                                                             | 0.025 593 331 044  | -0.028 910 260 879 | 0.000 649 593 211  |
| H                                                             | -0.004 385 557 066 | 0.018 045 877 834  | 0.007 667 311 629  |
| H                                                             | 0.001 251 947 362  | 0.001 129 524 784  | -0.003 203 607 634 |
| H                                                             | 0.000 392 347 159  | -0.001 216 539 428 | 0.000 326 224 665  |

Wavenumber/cm<sup>-1</sup>: 780.5396 , Max excitation: 3

| $l'$ -matrix coefficients/(u <sup>1/2</sup> Å <sup>-1</sup> ) |                    |                    |                    |
|---------------------------------------------------------------|--------------------|--------------------|--------------------|
| O                                                             | -0.000 726 653 340 | 0.001 731 825 531  | 0.001 523 829 188  |
| C                                                             | 0.020 671 814 436  | -0.082 113 655 386 | 0.201 627 869 686  |
| C                                                             | 0.002 233 445 091  | 0.000 643 876 267  | -0.011 420 535 987 |
| C                                                             | -0.002 302 204 724 | 0.000 731 857 841  | -0.008 128 729 941 |
| C                                                             | 0.036 655 182 550  | -0.044 447 624 714 | 0.136 009 184 823  |
| C                                                             | 0.008 798 072 376  | -0.020 592 387 924 | -0.007 240 535 970 |
| C                                                             | 0.001 919 701 579  | -0.000 114 179 099 | -0.002 435 471 348 |
| H                                                             | -0.112 819 363 121 | 0.311 888 517 997  | -0.728 691 347 009 |
| H                                                             | 0.002 355 870 911  | 0.001 350 717 501  | 0.037 860 411 171  |
| H                                                             | 0.001 225 926 508  | -0.002 429 716 075 | 0.047 645 315 449  |
| H                                                             | -0.000 252 519 264 | -0.002 741 670 251 | 0.000 182 143 302  |
| H                                                             | 0.004 355 991 559  | -0.000 206 592 114 | 0.029 496 500 966  |
| H                                                             | -0.125 270 179 436 | 0.193 838 993 749  | -0.479 812 584 784 |
| H                                                             | 0.006 332 508 487  | -0.006 229 958 026 | 0.018 001 951 492  |
| H                                                             | -0.002 407 069 630 | 0.005 415 873 158  | 0.003 001 348 330  |
| H                                                             | -0.002 477 340 849 | -0.002 592 930 084 | 0.003 532 330 513  |
| H                                                             | -0.002 800 731 209 | -0.001 576 054 395 | -0.001 918 969 765 |

Wavenumber/cm<sup>-1</sup>: 819.0758 , Max excitation: 1

| $l'$ -matrix coefficients/(u <sup>1/2</sup> Å <sup>-1</sup> ) |                    |                    |
|---------------------------------------------------------------|--------------------|--------------------|
| O                                                             | -0.006 424 067 283 | -0.002 135 422 666 |
| C                                                             | -0.009 636 257 971 | -0.078 621 836 153 |
| C                                                             | -0.010 673 561 709 | -0.018 003 130 845 |
| C                                                             | 0.077 325 261 542  | 0.098 537 585 351  |
| C                                                             | -0.025 059 919 939 | 0.034 148 953 426  |
| C                                                             | 0.015 662 856 682  | -0.010 057 975 016 |
| C                                                             | -0.051 295 532 743 | -0.018 780 457 205 |
| H                                                             | 0.021 120 878 541  | 0.201 217 575 288  |
| H                                                             | -0.036 308 002 323 | 0.136 459 848 973  |
| H                                                             | 0.029 475 878 029  | -0.001 934 857 255 |
| H                                                             | -0.117 803 285 749 | -0.070 451 504 040 |
| H                                                             | -0.149 066 411 005 | -0.271 050 842 668 |
| H                                                             | 0.039 487 665 545  | -0.060 240 913 872 |
| H                                                             | 0.035 464 072 656  | -0.043 972 299 128 |
| H                                                             | 0.313 686 577 231  | 0.244 783 671 409  |
| H                                                             | -0.290 196 207 785 | 0.191 719 338 328  |
| H                                                             | 0.192 426 301 522  | -0.342 956 468 403 |

Wavenumber/cm<sup>-1</sup>: 849.6265 , Max excitation: 1

| $l'$ -matrix coefficients/(u <sup>1/2</sup> Å <sup>-1</sup> ) |                    |                    |
|---------------------------------------------------------------|--------------------|--------------------|
| O                                                             | -0.004 447 858 498 | -0.001 975 268 952 |
| C                                                             | -0.012 796 162 490 | -0.066 117 616 931 |
| C                                                             | 0.075 921 899 789  | 0.057 604 365 126  |
| C                                                             | 0.082 036 713 780  | 0.113 558 330 017  |
| C                                                             | -0.056 117 765 914 | 0.061 143 567 581  |
| C                                                             | 0.001 705 145 210  | 0.009 005 573 973  |
| C                                                             | 0.043 200 347 113  | 0.115 472 105 649  |
| H                                                             | 0.012 450 349 922  | 0.121 506 278 741  |
| H                                                             | -0.024 151 309 922 | 0.082 221 381 835  |
| H                                                             | -0.056 507 131 420 | -0.030 539 258 390 |
| H                                                             | -0.102 560 447 881 | -0.121 731 292 029 |
| H                                                             | -0.211 136 917 517 | -0.303 681 715 821 |
| H                                                             | 0.110 715 692 167  | -0.136 301 666 487 |
| H                                                             | 0.072 321 865 595  | -0.105 969 575 215 |
| H                                                             | -0.053 544 101 797 | -0.162 397 890 886 |
| H                                                             | -0.009 758 921 026 | -0.487 449 042 066 |
| H                                                             | -0.182 502 023 496 | 0.148 837 556 611  |

 $1.703\,063\,600\,000 \times 10^{-5}$

Wavenumber/cm<sup>-1</sup>: 910.2669 , Max excitation: 1

| $l'$ -matrix coefficients/(u <sup>1/2</sup> Å <sup>-1</sup> ) |                    |                    |                    |
|---------------------------------------------------------------|--------------------|--------------------|--------------------|
| O                                                             | 0.008 707 428 062  | 0.002 437 376 356  | -0.001 026 482 218 |
| C                                                             | -0.012 709 300 009 | -0.045 612 355 298 | 0.019 953 575 083  |
| C                                                             | 0.041 083 663 859  | -0.099 475 866 364 | -0.037 258 971 031 |
| C                                                             | 0.048 205 882 851  | 0.114 338 501 745  | 0.052 309 626 001  |
| C                                                             | -0.055 696 147 421 | 0.046 812 939 318  | -0.014 828 517 201 |
| C                                                             | -0.015 820 201 069 | 0.001 769 792 194  | 0.000 506 114 095  |
| C                                                             | -0.004 368 603 452 | -0.123 063 959 544 | -0.068 805 561 969 |
| H                                                             | 0.008 234 298 127  | 0.127 520 702 111  | 0.055 689 035 639  |
| H                                                             | 0.006 540 741 199  | 0.094 957 415 448  | -0.117 953 287 146 |
| H                                                             | -0.044 343 608 390 | 0.059 867 512 038  | -0.010 954 692 236 |
| H                                                             | -0.071 047 318 722 | -0.066 891 530 005 | -0.224 274 122 757 |
| H                                                             | -0.116 861 554 724 | -0.213 340 636 195 | 0.052 347 578 927  |
| H                                                             | 0.104 551 140 002  | -0.126 875 373 737 | -0.085 757 348 694 |
| H                                                             | 0.089 291 648 052  | -0.096 138 575 009 | 0.146 739 371 584  |
| H                                                             | -0.316 801 479 080 | -0.050 376 044 001 | -0.162 493 173 411 |
| H                                                             | 0.308 078 186 235  | 0.424 470 566 438  | 0.014 058 817 048  |
| H                                                             | -0.004 733 287 077 | 0.200 350 573 392  | 0.502 809 663 718  |

Wavenumber/cm<sup>-1</sup>: 924.6567 , Max excitation: 1

| $l'$ -matrix coefficients/(u <sup>1/2</sup> Å <sup>-1</sup> ) |                    |                    |                    |
|---------------------------------------------------------------|--------------------|--------------------|--------------------|
| O                                                             | 0.026 656 917 546  | 0.012 494 559 580  | -0.000 928 315 835 |
| C                                                             | -0.009 482 106 294 | -0.024 102 591 272 | 0.006 440 340 686  |
| C                                                             | 0.016 904 691 962  | 0.000 960 769 934  | -0.004 253 821 532 |
| C                                                             | 0.055 121 146 457  | 0.053 468 043 223  | 0.046 039 353 867  |
| C                                                             | 0.179 533 055 252  | -0.137 083 216 190 | 0.052 940 266 420  |
| C                                                             | -0.022 713 672 382 | -0.083 749 906 339 | 0.009 758 680 222  |
| C                                                             | 0.017 523 370 041  | -0.008 705 762 544 | -0.023 490 965 695 |
| H                                                             | 0.002 987 221 426  | 0.088 276 701 374  | 0.036 999 651 862  |
| H                                                             | -0.013 404 328 860 | 0.062 492 602 782  | -0.072 940 899 009 |
| H                                                             | 0.000 985 527 017  | -0.015 915 989 337 | -0.000 199 759 226 |
| H                                                             | -0.089 713 313 135 | -0.075 672 964 113 | -0.226 542 125 499 |
| H                                                             | -0.152 608 006 674 | -0.205 458 613 175 | 0.055 040 809 146  |
| H                                                             | -0.353 241 380 651 | 0.406 569 053 064  | 0.278 766 785 251  |
| H                                                             | -0.249 748 388 184 | 0.338 163 248 856  | -0.460 085 934 021 |
| H                                                             | -0.073 610 948 284 | -0.038 465 907 368 | 0.030 164 912 853  |
| H                                                             | 0.037 664 115 901  | 0.010 346 744 609  | -0.002 923 687 049 |
| H                                                             | -0.033 241 614 434 | 0.067 564 278 391  | 0.063 598 661 222  |



Wavenumber/cm<sup>-1</sup>: 957.0445 , Max excitation: 1

| $l'$ -matrix coefficients/(u <sup>1/2</sup> Å <sup>-1</sup> ) |                    |                    |                    |
|---------------------------------------------------------------|--------------------|--------------------|--------------------|
| O                                                             | -0.007 881 005 673 | 0.000 477 382 959  | 0.000 758 508 039  |
| C                                                             | -0.031 420 309 166 | -0.217 554 892 358 | 0.065 991 956 968  |
| C                                                             | 0.029 792 496 747  | -0.023 348 745 147 | -0.014 861 705 489 |
| C                                                             | -0.083 214 165 600 | -0.087 005 160 414 | -0.055 076 677 977 |
| C                                                             | 0.004 752 858 854  | -0.001 045 927 908 | -0.004 538 902 104 |
| C                                                             | 0.037 998 618 165  | -0.053 467 454 289 | 0.010 345 818 140  |
| C                                                             | 0.014 773 248 357  | 0.013 828 085 465  | -0.004 246 384 430 |
| H                                                             | 0.019 020 133 706  | 0.537 890 114 426  | 0.247 475 000 669  |
| H                                                             | -0.065 567 981 125 | 0.392 116 615 683  | -0.468 580 387 421 |
| H                                                             | -0.003 370 050 367 | 0.030 114 172 239  | -0.002 913 842 715 |
| H                                                             | 0.102 767 692 136  | 0.079 463 252 435  | 0.265 123 573 757  |
| H                                                             | 0.171 158 285 889  | 0.242 119 957 654  | -0.062 715 866 420 |
| H                                                             | -0.008 684 639 154 | 0.022 947 684 881  | 0.008 408 438 786  |
| H                                                             | -0.009 833 281 361 | 0.014 735 212 408  | -0.018 321 745 140 |
| H                                                             | -0.043 045 509 874 | -0.031 464 151 055 | 0.054 405 514 892  |
| H                                                             | 0.004 203 904 986  | -0.061 269 545 479 | -0.003 618 371 602 |
| H                                                             | -0.040 951 340 335 | 0.043 824 845 956  | -0.014 048 205 833 |

Wavenumber/cm<sup>-1</sup>: 988.1871 , Max excitation: 1

| $l'$ -matrix coefficients/(u <sup>1/2</sup> Å <sup>-1</sup> ) |                    |                    |                    |
|---------------------------------------------------------------|--------------------|--------------------|--------------------|
| O                                                             | 0.052 740 905 535  | 0.019 494 296 033  | -0.004 121 660 832 |
| C                                                             | 0.015 476 228 925  | -0.003 201 404 305 | -0.005 191 611 169 |
| C                                                             | 0.055 607 479 130  | -0.018 385 487 054 | 0.015 790 436 084  |
| C                                                             | 0.023 205 475 171  | -0.008 870 285 954 | -0.013 226 408 948 |
| C                                                             | -0.000 451 440 083 | 0.009 046 661 164  | 0.008 812 713 406  |
| C                                                             | -0.079 094 039 798 | -0.036 082 120 604 | 0.008 733 545 890  |
| C                                                             | -0.401 297 218 180 | 0.120 216 135 365  | -0.145 918 481 778 |
| H                                                             | -0.009 587 824 203 | 0.031 655 618 427  | 0.010 435 846 556  |
| H                                                             | -0.022 421 037 770 | 0.019 877 813 716  | -0.019 032 784 892 |
| H                                                             | -0.034 627 969 603 | 0.005 103 672 715  | 0.004 930 934 639  |
| H                                                             | -0.018 186 688 731 | 0.010 658 338 622  | -0.003 983 151 392 |
| H                                                             | -0.035 178 203 643 | 0.001 679 555 583  | 0.002 097 169 953  |
| H                                                             | 0.005 927 435 900  | 0.008 493 877 274  | 0.002 726 951 123  |
| H                                                             | -0.016 611 253 503 | -0.000 336 792 238 | -0.005 723 136 830 |
| H                                                             | 0.427 181 328 851  | 0.059 441 715 819  | 0.253 727 503 518  |
| H                                                             | 0.498 931 894 404  | -0.128 531 361 965 | -0.032 103 488 453 |
| H                                                             | 0.328 824 015 934  | -0.302 229 644 940 | 0.255 554 124 509  |

Wavenumber/cm<sup>-1</sup>: 1040.0914 , Max excitation: 2

| $l'$ -matrix coefficients/(u <sup>1/2</sup> Å <sup>-1</sup> ) |                    |                    |                    |
|---------------------------------------------------------------|--------------------|--------------------|--------------------|
| O                                                             | 0.407 035 994 253  | 0.149 440 569 544  | -0.028 342 210 859 |
| C                                                             | -0.040 496 200 868 | 0.032 920 849 828  | -0.018 202 718 547 |
| C                                                             | 0.304 831 140 829  | -0.168 871 994 421 | 0.022 668 183 900  |
| C                                                             | -0.107 816 852 528 | 0.139 580 561 907  | -0.045 516 782 399 |
| C                                                             | 0.005 049 747 329  | -0.022 625 870 475 | -0.004 188 906 380 |
| C                                                             | -0.592 464 020 876 | -0.209 293 222 977 | 0.041 603 048 086  |
| C                                                             | -0.031 099 183 342 | 0.037 570 937 452  | 0.082 797 821 806  |
| H                                                             | 0.091 206 671 293  | -0.012 942 937 189 | -0.031 026 706 023 |
| H                                                             | 0.030 113 308 792  | -0.015 238 969 564 | 0.014 028 529 596  |
| H                                                             | -0.342 829 786 499 | 0.186 468 125 465  | -0.000 476 993 492 |
| H                                                             | 0.145 809 665 547  | -0.025 540 834 829 | 0.040 541 828 246  |
| H                                                             | 0.139 900 126 405  | -0.093 606 076 899 | -0.034 985 254 179 |
| H                                                             | 0.045 105 999 351  | 0.032 617 710 453  | 0.004 480 983 121  |
| H                                                             | 0.018 559 166 242  | -0.004 698 613 983 | 0.007 930 551 790  |
| H                                                             | -0.067 923 110 039 | 0.031 874 953 721  | -0.074 447 908 201 |
| H                                                             | -0.038 117 060 490 | -0.031 476 554 354 | 0.016 693 145 571  |
| H                                                             | -0.048 689 336 085 | -0.004 482 372 609 | -0.103 081 650 016 |

Wavenumber/cm<sup>-1</sup>: 1056.1927 , Max excitation: 1

| $l'$ -matrix coefficients/(u <sup>1/2</sup> Å <sup>-1</sup> ) |                    |                    |                    |
|---------------------------------------------------------------|--------------------|--------------------|--------------------|
| O                                                             | -0.307 681 807 526 | -0.115 460 536 511 | 0.022 715 433 708  |
| C                                                             | -0.148 193 725 978 | 0.015 967 289 234  | 0.005 833 508 502  |
| C                                                             | 0.268 041 699 738  | -0.178 426 364 170 | 0.008 073 947 504  |
| C                                                             | -0.191 266 245 999 | 0.113 197 759 008  | -0.023 036 096 804 |
| C                                                             | -0.032 697 635 578 | -0.069 463 719 231 | -0.024 960 407 382 |
| C                                                             | 0.460 137 393 638  | 0.187 304 373 390  | -0.033 818 844 051 |
| C                                                             | -0.090 738 405 521 | 0.036 967 181 861  | 0.089 637 941 525  |
| H                                                             | 0.102 839 998 664  | -0.029 726 675 483 | -0.033 077 691 652 |
| H                                                             | 0.157 856 189 832  | -0.026 036 393 806 | 0.008 450 480 183  |
| H                                                             | -0.387 185 249 898 | 0.315 115 113 760  | -0.000 434 294 279 |
| H                                                             | 0.071 493 969 376  | -0.041 509 528 448 | -0.000 909 412 657 |
| H                                                             | 0.261 159 423 440  | -0.199 816 767 904 | -0.050 828 577 074 |
| H                                                             | -0.034 912 950 583 | 0.038 028 937 274  | 0.021 475 556 499  |
| H                                                             | 0.077 904 487 669  | 0.094 927 057 491  | -0.032 447 255 749 |
| H                                                             | -0.006 677 813 629 | 0.036 969 011 849  | -0.036 872 414 565 |
| H                                                             | 0.085 005 387 068  | -0.055 488 971 178 | 0.022 256 025 272  |
| H                                                             | -0.017 406 875 844 | -0.036 802 437 130 | -0.063 124 253 728 |

Wavenumber/cm<sup>-1</sup>: 1078.9385 , Max excitation: 1

| $l'$ -matrix coefficients/(u <sup>1/2</sup> Å <sup>-1</sup> ) |                    |                    |                    |
|---------------------------------------------------------------|--------------------|--------------------|--------------------|
| O                                                             | -0.045 185 829 110 | -0.018 222 211 556 | 0.004 354 794 810  |
| C                                                             | -0.067 488 404 657 | -0.047 335 778 497 | -0.116 909 286 289 |
| C                                                             | 0.270 183 397 908  | 0.316 501 474 334  | -0.025 620 251 728 |
| C                                                             | -0.002 532 706 555 | -0.110 369 079 973 | 0.071 199 959 019  |
| C                                                             | 0.014 157 703 727  | 0.021 813 545 793  | 0.035 886 185 655  |
| C                                                             | 0.051 684 606 145  | 0.042 799 226 647  | -0.008 039 501 686 |
| C                                                             | -0.066 159 792 996 | -0.089 530 245 124 | 0.083 052 714 667  |
| H                                                             | 0.146 641 511 840  | 0.066 577 575 521  | -0.024 942 673 067 |
| H                                                             | -0.050 224 965 147 | -0.055 863 649 000 | 0.019 269 411 325  |
| H                                                             | -0.487 309 575 971 | -0.600 319 363 266 | -0.058 824 220 332 |
| H                                                             | 0.081 266 855 961  | -0.106 087 681 015 | -0.025 836 522 765 |
| H                                                             | -0.168 010 575 392 | 0.197 958 343 972  | 0.036 115 560 710  |
| H                                                             | -0.007 462 557 641 | -0.028 548 693 821 | -0.001 030 434 336 |
| H                                                             | -0.054 962 140 428 | -0.023 549 788 252 | -0.007 998 165 358 |
| H                                                             | 0.041 998 166 201  | 0.040 047 218 712  | -0.086 277 384 989 |
| H                                                             | 0.076 989 903 526  | 0.084 939 930 568  | 0.025 207 726 286  |
| H                                                             | -0.088 763 283 658 | 0.035 296 494 177  | -0.029 627 443 733 |

Wavenumber/cm<sup>-1</sup>: 1106.6913 , Max excitation: 1

| $l'$ -matrix coefficients/(u <sup>1/2</sup> Å <sup>-1</sup> ) |                    |                    |                    |
|---------------------------------------------------------------|--------------------|--------------------|--------------------|
| O                                                             | 0.044 597 252 610  | 0.019 534 474 249  | -0.003 405 268 031 |
| C                                                             | -0.067 724 595 287 | -0.017 121 678 455 | -0.000 777 173 717 |
| C                                                             | -0.035 767 152 904 | 0.149 505 608 323  | 0.059 115 785 094  |
| C                                                             | -0.290 747 323 612 | 0.219 309 573 318  | 0.166 733 133 264  |
| C                                                             | -0.067 865 637 082 | -0.160 320 167 464 | -0.089 477 923 754 |
| C                                                             | -0.033 665 181 529 | 0.004 630 623 251  | -0.007 435 063 620 |
| C                                                             | 0.007 813 817 032  | -0.043 906 210 875 | -0.139 894 588 608 |
| H                                                             | 0.105 608 600 046  | 0.012 764 961 295  | -0.011 674 702 326 |
| H                                                             | 0.052 558 653 332  | -0.001 911 562 441 | -0.011 679 925 793 |
| H                                                             | 0.317 980 776 864  | -0.354 929 958 525 | 0.013 395 253 486  |
| H                                                             | 0.330 957 041 943  | -0.262 136 307 155 | -0.074 552 449 128 |
| H                                                             | 0.401 518 258 611  | -0.207 092 068 597 | -0.025 053 075 933 |
| H                                                             | -0.003 057 803 969 | 0.050 847 397 263  | 0.012 589 384 056  |
| H                                                             | 0.250 504 943 730  | 0.127 843 519 394  | 0.030 123 317 673  |
| H                                                             | 0.090 874 797 042  | -0.033 201 946 838 | 0.077 677 456 207  |
| H                                                             | -0.069 121 020 048 | 0.053 957 110 595  | -0.034 072 380 917 |
| H                                                             | 0.028 912 196 787  | 0.010 993 295 901  | 0.077 325 858 469  |

Wavenumber/cm<sup>-1</sup>: 1134.5688 , Max excitation: 1

| $l'$ -matrix coefficients/(u <sup>1/2</sup> Å <sup>-1</sup> ) |                    |                    |                    |
|---------------------------------------------------------------|--------------------|--------------------|--------------------|
| O                                                             | -0.019 278 011 839 | -0.020 339 433 940 | 0.003 567 505 355  |
| C                                                             | 0.123 167 392 149  | -0.033 253 407 071 | -0.056 906 690 071 |
| C                                                             | 0.009 534 585 074  | 0.118 156 836 813  | 0.154 181 504 456  |
| C                                                             | -0.110 409 796 338 | -0.090 268 972 695 | 0.033 892 068 602  |
| C                                                             | 0.309 823 710 079  | 0.228 891 092 162  | -0.092 464 369 337 |
| C                                                             | -0.074 304 790 391 | 0.067 311 720 518  | -0.013 238 336 575 |
| C                                                             | -0.004 449 595 487 | -0.060 454 946 691 | -0.044 838 033 197 |
| H                                                             | -0.052 815 911 755 | 0.028 388 160 692  | 0.015 768 473 319  |
| H                                                             | -0.169 832 137 347 | -0.024 609 722 444 | 0.031 368 146 312  |
| H                                                             | -0.062 590 051 864 | -0.020 568 314 679 | 0.042 544 077 931  |
| H                                                             | -0.198 850 473 093 | 0.063 125 682 828  | -0.008 815 405 286 |
| H                                                             | 0.390 065 013 474  | -0.235 839 247 265 | -0.057 879 591 901 |
| H                                                             | -0.454 839 879 439 | -0.317 536 171 706 | -0.041 231 039 777 |
| H                                                             | -0.243 168 984 241 | -0.270 158 096 132 | 0.002 661 586 872  |
| H                                                             | 0.050 813 140 479  | -0.019 252 065 904 | 0.042 372 760 084  |
| H                                                             | -0.021 490 326 631 | 0.042 160 422 139  | -0.005 650 299 485 |
| H                                                             | -0.035 084 543 009 | 0.040 047 706 814  | 0.031 526 263 309  |

Wavenumber/cm<sup>-1</sup>: 1193.2746 , Max excitation: 1

| $l'$ -matrix coefficients/(u <sup>1/2</sup> Å <sup>-1</sup> ) |                    |                    |                    |
|---------------------------------------------------------------|--------------------|--------------------|--------------------|
| O                                                             | 0.060 998 224 546  | -0.004 238 427 582 | -0.002 747 824 352 |
| C                                                             | -0.407 044 706 879 | -0.030 714 805 113 | 0.071 760 567 834  |
| C                                                             | 0.030 303 093 990  | -0.116 779 652 430 | 0.017 874 901 848  |
| C                                                             | 0.037 455 963 903  | -0.058 865 151 073 | 0.026 514 354 564  |
| C                                                             | 0.114 334 451 707  | 0.064 814 895 351  | 0.017 086 113 227  |
| C                                                             | -0.077 010 713 986 | 0.147 782 911 743  | -0.023 192 262 861 |
| C                                                             | 0.012 074 737 316  | 0.066 090 879 942  | -0.077 440 280 899 |
| H                                                             | 0.546 495 144 772  | -0.008 512 079 391 | -0.082 786 911 267 |
| H                                                             | 0.528 449 291 564  | 0.000 829 355 242  | -0.077 246 165 967 |
| H                                                             | 0.192 555 057 216  | -0.050 072 577 006 | 0.011 248 880 118  |
| H                                                             | -0.090 145 394 600 | 0.041 929 494 480  | 0.003 604 032 405  |
| H                                                             | -0.099 578 131 742 | 0.093 138 264 449  | 0.021 301 848 944  |
| H                                                             | -0.137 839 110 211 | -0.130 818 104 158 | -0.010 134 021 761 |
| H                                                             | -0.148 940 481 680 | -0.126 089 188 492 | -0.009 580 997 997 |
| H                                                             | -0.030 223 116 746 | -0.012 802 193 447 | 0.025 099 528 321  |
| H                                                             | -0.069 571 800 504 | -0.016 191 857 642 | -0.021 864 920 036 |
| H                                                             | 0.066 461 975 058  | -0.024 203 539 001 | 0.038 759 958 786  |

Wavenumber/cm<sup>-1</sup>: 1223.0983 , Max excitation: 1

| $l'$ -matrix coefficients/(u <sup>1/2</sup> Å <sup>-1</sup> ) |                    |                    |
|---------------------------------------------------------------|--------------------|--------------------|
| O -0.025 270 813 930                                          | -0.013 172 381 187 | -0.000 993 176 980 |
| C 0.029 517 485 274                                           | 0.015 157 052 385  | 0.162 472 640 115  |
| C 0.081 983 010 163                                           | -0.005 390 620 864 | -0.394 122 981 611 |
| C -0.214 729 868 060                                          | 0.047 275 496 153  | 0.126 694 775 106  |
| C 0.216 579 093 388                                           | 0.040 240 557 561  | 0.068 010 778 006  |
| C -0.027 513 611 269                                          | 0.049 268 329 355  | 0.011 117 588 950  |
| C -0.043 257 280 133                                          | -0.016 550 230 103 | 0.137 435 316 107  |
| H -0.338 819 360 201                                          | -0.109 868 943 431 | 0.046 082 337 360  |
| H 0.173 199 314 911                                           | 0.072 326 230 326  | -0.060 485 116 092 |
| H 0.150 086 750 405                                           | 0.120 808 899 834  | -0.106 985 938 381 |
| H 0.341 044 812 039                                           | -0.321 663 488 312 | -0.118 246 219 045 |
| H -0.160 228 028 566                                          | 0.185 815 104 959  | 0.038 241 744 651  |
| H -0.168 884 191 632                                          | -0.191 942 300 468 | -0.003 322 218 110 |
| H -0.149 214 875 372                                          | -0.144 447 368 785 | -0.009 623 961 050 |
| H 0.010 468 673 409                                           | 0.049 250 072 019  | -0.091 988 844 249 |
| H 0.142 865 396 459                                           | -0.033 640 595 102 | 0.030 258 233 175  |
| H -0.046 818 890 630                                          | -0.022 917 437 506 | -0.105 242 304 617 |

Wavenumber/cm<sup>-1</sup>: 1265.4316 , Max excitation: 1

| $l'$ -matrix coefficients/(u <sup>1/2</sup> Å <sup>-1</sup> ) |                    |                    |
|---------------------------------------------------------------|--------------------|--------------------|
| O -0.045 190 452 186                                          | -0.016 809 663 659 | 0.000 914 542 082  |
| C -0.047 158 602 102                                          | -0.066 096 442 159 | 0.010 111 273 212  |
| C 0.125 783 326 705                                           | 0.219 782 657 873  | 0.248 361 137 886  |
| C -0.138 312 638 153                                          | -0.043 406 780 746 | -0.364 906 154 832 |
| C 0.076 903 028 701                                           | 0.014 780 186 858  | 0.202 839 240 146  |
| C 0.039 014 633 543                                           | 0.040 406 765 963  | 0.013 307 702 764  |
| C -0.035 253 760 573                                          | -0.146 145 048 438 | -0.157 081 207 804 |
| H 0.091 563 414 545                                           | 0.010 476 578 387  | 0.000 970 962 073  |
| H -0.109 313 959 873                                          | -0.034 505 809 786 | 0.035 327 784 335  |
| H 0.100 970 652 487                                           | 0.218 758 736 802  | 0.078 599 923 590  |
| H 0.297 598 494 576                                           | -0.135 071 838 489 | 0.035 953 241 782  |
| H -0.184 393 416 102                                          | -0.143 771 260 120 | -0.067 282 639 428 |
| H 0.308 746 416 938                                           | 0.077 997 760 723  | 0.010 004 880 779  |
| H -0.346 823 910 717                                          | -0.186 394 240 263 | -0.059 652 459 538 |
| H 0.168 193 699 330                                           | -0.041 698 596 405 | 0.100 133 427 553  |
| H -0.130 864 882 507                                          | 0.145 008 316 252  | -0.033 514 790 953 |
| H -0.088 042 862 584                                          | 0.089 474 485 851  | 0.059 329 562 757  |

Wavenumber/cm<sup>-1</sup>: 1296.8741 , Max excitation: 1

| $l'$ -matrix coefficients/(u <sup>1/2</sup> Å <sup>-1</sup> ) |                    |                    |                    |
|---------------------------------------------------------------|--------------------|--------------------|--------------------|
| O                                                             | -0.102 380 566 295 | -0.040 905 585 907 | 0.007 593 494 433  |
| C                                                             | 0.228 135 261 890  | 0.131 790 358 627  | -0.147 718 023 211 |
| C                                                             | -0.104 576 811 741 | -0.431 454 126 185 | 0.125 640 268 303  |
| C                                                             | -0.126 313 722 010 | 0.229 390 251 451  | -0.012 501 261 653 |
| C                                                             | 0.166 762 420 589  | -0.105 688 544 069 | 0.095 674 363 483  |
| C                                                             | 0.014 281 479 603  | 0.148 719 429 792  | -0.036 730 316 181 |
| C                                                             | 0.070 276 071 032  | 0.252 270 489 173  | -0.078 951 481 631 |
| H                                                             | 0.123 489 780 252  | 0.081 567 765 979  | -0.034 098 183 488 |
| H                                                             | -0.249 353 550 452 | 0.018 951 625 190  | 0.030 775 589 687  |
| H                                                             | -0.086 818 460 127 | -0.210 391 342 065 | 0.029 997 745 405  |
| H                                                             | 0.217 213 733 292  | -0.059 719 522 860 | 0.049 416 468 512  |
| H                                                             | -0.175 065 625 211 | 0.055 535 059 459  | 0.025 762 386 084  |
| H                                                             | -0.009 550 016 563 | -0.093 817 444 729 | 0.012 726 015 878  |
| H                                                             | -0.122 765 067 697 | -0.122 273 539 687 | -0.019 557 121 002 |
| H                                                             | -0.258 626 718 838 | -0.018 054 088 986 | -0.007 591 870 185 |
| H                                                             | -0.146 271 664 604 | -0.117 927 861 988 | -0.030 910 526 498 |
| H                                                             | 0.257 599 143 320  | -0.147 691 589 379 | 0.101 657 839 422  |

Wavenumber/cm<sup>-1</sup>: 1311.8062 , Max excitation: 1

| $l'$ -matrix coefficients/(u <sup>1/2</sup> Å <sup>-1</sup> ) |                    |                    |                    |
|---------------------------------------------------------------|--------------------|--------------------|--------------------|
| O                                                             | -0.042 391 772 052 | -0.008 894 330 762 | 0.001 800 115 948  |
| C                                                             | -0.197 717 233 363 | 0.203 066 052 753  | -0.046 955 070 352 |
| C                                                             | 0.417 576 035 486  | -0.187 754 209 814 | 0.094 250 013 239  |
| C                                                             | -0.131 650 171 647 | -0.018 023 720 552 | 0.065 066 075 935  |
| C                                                             | 0.072 191 916 360  | 0.305 688 369 749  | -0.027 287 016 525 |
| C                                                             | 0.189 192 839 298  | -0.424 478 512 025 | 0.096 423 769 355  |
| C                                                             | -0.160 324 837 882 | 0.107 696 699 552  | -0.218 291 525 865 |
| H                                                             | -0.308 485 411 094 | 0.031 666 612 416  | 0.032 445 019 524  |
| H                                                             | 0.067 321 353 609  | -0.014 173 046 961 | 0.040 016 965 552  |
| H                                                             | 0.153 965 939 224  | -0.161 089 956 011 | 0.023 333 812 583  |
| H                                                             | -0.138 907 085 477 | 0.038 043 267 675  | -0.016 905 327 768 |
| H                                                             | -0.019 007 984 189 | 0.077 143 162 231  | 0.009 099 396 396  |
| H                                                             | 0.068 787 136 338  | 0.080 780 078 052  | -0.006 656 530 160 |
| H                                                             | -0.010 594 837 727 | -0.000 549 700 594 | 0.027 340 676 542  |
| H                                                             | -0.083 651 377 330 | -0.012 594 622 100 | 0.024 822 382 693  |
| H                                                             | -0.236 230 862 297 | 0.043 392 096 879  | -0.062 386 427 471 |
| H                                                             | 0.022 343 761 975  | 0.000 473 547 235  | 0.048 729 594 621  |

Wavenumber/cm<sup>-1</sup>: 1341.7992 , Max excitation: 1

| $l'$ -matrix coefficients/(u <sup>1/2</sup> Å <sup>-1</sup> ) |                    |                    |                    |
|---------------------------------------------------------------|--------------------|--------------------|--------------------|
| O                                                             | -0.008 910 054 594 | -0.005 593 909 394 | -0.000 192 393 654 |
| C                                                             | 0.105 190 089 023  | -0.174 569 815 889 | 0.045 088 400 310  |
| C                                                             | 0.393 880 605 950  | -0.043 391 802 048 | 0.115 607 116 874  |
| C                                                             | 0.100 615 485 779  | -0.004 757 041 616 | 0.038 498 873 847  |
| C                                                             | -0.134 043 564 761 | -0.133 737 660 352 | 0.105 688 576 912  |
| C                                                             | -0.089 836 249 951 | 0.253 650 457 128  | -0.136 995 008 243 |
| C                                                             | -0.223 891 243 291 | -0.001 371 613 718 | -0.188 664 916 410 |
| H                                                             | 0.013 710 661 624  | -0.046 613 245 231 | 0.014 187 036 553  |
| H                                                             | -0.188 860 805 878 | -0.032 178 941 816 | 0.028 479 978 934  |
| H                                                             | 0.157 250 748 071  | 0.134 052 975 303  | 0.041 978 666 254  |
| H                                                             | 0.013 221 216 172  | 0.020 420 445 419  | 0.029 806 139 605  |
| H                                                             | -0.176 172 637 545 | 0.154 633 012 884  | 0.043 276 587 119  |
| H                                                             | -0.280 272 584 047 | -0.328 255 770 832 | -0.037 634 255 007 |
| H                                                             | 0.233 353 147 141  | 0.310 438 627 080  | -0.041 775 692 787 |
| H                                                             | 0.031 609 195 600  | -0.006 430 514 494 | 0.043 348 522 223  |
| H                                                             | -0.184 673 346 070 | 0.105 527 977 233  | -0.049 601 487 793 |
| H                                                             | -0.108 075 457 782 | 0.070 310 765 211  | 0.000 422 692 159  |

Wavenumber/cm<sup>-1</sup>: 1364.8359 , Max excitation: 3

| $l'$ -matrix coefficients/(u <sup>1/2</sup> Å <sup>-1</sup> ) |                    |                    |                    |
|---------------------------------------------------------------|--------------------|--------------------|--------------------|
| O                                                             | 0.012 187 795 050  | 0.005 607 676 766  | 0.003 425 719 209  |
| C                                                             | 0.157 044 876 989  | -0.178 357 364 481 | -0.137 600 536 655 |
| C                                                             | 0.071 337 469 967  | -0.041 599 795 858 | 0.068 203 157 841  |
| C                                                             | 0.077 219 716 868  | 0.062 704 903 724  | -0.062 746 976 074 |
| C                                                             | -0.091 576 119 642 | -0.213 358 212 181 | 0.012 357 219 318  |
| C                                                             | -0.132 320 176 415 | 0.389 052 500 990  | 0.135 501 389 737  |
| C                                                             | -0.040 121 029 496 | 0.024 469 423 316  | -0.085 832 365 310 |
| H                                                             | -0.469 268 910 862 | 0.124 766 644 109  | 0.107 556 518 422  |
| H                                                             | 0.504 392 651 895  | -0.126 525 770 100 | -0.003 827 609 516 |
| H                                                             | -0.066 206 840 559 | -0.172 692 038 684 | 0.007 904 121 184  |
| H                                                             | -0.061 337 165 304 | 0.124 648 120 503  | 0.079 632 568 285  |
| H                                                             | 0.043 614 544 516  | -0.108 577 908 830 | -0.012 230 362 348 |
| H                                                             | 0.076 990 643 949  | 0.086 241 326 055  | 0.018 966 088 168  |
| H                                                             | -0.116 239 792 444 | -0.111 462 600 394 | -0.013 940 851 861 |
| H                                                             | -0.005 909 806 877 | -0.013 709 650 030 | 0.030 731 413 042  |
| H                                                             | -0.113 452 402 470 | 0.024 290 078 844  | -0.023 843 650 852 |
| H                                                             | 0.015 310 170 330  | 0.002 550 804 316  | 0.037 449 866 871  |

Wavenumber/cm<sup>-1</sup>: 1392.9017 , Max excitation: 4

| $l'$ -matrix coefficients/(u <sup>1/2</sup> Å <sup>-1</sup> ) |                    |                    |                    |
|---------------------------------------------------------------|--------------------|--------------------|--------------------|
| O                                                             | 0.072 520 819 098  | 0.027 289 869 510  | -0.007 696 485 637 |
| C                                                             | -0.126 744 414 047 | 0.114 847 188 290  | -0.166 041 861 931 |
| C                                                             | -0.294 414 687 557 | 0.082 832 714 746  | 0.118 657 805 993  |
| C                                                             | -0.001 064 136 679 | -0.014 828 369 108 | -0.149 586 679 265 |
| C                                                             | 0.039 462 472 164  | 0.099 957 159 937  | 0.187 266 578 900  |
| C                                                             | 0.071 753 845 115  | -0.235 043 452 041 | -0.024 488 395 623 |
| C                                                             | 0.229 787 515 059  | -0.062 129 291 220 | -0.033 738 614 619 |
| H                                                             | -0.175 682 025 963 | 0.144 152 281 045  | 0.035 824 701 794  |
| H                                                             | 0.267 630 409 539  | -0.056 767 485 538 | 0.019 191 153 825  |
| H                                                             | -0.269 779 594 252 | 0.078 099 004 838  | 0.027 886 658 064  |
| H                                                             | 0.186 085 628 369  | -0.059 894 751 518 | 0.054 661 908 829  |
| H                                                             | -0.147 411 306 759 | -0.054 424 259 391 | -0.008 264 608 010 |
| H                                                             | -0.177 719 507 206 | -0.363 512 130 138 | -0.058 449 938 335 |
| H                                                             | 0.181 944 440 499  | 0.300 935 831 051  | -0.051 003 791 479 |
| H                                                             | 0.113 934 899 580  | -0.055 552 963 723 | 0.123 829 510 752  |
| H                                                             | -0.106 706 305 971 | 0.029 626 889 598  | -0.004 804 899 040 |
| H                                                             | 0.119 142 528 644  | -0.021 803 001 666 | 0.126 289 865 456  |

Wavenumber/cm<sup>-1</sup>: 1412.6378 , Max excitation: 1

| $l'$ -matrix coefficients/(u <sup>1/2</sup> Å <sup>-1</sup> ) |                    |                    |                    |
|---------------------------------------------------------------|--------------------|--------------------|--------------------|
| O                                                             | 0.023 351 598 803  | 0.016 221 396 200  | -0.001 039 773 147 |
| C                                                             | -0.146 922 751 086 | -0.072 388 333 895 | -0.018 055 641 119 |
| C                                                             | 0.079 389 607 920  | 0.129 271 310 940  | 0.019 023 918 107  |
| C                                                             | 0.437 553 263 643  | -0.154 041 240 128 | 0.011 351 936 135  |
| C                                                             | -0.438 854 940 691 | 0.095 034 988 467  | 0.008 500 487 134  |
| C                                                             | 0.061 467 025 487  | -0.070 506 965 778 | 0.002 894 991 432  |
| C                                                             | -0.007 465 193 853 | 0.226 030 898 898  | 0.029 288 426 048  |
| H                                                             | -0.057 377 240 563 | 0.026 819 166 890  | 0.025 442 759 041  |
| H                                                             | -0.068 663 533 708 | -0.069 430 506 028 | 0.053 183 751 241  |
| H                                                             | 0.073 019 012 626  | 0.024 660 556 702  | 0.006 522 509 730  |
| H                                                             | 0.299 175 154 026  | -0.163 984 004 891 | -0.025 761 475 861 |
| H                                                             | 0.211 195 317 580  | -0.095 131 106 688 | -0.009 343 572 556 |
| H                                                             | -0.102 545 419 270 | -0.093 228 651 518 | -0.058 144 747 823 |
| H                                                             | -0.297 738 470 021 | -0.015 613 174 876 | -0.085 366 497 535 |
| H                                                             | -0.291 887 262 375 | 0.027 291 701 980  | -0.110 395 703 823 |
| H                                                             | 0.016 064 019 681  | -0.108 127 568 684 | -0.001 403 105 354 |
| H                                                             | 0.176 926 991 451  | -0.127 420 027 131 | 0.026 439 374 736  |



Wavenumber/cm<sup>-1</sup>: 1477.2679 , Max excitation: 1

| $l'$ -matrix coefficients/(u <sup>1/2</sup> Å <sup>-1</sup> ) |                    |                    |
|---------------------------------------------------------------|--------------------|--------------------|
| O                                                             | -0.004 962 206 303 | 0.001 749 408 445  |
| C                                                             | 0.009 077 007 955  | 0.006 791 793 369  |
| C                                                             | 0.011 873 779 169  | -0.090 998 874 369 |
| C                                                             | -0.017 355 210 179 | 0.222 762 674 413  |
| C                                                             | 0.017 784 931 281  | 0.075 684 522 646  |
| C                                                             | 0.032 770 659 287  | -0.091 240 184 922 |
| C                                                             | -0.142 041 727 071 | -0.017 247 199 318 |
| H                                                             | 0.003 054 259 299  | -0.046 371 942 141 |
| H                                                             | 0.031 980 801 408  | 0.025 886 539 578  |
| H                                                             | 0.221 573 971 005  | -0.293 451 669 680 |
| H                                                             | -0.030 058 358 682 | 0.251 202 005 202  |
| H                                                             | 0.014 878 242 403  | -0.293 218 796 060 |
| H                                                             | 0.134 153 482 847  | -0.269 350 962 948 |
| H                                                             | -0.114 496 944 276 | 0.209 659 425 929  |
| H                                                             | -0.064 916 627 431 | 0.070 011 523 137  |
| H                                                             | 0.307 401 089 232  | -0.077 934 118 168 |
| H                                                             | -0.180 403 480 831 | 0.051 541 710 893  |

Wavenumber/cm<sup>-1</sup>: 1480.285 , Max excitation: 1

| $l'$ -matrix coefficients/(u <sup>1/2</sup> Å <sup>-1</sup> ) |                    |                    |
|---------------------------------------------------------------|--------------------|--------------------|
| O                                                             | 0.043 978 059 129  | -0.004 294 859 351 |
| C                                                             | -0.189 465 984 198 | -0.336 856 352 926 |
| C                                                             | 0.043 086 999 534  | 0.228 725 164 470  |
| C                                                             | -0.230 635 765 839 | -0.068 451 226 924 |
| C                                                             | 0.280 008 771 874  | -0.010 372 664 562 |
| C                                                             | -0.017 243 208 445 | 0.048 037 660 304  |
| C                                                             | 0.014 946 125 657  | 0.158 130 114 445  |
| H                                                             | -0.013 243 121 765 | 0.261 443 775 825  |
| H                                                             | -0.088 735 941 046 | -0.332 472 502 574 |
| H                                                             | 0.179 480 879 390  | 0.126 735 561 199  |
| H                                                             | -0.093 739 087 616 | -0.004 776 566 488 |
| H                                                             | -0.092 295 494 268 | 0.020 610 562 028  |
| H                                                             | 0.035 600 228 266  | 0.040 689 383 890  |
| H                                                             | 0.223 773 951 024  | 0.052 901 110 805  |
| H                                                             | -0.274 721 207 741 | 0.037 169 180 023  |
| H                                                             | 0.168 973 526 276  | -0.134 743 780 171 |
| H                                                             | 0.122 486 520 465  | -0.116 767 533 519 |

Wavenumber/cm<sup>-1</sup>: 1493.901 , Max excitation: 1

| $l'$ -matrix coefficients/(u <sup>1/2</sup> Å <sup>-1</sup> ) |                    |                    |
|---------------------------------------------------------------|--------------------|--------------------|
| O -0.027 872 175 091                                          | -0.009 354 467 451 | 0.000 747 460 542  |
| C -0.076 429 061 747                                          | 0.029 826 906 046  | -0.279 934 126 972 |
| C -0.068 452 908 724                                          | -0.192 061 162 121 | 0.036 578 152 599  |
| C 0.241 135 292 708                                           | 0.336 412 158 948  | 0.103 440 595 673  |
| C -0.073 931 704 788                                          | -0.005 495 467 818 | -0.182 500 088 051 |
| C 0.083 575 048 060                                           | -0.126 007 325 258 | 0.145 818 142 917  |
| C -0.096 612 176 661                                          | -0.150 141 366 870 | 0.038 614 681 509  |
| H 0.075 798 019 901                                           | 0.301 494 091 496  | 0.045 031 057 047  |
| H -0.029 535 786 929                                          | -0.212 244 644 093 | 0.183 703 254 311  |
| H 0.105 370 096 897                                           | 0.068 408 854 955  | 0.020 341 095 316  |
| H 0.219 644 882 654                                           | 0.054 320 758 698  | 0.110 491 734 563  |
| H -0.102 889 794 690                                          | 0.073 531 544 027  | 0.066 714 445 049  |
| H -0.244 523 728 814                                          | 0.075 980 422 200  | 0.046 000 096 173  |
| H -0.032 677 892 992                                          | -0.200 454 025 250 | 0.100 051 729 212  |
| H 0.209 367 254 644                                           | 0.022 474 884 674  | 0.017 283 967 715  |
| H 0.135 974 827 519                                           | 0.073 892 263 529  | 0.016 251 865 035  |
| H -0.257 532 790 404                                          | 0.150 836 355 038  | -0.132 533 622 683 |

Wavenumber/cm<sup>-1</sup>: 1496.0701 , Max excitation: 0

| $l'$ -matrix coefficients/(u <sup>1/2</sup> Å <sup>-1</sup> ) |                    |                    |
|---------------------------------------------------------------|--------------------|--------------------|
| O 0.009 057 982 743                                           | -0.014 543 274 889 | -0.005 153 835 592 |
| C -0.366 318 711 059                                          | -0.188 859 658 196 | 0.249 148 699 374  |
| C 0.083 270 493 113                                           | 0.181 773 782 600  | -0.150 050 796 127 |
| C 0.127 551 230 547                                           | 0.349 395 961 915  | -0.083 493 094 086 |
| C 0.118 666 864 014                                           | -0.177 622 274 765 | -0.107 471 368 608 |
| C 0.053 465 866 091                                           | -0.062 078 374 452 | -0.017 446 773 512 |
| C 0.137 669 249 304                                           | 0.025 722 558 068  | -0.033 348 769 831 |
| H -0.155 438 190 199                                          | -0.239 539 426 132 | -0.003 312 493 701 |
| H -0.184 102 152 158                                          | 0.062 225 341 817  | -0.067 869 560 302 |
| H -0.086 681 892 970                                          | -0.061 693 029 600 | -0.051 373 115 357 |
| H 0.064 399 360 157                                           | 0.261 021 695 282  | 0.273 513 394 440  |
| H -0.148 098 511 674                                          | -0.161 253 971 894 | 0.033 387 599 362  |
| H -0.163 591 769 270                                          | 0.034 316 553 514  | 0.063 739 456 844  |
| H 0.073 749 401 080                                           | -0.178 032 515 099 | 0.105 347 361 370  |
| H -0.007 359 093 737                                          | -0.030 632 054 213 | 0.053 560 746 668  |
| H -0.118 522 394 577                                          | -0.004 007 772 715 | -0.010 416 661 593 |
| H 0.156 899 498 261                                           | -0.067 462 957 431 | 0.116 423 541 764  |

Wavenumber/cm<sup>-1</sup>: 1500.0519 , Max excitation: 0

| $l'$ -matrix coefficients/(u <sup>1/2</sup> Å <sup>-1</sup> ) |                    |                    |                    |
|---------------------------------------------------------------|--------------------|--------------------|--------------------|
| O                                                             | 0.067 124 602 019  | 0.029 144 560 397  | -0.004 822 450 724 |
| C                                                             | -0.064 091 280 495 | 0.482 561 499 512  | 0.003 546 264 786  |
| C                                                             | 0.007 217 327 672  | 0.112 350 922 337  | 0.256 839 064 138  |
| C                                                             | 0.067 372 531 906  | -0.306 838 973 219 | -0.189 213 980 179 |
| C                                                             | 0.101 222 311 111  | -0.389 402 275 609 | -0.111 574 540 423 |
| C                                                             | 0.035 644 000 733  | 0.021 887 480 974  | 0.041 445 184 318  |
| C                                                             | -0.194 270 495 016 | 0.086 120 676 689  | 0.016 042 974 920  |
| H                                                             | -0.076 895 715 462 | 0.015 313 237 054  | -0.041 053 792 821 |
| H                                                             | 0.047 325 602 241  | 0.200 392 685 424  | -0.084 943 192 594 |
| H                                                             | 0.067 982 625 564  | -0.028 342 249 983 | 0.071 835 462 934  |
| H                                                             | 0.066 623 129 692  | -0.051 688 074 167 | 0.063 106 816 865  |
| H                                                             | -0.119 984 439 410 | -0.147 734 542 453 | -0.020 171 541 258 |
| H                                                             | -0.178 614 370 847 | 0.003 770 386 315  | 0.072 106 932 093  |
| H                                                             | 0.202 528 011 293  | -0.160 603 797 497 | 0.139 093 559 701  |
| H                                                             | -0.144 720 633 339 | 0.054 128 281 046  | -0.134 022 457 544 |
| H                                                             | 0.128 473 508 452  | -0.048 731 247 172 | 0.000 623 327 287  |
| H                                                             | -0.098 230 209 509 | 0.024 324 135 042  | -0.106 339 081 789 |

Wavenumber/cm<sup>-1</sup>: 2885.9006 , Max excitation: 2

| $l'$ -matrix coefficients/(u <sup>1/2</sup> Å <sup>-1</sup> ) |                    |                    |                    |
|---------------------------------------------------------------|--------------------|--------------------|--------------------|
| O                                                             | 0.234 580 824 559  | 0.079 304 563 383  | -0.009 843 490 627 |
| C                                                             | -0.369 104 250 441 | 0.259 658 101 758  | -0.086 047 487 753 |
| C                                                             | 0.038 472 696 665  | -0.038 639 680 644 | -0.143 754 642 212 |
| C                                                             | -0.051 203 986 166 | 0.030 084 915 928  | 0.150 125 517 156  |
| C                                                             | -0.035 523 852 653 | -0.440 594 175 729 | 0.168 590 543 271  |
| C                                                             | 0.103 486 104 798  | 0.113 502 109 745  | -0.042 518 616 163 |
| C                                                             | 0.125 364 411 714  | -0.054 672 370 238 | 0.011 079 648 624  |
| H                                                             | -0.111 258 496 765 | 0.184 684 430 751  | 0.036 887 987 919  |
| H                                                             | -0.223 289 159 699 | -0.027 593 236 796 | 0.111 121 446 301  |
| H                                                             | 0.021 523 790 217  | 0.041 966 098 174  | -0.037 894 046 915 |
| H                                                             | -0.227 848 006 645 | 0.031 893 499 123  | -0.133 894 675 789 |
| H                                                             | 0.164 412 729 310  | 0.131 625 547 145  | -0.003 165 229 405 |
| H                                                             | 0.181 522 056 550  | -0.229 327 356 140 | -0.065 102 272 224 |
| H                                                             | -0.206 552 501 505 | -0.044 230 114 026 | -0.157 861 152 356 |
| H                                                             | 0.116 295 743 881  | -0.016 274 919 179 | 0.064 997 003 833  |
| H                                                             | -0.009 486 756 031 | 0.040 800 735 764  | 0.006 558 595 038  |
| H                                                             | 0.010 821 042 619  | 0.021 539 325 234  | 0.019 167 073 659  |

Wavenumber/cm<sup>-1</sup>: 2894.6074 , Max excitation: 1

| $l'$ -matrix coefficients/(u <sup>1/2</sup> Å <sup>-1</sup> ) |                    |                    |                    |
|---------------------------------------------------------------|--------------------|--------------------|--------------------|
| O                                                             | -0.324 824 153 232 | -0.127 960 507 379 | 0.019 505 661 300  |
| C                                                             | 0.018 063 620 211  | -0.019 076 300 888 | -0.001 627 630 229 |
| C                                                             | -0.104 659 735 336 | 0.193 447 214 538  | 0.059 874 048 467  |
| C                                                             | 0.374 808 198 941  | 0.201 296 691 714  | 0.089 622 900 594  |
| C                                                             | 0.414 984 079 505  | -0.198 511 597 533 | 0.051 599 185 681  |
| C                                                             | -0.154 740 554 688 | -0.224 882 170 878 | -0.076 049 524 000 |
| C                                                             | -0.274 251 297 329 | 0.121 134 092 440  | -0.051 956 310 363 |
| H                                                             | 0.017 573 096 724  | -0.008 184 348 764 | -0.003 872 934 461 |
| H                                                             | 0.110 120 856 615  | 0.000 251 980 649  | -0.020 849 619 236 |
| H                                                             | -0.074 215 305 036 | 0.093 486 679 362  | 0.016 755 964 034  |
| H                                                             | 0.037 385 361 455  | 0.000 204 343 081  | -0.145 460 112 240 |
| H                                                             | 0.231 146 541 936  | 0.185 472 661 706  | -0.008 645 820 244 |
| H                                                             | 0.242 735 080 023  | -0.112 625 146 975 | -0.042 676 838 510 |
| H                                                             | 0.038 275 907 047  | 0.005 535 419 665  | -0.101 600 007 561 |
| H                                                             | -0.089 188 799 741 | 0.028 746 306 491  | -0.005 491 248 891 |
| H                                                             | -0.102 187 752 793 | 0.038 687 788 569  | -0.014 791 695 845 |
| H                                                             | -0.064 067 871 008 | 0.024 826 374 779  | 0.002 232 365 101  |

Wavenumber/cm<sup>-1</sup>: 2978.6944 , Max excitation: 1

| $l'$ -matrix coefficients/(u <sup>1/2</sup> Å <sup>-1</sup> ) |                    |                    |                    |
|---------------------------------------------------------------|--------------------|--------------------|--------------------|
| O                                                             | 0.493 655 466 789  | 0.193 202 126 873  | -0.025 915 506 418 |
| C                                                             | -0.035 980 093 986 | -0.308 925 159 888 | 0.052 434 252 237  |
| C                                                             | -0.320 319 459 694 | -0.055 410 678 182 | 0.213 807 310 723  |
| C                                                             | -0.082 812 624 681 | 0.093 884 339 749  | 0.045 640 314 460  |
| C                                                             | 0.020 476 418 773  | 0.002 247 061 201  | -0.016 619 359 638 |
| C                                                             | 0.370 076 819 183  | -0.016 189 619 537 | -0.091 380 863 762 |
| C                                                             | -0.361 954 547 546 | 0.086 830 664 036  | -0.087 118 725 647 |
| H                                                             | -0.067 742 973 201 | -0.194 026 094 732 | -0.023 304 867 106 |
| H                                                             | 0.007 988 031 369  | -0.009 123 633 683 | -0.088 585 329 696 |
| H                                                             | -0.147 096 971 742 | -0.009 122 320 038 | 0.058 841 320 303  |
| H                                                             | -0.000 664 018 751 | -0.054 240 294 705 | -0.100 658 880 992 |
| H                                                             | 0.005 676 698 121  | 0.135 459 091 825  | -0.001 539 330 313 |
| H                                                             | -0.003 942 999 999 | 0.000 499 156 350  | -0.002 754 421 870 |
| H                                                             | -0.058 545 544 330 | -0.057 580 506 915 | -0.003 446 206 958 |
| H                                                             | -0.101 142 901 689 | 0.036 272 733 988  | -0.052 534 463 893 |
| H                                                             | -0.043 055 677 326 | 0.014 228 143 510  | -0.025 270 043 402 |
| H                                                             | -0.141 151 417 533 | 0.049 886 232 034  | -0.060 561 825 386 |

Wavenumber/cm<sup>-1</sup>: 2984.5747 , Max excitation: 2

| $l'$ -matrix coefficients/(u <sup>1/2</sup> Å <sup>-1</sup> ) |                    |                    |
|---------------------------------------------------------------|--------------------|--------------------|
| O -0.092 969 445 342                                          | -0.142 558 479 426 | 0.035 699 440 447  |
| C -0.216 986 995 797                                          | -0.068 846 478 057 | -0.093 911 786 934 |
| C 0.062 917 791 145                                           | -0.072 234 113 314 | 0.482 737 715 404  |
| C 0.022 324 859 312                                           | 0.177 819 046 576  | -0.058 176 765 466 |
| C -0.046 346 522 390                                          | 0.072 291 108 711  | -0.024 199 555 635 |
| C -0.137 995 064 611                                          | 0.082 142 046 199  | -0.091 345 229 329 |
| C 0.366 299 557 800                                           | -0.065 528 162 175 | -0.061 381 217 930 |
| H -0.207 598 494 911                                          | -0.203 881 952 489 | -0.090 262 194 674 |
| H -0.038 462 839 014                                          | 0.104 120 732 562  | -0.182 412 520 368 |
| H 0.031 335 323 833                                           | -0.024 534 752 300 | 0.138 133 551 283  |
| H -0.023 980 852 739                                          | -0.044 602 668 015 | -0.210 636 668 957 |
| H 0.045 713 031 951                                           | 0.283 599 057 052  | -0.041 405 942 292 |
| H -0.020 955 027 098                                          | 0.041 484 667 882  | 0.003 389 169 764  |
| H -0.010 004 667 216                                          | 0.014 772 473 451  | 0.001 442 540 376  |
| H 0.072 365 828 490                                           | 0.014 551 324 023  | -0.129 934 922 240 |
| H 0.324 706 787 498                                           | -0.072 186 339 039 | -0.019 918 705 645 |
| H 0.023 942 093 186                                           | 0.020 922 945 997  | -0.141 273 276 686 |

Wavenumber/cm<sup>-1</sup>: 3015.1866 , Max excitation: 1

| $l'$ -matrix coefficients/(u <sup>1/2</sup> Å <sup>-1</sup> ) |                    |                    |
|---------------------------------------------------------------|--------------------|--------------------|
| O 0.160 894 003 717                                           | -0.415 605 073 080 | 0.008 752 122 089  |
| C -0.291 926 912 318                                          | 0.004 956 473 113  | -0.013 244 882 606 |
| C -0.135 239 866 156                                          | -0.224 334 207 349 | -0.092 127 693 761 |
| C 0.169 484 733 012                                           | -0.221 756 160 193 | 0.039 182 204 096  |
| C 0.210 248 320 287                                           | 0.245 920 971 223  | 0.002 764 130 628  |
| C -0.106 879 665 969                                          | 0.299 298 671 233  | -0.014 447 445 857 |
| C -0.050 266 981 491                                          | 0.273 276 300 434  | 0.026 892 172 809  |
| H -0.126 844 312 096                                          | 0.001 624 644 292  | 0.000 575 450 081  |
| H -0.171 401 261 488                                          | 0.006 537 638 518  | 0.003 252 438 096  |
| H -0.046 722 850 814                                          | -0.076 635 274 348 | -0.026 989 453 969 |
| H 0.143 180 655 670                                           | -0.081 658 539 405 | 0.077 672 873 583  |
| H 0.041 063 678 743                                           | -0.157 261 348 756 | 0.020 236 975 684  |
| H 0.119 754 943 793                                           | 0.103 421 503 549  | -0.002 368 910 011 |
| H 0.108 615 219 572                                           | 0.119 826 386 043  | -0.003 330 644 013 |
| H 0.131 960 877 754                                           | 0.088 148 949 476  | 0.096 792 038 087  |
| H -0.023 883 143 034                                          | 0.182 784 024 638  | 0.012 502 425 581  |
| H -0.110 530 667 791                                          | 0.166 368 946 849  | -0.037 225 088 517 |

Wavenumber/cm<sup>-1</sup>: 3021.7666 , Max excitation: 1

| $l'$ -matrix coefficients/(u <sup>1/2</sup> Å <sup>-1</sup> ) |                    |                    |                    |
|---------------------------------------------------------------|--------------------|--------------------|--------------------|
| O                                                             | 0.250 414 077 863  | -0.472 624 936 108 | -0.009 790 489 294 |
| C                                                             | 0.010 477 330 762  | 0.231 854 678 989  | 0.114 629 146 868  |
| C                                                             | -0.023 372 395 712 | 0.158 942 519 765  | 0.006 346 695 411  |
| C                                                             | 0.014 238 357 154  | 0.216 485 935 902  | -0.051 718 744 622 |
| C                                                             | -0.032 531 292 479 | 0.171 786 187 672  | -0.045 326 250 954 |
| C                                                             | -0.000 898 118 931 | 0.172 901 554 423  | 0.010 587 438 304  |
| C                                                             | -0.190 976 778 994 | -0.387 163 407 594 | -0.024 380 699 025 |
| H                                                             | 0.004 938 424 543  | 0.117 571 910 180  | 0.056 053 798 500  |
| H                                                             | 0.004 913 752 886  | 0.033 550 138 650  | 0.075 322 096 790  |
| H                                                             | -0.011 550 560 836 | 0.040 007 940 310  | 0.001 240 692 108  |
| H                                                             | -0.003 546 318 768 | 0.051 490 882 261  | -0.041 024 977 477 |
| H                                                             | 0.008 475 876 791  | 0.092 052 718 122  | -0.018 146 765 010 |
| H                                                             | -0.004 063 418 589 | 0.043 644 146 978  | -0.019 209 160 509 |
| H                                                             | -0.007 020 327 480 | 0.063 686 175 118  | -0.021 881 799 201 |
| H                                                             | -0.094 640 507 296 | -0.039 420 018 948 | -0.222 174 774 452 |
| H                                                             | -0.135 426 278 994 | -0.378 017 661 318 | -0.020 663 957 626 |
| H                                                             | 0.010 258 706 686  | -0.091 295 780 446 | 0.214 496 177 086  |

Wavenumber/cm<sup>-1</sup>: 3034.0979 , Max excitation: 0

| $l'$ -matrix coefficients/(u <sup>1/2</sup> Å <sup>-1</sup> ) |                    |                    |                    |
|---------------------------------------------------------------|--------------------|--------------------|--------------------|
| O                                                             | -0.108 682 373 520 | 0.195 813 070 492  | -0.030 669 517 761 |
| C                                                             | -0.025 953 832 343 | -0.097 410 681 718 | 0.079 261 442 694  |
| C                                                             | -0.002 798 207 970 | -0.125 801 984 071 | -0.023 875 610 040 |
| C                                                             | 0.030 404 425 114  | -0.087 239 509 713 | -0.119 174 078 408 |
| C                                                             | 0.022 277 850 272  | -0.056 486 026 882 | 0.042 688 496 513  |
| C                                                             | -0.006 816 627 059 | -0.048 446 943 638 | 0.025 002 748 612  |
| C                                                             | 0.075 412 003 472  | 0.168 339 958 912  | 0.017 471 123 150  |
| H                                                             | -0.001 862 383 778 | -0.000 103 716 795 | 0.035 857 198 647  |
| H                                                             | -0.027 126 505 968 | -0.047 469 970 534 | 0.050 283 703 936  |
| H                                                             | -0.000 791 020 281 | -0.058 621 075 754 | -0.008 031 204 239 |
| H                                                             | 0.001 290 719 563  | -0.045 145 063 479 | -0.075 761 518 954 |
| H                                                             | 0.044 635 904 154  | 0.007 877 689 621  | -0.043 820 189 155 |
| H                                                             | -0.026 365 760 814 | -0.007 900 180 714 | 0.025 015 505 894  |
| H                                                             | 0.033 087 760 528  | -0.021 772 250 333 | 0.034 654 924 909  |
| H                                                             | 0.324 077 287 691  | 0.281 418 411 035  | -0.368 349 342 896 |
| H                                                             | -0.120 174 864 857 | -0.406 855 763 937 | -0.017 886 937 030 |
| H                                                             | -0.113 168 594 094 | 0.371 232 472 354  | 0.416 444 588 606  |

Wavenumber/cm<sup>-1</sup>: 3071.7265 , Max excitation: 1

| $l'$ -matrix coefficients/(u <sup>1/2</sup> Å <sup>-1</sup> ) |                    |                    |                    |
|---------------------------------------------------------------|--------------------|--------------------|--------------------|
| O                                                             | -0.010 473 373 957 | -0.020 221 258 276 | -0.302 614 937 982 |
| C                                                             | -0.011 285 677 473 | -0.040 746 459 539 | -0.120 315 870 694 |
| C                                                             | -0.013 386 586 565 | 0.023 132 635 113  | -0.012 209 121 767 |
| C                                                             | -0.003 471 590 969 | 0.028 932 615 555  | -0.022 162 528 640 |
| C                                                             | 0.023 998 368 314  | -0.024 327 869 724 | -0.128 888 575 234 |
| C                                                             | 0.037 519 351 092  | 0.053 162 989 829  | 0.822 493 043 709  |
| C                                                             | -0.016 765 557 967 | 0.005 491 411 232  | -0.011 610 447 588 |
| H                                                             | 0.064 137 718 476  | -0.175 792 933 489 | -0.127 421 430 193 |
| H                                                             | -0.086 434 632 623 | 0.096 586 653 373  | -0.159 906 461 313 |
| H                                                             | 0.003 689 656 510  | 0.020 940 889 584  | -0.003 422 264 865 |
| H                                                             | -0.002 268 925 425 | 0.004 280 562 440  | -0.014 717 340 578 |
| H                                                             | -0.014 870 275 311 | 0.021 190 099 541  | -0.005 270 520 807 |
| H                                                             | 0.050 858 929 829  | -0.175 035 495 914 | -0.132 381 994 693 |
| H                                                             | -0.012 011 588 658 | 0.128 584 227 833  | -0.165 919 328 912 |
| H                                                             | -0.002 678 412 698 | 0.005 293 152 934  | -0.010 505 855 791 |
| H                                                             | -0.012 423 442 259 | -0.008 451 311 564 | -0.003 716 536 404 |
| H                                                             | -0.003 603 839 500 | 0.005 400 444 400  | 0.008 651 421 943  |

Wavenumber/cm<sup>-1</sup>: 3085.0111 , Max excitation: 1

| $l'$ -matrix coefficients/(u <sup>1/2</sup> Å <sup>-1</sup> ) |                    |                    |                    |
|---------------------------------------------------------------|--------------------|--------------------|--------------------|
| O                                                             | -0.024 220 585 400 | 0.050 703 856 586  | 0.183 277 805 836  |
| C                                                             | 0.010 990 530 485  | 0.009 915 239 187  | 0.085 348 945 741  |
| C                                                             | -0.022 419 652 201 | 0.064 515 881 622  | 0.131 923 555 397  |
| C                                                             | -0.093 270 364 042 | -0.091 043 417 768 | 0.413 797 452 956  |
| C                                                             | 0.055 496 126 448  | -0.020 517 267 885 | -0.437 792 228 384 |
| C                                                             | -0.026 219 851 887 | 0.001 458 297 859  | -0.090 568 650 773 |
| C                                                             | 0.092 199 440 674  | -0.001 460 025 885 | -0.243 083 756 075 |
| H                                                             | -0.020 295 407 295 | 0.032 227 400 246  | 0.041 517 889 551  |
| H                                                             | 0.033 275 526 852  | -0.013 192 951 011 | 0.040 879 500 219  |
| H                                                             | -0.059 879 972 003 | 0.090 167 930 173  | 0.037 725 737 969  |
| H                                                             | 0.066 096 321 030  | 0.019 615 630 959  | 0.289 278 391 149  |
| H                                                             | -0.199 439 329 605 | -0.156 632 775 248 | 0.163 760 938 739  |
| H                                                             | 0.208 485 631 705  | -0.109 921 527 707 | -0.225 719 530 443 |
| H                                                             | -0.103 932 429 286 | 0.080 691 477 325  | -0.287 516 412 071 |
| H                                                             | 0.028 852 136 484  | 0.045 780 509 840  | -0.186 476 831 435 |
| H                                                             | 0.092 697 789 803  | -0.110 708 434 486 | -0.075 324 621 175 |
| H                                                             | -0.007 274 757 163 | 0.048 141 067 187  | -0.043 747 655 250 |

Wavenumber/cm<sup>-1</sup>: 3088.7315 , Max excitation: 1

| $l'$ -matrix coefficients/(u <sup>1/2</sup> Å <sup>-1</sup> ) |                    |                    |                    |
|---------------------------------------------------------------|--------------------|--------------------|--------------------|
| O                                                             | 0.061 461 580 493  | 0.002 977 626 911  | 0.536 058 649 026  |
| C                                                             | -0.012 483 621 363 | -0.032 727 682 942 | -0.519 352 478 477 |
| C                                                             | 0.075 124 876 230  | 0.055 144 843 860  | -0.079 905 391 018 |
| C                                                             | -0.024 602 688 971 | 0.012 946 329 362  | -0.049 712 758 950 |
| C                                                             | 0.000 516 953 363  | -0.005 532 668 019 | -0.164 311 726 604 |
| C                                                             | 0.015 986 875 027  | 0.002 446 923 220  | -0.071 454 133 712 |
| C                                                             | -0.105 006 320 926 | -0.020 233 608 733 | 0.333 627 557 686  |
| H                                                             | -0.016 710 427 068 | -0.150 624 147 648 | -0.213 897 248 340 |
| H                                                             | -0.013 522 249 425 | 0.083 645 377 034  | -0.263 182 794 496 |
| H                                                             | 0.124 385 966 847  | 0.052 433 466 999  | -0.017 430 880 557 |
| H                                                             | 0.001 198 351 035  | 0.014 924 263 294  | 0.011 561 419 717  |
| H                                                             | -0.037 790 268 304 | -0.009 792 021 164 | -0.007 998 822 514 |
| H                                                             | 0.023 764 582 599  | -0.019 211 388 874 | -0.062 955 830 751 |
| H                                                             | -0.016 277 682 534 | 0.009 597 477 675  | -0.070 897 555 418 |
| H                                                             | 0.013 651 571 563  | 0.012 364 258 481  | 0.081 734 621 235  |
| H                                                             | -0.150 460 580 254 | -0.057 289 272 348 | 0.093 666 669 407  |
| H                                                             | 0.001 093 439 266  | 0.010 512 742 525  | 0.216 117 883 485  |

Wavenumber/cm<sup>-1</sup>: 72.5908

| $\frac{\partial \mu_{x,y,z}}{\partial Q_r} / (e u^{-0.5})$   | 0.000 491 133 779  | -0.001 200 355 570 | -0.002 722 597 921                    |
|--------------------------------------------------------------|--------------------|--------------------|---------------------------------------|
| $l$ -matrix coefficients/(u <sup>1/2</sup> Å <sup>-1</sup> ) |                    |                    |                                       |
| O                                                            | 0.001 600 030 885  | -0.000 355 431 779 | -8.182 581 400 000 × 10 <sup>-5</sup> |
| C                                                            | 0.002 528 839 629  | 0.096 403 669 044  | 0.052 161 102 370                     |
| C                                                            | 0.011 113 013 496  | 0.003 533 832 360  | -0.011 852 768 166                    |
| C                                                            | -0.023 664 070 998 | -0.003 211 661 530 | -0.060 067 445 514                    |
| C                                                            | -0.151 133 167 178 | -0.163 252 439 744 | -0.144 477 231 406                    |
| C                                                            | -0.004 566 063 314 | 0.000 678 069 648  | -0.000 585 775 362                    |
| C                                                            | 0.014 543 887 360  | 0.026 381 727 714  | -0.016 582 961 861                    |
| H                                                            | 0.008 117 646 490  | -0.335 163 206 722 | -0.107 073 802 992                    |
| H                                                            | -0.018 069 699 946 | 0.005 180 361 262  | -0.081 523 549 353                    |
| H                                                            | -0.030 914 384 873 | -0.006 642 425 059 | 0.037 900 192 441                     |
| H                                                            | 0.016 382 183 722  | 0.064 446 514 430  | 0.159 132 849 644                     |
| H                                                            | 0.071 866 414 104  | -0.058 590 621 427 | 0.047 583 096 662                     |
| H                                                            | 0.493 715 264 850  | 0.588 537 494 729  | 0.213 941 718 123                     |
| H                                                            | 0.025 313 018 455  | -0.027 980 910 674 | 0.298 003 132 770                     |
| H                                                            | -0.019 991 839 368 | -0.082 399 576 000 | 0.004 526 595 337                     |
| H                                                            | -0.040 217 621 229 | -0.005 989 311 723 | 0.054 298 812 850                     |
| H                                                            | 0.009 286 549 707  | -0.003 743 567 866 | -0.000 256 018 053                    |

Axial (R)-(+)-3-methylcyclopentanone

*Initial state*



Wavenumber/cm<sup>-1</sup>: 173.9765

| $\frac{\partial \mu_{x,y,z}}{\partial Q_r} / (e u^{-0.5})$        | 0.001 565 605 766  | -0.000 647 267 375 | -0.003 178 191 722 |
|-------------------------------------------------------------------|--------------------|--------------------|--------------------|
| <i>l</i> -matrix coefficients/(u <sup>1/2</sup> Å <sup>-1</sup> ) |                    |                    |                    |
| O                                                                 | 0.000 634 293 682  | -0.000 716 465 465 | -0.000 684 999 973 |
| C                                                                 | 0.008 990 069 022  | 0.228 041 225 699  | 0.136 741 720 889  |
| C                                                                 | 0.001 858 379 836  | 0.000 765 393 903  | 0.002 314 320 115  |
| C                                                                 | 0.014 489 747 670  | -0.003 827 379 147 | 0.028 996 770 203  |
| C                                                                 | 0.063 088 398 423  | 0.067 630 586 511  | 0.065 405 940 657  |
| C                                                                 | -0.001 669 392 908 | 0.001 330 893 033  | 0.003 789 183 688  |
| C                                                                 | 0.004 117 482 905  | 0.043 746 878 021  | -0.017 900 662 722 |
| H                                                                 | 0.019 624 580 857  | -0.793 702 607 956 | -0.254 314 111 550 |
| H                                                                 | -0.053 340 965 825 | 0.011 929 841 010  | -0.230 260 629 846 |
| H                                                                 | 0.001 903 755 941  | 0.001 028 190 320  | -0.003 523 615 263 |
| H                                                                 | -0.006 487 470 854 | -0.028 772 897 427 | -0.069 116 789 650 |
| H                                                                 | -0.044 035 183 034 | 0.035 384 476 414  | -0.030 099 913 028 |
| H                                                                 | -0.206 133 659 999 | -0.245 781 173 415 | -0.089 495 218 049 |
| H                                                                 | -0.011 262 222 832 | 0.012 202 687 576  | -0.136 936 132 198 |
| H                                                                 | -0.030 951 480 807 | -0.121 120 066 696 | 0.006 363 372 575  |
| H                                                                 | -0.035 147 440 284 | -0.004 828 275 984 | 0.044 770 770 525  |
| H                                                                 | 0.049 605 255 349  | -0.029 177 146 576 | 0.008 158 576 560  |

Wavenumber/cm<sup>-1</sup>: 234.823

| $\frac{\partial \mu_{x,y,z}}{\partial Q_r} / (e \text{ u}^{-0.5})$ | 0.001 366 874 690  | -0.000 463 638 029                    | 0.002 184 339 848  |
|--------------------------------------------------------------------|--------------------|---------------------------------------|--------------------|
| <i>l</i> -matrix coefficients/(u <sup>1/2</sup> Å <sup>-1</sup> )  |                    |                                       |                    |
| O                                                                  | -0.000 285 530 233 | -0.000 223 242 851                    | 0.000 404 139 119  |
| C                                                                  | -0.000 151 468 179 | -0.033 052 153 523                    | -0.020 514 752 876 |
| C                                                                  | -0.007 154 345 785 | 0.003 030 313 967                     | 0.001 340 695 661  |
| C                                                                  | -0.067 109 430 373 | 0.035 208 063 224                     | -0.075 922 491 059 |
| C                                                                  | 0.015 214 164 614  | 0.019 103 276 127                     | 0.002 075 464 768  |
| C                                                                  | 0.001 156 539 989  | -2.084 643 600 000 × 10 <sup>-5</sup> | -0.000 944 529 223 |
| C                                                                  | -0.123 132 545 836 | 0.251 158 129 471                     | -0.030 353 440 290 |
| H                                                                  | -0.001 022 771 006 | 0.108 385 589 631                     | 0.035 435 685 615  |
| H                                                                  | 0.009 892 361 653  | -0.000 750 503 611                    | 0.039 153 429 878  |
| H                                                                  | 0.010 404 500 622  | 0.000 689 662 985                     | -0.011 047 218 820 |
| H                                                                  | 0.015 061 957 323  | 0.051 074 435 947                     | 0.118 863 005 262  |
| H                                                                  | 0.214 619 493 843  | -0.175 493 898 913                    | 0.147 090 650 194  |
| H                                                                  | -0.053 631 918 225 | -0.063 952 694 465                    | -0.025 223 145 066 |
| H                                                                  | 0.002 961 830 121  | 0.000 130 872 671                     | 0.016 516 434 557  |
| H                                                                  | -0.147 665 336 132 | -0.565 171 326 701                    | 0.043 956 156 446  |
| H                                                                  | 0.026 435 492 476  | 0.024 552 469 853                     | -0.046 361 233 159 |
| H                                                                  | 0.549 501 959 044  | -0.329 343 420 161                    | 0.109 153 215 787  |

Wavenumber/cm<sup>-1</sup>: 349.5071

| $\frac{\partial \mu_{x,y,z}}{\partial Q_r} / (e \text{ u}^{-0.5})$ | 0.000 104 918 680  | -0.006 000 759 444 | -0.000 476 475 305                   |
|--------------------------------------------------------------------|--------------------|--------------------|--------------------------------------|
| <i>l</i> -matrix coefficients/(u <sup>1/2</sup> Å <sup>-1</sup> )  |                    |                    |                                      |
| O                                                                  | 0.000 558 041 668  | -0.000 165 707 988 | -0.000 210 790 302                   |
| C                                                                  | 0.000 245 667 736  | 0.002 999 126 647  | 0.001 885 516 126                    |
| C                                                                  | -0.038 911 775 520 | -0.007 641 341 497 | 0.049 952 460 570                    |
| C                                                                  | 0.133 168 227 791  | -0.067 940 634 941 | 0.159 160 449 578                    |
| C                                                                  | -0.038 055 424 145 | -0.047 921 986 525 | 0.003 616 673 033                    |
| C                                                                  | -0.001 368 783 117 | 0.001 153 225 913  | 0.000 555 672 446                    |
| C                                                                  | -0.169 483 515 125 | 0.028 727 029 420  | 0.073 308 681 515                    |
| H                                                                  | 0.000 234 071 688  | -0.007 468 978 008 | -0.001 699 269 395                   |
| H                                                                  | -0.002 378 086 981 | 0.000 811 446 243  | -0.005 728 781 175                   |
| H                                                                  | 0.133 470 989 291  | 0.026 112 535 210  | -0.165 219 185 324                   |
| H                                                                  | -0.023 361 882 294 | -0.111 114 435 642 | -0.261 768 686 880                   |
| H                                                                  | -0.427 460 970 809 | 0.343 562 825 304  | -0.292 960 066 607                   |
| H                                                                  | 0.136 666 913 779  | 0.161 212 262 158  | 0.063 383 095 838                    |
| H                                                                  | -0.009 424 934 692 | 0.000 955 009 710  | -0.072 457 172 148                   |
| H                                                                  | 0.002 363 446 824  | 0.063 719 603 710  | 8.547 821 100 000 × 10 <sup>-5</sup> |
| H                                                                  | 0.247 837 119 169  | 0.050 462 057 844  | -0.331 766 406 547                   |
| H                                                                  | 0.334 756 103 889  | -0.214 757 732 233 | 0.073 144 989 066                    |

Wavenumber/cm<sup>-1</sup>: 367.9687

| $\frac{\partial \mu_{x,y,z}}{\partial Q_r} / (e u^{-0.5})$        | 0.002 975 570 223  | -0.003 619 639 010 | 0.001 548 401 602                    |
|-------------------------------------------------------------------|--------------------|--------------------|--------------------------------------|
| <i>l</i> -matrix coefficients/(u <sup>1/2</sup> Å <sup>-1</sup> ) |                    |                    |                                      |
| O                                                                 | -0.000 286 132 114 | 0.000 379 602 400  | 5.177 819 700 000 × 10 <sup>-5</sup> |
| C                                                                 | 0.004 158 020 172  | 0.033 132 313 705  | 0.023 802 433 977                    |
| C                                                                 | -0.048 821 317 860 | -0.011 382 122 834 | 0.055 474 277 853                    |
| C                                                                 | -0.100 258 129 896 | 0.057 688 622 461  | -0.111 931 238 878                   |
| C                                                                 | 0.012 026 870 561  | 0.016 671 140 505  | -0.013 177 306 210                   |
| C                                                                 | 0.001 716 347 207  | -0.000 528 654 121 | 0.000 316 094 382                    |
| C                                                                 | -0.159 564 790 415 | -0.133 702 559 263 | 0.117 054 460 810                    |
| H                                                                 | 0.001 635 584 746  | -0.116 818 054 030 | -0.036 650 737 468                   |
| H                                                                 | -0.012 312 864 781 | 0.000 148 068 447  | -0.046 774 899 741                   |
| H                                                                 | 0.153 755 216 138  | 0.031 513 760 287  | -0.190 521 401 621                   |
| H                                                                 | 0.016 990 849 539  | 0.070 495 824 550  | 0.165 495 333 579                    |
| H                                                                 | 0.326 908 913 049  | -0.263 605 011 200 | 0.225 197 971 272                    |
| H                                                                 | -0.045 887 585 248 | -0.053 500 831 377 | -0.023 982 665 012                   |
| H                                                                 | 0.008 937 096 452  | -0.002 459 179 989 | 0.063 620 590 922                    |
| H                                                                 | 0.112 272 524 014  | 0.501 379 470 194  | -0.029 592 824 120                   |
| H                                                                 | 0.313 676 043 161  | 0.054 737 438 918  | -0.410 952 503 960                   |
| H                                                                 | 0.128 803 729 346  | -0.091 809 959 545 | 0.037 004 484 531                    |

Wavenumber/cm<sup>-1</sup>: 459.7155

| $\frac{\partial \mu_{x,y,z}}{\partial Q_r} / (e u^{-0.5})$        | 0.016 187 380 884  | 0.054 590 193 419                    | -0.025 073 540 562                   |
|-------------------------------------------------------------------|--------------------|--------------------------------------|--------------------------------------|
| <i>l</i> -matrix coefficients/(u <sup>1/2</sup> Å <sup>-1</sup> ) |                    |                                      |                                      |
| O                                                                 | -0.000 487 608 813 | 8.740 357 600 000 × 10 <sup>-5</sup> | 0.000 202 737 758                    |
| C                                                                 | 0.014 430 398 280  | -0.021 868 879 846                   | 0.047 243 571 843                    |
| C                                                                 | -0.145 326 202 447 | -0.030 703 002 054                   | 0.175 734 726 711                    |
| C                                                                 | -0.028 646 111 374 | 0.066 989 261 415                    | 0.064 025 340 691                    |
| C                                                                 | -0.010 128 134 274 | -0.014 620 532 717                   | -0.009 503 724 581                   |
| C                                                                 | 0.002 427 810 294  | -0.000 289 810 458                   | 2.899 468 300 000 × 10 <sup>-5</sup> |
| C                                                                 | 0.080 379 233 450  | 0.024 973 986 257                    | -0.049 676 732 471                   |
| H                                                                 | -0.002 710 029 803 | 0.071 632 195 254                    | 0.026 568 018 042                    |
| H                                                                 | -0.046 135 321 416 | -0.001 102 717 067                   | -0.192 373 318 419                   |
| H                                                                 | 0.495 933 214 932  | 0.109 477 979 568                    | -0.605 104 181 684                   |
| H                                                                 | -0.041 791 627 863 | -0.125 654 965 691                   | -0.317 417 674 523                   |
| H                                                                 | 0.132 474 139 859  | -0.104 692 948 508                   | 0.098 159 621 030                    |
| H                                                                 | 0.043 275 856 609  | 0.054 434 643 496                    | 0.020 846 898 488                    |
| H                                                                 | -0.001 730 318 616 | -0.002 128 297 702                   | 0.009 452 090 633                    |
| H                                                                 | -0.024 381 604 916 | -0.134 076 132 268                   | 0.008 727 486 414                    |
| H                                                                 | -0.144 393 968 966 | -0.028 003 031 730                   | 0.188 453 783 106                    |
| H                                                                 | -0.108 748 154 879 | 0.075 257 008 379                    | -0.024 662 004 729                   |

Wavenumber/cm<sup>-1</sup>: 475.9186

| $\frac{\partial \mu_{x,y,z}}{\partial Q_r} / (e u^{-0.5})$        | 0.010 755 248 322  | 0.032 902 228 671  | -0.020 619 308 647 |
|-------------------------------------------------------------------|--------------------|--------------------|--------------------|
| <i>l</i> -matrix coefficients/(u <sup>1/2</sup> Å <sup>-1</sup> ) |                    |                    |                    |
| O                                                                 | -0.000 194 360 646 | -0.000 150 866 755 | -0.000 183 663 305 |
| C                                                                 | -0.002 074 060 292 | 0.002 064 264 678  | -0.011 826 252 040 |
| C                                                                 | 0.011 287 270 928  | 0.003 479 369 560  | -0.014 245 637 326 |
| C                                                                 | -0.036 200 947 059 | 0.035 505 271 720  | -0.020 158 830 688 |
| C                                                                 | -0.032 208 772 412 | -0.081 731 836 963 | 0.221 138 425 640  |
| C                                                                 | -0.000 164 137 617 | -0.000 494 187 995 | 0.002 531 513 097  |
| C                                                                 | 0.005 897 371 738  | -0.003 286 631 252 | 0.011 608 276 773  |
| H                                                                 | 0.000 280 340 172  | -0.008 362 027 929 | -0.003 164 681 995 |
| H                                                                 | 0.010 547 988 834  | 0.000 667 618 975  | 0.044 149 129 800  |
| H                                                                 | -0.039 549 512 931 | -0.008 641 378 834 | 0.048 124 781 372  |
| H                                                                 | -0.004 671 604 267 | -0.007 027 608 798 | -0.028 418 695 242 |
| H                                                                 | 0.134 442 000 556  | -0.111 261 380 051 | 0.095 897 378 174  |
| H                                                                 | 0.202 644 560 104  | 0.233 857 689 588  | 0.108 512 952 827  |
| H                                                                 | -0.102 666 327 737 | 0.042 639 173 704  | -0.876 905 388 241 |
| H                                                                 | -0.002 983 500 254 | -0.017 449 729 859 | 0.001 569 584 106  |
| H                                                                 | 0.025 413 968 180  | 0.005 449 122 784  | -0.034 066 919 975 |
| H                                                                 | -0.038 129 315 241 | 0.024 217 640 414  | -0.007 554 917 338 |

Wavenumber/cm<sup>-1</sup>: 582.873

| $\frac{\partial \mu_{x,y,z}}{\partial Q_r} / (e u^{-0.5})$        | 0.011 887 261 230  | 0.002 400 104 636  | -0.004 261 035 560                    |
|-------------------------------------------------------------------|--------------------|--------------------|---------------------------------------|
| <i>l</i> -matrix coefficients/(u <sup>1/2</sup> Å <sup>-1</sup> ) |                    |                    |                                       |
| O                                                                 | -0.000 473 613 268 | 0.000 591 614 865  | -3.115 201 300 000 × 10 <sup>-5</sup> |
| C                                                                 | -0.004 975 620 089 | 0.009 518 554 542  | -0.019 774 152 347                    |
| C                                                                 | 0.068 211 912 941  | 0.013 194 252 625  | -0.079 868 225 911                    |
| C                                                                 | -0.041 536 302 438 | 0.135 459 109 710  | 0.162 981 357 431                     |
| C                                                                 | -0.012 866 775 002 | -0.009 708 664 837 | -0.043 507 923 189                    |
| C                                                                 | -0.000 421 485 809 | -0.001 638 363 855 | -0.000 358 099 378                    |
| C                                                                 | -0.034 381 350 845 | -0.014 284 276 617 | -0.006 403 361 711                    |
| H                                                                 | 0.000 442 586 765  | -0.032 521 413 898 | -0.013 044 376 766                    |
| H                                                                 | 0.018 448 168 524  | 0.001 331 382 181  | 0.080 711 313 773                     |
| H                                                                 | -0.231 176 898 864 | -0.046 761 583 974 | 0.279 725 264 832                     |
| H                                                                 | -0.094 312 384 003 | -0.284 345 500 350 | -0.735 358 455 769                    |
| H                                                                 | 0.232 328 920 202  | -0.177 267 906 207 | 0.174 459 551 452                     |
| H                                                                 | 0.030 437 391 466  | 0.042 335 964 086  | 0.011 730 131 078                     |
| H                                                                 | 0.019 030 370 861  | -0.008 713 052 142 | 0.139 041 116 000                     |
| H                                                                 | 0.023 996 773 718  | 0.111 028 001 237  | -0.007 893 330 035                    |
| H                                                                 | -0.005 625 876 202 | -0.000 829 809 104 | 0.005 518 690 717                     |
| H                                                                 | 0.097 964 519 455  | -0.064 140 896 142 | 0.020 118 203 661                     |

Wavenumber/cm<sup>-1</sup>: 672.4893

| $\frac{\partial \mu_{x,y,z}}{\partial Q_r} / (e u^{-0.5})$        |                    |                    |                    |
|-------------------------------------------------------------------|--------------------|--------------------|--------------------|
|                                                                   | -0.002 652 950 897 | 0.021 895 448 523  | -0.008 557 225 671 |
| <i>l</i> -matrix coefficients/(u <sup>1/2</sup> Å <sup>-1</sup> ) |                    |                    |                    |
| O                                                                 | 0.000 426 957 615  | -0.000 235 720 057 | -0.000 152 079 021 |
| C                                                                 | 0.043 849 464 946  | -0.049 748 077 983 | 0.155 921 968 363  |
| C                                                                 | 0.023 888 339 176  | 0.006 941 382 011  | -0.026 731 898 254 |
| C                                                                 | 0.007 180 901 682  | -0.013 005 285 085 | -0.013 334 019 363 |
| C                                                                 | -0.002 359 194 838 | -0.006 235 092 354 | 0.019 634 067 068  |
| C                                                                 | -0.000 391 461 584 | 0.000 835 322 111  | 0.002 222 461 544  |
| C                                                                 | -0.048 681 922 472 | -0.032 135 672 418 | -0.104 842 674 935 |
| H                                                                 | -0.003 017 235 914 | 0.178 679 560 737  | 0.071 724 466 225  |
| H                                                                 | -0.145 439 663 806 | -0.012 419 831 468 | -0.618 119 135 101 |
| H                                                                 | -0.082 316 336 969 | -0.018 989 440 228 | 0.099 217 706 417  |
| H                                                                 | 0.008 572 096 151  | 0.024 049 474 911  | 0.065 950 397 831  |
| H                                                                 | -0.030 760 995 581 | 0.022 089 824 729  | -0.022 733 622 071 |
| H                                                                 | 0.015 058 541 678  | 0.017 427 266 191  | 0.008 641 455 246  |
| H                                                                 | -0.008 502 479 144 | 0.004 342 193 399  | -0.074 790 934 162 |
| H                                                                 | 0.086 938 335 839  | 0.368 760 518 817  | -0.034 587 711 251 |
| H                                                                 | -0.259 453 309 330 | -0.051 146 696 651 | 0.329 471 933 034  |
| H                                                                 | 0.336 146 332 132  | -0.209 620 139 007 | 0.062 365 028 339  |

Wavenumber/cm<sup>-1</sup>: 737.6533

| $\frac{\partial \mu_{x,y,z}}{\partial Q_r} / (e u^{-0.5})$        |                    |                                       |                    |
|-------------------------------------------------------------------|--------------------|---------------------------------------|--------------------|
|                                                                   | 0.001 948 693 444  | -0.007 452 265 661                    | 0.001 985 694 864  |
| <i>l</i> -matrix coefficients/(u <sup>1/2</sup> Å <sup>-1</sup> ) |                    |                                       |                    |
| O                                                                 | -0.000 536 463 952 | 0.000 455 913 794                     | 0.000 741 354 363  |
| C                                                                 | -0.041 937 830 858 | 0.047 211 666 461                     | -0.158 645 602 711 |
| C                                                                 | -0.031 489 992 848 | -0.008 534 645 264                    | 0.040 845 972 815  |
| C                                                                 | 0.006 332 121 025  | -0.013 366 743 766                    | -0.012 252 569 472 |
| C                                                                 | 0.002 400 551 839  | -0.000 564 172 472                    | 0.009 982 514 048  |
| C                                                                 | -0.000 101 574 937 | -3.884 258 700 000 × 10 <sup>-5</sup> | -0.002 617 696 175 |
| C                                                                 | -0.020 847 570 698 | -0.027 120 132 879                    | -0.114 602 382 822 |
| H                                                                 | 0.000 942 030 375  | -0.169 734 790 176                    | -0.069 495 529 649 |
| H                                                                 | 0.142 695 473 487  | 0.010 817 538 705                     | 0.623 506 915 221  |
| H                                                                 | 0.113 237 439 300  | 0.028 027 993 455                     | -0.139 940 579 838 |
| H                                                                 | 0.007 852 233 990  | 0.022 794 481 023                     | 0.061 690 540 601  |
| H                                                                 | -0.028 265 260 042 | 0.021 385 724 438                     | -0.020 532 697 276 |
| H                                                                 | -0.000 398 737 569 | -0.001 006 067 646                    | 0.000 783 716 753  |
| H                                                                 | -0.007 690 992 075 | 0.002 417 033 497                     | -0.035 711 533 508 |
| H                                                                 | 0.080 387 360 356  | 0.330 243 854 250                     | -0.032 218 161 533 |
| H                                                                 | -0.299 106 536 859 | -0.059 831 133 336                    | 0.377 896 357 854  |
| H                                                                 | 0.288 126 853 473  | -0.178 601 846 241                    | 0.050 187 294 216  |

Wavenumber/cm<sup>-1</sup>: 794.8424

| $\frac{\partial \mu_{x,y,z}}{\partial Q_r} / (e \text{ u}^{-0.5})$ | 0.001 993 802 939  | -0.020 224 664 947 | 0.008 639 166 363  |
|--------------------------------------------------------------------|--------------------|--------------------|--------------------|
| <i>l</i> -matrix coefficients/(u <sup>1/2</sup> Å <sup>-1</sup> )  |                    |                    |                    |
| O                                                                  | -0.557 411 897 369 | 0.174 734 045 420  | 0.133 913 179 175  |
| C                                                                  | -0.039 348 289 190 | 0.012 917 095 817  | 0.009 583 550 756  |
| C                                                                  | -0.021 592 276 501 | 0.005 516 109 404  | 0.005 691 950 336  |
| C                                                                  | -0.020 589 896 713 | 0.007 608 976 192  | 0.000 595 127 264  |
| C                                                                  | -0.038 550 456 107 | 0.010 493 330 155  | 0.012 479 992 729  |
| C                                                                  | 0.739 995 685 393  | -0.232 016 575 170 | -0.175 760 436 342 |
| C                                                                  | 0.002 753 434 843  | 0.001 124 256 529  | -0.001 342 266 083 |
| H                                                                  | 0.041 694 394 014  | 0.007 090 189 670  | -0.016 582 038 850 |
| H                                                                  | 0.003 551 570 868  | 0.000 924 675 652  | -0.003 126 901 581 |
| H                                                                  | -0.006 074 445 131 | -0.001 531 542 168 | 0.004 069 966 085  |
| H                                                                  | 0.009 195 721 512  | -0.000 215 250 779 | -0.000 108 117 392 |
| H                                                                  | -0.006 798 694 012 | 0.004 623 217 739  | -0.000 740 073 178 |
| H                                                                  | 0.030 113 037 321  | -0.023 194 601 306 | -0.006 628 785 312 |
| H                                                                  | -0.001 601 691 819 | -0.007 508 794 698 | 0.002 326 357 037  |
| H                                                                  | 0.001 650 913 517  | -0.000 389 643 161 | -0.003 031 501 236 |
| H                                                                  | -0.000 577 346 131 | -0.005 714 983 438 | -0.001 849 592 891 |
| H                                                                  | 0.000 180 829 735  | 0.000 678 478 318  | 0.005 639 346 540  |

Wavenumber/cm<sup>-1</sup>: 813.0515

| $\frac{\partial \mu_{x,y,z}}{\partial Q_r} / (e \text{ u}^{-0.5})$ | 0.006 317 423 475  | -0.003 254 990 722                   | -0.001 133 283 395 |
|--------------------------------------------------------------------|--------------------|--------------------------------------|--------------------|
| <i>l</i> -matrix coefficients/(u <sup>1/2</sup> Å <sup>-1</sup> )  |                    |                                      |                    |
| O                                                                  | 0.004 436 266 354  | 4.538 886 000 000 × 10 <sup>-6</sup> | -0.001 667 780 832 |
| C                                                                  | 0.037 254 016 498  | -0.033 017 835 722                   | 0.014 842 640 610  |
| C                                                                  | -0.075 472 700 277 | -0.018 027 650 222                   | 0.022 875 379 345  |
| C                                                                  | -0.106 983 466 441 | 0.169 840 080 817                    | 0.076 878 883 682  |
| C                                                                  | 0.010 226 411 041  | 0.022 903 421 722                    | -0.006 994 222 791 |
| C                                                                  | -0.004 824 273 687 | -0.007 159 718 673                   | 0.007 574 213 972  |
| C                                                                  | -0.084 703 205 200 | -0.041 721 520 382                   | 0.034 917 257 117  |
| H                                                                  | -0.040 347 839 891 | 0.017 554 013 741                    | -0.082 363 695 984 |
| H                                                                  | -0.021 019 454 933 | 0.089 142 152 528                    | 0.008 865 560 386  |
| H                                                                  | 0.031 481 546 127  | 0.027 785 225 270                    | 0.063 483 240 346  |
| H                                                                  | 0.355 954 261 233  | -0.347 669 546 711                   | 0.119 936 665 131  |
| H                                                                  | 0.031 599 077 322  | -0.272 618 799 407                   | -0.423 767 502 220 |
| H                                                                  | 0.001 728 676 697  | 0.000 206 764 796                    | 0.024 051 374 078  |
| H                                                                  | -0.011 652 440 720 | -0.014 318 770 677                   | 0.000 974 711 898  |
| H                                                                  | 0.381 595 111 596  | -0.103 291 520 962                   | 0.016 726 230 824  |
| H                                                                  | -0.192 041 495 312 | -0.060 447 451 536                   | -0.140 411 802 344 |
| H                                                                  | 0.220 009 131 535  | 0.343 238 026 726                    | -0.098 972 484 473 |

Wavenumber/cm<sup>-1</sup>: 884.8141

| $\frac{\partial \mu_{x,y,z}}{\partial Q_r} / (e u^{-0.5})$        | 0.003 140 912 006  | -0.031 592 167 441 | 0.012 981 775 630  |
|-------------------------------------------------------------------|--------------------|--------------------|--------------------|
| <i>l</i> -matrix coefficients/(u <sup>1/2</sup> Å <sup>-1</sup> ) |                    |                    |                    |
| O                                                                 | 0.004 654 705 304  | -0.003 479 779 119 | 0.000 473 121 904  |
| C                                                                 | 0.001 468 257 656  | -0.016 716 122 089 | 0.006 436 081 176  |
| C                                                                 | -0.066 943 907 407 | 0.070 568 563 124  | -0.014 734 082 165 |
| C                                                                 | 0.060 720 202 603  | -0.073 257 022 248 | -0.031 037 573 542 |
| C                                                                 | -0.018 259 496 366 | -0.019 968 420 377 | 0.019 995 684 030  |
| C                                                                 | -0.003 015 782 031 | 0.009 562 148 765  | -0.001 475 919 955 |
| C                                                                 | -0.106 793 771 029 | 0.123 708 640 734  | 0.028 740 260 622  |
| H                                                                 | 0.011 433 450 842  | -0.002 881 201 533 | -0.003 018 783 412 |
| H                                                                 | 0.006 138 778 050  | 0.002 627 831 270  | 0.000 606 953 000  |
| H                                                                 | 0.035 480 843 462  | -0.038 518 109 932 | 0.031 843 219 290  |
| H                                                                 | -0.136 841 722 337 | 0.139 648 479 895  | -0.050 011 930 459 |
| H                                                                 | -0.033 064 793 859 | 0.079 503 927 648  | 0.173 797 498 007  |
| H                                                                 | 0.010 318 112 226  | 0.010 295 376 515  | -0.068 806 412 913 |
| H                                                                 | 0.048 699 096 989  | 0.053 526 885 970  | 0.001 468 002 935  |
| H                                                                 | 0.407 140 919 230  | -0.111 619 356 046 | -0.413 517 901 060 |
| H                                                                 | 0.079 544 577 596  | -0.613 395 090 638 | -0.013 841 875 612 |
| H                                                                 | 0.011 113 758 981  | 0.170 541 524 040  | 0.312 241 217 312  |

Wavenumber/cm<sup>-1</sup>: 936.0508

| $\frac{\partial \mu_{x,y,z}}{\partial Q_r} / (e u^{-0.5})$        | 0.001 374 591 724  | -0.006 105 235 341 | 0.007 559 534 652  |
|-------------------------------------------------------------------|--------------------|--------------------|--------------------|
| <i>l</i> -matrix coefficients/(u <sup>1/2</sup> Å <sup>-1</sup> ) |                    |                    |                    |
| O                                                                 | -0.005 075 750 150 | 0.000 629 628 392  | 0.000 451 776 819  |
| C                                                                 | 0.002 519 899 433  | 0.018 954 730 585  | -0.008 513 722 325 |
| C                                                                 | -0.026 663 930 449 | -0.076 311 889 842 | 0.009 742 663 767  |
| C                                                                 | 0.094 021 816 373  | -0.103 912 888 765 | -0.065 959 925 154 |
| C                                                                 | -0.014 706 623 158 | -0.030 036 222 326 | 0.012 658 512 554  |
| C                                                                 | 0.008 717 015 700  | 0.002 359 942 313  | 0.005 008 155 837  |
| C                                                                 | -0.039 286 741 949 | -0.097 159 346 356 | 0.096 642 197 567  |
| H                                                                 | -0.015 213 598 211 | -0.005 620 415 134 | 0.025 736 243 769  |
| H                                                                 | 0.005 326 050 213  | -0.023 331 558 461 | -0.004 670 228 983 |
| H                                                                 | 0.011 381 179 748  | 0.033 526 748 352  | 0.028 903 875 236  |
| H                                                                 | -0.278 925 091 585 | 0.245 978 871 240  | -0.082 706 134 308 |
| H                                                                 | -0.035 021 339 429 | 0.201 812 940 191  | 0.320 186 533 230  |
| H                                                                 | -0.000 570 535 483 | 0.012 391 521 307  | -0.061 531 909 012 |
| H                                                                 | 0.034 838 332 264  | 0.051 816 575 413  | 0.001 489 209 766  |
| H                                                                 | 0.276 253 910 216  | -0.075 408 828 928 | 0.174 845 535 744  |
| H                                                                 | -0.347 986 877 693 | 0.218 340 277 642  | -0.210 140 583 962 |
| H                                                                 | 0.285 216 456 234  | 0.325 616 947 518  | -0.365 054 401 585 |

Wavenumber/cm<sup>-1</sup>: 964.5509

| $\frac{\partial \mu_{x,y,z}}{\partial Q_r} / (e u^{-0.5})$        | 0.024 513 921 874  | 0.030 757 459 697  | -0.018 130 496 338 |
|-------------------------------------------------------------------|--------------------|--------------------|--------------------|
| <i>l</i> -matrix coefficients/(u <sup>1/2</sup> Å <sup>-1</sup> ) |                    |                    |                    |
| O                                                                 | -0.000 528 202 796 | 0.002 315 930 519  | -0.001 004 965 070 |
| C                                                                 | -0.061 343 762 019 | 0.100 238 117 029  | -0.071 965 676 535 |
| C                                                                 | 0.031 114 291 962  | 0.023 806 730 548  | -0.002 944 260 322 |
| C                                                                 | -0.032 940 853 104 | -0.004 642 922 828 | 0.031 056 946 513  |
| C                                                                 | -0.119 499 026 383 | -0.121 582 966 505 | 0.145 832 720 115  |
| C                                                                 | -0.010 452 307 663 | -0.012 613 139 867 | 0.011 122 628 414  |
| C                                                                 | 0.032 319 881 062  | 0.012 499 030 426  | 0.061 475 210 501  |
| H                                                                 | 0.109 453 529 156  | -0.074 051 792 641 | 0.291 820 562 886  |
| H                                                                 | 0.043 314 467 732  | -0.302 058 512 992 | -0.022 564 585 463 |
| H                                                                 | -0.012 067 215 437 | -0.022 333 662 977 | -0.028 324 485 210 |
| H                                                                 | 0.103 515 354 629  | -0.066 048 298 224 | 0.017 490 146 727  |
| H                                                                 | 0.035 973 055 646  | -0.048 863 095 590 | -0.106 609 535 161 |
| H                                                                 | 0.054 865 857 252  | 0.132 711 853 929  | -0.566 512 695 301 |
| H                                                                 | 0.365 002 924 375  | 0.438 659 214 969  | 0.009 061 324 770  |
| H                                                                 | -0.063 360 822 050 | 0.012 750 989 175  | -0.070 667 728 924 |
| H                                                                 | -0.062 506 542 963 | -0.007 126 770 103 | -0.037 146 991 522 |
| H                                                                 | -0.017 001 408 188 | -0.064 943 957 821 | -0.085 180 734 161 |

Wavenumber/cm<sup>-1</sup>: 1000.3539

| $\frac{\partial \mu_{x,y,z}}{\partial Q_r} / (e u^{-0.5})$        | -0.008 136 764 394 | -0.019 795 575 160 | 0.009 890 021 369  |
|-------------------------------------------------------------------|--------------------|--------------------|--------------------|
| <i>l</i> -matrix coefficients/(u <sup>1/2</sup> Å <sup>-1</sup> ) |                    |                    |                    |
| O                                                                 | -0.002 314 006 102 | -0.001 642 782 141 | 0.000 917 772 949  |
| C                                                                 | -0.073 638 942 523 | 0.183 942 018 670  | -0.120 669 303 698 |
| C                                                                 | 0.012 554 493 721  | 0.013 499 878 508  | -0.023 743 272 141 |
| C                                                                 | -0.021 750 277 036 | 0.016 277 730 932  | 0.008 513 889 944  |
| C                                                                 | 0.069 491 544 361  | 0.080 799 856 849  | -0.070 784 502 284 |
| C                                                                 | -0.001 973 313 822 | 0.023 891 312 946  | -0.032 213 612 241 |
| C                                                                 | -0.006 782 197 777 | 0.009 566 992 058  | 0.042 513 588 535  |
| H                                                                 | 0.170 713 118 955  | -0.142 374 860 251 | 0.544 627 186 766  |
| H                                                                 | 0.055 586 188 403  | -0.576 673 644 360 | -0.032 037 103 094 |
| H                                                                 | 0.006 377 742 821  | -0.000 709 358 397 | -0.006 390 241 442 |
| H                                                                 | 0.040 258 655 465  | -0.014 062 019 803 | 0.001 492 942 766  |
| H                                                                 | 0.002 868 324 986  | -0.017 441 878 518 | -0.032 993 832 841 |
| H                                                                 | -0.027 635 306 297 | -0.074 053 979 913 | 0.321 870 645 044  |
| H                                                                 | -0.203 782 199 710 | -0.269 790 333 382 | -0.002 875 328 795 |
| H                                                                 | 0.056 579 802 213  | -0.017 094 807 651 | -0.057 763 706 628 |
| H                                                                 | -0.041 698 405 820 | -0.046 101 781 521 | -0.029 194 100 550 |
| H                                                                 | 0.026 235 549 682  | 0.032 674 291 044  | -0.032 481 676 932 |



Wavenumber/cm<sup>-1</sup>: 1007.6883

| $\frac{\partial \mu_{x,y,z}}{\partial Q_r} / (e u^{-0.5})$        | -0.026 829 607 577 | 0.015 642 419 016  | 0.000 112 437 128  |
|-------------------------------------------------------------------|--------------------|--------------------|--------------------|
| <i>l</i> -matrix coefficients/(u <sup>1/2</sup> Å <sup>-1</sup> ) |                    |                    |                    |
| O                                                                 | 0.006 451 601 697  | 0.001 679 431 655  | -0.005 411 576 615 |
| C                                                                 | -0.011 712 330 588 | -0.025 470 815 567 | 0.041 847 864 970  |
| C                                                                 | -0.050 552 604 102 | -0.038 959 981 542 | -0.081 892 586 763 |
| C                                                                 | -0.045 024 039 078 | -0.018 196 419 208 | 0.041 723 735 669  |
| C                                                                 | 0.021 284 304 902  | 0.036 289 460 600  | -0.027 209 704 229 |
| C                                                                 | -0.000 152 262 344 | -0.012 261 185 756 | 0.015 031 927 713  |
| C                                                                 | 0.218 132 539 467  | 0.143 780 972 534  | 0.342 266 499 643  |
| H                                                                 | -0.021 501 205 724 | 0.033 444 395 110  | -0.103 164 942 467 |
| H                                                                 | 0.043 339 894 087  | 0.093 966 926 492  | -0.005 228 183 069 |
| H                                                                 | 0.078 323 664 317  | 0.054 319 424 772  | 0.062 931 207 006  |
| H                                                                 | 0.074 003 392 665  | 0.047 563 189 312  | -0.020 632 570 871 |
| H                                                                 | 0.029 571 268 107  | -0.003 137 556 098 | -0.039 618 571 068 |
| H                                                                 | 0.005 064 526 977  | -0.024 218 195 971 | 0.082 531 550 272  |
| H                                                                 | -0.045 858 132 886 | -0.059 192 750 815 | -0.002 330 954 750 |
| H                                                                 | -0.208 931 466 159 | 0.058 545 509 586  | -0.440 471 274 938 |
| H                                                                 | -0.369 512 207 921 | -0.198 390 312 721 | -0.280 100 159 012 |
| H                                                                 | -0.065 780 822 688 | -0.303 638 437 022 | -0.377 612 123 398 |

Wavenumber/cm<sup>-1</sup>: 1041.2194

| $\frac{\partial \mu_{x,y,z}}{\partial Q_r} / (e u^{-0.5})$        | 0.005 236 201 513  | -0.015 077 450 609 | -0.000 983 730 256 |
|-------------------------------------------------------------------|--------------------|--------------------|--------------------|
| <i>l</i> -matrix coefficients/(u <sup>1/2</sup> Å <sup>-1</sup> ) |                    |                    |                    |
| O                                                                 | -0.014 605 368 299 | -0.004 011 895 067 | 0.002 872 776 338  |
| C                                                                 | 0.027 667 836 135  | 0.000 498 842 365  | 0.086 598 863 563  |
| C                                                                 | -0.349 872 645 729 | -0.150 577 281 938 | -0.322 851 737 779 |
| C                                                                 | -0.016 625 319 681 | 0.003 466 542 804  | 0.090 657 697 522  |
| C                                                                 | 0.047 272 689 320  | -0.046 621 101 783 | 0.021 309 840 593  |
| C                                                                 | 0.006 644 895 451  | 0.043 239 630 702  | 0.003 614 954 425  |
| C                                                                 | 0.147 603 597 373  | 0.028 928 509 224  | -0.100 040 647 883 |
| H                                                                 | -0.104 031 149 414 | -0.010 685 788 442 | 0.036 192 609 193  |
| H                                                                 | 0.153 377 492 767  | -0.078 132 783 015 | -0.009 580 187 103 |
| H                                                                 | 0.491 432 477 142  | 0.244 269 964 594  | 0.444 280 545 187  |
| H                                                                 | 0.126 676 511 890  | 0.195 162 288 887  | -0.068 823 392 550 |
| H                                                                 | -0.079 467 696 528 | -0.080 089 171 011 | 0.030 600 306 014  |
| H                                                                 | -0.014 939 693 515 | 0.027 672 282 909  | -0.032 775 076 830 |
| H                                                                 | -0.026 325 983 627 | 0.064 553 317 278  | 0.013 921 742 038  |
| H                                                                 | -0.031 884 657 410 | 0.044 576 314 594  | 0.180 996 273 425  |
| H                                                                 | 0.019 664 746 169  | 0.018 151 574 394  | -0.034 885 509 412 |
| H                                                                 | -0.002 325 111 713 | 0.008 419 394 077  | 0.190 517 767 364  |

Wavenumber/cm<sup>-1</sup>: 1125.4678

| $\frac{\partial \mu_{x,y,z}}{\partial Q_r} / (e u^{-0.5})$        | 0.016 029 031 849  | 0.028 268 371 842  | -0.011 898 670 155 |
|-------------------------------------------------------------------|--------------------|--------------------|--------------------|
| <i>l</i> -matrix coefficients/(u <sup>1/2</sup> Å <sup>-1</sup> ) |                    |                    |                    |
| O                                                                 | -0.005 191 890 963 | -0.032 416 056 039 | 0.018 237 201 793  |
| C                                                                 | -0.012 785 326 305 | -0.091 368 492 585 | 0.071 383 485 977  |
| C                                                                 | -0.214 434 271 783 | 0.240 254 324 563  | -0.001 806 901 540 |
| C                                                                 | 0.339 120 532 864  | 0.200 669 985 348  | -0.152 732 969 598 |
| C                                                                 | -0.057 749 656 479 | -0.108 281 759 453 | 0.026 448 909 808  |
| C                                                                 | 0.030 288 772 109  | 0.149 074 378 863  | -0.083 268 584 399 |
| C                                                                 | 0.078 657 680 224  | -0.041 800 157 065 | 0.023 731 824 575  |
| H                                                                 | 0.018 415 671 357  | -0.028 851 382 019 | 0.022 706 504 726  |
| H                                                                 | 0.041 313 037 307  | -0.025 363 676 710 | 0.012 818 953 953  |
| H                                                                 | 0.160 152 522 372  | -0.442 465 651 398 | 0.092 502 522 634  |
| H                                                                 | -0.312 378 784 130 | -0.302 331 558 540 | 0.144 618 837 957  |
| H                                                                 | -0.283 658 295 998 | -0.290 251 279 763 | 0.106 514 279 012  |
| H                                                                 | -0.064 873 989 460 | -0.001 010 427 569 | 0.029 135 461 300  |
| H                                                                 | 0.046 574 114 790  | -0.028 616 876 034 | 0.002 897 136 716  |
| H                                                                 | -0.095 680 573 253 | 0.015 046 740 703  | -0.032 818 710 064 |
| H                                                                 | -0.068 648 350 153 | 0.042 097 908 773  | -0.052 733 297 685 |
| H                                                                 | 0.016 459 164 870  | -0.012 287 941 917 | 0.002 972 820 814  |

Wavenumber/cm<sup>-1</sup>: 1159.1253

| $\frac{\partial \mu_{x,y,z}}{\partial Q_r} / (e u^{-0.5})$        | -0.004 856 128 148 | -0.005 074 689 902 | 0.007 835 182 045  |
|-------------------------------------------------------------------|--------------------|--------------------|--------------------|
| <i>l</i> -matrix coefficients/(u <sup>1/2</sup> Å <sup>-1</sup> ) |                    |                    |                    |
| O                                                                 | -0.076 127 879 921 | 0.032 059 279 226  | 0.019 995 798 053  |
| C                                                                 | 0.295 806 107 172  | 0.116 852 164 949  | -0.129 342 549 125 |
| C                                                                 | -0.031 087 570 624 | -0.325 672 632 094 | 0.097 061 235 593  |
| C                                                                 | 0.099 529 267 869  | 0.251 719 931 138  | -0.012 485 807 369 |
| C                                                                 | 0.148 014 920 329  | -0.190 802 281 908 | -0.050 564 051 128 |
| C                                                                 | -0.017 013 064 077 | -0.046 206 094 252 | -0.002 453 771 927 |
| C                                                                 | 0.024 440 301 959  | 0.108 178 526 452  | -0.009 664 837 184 |
| H                                                                 | -0.307 926 809 916 | -0.018 102 680 563 | 0.088 980 289 102  |
| H                                                                 | -0.258 780 124 555 | -0.059 830 450 082 | 0.044 050 162 532  |
| H                                                                 | -0.192 332 319 653 | 0.365 015 328 330  | -0.037 248 511 571 |
| H                                                                 | -0.214 141 159 520 | -0.146 256 260 658 | 0.116 339 563 231  |
| H                                                                 | -0.156 817 271 423 | -0.095 244 074 089 | 0.066 880 629 965  |
| H                                                                 | -0.260 517 729 482 | 0.184 596 496 518  | 0.032 210 041 146  |
| H                                                                 | -0.040 280 549 829 | 0.111 855 957 198  | 0.003 052 682 376  |
| H                                                                 | 0.016 373 356 633  | 0.021 144 093 449  | 0.023 355 371 261  |
| H                                                                 | -0.012 630 120 256 | -0.105 672 271 121 | -0.039 807 418 598 |
| H                                                                 | -0.063 607 983 077 | -0.088 602 746 552 | -0.006 562 983 089 |

Wavenumber/cm<sup>-1</sup>: 1177.3215

| $\frac{\partial \mu_{x,y,z}}{\partial Q_r} / (e u^{-0.5})$        | 0.001 760 886 431  | 0.018 750 133 415  | -0.002 760 724 821 |
|-------------------------------------------------------------------|--------------------|--------------------|--------------------|
| <i>l</i> -matrix coefficients/(u <sup>1/2</sup> Å <sup>-1</sup> ) |                    |                    |                    |
| O                                                                 | 0.050 264 295 990  | -0.006 164 326 164 | 0.004 690 890 665  |
| C                                                                 | -0.017 355 480 119 | 0.041 988 249 101  | -0.010 597 743 040 |
| C                                                                 | -0.011 671 445 756 | -0.086 763 363 149 | 0.114 122 391 120  |
| C                                                                 | 0.070 861 270 493  | -0.021 801 448 254 | 0.124 891 040 509  |
| C                                                                 | -0.278 209 566 366 | 0.205 547 293 484  | -0.102 809 955 882 |
| C                                                                 | -0.026 535 397 969 | -0.086 909 068 067 | -0.067 029 977 622 |
| C                                                                 | 0.063 085 702 300  | 0.048 395 413 617  | -0.106 977 098 443 |
| H                                                                 | 0.079 528 149 749  | 0.017 325 959 790  | -0.014 123 558 558 |
| H                                                                 | -0.107 394 927 255 | -0.016 265 549 110 | 0.021 265 572 563  |
| H                                                                 | 0.133 625 841 565  | 0.184 462 450 319  | 0.180 006 535 592  |
| H                                                                 | -0.365 205 245 398 | -0.195 382 392 693 | 0.158 333 161 916  |
| H                                                                 | 0.279 373 807 151  | 0.153 963 416 307  | -0.154 257 206 386 |
| H                                                                 | 0.068 920 343 338  | -0.086 645 551 333 | 0.026 107 918 337  |
| H                                                                 | 0.474 426 107 627  | -0.304 066 077 642 | -0.111 624 796 659 |
| H                                                                 | -0.002 735 577 247 | 0.023 734 747 743  | 0.074 978 616 195  |
| H                                                                 | -0.043 592 014 345 | -0.063 253 529 939 | -0.085 377 137 351 |
| H                                                                 | -0.027 411 489 196 | -0.036 090 301 557 | 0.053 082 565 269  |

Wavenumber/cm<sup>-1</sup>: 1206.8324

| $\frac{\partial \mu_{x,y,z}}{\partial Q_r} / (e u^{-0.5})$        | 0.006 795 038 200  | 0.003 591 744 611  | -0.000 862 737 461 |
|-------------------------------------------------------------------|--------------------|--------------------|--------------------|
| <i>l</i> -matrix coefficients/(u <sup>1/2</sup> Å <sup>-1</sup> ) |                    |                    |                    |
| O                                                                 | -0.023 478 829 389 | -0.033 717 280 677 | 0.030 625 103 580  |
| C                                                                 | 0.433 495 199 245  | 0.008 063 407 439  | -0.081 450 649 443 |
| C                                                                 | -0.231 491 588 584 | 0.101 640 878 462  | -0.037 029 372 693 |
| C                                                                 | 0.089 080 820 762  | -0.146 414 421 124 | -0.021 392 979 639 |
| C                                                                 | -0.210 718 661 016 | 0.204 274 667 380  | 0.112 057 008 930  |
| C                                                                 | -0.001 095 034 831 | 0.058 080 744 615  | -0.054 643 180 149 |
| C                                                                 | 0.049 566 729 304  | -0.057 668 539 015 | 0.056 977 921 609  |
| H                                                                 | -0.397 991 957 494 | -0.054 767 395 722 | 0.107 880 937 308  |
| H                                                                 | -0.328 628 527 438 | -0.066 466 108 049 | 0.085 317 926 273  |
| H                                                                 | -0.124 783 103 252 | -0.108 275 209 497 | -0.081 541 470 335 |
| H                                                                 | 0.193 491 248 726  | 0.162 783 791 999  | -0.110 699 108 574 |
| H                                                                 | -0.031 831 047 400 | -0.101 188 316 174 | 0.006 182 894 254  |
| H                                                                 | 0.297 712 893 763  | -0.210 220 426 718 | -0.061 296 455 825 |
| H                                                                 | 0.095 411 629 028  | -0.144 971 198 138 | 0.005 325 316 498  |
| H                                                                 | -0.064 035 624 686 | -0.000 992 557 990 | -0.039 245 435 339 |
| H                                                                 | -0.019 338 378 876 | 0.048 757 253 047  | 0.003 525 536 469  |
| H                                                                 | 0.028 789 822 454  | 0.029 819 874 548  | 0.050 497 813 117  |

Wavenumber/cm<sup>-1</sup>: 1232.4535

| $\frac{\partial \mu_{x,y,z}}{\partial Q_r} / (e u^{-0.5})$        | 0.021 867 641 046  | -0.004 557 938 138 | -0.011 852 160 746 |
|-------------------------------------------------------------------|--------------------|--------------------|--------------------|
| <i>l</i> -matrix coefficients/(u <sup>1/2</sup> Å <sup>-1</sup> ) |                    |                    |                    |
| O                                                                 | -0.020 113 808 110 | 0.030 814 984 606  | 0.024 384 449 097  |
| C                                                                 | 0.096 394 086 671  | -0.087 382 783 006 | -0.076 149 618 630 |
| C                                                                 | -0.040 496 173 697 | 0.289 823 970 199  | 0.307 833 034 869  |
| C                                                                 | -0.176 369 427 891 | -0.126 976 788 581 | -0.077 138 968 863 |
| C                                                                 | 0.219 442 151 232  | -0.027 300 840 222 | 0.033 073 838 195  |
| C                                                                 | -0.072 469 322 720 | -0.077 125 729 654 | -0.109 256 982 732 |
| C                                                                 | 0.134 697 628 664  | -0.100 639 025 025 | -0.176 661 968 320 |
| H                                                                 | 0.254 504 339 893  | -0.030 817 270 313 | 0.011 528 651 570  |
| H                                                                 | -0.508 703 457 962 | 0.003 464 395 919  | 0.104 412 507 878  |
| H                                                                 | 0.161 477 202 719  | -0.031 472 595 687 | 0.213 424 872 600  |
| H                                                                 | 0.058 894 499 635  | -0.038 501 422 538 | -0.031 445 520 077 |
| H                                                                 | 0.074 056 555 063  | 0.153 647 646 982  | 0.018 527 023 030  |
| H                                                                 | -0.102 137 663 728 | 0.151 553 127 150  | -0.044 469 117 038 |
| H                                                                 | -0.175 775 638 358 | 0.083 317 725 471  | 0.038 174 618 234  |
| H                                                                 | -0.124 751 006 507 | 0.013 362 793 999  | -0.016 117 416 759 |
| H                                                                 | -0.144 279 155 766 | -0.012 002 935 789 | -0.185 085 370 019 |
| H                                                                 | 0.030 393 536 448  | 0.032 060 137 970  | 0.133 232 259 943  |

Wavenumber/cm<sup>-1</sup>: 1269.8232

| $\frac{\partial \mu_{x,y,z}}{\partial Q_r} / (e u^{-0.5})$        | -0.009 709 747 658 | 0.018 070 862 983  | 0.006 909 752 325  |
|-------------------------------------------------------------------|--------------------|--------------------|--------------------|
| <i>l</i> -matrix coefficients/(u <sup>1/2</sup> Å <sup>-1</sup> ) |                    |                    |                    |
| O                                                                 | -0.035 083 871 033 | 0.047 474 274 210  | 0.047 566 703 038  |
| C                                                                 | 0.104 772 198 925  | -0.000 298 664 872 | 0.115 545 895 799  |
| C                                                                 | -0.037 647 803 801 | 0.161 175 545 314  | -0.295 305 689 644 |
| C                                                                 | -0.001 444 402 348 | -0.012 445 859 555 | 0.293 945 465 544  |
| C                                                                 | 0.128 141 618 640  | -0.041 633 810 061 | -0.060 657 887 686 |
| C                                                                 | -0.103 514 645 094 | -0.138 302 220 348 | -0.211 175 461 706 |
| C                                                                 | -0.052 731 013 523 | -0.131 276 346 049 | 0.169 323 838 598  |
| H                                                                 | 0.069 372 867 778  | 0.034 830 493 659  | -0.077 930 368 467 |
| H                                                                 | -0.105 148 620 793 | -0.068 704 474 748 | 0.063 006 203 090  |
| H                                                                 | -0.024 651 101 284 | -0.078 314 593 144 | -0.121 020 032 299 |
| H                                                                 | 0.008 130 249 457  | 0.233 359 786 723  | -0.011 382 655 008 |
| H                                                                 | 0.030 887 115 199  | -0.089 205 377 806 | -0.071 809 864 342 |
| H                                                                 | -0.407 539 885 782 | 0.329 995 251 767  | 0.069 136 102 672  |
| H                                                                 | 0.317 196 889 787  | -0.180 727 935 185 | -0.060 498 076 379 |
| H                                                                 | -0.034 434 883 371 | -0.041 115 685 604 | -0.149 632 682 980 |
| H                                                                 | 0.077 307 394 883  | 0.134 285 514 994  | 0.140 911 098 132  |
| H                                                                 | 0.078 945 417 632  | 0.098 373 985 410  | -0.010 595 166 696 |

Wavenumber/cm<sup>-1</sup>: 1295.6277

| $\frac{\partial \mu_{x,y,z}}{\partial Q_r} / (e u^{-0.5})$        | 0.016 278 285 946  | -0.014 421 858 640 | 0.016 852 108 442  |
|-------------------------------------------------------------------|--------------------|--------------------|--------------------|
| <i>l</i> -matrix coefficients/(u <sup>1/2</sup> Å <sup>-1</sup> ) |                    |                    |                    |
| O                                                                 | -0.122 585 757 327 | 0.005 483 508 497  | -0.005 309 996 410 |
| C                                                                 | 0.153 241 207 424  | -0.133 182 469 938 | -0.040 664 973 503 |
| C                                                                 | -0.012 088 197 969 | 0.155 282 608 989  | -0.038 119 320 495 |
| C                                                                 | -0.125 312 718 049 | -0.114 772 462 662 | 0.126 725 978 360  |
| C                                                                 | 0.131 134 763 871  | -0.072 493 122 505 | -0.256 040 902 601 |
| C                                                                 | 0.061 920 454 651  | 0.154 002 550 924  | 0.191 373 191 815  |
| C                                                                 | -0.016 799 483 411 | -0.031 504 498 800 | 0.014 966 266 384  |
| H                                                                 | -0.449 548 384 297 | -0.108 073 698 751 | 0.167 179 501 681  |
| H                                                                 | 0.172 330 032 603  | 0.015 812 580 538  | -0.037 786 523 553 |
| H                                                                 | 0.104 373 973 342  | -0.249 327 777 249 | 0.026 865 221 994  |
| H                                                                 | -0.205 002 665 171 | -0.091 472 513 293 | 0.078 564 376 378  |
| H                                                                 | 0.365 645 899 151  | 0.268 752 213 602  | -0.196 929 243 042 |
| H                                                                 | -0.091 703 438 887 | 0.043 348 651 315  | 0.058 299 134 468  |
| H                                                                 | -0.080 103 154 131 | 0.208 937 902 316  | -0.047 105 782 599 |
| H                                                                 | -0.017 029 631 146 | -0.008 016 724 099 | -0.037 448 879 097 |
| H                                                                 | 0.010 685 997 474  | 0.025 013 981 958  | 0.020 089 237 816  |
| H                                                                 | 0.015 630 849 487  | 0.020 465 713 152  | -0.004 496 934 264 |

Wavenumber/cm<sup>-1</sup>: 1325.1964

| $\frac{\partial \mu_{x,y,z}}{\partial Q_r} / (e u^{-0.5})$        | 0.002 055 225 747  | 0.005 157 436 534  | -0.005 354 639 048 |
|-------------------------------------------------------------------|--------------------|--------------------|--------------------|
| <i>l</i> -matrix coefficients/(u <sup>1/2</sup> Å <sup>-1</sup> ) |                    |                    |                    |
| O                                                                 | -0.023 924 175 837 | -0.115 992 667 391 | 0.054 870 279 647  |
| C                                                                 | -0.130 022 125 009 | -0.260 471 671 165 | 0.087 926 546 564  |
| C                                                                 | 0.232 986 274 512  | 0.011 166 082 274  | -0.002 171 152 006 |
| C                                                                 | -0.159 191 130 624 | 0.069 222 211 270  | 0.053 752 755 412  |
| C                                                                 | -0.000 907 143 357 | -0.294 140 901 268 | 0.090 200 756 546  |
| C                                                                 | 0.128 721 622 208  | 0.647 847 724 411  | -0.321 761 790 048 |
| C                                                                 | -0.060 101 448 350 | -0.035 326 383 574 | -0.009 072 816 924 |
| H                                                                 | -0.067 313 615 404 | -0.092 286 904 664 | 0.080 431 785 287  |
| H                                                                 | -0.151 039 012 695 | 0.021 447 742 162  | 0.050 603 475 937  |
| H                                                                 | 0.045 891 624 902  | 0.213 477 531 130  | 0.019 029 624 624  |
| H                                                                 | 0.045 175 623 236  | 0.019 599 244 778  | 0.005 976 216 845  |
| H                                                                 | -0.036 856 350 698 | 0.049 134 760 897  | 0.039 358 945 390  |
| H                                                                 | 0.034 784 479 580  | -0.116 667 285 168 | 0.035 130 228 575  |
| H                                                                 | 0.149 013 965 182  | -0.110 466 408 856 | 0.007 098 994 822  |
| H                                                                 | 0.005 689 795 542  | -0.020 325 254 532 | -0.079 048 981 620 |
| H                                                                 | 0.026 445 121 329  | 0.016 348 371 567  | 0.029 891 437 808  |
| H                                                                 | 0.003 874 565 344  | 0.004 463 328 014  | -0.057 995 235 334 |

Wavenumber/cm<sup>-1</sup>: 1350.875

| $\frac{\partial \mu_{x,y,z}}{\partial Q_r} / (e u^{-0.5})$        | -0.001 619 160 063 | 0.000 563 687 692  | 0.000 183 450 814  |
|-------------------------------------------------------------------|--------------------|--------------------|--------------------|
| <i>l</i> -matrix coefficients/(u <sup>1/2</sup> Å <sup>-1</sup> ) |                    |                    |                    |
| O                                                                 | 0.001 746 886 113  | -0.012 823 039 384 | -0.043 837 565 503 |
| C                                                                 | 0.005 124 706 982  | -0.109 096 880 966 | -0.191 252 777 728 |
| C                                                                 | -0.120 700 998 959 | 0.262 307 452 047  | -0.008 173 746 674 |
| C                                                                 | 0.019 903 384 256  | -0.055 394 685 952 | 0.196 325 129 119  |
| C                                                                 | -0.029 100 861 073 | -0.041 521 077 658 | -0.180 926 168 116 |
| C                                                                 | 0.065 732 476 432  | 0.036 871 062 674  | 0.235 430 106 480  |
| C                                                                 | 0.112 276 804 816  | -0.246 835 324 186 | 0.020 539 488 318  |
| H                                                                 | 0.189 855 922 958  | -0.058 723 603 115 | 0.054 150 411 627  |
| H                                                                 | 0.128 621 871 017  | 0.125 446 882 527  | -0.082 012 180 029 |
| H                                                                 | -0.203 491 221 151 | 0.442 430 434 500  | -0.074 702 970 296 |
| H                                                                 | -0.165 165 992 890 | 0.030 468 258 683  | 0.056 523 054 760  |
| H                                                                 | -0.108 232 825 857 | -0.205 475 840 837 | -0.006 172 688 062 |
| H                                                                 | 0.103 831 173 128  | -0.142 766 020 567 | 0.052 518 191 741  |
| H                                                                 | -0.006 756 573 728 | 0.127 349 284 515  | -0.039 614 268 723 |
| H                                                                 | -0.185 039 494 020 | -0.026 810 595 924 | -0.211 463 886 444 |
| H                                                                 | -0.068 042 372 733 | 0.128 957 949 370  | -0.042 911 984 012 |
| H                                                                 | 0.123 691 761 443  | 0.160 675 417 130  | 0.219 996 105 129  |

Wavenumber/cm<sup>-1</sup>: 1378.6697

| $\frac{\partial \mu_{x,y,z}}{\partial Q_r} / (e u^{-0.5})$        | 0.004 452 455 246  | -0.009 542 756 663 | 0.002 380 531 328  |
|-------------------------------------------------------------------|--------------------|--------------------|--------------------|
| <i>l</i> -matrix coefficients/(u <sup>1/2</sup> Å <sup>-1</sup> ) |                    |                    |                    |
| O                                                                 | -0.020 255 895 802 | 0.047 192 852 003  | -0.004 097 692 184 |
| C                                                                 | 0.035 513 893 459  | 0.140 166 478 102  | 0.027 784 757 984  |
| C                                                                 | 0.316 467 516 231  | 0.164 132 564 094  | -0.093 573 818 130 |
| C                                                                 | -0.094 025 423 929 | -0.118 484 726 942 | 0.033 769 842 278  |
| C                                                                 | 0.072 027 013 695  | 0.086 769 784 772  | -0.036 360 923 381 |
| C                                                                 | -0.057 989 070 845 | -0.191 839 746 304 | 0.064 855 333 492  |
| C                                                                 | -0.260 933 205 662 | -0.079 142 416 052 | 0.017 874 060 534  |
| H                                                                 | -0.131 784 236 530 | 0.049 251 266 494  | -0.027 894 407 659 |
| H                                                                 | -0.169 216 455 241 | -0.052 630 505 129 | 0.049 597 665 863  |
| H                                                                 | 0.341 243 182 505  | 0.158 699 828 064  | 0.195 672 195 151  |
| H                                                                 | -0.168 711 153 947 | -0.158 254 422 453 | 0.074 926 017 696  |
| H                                                                 | -0.174 871 114 015 | -0.159 104 171 263 | 0.080 218 879 609  |
| H                                                                 | 0.200 136 673 219  | -0.098 910 514 537 | -0.089 038 868 826 |
| H                                                                 | -0.099 163 700 196 | 0.033 971 144 795  | 0.002 346 437 821  |
| H                                                                 | 0.043 207 112 548  | -0.066 235 282 577 | -0.247 808 513 373 |
| H                                                                 | 0.203 751 999 140  | 0.112 378 780 647  | 0.222 886 611 581  |
| H                                                                 | -0.002 072 613 017 | -0.012 716 079 074 | -0.294 113 843 426 |

Wavenumber/cm<sup>-1</sup>: 1416.786

| $\frac{\partial \mu_{x,y,z}}{\partial Q_r} / (e \text{ u}^{-0.5})$ | -0.001 871 179 114 | -0.000 994 467 417 | -0.000 132 737 468 |
|--------------------------------------------------------------------|--------------------|--------------------|--------------------|
| <i>l</i> -matrix coefficients/(u <sup>1/2</sup> Å <sup>-1</sup> )  |                    |                    |                    |
| O                                                                  | -0.028 298 960 253 | 0.027 022 013 986  | -0.015 044 102 466 |
| C                                                                  | -0.121 855 095 044 | 0.102 405 599 805  | -0.103 220 588 446 |
| C                                                                  | 0.255 222 795 498  | 0.129 217 902 744  | 0.350 128 325 089  |
| C                                                                  | -0.006 492 718 274 | -0.083 266 421 412 | 0.040 225 079 713  |
| C                                                                  | 0.012 031 375 413  | 0.031 605 414 997  | 0.000 966 429 418  |
| C                                                                  | 0.004 279 980 361  | -0.057 813 232 742 | 0.097 983 863 228  |
| C                                                                  | -0.055 202 008 295 | -0.108 927 896 256 | -0.343 780 992 193 |
| H                                                                  | -0.354 768 410 517 | -0.010 460 906 558 | 0.080 328 191 530  |
| H                                                                  | 0.249 470 206 953  | 0.075 741 343 073  | -0.092 912 230 678 |
| H                                                                  | 0.063 844 930 100  | -0.034 662 571 055 | 0.078 534 783 272  |
| H                                                                  | 0.201 193 027 919  | 0.145 817 004 016  | -0.076 308 023 567 |
| H                                                                  | -0.198 723 359 147 | -0.182 216 082 257 | 0.115 591 512 815  |
| H                                                                  | -0.172 816 546 441 | 0.134 266 496 563  | 0.061 026 061 123  |
| H                                                                  | 0.270 035 801 980  | -0.177 919 890 995 | -0.038 362 979 718 |
| H                                                                  | -0.079 447 017 376 | -0.012 440 036 630 | -0.032 054 368 884 |
| H                                                                  | -0.135 969 216 956 | -0.073 291 354 011 | -0.193 190 357 987 |
| H                                                                  | -0.033 794 397 400 | -0.018 131 784 435 | 0.011 258 183 516  |

Wavenumber/cm<sup>-1</sup>: 1449.5118

| $\frac{\partial \mu_{x,y,z}}{\partial Q_r} / (e \text{ u}^{-0.5})$ | 0.001 428 274 403  | -0.005 081 178 653 | -0.000 551 823 631 |
|--------------------------------------------------------------------|--------------------|--------------------|--------------------|
| <i>l</i> -matrix coefficients/(u <sup>1/2</sup> Å <sup>-1</sup> )  |                    |                    |                    |
| O                                                                  | -0.040 269 697 096 | 0.034 240 232 899  | 0.028 634 201 105  |
| C                                                                  | 0.169 711 225 476  | -0.130 698 912 364 | 0.116 002 353 818  |
| C                                                                  | -0.161 522 425 262 | 0.127 787 618 252  | -0.019 499 387 161 |
| C                                                                  | -0.407 419 174 033 | -0.137 290 656 373 | 0.032 548 343 028  |
| C                                                                  | 0.444 995 870 679  | 0.116 332 023 354  | -0.057 462 205 167 |
| C                                                                  | -0.072 461 016 050 | -0.011 336 683 284 | -0.111 416 928 105 |
| C                                                                  | 0.031 904 858 908  | 0.158 689 697 549  | 0.003 077 894 546  |
| H                                                                  | 0.028 410 039 567  | -0.025 375 788 928 | -0.013 043 063 643 |
| H                                                                  | 0.246 781 197 395  | -0.057 613 432 578 | -0.013 947 015 587 |
| H                                                                  | -0.163 903 822 569 | 0.036 041 621 076  | -0.098 628 074 233 |
| H                                                                  | -0.103 665 093 591 | -0.190 077 700 394 | 0.070 303 035 709  |
| H                                                                  | -0.211 417 809 494 | -0.023 743 970 336 | 0.159 023 983 550  |
| H                                                                  | 0.218 221 690 430  | 0.021 905 943 234  | -0.188 818 542 832 |
| H                                                                  | 0.148 903 889 013  | -0.207 816 301 832 | -0.037 725 414 349 |
| H                                                                  | 0.082 007 313 826  | 0.040 931 316 790  | 0.208 122 735 568  |
| H                                                                  | -0.041 111 485 555 | -0.078 448 805 873 | -0.051 961 257 052 |
| H                                                                  | -0.061 770 771 937 | -0.078 480 070 783 | -0.020 547 248 943 |

Wavenumber/cm<sup>-1</sup>: 1455.2412

| $\frac{\partial \mu_{x,y,z}}{\partial Q_r} / (e u^{-0.5})$        | 0.005 341 286 483  | -0.000 103 467 667 | -0.000 225 956 269 |
|-------------------------------------------------------------------|--------------------|--------------------|--------------------|
| <i>l</i> -matrix coefficients/(u <sup>1/2</sup> Å <sup>-1</sup> ) |                    |                    |                    |
| O                                                                 | -0.023 634 734 469 | -0.000 110 057 659 | -0.039 918 222 033 |
| C                                                                 | -0.042 308 605 908 | -0.084 648 714 032 | -0.130 645 161 187 |
| C                                                                 | -0.008 021 318 220 | 0.001 595 107 069  | 0.025 291 544 711  |
| C                                                                 | 0.021 964 784 215  | -0.040 814 537 802 | 0.299 052 355 432  |
| C                                                                 | 0.053 392 360 282  | -0.043 008 812 562 | -0.303 521 245 816 |
| C                                                                 | 0.059 627 795 748  | 0.076 865 784 416  | 0.187 803 006 115  |
| C                                                                 | -0.072 166 868 458 | 0.203 847 157 346  | -0.057 170 599 073 |
| H                                                                 | 0.202 812 076 242  | -0.054 820 230 452 | 0.076 387 579 027  |
| H                                                                 | -0.288 193 949 916 | 0.110 196 105 907  | 0.029 227 329 008  |
| H                                                                 | 0.034 581 115 646  | -0.195 950 769 310 | 0.003 276 911 552  |
| H                                                                 | -0.043 703 070 879 | 0.301 346 437 921  | -0.036 129 827 530 |
| H                                                                 | -0.100 623 142 932 | -0.288 144 880 926 | -0.085 244 604 162 |
| H                                                                 | 0.060 035 832 851  | -0.117 220 994 751 | 0.107 341 591 274  |
| H                                                                 | 0.105 489 439 901  | 0.161 906 350 682  | -0.081 393 235 652 |
| H                                                                 | 0.185 669 028 876  | 0.025 598 967 161  | 0.288 109 094 985  |
| H                                                                 | 0.024 606 218 055  | -0.147 044 319 249 | -0.008 676 797 563 |
| H                                                                 | -0.129 619 734 057 | -0.188 387 930 204 | -0.205 696 048 750 |

Wavenumber/cm<sup>-1</sup>: 1496.5581

| $\frac{\partial \mu_{x,y,z}}{\partial Q_r} / (e u^{-0.5})$        | 0.002 862 065 561  | -0.003 242 925 693 | 0.005 784 443 712  |
|-------------------------------------------------------------------|--------------------|--------------------|--------------------|
| <i>l</i> -matrix coefficients/(u <sup>1/2</sup> Å <sup>-1</sup> ) |                    |                    |                    |
| O                                                                 | -0.058 443 385 548 | -0.033 314 103 102 | 0.049 972 411 292  |
| C                                                                 | 0.272 750 591 264  | -0.222 074 778 824 | 0.061 146 694 639  |
| C                                                                 | -0.075 035 995 804 | 0.321 294 561 990  | 0.043 706 403 239  |
| C                                                                 | 0.250 556 607 065  | -0.276 838 915 799 | -0.121 003 437 912 |
| C                                                                 | -0.235 388 068 695 | 0.027 806 131 707  | 0.176 149 214 871  |
| C                                                                 | -0.029 950 043 428 | 0.042 008 139 766  | -0.063 811 551 454 |
| C                                                                 | -0.165 544 400 351 | 0.128 413 361 095  | -0.118 802 736 077 |
| H                                                                 | 0.128 470 313 930  | -0.070 919 045 518 | 0.045 175 987 860  |
| H                                                                 | 0.213 711 649 437  | 0.007 461 452 547  | -0.014 026 379 065 |
| H                                                                 | -0.043 825 438 831 | 0.305 318 314 873  | 0.031 162 515 700  |
| H                                                                 | 0.019 634 931 513  | -0.028 789 626 382 | -0.049 753 454 163 |
| H                                                                 | 0.117 080 172 623  | -0.077 702 783 593 | -0.096 191 938 462 |
| H                                                                 | -0.221 725 554 660 | 0.138 992 820 001  | 0.035 629 562 315  |
| H                                                                 | -0.134 663 617 904 | 0.011 777 030 246  | 0.057 591 894 447  |
| H                                                                 | 0.147 824 210 522  | -0.000 943 019 768 | 0.110 749 073 519  |
| H                                                                 | 0.064 850 578 812  | -0.059 716 675 835 | 0.032 900 635 718  |
| H                                                                 | -0.118 539 565 769 | -0.163 892 582 217 | -0.274 263 987 637 |



Wavenumber/cm<sup>-1</sup>: 1499.2874

| $\frac{\partial \mu_{x,y,z}}{\partial Q_r} / (e \text{ u}^{-0.5})$ |                    |                    |                    |
|--------------------------------------------------------------------|--------------------|--------------------|--------------------|
|                                                                    | -0.000 280 886 487 | 0.001 349 698 611  | -0.000 201 432 097 |
| <i>l</i> -matrix coefficients/(u <sup>1/2</sup> Å <sup>-1</sup> )  |                    |                    |                    |
| O                                                                  | -0.020 399 357 414 | -0.010 710 324 429 | -0.028 800 479 605 |
| C                                                                  | 0.180 124 101 258  | -0.308 894 332 251 | -0.231 000 193 905 |
| C                                                                  | -0.085 538 824 144 | -0.041 131 911 007 | -0.003 131 514 243 |
| C                                                                  | -0.148 344 489 804 | 0.347 652 496 376  | -0.178 024 291 828 |
| C                                                                  | -0.093 022 596 892 | 0.078 992 553 023  | -0.033 759 489 824 |
| C                                                                  | 0.015 238 107 725  | -0.121 041 836 429 | 0.247 391 688 833  |
| C                                                                  | -0.058 897 198 889 | -0.002 333 252 919 | 0.098 725 622 003  |
| H                                                                  | 0.157 188 000 336  | -0.177 076 597 519 | 0.223 865 104 919  |
| H                                                                  | 0.011 759 904 829  | 0.221 497 572 713  | -0.051 516 857 024 |
| H                                                                  | 0.104 718 092 498  | -0.025 587 274 103 | 0.102 478 214 800  |
| H                                                                  | 0.231 203 635 511  | -0.074 305 765 504 | -0.008 631 888 722 |
| H                                                                  | -0.109 969 793 954 | 0.258 407 645 782  | 0.232 470 186 731  |
| H                                                                  | -0.080 328 163 488 | 0.039 604 659 182  | 0.072 592 760 783  |
| H                                                                  | 0.238 503 013 825  | -0.079 684 759 547 | -0.042 426 798 830 |
| H                                                                  | 0.032 659 378 971  | -0.019 425 154 136 | -0.098 495 374 227 |
| H                                                                  | 0.141 875 479 549  | 0.070 209 879 927  | 0.158 021 241 919  |
| H                                                                  | 0.011 061 638 221  | -0.009 567 581 261 | -0.129 111 683 714 |

Wavenumber/cm<sup>-1</sup>: 1507.3232

| $\frac{\partial \mu_{x,y,z}}{\partial Q_r} / (e \text{ u}^{-0.5})$ |                    |                    |                    |
|--------------------------------------------------------------------|--------------------|--------------------|--------------------|
|                                                                    | -0.002 776 029 021 | 0.001 506 561 416  | -0.002 994 555 152 |
| <i>l</i> -matrix coefficients/(u <sup>1/2</sup> Å <sup>-1</sup> )  |                    |                    |                    |
| O                                                                  | 0.087 133 534 797  | -0.008 777 050 658 | -0.033 021 989 992 |
| C                                                                  | -0.395 035 298 158 | -0.332 941 271 563 | -0.012 062 745 379 |
| C                                                                  | 0.098 142 232 966  | -0.089 630 038 457 | -0.091 454 825 075 |
| C                                                                  | 0.115 620 643 003  | -0.138 314 456 410 | -0.054 775 004 358 |
| C                                                                  | 0.053 552 749 463  | 0.477 403 339 698  | 0.000 631 274 708  |
| C                                                                  | 0.081 963 538 723  | -0.011 404 280 971 | -0.027 773 631 085 |
| C                                                                  | 0.125 011 487 566  | 0.056 201 790 128  | 0.177 046 936 138  |
| H                                                                  | -0.182 453 189 899 | -0.173 783 923 244 | 0.241 786 154 021  |
| H                                                                  | -0.166 896 549 949 | 0.156 170 815 499  | 0.010 002 230 642  |
| H                                                                  | -0.009 923 531 627 | 0.075 240 560 379  | -0.037 254 834 212 |
| H                                                                  | -0.077 763 607 157 | -0.033 820 811 140 | -0.006 650 722 341 |
| H                                                                  | -0.037 115 617 777 | -0.143 816 869 876 | -0.037 738 664 833 |
| H                                                                  | -0.076 896 619 466 | 0.282 719 852 887  | -0.192 312 917 122 |
| H                                                                  | -0.140 625 636 389 | -0.053 842 966 601 | 0.001 410 327 639  |
| H                                                                  | 0.026 955 511 735  | 0.019 513 105 350  | 0.058 501 540 723  |
| H                                                                  | 0.008 418 564 890  | 0.012 441 080 397  | 0.028 684 454 423  |
| H                                                                  | 0.035 565 671 982  | 0.027 687 257 687  | 0.094 089 885 182  |

Wavenumber/cm<sup>-1</sup>: 1812.7458

| $\frac{\partial \mu_{x,y,z}}{\partial Q_r} / (e \text{ u}^{-0.5})$ |                    |                    |                    |
|--------------------------------------------------------------------|--------------------|--------------------|--------------------|
|                                                                    | -0.002 443 474 682 | 0.004 115 058 744  | 0.000 985 479 888  |
| <i>l</i> -matrix coefficients/(u <sup>1/2</sup> Å <sup>-1</sup> )  |                    |                    |                    |
| O                                                                  | -0.050 510 569 119 | 0.020 723 861 251  | -0.024 270 583 268 |
| C                                                                  | -0.078 686 111 491 | 0.226 889 183 896  | -0.234 754 042 917 |
| C                                                                  | 0.169 678 848 687  | 0.213 084 195 080  | -0.271 659 146 506 |
| C                                                                  | -0.109 309 619 673 | -0.341 948 606 136 | -0.140 953 759 431 |
| C                                                                  | -0.147 478 301 126 | -0.269 307 709 061 | 0.086 623 954 285  |
| C                                                                  | -0.006 004 599 277 | -0.010 504 915 393 | 0.139 443 948 369  |
| C                                                                  | 0.232 342 598 259  | 0.186 032 053 393  | 0.283 161 514 620  |
| H                                                                  | -0.056 676 385 516 | 0.045 907 435 779  | 0.000 720 741 308  |
| H                                                                  | -0.118 002 680 402 | 0.118 542 753 584  | -0.044 411 187 914 |
| H                                                                  | 0.067 063 793 595  | 0.034 540 011 643  | -0.068 724 589 166 |
| H                                                                  | 0.085 391 955 259  | -0.252 475 249 183 | 0.009 189 872 522  |
| H                                                                  | -0.053 031 998 967 | 0.006 342 998 995  | 0.120 438 899 328  |
| H                                                                  | -0.146 489 078 414 | -0.038 154 844 643 | 0.153 708 266 858  |
| H                                                                  | 0.125 327 086 713  | -0.049 796 170 878 | 0.010 613 511 406  |
| H                                                                  | 0.087 788 707 449  | 0.060 593 056 766  | 0.248 326 983 420  |
| H                                                                  | -0.029 871 290 206 | -0.037 030 870 003 | -0.002 272 741 838 |
| H                                                                  | 0.030 745 341 849  | 0.014 314 450 738  | 0.145 954 427 407  |

Wavenumber/cm<sup>-1</sup>: 3023.0136

| $\frac{\partial \mu_{x,y,z}}{\partial Q_r} / (e \text{ u}^{-0.5})$ |                    |                    |                    |
|--------------------------------------------------------------------|--------------------|--------------------|--------------------|
|                                                                    | -0.013 511 328 598 | -0.020 793 783 042 | 0.047 308 690 007  |
| <i>l</i> -matrix coefficients/(u <sup>1/2</sup> Å <sup>-1</sup> )  |                    |                    |                    |
| O                                                                  | 0.231 208 838 139  | -0.082 598 329 567 | -0.032 249 993 099 |
| C                                                                  | 0.046 070 625 965  | -0.210 995 122 843 | 0.364 481 625 012  |
| C                                                                  | 0.189 423 363 278  | 0.178 351 913 297  | -0.152 133 988 242 |
| C                                                                  | -0.184 445 275 649 | 0.163 763 697 950  | 0.005 892 694 998  |
| C                                                                  | -0.300 074 670 763 | 0.144 532 811 118  | -0.185 000 747 661 |
| C                                                                  | 0.129 673 926 430  | -0.192 448 928 033 | -0.017 843 082 726 |
| C                                                                  | 0.004 906 256 879  | 0.016 323 730 505  | -0.076 273 983 349 |
| H                                                                  | -0.110 980 527 127 | -0.009 270 227 621 | -0.083 462 476 470 |
| H                                                                  | -0.058 454 256 694 | -0.281 312 821 890 | 0.119 227 076 383  |
| H                                                                  | -0.026 277 308 129 | 0.058 185 888 251  | -0.108 787 343 826 |
| H                                                                  | 0.058 927 639 922  | -0.042 312 793 048 | 0.026 857 727 276  |
| H                                                                  | -0.137 211 343 580 | 0.068 073 729 471  | 0.148 789 884 312  |
| H                                                                  | -0.081 703 217 778 | -0.051 611 674 509 | 0.206 632 235 573  |
| H                                                                  | 0.021 117 883 001  | 0.309 144 200 797  | -0.043 483 420 754 |
| H                                                                  | -0.018 049 589 884 | 0.017 209 205 003  | 0.117 837 352 286  |
| H                                                                  | -0.140 438 164 635 | -0.072 438 127 464 | -0.138 218 468 234 |
| H                                                                  | -0.033 020 887 531 | -0.010 158 222 855 | 0.093 241 941 582  |

Wavenumber/cm<sup>-1</sup>: 3025.9631

| $\frac{\partial \mu_{x,y,z}}{\partial Q_r} / (e u^{-0.5})$        | 0.018 233 992 202  | 0.026 507 334 811  | -0.055 233 218 924 |
|-------------------------------------------------------------------|--------------------|--------------------|--------------------|
| <i>l</i> -matrix coefficients/(u <sup>1/2</sup> Å <sup>-1</sup> ) |                    |                    |                    |
| O                                                                 | -0.259 955 168 421 | 0.080 420 268 701  | 0.124 820 925 159  |
| C                                                                 | 0.201 512 029 951  | -0.163 287 282 350 | -0.076 303 621 206 |
| C                                                                 | 0.433 107 909 155  | 0.045 346 125 978  | -0.240 707 245 835 |
| C                                                                 | 0.015 527 521 506  | 0.301 110 905 598  | 0.091 773 511 924  |
| C                                                                 | -0.072 844 717 346 | -0.068 062 809 058 | 0.186 577 787 069  |
| C                                                                 | -0.284 598 162 544 | -0.155 193 620 506 | -0.038 678 378 272 |
| C                                                                 | 0.049 629 740 190  | -0.008 251 688 759 | -0.044 103 488 667 |
| H                                                                 | 0.061 793 560 297  | -0.089 768 688 186 | 0.119 587 871 207  |
| H                                                                 | 0.083 229 396 099  | 0.128 085 117 780  | -0.027 772 489 904 |
| H                                                                 | 0.110 400 810 789  | -0.050 887 361 240 | -0.094 645 343 886 |
| H                                                                 | -0.158 926 651 536 | 0.164 297 446 108  | 0.012 077 054 103  |
| H                                                                 | 0.012 858 545 710  | -0.032 307 624 314 | -0.128 144 020 151 |
| H                                                                 | 0.118 188 795 133  | -0.072 169 917 432 | -0.138 986 607 707 |
| H                                                                 | -0.166 489 558 710 | -0.131 665 313 252 | 0.061 158 493 111  |
| H                                                                 | -0.031 224 737 315 | 0.017 803 944 232  | 0.130 861 746 085  |
| H                                                                 | -0.164 707 935 127 | -0.098 328 039 287 | -0.160 531 505 254 |
| H                                                                 | -0.011 171 882 201 | 0.011 402 823 897  | 0.148 311 875 515  |

Wavenumber/cm<sup>-1</sup>: 3036.4003

| $\frac{\partial \mu_{x,y,z}}{\partial Q_r} / (e u^{-0.5})$        | 0.004 166 676 325  | -0.007 638 565 036 | 0.001 791 537 150  |
|-------------------------------------------------------------------|--------------------|--------------------|--------------------|
| <i>l</i> -matrix coefficients/(u <sup>1/2</sup> Å <sup>-1</sup> ) |                    |                    |                    |
| O                                                                 | 0.458 130 190 887  | -0.153 026 071 073 | -0.084 709 125 211 |
| C                                                                 | -0.040 282 837 792 | 0.132 321 192 260  | -0.178 348 493 958 |
| C                                                                 | -0.166 149 166 640 | 0.194 737 173 738  | 0.018 500 426 445  |
| C                                                                 | -0.312 127 364 728 | 0.185 428 648 784  | 0.175 547 243 155  |
| C                                                                 | -0.154 916 304 308 | -0.157 763 297 899 | 0.238 334 233 022  |
| C                                                                 | 0.296 619 452 041  | -0.172 439 752 774 | -0.113 788 988 716 |
| C                                                                 | -0.001 110 924 602 | -0.005 878 256 342 | -0.010 209 935 273 |
| H                                                                 | -0.110 729 899 036 | -0.007 425 463 049 | 0.085 442 952 356  |
| H                                                                 | 0.018 049 155 152  | 0.141 681 283 031  | -0.056 543 101 380 |
| H                                                                 | -0.021 402 098 302 | -0.034 431 921 396 | 0.012 512 408 335  |
| H                                                                 | -0.210 996 289 337 | 0.135 025 127 108  | 0.030 256 225 286  |
| H                                                                 | -0.019 415 964 644 | 0.014 929 221 916  | -0.103 973 673 777 |
| H                                                                 | -0.058 243 144 935 | 0.038 519 334 430  | -0.139 060 011 660 |
| H                                                                 | -0.199 501 057 382 | -0.170 651 320 349 | 0.074 229 393 933  |
| H                                                                 | 0.053 449 215 162  | -0.010 563 367 183 | 0.057 221 791 366  |
| H                                                                 | 0.046 100 053 426  | -0.041 428 285 891 | 0.026 242 368 516  |
| H                                                                 | -0.017 801 584 395 | -0.064 935 792 441 | -0.097 717 094 765 |

Wavenumber/cm<sup>-1</sup>: 3043.6287

| $\frac{\partial \mu_{x,y,z}}{\partial Q_r} / (e u^{-0.5})$        | -0.011 892 879 646 | 0.036 260 276 612  | -0.058 497 419 934 |
|-------------------------------------------------------------------|--------------------|--------------------|--------------------|
| <i>l</i> -matrix coefficients/(u <sup>1/2</sup> Å <sup>-1</sup> ) |                    |                    |                    |
| O                                                                 | -0.152 466 597 262 | -0.555 802 120 121 | 0.066 457 846 705  |
| C                                                                 | 0.233 211 605 787  | 0.151 179 040 524  | -0.116 294 205 062 |
| C                                                                 | 0.140 427 904 864  | -0.100 891 507 307 | -0.046 133 302 447 |
| C                                                                 | -0.150 729 035 068 | -0.016 835 675 659 | 0.025 195 098 660  |
| C                                                                 | -0.121 732 960 657 | 0.269 282 881 864  | -0.055 034 412 069 |
| C                                                                 | 0.155 547 098 646  | 0.304 044 826 366  | 0.243 734 591 164  |
| C                                                                 | -0.016 514 341 146 | 0.023 263 464 724  | -0.013 235 000 501 |
| H                                                                 | 0.168 742 708 937  | 0.100 234 419 399  | -0.204 338 138 226 |
| H                                                                 | 0.011 298 874 109  | -0.116 392 838 143 | -0.020 254 452 139 |
| H                                                                 | 0.065 098 225 707  | -0.078 511 885 761 | -0.001 849 629 210 |
| H                                                                 | -0.059 850 755 401 | -0.002 402 671 671 | 0.007 912 865 349  |
| H                                                                 | -0.083 010 051 674 | -0.047 400 962 880 | 0.013 320 217 219  |
| H                                                                 | -0.135 855 496 463 | 0.219 159 490 817  | -0.173 110 932 831 |
| H                                                                 | -0.109 962 379 081 | -0.105 327 546 140 | -0.020 599 040 437 |
| H                                                                 | -0.058 899 691 610 | 0.019 099 327 710  | -0.015 566 133 372 |
| H                                                                 | -0.034 787 695 306 | -0.006 621 686 225 | -0.028 221 287 201 |
| H                                                                 | 0.015 463 895 253  | 0.057 627 387 064  | 0.045 954 332 580  |

Wavenumber/cm<sup>-1</sup>: 3054.2354

| $\frac{\partial \mu_{x,y,z}}{\partial Q_r} / (e u^{-0.5})$        | -0.028 455 300 381 | 0.001 797 773 965  | 0.004 978 130 074  |
|-------------------------------------------------------------------|--------------------|--------------------|--------------------|
| <i>l</i> -matrix coefficients/(u <sup>1/2</sup> Å <sup>-1</sup> ) |                    |                    |                    |
| O                                                                 | -0.037 665 674 544 | 0.230 155 679 678  | -0.376 310 751 653 |
| C                                                                 | -0.092 974 575 822 | -0.149 406 212 505 | 0.140 320 468 814  |
| C                                                                 | -0.033 968 934 534 | 0.110 935 448 694  | -0.108 969 581 160 |
| C                                                                 | 0.110 153 334 111  | 0.100 553 364 766  | -0.028 224 380 544 |
| C                                                                 | 0.062 499 606 588  | -0.173 329 094 012 | 0.097 152 674 874  |
| C                                                                 | 0.129 949 455 968  | 0.074 824 789 246  | 0.523 461 858 022  |
| C                                                                 | -0.059 306 752 661 | -0.071 939 635 919 | -0.072 190 377 526 |
| H                                                                 | -0.039 388 926 000 | 0.021 038 018 578  | -0.168 822 065 303 |
| H                                                                 | -0.166 596 599 086 | -0.270 834 713 571 | 0.073 230 785 268  |
| H                                                                 | -0.037 808 739 233 | 0.064 672 267 771  | -0.048 803 528 467 |
| H                                                                 | 0.025 542 903 582  | 0.011 791 189 488  | 0.000 177 312 871  |
| H                                                                 | 0.068 679 858 013  | 0.064 361 855 729  | -0.021 765 112 198 |
| H                                                                 | -0.001 543 697 729 | 0.055 352 865 009  | -0.223 832 432 604 |
| H                                                                 | -0.027 598 342 792 | -0.354 859 065 905 | 0.012 395 059 199  |
| H                                                                 | 0.025 976 277 781  | -0.029 338 879 186 | 0.033 483 473 438  |
| H                                                                 | -0.049 933 059 344 | -0.034 674 558 630 | -0.046 819 077 142 |
| H                                                                 | -0.048 912 059 387 | -0.070 406 239 835 | -0.013 935 120 451 |

Wavenumber/cm<sup>-1</sup>: 3084.7021

| $\frac{\partial \mu_{x,y,z}}{\partial Q_r} / (e u^{-0.5})$        |                    |                    |                    |
|-------------------------------------------------------------------|--------------------|--------------------|--------------------|
|                                                                   | -0.020 779 924 857 | 0.019 566 590 968  | 0.001 294 426 047  |
| <i>l</i> -matrix coefficients/(u <sup>1/2</sup> Å <sup>-1</sup> ) |                    |                    |                    |
| O                                                                 | 0.072 257 563 473  | -0.049 419 987 465 | 0.007 188 866 879  |
| C                                                                 | 0.010 026 564 388  | 0.236 643 103 580  | 0.087 072 933 415  |
| C                                                                 | -0.070 217 403 014 | -0.021 553 827 426 | -0.326 673 642 653 |
| C                                                                 | 0.195 509 638 020  | -0.057 473 967 659 | 0.238 677 537 276  |
| C                                                                 | 0.091 393 435 315  | 0.076 506 391 278  | 0.023 227 469 992  |
| C                                                                 | 0.086 664 697 879  | 0.068 153 616 285  | -0.014 307 716 926 |
| C                                                                 | -0.339 903 542 873 | -0.238 364 526 934 | -0.166 756 296 598 |
| H                                                                 | 0.087 482 311 697  | 0.004 245 112 221  | 0.242 502 403 771  |
| H                                                                 | -0.076 303 391 314 | 0.309 205 713 056  | 0.044 411 490 225  |
| H                                                                 | -0.021 869 623 950 | -0.008 875 432 330 | -0.094 420 154 483 |
| H                                                                 | 0.165 867 530 154  | -0.236 614 319 392 | 0.147 063 904 283  |
| H                                                                 | 0.072 157 276 006  | 0.152 730 166 131  | 0.250 512 350 471  |
| H                                                                 | 0.026 329 161 967  | 0.035 259 040 429  | -0.028 940 890 348 |
| H                                                                 | -0.042 347 218 229 | 0.011 054 675 502  | 0.011 801 940 056  |
| H                                                                 | -0.093 627 677 368 | -0.062 911 094 492 | 0.062 551 250 292  |
| H                                                                 | -0.188 019 306 881 | -0.135 152 459 489 | -0.123 936 345 744 |
| H                                                                 | -0.125 979 597 084 | -0.092 667 098 707 | 0.007 848 672 950  |

Wavenumber/cm<sup>-1</sup>: 3086.0098

| $\frac{\partial \mu_{x,y,z}}{\partial Q_r} / (e u^{-0.5})$        |                    |                    |                    |
|-------------------------------------------------------------------|--------------------|--------------------|--------------------|
|                                                                   | 0.006 658 287 850  | -0.020 125 074 767 | 0.006 946 511 826  |
| <i>l</i> -matrix coefficients/(u <sup>1/2</sup> Å <sup>-1</sup> ) |                    |                    |                    |
| O                                                                 | -0.135 280 606 339 | -0.104 307 367 292 | 0.139 180 484 448  |
| C                                                                 | -0.185 980 124 230 | -0.009 272 856 507 | -0.292 722 913 587 |
| C                                                                 | -0.050 095 043 423 | 0.223 486 081 599  | 0.017 297 908 514  |
| C                                                                 | 0.142 512 828 995  | 0.212 091 307 629  | 0.175 951 593 581  |
| C                                                                 | 0.033 970 839 866  | 0.142 225 229 670  | -0.034 614 982 973 |
| C                                                                 | -0.127 428 936 106 | 0.033 446 717 725  | -0.109 188 527 287 |
| C                                                                 | 0.238 158 966 029  | -0.358 756 438 087 | 0.093 326 521 467  |
| H                                                                 | -0.127 408 085 534 | 0.046 315 327 634  | -0.247 775 308 775 |
| H                                                                 | 0.005 630 452 577  | -0.185 543 273 534 | -0.099 549 035 609 |
| H                                                                 | -0.014 714 475 222 | 0.074 339 850 431  | 0.006 491 481 035  |
| H                                                                 | 0.121 519 874 270  | -0.030 194 010 035 | 0.079 612 622 659  |
| H                                                                 | 0.043 063 490 891  | 0.143 306 457 253  | 0.145 966 475 872  |
| H                                                                 | 0.051 306 476 858  | 0.010 589 750 942  | -0.024 049 035 519 |
| H                                                                 | -0.042 005 030 447 | 0.061 424 899 553  | -0.003 564 258 919 |
| H                                                                 | 0.271 871 925 635  | -0.146 843 446 037 | 0.142 375 455 099  |
| H                                                                 | 0.083 444 138 044  | -0.094 145 967 328 | 0.038 585 175 737  |
| H                                                                 | -0.030 269 292 443 | -0.303 271 846 665 | -0.074 973 702 534 |

Wavenumber/cm<sup>-1</sup>: 3091.4929

| $\frac{\partial \mu_{x,y,z}}{\partial Q_r} / (e u^{-0.5})$        |                    |                    |                    |
|-------------------------------------------------------------------|--------------------|--------------------|--------------------|
|                                                                   | -0.008 643 385 296 | 0.001 416 818 818  | 0.004 666 436 579  |
| <i>l</i> -matrix coefficients/(u <sup>1/2</sup> Å <sup>-1</sup> ) |                    |                    |                    |
| O                                                                 | 0.007 125 944 401  | -0.072 987 542 522 | 0.026 666 108 546  |
| C                                                                 | 0.016 635 642 806  | 0.043 625 059 976  | 0.067 877 767 160  |
| C                                                                 | 0.008 351 401 971  | -0.013 367 992 577 | 0.002 707 252 470  |
| C                                                                 | -0.019 804 235 517 | -0.006 237 118 354 | -0.042 581 109 281 |
| C                                                                 | 0.000 145 580 646  | -0.042 209 688 199 | -0.040 522 279 250 |
| C                                                                 | 0.013 253 240 867  | -0.027 853 932 384 | 0.015 350 274 767  |
| C                                                                 | -0.017 383 618 758 | 0.089 167 009 738  | -0.025 253 108 327 |
| H                                                                 | 0.013 800 572 347  | -0.002 259 707 699 | 0.065 899 320 594  |
| H                                                                 | -0.006 769 453 980 | 0.060 820 802 076  | 0.022 350 237 133  |
| H                                                                 | 0.003 995 185 694  | -0.017 808 595 433 | -0.000 789 113 864 |
| H                                                                 | -0.010 395 028 613 | 0.018 657 039 452  | -0.019 976 231 137 |
| H                                                                 | -0.004 006 280 556 | -0.013 523 614 597 | -0.030 104 117 316 |
| H                                                                 | -0.003 747 413 044 | -0.004 848 860 763 | -0.022 653 557 063 |
| H                                                                 | 0.002 634 778 530  | -0.024 952 236 620 | -0.012 014 528 274 |
| H                                                                 | 0.477 007 500 020  | -0.106 904 546 074 | -0.251 699 873 661 |
| H                                                                 | -0.217 293 517 093 | 0.560 006 285 998  | -0.091 728 423 008 |
| H                                                                 | -0.287 752 191 130 | -0.327 259 338 459 | 0.311 873 960 108  |

Wavenumber/cm<sup>-1</sup>: 3097.6727

| $\frac{\partial \mu_{x,y,z}}{\partial Q_r} / (e u^{-0.5})$        |                    |                    |                    |
|-------------------------------------------------------------------|--------------------|--------------------|--------------------|
|                                                                   | 0.026 453 270 280  | 0.088 177 061 480  | -0.044 234 322 679 |
| <i>l</i> -matrix coefficients/(u <sup>1/2</sup> Å <sup>-1</sup> ) |                    |                    |                    |
| O                                                                 | 0.052 416 762 805  | -0.042 642 410 763 | -0.068 135 739 407 |
| C                                                                 | 0.008 578 891 309  | -0.014 558 543 475 | -0.165 124 102 198 |
| C                                                                 | 0.002 848 879 196  | 0.012 467 818 450  | -0.076 214 281 226 |
| C                                                                 | -0.071 831 880 783 | 0.048 018 754 680  | -0.299 198 969 266 |
| C                                                                 | 0.274 979 924 725  | 0.183 898 034 106  | 0.343 910 826 800  |
| C                                                                 | 0.096 650 873 340  | 0.038 416 998 520  | 0.046 300 726 084  |
| C                                                                 | -0.322 263 859 054 | -0.217 766 048 927 | 0.181 057 323 012  |
| H                                                                 | 0.000 729 484 763  | 0.010 857 308 755  | -0.096 049 784 909 |
| H                                                                 | -0.007 362 302 344 | -0.061 335 447 935 | -0.044 310 732 696 |
| H                                                                 | 0.048 837 813 381  | 0.042 278 907 742  | 0.023 520 200 089  |
| H                                                                 | -0.189 059 169 967 | 0.098 719 672 736  | -0.101 206 947 553 |
| H                                                                 | 0.021 033 184 871  | -0.058 602 956 737 | -0.234 843 817 371 |
| H                                                                 | 0.052 541 709 854  | 0.003 806 710 306  | 0.304 791 187 104  |
| H                                                                 | 0.255 081 226 338  | 0.197 077 647 671  | 0.090 055 929 129  |
| H                                                                 | -0.059 285 333 876 | -0.067 120 218 005 | 0.118 814 248 017  |
| H                                                                 | -0.168 400 763 990 | -0.075 009 040 930 | -0.007 060 561 395 |
| H                                                                 | -0.124 848 308 849 | -0.095 027 539 215 | 0.111 663 855 270  |

Wavenumber/cm<sup>-1</sup>: 3098.3403

| $\frac{\partial \mu_{x,y,z}}{\partial Q_r} / (e u^{-0.5})$        | 0.012 179 974 750  | 0.046 495 489 779  | -0.018 033 728 982 |
|-------------------------------------------------------------------|--------------------|--------------------|--------------------|
| <i>l</i> -matrix coefficients/(u <sup>1/2</sup> Å <sup>-1</sup> ) |                    |                    |                    |
| O                                                                 | 0.287 536 806 749  | 0.235 390 769 968  | 0.473 450 685 250  |
| C                                                                 | 0.001 722 415 767  | -0.162 303 851 861 | -0.319 694 173 264 |
| C                                                                 | 0.009 610 561 189  | -0.023 054 853 311 | -0.001 856 748 890 |
| C                                                                 | 0.092 710 821 205  | -0.044 504 900 923 | -0.013 217 941 275 |
| C                                                                 | -0.039 506 376 786 | -0.108 172 142 404 | -0.245 185 362 310 |
| C                                                                 | 0.079 787 778 391  | 0.008 082 563 230  | -0.028 684 963 487 |
| C                                                                 | -0.372 490 938 904 | 0.115 262 952 124  | 0.150 240 277 686  |
| H                                                                 | -0.022 086 344 828 | -0.011 822 980 680 | -0.208 752 234 831 |
| H                                                                 | 0.015 496 870 007  | -0.179 403 302 110 | -0.096 166 010 455 |
| H                                                                 | 0.056 212 540 077  | -0.001 483 796 868 | 0.045 059 893 148  |
| H                                                                 | 0.090 576 881 440  | -0.026 046 605 746 | -0.006 195 022 115 |
| H                                                                 | 0.011 702 212 167  | 0.007 903 065 593  | 0.042 439 120 885  |
| H                                                                 | -0.011 136 075 274 | 0.005 147 703 235  | -0.174 890 575 812 |
| H                                                                 | -0.084 386 720 558 | -0.121 162 675 948 | -0.069 850 427 483 |
| H                                                                 | -0.132 829 874 366 | 0.038 867 742 008  | 0.045 759 203 889  |
| H                                                                 | -0.172 818 564 358 | 0.030 135 824 771  | -0.006 065 952 607 |
| H                                                                 | -0.108 676 581 346 | 0.061 156 147 401  | 0.124 781 304 035  |

Wavenumber/cm<sup>-1</sup>: 101.9634 , Max excitation: 3

| <i>l'</i> -matrix coefficients/(u <sup>1/2</sup> Å <sup>-1</sup> ) |                    |                    |                    |
|--------------------------------------------------------------------|--------------------|--------------------|--------------------|
| O                                                                  | 0.000 144 117 720  | -0.000 300 306 732 | 0.000 161 353 514  |
| C                                                                  | 0.001 129 034 481  | 0.007 584 723 554  | 0.004 141 039 444  |
| C                                                                  | 0.011 798 756 697  | 0.007 409 710 356  | -0.019 579 639 723 |
| C                                                                  | -0.023 682 350 912 | 0.004 511 488 432  | -0.037 041 657 610 |
| C                                                                  | -0.000 113 060 084 | 0.001 188 973 689  | -0.000 787 210 559 |
| C                                                                  | -0.000 414 592 642 | -0.000 356 151 018 | 0.000 351 780 823  |
| C                                                                  | -0.006 288 022 723 | 0.284 562 654 941  | -0.097 708 500 317 |
| H                                                                  | 0.001 099 564 378  | -0.031 060 097 504 | -0.012 303 294 375 |
| H                                                                  | 0.000 451 473 174  | 0.002 275 544 039  | -0.003 380 437 771 |
| H                                                                  | -0.045 219 768 940 | -0.010 493 868 030 | 0.061 427 989 129  |
| H                                                                  | 0.012 816 518 912  | 0.035 493 399 992  | 0.083 322 804 685  |
| H                                                                  | 0.069 162 192 140  | -0.058 729 431 035 | 0.046 970 310 436  |
| H                                                                  | -0.000 486 784 025 | -0.001 310 194 697 | -0.000 557 865 582 |
| H                                                                  | -0.000 364 490 487 | -0.000 794 598 023 | 0.004 285 818 275  |
| H                                                                  | -0.190 413 914 204 | -0.752 017 152 648 | 0.058 992 560 269  |
| H                                                                  | -0.169 018 445 409 | -0.012 743 627 213 | 0.218 913 007 435  |
| H                                                                  | 0.382 051 609 285  | -0.221 937 599 626 | 0.061 638 211 357  |

*Final state*

Wavenumber/cm<sup>-1</sup>: 168.7707 , Max excitation: 1

| $l'$ -matrix coefficients/(u <sup>1/2</sup> Å <sup>-1</sup> ) |                    |                                        |                    |
|---------------------------------------------------------------|--------------------|----------------------------------------|--------------------|
| O                                                             | -0.000 572 666 498 | 0.000 235 619 366                      | 0.000 370 343 432  |
| C                                                             | 0.001 091 822 663  | -0.003 025 786 883                     | -0.001 465 014 505 |
| C                                                             | -0.031 501 599 289 | -0.005 418 809 493                     | 0.036 399 905 731  |
| C                                                             | -0.011 431 203 836 | 0.005 928 442 810                      | -0.014 905 938 517 |
| C                                                             | -0.000 733 461 550 | $-4.550\,693\,100\,000 \times 10^{-5}$ | -0.001 364 353 200 |
| C                                                             | 0.001 094 339 273  | $4.746\,798\,200\,000 \times 10^{-5}$  | -0.000 907 252 024 |
| C                                                             | -0.268 027 385 905 | 0.039 833 722 208                      | 0.128 964 952 978  |
| H                                                             | 0.000 693 380 638  | 0.008 817 025 635                      | 0.005 023 888 297  |
| H                                                             | -0.000 233 114 410 | -0.000 991 798 180                     | 0.003 003 638 660  |
| H                                                             | 0.093 471 753 803  | 0.017 974 612 497                      | -0.123 884 999 358 |
| H                                                             | 0.007 753 149 247  | 0.012 429 550 202                      | 0.027 825 364 117  |
| H                                                             | 0.035 513 954 877  | -0.030 563 121 216                     | 0.025 172 978 447  |
| H                                                             | 0.001 206 415 156  | 0.001 488 486 758                      | -0.000 392 431 857 |
| H                                                             | 0.002 321 722 561  | -0.000 331 101 548                     | 0.003 469 658 814  |
| H                                                             | 0.008 235 828 148  | 0.110 821 265 227                      | 0.000 237 504 527  |
| H                                                             | 0.401 917 355 067  | 0.083 479 356 871                      | -0.553 155 126 800 |
| H                                                             | 0.519 815 308 934  | -0.332 889 338 373                     | 0.104 741 342 550  |



Wavenumber/cm<sup>-1</sup>: -218.0028, replaced by 218.0028 , Max excitation: 7

| $l'$ -matrix coefficients/(u <sup>1/2</sup> Å <sup>-1</sup> ) |                                      |                                      |                    |
|---------------------------------------------------------------|--------------------------------------|--------------------------------------|--------------------|
| O                                                             | 0.001 089 722 135                    | -0.000 762 222 874                   | -0.000 538 123 187 |
| C                                                             | -0.001 039 259 867                   | 0.001 216 007 140                    | 0.000 168 400 239  |
| C                                                             | -0.009 192 679 847                   | -0.003 050 669 355                   | 0.018 566 256 267  |
| C                                                             | 0.147 110 574 602                    | -0.024 822 670 880                   | 0.266 679 948 861  |
| C                                                             | 0.004 394 745 524                    | 0.000 545 658 053                    | 0.014 807 249 664  |
| C                                                             | -0.001 856 587 929                   | 0.001 082 352 461                    | -0.000 451 175 392 |
| C                                                             | -0.013 570 621 704                   | 0.046 180 314 606                    | -0.007 109 778 036 |
| H                                                             | 6.874 077 600 000 × 10 <sup>-5</sup> | 2.214 620 400 000 × 10 <sup>-5</sup> | -0.000 407 417 222 |
| H                                                             | -0.000 100 153 412                   | 0.001 176 980 910                    | 0.001 449 711 771  |
| H                                                             | 0.042 417 319 882                    | 0.010 389 307 765                    | -0.056 441 482 811 |
| H                                                             | -0.083 378 458 135                   | -0.265 810 737 341                   | -0.635 107 948 885 |
| H                                                             | -0.428 229 991 688                   | 0.352 339 083 591                    | -0.291 948 400 989 |
| H                                                             | -0.009 408 792 167                   | -0.010 051 772 081                   | -0.000 466 641 959 |
| H                                                             | -0.003 158 534 745                   | 0.004 574 387 887                    | -0.044 302 037 624 |
| H                                                             | -0.031 247 907 387                   | -0.116 228 720 538                   | 0.009 199 271 110  |
| H                                                             | -0.000 344 269 454                   | 0.001 090 562 519                    | -0.002 790 745 095 |
| H                                                             | 0.074 621 820 324                    | -0.047 477 320 690                   | 0.012 699 523 748  |

Wavenumber/cm<sup>-1</sup>: 220.0415 , Max excitation: 1

| $l'$ -matrix coefficients/(u <sup>1/2</sup> Å <sup>-1</sup> ) |                                      |                    |                    |
|---------------------------------------------------------------|--------------------------------------|--------------------|--------------------|
| O                                                             | -0.002 620 887 126                   | 0.001 018 310 278  | 0.000 762 453 170  |
| C                                                             | 0.002 874 597 770                    | -0.005 117 397 216 | 0.005 913 360 980  |
| C                                                             | -0.055 633 741 635                   | -0.013 776 816 480 | 0.070 155 747 724  |
| C                                                             | -0.111 498 016 161                   | 0.171 498 594 201  | 0.062 867 195 912  |
| C                                                             | 0.017 200 565 029                    | 0.019 036 361 164  | 0.006 438 065 474  |
| C                                                             | 0.003 513 958 662                    | -0.001 841 378 388 | -0.001 134 899 787 |
| C                                                             | 0.010 598 010 171                    | -0.006 764 773 905 | -0.029 728 422 200 |
| H                                                             | 5.264 149 700 000 × 10 <sup>-5</sup> | 0.011 583 760 477  | 0.004 413 151 285  |
| H                                                             | -0.006 713 575 146                   | 0.002 941 769 756  | -0.023 859 040 134 |
| H                                                             | 0.186 520 107 257                    | 0.046 523 762 934  | -0.242 748 892 524 |
| H                                                             | -0.085 179 343 249                   | -0.214 260 810 486 | -0.546 540 915 272 |
| H                                                             | 0.464 521 496 221                    | -0.371 656 764 401 | 0.337 723 690 238  |
| H                                                             | -0.055 065 955 044                   | -0.064 395 466 732 | -0.028 155 063 262 |
| H                                                             | 0.002 530 486 610                    | 0.001 299 623 653  | -0.000 860 472 547 |
| H                                                             | 0.014 695 107 710                    | 0.048 281 470 050  | -0.003 656 253 068 |
| H                                                             | -0.076 795 513 897                   | -0.014 184 069 521 | 0.101 120 657 033  |
| H                                                             | 0.024 798 796 292                    | -0.012 982 733 819 | 0.004 235 414 668  |

Wavenumber/cm<sup>-1</sup>: 316.3989 , Max excitation: 2

| $l'$ -matrix coefficients/(u <sup>1/2</sup> Å <sup>-1</sup> ) |                                        |                                        |                                        |
|---------------------------------------------------------------|----------------------------------------|----------------------------------------|----------------------------------------|
| O                                                             | 0.000 989 650 696                      | $-2.004\,574\,100\,000 \times 10^{-5}$ | $-6.822\,672\,400\,000 \times 10^{-5}$ |
| C                                                             | 0.001 660 071 353                      | 0.000 355 959 403                      | -0.001 778 165 418                     |
| C                                                             | 0.047 643 215 674                      | 0.010 984 853 686                      | -0.057 247 333 603                     |
| C                                                             | 0.009 922 547 705                      | -0.005 446 029 751                     | 0.006 873 817 765                      |
| C                                                             | 0.001 368 852 779                      | 0.001 508 624 096                      | -0.000 184 540 027                     |
| C                                                             | -0.001 979 402 896                     | 0.000 407 652 511                      | 0.000 608 145 906                      |
| C                                                             | -0.081 082 724 909                     | -0.046 140 059 822                     | -0.131 500 088 778                     |
| H                                                             | -0.000 496 860 215                     | 0.002 318 658 731                      | 0.000 464 154 634                      |
| H                                                             | -0.002 020 914 641                     | -0.001 970 834 888                     | 0.001 835 257 502                      |
| H                                                             | -0.161 623 943 871                     | -0.035 931 193 941                     | 0.206 063 809 479                      |
| H                                                             | -0.000 526 763 876                     | -0.003 795 864 039                     | -0.006 327 535 643                     |
| H                                                             | -0.029 997 285 075                     | 0.023 512 374 381                      | -0.021 079 145 918                     |
| H                                                             | -0.005 916 356 348                     | -0.007 016 244 292                     | -0.002 818 916 939                     |
| H                                                             | $-4.689\,687\,200\,000 \times 10^{-5}$ | 0.000 180 325 433                      | 0.005 386 862 045                      |
| H                                                             | 0.123 645 700 244                      | 0.519 549 951 701                      | -0.051 604 397 583                     |
| H                                                             | -0.323 586 229 838                     | -0.063 664 596 713                     | 0.421 865 161 374                      |
| H                                                             | 0.474 183 897 050                      | -0.300 791 704 143                     | 0.078 986 852 073                      |

Wavenumber/cm<sup>-1</sup>: 372.9528 , Max excitation: 1

| $l'$ -matrix coefficients/(u <sup>1/2</sup> Å <sup>-1</sup> ) |                    |                    |                    |
|---------------------------------------------------------------|--------------------|--------------------|--------------------|
| O                                                             | 0.001 713 534 346  | -0.000 104 188 136 | -0.000 159 653 583 |
| C                                                             | -0.001 212 066 563 | 0.003 135 023 424  | -0.010 253 735 229 |
| C                                                             | 0.147 300 778 759  | 0.034 189 466 993  | -0.191 119 848 016 |
| C                                                             | -0.029 295 139 378 | 0.061 476 300 594  | 0.042 907 175 164  |
| C                                                             | 0.006 373 943 732  | 0.009 754 988 266  | 0.006 277 725 577  |
| C                                                             | -0.003 024 835 251 | -0.000 949 783 898 | 0.000 317 918 215  |
| C                                                             | -0.020 338 475 348 | -0.003 014 042 587 | 0.062 235 534 598  |
| H                                                             | 0.000 960 985 979  | -0.004 437 806 255 | -0.002 708 930 385 |
| H                                                             | 0.008 660 481 943  | -0.003 810 851 102 | 0.033 559 769 030  |
| H                                                             | -0.513 756 002 933 | -0.118 311 474 644 | 0.664 964 763 123  |
| H                                                             | -0.038 627 897 168 | -0.096 908 870 545 | -0.253 716 985 858 |
| H                                                             | 0.144 183 511 383  | -0.112 069 172 468 | 0.106 081 818 768  |
| H                                                             | -0.030 565 473 824 | -0.035 913 560 755 | -0.015 719 982 172 |
| H                                                             | 0.005 605 780 151  | 0.001 352 382 711  | -0.005 961 247 281 |
| H                                                             | -0.019 544 456 755 | -0.063 943 659 751 | 0.008 297 785 902  |
| H                                                             | 0.163 928 635 287  | 0.032 577 566 408  | -0.215 225 371 389 |
| H                                                             | -0.072 194 720 254 | 0.040 831 027 149  | -0.009 516 369 286 |

Wavenumber/cm<sup>-1</sup>: 378.5797 , Max excitation: 1

| $l'$ -matrix coefficients/(u <sup>1/2</sup> Å <sup>-1</sup> ) |                    |                    |                    |
|---------------------------------------------------------------|--------------------|--------------------|--------------------|
| O                                                             | 0.002 655 363 942  | -0.001 114 753 364 | -0.000 468 454 267 |
| C                                                             | -0.001 357 195 197 | 0.238 119 878 549  | 0.098 597 557 700  |
| C                                                             | 0.001 436 789 580  | 0.000 602 475 749  | 0.002 385 710 385  |
| C                                                             | -0.002 461 759 281 | 0.005 672 046 230  | 0.004 738 394 547  |
| C                                                             | -0.044 976 916 713 | -0.055 260 857 300 | -0.013 466 183 536 |
| C                                                             | 0.001 000 296 873  | 0.002 768 650 528  | -0.003 659 115 554 |
| C                                                             | -0.001 892 205 061 | -0.009 697 584 050 | 0.003 680 260 326  |
| H                                                             | -0.015 124 997 720 | -0.852 665 445 102 | -0.352 955 111 804 |
| H                                                             | -0.002 209 734 257 | 0.024 386 790 984  | 0.014 747 856 722  |
| H                                                             | 0.003 837 306 705  | 0.001 872 346 460  | -0.005 767 040 231 |
| H                                                             | -0.004 438 058 337 | -0.010 963 106 091 | -0.027 538 443 705 |
| H                                                             | 0.016 017 674 111  | -0.013 171 092 504 | 0.012 827 371 398  |
| H                                                             | 0.159 216 857 310  | 0.200 256 704 865  | 0.081 719 583 438  |
| H                                                             | -0.008 078 023 890 | -0.003 671 116 978 | -0.025 281 526 596 |
| H                                                             | 0.005 615 198 390  | 0.029 275 630 834  | -0.004 573 007 613 |
| H                                                             | 0.006 186 579 817  | -0.000 513 404 686 | -0.008 800 487 438 |
| H                                                             | -0.005 040 447 755 | 0.000 666 969 729  | -0.001 050 057 246 |

Wavenumber/cm<sup>-1</sup>: 551.7105 , Max excitation: 1

| $l'$ -matrix coefficients/(u <sup>1/2</sup> Å <sup>-1</sup> ) |                    |                                      |                                       |
|---------------------------------------------------------------|--------------------|--------------------------------------|---------------------------------------|
| O                                                             | 0.002 123 532 710  | 7.664 114 300 000 × 10 <sup>-5</sup> | -0.000 649 013 760                    |
| C                                                             | -0.000 322 811 551 | -0.069 034 775 244                   | -0.037 649 779 181                    |
| C                                                             | 0.003 557 047 805  | 0.001 108 146 238                    | -0.004 562 186 205                    |
| C                                                             | -0.007 388 865 624 | 0.018 010 654 764                    | 0.009 307 317 732                     |
| C                                                             | -0.158 072 338 596 | -0.186 049 470 007                   | -0.068 091 308 237                    |
| C                                                             | -0.000 202 281 322 | -0.008 896 539 273                   | 0.007 255 650 822                     |
| C                                                             | 0.000 159 224 928  | 0.002 929 723 640                    | -0.002 269 770 150                    |
| H                                                             | 0.002 313 143 049  | 0.249 374 771 592                    | 0.104 586 833 543                     |
| H                                                             | 0.004 622 244 999  | -0.008 504 694 677                   | 0.013 935 952 726                     |
| H                                                             | -0.011 956 339 127 | -0.002 215 357 241                   | 0.013 950 795 683                     |
| H                                                             | -0.011 048 185 333 | -0.026 489 864 426                   | -0.066 722 796 670                    |
| H                                                             | 0.042 857 462 139  | -0.034 543 986 655                   | 0.030 733 507 060                     |
| H                                                             | 0.549 182 715 778  | 0.678 511 985 848                    | 0.283 016 549 468                     |
| H                                                             | -0.025 156 437 414 | -0.013 548 270 672                   | -0.053 628 181 223                    |
| H                                                             | -0.000 309 778 715 | -0.004 851 153 891                   | 0.001 075 032 193                     |
| H                                                             | -0.004 851 165 684 | 9.746 536 900 000 × 10 <sup>-5</sup> | 0.007 152 710 799                     |
| H                                                             | 0.006 039 180 256  | -0.002 990 491 786                   | -8.965 258 900 000 × 10 <sup>-5</sup> |

Wavenumber/cm<sup>-1</sup>: 676.3676 , Max excitation: 2

| $l'$ -matrix coefficients/(u <sup>1/2</sup> Å <sup>-1</sup> ) |                                        |                    |
|---------------------------------------------------------------|----------------------------------------|--------------------|
| O -0.004 402 790 995                                          | 0.000 904 093 848                      | 0.000 476 035 969  |
| C 0.030 031 948 549                                           | -0.005 566 293 352                     | 0.121 187 847 198  |
| C 0.003 201 602 521                                           | 0.002 259 113 217                      | -0.004 062 623 956 |
| C 0.005 061 738 222                                           | -0.002 135 366 860                     | 0.013 063 805 106  |
| C -0.030 469 554 268                                          | $2.472\,088\,200\,000 \times 10^{-5}$  | -0.233 348 884 903 |
| C -0.002 635 826 071                                          | 0.007 361 274 344                      | 0.001 135 122 608  |
| C -0.000 968 334 631                                          | $-8.330\,860\,000\,000 \times 10^{-6}$ | 0.001 240 131 429  |
| H 0.004 938 254 145                                           | -0.006 944 610 880                     | 0.012 956 595 378  |
| H -0.096 669 363 217                                          | 0.034 402 985 354                      | -0.450 032 333 037 |
| H -0.010 432 093 654                                          | -0.003 735 239 273                     | 0.016 389 276 266  |
| H -0.006 411 983 372                                          | -0.014 007 427 347                     | -0.029 890 543 914 |
| H -0.015 604 069 606                                          | 0.015 826 796 847                      | -0.013 622 244 262 |
| H 0.028 818 718 692                                           | 0.036 973 950 643                      | -0.017 402 879 508 |
| H 0.097 387 021 868                                           | -0.072 229 445 979                     | 0.834 169 802 164  |
| H -0.001 846 617 398                                          | -0.004 353 419 352                     | 0.000 191 485 700  |
| H 0.006 859 687 014                                           | 0.001 840 183 459                      | -0.006 956 111 172 |
| H -0.004 071 280 696                                          | 0.001 944 254 489                      | 0.000 206 996 452  |

Wavenumber/cm<sup>-1</sup>: 779.0073 , Max excitation: 2

| $l'$ -matrix coefficients/(u <sup>1/2</sup> Å <sup>-1</sup> ) |                    |                    |
|---------------------------------------------------------------|--------------------|--------------------|
| O -0.000 286 766 246                                          | 0.002 435 226 245  | 0.000 638 156 308  |
| C 0.061 221 070 204                                           | -0.009 619 696 616 | 0.223 796 227 149  |
| C 0.005 383 805 042                                           | 0.003 913 787 353  | -0.006 144 274 663 |
| C -0.000 946 591 567                                          | -0.001 699 284 103 | -0.006 067 690 475 |
| C 0.012 609 944 018                                           | -0.000 134 317 398 | 0.128 390 098 718  |
| C -0.007 914 394 614                                          | -0.021 606 107 798 | 0.002 577 347 580  |
| C -0.002 811 304 072                                          | -0.001 322 585 396 | 0.001 787 505 003  |
| H 0.010 307 468 941                                           | 0.008 003 281 476  | 0.032 720 846 294  |
| H -0.185 026 860 340                                          | 0.055 838 518 401  | -0.822 135 039 982 |
| H -0.019 397 413 876                                          | -0.006 655 516 107 | 0.027 026 513 820  |
| H 0.004 087 819 672                                           | 0.007 174 276 698  | 0.019 797 654 752  |
| H 0.001 317 339 123                                           | -0.002 329 897 249 | 0.001 569 089 411  |
| H -0.001 580 678 006                                          | -0.003 488 787 865 | 0.015 957 183 757  |
| H -0.048 573 741 863                                          | 0.034 312 244 017  | -0.456 801 680 980 |
| H 0.000 255 420 662                                           | 0.002 718 561 986  | -0.001 069 910 535 |
| H 0.007 758 891 010                                           | 0.000 206 987 499  | -0.009 364 768 171 |
| H -0.001 161 323 743                                          | -0.000 306 120 633 | 0.001 104 962 798  |

Wavenumber/cm<sup>-1</sup>: 795.6446 , Max excitation: 2

| $l'$ -matrix coefficients/(u <sup>1/2</sup> Å <sup>-1</sup> ) |                    |                    |                    |
|---------------------------------------------------------------|--------------------|--------------------|--------------------|
| O                                                             | 0.014 028 001 563  | -0.004 882 513 059 | -0.003 289 299 369 |
| C                                                             | -0.040 259 529 754 | 0.071 681 254 517  | -0.038 383 737 706 |
| C                                                             | 0.092 486 850 198  | 0.013 976 106 983  | -0.024 327 017 570 |
| C                                                             | 0.054 677 626 617  | -0.134 128 382 471 | -0.047 009 696 840 |
| C                                                             | 0.002 964 030 357  | -0.014 471 400 007 | -0.001 381 844 570 |
| C                                                             | -0.021 569 962 436 | 0.021 932 243 409  | -0.000 823 884 363 |
| C                                                             | 0.120 548 290 821  | 0.001 937 630 390  | -0.036 569 201 336 |
| H                                                             | 0.057 801 925 874  | -0.071 152 223 452 | 0.196 460 737 978  |
| H                                                             | 0.017 391 193 166  | -0.207 529 633 161 | -0.025 407 308 087 |
| H                                                             | -0.038 197 879 792 | -0.022 136 896 570 | -0.069 367 164 210 |
| H                                                             | -0.232 844 371 582 | 0.250 500 767 132  | -0.088 215 446 994 |
| H                                                             | -0.000 149 933 552 | 0.209 249 744 662  | 0.284 626 933 790  |
| H                                                             | -0.000 249 806 121 | -0.001 001 511 522 | -0.007 824 026 512 |
| H                                                             | -0.008 788 108 549 | 0.004 628 949 088  | 0.000 387 760 626  |
| H                                                             | -0.505 022 854 272 | 0.140 316 382 309  | 0.105 759 370 018  |
| H                                                             | 0.157 052 762 098  | 0.246 200 020 147  | 0.131 728 705 603  |
| H                                                             | -0.223 818 696 964 | -0.394 745 556 131 | -0.002 441 379 336 |

Wavenumber/cm<sup>-1</sup>: 844.5173 , Max excitation: 1

| $l'$ -matrix coefficients/(u <sup>1/2</sup> Å <sup>-1</sup> ) |                    |                    |                    |
|---------------------------------------------------------------|--------------------|--------------------|--------------------|
| O                                                             | -0.002 375 947 221 | 0.001 456 273 533  | 0.000 153 515 355  |
| C                                                             | -0.015 421 576 781 | 0.016 114 122 446  | -0.011 906 676 269 |
| C                                                             | -0.026 351 522 535 | 0.083 516 475 676  | -0.020 908 147 583 |
| C                                                             | 0.057 621 828 870  | -0.116 750 410 245 | -0.036 122 543 446 |
| C                                                             | -0.033 989 378 375 | -0.044 640 469 649 | 0.041 900 263 630  |
| C                                                             | 0.004 070 043 862  | -0.006 940 796 945 | 0.005 053 742 606  |
| C                                                             | -0.057 906 232 477 | 0.145 440 248 176  | 0.017 284 638 278  |
| H                                                             | 0.036 438 022 248  | -0.027 245 925 784 | 0.071 238 627 653  |
| H                                                             | 0.012 059 380 810  | -0.078 307 057 440 | -0.008 369 216 999 |
| H                                                             | 0.014 183 007 014  | -0.047 522 459 982 | -0.004 282 558 966 |
| H                                                             | -0.170 107 612 372 | 0.198 974 462 664  | -0.073 113 025 989 |
| H                                                             | -0.019 867 247 036 | 0.134 223 626 562  | 0.227 159 782 753  |
| H                                                             | 0.019 327 383 547  | 0.048 515 616 530  | -0.174 846 801 928 |
| H                                                             | 0.098 689 876 769  | 0.147 462 874 876  | 0.006 154 915 876  |
| H                                                             | 0.196 728 346 570  | -0.059 777 167 030 | -0.425 539 181 775 |
| H                                                             | 0.163 835 495 408  | -0.579 291 502 964 | 0.048 480 726 774  |
| H                                                             | -0.093 357 959 415 | -0.007 736 590 747 | 0.348 725 020 491  |

Wavenumber/cm<sup>-1</sup>: 901.395 , Max excitation: 1

| $l'$ -matrix coefficients/(u <sup>1/2</sup> Å <sup>-1</sup> ) |                    |                    |
|---------------------------------------------------------------|--------------------|--------------------|
| O -0.018 858 724 239                                          | 0.006 524 587 290  | 0.004 685 904 242  |
| C -0.018 681 684 001                                          | 0.069 222 528 745  | -0.035 718 569 493 |
| C -0.014 914 269 763                                          | -0.051 532 976 469 | 0.010 265 524 534  |
| C 0.065 829 546 689                                           | -0.102 744 504 770 | -0.050 391 061 962 |
| C -0.057 407 320 610                                          | -0.076 018 132 959 | 0.070 040 225 960  |
| C 0.028 690 874 674                                           | -0.017 970 560 754 | -0.002 454 059 691 |
| C -0.037 960 833 846                                          | -0.087 380 050 200 | 0.086 592 428 574  |
| H 0.032 257 277 197                                           | -0.065 256 710 779 | 0.177 482 357 068  |
| H 0.004 224 699 949                                           | -0.188 779 920 775 | -0.021 798 938 745 |
| H 0.003 890 602 342                                           | 0.017 485 790 936  | 0.013 791 042 892  |
| H -0.207 477 796 321                                          | 0.205 268 512 448  | -0.071 959 685 035 |
| H -0.015 437 255 762                                          | 0.174 133 108 782  | 0.252 843 551 186  |
| H 0.018 191 563 342                                           | 0.091 143 207 323  | -0.294 425 455 030 |
| H 0.165 674 049 972                                           | 0.249 404 494 982  | 0.009 693 854 514  |
| H 0.249 400 421 310                                           | -0.069 905 552 566 | 0.144 834 901 525  |
| H -0.303 634 002 719                                          | 0.191 642 728 730  | -0.173 349 714 758 |
| H 0.246 944 084 530                                           | 0.288 559 603 542  | -0.326 190 154 120 |

Wavenumber/cm<sup>-1</sup>: 920.0296 , Max excitation: 2

| $l'$ -matrix coefficients/(u <sup>1/2</sup> Å <sup>-1</sup> ) |                    |                    |
|---------------------------------------------------------------|--------------------|--------------------|
| O -0.007 980 240 303                                          | 0.004 010 979 109  | 0.001 790 051 366  |
| C -0.012 620 675 335                                          | 0.021 619 295 912  | -0.016 414 599 701 |
| C 0.025 987 894 198                                           | 0.017 748 595 375  | 0.011 801 091 451  |
| C -0.070 526 597 193                                          | 0.086 564 742 582  | 0.053 548 911 513  |
| C -0.111 307 484 490                                          | -0.111 879 857 981 | 0.131 567 445 967  |
| C 0.011 900 937 641                                           | -0.047 764 452 177 | 0.017 502 344 632  |
| C 0.044 468 768 306                                           | 0.011 969 004 735  | -0.020 577 799 941 |
| H 0.025 562 946 594                                           | -0.015 636 267 038 | 0.046 338 940 035  |
| H 0.001 398 216 113                                           | -0.048 197 759 181 | -0.006 079 691 606 |
| H -0.024 376 469 176                                          | -0.013 158 120 231 | -0.026 842 376 297 |
| H 0.240 912 646 422                                           | -0.232 286 930 318 | 0.077 129 968 185  |
| H 0.033 995 579 797                                           | -0.175 885 327 056 | -0.279 762 386 622 |
| H 0.037 800 024 884                                           | 0.169 484 802 205  | -0.533 511 349 290 |
| H 0.320 462 946 486                                           | 0.444 137 937 553  | 0.014 630 616 877  |
| H -0.188 873 789 664                                          | 0.051 298 347 833  | 0.001 929 503 997  |
| H 0.073 508 851 544                                           | 0.038 791 722 671  | 0.052 895 289 754  |
| H -0.101 639 696 915                                          | -0.159 473 162 299 | 0.033 663 649 941  |

Wavenumber/cm<sup>-1</sup>: 958.1734 , Max excitation: 1

| $l'$ -matrix coefficients/(u <sup>1/2</sup> Å <sup>-1</sup> ) |                    |                    |                    |
|---------------------------------------------------------------|--------------------|--------------------|--------------------|
| O                                                             | 0.009 406 379 429  | 0.000 943 541 900  | -0.002 506 240 661 |
| C                                                             | 0.083 109 897 978  | -0.177 818 486 933 | 0.109 135 583 575  |
| C                                                             | -0.006 069 076 199 | -0.032 813 988 082 | 0.003 141 280 600  |
| C                                                             | 0.050 463 958 462  | -0.083 069 665 346 | -0.033 529 064 164 |
| C                                                             | -0.034 255 480 659 | -0.032 376 383 882 | 0.029 552 657 809  |
| C                                                             | -0.028 864 622 700 | -0.062 447 409 693 | 0.046 623 249 662  |
| C                                                             | 0.019 468 285 655  | -0.008 544 287 711 | -0.018 820 026 648 |
| H                                                             | -0.152 398 174 102 | 0.216 214 896 248  | -0.560 979 103 073 |
| H                                                             | -0.020 996 269 071 | 0.591 458 224 098  | 0.062 703 445 069  |
| H                                                             | -0.003 091 675 052 | 0.015 850 238 695  | 0.004 469 963 885  |
| H                                                             | -0.160 749 460 555 | 0.160 904 548 973  | -0.053 120 202 897 |
| H                                                             | -0.007 018 815 174 | 0.130 097 466 042  | 0.187 005 938 715  |
| H                                                             | 0.011 396 302 204  | 0.052 593 026 257  | -0.164 561 048 294 |
| H                                                             | 0.092 839 996 701  | 0.145 313 543 659  | 0.001 366 528 808  |
| H                                                             | -0.077 053 442 540 | 0.025 116 600 849  | 0.068 025 927 122  |
| H                                                             | 0.013 131 595 875  | 0.080 736 292 006  | 0.014 057 851 991  |
| H                                                             | -0.022 994 723 039 | -0.051 364 821 230 | -0.018 811 661 660 |

Wavenumber/cm<sup>-1</sup>: 984.7985 , Max excitation: 1

| $l'$ -matrix coefficients/(u <sup>1/2</sup> Å <sup>-1</sup> ) |                    |                    |                    |
|---------------------------------------------------------------|--------------------|--------------------|--------------------|
| O                                                             | 0.007 677 612 307  | -0.002 997 384 658 | -0.000 601 861 206 |
| C                                                             | 0.022 143 955 561  | 0.006 229 186 591  | -0.028 123 470 691 |
| C                                                             | 0.049 501 657 362  | 0.039 551 098 476  | 0.077 865 272 192  |
| C                                                             | 0.039 855 036 221  | 0.009 336 072 538  | -0.039 447 178 846 |
| C                                                             | -0.005 498 341 986 | -0.026 797 261 769 | 0.009 123 379 795  |
| C                                                             | -0.017 229 289 547 | 0.012 031 070 974  | 0.000 619 273 855  |
| C                                                             | -0.220 766 695 910 | -0.138 153 054 045 | -0.354 735 295 783 |
| H                                                             | -0.005 624 451 397 | -0.024 019 367 710 | 0.046 477 900 174  |
| H                                                             | -0.050 475 373 485 | -0.032 450 636 628 | 0.005 401 018 747  |
| H                                                             | -0.070 138 593 178 | -0.047 376 986 385 | -0.052 111 944 787 |
| H                                                             | -0.079 978 513 895 | -0.032 734 558 010 | 0.017 755 497 415  |
| H                                                             | -0.025 746 757 479 | 0.014 696 710 229  | 0.048 370 162 555  |
| H                                                             | -0.011 444 225 191 | 0.020 233 201 469  | -0.041 940 647 112 |
| H                                                             | 0.014 851 324 311  | 0.036 251 340 072  | 0.001 560 488 460  |
| H                                                             | 0.198 893 552 859  | -0.052 839 507 968 | 0.434 530 383 615  |
| H                                                             | 0.397 714 685 610  | 0.182 618 316 339  | 0.283 400 560 298  |
| H                                                             | 0.056 999 900 314  | 0.285 177 091 367  | 0.414 325 901 633  |

Wavenumber/cm<sup>-1</sup>: 1022.1833 , Max excitation: 1

| $l'$ -matrix coefficients/(u <sup>1/2</sup> Å <sup>-1</sup> ) |                    |                    |                    |
|---------------------------------------------------------------|--------------------|--------------------|--------------------|
| O                                                             | -0.516 788 429 033 | 0.155 745 464 719  | 0.106 459 572 764  |
| C                                                             | -0.014 007 284 312 | 0.020 363 450 054  | -0.009 001 376 202 |
| C                                                             | -0.049 945 221 154 | -0.083 174 845 629 | 0.042 868 680 404  |
| C                                                             | -0.019 615 287 714 | 0.078 156 721 476  | -0.034 681 861 154 |
| C                                                             | -0.011 450 255 678 | -0.002 781 785 500 | 0.009 659 849 279  |
| C                                                             | 0.751 308 531 631  | -0.234 113 402 000 | -0.147 359 343 289 |
| C                                                             | 0.016 889 402 042  | 0.019 956 713 097  | -0.021 950 203 016 |
| H                                                             | 0.016 222 196 349  | 0.012 328 861 292  | -0.021 462 825 076 |
| H                                                             | -0.043 507 872 922 | 0.005 613 190 121  | 0.003 837 427 625  |
| H                                                             | -0.067 813 124 659 | 0.087 799 384 980  | -0.001 862 096 388 |
| H                                                             | -0.004 563 936 948 | 0.001 062 707 796  | 0.000 226 677 723  |
| H                                                             | -0.082 542 815 090 | -0.006 350 445 769 | 0.056 493 335 084  |
| H                                                             | 0.011 946 816 489  | -0.019 738 398 973 | 0.019 252 062 926  |
| H                                                             | -0.068 303 463 220 | 0.022 082 147 674  | 0.014 291 712 149  |
| H                                                             | -0.019 579 278 031 | 0.012 637 917 921  | 0.026 084 447 094  |
| H                                                             | 0.015 515 596 410  | -0.012 377 095 037 | 0.001 582 892 917  |
| H                                                             | -0.022 252 382 785 | -0.027 664 781 924 | 0.031 332 594 304  |

Wavenumber/cm<sup>-1</sup>: 1050.8196 , Max excitation: 2

| $l'$ -matrix coefficients/(u <sup>1/2</sup> Å <sup>-1</sup> ) |                    |                    |                    |
|---------------------------------------------------------------|--------------------|--------------------|--------------------|
| O                                                             | -0.020 935 018 226 | 0.004 511 639 595  | 0.007 082 363 172  |
| C                                                             | -0.038 577 733 202 | -0.039 365 749 988 | -0.059 201 720 793 |
| C                                                             | 0.321 505 785 709  | 0.244 279 504 473  | 0.298 161 942 289  |
| C                                                             | 0.034 026 626 575  | -0.015 366 420 694 | -0.108 701 584 205 |
| C                                                             | -0.039 947 507 413 | 0.022 597 570 163  | -0.019 209 360 384 |
| C                                                             | 0.031 546 079 494  | 0.000 809 308 711  | -0.019 322 134 897 |
| C                                                             | -0.141 707 811 069 | -0.055 517 159 642 | 0.099 388 250 776  |
| H                                                             | 0.104 851 339 014  | -0.003 422 357 238 | -0.029 418 290 981 |
| H                                                             | -0.095 113 581 220 | 0.076 719 786 107  | 0.009 324 878 191  |
| H                                                             | -0.453 194 371 611 | -0.356 999 438 633 | -0.412 412 789 217 |
| H                                                             | -0.152 170 093 181 | -0.220 300 300 096 | 0.080 705 321 571  |
| H                                                             | 0.051 379 191 439  | 0.053 772 188 388  | -0.014 662 722 869 |
| H                                                             | 0.025 407 621 984  | -0.036 477 497 582 | 0.019 794 413 731  |
| H                                                             | 0.028 215 808 298  | -0.046 309 592 133 | -0.012 977 836 613 |
| H                                                             | 0.009 390 812 433  | -0.047 029 444 163 | -0.181 838 085 949 |
| H                                                             | -0.021 646 628 443 | 0.012 966 705 798  | 0.038 159 747 611  |
| H                                                             | 0.010 339 271 948  | 0.005 635 381 561  | -0.184 618 186 244 |



Wavenumber/cm<sup>-1</sup>: 1062.4498 , Max excitation: 1

| $l'$ -matrix coefficients/(u <sup>1/2</sup> Å <sup>-1</sup> ) |                    |                    |                    |
|---------------------------------------------------------------|--------------------|--------------------|--------------------|
| O                                                             | 0.014 786 822 881  | -0.001 664 514 521 | -0.003 790 043 656 |
| C                                                             | 0.099 217 030 923  | 0.007 507 406 814  | -0.000 779 038 349 |
| C                                                             | -0.195 654 009 834 | -0.017 825 812 465 | 0.051 162 088 175  |
| C                                                             | 0.346 690 835 519  | 0.297 462 511 880  | -0.133 898 283 663 |
| C                                                             | 0.044 624 619 124  | -0.160 628 834 354 | -0.046 947 021 282 |
| C                                                             | -0.050 331 126 543 | 0.034 862 830 723  | -0.004 427 368 057 |
| C                                                             | 0.086 432 326 407  | 0.037 623 194 338  | -0.012 059 858 702 |
| H                                                             | -0.121 384 972 282 | -0.009 870 686 023 | 0.032 752 674 966  |
| H                                                             | -0.088 734 676 350 | -0.034 231 111 718 | 0.023 353 309 437  |
| H                                                             | 0.104 152 717 319  | -0.147 247 921 732 | 0.114 320 269 794  |
| H                                                             | -0.447 523 814 301 | -0.329 295 158 516 | 0.208 109 815 986  |
| H                                                             | -0.304 435 747 535 | -0.256 023 408 433 | 0.141 485 684 519  |
| H                                                             | -0.204 404 916 064 | 0.106 220 001 771  | 0.048 648 024 415  |
| H                                                             | 0.006 221 885 095  | 0.056 634 983 138  | -0.003 597 617 732 |
| H                                                             | -0.058 887 881 017 | 0.028 459 273 786  | 0.013 388 312 130  |
| H                                                             | -0.061 565 782 760 | -0.036 052 652 330 | -0.072 652 542 077 |
| H                                                             | -0.024 884 499 242 | -0.058 910 607 953 | 0.016 558 836 361  |

Wavenumber/cm<sup>-1</sup>: 1105.9033 , Max excitation: 1

| $l'$ -matrix coefficients/(u <sup>1/2</sup> Å <sup>-1</sup> ) |                    |                    |                    |
|---------------------------------------------------------------|--------------------|--------------------|--------------------|
| O                                                             | 0.021 716 888 069  | -0.010 000 232 294 | -0.002 270 185 913 |
| C                                                             | 0.266 009 400 483  | 0.078 412 445 435  | -0.126 921 405 175 |
| C                                                             | 0.145 746 747 134  | -0.339 478 056 322 | 0.082 067 552 943  |
| C                                                             | -0.093 896 759 267 | 0.105 107 250 812  | 0.029 644 048 874  |
| C                                                             | 0.182 748 782 338  | -0.136 715 365 735 | -0.028 788 017 648 |
| C                                                             | -0.112 419 555 083 | 0.029 296 471 956  | 0.024 421 629 517  |
| C                                                             | -0.059 184 792 910 | 0.091 629 518 386  | 0.030 837 782 329  |
| H                                                             | -0.325 892 680 934 | -0.019 968 755 882 | 0.082 050 539 650  |
| H                                                             | -0.292 527 372 030 | -0.017 642 013 173 | 0.042 310 356 172  |
| H                                                             | -0.331 196 094 035 | 0.420 350 835 089  | -0.171 213 722 235 |
| H                                                             | 0.057 411 817 887  | 0.055 455 113 712  | -0.009 433 055 820 |
| H                                                             | -0.005 601 231 307 | 0.057 470 928 767  | 0.011 095 850 471  |
| H                                                             | -0.196 994 361 732 | 0.143 863 377 673  | 0.035 450 002 893  |
| H                                                             | -0.171 412 689 092 | 0.143 382 583 796  | 0.033 533 970 781  |
| H                                                             | 0.067 702 333 187  | -0.004 024 174 132 | -0.011 170 480 789 |
| H                                                             | 0.029 602 841 498  | -0.085 793 558 108 | 0.022 207 193 936  |
| H                                                             | -0.053 329 576 170 | -0.060 382 562 875 | -0.064 660 859 029 |

Wavenumber/cm<sup>-1</sup>: 1136.5791 , Max excitation: 1

| $l'$ -matrix coefficients/(u <sup>1/2</sup> Å <sup>-1</sup> ) |                    |                    |                    |
|---------------------------------------------------------------|--------------------|--------------------|--------------------|
| O                                                             | 0.008 567 191 865  | -0.022 193 639 222 | 0.008 892 215 371  |
| C                                                             | 0.076 797 389 093  | 0.003 781 909 143  | -0.043 069 430 927 |
| C                                                             | 0.025 704 894 247  | -0.165 763 460 880 | 0.134 356 815 087  |
| C                                                             | 0.038 022 186 993  | -0.027 613 713 981 | 0.090 394 446 106  |
| C                                                             | -0.309 058 944 289 | 0.143 831 826 441  | -0.055 443 525 587 |
| C                                                             | 0.043 253 495 385  | 0.109 092 052 490  | -0.078 761 580 853 |
| C                                                             | 0.034 697 863 802  | 0.072 177 217 308  | -0.084 003 160 865 |
| H                                                             | -0.144 718 070 207 | -0.020 471 469 328 | 0.047 564 212 750  |
| H                                                             | -0.184 820 751 676 | -0.015 225 731 143 | 0.035 205 536 918  |
| H                                                             | 0.015 303 441 192  | 0.250 069 601 108  | 0.095 444 174 201  |
| H                                                             | -0.295 192 758 516 | -0.159 363 126 799 | 0.132 215 737 711  |
| H                                                             | 0.254 956 546 007  | 0.161 521 895 834  | -0.128 707 882 829 |
| H                                                             | 0.228 995 503 024  | -0.214 130 224 663 | -0.010 658 372 759 |
| H                                                             | 0.458 715 902 368  | -0.268 994 303 023 | -0.103 065 306 748 |
| H                                                             | 0.017 211 732 735  | 0.021 297 624 841  | 0.064 354 253 136  |
| H                                                             | -0.029 834 475 583 | -0.080 199 206 178 | -0.065 178 135 112 |
| H                                                             | -0.042 058 186 869 | -0.053 847 482 750 | 0.023 487 080 128  |

Wavenumber/cm<sup>-1</sup>: 1160.2179 , Max excitation: 1

| $l'$ -matrix coefficients/(u <sup>1/2</sup> Å <sup>-1</sup> ) |                    |                    |                    |
|---------------------------------------------------------------|--------------------|--------------------|--------------------|
| O                                                             | 0.031 129 573 167  | 0.008 723 127 244  | -0.012 066 482 573 |
| C                                                             | -0.354 390 436 845 | 0.055 664 030 261  | 0.031 708 928 313  |
| C                                                             | 0.235 870 837 954  | -0.201 357 659 763 | 0.075 681 862 520  |
| C                                                             | -0.078 879 232 038 | 0.111 343 065 649  | 0.041 942 830 989  |
| C                                                             | 0.095 198 436 366  | -0.080 745 116 124 | -0.134 585 710 449 |
| C                                                             | -0.030 335 432 513 | -0.129 344 851 436 | 0.074 974 153 401  |
| C                                                             | -0.052 772 663 869 | 0.100 981 920 150  | -0.072 156 475 456 |
| H                                                             | 0.382 763 343 422  | 0.048 188 917 920  | -0.089 609 595 006 |
| H                                                             | 0.384 890 578 339  | 0.046 952 968 261  | -0.098 268 214 522 |
| H                                                             | 0.044 890 353 067  | 0.247 438 216 019  | 0.058 488 990 293  |
| H                                                             | -0.250 865 423 549 | -0.175 059 302 636 | 0.131 801 371 546  |
| H                                                             | 0.156 171 592 759  | 0.182 925 519 466  | -0.065 616 228 207 |
| H                                                             | -0.225 151 553 542 | 0.139 590 993 699  | 0.066 062 692 497  |
| H                                                             | -0.033 645 097 028 | 0.098 748 700 524  | -0.020 981 950 115 |
| H                                                             | 0.088 953 008 425  | 0.007 903 390 615  | 0.073 066 735 059  |
| H                                                             | 0.019 805 788 523  | -0.081 263 593 522 | -0.013 219 932 304 |
| H                                                             | -0.052 153 768 272 | -0.054 962 937 520 | -0.054 286 131 865 |

Wavenumber/cm<sup>-1</sup>: 1217.8164 , Max excitation: 1

| $l'$ -matrix coefficients/(u <sup>1/2</sup> Å <sup>-1</sup> ) |                    |                    |                    |
|---------------------------------------------------------------|--------------------|--------------------|--------------------|
| O                                                             | -0.019 812 290 807 | 0.007 948 682 926  | 0.004 485 266 882  |
| C                                                             | 0.064 560 281 232  | -0.098 520 913 015 | -0.081 802 378 245 |
| C                                                             | -0.003 220 692 109 | 0.244 029 904 050  | 0.363 508 101 168  |
| C                                                             | -0.201 226 792 159 | -0.148 128 637 326 | -0.098 104 103 028 |
| C                                                             | 0.171 494 394 111  | -0.014 702 683 483 | -0.036 159 239 847 |
| C                                                             | -0.016 333 102 639 | -0.007 495 516 481 | -0.003 514 072 436 |
| C                                                             | 0.128 521 316 355  | -0.056 466 972 291 | -0.229 026 822 767 |
| H                                                             | 0.126 653 470 683  | -0.049 964 279 532 | 0.034 830 116 356  |
| H                                                             | -0.390 523 778 886 | 0.028 077 446 477  | 0.076 084 726 557  |
| H                                                             | 0.212 680 255 680  | -0.036 996 926 022 | 0.252 935 082 073  |
| H                                                             | -0.002 423 776 733 | -0.136 694 854 185 | 0.004 756 306 223  |
| H                                                             | 0.186 067 484 429  | 0.243 933 463 619  | -0.039 948 280 168 |
| H                                                             | -0.027 066 244 122 | 0.061 280 803 271  | -0.021 893 719 446 |
| H                                                             | -0.260 043 977 733 | 0.168 756 275 253  | 0.037 748 487 766  |
| H                                                             | -0.104 080 587 455 | 0.024 677 728 791  | 0.028 324 506 600  |
| H                                                             | -0.166 070 424 209 | -0.056 631 399 913 | -0.218 236 204 207 |
| H                                                             | 0.007 362 214 606  | 0.002 487 264 835  | 0.121 287 838 383  |

Wavenumber/cm<sup>-1</sup>: 1259.1615 , Max excitation: 1

| $l'$ -matrix coefficients/(u <sup>1/2</sup> Å <sup>-1</sup> ) |                    |                    |                    |
|---------------------------------------------------------------|--------------------|--------------------|--------------------|
| O                                                             | 0.105 816 660 265  | -0.033 719 502 954 | -0.024 618 853 155 |
| C                                                             | -0.128 782 705 387 | 0.077 933 348 935  | -0.026 724 995 522 |
| C                                                             | 0.067 554 853 973  | -0.241 261 467 088 | 0.241 375 849 196  |
| C                                                             | 0.068 736 419 361  | 0.061 837 081 286  | -0.365 105 676 057 |
| C                                                             | -0.113 708 520 903 | 0.072 545 656 745  | 0.247 191 158 335  |
| C                                                             | -0.065 832 904 561 | 0.050 546 918 698  | 0.034 820 296 724  |
| C                                                             | 0.002 258 319 534  | 0.171 123 124 608  | -0.131 703 277 226 |
| H                                                             | 0.117 308 910 216  | 0.028 829 178 994  | -0.028 160 946 443 |
| H                                                             | 0.055 297 012 332  | 0.025 885 277 077  | -0.028 827 092 789 |
| H                                                             | -0.059 394 421 199 | 0.057 445 158 312  | 0.031 736 562 746  |
| H                                                             | 0.199 680 277 438  | -0.100 459 345 264 | -0.079 455 969 515 |
| H                                                             | -0.258 616 631 647 | -0.070 010 561 877 | 0.202 889 133 906  |
| H                                                             | 0.379 764 682 601  | -0.243 397 037 657 | -0.113 572 873 560 |
| H                                                             | -0.207 873 246 246 | -0.005 997 440 789 | 0.085 741 304 776  |
| H                                                             | 0.087 936 932 304  | 0.038 390 458 391  | 0.183 710 692 334  |
| H                                                             | -0.050 179 896 406 | -0.140 605 669 295 | -0.099 419 297 393 |
| H                                                             | -0.099 447 045 688 | -0.121 020 843 988 | -0.056 051 820 523 |

Wavenumber/cm<sup>-1</sup>: 1282.2026 , Max excitation: 1

| $l'$ -matrix coefficients/(u <sup>1/2</sup> Å <sup>-1</sup> ) |                    |                    |
|---------------------------------------------------------------|--------------------|--------------------|
| O -0.054 037 152 358                                          | 0.019 192 528 755  | 0.007 704 047 835  |
| C 0.091 500 287 813                                           | 0.078 983 832 726  | 0.089 396 747 218  |
| C -0.023 302 939 084                                          | -0.186 212 848 119 | -0.070 786 140 066 |
| C -0.012 145 198 660                                          | -0.008 626 746 821 | -0.123 167 057 522 |
| C -0.004 303 798 282                                          | 0.100 145 711 756  | -0.047 308 859 625 |
| C 0.036 966 021 316                                           | -0.083 773 238 082 | 0.091 470 467 757  |
| C -0.065 767 958 171                                          | 0.197 726 399 838  | 0.037 480 746 686  |
| H -0.441 592 664 834                                          | 0.010 486 673 918  | 0.056 553 129 590  |
| H 0.177 104 401 593                                           | -0.069 719 732 957 | -0.016 305 986 586 |
| H 0.150 933 139 516                                           | -0.498 300 151 138 | 0.023 163 823 096  |
| H -0.004 905 820 507                                          | -0.105 150 274 453 | 0.004 898 553 104  |
| H 0.290 298 913 760                                           | 0.274 469 212 315  | -0.129 027 828 204 |
| H 0.011 638 114 884                                           | 0.006 075 719 145  | 0.004 324 001 023  |
| H -0.168 788 203 484                                          | 0.134 451 732 473  | 0.016 628 721 699  |
| H 0.143 676 639 498                                           | 0.024 913 989 389  | 0.172 246 487 773  |
| H 0.064 879 203 202                                           | -0.084 132 693 438 | 0.054 346 694 777  |
| H -0.087 165 994 168                                          | -0.108 692 472 340 | -0.138 422 098 922 |

Wavenumber/cm<sup>-1</sup>: 1317.748 , Max excitation: 1

| $l'$ -matrix coefficients/(u <sup>1/2</sup> Å <sup>-1</sup> ) |                    |                    |
|---------------------------------------------------------------|--------------------|--------------------|
| O -0.024 065 074 724                                          | 0.001 444 616 758  | 0.007 810 559 104  |
| C -0.247 147 779 873                                          | -0.161 900 022 023 | 0.232 852 700 048  |
| C 0.238 814 988 309                                           | -0.073 333 662 086 | -0.036 975 633 655 |
| C -0.120 703 859 255                                          | 0.093 265 340 993  | -0.015 306 064 950 |
| C 0.138 666 720 303                                           | -0.308 212 299 206 | 0.142 349 968 575  |
| C 0.095 506 052 580                                           | 0.463 603 314 026  | -0.336 878 102 762 |
| C -0.123 426 199 581                                          | 0.067 893 716 523  | -0.007 274 261 015 |
| H -0.031 955 040 160                                          | 0.015 286 309 992  | -0.062 107 962 658 |
| H -0.220 534 354 664                                          | -0.066 541 661 526 | 0.080 458 161 090  |
| H 0.209 883 881 786                                           | -0.136 682 846 856 | 0.080 621 908 883  |
| H 0.103 537 660 420                                           | 0.030 912 602 432  | -0.022 783 320 636 |
| H -0.049 830 806 453                                          | 0.060 923 124 318  | 0.064 954 977 330  |
| H -0.109 187 916 188                                          | 0.074 755 720 530  | -0.029 932 606 776 |
| H 0.138 739 008 326                                           | -0.162 860 477 243 | 0.006 994 130 047  |
| H 0.087 932 530 188                                           | -0.011 751 580 969 | 0.017 842 928 526  |
| H 0.082 931 594 728                                           | -0.024 005 738 538 | 0.076 956 228 359  |
| H -0.052 502 362 350                                          | -0.066 493 609 625 | -0.170 831 952 117 |

Wavenumber/cm<sup>-1</sup>: 1331.5974 , Max excitation: 1

| $l'$ -matrix coefficients/(u <sup>1/2</sup> Å <sup>-1</sup> ) |                    |                    |
|---------------------------------------------------------------|--------------------|--------------------|
| O -0.014 986 538 408                                          | 0.006 837 871 075  | 0.003 916 336 929  |
| C -0.020 361 480 418                                          | -0.111 639 939 896 | 0.053 546 668 709  |
| C 0.126 141 271 297                                           | 0.171 949 124 423  | -0.138 672 556 672 |
| C -0.140 012 966 232                                          | -0.084 847 348 778 | 0.028 810 436 314  |
| C 0.072 979 328 633                                           | -0.146 025 644 403 | -0.092 882 405 266 |
| C 0.079 392 537 926                                           | 0.234 591 021 236  | 0.046 926 176 758  |
| C -0.096 282 598 160                                          | -0.105 948 713 660 | 0.067 910 439 790  |
| H -0.231 234 792 605                                          | -0.055 183 742 734 | 0.084 845 369 163  |
| H 0.172 258 325 222                                           | 0.041 901 328 217  | -0.027 826 969 209 |
| H 0.103 938 768 482                                           | 0.259 159 647 719  | 0.052 682 521 649  |
| H -0.224 764 978 642                                          | -0.211 546 043 262 | 0.107 989 933 184  |
| H -0.052 982 903 447                                          | -0.033 159 344 091 | 0.019 333 700 977  |
| H 0.358 347 774 717                                           | -0.318 961 187 659 | -0.007 598 572 983 |
| H -0.252 725 703 906                                          | 0.301 501 427 542  | 0.025 079 951 723  |
| H -0.035 470 652 321                                          | -0.041 497 241 673 | -0.204 346 525 965 |
| H 0.099 579 906 072                                           | 0.115 611 233 460  | 0.123 921 131 448  |
| H 0.047 314 989 105                                           | 0.059 643 554 441  | -0.071 069 164 476 |

Wavenumber/cm<sup>-1</sup>: 1368.8591 , Max excitation: 1

| $l'$ -matrix coefficients/(u <sup>1/2</sup> Å <sup>-1</sup> ) |                    |                    |
|---------------------------------------------------------------|--------------------|--------------------|
| O -0.048 194 253 176                                          | 0.015 625 085 428  | 0.011 829 314 765  |
| C -0.053 864 399 982                                          | -0.167 176 188 508 | -0.128 339 670 221 |
| C -0.020 347 668 120                                          | 0.108 653 416 639  | 0.203 207 303 888  |
| C -0.119 943 063 492                                          | -0.043 601 513 194 | -0.057 025 089 948 |
| C 0.149 687 894 202                                           | -0.041 102 287 770 | 0.115 827 953 759  |
| C 0.048 765 508 302                                           | 0.170 469 757 528  | -0.012 910 350 919 |
| C 0.095 316 606 028                                           | -0.056 345 369 458 | -0.154 056 561 699 |
| H -0.373 553 241 936                                          | -0.145 428 004 286 | 0.231 313 377 168  |
| H 0.499 830 259 942                                           | 0.210 729 349 024  | -0.130 608 853 094 |
| H -0.118 754 238 629                                          | 0.037 757 419 883  | -0.025 860 303 297 |
| H 0.090 562 244 213                                           | -0.041 129 348 086 | -0.018 513 657 267 |
| H -0.057 837 353 948                                          | 0.045 993 674 136  | 0.087 429 561 732  |
| H -0.119 318 961 068                                          | 0.160 791 284 808  | -0.067 805 792 830 |
| H 0.150 604 579 801                                           | -0.230 173 439 030 | -0.009 642 888 169 |
| H -0.088 365 188 390                                          | 0.018 596 079 976  | 0.028 196 351 452  |
| H -0.149 920 410 011                                          | -0.046 637 771 067 | -0.173 646 903 936 |
| H 0.014 893 329 712                                           | 0.027 709 376 014  | 0.146 948 790 156  |

Wavenumber/cm<sup>-1</sup>: 1386.3265 , Max excitation: 5

| $l'$ -matrix coefficients/(u <sup>1/2</sup> Å <sup>-1</sup> ) |                    |                    |                    |
|---------------------------------------------------------------|--------------------|--------------------|--------------------|
| O                                                             | -0.050 951 454 766 | 0.016 793 686 282  | 0.005 598 336 299  |
| C                                                             | 0.062 785 361 080  | 0.185 359 806 980  | -0.079 896 305 788 |
| C                                                             | 0.364 438 998 034  | 0.166 570 399 475  | 0.103 090 433 890  |
| C                                                             | -0.033 453 679 396 | -0.119 929 914 762 | -0.019 481 577 300 |
| C                                                             | -0.033 248 790 480 | 0.204 970 799 809  | 0.057 138 483 243  |
| C                                                             | -0.054 766 606 368 | -0.341 733 130 339 | 0.110 270 697 713  |
| C                                                             | -0.258 408 600 836 | -0.062 765 981 976 | -0.152 702 523 542 |
| H                                                             | -0.196 751 626 079 | 0.033 723 102 697  | 0.028 263 544 239  |
| H                                                             | -0.033 815 599 044 | 0.004 103 815 016  | -0.002 472 200 525 |
| H                                                             | 0.323 512 962 756  | 0.102 782 029 857  | 0.205 035 370 697  |
| H                                                             | 0.037 083 883 421  | -0.042 729 178 829 | -0.007 106 603 676 |
| H                                                             | -0.186 002 494 097 | -0.149 329 708 196 | 0.114 850 876 366  |
| H                                                             | -0.092 737 707 923 | 0.147 139 746 501  | -0.061 655 239 160 |
| H                                                             | 0.085 008 088 135  | -0.191 650 168 065 | -0.008 446 297 449 |
| H                                                             | 0.037 140 424 648  | -0.054 719 767 926 | -0.171 994 967 842 |
| H                                                             | 0.118 968 750 297  | 0.031 271 422 712  | 0.096 467 786 244  |
| H                                                             | -0.052 851 895 498 | -0.059 591 362 369 | -0.278 829 259 061 |

Wavenumber/cm<sup>-1</sup>: 1413.6747 , Max excitation: 1

| $l'$ -matrix coefficients/(u <sup>1/2</sup> Å <sup>-1</sup> ) |                    |                    |                    |
|---------------------------------------------------------------|--------------------|--------------------|--------------------|
| O                                                             | -0.032 121 348 173 | 0.013 855 458 202  | 0.003 769 522 516  |
| C                                                             | 0.212 494 224 749  | -0.076 096 696 609 | 0.089 800 292 460  |
| C                                                             | -0.204 888 305 524 | 0.114 787 466 420  | -0.146 568 664 451 |
| C                                                             | -0.358 805 498 883 | -0.181 835 809 869 | 0.054 272 483 946  |
| C                                                             | 0.413 450 495 775  | 0.154 647 547 760  | -0.044 406 124 399 |
| C                                                             | -0.065 455 156 073 | -0.084 168 119 106 | -0.065 928 088 264 |
| C                                                             | 0.015 972 575 895  | 0.214 368 115 263  | 0.117 578 590 749  |
| H                                                             | 0.153 007 703 704  | 0.010 550 702 797  | -0.066 008 205 747 |
| H                                                             | 0.011 268 741 918  | -0.107 098 888 654 | 0.034 068 774 183  |
| H                                                             | -0.103 593 076 641 | 0.033 371 636 510  | -0.074 029 442 850 |
| H                                                             | -0.159 328 336 624 | -0.203 394 600 287 | 0.085 806 357 332  |
| H                                                             | -0.147 086 488 706 | -0.031 629 913 095 | 0.097 897 599 439  |
| H                                                             | 0.164 277 772 317  | 0.102 372 101 248  | -0.253 545 614 079 |
| H                                                             | 0.044 108 662 441  | -0.234 448 503 278 | -0.035 511 755 417 |
| H                                                             | 0.145 843 528 918  | 0.039 987 859 198  | 0.222 738 656 825  |
| H                                                             | 0.042 708 534 353  | -0.057 444 902 327 | 0.046 309 821 230  |
| H                                                             | -0.067 309 085 228 | -0.096 621 203 777 | -0.089 135 970 993 |

Wavenumber/cm<sup>-1</sup>: 1477.2015 , Max excitation: 1

| $l'$ -matrix coefficients/(u <sup>1/2</sup> Å <sup>-1</sup> ) |                    |                    |                    |
|---------------------------------------------------------------|--------------------|--------------------|--------------------|
| O                                                             | -0.020 150 665 110 | 0.007 694 195 481  | 0.006 590 800 200  |
| C                                                             | -0.008 428 671 941 | -0.064 971 240 060 | -0.043 265 252 992 |
| C                                                             | 0.047 563 931 967  | 0.152 290 627 762  | 0.131 854 795 358  |
| C                                                             | 0.021 988 317 679  | -0.162 422 761 833 | 0.304 613 364 987  |
| C                                                             | 0.021 145 083 119  | -0.084 709 416 231 | -0.286 163 273 818 |
| C                                                             | 0.054 558 351 271  | 0.087 980 645 276  | 0.085 839 552 404  |
| C                                                             | -0.090 680 974 270 | 0.166 104 484 923  | -0.216 079 333 370 |
| H                                                             | 0.008 669 237 589  | -0.057 649 929 117 | 0.085 181 604 897  |
| H                                                             | 0.009 759 927 644  | 0.092 962 115 956  | -0.006 995 554 650 |
| H                                                             | -0.026 149 957 973 | -0.101 140 951 980 | -0.018 023 642 834 |
| H                                                             | -0.028 256 988 053 | 0.287 001 126 651  | -0.046 868 765 831 |
| H                                                             | -0.112 811 032 934 | -0.336 907 438 661 | -0.082 739 085 579 |
| H                                                             | 0.018 350 972 618  | -0.136 223 553 479 | 0.189 653 284 807  |
| H                                                             | 0.120 791 784 842  | 0.248 461 962 582  | -0.065 034 487 041 |
| H                                                             | 0.151 623 134 824  | 0.026 986 063 307  | 0.295 117 874 577  |
| H                                                             | -0.068 226 473 511 | -0.185 505 947 548 | -0.122 054 978 491 |
| H                                                             | -0.152 764 025 014 | -0.194 064 135 096 | -0.174 408 039 054 |

Wavenumber/cm<sup>-1</sup>: 1481.1441 , Max excitation: 1

| $l'$ -matrix coefficients/(u <sup>1/2</sup> Å <sup>-1</sup> ) |                    |                    |                    |
|---------------------------------------------------------------|--------------------|--------------------|--------------------|
| O                                                             | -0.035 354 294 922 | -0.008 071 311 648 | 0.011 986 133 531  |
| C                                                             | 0.168 037 023 025  | -0.417 801 236 343 | -0.201 987 193 440 |
| C                                                             | -0.147 927 701 440 | 0.111 215 310 564  | -0.101 195 723 666 |
| C                                                             | 0.140 672 369 397  | 0.051 215 391 982  | -0.159 946 457 761 |
| C                                                             | -0.206 910 421 960 | 0.026 814 624 146  | 0.128 551 703 847  |
| C                                                             | 0.018 696 468 329  | 0.044 982 624 995  | 0.065 829 564 697  |
| C                                                             | -0.083 189 463 389 | 0.132 319 123 620  | 0.141 687 587 019  |
| H                                                             | 0.248 800 438 510  | -0.257 576 738 383 | 0.293 051 526 823  |
| H                                                             | -0.028 847 422 190 | 0.314 148 010 313  | 0.003 033 383 527  |
| H                                                             | 0.062 938 532 667  | 0.128 233 951 355  | 0.068 552 694 728  |
| H                                                             | 0.059 771 700 852  | -0.042 703 666 936 | -0.025 280 245 580 |
| H                                                             | 0.086 772 187 250  | 0.099 000 391 351  | -0.015 405 408 270 |
| H                                                             | -0.134 667 637 356 | 0.065 283 046 147  | 0.034 042 889 787  |
| H                                                             | -0.048 502 455 866 | -0.008 277 546 815 | 0.032 831 593 229  |
| H                                                             | 0.156 049 359 965  | -0.004 403 320 169 | 0.051 856 854 591  |
| H                                                             | 0.177 382 462 403  | 0.020 438 597 272  | 0.182 899 534 188  |
| H                                                             | -0.056 978 648 341 | -0.105 057 544 291 | -0.234 725 942 434 |

Wavenumber/cm<sup>-1</sup>: 1491.4737 , Max excitation: 1

| $l'$ -matrix coefficients/(u <sup>1/2</sup> Å <sup>-1</sup> ) |                    |                    |                    |
|---------------------------------------------------------------|--------------------|--------------------|--------------------|
| O                                                             | -0.035 400 623 503 | 0.002 735 775 368  | 0.011 228 819 873  |
| C                                                             | 0.060 218 897 994  | 0.050 661 395 076  | 0.226 880 498 217  |
| C                                                             | -0.061 930 177 160 | 0.239 010 090 737  | 0.007 932 995 014  |
| C                                                             | 0.335 912 177 182  | -0.419 315 288 497 | -0.090 181 085 973 |
| C                                                             | -0.160 472 944 681 | -0.042 865 671 218 | 0.236 730 048 256  |
| C                                                             | 0.022 613 971 816  | 0.131 216 312 678  | -0.180 251 615 760 |
| C                                                             | -0.046 239 328 627 | 0.056 577 894 758  | -0.092 675 106 562 |
| H                                                             | -0.059 678 066 320 | 0.109 438 228 912  | -0.170 014 977 084 |
| H                                                             | 0.129 660 775 901  | -0.222 766 446 925 | 0.011 308 210 915  |
| H                                                             | -0.112 915 756 260 | 0.256 509 560 717  | -0.038 333 916 953 |
| H                                                             | -0.076 783 091 683 | -0.054 225 315 189 | -0.032 553 161 942 |
| H                                                             | 0.194 419 714 767  | -0.142 131 398 429 | -0.190 666 366 334 |
| H                                                             | -0.170 623 511 699 | 0.131 579 636 940  | -0.048 973 259 153 |
| H                                                             | -0.242 460 192 311 | -0.047 174 039 568 | 0.081 023 789 648  |
| H                                                             | 0.045 812 732 897  | 0.008 683 016 882  | 0.078 053 452 394  |
| H                                                             | -0.030 003 123 924 | -0.042 329 949 032 | -0.048 994 856 122 |
| H                                                             | -0.054 541 992 175 | -0.061 245 463 439 | -0.059 903 604 424 |

Wavenumber/cm<sup>-1</sup>: 1499.6993 , Max excitation: 0

| $l'$ -matrix coefficients/(u <sup>1/2</sup> Å <sup>-1</sup> ) |                    |                    |                    |
|---------------------------------------------------------------|--------------------|--------------------|--------------------|
| O                                                             | 0.022 124 696 006  | 0.009 906 022 630  | -0.004 869 276 304 |
| C                                                             | -0.419 515 707 711 | -0.062 473 539 010 | -0.125 439 260 482 |
| C                                                             | 0.072 378 755 824  | -0.218 366 471 291 | -0.011 036 041 771 |
| C                                                             | 0.192 151 735 753  | -0.116 043 336 622 | 0.134 418 214 094  |
| C                                                             | 0.183 345 441 327  | 0.325 689 251 450  | 0.019 120 048 879  |
| C                                                             | 0.033 172 415 734  | 0.047 174 184 233  | -0.044 552 997 742 |
| C                                                             | 0.070 208 414 496  | -0.008 926 198 391 | 0.104 353 077 688  |
| H                                                             | -0.085 080 615 599 | -0.089 567 574 391 | 0.163 174 577 969  |
| H                                                             | -0.193 003 238 132 | 0.217 556 501 053  | -0.002 100 084 683 |
| H                                                             | 0.020 010 342 458  | -0.060 512 662 328 | -0.000 264 892 929 |
| H                                                             | -0.229 005 714 519 | 0.137 928 524 668  | 0.002 131 370 227  |
| H                                                             | 0.056 371 708 417  | -0.239 500 838 254 | -0.210 586 093 558 |
| H                                                             | 0.098 493 042 868  | 0.165 549 809 779  | -0.295 860 653 063 |
| H                                                             | -0.266 963 662 370 | -0.102 104 386 016 | 0.014 515 121 755  |
| H                                                             | -0.002 022 356 915 | 0.000 457 496 591  | -0.007 998 916 109 |
| H                                                             | 0.021 235 020 761  | 0.014 086 720 519  | 0.031 477 552 725  |
| H                                                             | 0.037 051 195 126  | 0.030 369 391 696  | 0.059 581 789 479  |



Wavenumber/cm<sup>-1</sup>: 1503.9734 , Max excitation: 1

| $l'$ -matrix coefficients/(u <sup>1/2</sup> Å <sup>-1</sup> ) |                    |                    |                    |
|---------------------------------------------------------------|--------------------|--------------------|--------------------|
| O                                                             | 0.097 605 820 802  | -0.036 915 914 871 | -0.015 807 539 232 |
| C                                                             | 0.135 540 803 937  | -0.339 407 670 662 | 0.309 934 089 146  |
| C                                                             | -0.203 209 753 847 | -0.111 948 920 467 | 0.254 737 733 099  |
| C                                                             | 0.074 919 954 163  | 0.311 618 226 816  | 0.069 710 044 168  |
| C                                                             | 0.087 959 264 904  | 0.310 770 939 214  | -0.117 731 449 002 |
| C                                                             | 0.032 316 866 710  | 0.018 364 506 594  | -0.073 791 969 310 |
| C                                                             | -0.249 236 361 822 | -0.159 887 057 051 | -0.279 814 500 791 |
| H                                                             | 0.039 496 034 419  | -0.049 492 299 253 | -0.037 009 639 046 |
| H                                                             | 0.141 296 470 110  | -0.207 512 420 540 | 0.050 878 604 484  |
| H                                                             | -0.089 471 402 375 | 0.023 300 196 111  | 0.059 701 841 881  |
| H                                                             | -0.011 328 979 754 | 0.181 158 487 698  | -0.013 068 358 782 |
| H                                                             | 0.018 473 215 296  | 0.038 078 210 263  | -0.042 599 934 821 |
| H                                                             | 0.085 197 659 817  | 0.070 478 910 467  | -0.110 633 018 503 |
| H                                                             | -0.062 880 925 742 | 0.044 750 121 236  | -0.026 053 716 673 |
| H                                                             | -0.074 036 584 358 | -0.057 231 621 290 | -0.222 833 576 933 |
| H                                                             | 0.033 382 427 735  | 0.033 545 032 473  | 0.005 889 680 542  |
| H                                                             | -0.048 859 280 904 | -0.031 866 726 993 | -0.164 118 113 995 |

Wavenumber/cm<sup>-1</sup>: 2889.9399 , Max excitation: 2

| $l'$ -matrix coefficients/(u <sup>1/2</sup> Å <sup>-1</sup> ) |                    |                    |                    |
|---------------------------------------------------------------|--------------------|--------------------|--------------------|
| O                                                             | 0.199 620 805 190  | -0.063 038 673 294 | -0.046 616 664 375 |
| C                                                             | -0.226 222 285 815 | -0.339 465 425 584 | 0.267 466 791 567  |
| C                                                             | 0.207 833 404 615  | 0.095 884 991 559  | -0.169 820 853 932 |
| C                                                             | -0.081 657 367 395 | -0.051 000 567 469 | -0.130 269 308 478 |
| C                                                             | -0.218 409 954 923 | 0.370 333 198 048  | -0.164 259 187 317 |
| C                                                             | 0.110 501 920 623  | -0.105 791 142 212 | 0.010 692 899 061  |
| C                                                             | 0.133 918 889 371  | 0.077 704 375 334  | 0.100 037 037 977  |
| H                                                             | -0.175 512 769 464 | -0.070 687 862 098 | 0.018 026 734 762  |
| H                                                             | -0.121 085 557 403 | -0.144 120 598 324 | 0.075 127 430 730  |
| H                                                             | -0.032 245 374 589 | 0.118 503 703 392  | -0.101 166 821 644 |
| H                                                             | 0.097 044 890 373  | -0.144 928 013 513 | 0.001 703 048 231  |
| H                                                             | -0.150 972 980 973 | 0.004 205 441 083  | 0.168 987 354 561  |
| H                                                             | -0.153 888 152 219 | 0.102 713 350 886  | 0.140 370 167 043  |
| H                                                             | 0.057 905 386 504  | 0.194 953 528 977  | -0.036 806 058 928 |
| H                                                             | 0.013 047 721 128  | 0.036 494 789 203  | 0.137 068 041 218  |
| H                                                             | -0.090 089 706 632 | -0.034 168 770 520 | -0.071 271 271 314 |
| H                                                             | 0.016 060 123 779  | 0.023 645 351 461  | 0.151 083 169 738  |

Wavenumber/cm<sup>-1</sup>: 2904.2003 , Max excitation: 1

| $l'$ -matrix coefficients/(u <sup>1/2</sup> Å <sup>-1</sup> ) |                    |                    |                    |
|---------------------------------------------------------------|--------------------|--------------------|--------------------|
| O                                                             | 0.113 983 776 388  | -0.019 317 142 065 | -0.025 049 437 080 |
| C                                                             | -0.218 634 669 984 | 0.173 489 539 034  | -0.061 645 077 505 |
| C                                                             | -0.390 552 912 960 | -0.137 649 959 989 | 0.280 306 911 144  |
| C                                                             | 0.073 691 000 906  | -0.368 927 987 385 | -0.130 416 494 066 |
| C                                                             | 0.165 963 083 026  | 0.107 963 770 377  | -0.209 900 759 506 |
| C                                                             | 0.114 228 671 506  | 0.157 667 241 873  | -0.002 610 902 455 |
| C                                                             | -0.008 597 519 214 | 0.014 403 751 381  | 0.102 906 615 442  |
| H                                                             | -0.028 874 127 744 | 0.056 320 550 694  | -0.032 376 677 405 |
| H                                                             | -0.034 221 593 160 | 0.029 461 705 108  | -0.029 545 696 808 |
| H                                                             | -0.071 632 740 763 | 0.032 847 129 224  | 0.124 475 870 740  |
| H                                                             | 0.190 012 451 313  | -0.180 824 854 853 | -0.027 835 360 507 |
| H                                                             | -0.004 167 867 798 | 0.000 476 154 812  | 0.127 366 053 969  |
| H                                                             | -0.075 913 847 524 | 0.047 261 492 535  | 0.166 415 561 066  |
| H                                                             | 0.221 572 426 243  | 0.158 243 629 015  | -0.063 381 096 829 |
| H                                                             | 0.032 804 477 142  | -0.017 321 910 394 | -0.155 745 777 407 |
| H                                                             | 0.197 242 471 530  | 0.125 960 655 508  | 0.191 629 276 046  |
| H                                                             | 0.030 043 959 605  | 0.007 676 700 486  | -0.127 469 874 105 |

Wavenumber/cm<sup>-1</sup>: 2979.5959 , Max excitation: 1

| $l'$ -matrix coefficients/(u <sup>1/2</sup> Å <sup>-1</sup> ) |                    |                    |                    |
|---------------------------------------------------------------|--------------------|--------------------|--------------------|
| O                                                             | -0.577 682 711 385 | 0.173 534 135 057  | 0.117 032 554 645  |
| C                                                             | 0.120 842 646 028  | -0.152 317 573 999 | 0.103 864 683 612  |
| C                                                             | 0.233 494 181 824  | -0.183 387 037 900 | -0.068 128 376 372 |
| C                                                             | 0.301 228 467 471  | -0.145 319 864 281 | -0.124 572 354 989 |
| C                                                             | 0.202 261 012 531  | 0.130 829 723 754  | -0.157 334 402 516 |
| C                                                             | -0.343 313 434 001 | 0.141 543 366 805  | 0.091 903 663 937  |
| C                                                             | 0.003 689 671 109  | 0.011 508 963 628  | -0.000 156 489 170 |
| H                                                             | 0.116 893 166 168  | -0.036 836 365 156 | 0.004 852 984 028  |
| H                                                             | 0.034 984 398 510  | -0.040 591 160 856 | 0.032 593 361 449  |
| H                                                             | 0.055 834 216 607  | 0.006 637 893 409  | -0.017 739 596 482 |
| H                                                             | 0.149 835 053 254  | -0.088 747 686 461 | -0.024 464 085 254 |
| H                                                             | 0.036 976 234 739  | -0.030 543 309 750 | 0.051 498 183 823  |
| H                                                             | 0.072 355 195 722  | -0.004 773 429 607 | 0.047 431 782 857  |
| H                                                             | 0.149 281 964 581  | 0.076 813 449 316  | -0.051 714 100 492 |
| H                                                             | -0.060 624 859 577 | 0.016 064 014 440  | -0.036 901 478 652 |
| H                                                             | -0.062 867 996 236 | 0.022 967 247 017  | -0.043 690 970 143 |
| H                                                             | 0.020 041 001 316  | 0.068 167 524 185  | 0.104 933 194 587  |

Wavenumber/cm<sup>-1</sup>: 2989.086 , Max excitation: 1

| $l'$ -matrix coefficients/(u <sup>1/2</sup> Å <sup>-1</sup> ) |                    |                    |                    |
|---------------------------------------------------------------|--------------------|--------------------|--------------------|
| O                                                             | 0.082 916 845 384  | 0.023 468 205 891  | -0.059 061 007 940 |
| C                                                             | -0.076 058 381 836 | 0.198 935 442 766  | 0.089 918 734 642  |
| C                                                             | -0.101 239 064 375 | 0.035 353 486 218  | -0.326 561 717 653 |
| C                                                             | 0.241 691 878 658  | -0.012 277 952 616 | 0.244 816 821 022  |
| C                                                             | 0.096 607 590 594  | 0.045 580 103 046  | 0.007 250 734 905  |
| C                                                             | 0.102 874 094 355  | 0.054 847 946 029  | 0.077 099 801 415  |
| C                                                             | -0.308 451 893 275 | -0.291 589 147 518 | -0.154 906 031 984 |
| H                                                             | 0.045 853 713 329  | 0.011 238 982 360  | 0.149 165 287 991  |
| H                                                             | -0.112 461 624 555 | 0.199 140 403 078  | 0.060 561 126 894  |
| H                                                             | -0.042 792 887 758 | 0.021 392 463 075  | -0.100 331 548 598 |
| H                                                             | 0.201 467 850 552  | -0.239 808 852 622 | 0.153 273 615 928  |
| H                                                             | 0.090 348 787 453  | 0.188 140 568 371  | 0.269 015 746 428  |
| H                                                             | 0.035 917 888 046  | 0.025 260 422 585  | -0.047 815 989 338 |
| H                                                             | -0.034 729 318 326 | -0.023 625 492 229 | 0.004 550 883 172  |
| H                                                             | -0.036 726 410 273 | -0.088 584 930 619 | 0.085 729 425 220  |
| H                                                             | -0.184 242 828 149 | -0.142 853 212 310 | -0.121 109 016 213 |
| H                                                             | -0.139 107 746 271 | -0.150 292 776 073 | -0.002 395 409 682 |

Wavenumber/cm<sup>-1</sup>: 3025.5057 , Max excitation: 1

| $l'$ -matrix coefficients/(u <sup>1/2</sup> Å <sup>-1</sup> ) |                    |                    |                    |
|---------------------------------------------------------------|--------------------|--------------------|--------------------|
| O                                                             | 0.092 173 923 186  | -0.286 013 538 049 | 0.049 307 865 570  |
| C                                                             | 0.288 804 335 104  | 0.160 217 161 934  | 0.176 459 205 514  |
| C                                                             | 0.086 371 895 690  | -0.252 486 259 985 | -0.078 858 723 311 |
| C                                                             | -0.178 048 042 084 | -0.208 083 821 855 | -0.069 279 964 910 |
| C                                                             | -0.109 970 330 084 | 0.072 668 178 378  | -0.003 287 484 142 |
| C                                                             | 0.174 319 948 664  | 0.164 087 674 294  | -0.018 996 925 261 |
| C                                                             | -0.259 393 522 433 | 0.255 258 146 637  | -0.094 886 954 476 |
| H                                                             | 0.199 828 829 063  | -0.008 091 543 729 | 0.190 297 061 997  |
| H                                                             | 0.050 952 755 297  | 0.221 760 649 170  | 0.075 360 294 828  |
| H                                                             | 0.042 390 526 009  | -0.113 098 229 791 | -0.014 995 047 270 |
| H                                                             | -0.097 602 953 597 | -0.032 560 799 106 | -0.025 754 661 561 |
| H                                                             | -0.078 625 344 207 | -0.115 610 873 730 | -0.044 768 996 620 |
| H                                                             | -0.101 465 527 775 | 0.071 845 511 733  | 0.016 018 143 906  |
| H                                                             | -0.026 092 055 451 | 0.026 755 386 987  | -0.001 405 420 123 |
| H                                                             | -0.275 051 811 771 | 0.119 192 070 278  | -0.106 413 719 588 |
| H                                                             | -0.109 759 601 632 | 0.043 033 894 179  | -0.056 565 424 140 |
| H                                                             | 0.021 001 991 545  | 0.264 664 186 273  | 0.078 492 791 653  |

Wavenumber/cm<sup>-1</sup>: 3027.1456 , Max excitation: 1

| $l'$ -matrix coefficients/(u <sup>1/2</sup> Å <sup>-1</sup> ) |                    |                    |                    |
|---------------------------------------------------------------|--------------------|--------------------|--------------------|
| O                                                             | 0.174 456 609 395  | 0.539 320 832 351  | -0.301 927 088 047 |
| C                                                             | -0.103 363 585 439 | -0.103 825 749 695 | 0.283 438 105 803  |
| C                                                             | -0.072 812 389 221 | -0.047 916 452 240 | -0.000 140 557 365 |
| C                                                             | 0.031 794 255 548  | -0.097 754 196 897 | -0.148 665 078 361 |
| C                                                             | 0.129 794 468 707  | -0.278 032 069 468 | 0.079 233 523 334  |
| C                                                             | 0.006 123 310 351  | -0.297 430 076 830 | 0.175 019 258 227  |
| C                                                             | -0.144 766 083 711 | 0.186 212 651 568  | -0.060 818 172 865 |
| H                                                             | -0.036 237 508 573 | -0.065 846 930 805 | 0.172 239 079 500  |
| H                                                             | -0.091 828 903 750 | 0.056 172 516 708  | 0.106 789 053 049  |
| H                                                             | -0.050 366 741 422 | 0.028 225 639 351  | -0.015 528 956 451 |
| H                                                             | -0.038 991 388 567 | 0.031 425 700 291  | -0.061 584 433 830 |
| H                                                             | 0.048 358 188 427  | -0.046 933 087 640 | -0.121 809 334 473 |
| H                                                             | 0.050 760 280 367  | -0.099 545 043 160 | 0.044 827 328 331  |
| H                                                             | 0.112 282 925 264  | -0.100 594 651 073 | 0.014 806 605 593  |
| H                                                             | -0.093 237 370 239 | 0.062 205 444 314  | -0.079 253 759 603 |
| H                                                             | -0.050 196 922 163 | 0.081 297 025 628  | -0.019 675 202 053 |
| H                                                             | -0.016 644 391 973 | 0.109 835 244 854  | 0.029 609 706 102  |

Wavenumber/cm<sup>-1</sup>: 3044.2981 , Max excitation: 1

| $l'$ -matrix coefficients/(u <sup>1/2</sup> Å <sup>-1</sup> ) |                    |                    |                    |
|---------------------------------------------------------------|--------------------|--------------------|--------------------|
| O                                                             | 0.007 551 037 985  | 0.118 871 419 604  | -0.009 436 056 130 |
| C                                                             | -0.025 181 001 376 | -0.046 641 853 291 | -0.049 414 849 072 |
| C                                                             | -0.015 759 782 489 | 0.009 813 783 904  | 0.009 629 090 889  |
| C                                                             | 0.038 911 099 605  | -0.005 099 850 390 | 0.084 966 684 139  |
| C                                                             | -0.035 033 850 392 | -0.001 964 527 413 | -0.016 714 645 769 |
| C                                                             | -0.030 629 261 063 | -0.009 661 390 317 | -0.023 327 564 169 |
| C                                                             | 0.043 707 546 048  | -0.047 345 407 512 | 0.001 554 007 916  |
| H                                                             | -0.018 791 147 109 | -0.002 796 164 398 | -0.040 713 367 072 |
| H                                                             | 0.003 530 900 520  | -0.041 789 968 364 | -0.019 798 736 345 |
| H                                                             | -0.010 659 487 953 | 0.011 942 263 237  | -0.000 278 697 937 |
| H                                                             | 0.043 800 661 482  | -0.034 385 716 071 | 0.033 629 995 629  |
| H                                                             | 0.004 944 877 049  | 0.024 211 811 552  | 0.065 215 487 484  |
| H                                                             | 0.000 616 479 430  | -0.004 164 782 339 | -0.020 134 731 506 |
| H                                                             | -0.034 943 491 353 | -0.006 936 057 731 | -0.002 424 013 238 |
| H                                                             | -0.465 335 408 166 | 0.122 525 988 813  | 0.236 119 894 106  |
| H                                                             | 0.235 868 377 604  | -0.534 784 214 785 | 0.092 765 577 201  |
| H                                                             | 0.293 680 943 790  | 0.340 885 953 945  | -0.329 890 567 229 |

Wavenumber/cm<sup>-1</sup>: 3078.338 , Max excitation: 1

| $l'$ -matrix coefficients/(u <sup>1/2</sup> Å <sup>-1</sup> ) |                    |                    |                    |
|---------------------------------------------------------------|--------------------|--------------------|--------------------|
| O                                                             | 0.094 783 704 503  | 0.111 285 447 927  | 0.278 789 987 632  |
| C                                                             | 0.013 286 490 211  | 0.076 300 626 595  | 0.075 231 075 934  |
| C                                                             | -0.006 937 681 172 | -0.002 698 581 266 | 0.014 507 458 340  |
| C                                                             | 0.011 286 940 748  | -0.009 691 744 587 | 0.032 955 352 929  |
| C                                                             | 0.065 459 556 440  | 0.064 548 466 117  | 0.108 635 072 234  |
| C                                                             | -0.235 765 114 182 | -0.304 855 879 906 | -0.729 653 979 666 |
| C                                                             | -0.007 237 437 916 | -0.027 206 251 936 | 0.023 094 830 161  |
| H                                                             | -0.018 895 646 484 | -0.039 417 149 567 | 0.188 805 380 647  |
| H                                                             | 0.073 824 881 108  | 0.203 329 608 105  | 0.030 025 924 591  |
| H                                                             | 0.000 983 101 657  | -0.001 031 959 856 | 0.006 064 847 086  |
| H                                                             | -0.009 783 519 499 | -0.013 764 344 971 | 0.016 785 232 038  |
| H                                                             | 0.006 240 877 326  | 0.003 608 666 793  | 0.013 694 530 151  |
| H                                                             | 0.066 040 410 153  | -0.075 751 584 640 | 0.190 860 671 755  |
| H                                                             | 0.062 553 318 860  | 0.212 012 912 068  | 0.054 336 178 238  |
| H                                                             | 0.004 737 873 316  | -0.008 783 148 197 | 0.011 007 739 798  |
| H                                                             | -0.003 434 670 561 | -0.004 979 153 674 | 0.007 278 450 567  |
| H                                                             | -0.007 895 586 710 | -0.015 758 865 908 | 0.010 905 392 537  |

Wavenumber/cm<sup>-1</sup>: 3089.475 , Max excitation: 0

| $l'$ -matrix coefficients/(u <sup>1/2</sup> Å <sup>-1</sup> ) |                    |                    |                    |
|---------------------------------------------------------------|--------------------|--------------------|--------------------|
| O                                                             | 0.006 645 939 689  | 0.084 457 972 468  | 0.144 144 856 762  |
| C                                                             | -0.006 769 920 911 | -0.003 132 158 095 | 0.136 090 773 598  |
| C                                                             | -0.000 420 663 104 | -0.023 058 951 139 | 0.079 793 219 682  |
| C                                                             | 0.081 724 101 873  | -0.054 921 520 154 | 0.284 151 761 750  |
| C                                                             | -0.287 395 669 992 | -0.211 695 887 673 | -0.370 283 356 143 |
| C                                                             | -0.080 110 333 289 | -0.069 101 791 681 | -0.082 405 536 061 |
| C                                                             | 0.252 406 288 433  | 0.256 183 605 768  | -0.165 295 975 256 |
| H                                                             | -0.008 418 082 388 | -0.021 501 096 627 | 0.091 938 551 472  |
| H                                                             | 0.016 993 748 404  | 0.061 617 572 280  | 0.040 334 571 201  |
| H                                                             | -0.039 948 700 534 | -0.045 372 360 867 | -0.014 015 606 326 |
| H                                                             | 0.193 405 114 531  | -0.097 319 201 873 | 0.092 582 911 112  |
| H                                                             | -0.020 599 199 271 | 0.053 945 460 431  | 0.226 769 181 790  |
| H                                                             | -0.048 001 321 467 | -0.020 433 505 323 | -0.295 251 487 390 |
| H                                                             | -0.254 267 145 037 | -0.188 683 368 494 | -0.103 542 797 392 |
| H                                                             | 0.105 001 525 375  | 0.058 687 925 151  | -0.154 137 133 788 |
| H                                                             | 0.107 082 756 279  | 0.168 444 711 984  | -0.009 224 748 390 |
| H                                                             | 0.062 307 121 070  | 0.059 093 198 717  | -0.042 579 891 371 |

Wavenumber/cm<sup>-1</sup>: 3091.1194 , Max excitation: 1

| $l'$ -matrix coefficients/(u <sup>1/2</sup> Å <sup>-1</sup> ) |                    |                    |                    |
|---------------------------------------------------------------|--------------------|--------------------|--------------------|
| O                                                             | -0.273 203 677 614 | -0.234 173 692 629 | -0.466 529 624 823 |
| C                                                             | -0.011 382 640 270 | 0.170 349 177 090  | 0.348 672 508 783  |
| C                                                             | -0.020 034 023 514 | 0.020 061 206 539  | 0.011 049 953 256  |
| C                                                             | -0.081 980 189 289 | 0.036 126 970 819  | 0.061 831 741 037  |
| C                                                             | 0.003 286 686 759  | 0.086 019 318 145  | 0.199 017 047 270  |
| C                                                             | -0.083 946 065 149 | -0.001 001 565 418 | 0.025 884 862 024  |
| C                                                             | 0.405 764 659 653  | -0.090 308 810 978 | -0.185 720 831 170 |
| H                                                             | 0.024 646 169 651  | 0.008 345 800 523  | 0.209 638 943 079  |
| H                                                             | -0.016 932 719 110 | 0.175 920 533 812  | 0.116 950 525 721  |
| H                                                             | -0.068 824 331 957 | -0.003 183 590 068 | -0.046 752 657 909 |
| H                                                             | -0.062 734 921 208 | 0.009 994 672 127  | 0.023 889 760 143  |
| H                                                             | -0.012 753 028 314 | 0.002 411 394 202  | -0.005 439 140 988 |
| H                                                             | -0.000 519 686 210 | 0.005 532 953 703  | 0.114 896 968 088  |
| H                                                             | 0.040 685 235 566  | 0.074 502 714 154  | 0.059 915 489 244  |
| H                                                             | 0.131 463 485 088  | -0.029 716 811 001 | -0.061 821 932 001 |
| H                                                             | 0.198 880 042 851  | -0.028 285 522 657 | 0.006 003 692 084  |
| H                                                             | 0.123 741 415 474  | -0.046 293 609 942 | -0.149 040 109 637 |

- 
- [1] E. B. Wilson, J. C. Decius, and P. C. Cross, *Molecular vibrations: the theory of infrared and Raman vibrational spectra* (McGraw-Hill Book Company, Inc, 1955).
- [2] H.-C. Jankowiak, J. L. Stuber, and R. Berger, Vibronic transitions in large molecular systems: Rigorous prescreening conditions for Franck-Condon factors, *J. Chem. Phys.* **127**, 234101 (2007).
- [3] J. Huh, *Unified description of vibronic transitions with coherent states*, Ph.D. thesis, Johann Wolfgang Goethe-Universität, Frankfurt am Main (2011).
